# Supplementary material for: Dimensional synthesis of spatial manipulators for velocity and force transmission for operation around a specified task point
Source: arXiv:2210.04446 source file (2022-10-10)
Supplement: Supplementary file 1 [file AppendixA.tex]

% Appendix Template

\section*{Appendix A} % Main appendix title

\label{AppendixA} % Change X to a consecutive letter; for referencing this appendix elsewhere, use \ref{AppendixX}
\begin{figure}[H]
\centering
\begin{subfigure}{\columnwidth}
  \begin{minipage}{\textwidth}\footnotesize
  \centering
\subsubfloat{\includegraphics[width=0.05\textwidth]{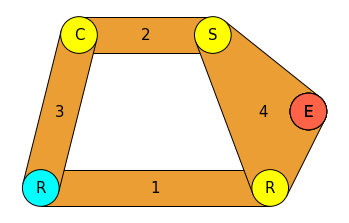}}{{\tiny 1D-M1}}
\qquad\subsubfloat{\includegraphics[width=0.05\textwidth]{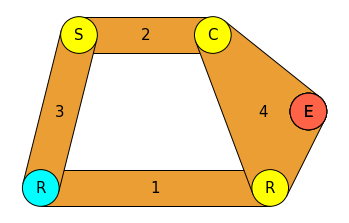}}{{\tiny 1D-M2}}
\qquad\subsubfloat{\includegraphics[width=0.05\textwidth]{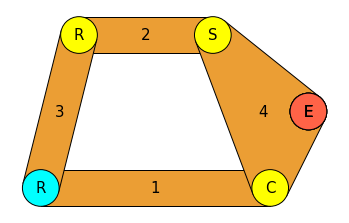}}{{\tiny 1D-M3}}
\qquad\subsubfloat{\includegraphics[width=0.05\textwidth]{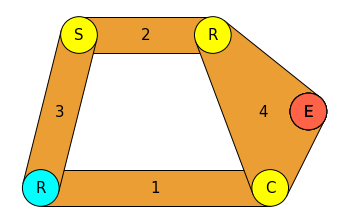}}{{\tiny 1D-M4}}
\qquad\subsubfloat{\includegraphics[width=0.05\textwidth]{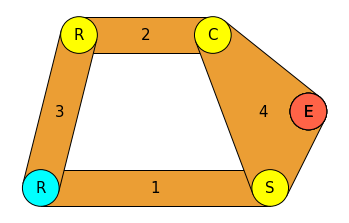}}{{\tiny 1D-M5}}
\qquad\subsubfloat{\includegraphics[width=0.05\textwidth]{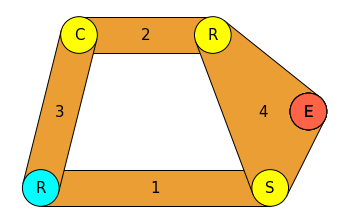}}{{\tiny 1D-M6}}
\qquad\subsubfloat{\includegraphics[width=0.05\textwidth]{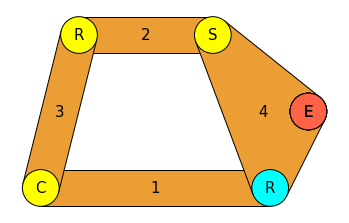}}{{\tiny 1D-M7}}
\qquad\subsubfloat{\includegraphics[width=0.05\textwidth]{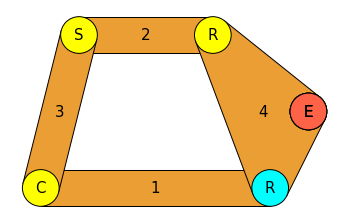}}{{\tiny 1D-M8}}
\qquad\subsubfloat{\includegraphics[width=0.05\textwidth]{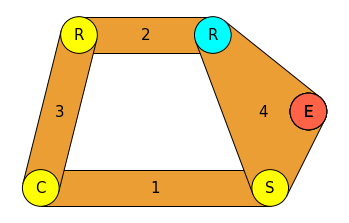}}{{\tiny 1D-M9}}
\qquad\subsubfloat{\includegraphics[width=0.05\textwidth]{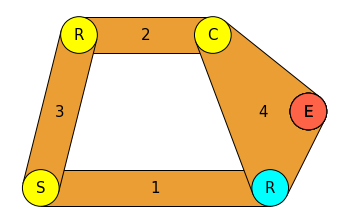}}{{\tiny 1D-M10}}
\qquad\subsubfloat{\includegraphics[width=0.05\textwidth]{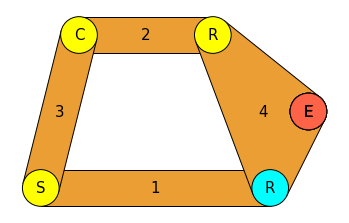}}{{\tiny 1D-M11}}
\qquad\subsubfloat{\includegraphics[width=0.05\textwidth]{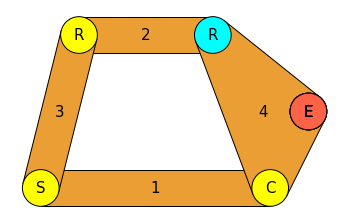}}{{\tiny 1D-M12}}
\qquad\subsubfloat{\includegraphics[width=0.04\textwidth]{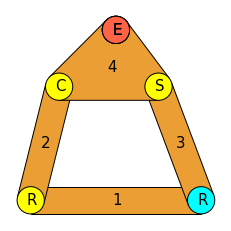}}{{\tiny 1D-M13}}
\qquad\subsubfloat{\includegraphics[width=0.04\textwidth]{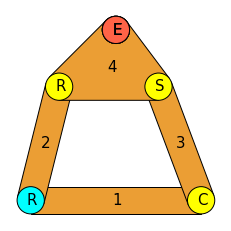}}{{\tiny 1D-M14}}
\qquad\subsubfloat{\includegraphics[width=0.04\textwidth]{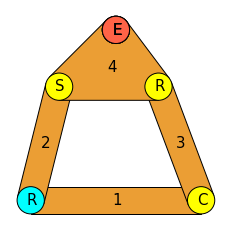}}{{\tiny 1D-M15}}
\qquad\subsubfloat{\includegraphics[width=0.04\textwidth]{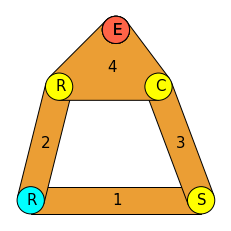}}{{\tiny 1D-M16}}
\qquad\subsubfloat{\includegraphics[width=0.04\textwidth]{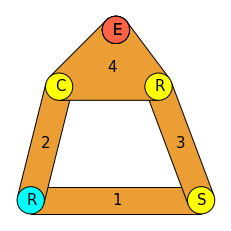}}{{\tiny 1D-M17}}
\qquad\subsubfloat{\includegraphics[width=0.04\textwidth]{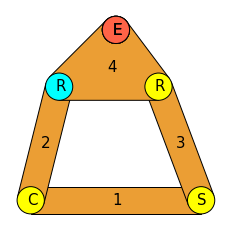}}{{\tiny 1D-M18}}
\qquad \subsubfloat{\includegraphics[width=0.05\textwidth]{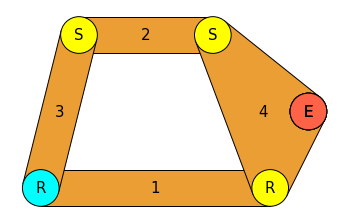}}{{\tiny 1D-M19}}
\qquad\subsubfloat{\includegraphics[width=0.05\textwidth]{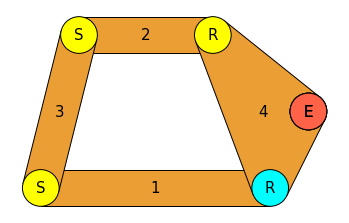}}{{\tiny 1D-M20}}
\qquad\subsubfloat{\includegraphics[width=0.04\textwidth]{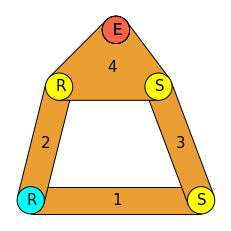}}{{\tiny 1D-M21}}
\qquad\subsubfloat{\includegraphics[width=0.05\textwidth]{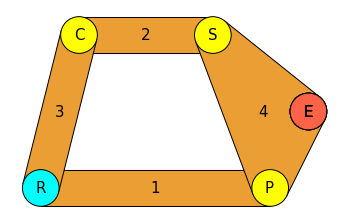}}{{\tiny 1D-M22}}
\qquad\subsubfloat{\includegraphics[width=0.05\textwidth]{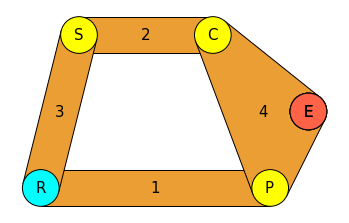}}{{\tiny 1D-M23}}
\qquad\subsubfloat{\includegraphics[width=0.05\textwidth]{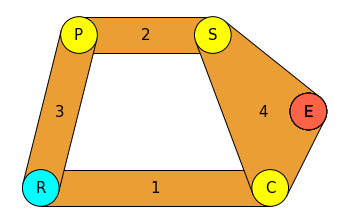}}{{\tiny 1D-M24}}
\qquad\subsubfloat{\includegraphics[width=0.05\textwidth]{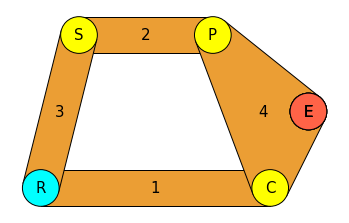}}{{\tiny 1D-M25}}
\qquad\subsubfloat{\includegraphics[width=0.05\textwidth]{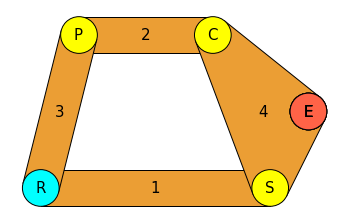}}{{\tiny 1D-M26}}
\qquad\subsubfloat{\includegraphics[width=0.05\textwidth]{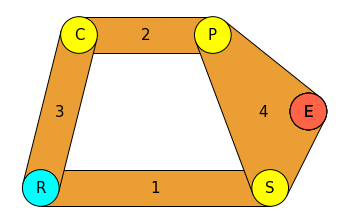}}{{\tiny 1D-M27}}
\qquad\subsubfloat{\includegraphics[width=0.05\textwidth]{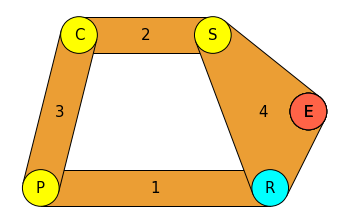}}{{\tiny 1D-M28}}
\qquad\subsubfloat{\includegraphics[width=0.05\textwidth]{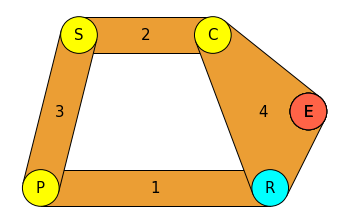}}{{\tiny 1D-M29}}
\qquad\subsubfloat{\includegraphics[width=0.05\textwidth]{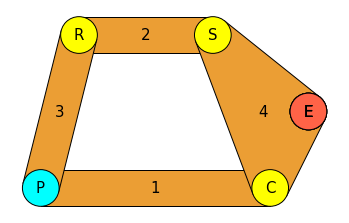}}{{\tiny 1D-M30}}
\qquad\subsubfloat{\includegraphics[width=0.05\textwidth]{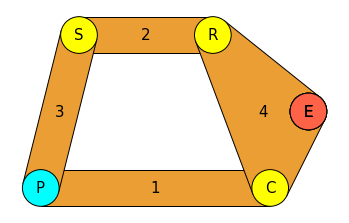}}{{\tiny 1D-M31}}
\qquad\subsubfloat{\includegraphics[width=0.05\textwidth]{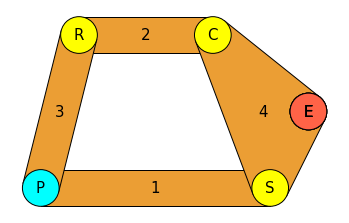}}{{\tiny 1D-M32}}
\qquad\subsubfloat{\includegraphics[width=0.05\textwidth]{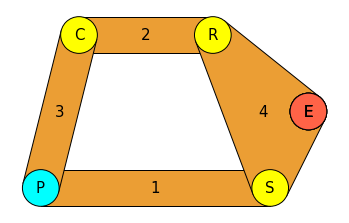}}{{\tiny 1D-M33}}
\qquad\subsubfloat{\includegraphics[width=0.05\textwidth]{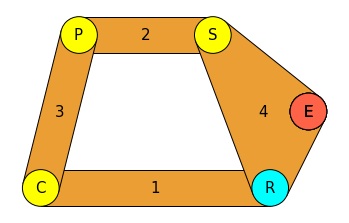}}{{\tiny 1D-M34}}
\qquad\subsubfloat{\includegraphics[width=0.05\textwidth]{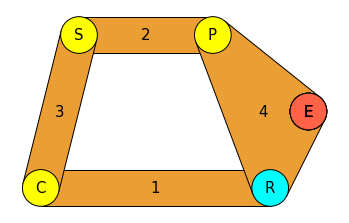}}{{\tiny 1D-M35}}
\qquad\subsubfloat{\includegraphics[width=0.05\textwidth]{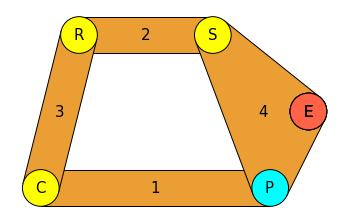}}{{\tiny 1D-M36}}
\qquad\subsubfloat{\includegraphics[width=0.05\textwidth]{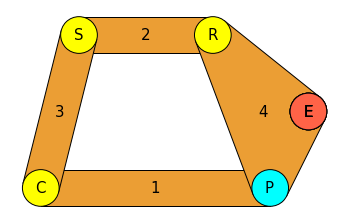}}{{\tiny 1D-M37}}
\qquad\subsubfloat{\includegraphics[width=0.05\textwidth]{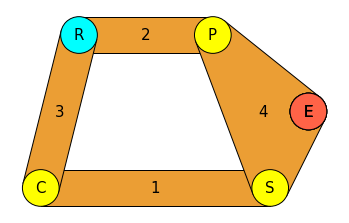}}{{\tiny 1D-M38}}
\qquad\subsubfloat{\includegraphics[width=0.05\textwidth]{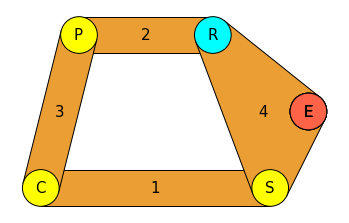}}{{\tiny 1D-M39}}
\qquad\subsubfloat{\includegraphics[width=0.05\textwidth]{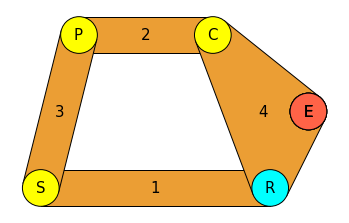}}{{\tiny 1D-M40}}
\qquad\subsubfloat{\includegraphics[width=0.05\textwidth]{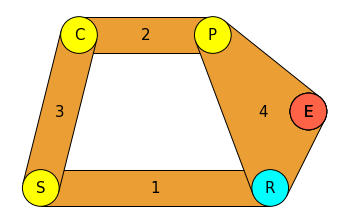}}{{\tiny 1D-M41}}
\qquad\subsubfloat{\includegraphics[width=0.05\textwidth]{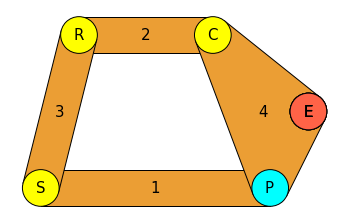}}{{\tiny 1D-M42}}
\qquad\subsubfloat{\includegraphics[width=0.05\textwidth]{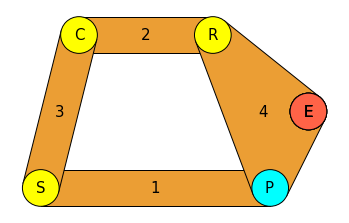}}{{\tiny 1D-M43}}
\qquad\subsubfloat{\includegraphics[width=0.05\textwidth]{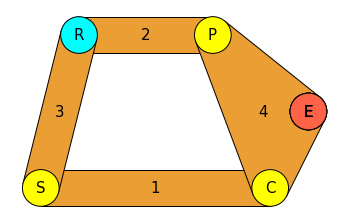}}{{\tiny 1D-M44}}
\qquad\subsubfloat{\includegraphics[width=0.05\textwidth]{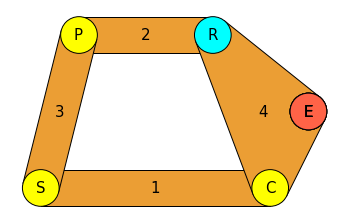}}{{\tiny 1D-M45}}
\qquad\subsubfloat{\includegraphics[width=0.04\textwidth]{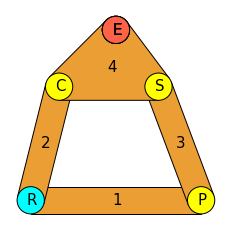}}{{\tiny 1D-M46}}
\qquad\subsubfloat{\includegraphics[width=0.04\textwidth]{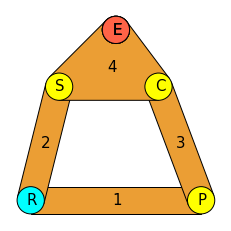}}{{\tiny 1D-M47}}
\qquad\subsubfloat{\includegraphics[width=0.04\textwidth]{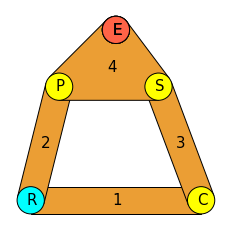}}{{\tiny 1D-M48}}
\qquad\subsubfloat{\includegraphics[width=0.04\textwidth]{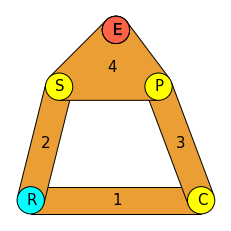}}{{\tiny 1D-M49}}
\qquad\subsubfloat{\includegraphics[width=0.04\textwidth]{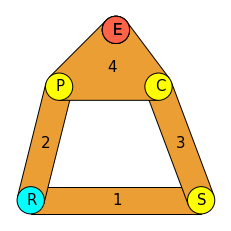}}{{\tiny 1D-M50}}
\qquad\subsubfloat{\includegraphics[width=0.04\textwidth]{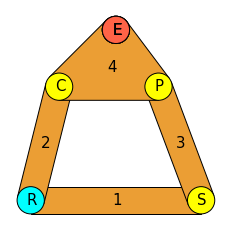}}{{\tiny 1D-M51}}
\qquad\subsubfloat{\includegraphics[width=0.04\textwidth]{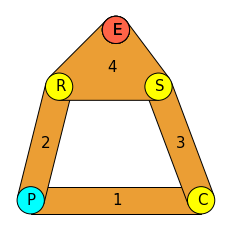}}{{\tiny 1D-M52}}
\qquad\subsubfloat{\includegraphics[width=0.04\textwidth]{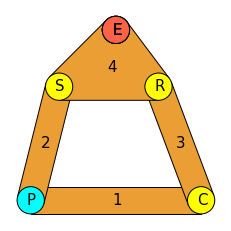}}{{\tiny 1D-M53}}
\qquad\subsubfloat{\includegraphics[width=0.04\textwidth]{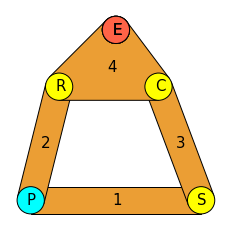}}{{\tiny 1D-M54}}
\qquad\subsubfloat{\includegraphics[width=0.04\textwidth]{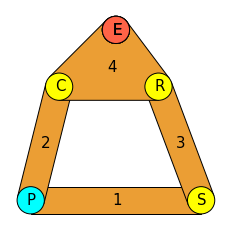}}{{\tiny 1D-M55}}
\qquad\subsubfloat{\includegraphics[width=0.04\textwidth]{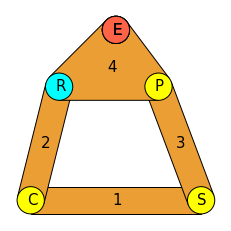}}{{\tiny 1D-M56}}
\qquad\subsubfloat{\includegraphics[width=0.04\textwidth]{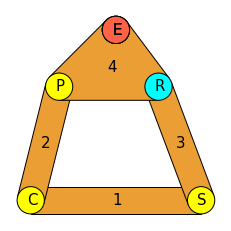}}{{\tiny 1D-M57}}
\qquad\subsubfloat{\includegraphics[width=0.05\textwidth]{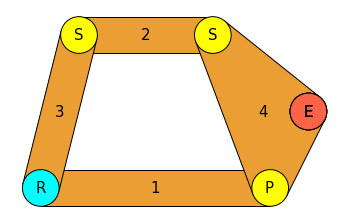}}{{\tiny 1D-M58}}
\qquad\subsubfloat{\includegraphics[width=0.05\textwidth]{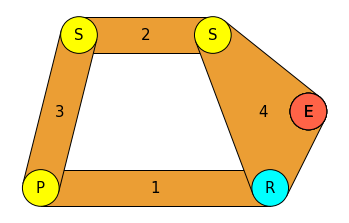}}{{\tiny 1D-M59}}
\qquad\subsubfloat{\includegraphics[width=0.05\textwidth]{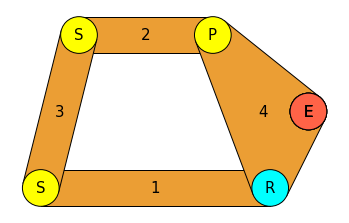}}{{\tiny 1D-M60}}
\qquad\subsubfloat{\includegraphics[width=0.05\textwidth]{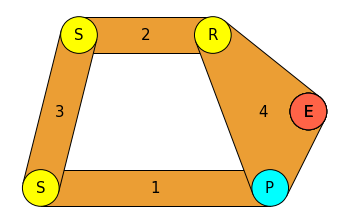}}{{\tiny 1D-M61}}
\qquad\subsubfloat{\includegraphics[width=0.04\textwidth]{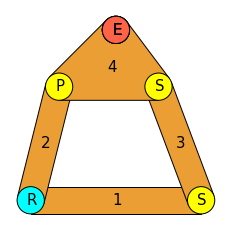}}{{\tiny 1D-M62}}
\qquad\subsubfloat{\includegraphics[width=0.04\textwidth]{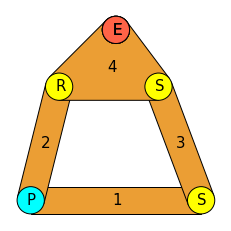}}{{\tiny 1D-M63}}
\qquad\subsubfloat{\includegraphics[width=0.05\textwidth]{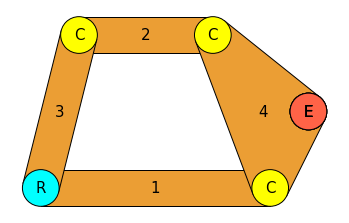}}{{\tiny 1D-M64}}
\qquad\subsubfloat{\includegraphics[width=0.05\textwidth]{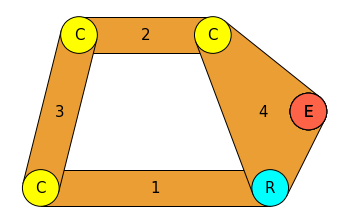}}{{\tiny 1D-M65}}
\qquad\subsubfloat{\includegraphics[width=0.05\textwidth]{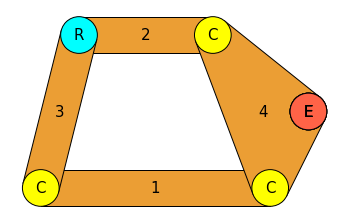}}{{\tiny 1D-M66}}
\qquad\subsubfloat{\includegraphics[width=0.05\textwidth]{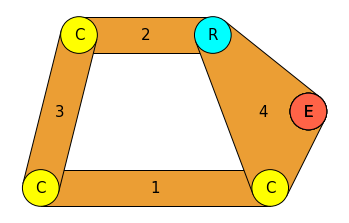}}{{\tiny 1D-M67}}
\qquad\subsubfloat{\includegraphics[width=0.04\textwidth]{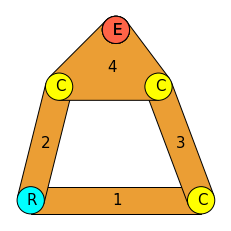}}{{\tiny 1D-M68}}
\qquad\subsubfloat{\includegraphics[width=0.04\textwidth]{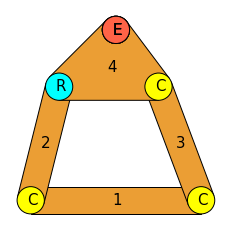}}{{\tiny 1D-M69}}
\qquad\subsubfloat{\includegraphics[width=0.05\textwidth]{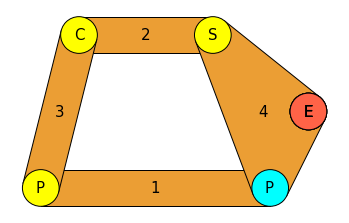}}{{\tiny 1D-M70}}
\qquad\subsubfloat{\includegraphics[width=0.05\textwidth]{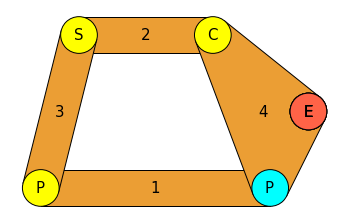}}{{\tiny 1D-M71}}
\qquad\subsubfloat{\includegraphics[width=0.05\textwidth]{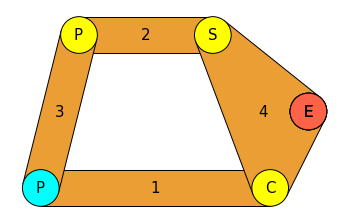}}{{\tiny 1D-M72}}
\qquad\subsubfloat{\includegraphics[width=0.05\textwidth]{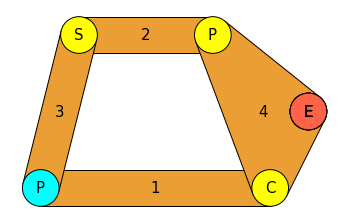}}{{\tiny 1D-M73}}
\qquad\subsubfloat{\includegraphics[width=0.05\textwidth]{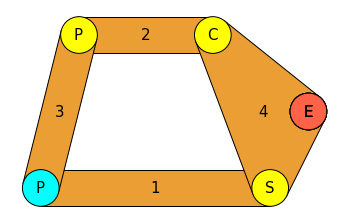}}{{\tiny 1D-M74}}
\qquad\subsubfloat{\includegraphics[width=0.05\textwidth]{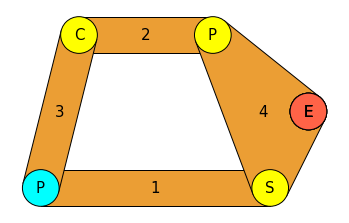}}{{\tiny 1D-M75}}
\qquad\subsubfloat{\includegraphics[width=0.05\textwidth]{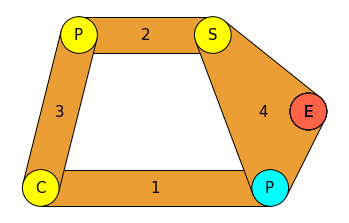}}{{\tiny 1D-M76}}
\qquad\subsubfloat{\includegraphics[width=0.05\textwidth]{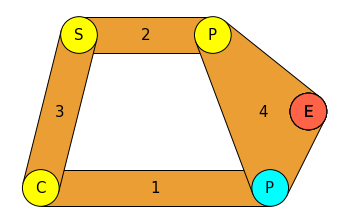}}{{\tiny 1D-M77}}
\qquad\subsubfloat{\includegraphics[width=0.05\textwidth]{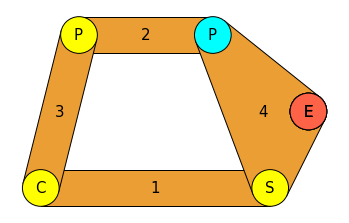}}{{\tiny 1D-M78}}
\qquad\subsubfloat{\includegraphics[width=0.05\textwidth]{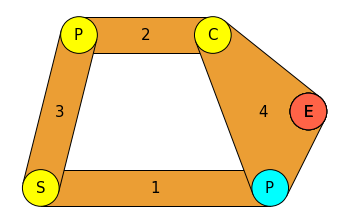}}{{\tiny 1D-M79}}
\qquad\subsubfloat{\includegraphics[width=0.05\textwidth]{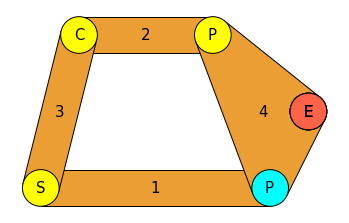}}{{\tiny 1D-M80}}
\qquad\subsubfloat{\includegraphics[width=0.05\textwidth]{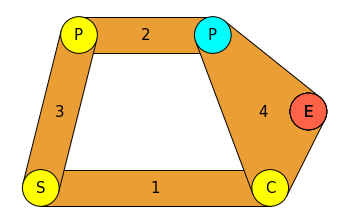}}{{\tiny 1D-M81}}
\qquad\subsubfloat{\includegraphics[width=0.04\textwidth]{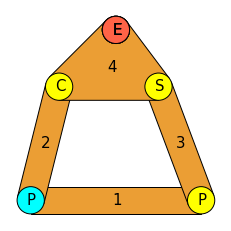}}{{\tiny 1D-M82}}
\qquad\subsubfloat{\includegraphics[width=0.04\textwidth]{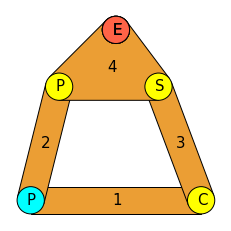}}{{\tiny 1D-M83}}
\qquad\subsubfloat{\includegraphics[width=0.04\textwidth]{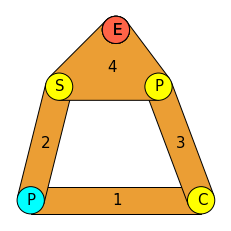}}{{\tiny 1D-M84}}
\qquad\subsubfloat{\includegraphics[width=0.04\textwidth]{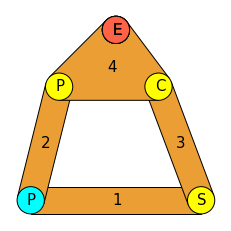}}{{\tiny 1D-M85}}
\qquad\qquad\subsubfloat{\includegraphics[width=0.04\textwidth]{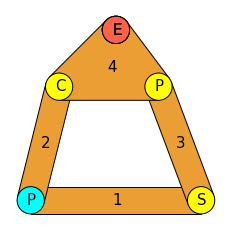}}{{\tiny 1D-M86}}
\qquad\subsubfloat{\includegraphics[width=0.04\textwidth]{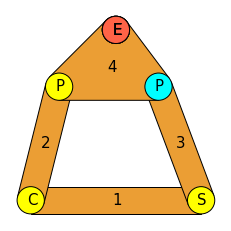}}{{\tiny 1D-M87}}
\qquad\subsubfloat{\includegraphics[width=0.05\textwidth]{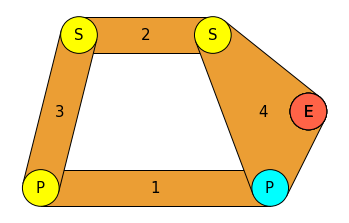}}{{\tiny 1D-M88}}
\qquad\subsubfloat{\includegraphics[width=0.05\textwidth]{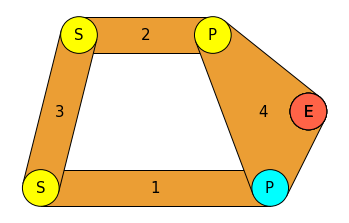}}{{\tiny 1D-M89}}
\qquad\subsubfloat{\includegraphics[width=0.04\textwidth]{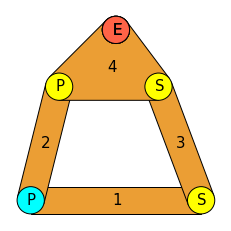}}{{\tiny 1D-M90}}
\qquad\subsubfloat{\includegraphics[width=0.05\textwidth]{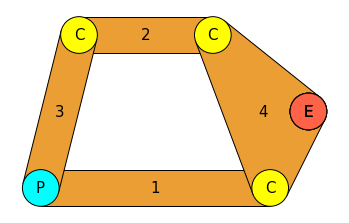}}{{\tiny 1D-M91}}
\qquad\subsubfloat{\includegraphics[width=0.05\textwidth]{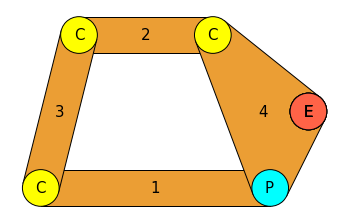}}{{\tiny 1D-M92}}
\qquad\subsubfloat{\includegraphics[width=0.05\textwidth]{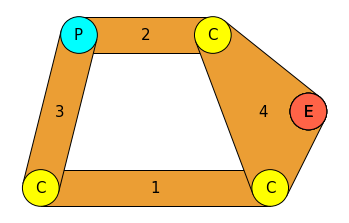}}{{\tiny 1D-M93}}
\qquad\subsubfloat{\includegraphics[width=0.05\textwidth]{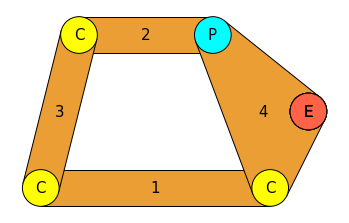}}{{\tiny 1D-M94}}
\qquad\subsubfloat{\includegraphics[width=0.04\textwidth]{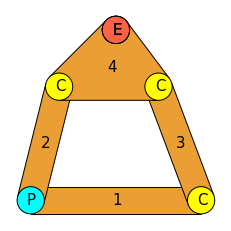}}{{\tiny 1D-M95}}
\qquad\subsubfloat{\includegraphics[width=0.04\textwidth]{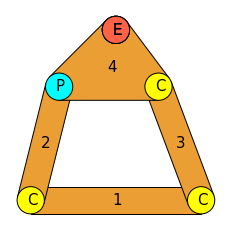}}{{\tiny 1D-M96}}

  \end{minipage}
\end{subfigure}
\caption{Schematic diagrams of 1-DOF Manipulators}
\end{figure}

\begin{figure}[H]
\centering
\begin{subfigure}{\columnwidth}
  \begin{minipage}{\textwidth}\footnotesize
  \centering
\subsubfloat{\includegraphics[width=0.05\textwidth]{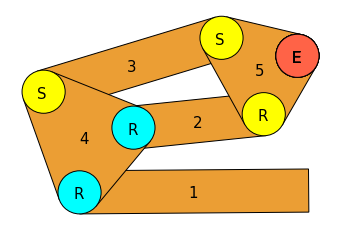}}{{\tiny 2D-M1}}
\qquad\subsubfloat{\includegraphics[width=0.05\textwidth]{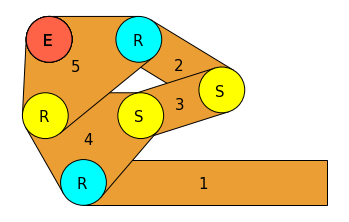}}{{\tiny 2D-M2}}
\qquad\subsubfloat{\includegraphics[width=0.05\textwidth]{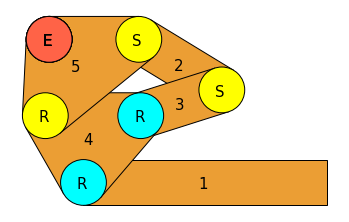}}{{\tiny 2D-M3}}
\qquad\subsubfloat{\includegraphics[width=0.05\textwidth]{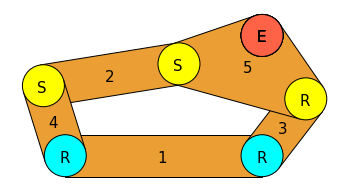}}{{\tiny 2D-M4}}
\qquad\subsubfloat{\includegraphics[width=0.05\textwidth]{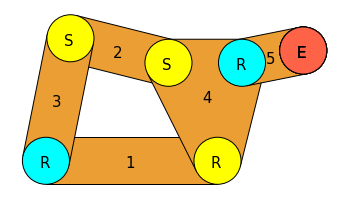}}{{\tiny 2D-M5}}
\qquad\subsubfloat{\includegraphics[width=0.05\textwidth]{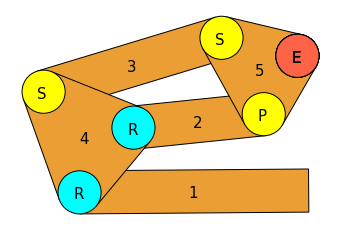}}{{\tiny 2D-M6}}
\qquad\subsubfloat{\includegraphics[width=0.05\textwidth]{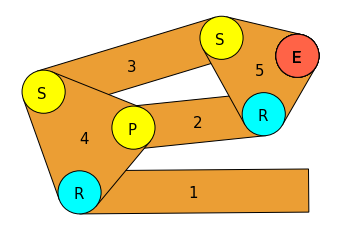}}{{\tiny 2D-M7}}
\qquad\subsubfloat{\includegraphics[width=0.05\textwidth]{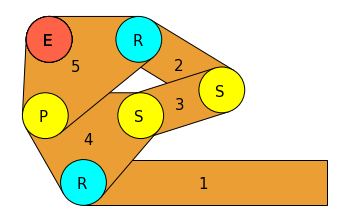}}{{\tiny 2D-M8}}
\qquad\subsubfloat{\includegraphics[width=0.05\textwidth]{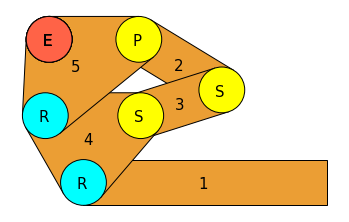}}{{\tiny 2D-M9}}
\qquad\subsubfloat{\includegraphics[width=0.05\textwidth]{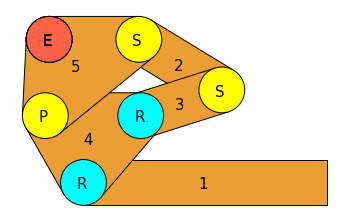}}{{\tiny 2D-M10}}
\qquad\subsubfloat{\includegraphics[width=0.05\textwidth]{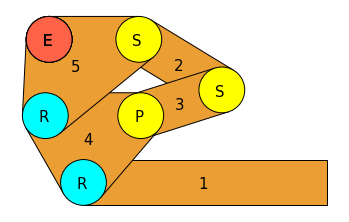}}{{\tiny 2D-M11}}    
\qquad\subsubfloat{\includegraphics[width=0.05\textwidth]{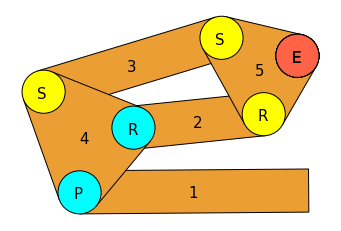}}{{\tiny 2D-M12}}
\qquad\subsubfloat{\includegraphics[width=0.05\textwidth]{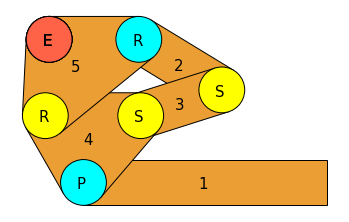}}{{\tiny 2D-M13}}
\qquad\subsubfloat{\includegraphics[width=0.05\textwidth]{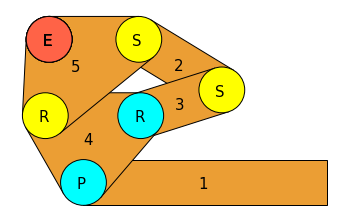}}{{\tiny 2D-M14}}
\qquad\subsubfloat{\includegraphics[width=0.05\textwidth]{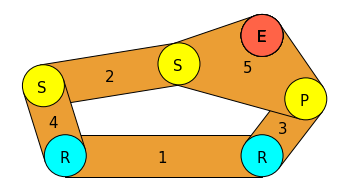}}{{\tiny 2D-M15}}
\qquad\subsubfloat{\includegraphics[width=0.05\textwidth]{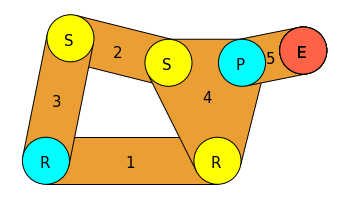}}{{\tiny 2D-M16}}
\qquad\subsubfloat{\includegraphics[width=0.05\textwidth]{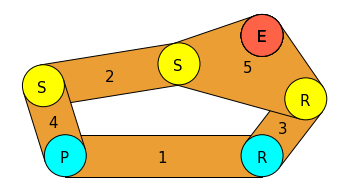}}{{\tiny 2D-M17}}
\qquad\subsubfloat{\includegraphics[width=0.05\textwidth]{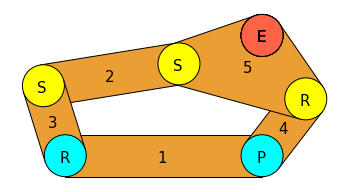}}{{\tiny 2D-M18}}
\qquad\subsubfloat{\includegraphics[width=0.05\textwidth]{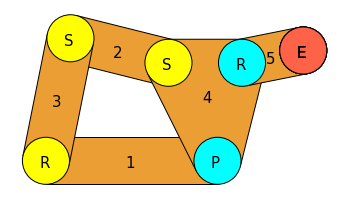}}{{\tiny 2D-M19}}
\qquad\subsubfloat{\includegraphics[width=0.05\textwidth]{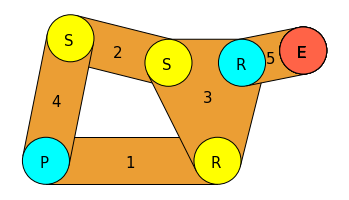}}{{\tiny 2D-M20}}
\qquad\subsubfloat{\includegraphics[width=0.05\textwidth]{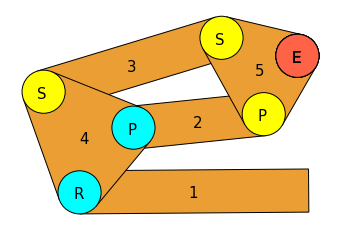}}{{\tiny 2D-M21}}
\qquad\subsubfloat{\includegraphics[width=0.05\textwidth]{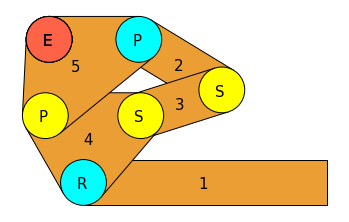}}{{\tiny 2D-M22}}
\qquad\subsubfloat{\includegraphics[width=0.05\textwidth]{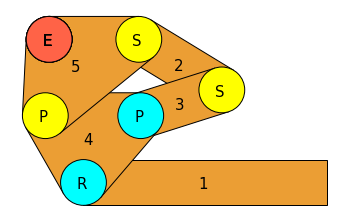}}{{\tiny 2D-M23}}
\qquad\subsubfloat{\includegraphics[width=0.05\textwidth]{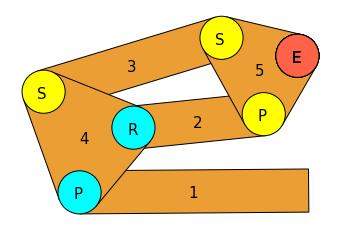}}{{\tiny 2D-M24}}
\qquad\subsubfloat{\includegraphics[width=0.05\textwidth]{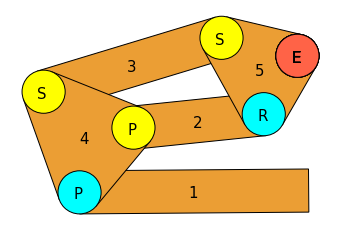}}{{\tiny 2D-M25}}
\qquad\subsubfloat{\includegraphics[width=0.05\textwidth]{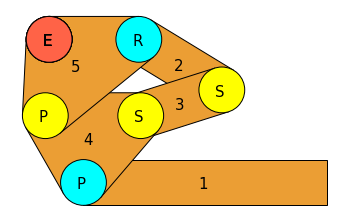}}{{\tiny 2D-M26}}
\qquad\subsubfloat{\includegraphics[width=0.05\textwidth]{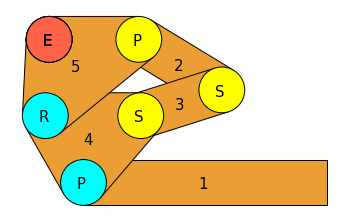}}{{\tiny 2D-M27}}
\qquad\subsubfloat{\includegraphics[width=0.05\textwidth]{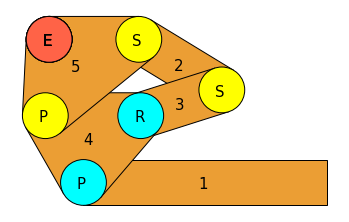}}{{\tiny 2D-M28}}
\qquad\subsubfloat{\includegraphics[width=0.05\textwidth]{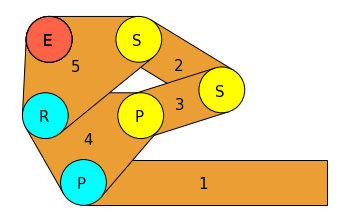}}{{\tiny 2D-M29}}
\qquad\subsubfloat{\includegraphics[width=0.05\textwidth]{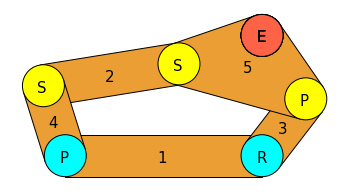}}{{\tiny 2D-M30}}
\qquad\subsubfloat{\includegraphics[width=0.05\textwidth]{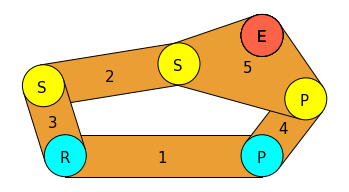}}{{\tiny 2D-M31}}
\qquad\subsubfloat{\includegraphics[width=0.05\textwidth]{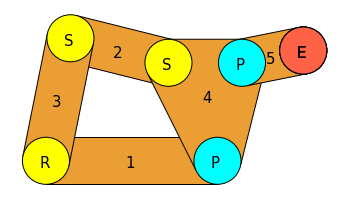}}{{\tiny 2D-M32}}
\qquad\subsubfloat{\includegraphics[width=0.05\textwidth]{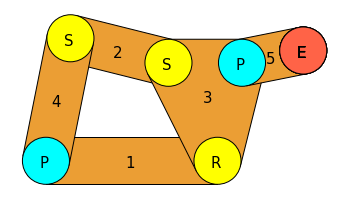}}{{\tiny 2D-M33}}
\qquad\subsubfloat{\includegraphics[width=0.05\textwidth]{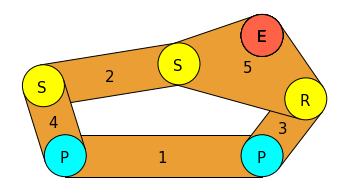}}{{\tiny 2D-M34}}
\qquad\subsubfloat{\includegraphics[width=0.05\textwidth]{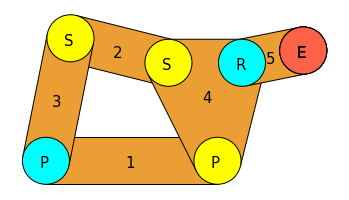}}{{\tiny 2D-M35}}
\qquad\subsubfloat{\includegraphics[width=0.05\textwidth]{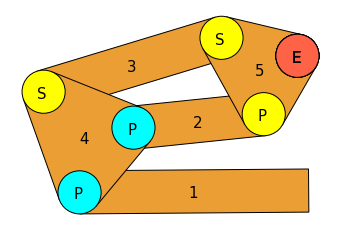}}{{\tiny 2D-M36}}
\qquad\subsubfloat{\includegraphics[width=0.05\textwidth]{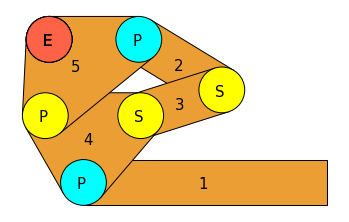}}{{\tiny 2D-M37}}
\qquad\subsubfloat{\includegraphics[width=0.05\textwidth]{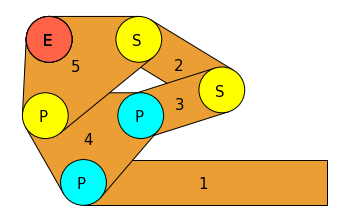}}{{\tiny 2D-M38}}
\qquad\subsubfloat{\includegraphics[width=0.05\textwidth]{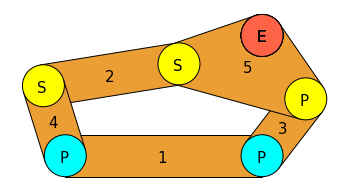}}{{\tiny 2D-M39}}
\qquad\subsubfloat{\includegraphics[width=0.05\textwidth]{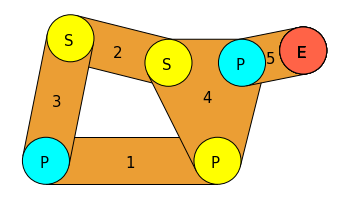}}{{\tiny 2D-M40}}
\qquad\subsubfloat{\includegraphics[width=0.05\textwidth]{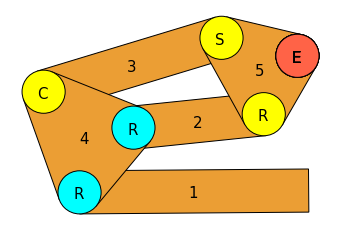}}{{\tiny 2D-M41}}
\qquad\subsubfloat{\includegraphics[width=0.05\textwidth]{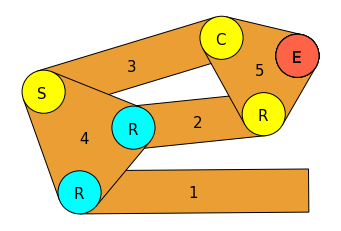}}{{\tiny 2D-M42}}
\qquad\subsubfloat{\includegraphics[width=0.05\textwidth]{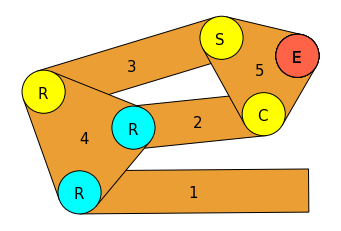}}{{\tiny 2D-M43}}
\qquad\subsubfloat{\includegraphics[width=0.05\textwidth]{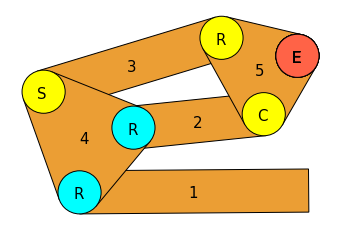}}{{\tiny 2D-M44}}
\qquad\subsubfloat{\includegraphics[width=0.05\textwidth]{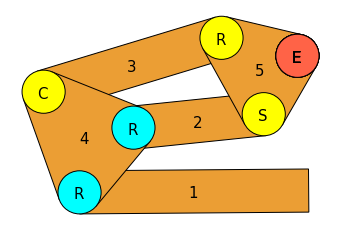}}{{\tiny 2D-M45}}
\qquad\subsubfloat{\includegraphics[width=0.05\textwidth]{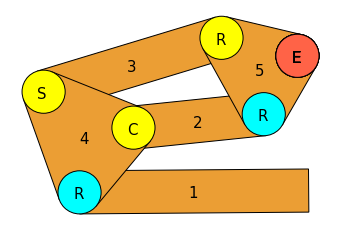}}{{\tiny 2D-M46}}
\qquad\subsubfloat{\includegraphics[width=0.05\textwidth]{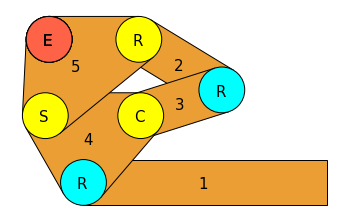}}{{\tiny 2D-M47}}
\qquad\subsubfloat{\includegraphics[width=0.05\textwidth]{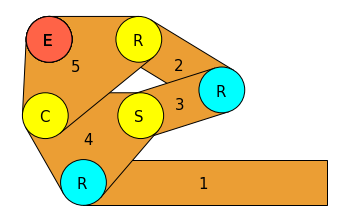}}{{\tiny 2D-M48}}
\qquad\subsubfloat{\includegraphics[width=0.05\textwidth]{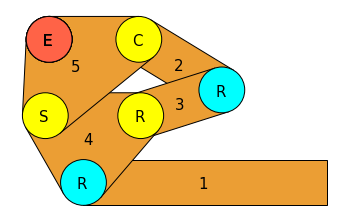}}{{\tiny 2D-M49}}
\qquad\subsubfloat{\includegraphics[width=0.05\textwidth]{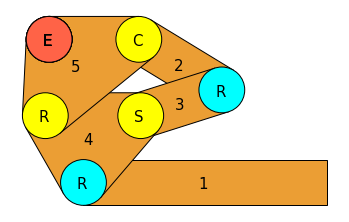}}{{\tiny 2D-M50}}
\qquad\subsubfloat{\includegraphics[width=0.05\textwidth]{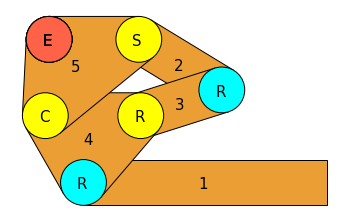}}{{\tiny 2D-M51}}
\qquad\subsubfloat{\includegraphics[width=0.05\textwidth]{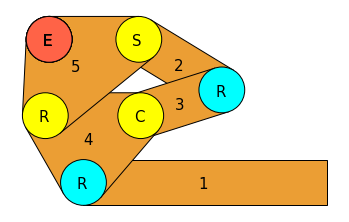}}{{\tiny 2D-M52}}
\qquad\subsubfloat{\includegraphics[width=0.05\textwidth]{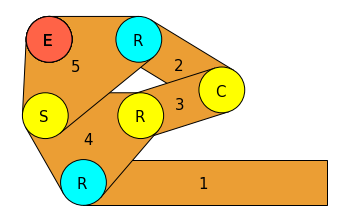}}{{\tiny 2D-M53}}
\qquad\subsubfloat{\includegraphics[width=0.05\textwidth]{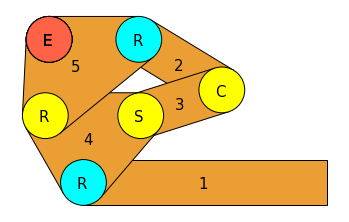}}{{\tiny 2D-M54}}
\qquad\subsubfloat{\includegraphics[width=0.05\textwidth]{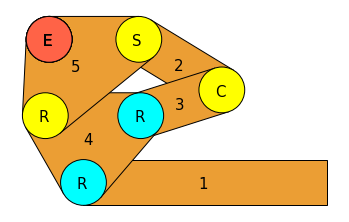}}{{\tiny 2D-M55}}
\qquad\subsubfloat{\includegraphics[width=0.05\textwidth]{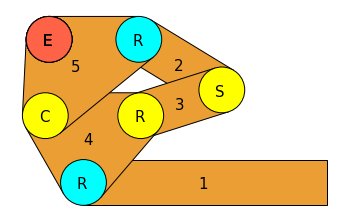}}{{\tiny 2D-M56}}
\qquad\subsubfloat{\includegraphics[width=0.05\textwidth]{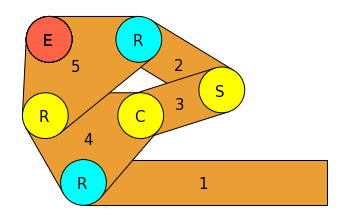}}{{\tiny 2D-M57}}
\qquad\subsubfloat{\includegraphics[width=0.05\textwidth]{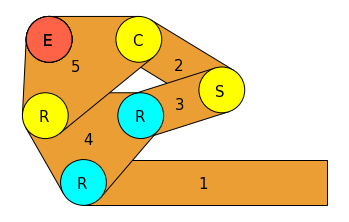}}{{\tiny 2D-M58}}
\qquad\subsubfloat{\includegraphics[width=0.05\textwidth]{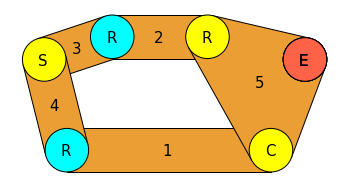}}{{\tiny 2D-M59}}
\qquad\subsubfloat{\includegraphics[width=0.05\textwidth]{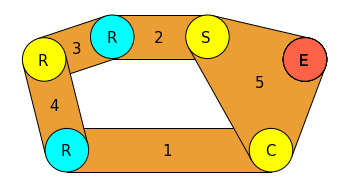}}{{\tiny 2D-M60}}
\qquad\subsubfloat{\includegraphics[width=0.05\textwidth]{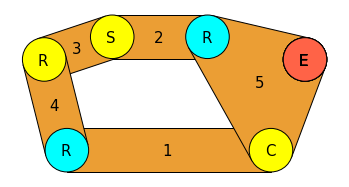}}{{\tiny 2D-M61}}
\qquad\subsubfloat{\includegraphics[width=0.05\textwidth]{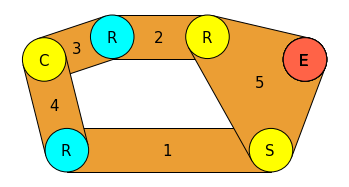}}{{\tiny 2D-M62}}
\qquad\subsubfloat{\includegraphics[width=0.05\textwidth]{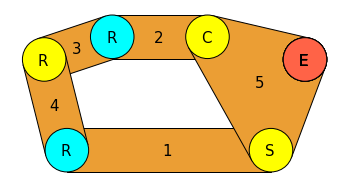}}{{\tiny 2D-M63}}
\qquad\subsubfloat{\includegraphics[width=0.05\textwidth]{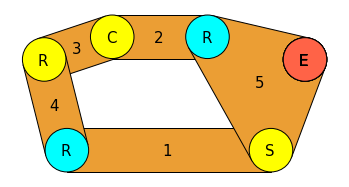}}{{\tiny 2D-M64}}
\qquad\subsubfloat{\includegraphics[width=0.05\textwidth]{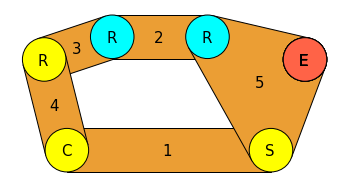}}{{\tiny 2D-M65}}
\qquad\subsubfloat{\includegraphics[width=0.05\textwidth]{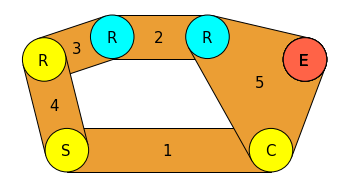}}{{\tiny 2D-M66}}
\qquad\subsubfloat{\includegraphics[width=0.05\textwidth]{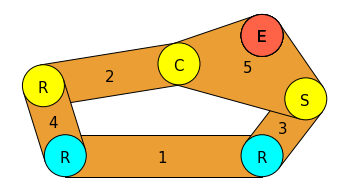}}{{\tiny 2D-M67}}
\qquad\subsubfloat{\includegraphics[width=0.05\textwidth]{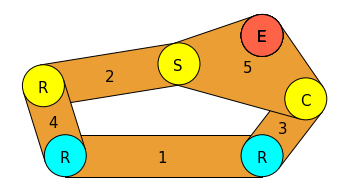}}{{\tiny 2D-M68}}
\qquad\subsubfloat{\includegraphics[width=0.05\textwidth]{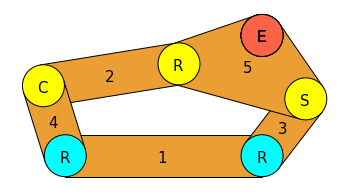}}{{\tiny 2D-M69}}
\qquad\subsubfloat{\includegraphics[width=0.05\textwidth]{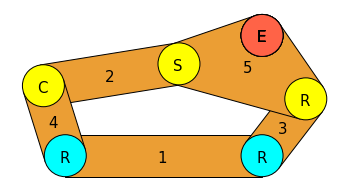}}{{\tiny 2D-M70}}
\qquad\subsubfloat{\includegraphics[width=0.05\textwidth]{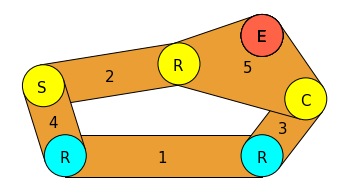}}{{\tiny 2D-M71}}
\qquad\subsubfloat{\includegraphics[width=0.05\textwidth]{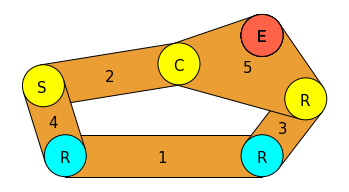}}{{\tiny 2D-M72}}
\qquad\subsubfloat{\includegraphics[width=0.05\textwidth]{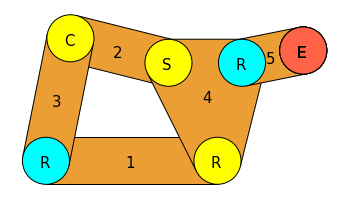}}{{\tiny 2D-M73}}
\qquad\subsubfloat{\includegraphics[width=0.05\textwidth]{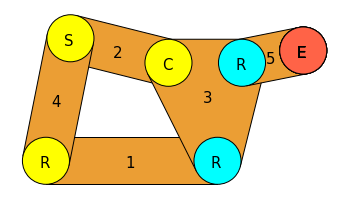}}{{\tiny 2D-M74}}
\qquad\subsubfloat{\includegraphics[width=0.05\textwidth]{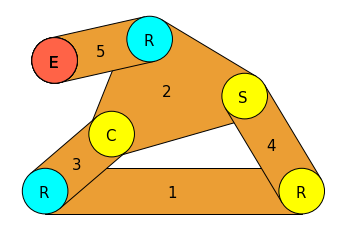}}{{\tiny 2D-M75}}
\qquad\subsubfloat{\includegraphics[width=0.05\textwidth]{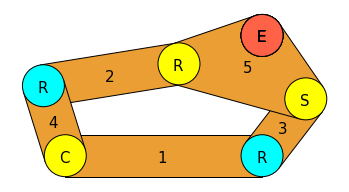}}{{\tiny 2D-M76}}
\qquad\subsubfloat{\includegraphics[width=0.05\textwidth]{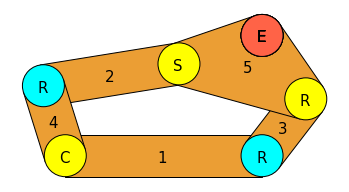}}{{\tiny 2D-M77}}
\qquad\subsubfloat{\includegraphics[width=0.05\textwidth]{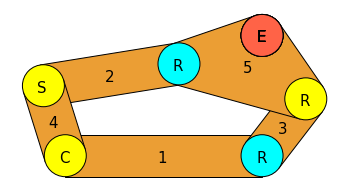}}{{\tiny 2D-M78}}
\qquad\subsubfloat{\includegraphics[width=0.05\textwidth]{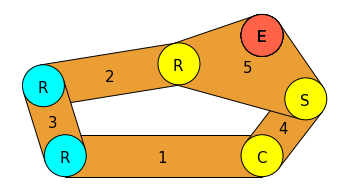}}{{\tiny 2D-M79}}
\qquad\subsubfloat{\includegraphics[width=0.05\textwidth]{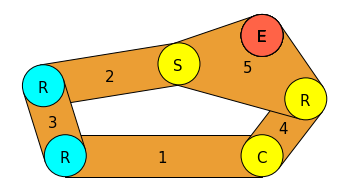}}{{\tiny 2D-M80}}
\qquad\subsubfloat{\includegraphics[width=0.05\textwidth]{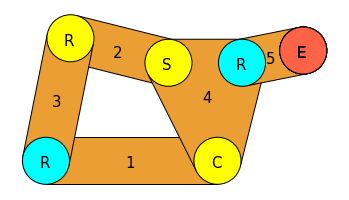}}{{\tiny 2D-M81}}
\qquad\subsubfloat{\includegraphics[width=0.05\textwidth]{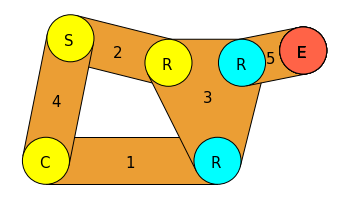}}{{\tiny 2D-M82}}
\qquad\subsubfloat{\includegraphics[width=0.05\textwidth]{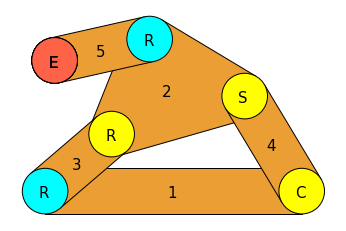}}{{\tiny 2D-M83}}
\qquad\subsubfloat{\includegraphics[width=0.05\textwidth]{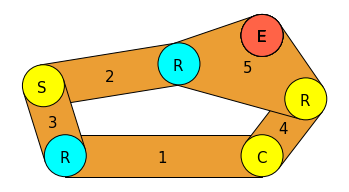}}{{\tiny 2D-M84}}
\qquad\subsubfloat{\includegraphics[width=0.05\textwidth]{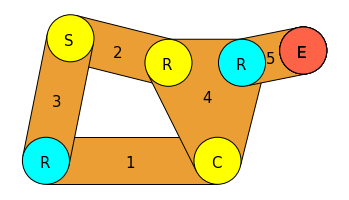}}{{\tiny 2D-M85}}
\qquad\subsubfloat{\includegraphics[width=0.05\textwidth]{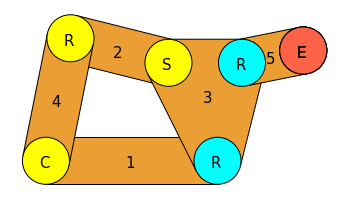}}{{\tiny 2D-M86}}
\qquad\subsubfloat{\includegraphics[width=0.05\textwidth]{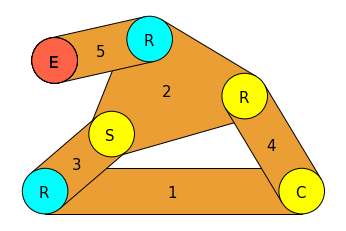}}{{\tiny 2D-M87}}
\qquad\subsubfloat{\includegraphics[width=0.05\textwidth]{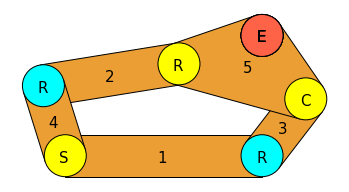}}{{\tiny 2D-M88}}
\qquad\subsubfloat{\includegraphics[width=0.05\textwidth]{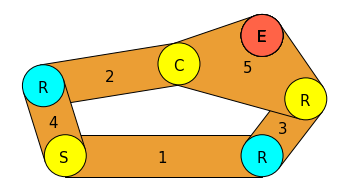}}{{\tiny 2D-M89}}
\qquad\subsubfloat{\includegraphics[width=0.05\textwidth]{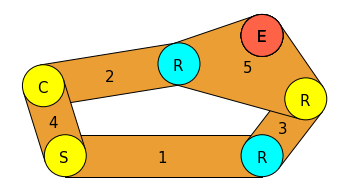}}{{\tiny 2D-M90}}
\qquad\subsubfloat{\includegraphics[width=0.05\textwidth]{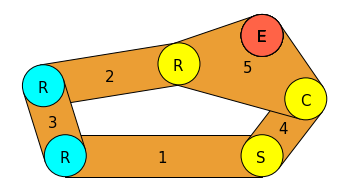}}{{\tiny 2D-M91}}
\qquad\subsubfloat{\includegraphics[width=0.05\textwidth]{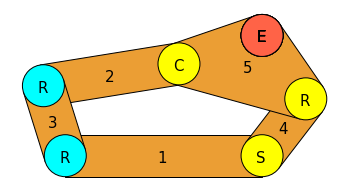}}{{\tiny 2D-M92}}
\qquad\subsubfloat{\includegraphics[width=0.05\textwidth]{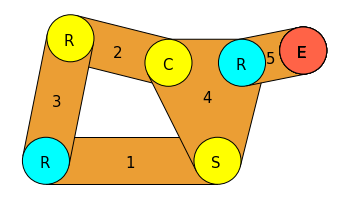}}{{\tiny 2D-M93}}
\qquad\subsubfloat{\includegraphics[width=0.05\textwidth]{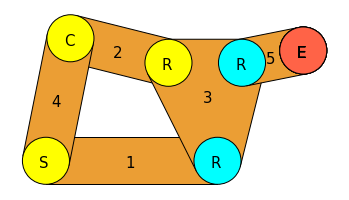}}{{\tiny 2D-M94}}
\qquad\subsubfloat{\includegraphics[width=0.05\textwidth]{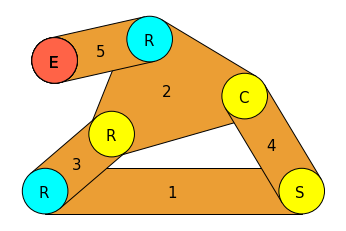}}{{\tiny 2D-M95}}
\qquad\subsubfloat{\includegraphics[width=0.05\textwidth]{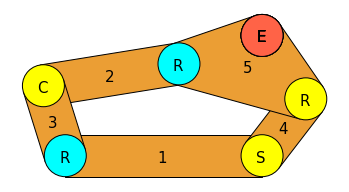}}{{\tiny 2D-M96}} 
\qquad\subsubfloat{\includegraphics[width=0.05\textwidth]{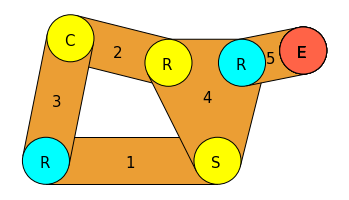}}{{\tiny 2D-M97}}
\qquad\subsubfloat{\includegraphics[width=0.05\textwidth]{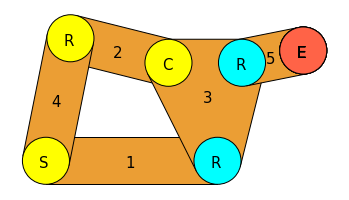}}{{\tiny 2D-M98}}
\qquad\subsubfloat{\includegraphics[width=0.05\textwidth]{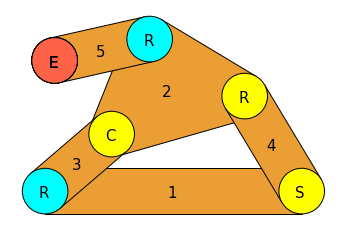}}{{\tiny 2D-M99}}
\qquad\subsubfloat{\includegraphics[width=0.05\textwidth]{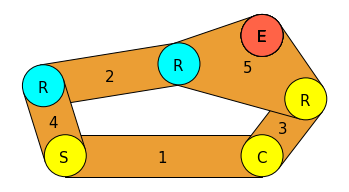}}{{\tiny 2D-M100}}
\qquad\subsubfloat{\includegraphics[width=0.05\textwidth]{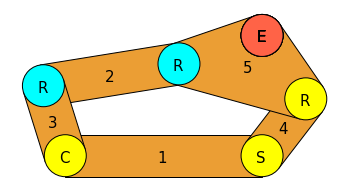}}{{\tiny 2D-M101}}
\qquad\subsubfloat{\includegraphics[width=0.05\textwidth]{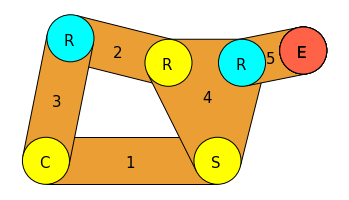}}{{\tiny 2D-M102}}
\qquad\subsubfloat{\includegraphics[width=0.05\textwidth]{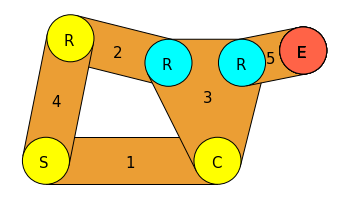}}{{\tiny 2D-M103}}
\qquad\subsubfloat{\includegraphics[width=0.05\textwidth]{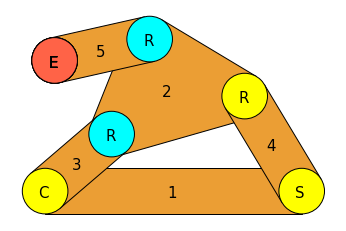}}{{\tiny 2D-M104}}
\qquad\subsubfloat{\includegraphics[width=0.05\textwidth]{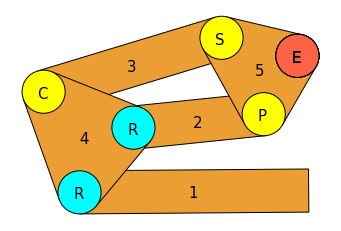}}{{\tiny 2D-M105}}
\qquad\subsubfloat{\includegraphics[width=0.05\textwidth]{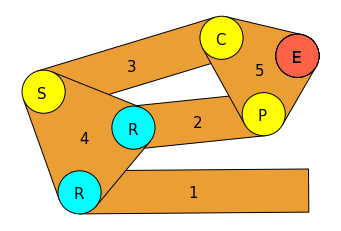}}{{\tiny 2D-M106}}
\qquad\subsubfloat{\includegraphics[width=0.05\textwidth]{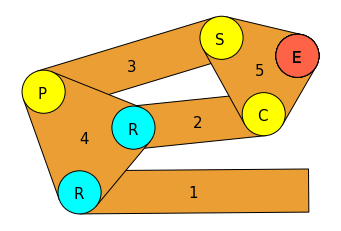}}{{\tiny 2D-M107}}
\qquad\subsubfloat{\includegraphics[width=0.05\textwidth]{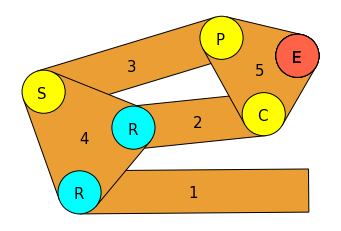}}{{\tiny 2D-M108}}
\qquad\subsubfloat{\includegraphics[width=0.05\textwidth]{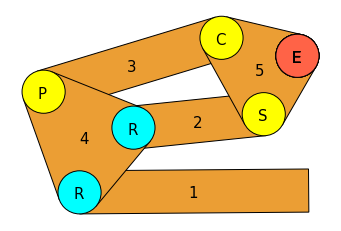}}{{\tiny 2D-M109}}
\qquad\subsubfloat{\includegraphics[width=0.05\textwidth]{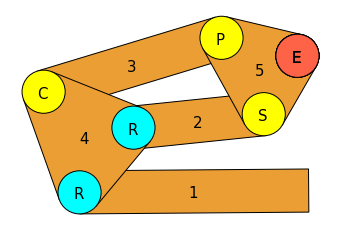}}{{\tiny 2D-M110}}
\qquad\subsubfloat{\includegraphics[width=0.05\textwidth]{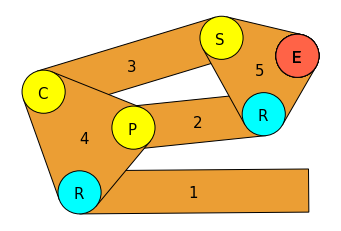}}{{\tiny 2D-M111}}
\qquad\subsubfloat{\includegraphics[width=0.05\textwidth]{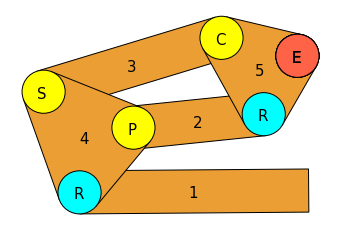}}{{\tiny 2D-M112}}
\qquad\subsubfloat{\includegraphics[width=0.05\textwidth]{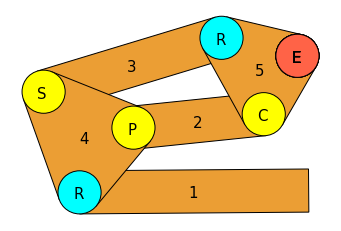}}{{\tiny 2D-M113}}
\qquad\subsubfloat{\includegraphics[width=0.05\textwidth]{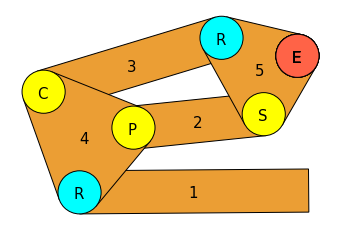}}{{\tiny 2D-M114}}
\qquad\subsubfloat{\includegraphics[width=0.05\textwidth]{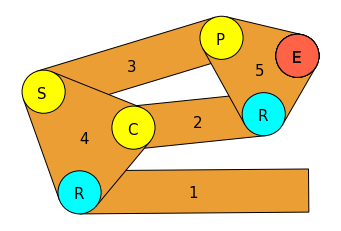}}{{\tiny 2D-M115}}
\qquad\subsubfloat{\includegraphics[width=0.05\textwidth]{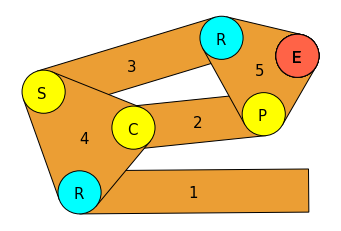}}{{\tiny 2D-M116}}
\qquad\subsubfloat{\includegraphics[width=0.05\textwidth]{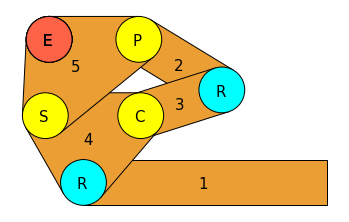}}{{\tiny 2D-M117}}
\qquad\subsubfloat{\includegraphics[width=0.05\textwidth]{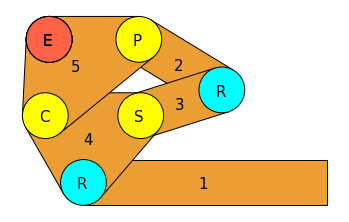}}{{\tiny 2D-M118}}
\qquad\subsubfloat{\includegraphics[width=0.05\textwidth]{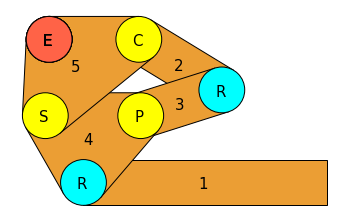}}{{\tiny 2D-M119}}
\qquad\subsubfloat{\includegraphics[width=0.05\textwidth]{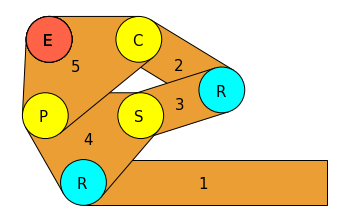}}{{\tiny 2D-M120}}
\qquad\subsubfloat{\includegraphics[width=0.05\textwidth]{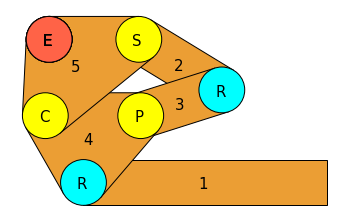}}{{\tiny 2D-M121}}
\qquad\subsubfloat{\includegraphics[width=0.05\textwidth]{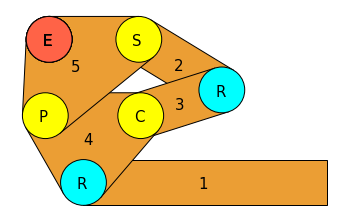}}{{\tiny 2D-M122}}
\qquad\subsubfloat{\includegraphics[width=0.05\textwidth]{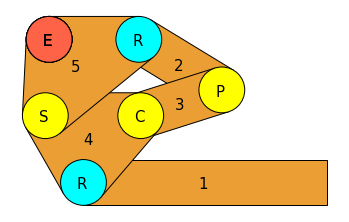}}{{\tiny 2D-M123}}
\qquad\subsubfloat{\includegraphics[width=0.05\textwidth]{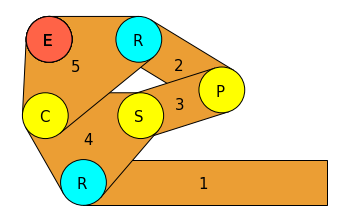}}{{\tiny 2D-M124}}
\qquad\subsubfloat{\includegraphics[width=0.05\textwidth]{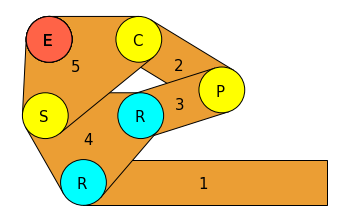}}{{\tiny 2D-M125}}
\qquad\subsubfloat{\includegraphics[width=0.05\textwidth]{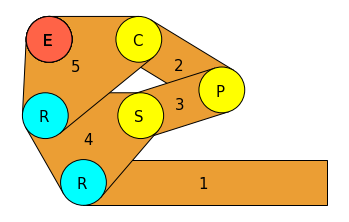}}{{\tiny 2D-M126}}
\qquad\subsubfloat{\includegraphics[width=0.05\textwidth]{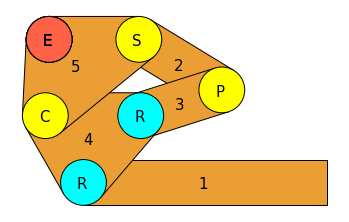}}{{\tiny 2D-M127}}
\qquad\subsubfloat{\includegraphics[width=0.05\textwidth]{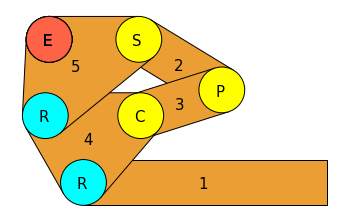}}{{\tiny 2D-M128}}
\qquad\subsubfloat{\includegraphics[width=0.05\textwidth]{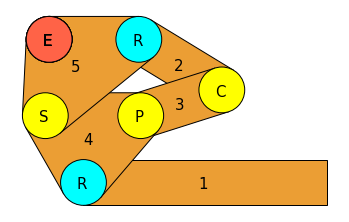}}{{\tiny 2D-M129}}
\qquad\subsubfloat{\includegraphics[width=0.05\textwidth]{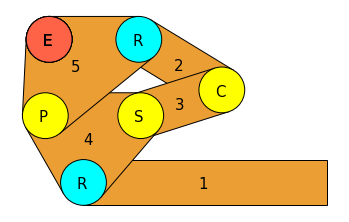}}{{\tiny 2D-M130}}
\qquad\subsubfloat{\includegraphics[width=0.05\textwidth]{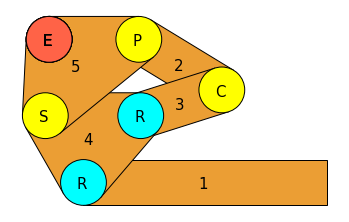}}{{\tiny 2D-M131}}
\qquad\subsubfloat{\includegraphics[width=0.05\textwidth]{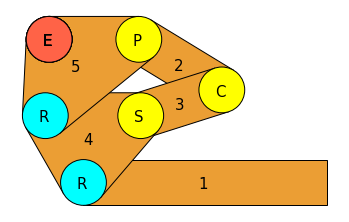}}{{\tiny 2D-M132}}
\qquad\subsubfloat{\includegraphics[width=0.05\textwidth]{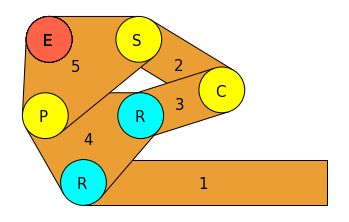}}{{\tiny 2D-M133}}
\qquad\subsubfloat{\includegraphics[width=0.05\textwidth]{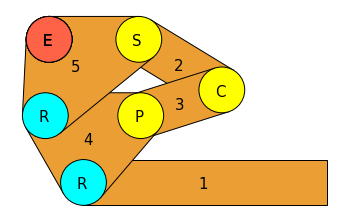}}{{\tiny 2D-M134}}
\qquad\subsubfloat{\includegraphics[width=0.05\textwidth]{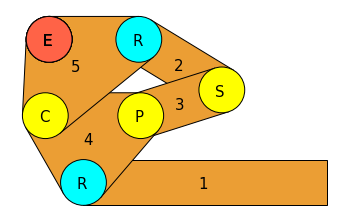}}{{\tiny 2D-M135}}
\qquad\subsubfloat{\includegraphics[width=0.05\textwidth]{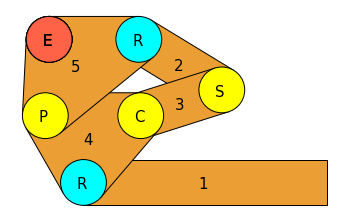}}{{\tiny 2D-M136}}
\qquad\subsubfloat{\includegraphics[width=0.05\textwidth]{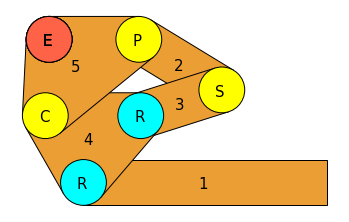}}{{\tiny 2D-M137}}
\qquad\subsubfloat{\includegraphics[width=0.05\textwidth]{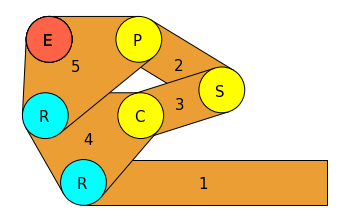}}{{\tiny 2D-M138}}
\qquad\subsubfloat{\includegraphics[width=0.05\textwidth]{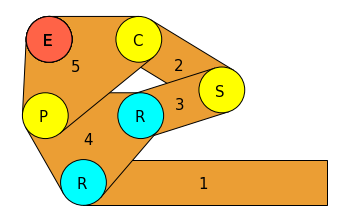}}{{\tiny 2D-M139}}
\qquad\subsubfloat{\includegraphics[width=0.05\textwidth]{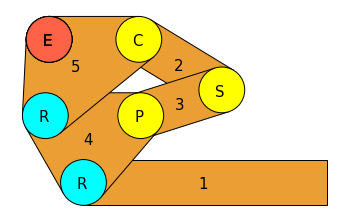}}{{\tiny 2D-M140}}
\qquad  \subsubfloat{\includegraphics[width=0.05\textwidth]{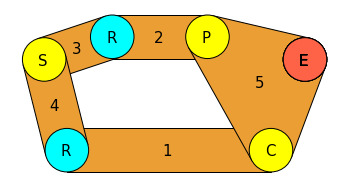}}{{\tiny 2D-M141}}
\qquad\subsubfloat{\includegraphics[width=0.05\textwidth]{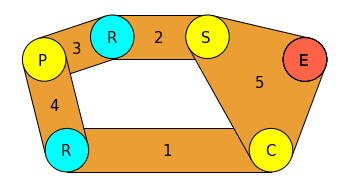}}{{\tiny 2D-M142}}
\qquad\subsubfloat{\includegraphics[width=0.05\textwidth]{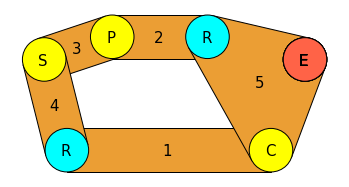}}{{\tiny 2D-M143}}
\qquad\subsubfloat{\includegraphics[width=0.05\textwidth]{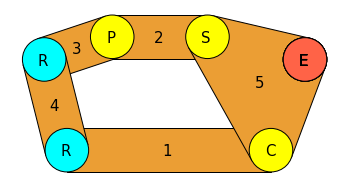}}{{\tiny 2D-M144}}
\qquad\subsubfloat{\includegraphics[width=0.05\textwidth]{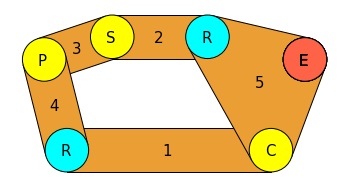}}{{\tiny 2D-M145}}
\qquad\subsubfloat{\includegraphics[width=0.05\textwidth]{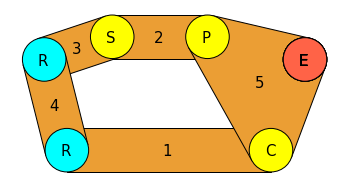}}{{\tiny 2D-M146}}
\qquad\subsubfloat{\includegraphics[width=0.05\textwidth]{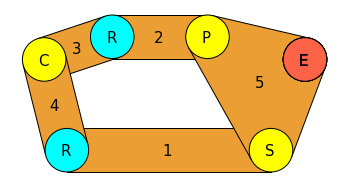}}{{\tiny 2D-M147}}
\qquad\subsubfloat{\includegraphics[width=0.05\textwidth]{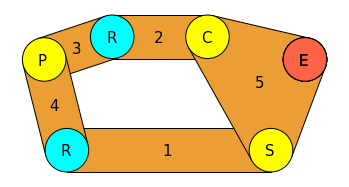}}{{\tiny 2D-M148}}
\qquad\subsubfloat{\includegraphics[width=0.05\textwidth]{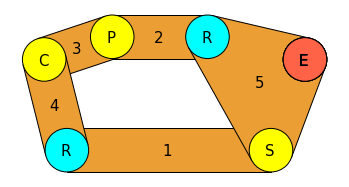}}{{\tiny 2D-M149}}
\qquad\subsubfloat{\includegraphics[width=0.05\textwidth]{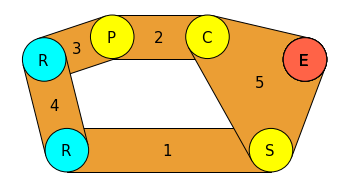}}{{\tiny 2D-M150}}
\qquad\subsubfloat{\includegraphics[width=0.05\textwidth]{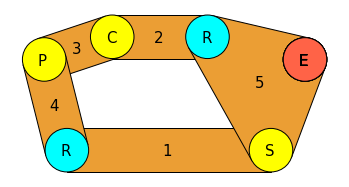}}{{\tiny 2D-M151}}
\qquad\subsubfloat{\includegraphics[width=0.05\textwidth]{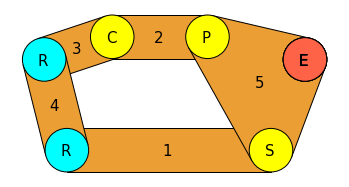}}{{\tiny 2D-M152}}
\qquad\subsubfloat{\includegraphics[width=0.05\textwidth]{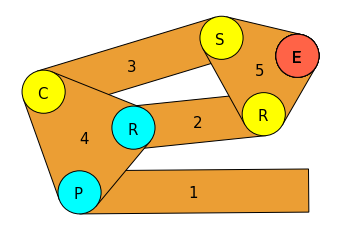}}{{\tiny 2D-M153}}
\qquad\subsubfloat{\includegraphics[width=0.05\textwidth]{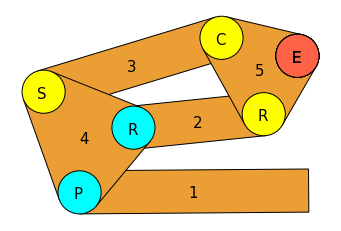}}{{\tiny 2D-M154}}
\qquad\subsubfloat{\includegraphics[width=0.05\textwidth]{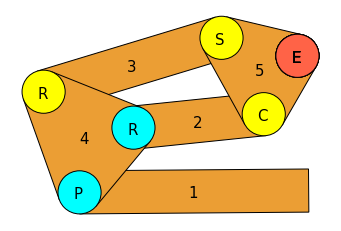}}{{\tiny 2D-M155}}
\qquad\subsubfloat{\includegraphics[width=0.05\textwidth]{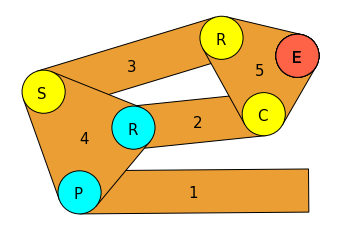}}{{\tiny 2D-M156}}
\qquad\subsubfloat{\includegraphics[width=0.05\textwidth]{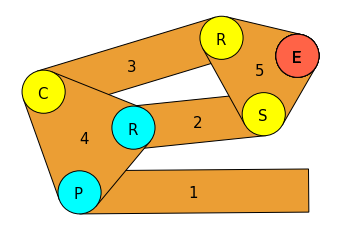}}{{\tiny 2D-M157}}
\qquad\subsubfloat{\includegraphics[width=0.05\textwidth]{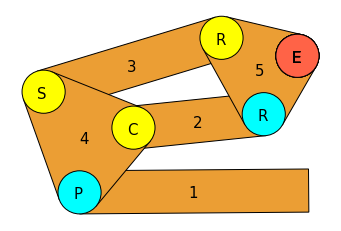}}{{\tiny 2D-M158}}
\qquad\subsubfloat{\includegraphics[width=0.05\textwidth]{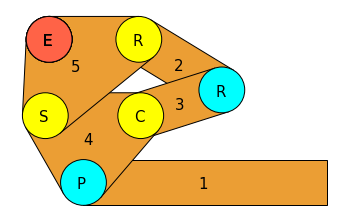}}{{\tiny 2D-M159}}
\qquad\subsubfloat{\includegraphics[width=0.05\textwidth]{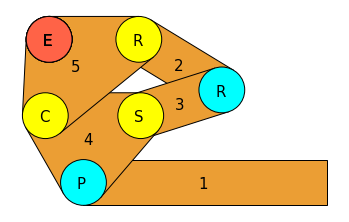}}{{\tiny 2D-M160}} 
\qquad\subsubfloat{\includegraphics[width=0.05\textwidth]{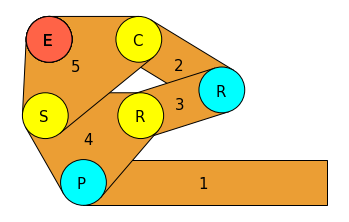}}{{\tiny 2D-M161}}
\qquad\subsubfloat{\includegraphics[width=0.05\textwidth]{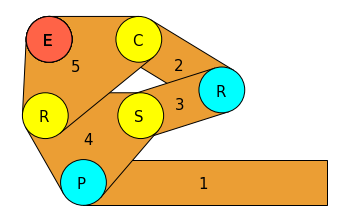}}{{\tiny 2D-M162}}
\qquad\subsubfloat{\includegraphics[width=0.05\textwidth]{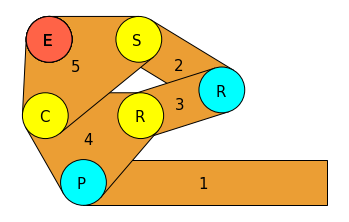}}{{\tiny 2D-M163}}
\qquad\subsubfloat{\includegraphics[width=0.05\textwidth]{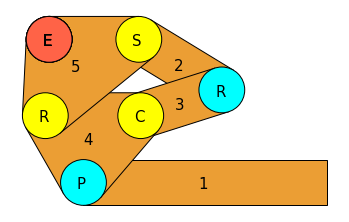}}{{\tiny 2D-M164}}
\qquad\subsubfloat{\includegraphics[width=0.05\textwidth]{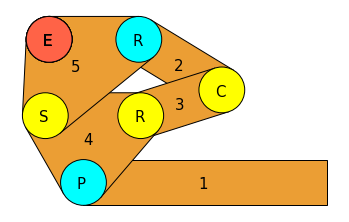}}{{\tiny 2D-M165}}
\qquad\subsubfloat{\includegraphics[width=0.05\textwidth]{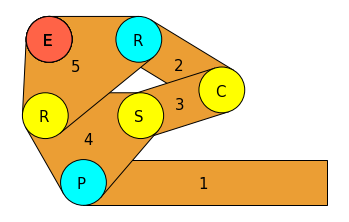}}{{\tiny 2D-M166}}
\qquad\subsubfloat{\includegraphics[width=0.05\textwidth]{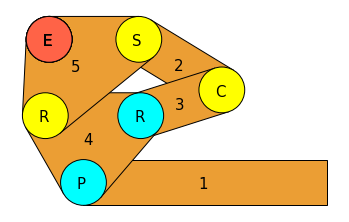}}{{\tiny 2D-M167}}
\qquad\subsubfloat{\includegraphics[width=0.05\textwidth]{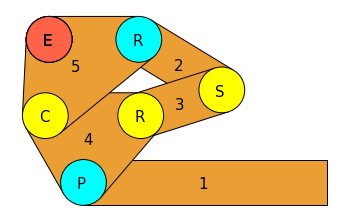}}{{\tiny 2D-M168}}
\qquad\subsubfloat{\includegraphics[width=0.05\textwidth]{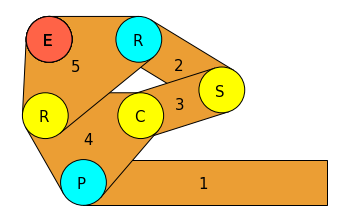}}{{\tiny 2D-M169}}
\qquad\subsubfloat{\includegraphics[width=0.05\textwidth]{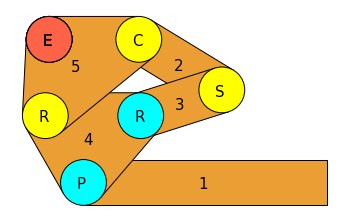}}{{\tiny 2D-M170}}
\qquad\subsubfloat{\includegraphics[width=0.05\textwidth]{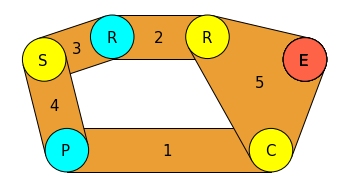}}{{\tiny 2D-M171}}
\qquad\subsubfloat{\includegraphics[width=0.05\textwidth]{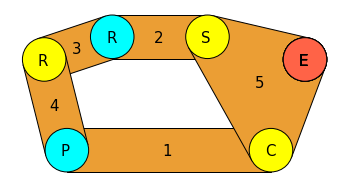}}{{\tiny 2D-M172}}
\qquad\subsubfloat{\includegraphics[width=0.05\textwidth]{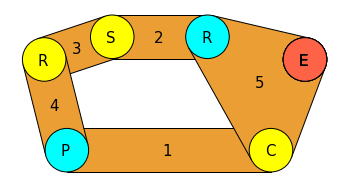}}{{\tiny 2D-M173}}
\qquad\subsubfloat{\includegraphics[width=0.05\textwidth]{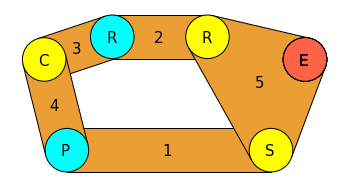}}{{\tiny 2D-M174}}
\qquad\subsubfloat{\includegraphics[width=0.05\textwidth]{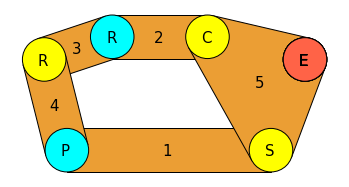}}{{\tiny 2D-M175}}
\qquad\subsubfloat{\includegraphics[width=0.05\textwidth]{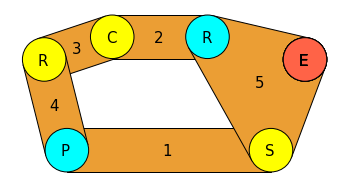}}{{\tiny 2D-M176}}
\qquad\subsubfloat{\includegraphics[width=0.05\textwidth]{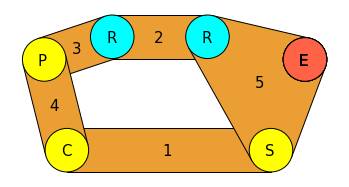}}{{\tiny 2D-M177}}
\qquad\subsubfloat{\includegraphics[width=0.05\textwidth]{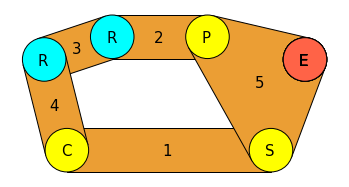}}{{\tiny 2D-M178}}
\qquad\subsubfloat{\includegraphics[width=0.05\textwidth]{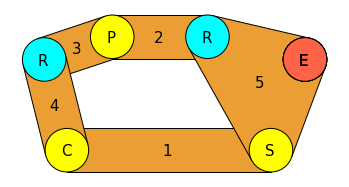}}{{\tiny 2D-M179}}
\qquad\subsubfloat{\includegraphics[width=0.05\textwidth]{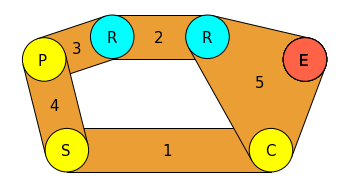}}{{\tiny 2D-M180}}
\qquad\subsubfloat{\includegraphics[width=0.05\textwidth]{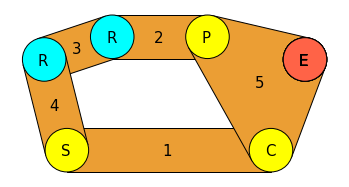}}{{\tiny 2D-M181}}
\qquad\subsubfloat{\includegraphics[width=0.05\textwidth]{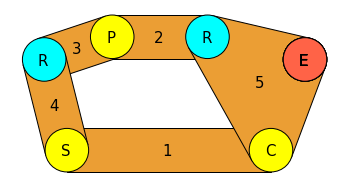}}{{\tiny 2D-M182}}
\qquad\subsubfloat{\includegraphics[width=0.05\textwidth]{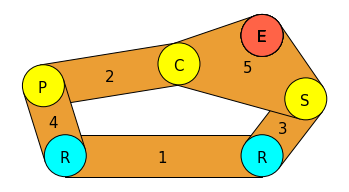}}{{\tiny 2D-M183}}
\qquad\subsubfloat{\includegraphics[width=0.05\textwidth]{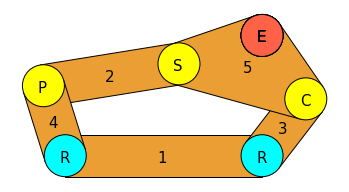}}{{\tiny 2D-M184}}
\qquad\subsubfloat{\includegraphics[width=0.05\textwidth]{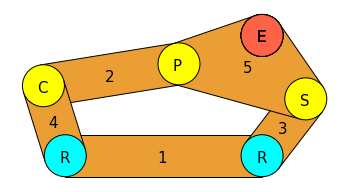}}{{\tiny 2D-M185}}
\qquad\subsubfloat{\includegraphics[width=0.05\textwidth]{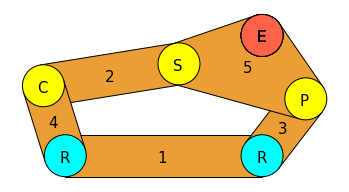}}{{\tiny 2D-M186}}
\qquad\subsubfloat{\includegraphics[width=0.05\textwidth]{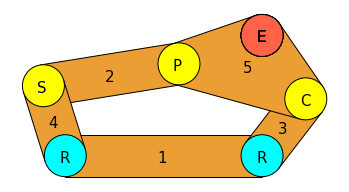}}{{\tiny 2D-M187}}
\qquad\subsubfloat{\includegraphics[width=0.05\textwidth]{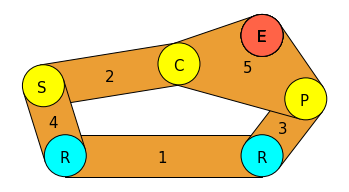}}{{\tiny 2D-M188}}
\qquad\subsubfloat{\includegraphics[width=0.05\textwidth]{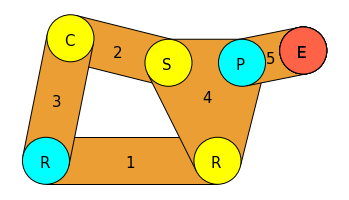}}{{\tiny 2D-M189}}
\qquad\subsubfloat{\includegraphics[width=0.05\textwidth]{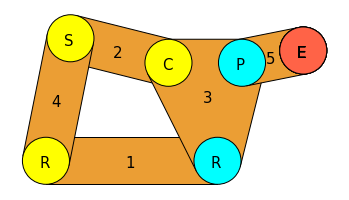}}{{\tiny 2D-M190}}
\qquad\subsubfloat{\includegraphics[width=0.05\textwidth]{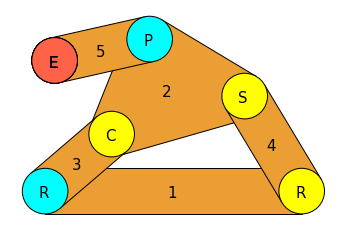}}{{\tiny 2D-M191}}
\qquad\subsubfloat{\includegraphics[width=0.05\textwidth]{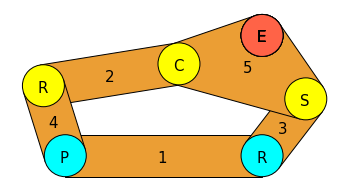}}{{\tiny 2D-M192}}
\qquad\subsubfloat{\includegraphics[width=0.05\textwidth]{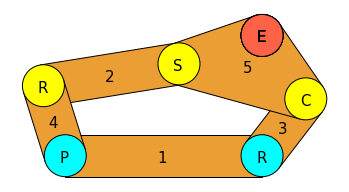}}{{\tiny 2D-M193}}
\qquad\subsubfloat{\includegraphics[width=0.05\textwidth]{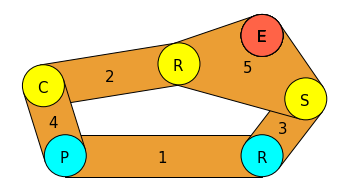}}{{\tiny 2D-M194}}
\qquad\subsubfloat{\includegraphics[width=0.05\textwidth]{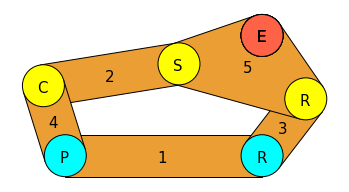}}{{\tiny 2D-M195}}
\qquad\subsubfloat{\includegraphics[width=0.05\textwidth]{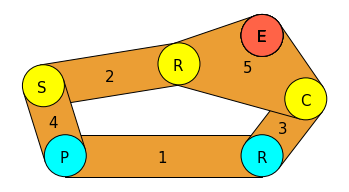}}{{\tiny 2D-M196}}
\qquad\subsubfloat{\includegraphics[width=0.05\textwidth]{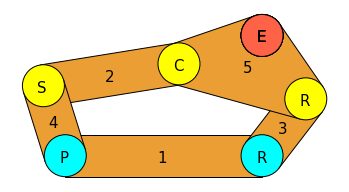}}{{\tiny 2D-M197}}
\qquad\subsubfloat{\includegraphics[width=0.05\textwidth]{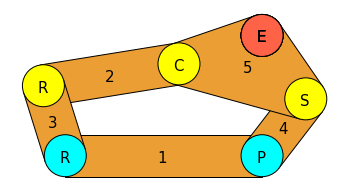}}{{\tiny 2D-M198}}
\qquad\subsubfloat{\includegraphics[width=0.05\textwidth]{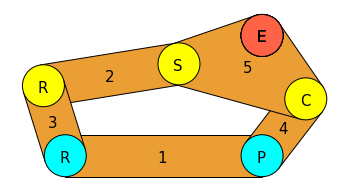}}{{\tiny 2D-M199}}
\qquad\subsubfloat{\includegraphics[width=0.05\textwidth]{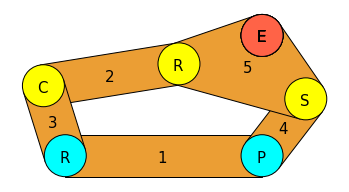}}{{\tiny 2D-M200}}
\qquad\subsubfloat{\includegraphics[width=0.05\textwidth]{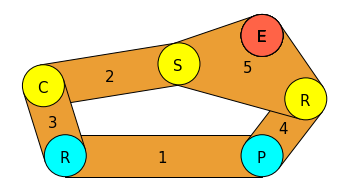}}{{\tiny 2D-M201}}
\qquad\subsubfloat{\includegraphics[width=0.05\textwidth]{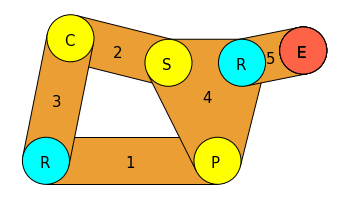}}{{\tiny 2D-M202}}
\qquad\subsubfloat{\includegraphics[width=0.05\textwidth]{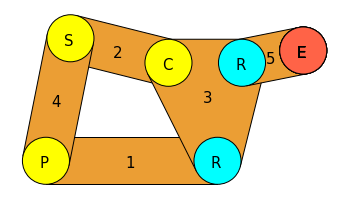}}{{\tiny 2D-M203}}
\qquad\subsubfloat{\includegraphics[width=0.05\textwidth]{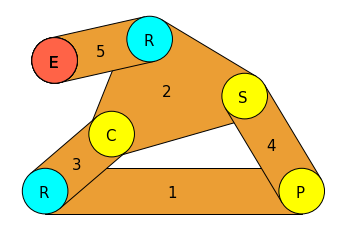}}{{\tiny 2D-M204}}
\qquad\subsubfloat{\includegraphics[width=0.05\textwidth]{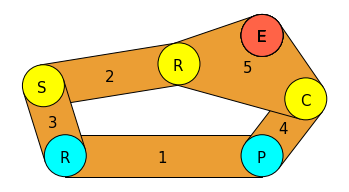}}{{\tiny 2D-M205}}
\qquad\subsubfloat{\includegraphics[width=0.05\textwidth]{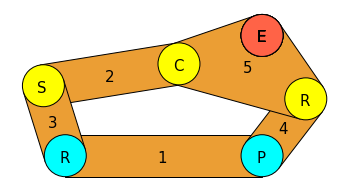}}{{\tiny 2D-M206}}
\qquad\subsubfloat{\includegraphics[width=0.05\textwidth]{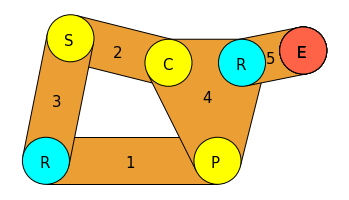}}{{\tiny 2D-M207}}
\qquad\subsubfloat{\includegraphics[width=0.05\textwidth]{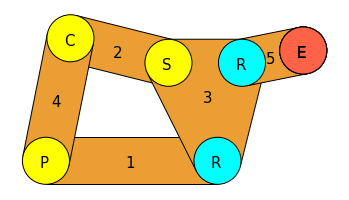}}{{\tiny 2D-M208}}
\qquad\subsubfloat{\includegraphics[width=0.05\textwidth]{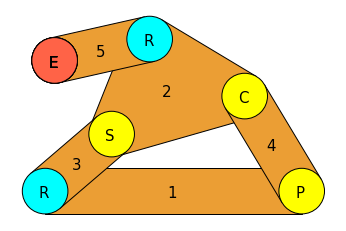}}{{\tiny 2D-M209}}
\qquad\subsubfloat{\includegraphics[width=0.05\textwidth]{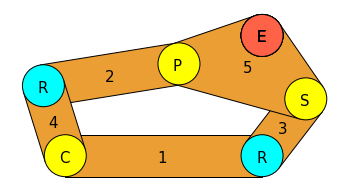}}{{\tiny 2D-M210}}
\qquad\subsubfloat{\includegraphics[width=0.05\textwidth]{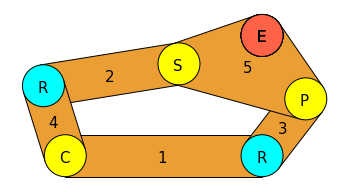}}{{\tiny 2D-M211}}
\qquad\subsubfloat{\includegraphics[width=0.05\textwidth]{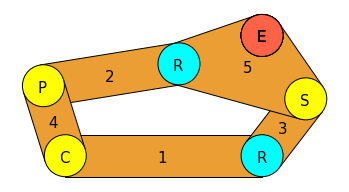}}{{\tiny 2D-M212}}
\qquad\subsubfloat{\includegraphics[width=0.05\textwidth]{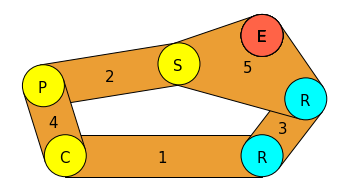}}{{\tiny 2D-M213}}
\qquad\subsubfloat{\includegraphics[width=0.05\textwidth]{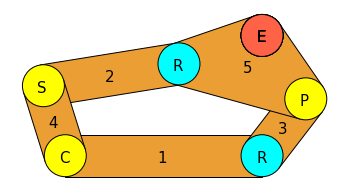}}{{\tiny 2D-M214}}
\qquad\subsubfloat{\includegraphics[width=0.05\textwidth]{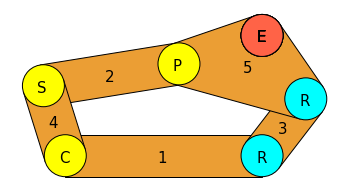}}{{\tiny 2D-M215}}
\qquad\subsubfloat{\includegraphics[width=0.05\textwidth]{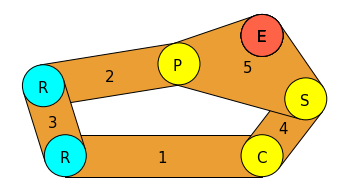}}{{\tiny 2D-M216}}
\qquad\subsubfloat{\includegraphics[width=0.05\textwidth]{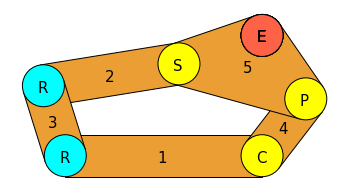}}{{\tiny 2D-M217}}
\qquad\subsubfloat{\includegraphics[width=0.05\textwidth]{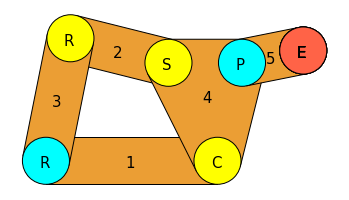}}{{\tiny 2D-M218}}
\qquad\subsubfloat{\includegraphics[width=0.05\textwidth]{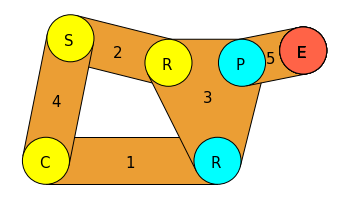}}{{\tiny 2D-M219}}
\qquad\subsubfloat{\includegraphics[width=0.05\textwidth]{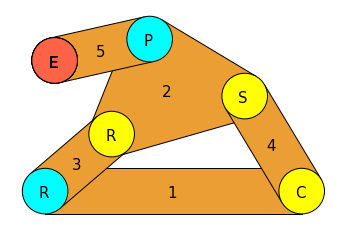}}{{\tiny 2D-M220}}
\qquad\subsubfloat{\includegraphics[width=0.05\textwidth]{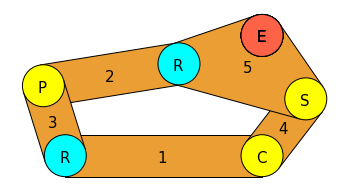}}{{\tiny 2D-M221}}
\qquad\subsubfloat{\includegraphics[width=0.05\textwidth]{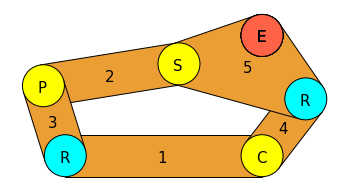}}{{\tiny 2D-M222}}
\qquad\subsubfloat{\includegraphics[width=0.05\textwidth]{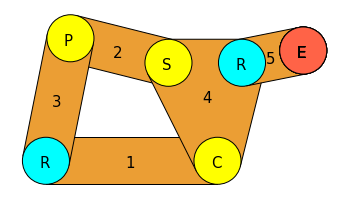}}{{\tiny 2D-M223}}
\qquad\subsubfloat{\includegraphics[width=0.05\textwidth]{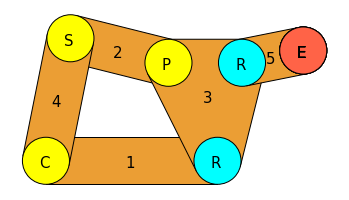}}{{\tiny 2D-M224}}
\qquad\subsubfloat{\includegraphics[width=0.05\textwidth]{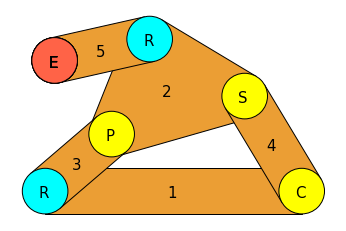}}{{\tiny 2D-M225}}
\qquad\subsubfloat{\includegraphics[width=0.05\textwidth]{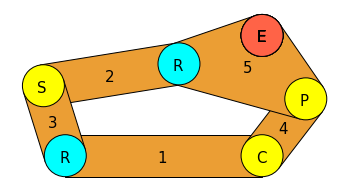}}{{\tiny 2D-M226}}
\qquad\subsubfloat{\includegraphics[width=0.05\textwidth]{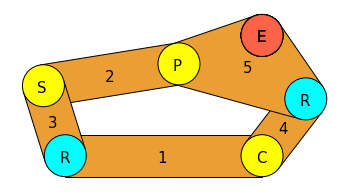}}{{\tiny 2D-M227}}
\qquad\subsubfloat{\includegraphics[width=0.05\textwidth]{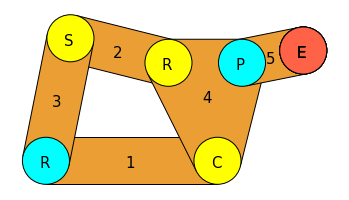}}{{\tiny 2D-M228}}
\qquad\subsubfloat{\includegraphics[width=0.05\textwidth]{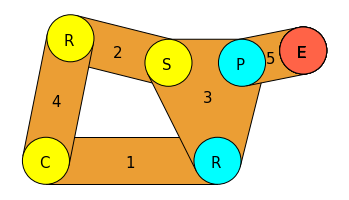}}{{\tiny 2D-M229}}
\qquad\subsubfloat{\includegraphics[width=0.05\textwidth]{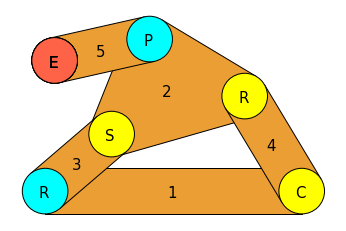}}{{\tiny 2D-M230}}
\qquad\subsubfloat{\includegraphics[width=0.05\textwidth]{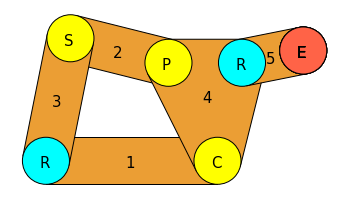}}{{\tiny 2D-M231}}
\qquad\subsubfloat{\includegraphics[width=0.05\textwidth]{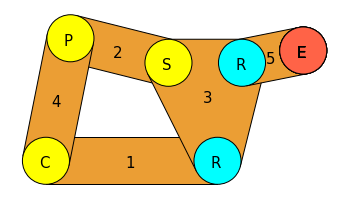}}{{\tiny 2D-M232}}
\qquad\subsubfloat{\includegraphics[width=0.05\textwidth]{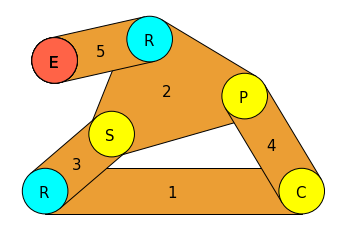}}{{\tiny 2D-M233}}
\qquad\subsubfloat{\includegraphics[width=0.05\textwidth]{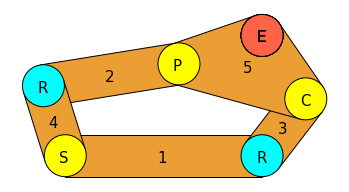}}{{\tiny 2D-M234}}
\qquad\subsubfloat{\includegraphics[width=0.05\textwidth]{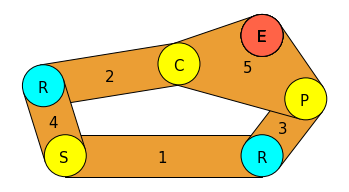}}{{\tiny 2D-M235}}
\qquad\subsubfloat{\includegraphics[width=0.05\textwidth]{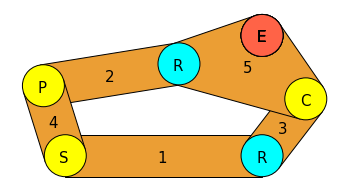}}{{\tiny 2D-M236}}
\qquad\subsubfloat{\includegraphics[width=0.05\textwidth]{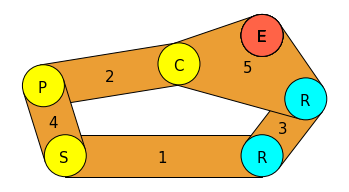}}{{\tiny 2D-M237}}
\qquad\subsubfloat{\includegraphics[width=0.05\textwidth]{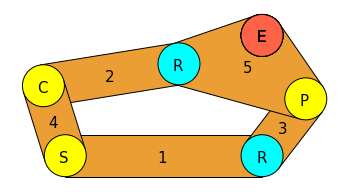}}{{\tiny 2D-M238}}
\qquad\subsubfloat{\includegraphics[width=0.05\textwidth]{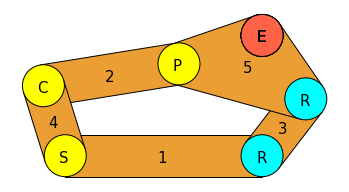}}{{\tiny 2D-M239}}
\qquad\subsubfloat{\includegraphics[width=0.05\textwidth]{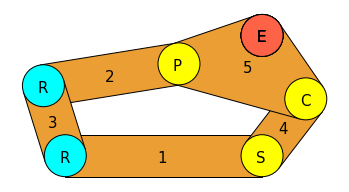}}{{\tiny 2D-M240}}
\qquad\subsubfloat{\includegraphics[width=0.05\textwidth]{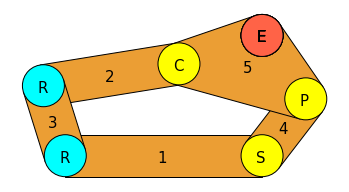}}{{\tiny 2D-M241}}
\qquad\subsubfloat{\includegraphics[width=0.05\textwidth]{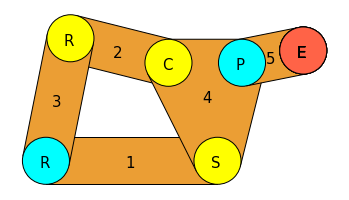}}{{\tiny 2D-M242}}
\qquad\subsubfloat{\includegraphics[width=0.05\textwidth]{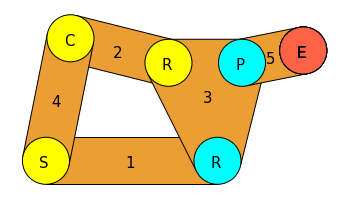}}{{\tiny 2D-M243}}
\qquad\subsubfloat{\includegraphics[width=0.05\textwidth]{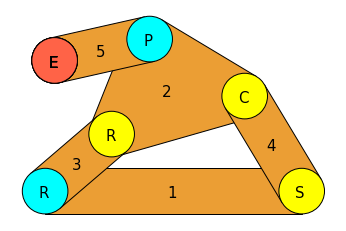}}{{\tiny 2D-M244}}
\qquad\subsubfloat{\includegraphics[width=0.05\textwidth]{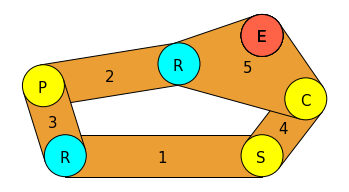}}{{\tiny 2D-M245}}
\qquad\subsubfloat{\includegraphics[width=0.05\textwidth]{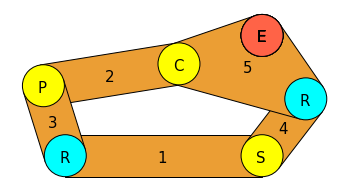}}{{\tiny 2D-M246}}
\qquad\subsubfloat{\includegraphics[width=0.05\textwidth]{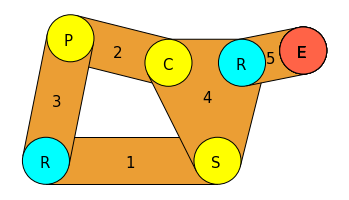}}{{\tiny 2D-M247}}
\qquad\subsubfloat{\includegraphics[width=0.05\textwidth]{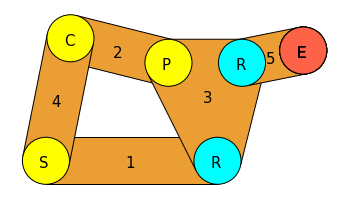}}{{\tiny 2D-M248}}
\qquad\subsubfloat{\includegraphics[width=0.05\textwidth]{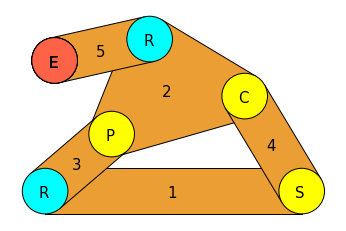}}{{\tiny 2D-M249}}
\qquad\subsubfloat{\includegraphics[width=0.05\textwidth]{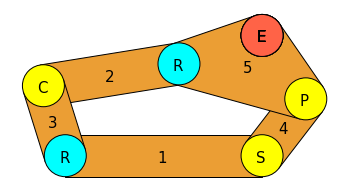}}{{\tiny 2D-M250}}
\qquad\subsubfloat{\includegraphics[width=0.05\textwidth]{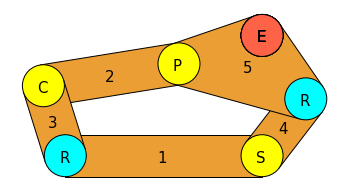}}{{\tiny 2D-M251}}
\qquad\subsubfloat{\includegraphics[width=0.05\textwidth]{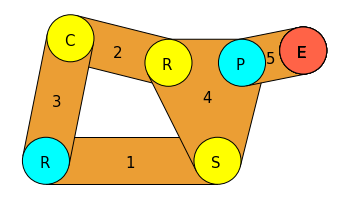}}{{\tiny 2D-M252}}
\qquad\subsubfloat{\includegraphics[width=0.05\textwidth]{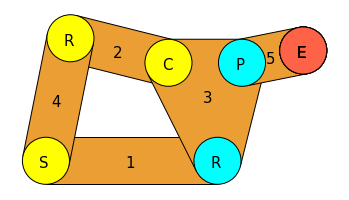}}{{\tiny 2D-M253}}
\qquad\subsubfloat{\includegraphics[width=0.05\textwidth]{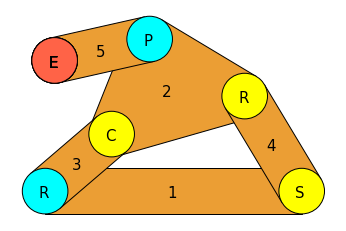}}{{\tiny 2D-M254}}
\qquad\subsubfloat{\includegraphics[width=0.05\textwidth]{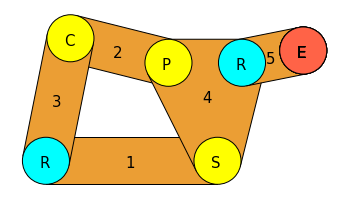}}{{\tiny 2D-M255}}
\qquad\subsubfloat{\includegraphics[width=0.05\textwidth]{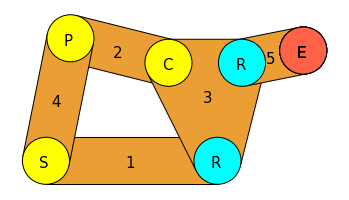}}{{\tiny 2D-M256}}
\qquad\subsubfloat{\includegraphics[width=0.05\textwidth]{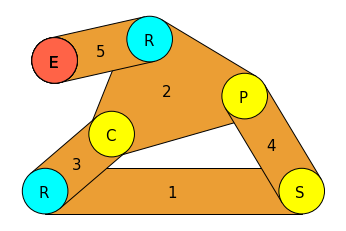}}{{\tiny 2D-M257}}
\qquad\subsubfloat{\includegraphics[width=0.05\textwidth]{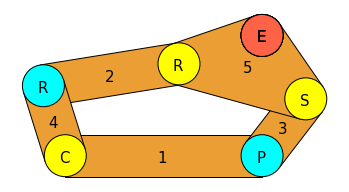}}{{\tiny 2D-M258}}
\qquad\subsubfloat{\includegraphics[width=0.05\textwidth]{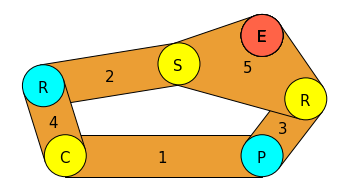}}{{\tiny 2D-M259}}
\qquad\subsubfloat{\includegraphics[width=0.05\textwidth]{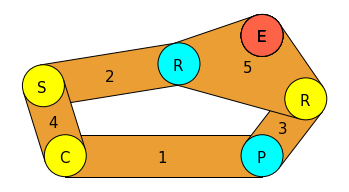}}{{\tiny 2D-M260}}
\qquad\subsubfloat{\includegraphics[width=0.05\textwidth]{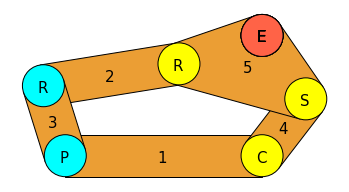}}{{\tiny 2D-M261}}
\qquad\subsubfloat{\includegraphics[width=0.05\textwidth]{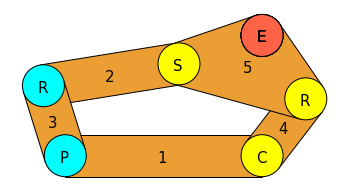}}{{\tiny 2D-M262}}
\qquad\subsubfloat{\includegraphics[width=0.05\textwidth]{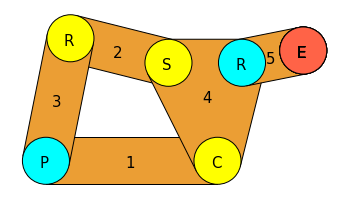}}{{\tiny 2D-M263}}
\qquad\subsubfloat{\includegraphics[width=0.05\textwidth]{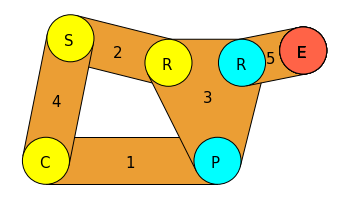}}{{\tiny 2D-M264}}

  \end{minipage}
\end{subfigure}
\caption{Schematic diagrams of 2-DOF Manipulators}
\end{figure}

  \begin{figure}[H]\ContinuedFloat
    \centering
    \begin{subfigure}{\columnwidth}
      \begin{minipage}{\textwidth}\footnotesize
      \centering
\subsubfloat{\includegraphics[width=0.05\textwidth]{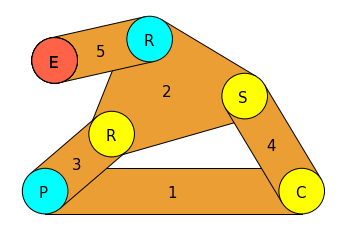}}{{\tiny 2D-M265}}
\qquad\subsubfloat{\includegraphics[width=0.05\textwidth]{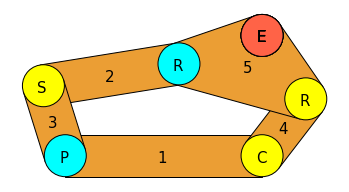}}{{\tiny 2D-M266}}
\qquad\subsubfloat{\includegraphics[width=0.05\textwidth]{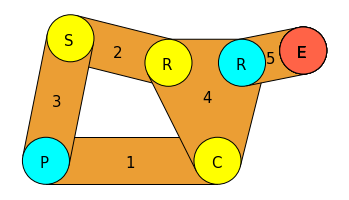}}{{\tiny 2D-M267}}
\qquad\subsubfloat{\includegraphics[width=0.05\textwidth]{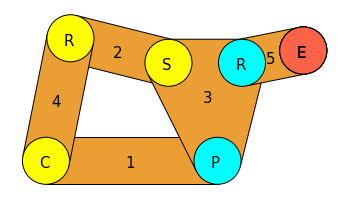}}{{\tiny 2D-M268}}
\qquad\subsubfloat{\includegraphics[width=0.05\textwidth]{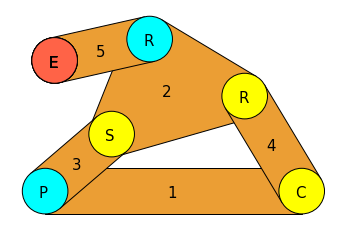}}{{\tiny 2D-M269}}
\qquad\subsubfloat{\includegraphics[width=0.05\textwidth]{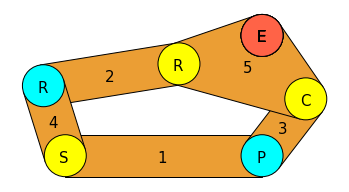}}{{\tiny 2D-M270}}
\qquad\subsubfloat{\includegraphics[width=0.05\textwidth]{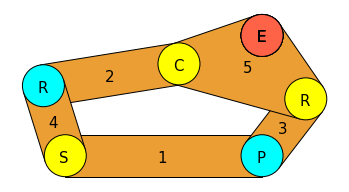}}{{\tiny 2D-M271}}
\qquad\subsubfloat{\includegraphics[width=0.05\textwidth]{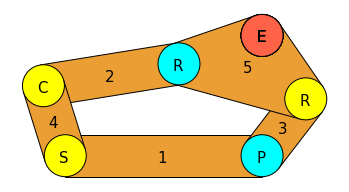}}{{\tiny 2D-M272}}
\qquad\subsubfloat{\includegraphics[width=0.05\textwidth]{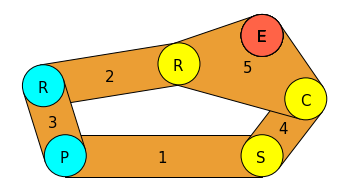}}{{\tiny 2D-M273}}
\qquad\subsubfloat{\includegraphics[width=0.05\textwidth]{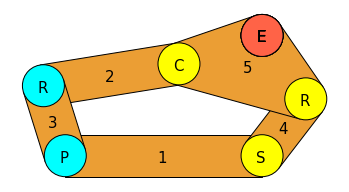}}{{\tiny 2D-M274}}
\qquad\subsubfloat{\includegraphics[width=0.05\textwidth]{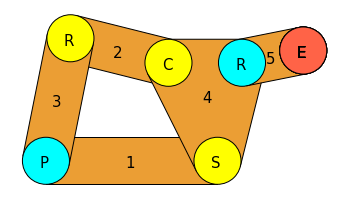}}{{\tiny 2D-M275}}
\qquad\subsubfloat{\includegraphics[width=0.05\textwidth]{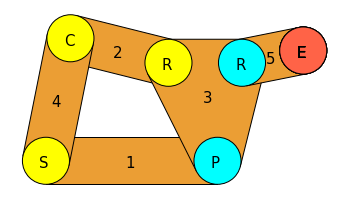}}{{\tiny 2D-M276}}
\qquad\subsubfloat{\includegraphics[width=0.05\textwidth]{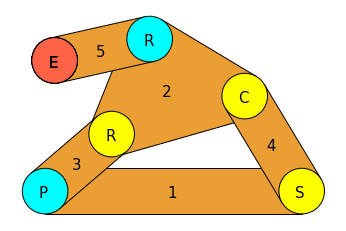}}{{\tiny 2D-M277}}
\qquad\subsubfloat{\includegraphics[width=0.05\textwidth]{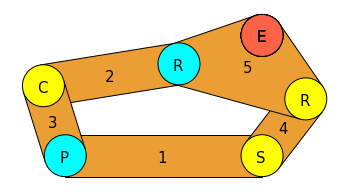}}{{\tiny 2D-M278}}
\qquad\subsubfloat{\includegraphics[width=0.05\textwidth]{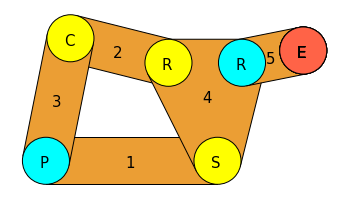}}{{\tiny 2D-M279}}
\qquad\subsubfloat{\includegraphics[width=0.05\textwidth]{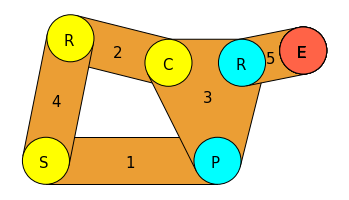}}{{\tiny 2D-M280}}
\qquad\subsubfloat{\includegraphics[width=0.05\textwidth]{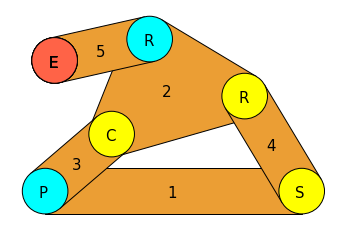}}{{\tiny 2D-M281}}
\qquad\subsubfloat{\includegraphics[width=0.05\textwidth]{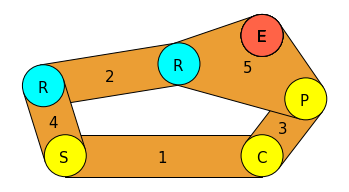}}{{\tiny 2D-M282}}
\qquad\subsubfloat{\includegraphics[width=0.05\textwidth]{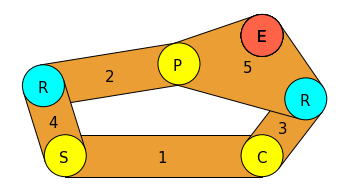}}{{\tiny 2D-M283}}
\qquad\subsubfloat{\includegraphics[width=0.05\textwidth]{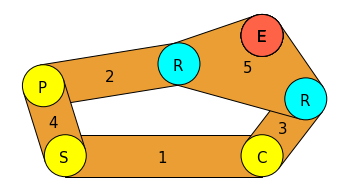}}{{\tiny 2D-M284}}
\qquad\subsubfloat{\includegraphics[width=0.05\textwidth]{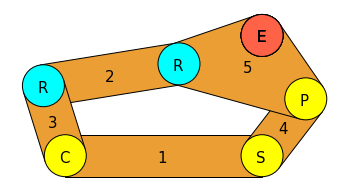}}{{\tiny 2D-M285}}
\qquad\subsubfloat{\includegraphics[width=0.05\textwidth]{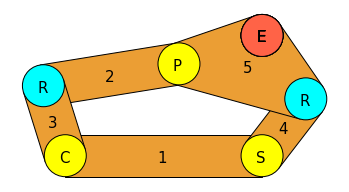}}{{\tiny 2D-M286}}
\qquad\subsubfloat{\includegraphics[width=0.05\textwidth]{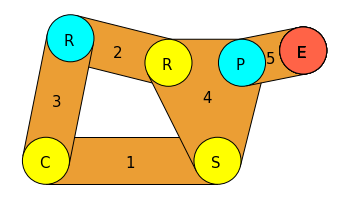}}{{\tiny 2D-M287}}
\qquad\subsubfloat{\includegraphics[width=0.05\textwidth]{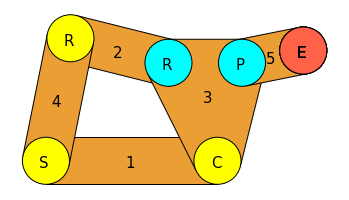}}{{\tiny 2D-M288}}
\qquad\subsubfloat{\includegraphics[width=0.05\textwidth]{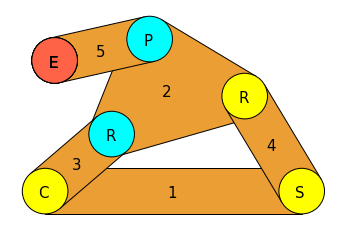}}{{\tiny 2D-M289}}
\qquad\subsubfloat{\includegraphics[width=0.05\textwidth]{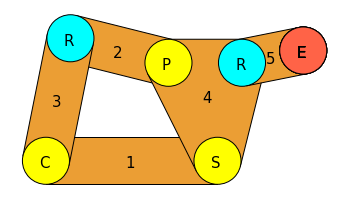}}{{\tiny 2D-M290}}
\qquad\subsubfloat{\includegraphics[width=0.05\textwidth]{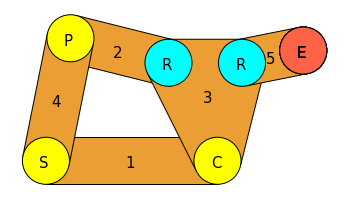}}{{\tiny 2D-M291}}
\qquad\subsubfloat{\includegraphics[width=0.05\textwidth]{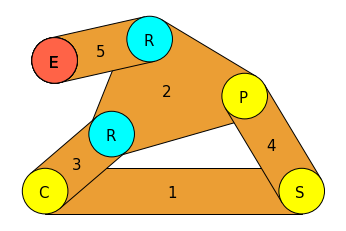}}{{\tiny 2D-M292}}
\qquad\subsubfloat{\includegraphics[width=0.05\textwidth]{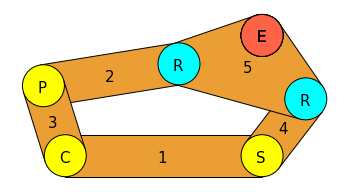}}{{\tiny 2D-M293}}
\qquad\subsubfloat{\includegraphics[width=0.05\textwidth]{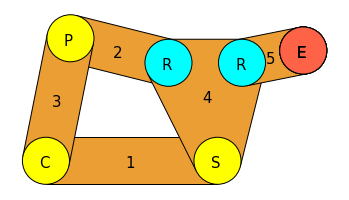}}{{\tiny 2D-M294}}
\qquad\subsubfloat{\includegraphics[width=0.05\textwidth]{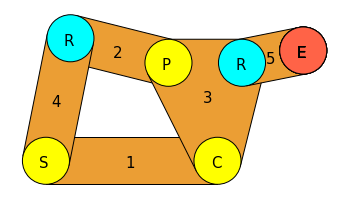}}{{\tiny 2D-M295}}
\qquad\subsubfloat{\includegraphics[width=0.05\textwidth]{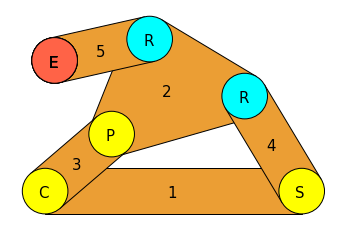}}{{\tiny 2D-M296}}
\qquad\subsubfloat{\includegraphics[width=0.05\textwidth]{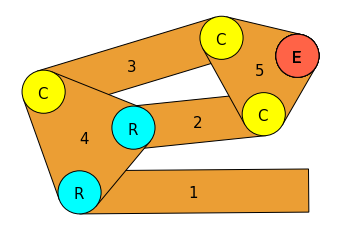}}{{\tiny 2D-M297}}
\qquad\subsubfloat{\includegraphics[width=0.05\textwidth]{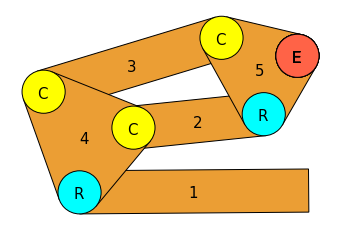}}{{\tiny 2D-M298}}
\qquad\subsubfloat{\includegraphics[width=0.05\textwidth]{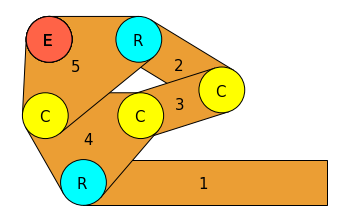}}{{\tiny 2D-M299}}
\qquad\subsubfloat{\includegraphics[width=0.05\textwidth]{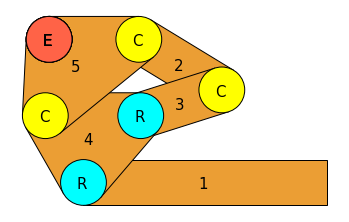}}{{\tiny 2D-M300}}
\qquad\subsubfloat{\includegraphics[width=0.05\textwidth]{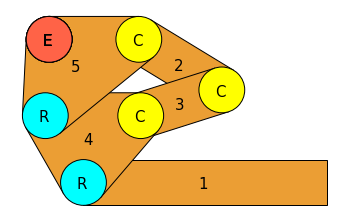}}{{\tiny 2D-M301}}
\qquad\subsubfloat{\includegraphics[width=0.05\textwidth]{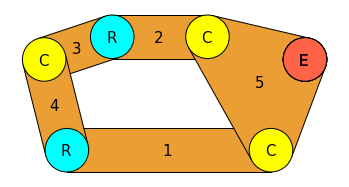}}{{\tiny 2D-M302}}
\qquad\subsubfloat{\includegraphics[width=0.05\textwidth]{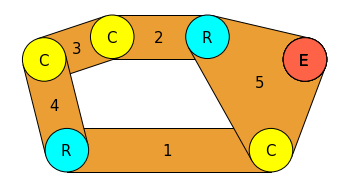}}{{\tiny 2D-M303}}
\qquad\subsubfloat{\includegraphics[width=0.05\textwidth]{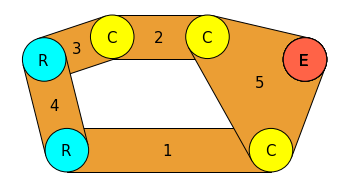}}{{\tiny 2D-M304}}
\qquad\subsubfloat{\includegraphics[width=0.05\textwidth]{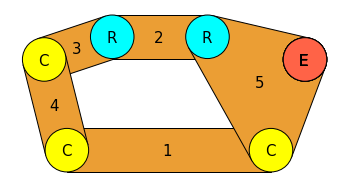}}{{\tiny 2D-M305}}
\qquad\subsubfloat{\includegraphics[width=0.05\textwidth]{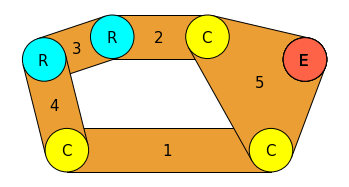}}{{\tiny 2D-M306}}
\qquad\subsubfloat{\includegraphics[width=0.05\textwidth]{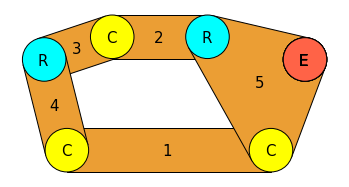}}{{\tiny 2D-M307}}
\qquad\subsubfloat{\includegraphics[width=0.05\textwidth]{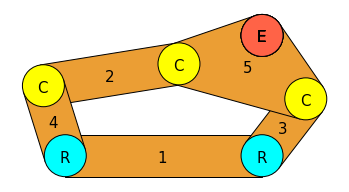}}{{\tiny 2D-M308}}
\qquad\subsubfloat{\includegraphics[width=0.05\textwidth]{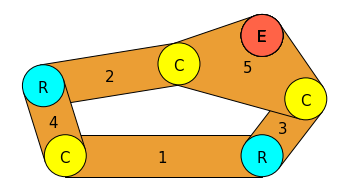}}{{\tiny 2D-M309}}
\qquad\subsubfloat{\includegraphics[width=0.05\textwidth]{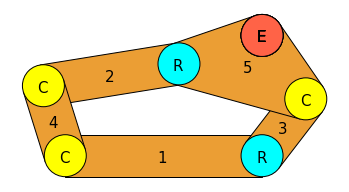}}{{\tiny 2D-M310}}
\qquad\subsubfloat{\includegraphics[width=0.05\textwidth]{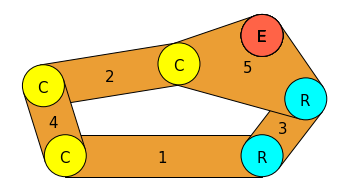}}{{\tiny 2D-M311}}
\qquad\subsubfloat{\includegraphics[width=0.05\textwidth]{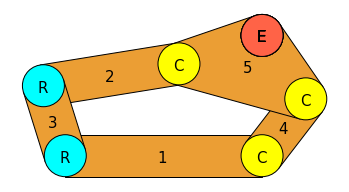}}{{\tiny 2D-M312}}
\qquad\subsubfloat{\includegraphics[width=0.05\textwidth]{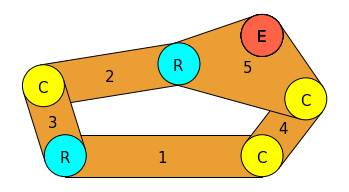}}{{\tiny 2D-M313}}
\qquad\subsubfloat{\includegraphics[width=0.05\textwidth]{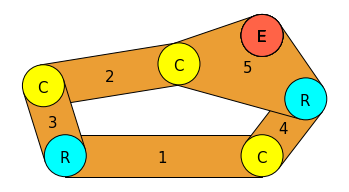}}{{\tiny 2D-M314}}
\qquad\subsubfloat{\includegraphics[width=0.05\textwidth]{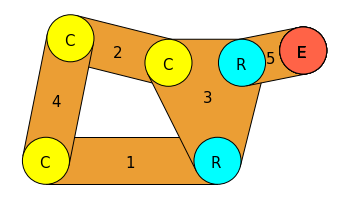}}{{\tiny 2D-M315}}
\qquad\subsubfloat{\includegraphics[width=0.05\textwidth]{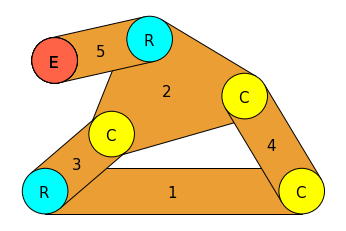}}{{\tiny 2D-M316}}
\qquad\subsubfloat{\includegraphics[width=0.05\textwidth]{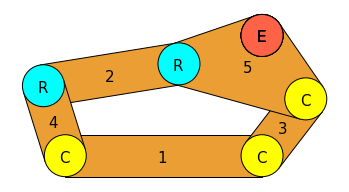}}{{\tiny 2D-M317}}
\qquad\subsubfloat{\includegraphics[width=0.05\textwidth]{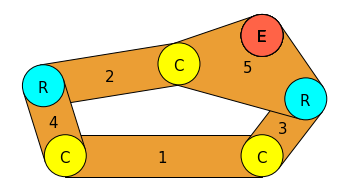}}{{\tiny 2D-M318}}
\qquad\subsubfloat{\includegraphics[width=0.05\textwidth]{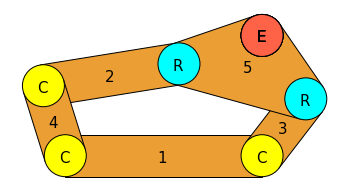}}{{\tiny 2D-M319}}
\qquad\subsubfloat{\includegraphics[width=0.05\textwidth]{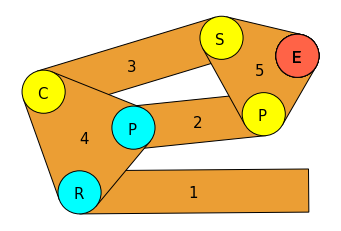}}{{\tiny 2D-M320}}
\qquad\subsubfloat{\includegraphics[width=0.05\textwidth]{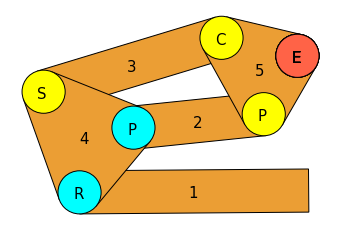}}{{\tiny 2D-M321}}
\qquad\subsubfloat{\includegraphics[width=0.05\textwidth]{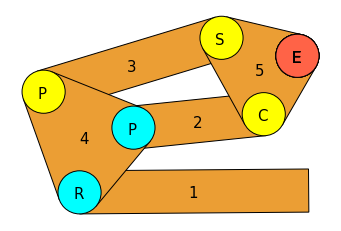}}{{\tiny 2D-M322}}
\qquad\subsubfloat{\includegraphics[width=0.05\textwidth]{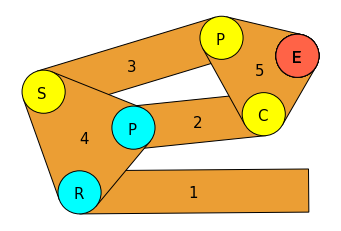}}{{\tiny 2D-M323}}
\qquad\subsubfloat{\includegraphics[width=0.05\textwidth]{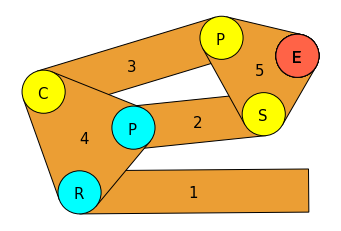}}{{\tiny 2D-M324}}
\qquad\subsubfloat{\includegraphics[width=0.05\textwidth]{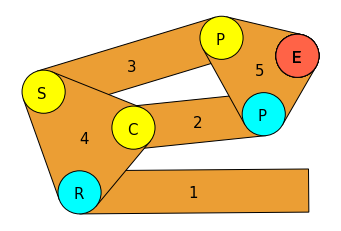}}{{\tiny 2D-M325}}
\qquad\subsubfloat{\includegraphics[width=0.05\textwidth]{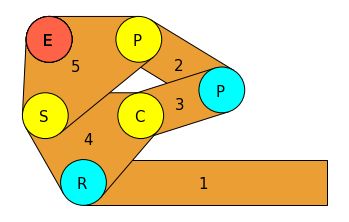}}{{\tiny 2D-M326}}
\qquad\subsubfloat{\includegraphics[width=0.05\textwidth]{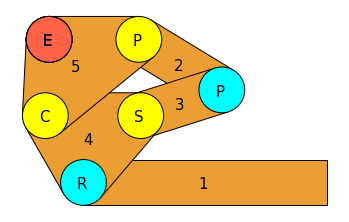}}{{\tiny 2D-M327}}
\qquad\subsubfloat{\includegraphics[width=0.05\textwidth]{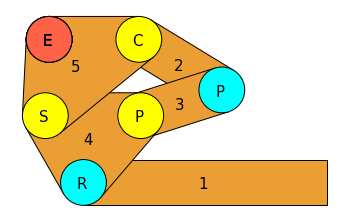}}{{\tiny 2D-M328}}
\qquad\subsubfloat{\includegraphics[width=0.05\textwidth]{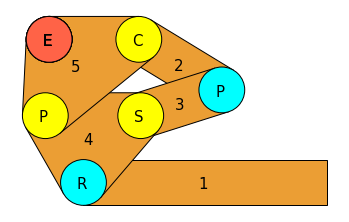}}{{\tiny 2D-M329}}
\qquad\subsubfloat{\includegraphics[width=0.05\textwidth]{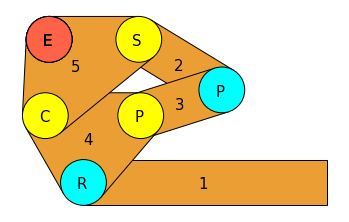}}{{\tiny 2D-M330}}
\qquad\subsubfloat{\includegraphics[width=0.05\textwidth]{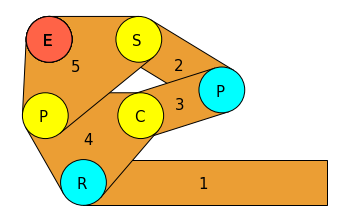}}{{\tiny 2D-M331}}
\qquad\subsubfloat{\includegraphics[width=0.05\textwidth]{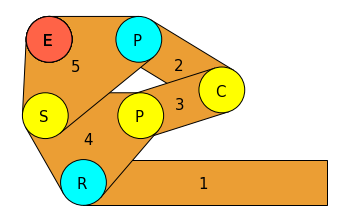}}{{\tiny 2D-M332}}
\qquad\subsubfloat{\includegraphics[width=0.05\textwidth]{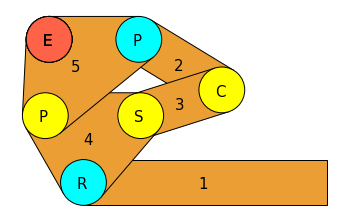}}{{\tiny 2D-M333}}
\qquad\subsubfloat{\includegraphics[width=0.05\textwidth]{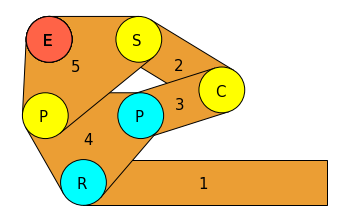}}{{\tiny 2D-M334}}
\qquad\subsubfloat{\includegraphics[width=0.05\textwidth]{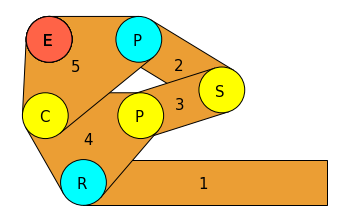}}{{\tiny 2D-M335}}
\qquad\subsubfloat{\includegraphics[width=0.05\textwidth]{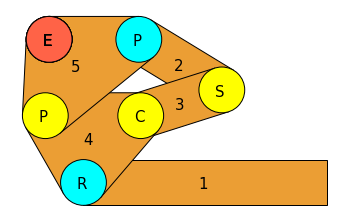}}{{\tiny 2D-M336}}
\qquad\subsubfloat{\includegraphics[width=0.05\textwidth]{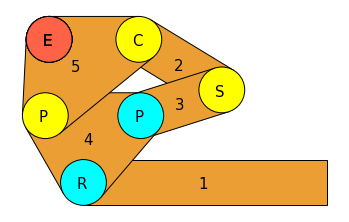}}{{\tiny 2D-M337}}
\qquad\subsubfloat{\includegraphics[width=0.05\textwidth]{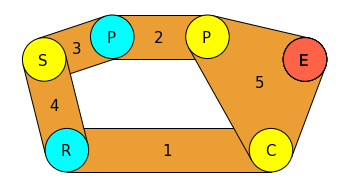}}{{\tiny 2D-M338}}
\qquad\subsubfloat{\includegraphics[width=0.05\textwidth]{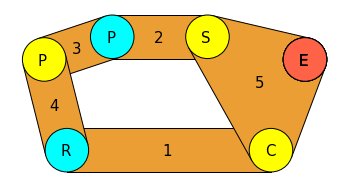}}{{\tiny 2D-M339}}
\qquad\subsubfloat{\includegraphics[width=0.05\textwidth]{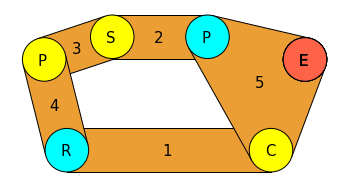}}{{\tiny 2D-M340}}
\qquad\subsubfloat{\includegraphics[width=0.05\textwidth]{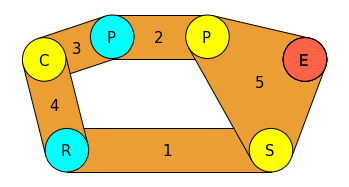}}{{\tiny 2D-M341}}
\qquad\subsubfloat{\includegraphics[width=0.05\textwidth]{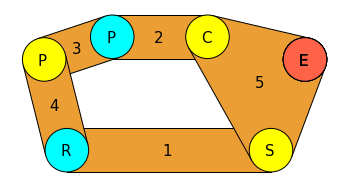}}{{\tiny 2D-M342}}
\qquad\subsubfloat{\includegraphics[width=0.05\textwidth]{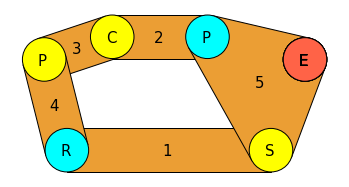}}{{\tiny 2D-M343}}
\qquad\subsubfloat{\includegraphics[width=0.05\textwidth]{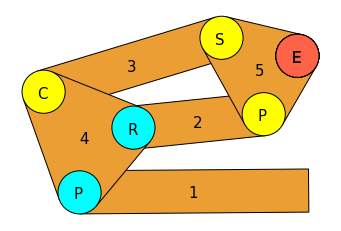}}{{\tiny 2D-M344}}
\qquad\subsubfloat{\includegraphics[width=0.05\textwidth]{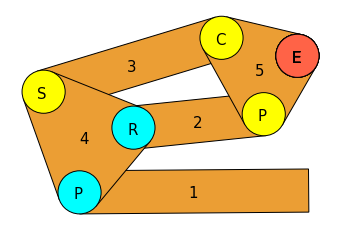}}{{\tiny 2D-M345}}
\qquad\subsubfloat{\includegraphics[width=0.05\textwidth]{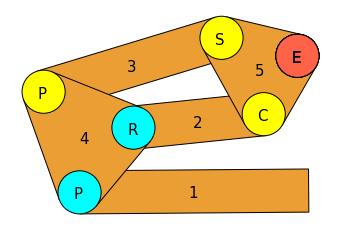}}{{\tiny 2D-M346}}
\qquad\subsubfloat{\includegraphics[width=0.05\textwidth]{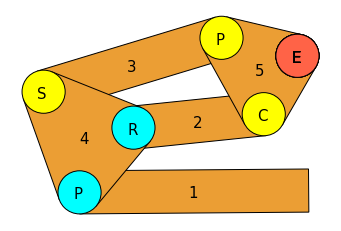}}{{\tiny 2D-M347}}
\qquad\subsubfloat{\includegraphics[width=0.05\textwidth]{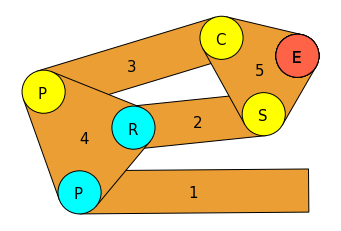}}{{\tiny 2D-M348}}
\qquad\subsubfloat{\includegraphics[width=0.05\textwidth]{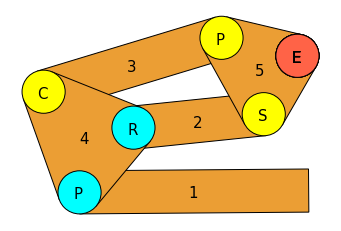}}{{\tiny 2D-M349}}
\qquad  \subsubfloat{\includegraphics[width=0.05\textwidth]{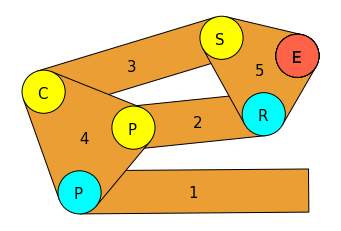}}{{\tiny 2D-M350}}
\qquad\subsubfloat{\includegraphics[width=0.05\textwidth]{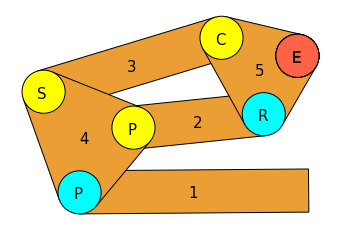}}{{\tiny 2D-M351}}
\qquad\subsubfloat{\includegraphics[width=0.05\textwidth]{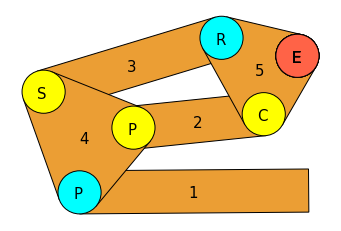}}{{\tiny 2D-M352}}
\qquad\subsubfloat{\includegraphics[width=0.05\textwidth]{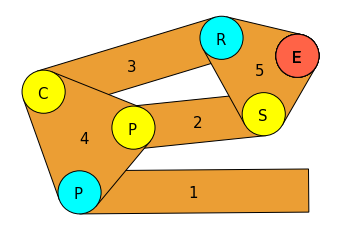}}{{\tiny 2D-M353}}
\qquad\subsubfloat{\includegraphics[width=0.05\textwidth]{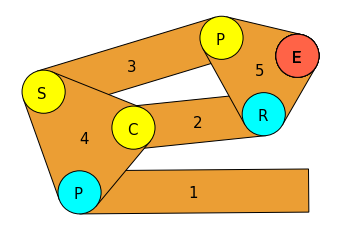}}{{\tiny 2D-M354}}
\qquad\subsubfloat{\includegraphics[width=0.05\textwidth]{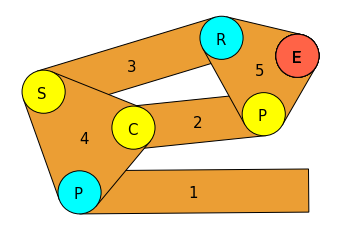}}{{\tiny 2D-M355}}  
\qquad\subsubfloat{\includegraphics[width=0.05\textwidth]{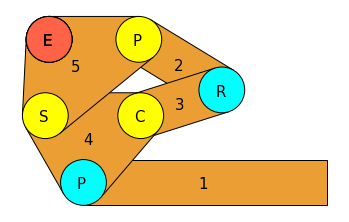}}{{\tiny 2D-M356}}
\qquad\subsubfloat{\includegraphics[width=0.05\textwidth]{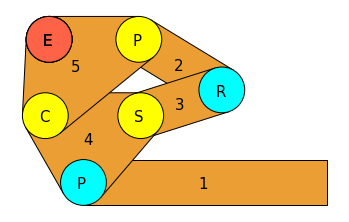}}{{\tiny 2D-M357}}
\qquad\subsubfloat{\includegraphics[width=0.05\textwidth]{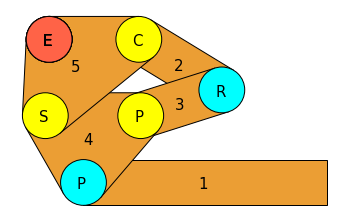}}{{\tiny 2D-M358}}
\qquad\subsubfloat{\includegraphics[width=0.05\textwidth]{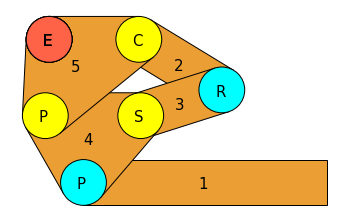}}{{\tiny 2D-M359}}
\qquad\subsubfloat{\includegraphics[width=0.05\textwidth]{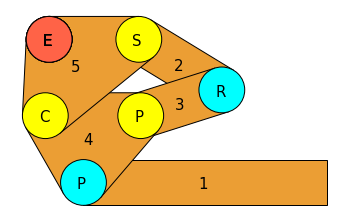}}{{\tiny 2D-M360}}
\qquad\subsubfloat{\includegraphics[width=0.05\textwidth]{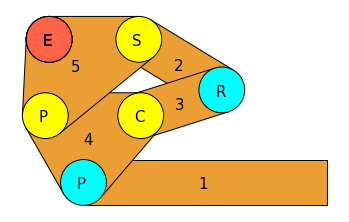}}{{\tiny 2D-M361}}
\qquad\subsubfloat{\includegraphics[width=0.05\textwidth]{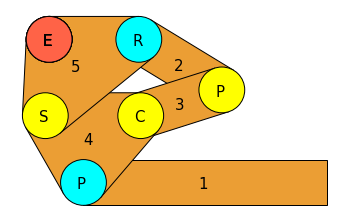}}{{\tiny 2D-M362}}
\qquad\subsubfloat{\includegraphics[width=0.05\textwidth]{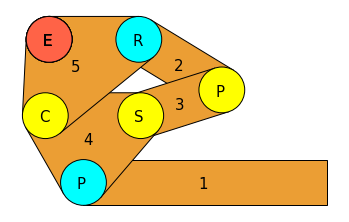}}{{\tiny 2D-M363}}
\qquad\subsubfloat{\includegraphics[width=0.05\textwidth]{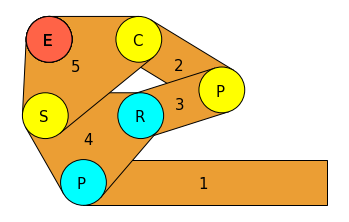}}{{\tiny 2D-M364}}
\qquad\subsubfloat{\includegraphics[width=0.05\textwidth]{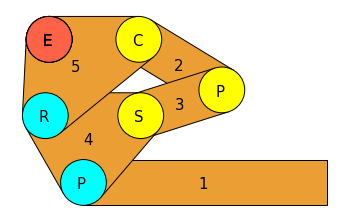}}{{\tiny 2D-M365}}
\qquad\subsubfloat{\includegraphics[width=0.05\textwidth]{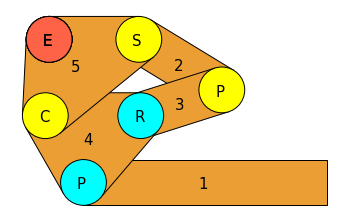}}{{\tiny 2D-M366}}
\qquad\subsubfloat{\includegraphics[width=0.05\textwidth]{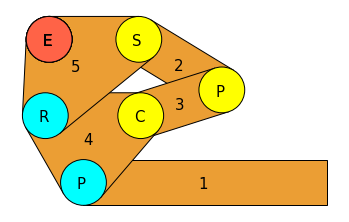}}{{\tiny 2D-M367}}
\qquad\subsubfloat{\includegraphics[width=0.05\textwidth]{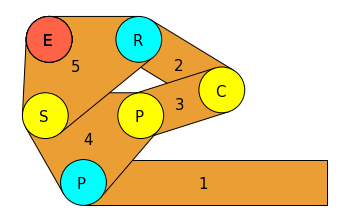}}{{\tiny 2D-M368}}
\qquad\subsubfloat{\includegraphics[width=0.05\textwidth]{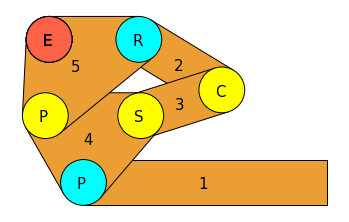}}{{\tiny 2D-M369}}
\qquad\subsubfloat{\includegraphics[width=0.05\textwidth]{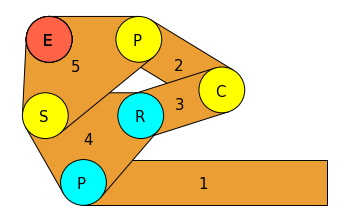}}{{\tiny 2D-M370}}
\qquad\subsubfloat{\includegraphics[width=0.05\textwidth]{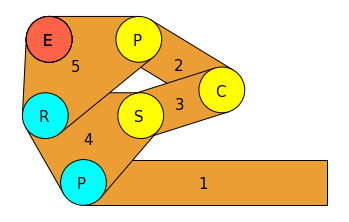}}{{\tiny 2D-M371}}
\qquad\subsubfloat{\includegraphics[width=0.05\textwidth]{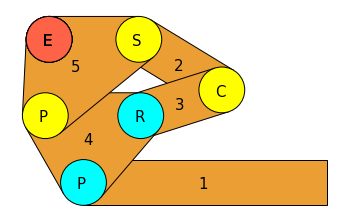}}{{\tiny 2D-M372}}
\qquad\subsubfloat{\includegraphics[width=0.05\textwidth]{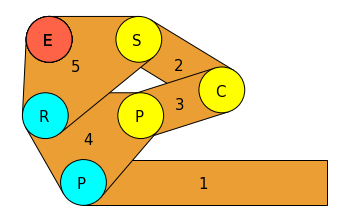}}{{\tiny 2D-M373}}
\qquad\subsubfloat{\includegraphics[width=0.05\textwidth]{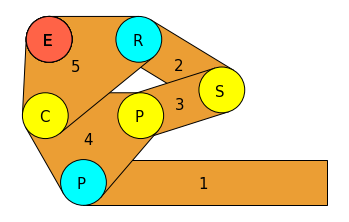}}{{\tiny 2D-M374}}
\qquad\subsubfloat{\includegraphics[width=0.05\textwidth]{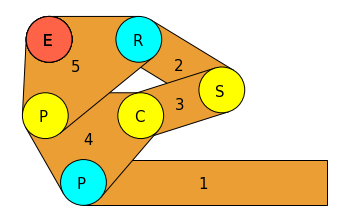}}{{\tiny 2D-M375}}
\qquad\subsubfloat{\includegraphics[width=0.05\textwidth]{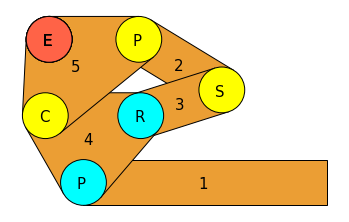}}{{\tiny 2D-M376}}
\qquad\subsubfloat{\includegraphics[width=0.05\textwidth]{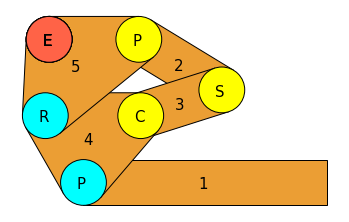}}{{\tiny 2D-M377}}
\qquad\subsubfloat{\includegraphics[width=0.05\textwidth]{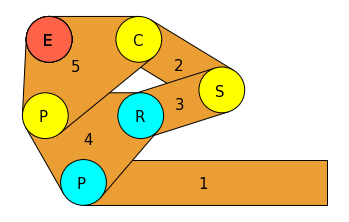}}{{\tiny 2D-M378}}
\qquad\subsubfloat{\includegraphics[width=0.05\textwidth]{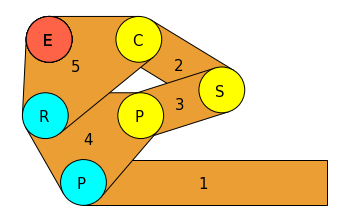}}{{\tiny 2D-M379}}
\qquad\subsubfloat{\includegraphics[width=0.05\textwidth]{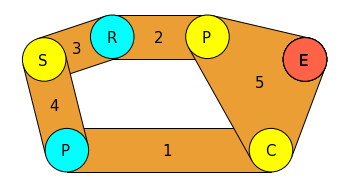}}{{\tiny 2D-M380}}
\qquad\subsubfloat{\includegraphics[width=0.05\textwidth]{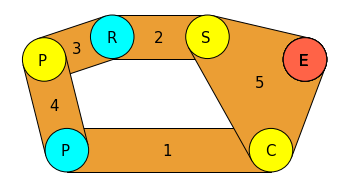}}{{\tiny 2D-M381}}
\qquad\subsubfloat{\includegraphics[width=0.05\textwidth]{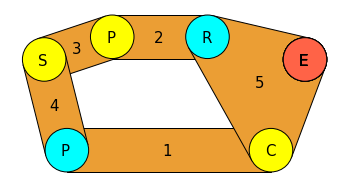}}{{\tiny 2D-M382}}
\qquad\subsubfloat{\includegraphics[width=0.05\textwidth]{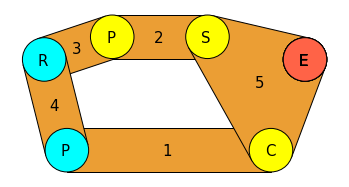}}{{\tiny 2D-M383}}
\qquad\subsubfloat{\includegraphics[width=0.05\textwidth]{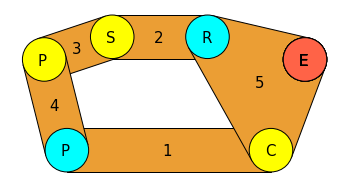}}{{\tiny 2D-M384}}
\qquad\subsubfloat{\includegraphics[width=0.05\textwidth]{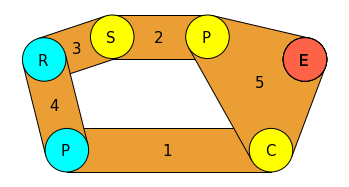}}{{\tiny 2D-M385}}
\qquad\subsubfloat{\includegraphics[width=0.05\textwidth]{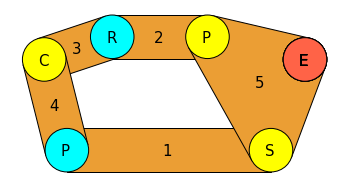}}{{\tiny 2D-M386}}
\qquad\subsubfloat{\includegraphics[width=0.05\textwidth]{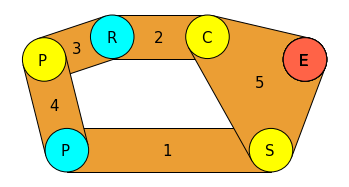}}{{\tiny 2D-M387}}
\qquad\subsubfloat{\includegraphics[width=0.05\textwidth]{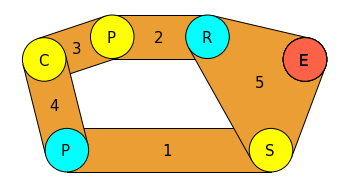}}{{\tiny 2D-M388}}
\qquad\subsubfloat{\includegraphics[width=0.05\textwidth]{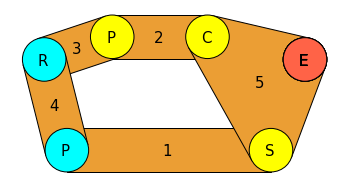}}{{\tiny 2D-M389}}
\qquad\subsubfloat{\includegraphics[width=0.05\textwidth]{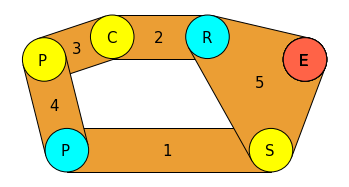}}{{\tiny 2D-M390}}
\qquad\subsubfloat{\includegraphics[width=0.05\textwidth]{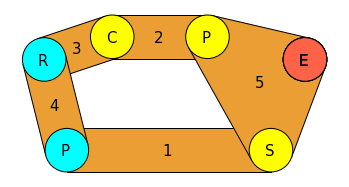}}{{\tiny 2D-M391}}
\qquad\subsubfloat{\includegraphics[width=0.05\textwidth]{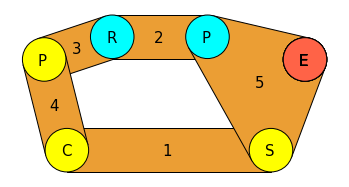}}{{\tiny 2D-M392}}
\qquad\subsubfloat{\includegraphics[width=0.05\textwidth]{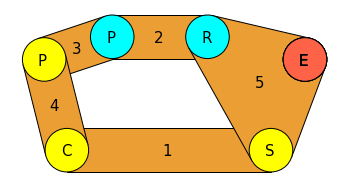}}{{\tiny 2D-M393}}
\qquad\subsubfloat{\includegraphics[width=0.05\textwidth]{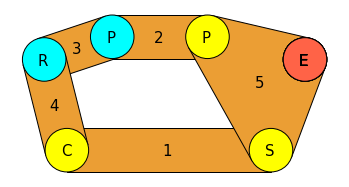}}{{\tiny 2D-M394}}
\qquad\subsubfloat{\includegraphics[width=0.05\textwidth]{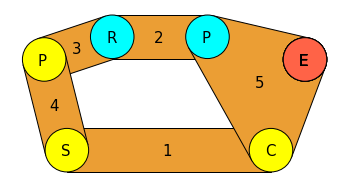}}{{\tiny 2D-M395}}
\qquad\subsubfloat{\includegraphics[width=0.05\textwidth]{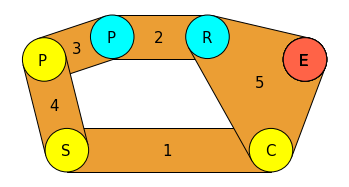}}{{\tiny 2D-M396}}
\qquad\subsubfloat{\includegraphics[width=0.05\textwidth]{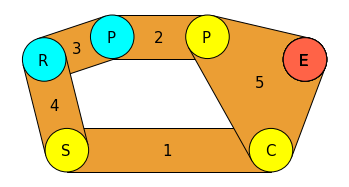}}{{\tiny 2D-M397}}
\qquad\subsubfloat{\includegraphics[width=0.05\textwidth]{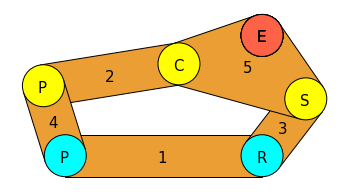}}{{\tiny 2D-M398}}
\qquad\subsubfloat{\includegraphics[width=0.05\textwidth]{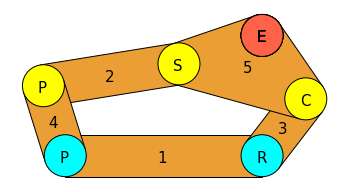}}{{\tiny 2D-M399}}
\qquad\subsubfloat{\includegraphics[width=0.05\textwidth]{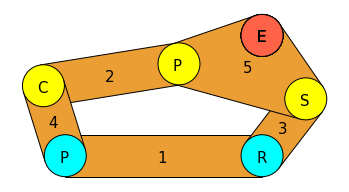}}{{\tiny 2D-M400}}
\qquad\subsubfloat{\includegraphics[width=0.05\textwidth]{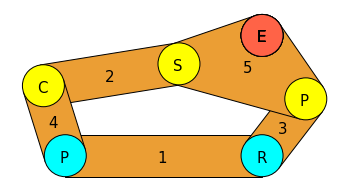}}{{\tiny 2D-M401}}
\qquad\subsubfloat{\includegraphics[width=0.05\textwidth]{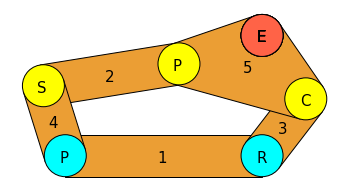}}{{\tiny 2D-M402}}
\qquad\subsubfloat{\includegraphics[width=0.05\textwidth]{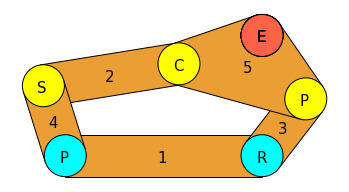}}{{\tiny 2D-M403}}
\qquad\subsubfloat{\includegraphics[width=0.05\textwidth]{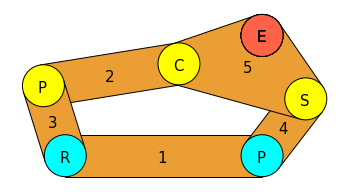}}{{\tiny 2D-M404}}
\qquad\subsubfloat{\includegraphics[width=0.05\textwidth]{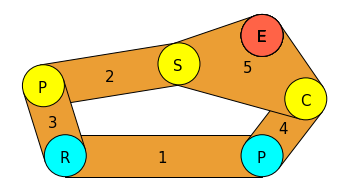}}{{\tiny 2D-M405}}
\qquad\subsubfloat{\includegraphics[width=0.05\textwidth]{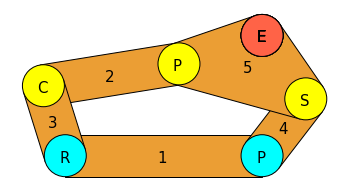}}{{\tiny 2D-M406}}
\qquad\subsubfloat{\includegraphics[width=0.05\textwidth]{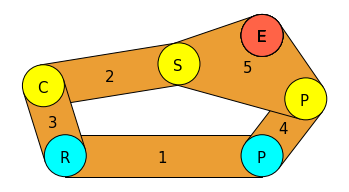}}{{\tiny 2D-M407}}
\qquad\subsubfloat{\includegraphics[width=0.05\textwidth]{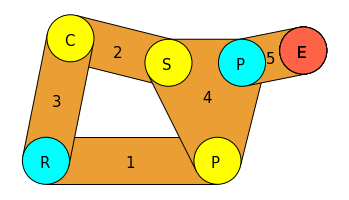}}{{\tiny 2D-M408}}
\qquad\subsubfloat{\includegraphics[width=0.05\textwidth]{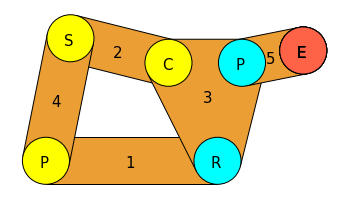}}{{\tiny 2D-M409}}
\qquad\subsubfloat{\includegraphics[width=0.05\textwidth]{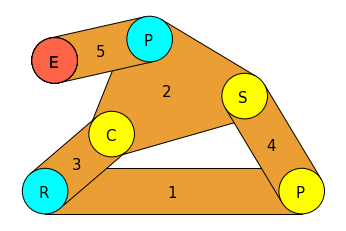}}{{\tiny 2D-M410}}
\qquad\subsubfloat{\includegraphics[width=0.05\textwidth]{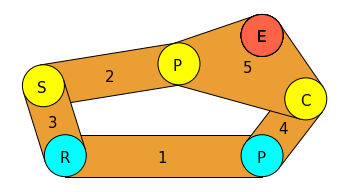}}{{\tiny 2D-M411}}
\qquad\subsubfloat{\includegraphics[width=0.05\textwidth]{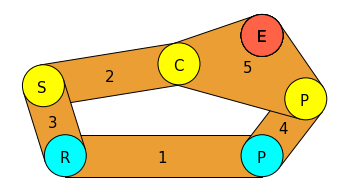}}{{\tiny 2D-M412}}
\qquad\subsubfloat{\includegraphics[width=0.05\textwidth]{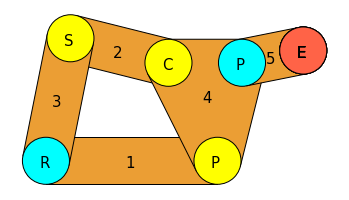}}{{\tiny 2D-M413}}
\qquad\subsubfloat{\includegraphics[width=0.05\textwidth]{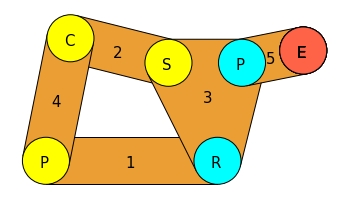}}{{\tiny 2D-M414}}
\qquad\subsubfloat{\includegraphics[width=0.05\textwidth]{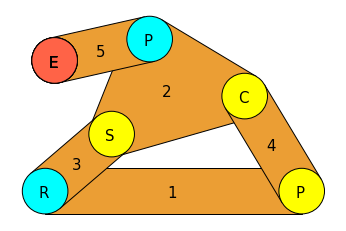}}{{\tiny 2D-M415}}
\qquad\subsubfloat{\includegraphics[width=0.05\textwidth]{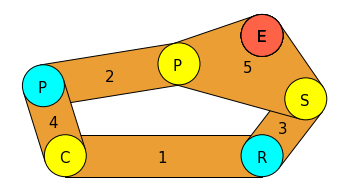}}{{\tiny 2D-M416}}
\qquad\subsubfloat{\includegraphics[width=0.05\textwidth]{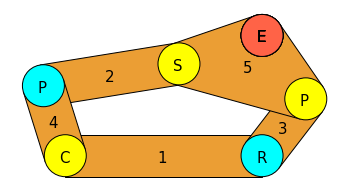}}{{\tiny 2D-M417}}
\qquad\subsubfloat{\includegraphics[width=0.05\textwidth]{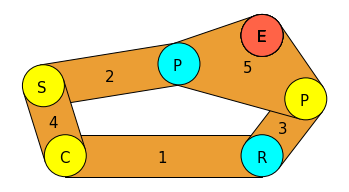}}{{\tiny 2D-M418}}
\qquad\subsubfloat{\includegraphics[width=0.05\textwidth]{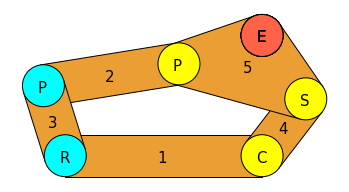}}{{\tiny 2D-M419}}
\qquad\subsubfloat{\includegraphics[width=0.05\textwidth]{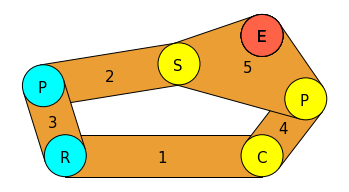}}{{\tiny 2D-M420}}
\qquad\subsubfloat{\includegraphics[width=0.05\textwidth]{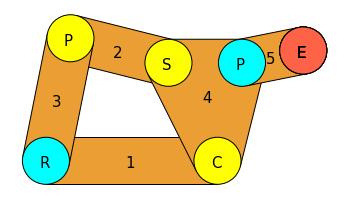}}{{\tiny 2D-M421}}
\qquad\subsubfloat{\includegraphics[width=0.05\textwidth]{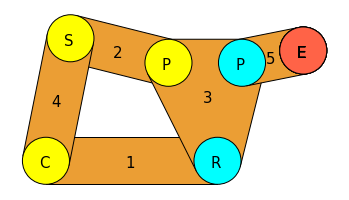}}{{\tiny 2D-M422}}
\qquad\subsubfloat{\includegraphics[width=0.05\textwidth]{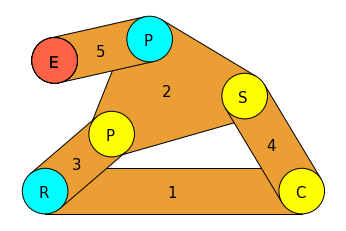}}{{\tiny 2D-M423}}
\qquad\subsubfloat{\includegraphics[width=0.05\textwidth]{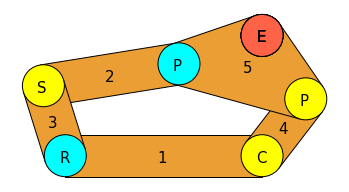}}{{\tiny 2D-M424}}
\qquad\subsubfloat{\includegraphics[width=0.05\textwidth]{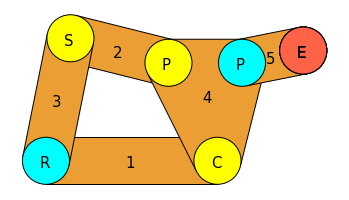}}{{\tiny 2D-M425}}
\qquad\subsubfloat{\includegraphics[width=0.05\textwidth]{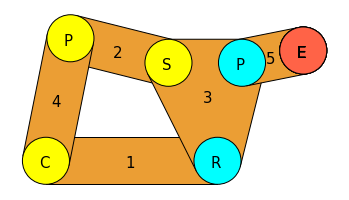}}{{\tiny 2D-M426}}
\qquad\subsubfloat{\includegraphics[width=0.05\textwidth]{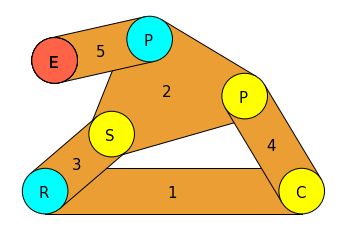}}{{\tiny 2D-M427}}
\qquad\subsubfloat{\includegraphics[width=0.05\textwidth]{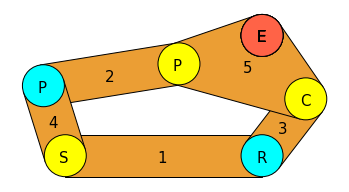}}{{\tiny 2D-M428}}
\qquad\subsubfloat{\includegraphics[width=0.05\textwidth]{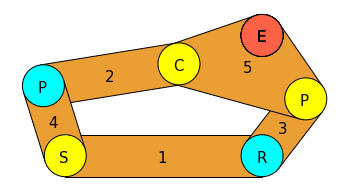}}{{\tiny 2D-M429}}
\qquad\subsubfloat{\includegraphics[width=0.05\textwidth]{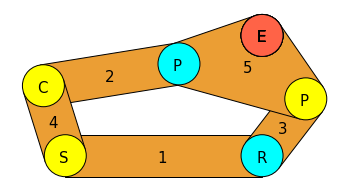}}{{\tiny 2D-M430}}
\qquad\subsubfloat{\includegraphics[width=0.05\textwidth]{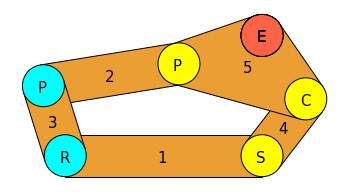}}{{\tiny 2D-M431}}
\qquad\subsubfloat{\includegraphics[width=0.05\textwidth]{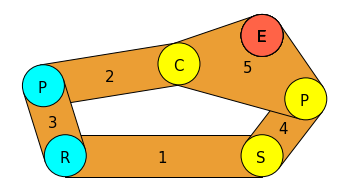}}{{\tiny 2D-M432}}
\qquad\subsubfloat{\includegraphics[width=0.05\textwidth]{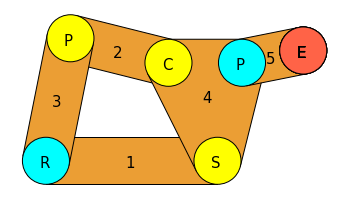}}{{\tiny 2D-M433}}
\qquad\subsubfloat{\includegraphics[width=0.05\textwidth]{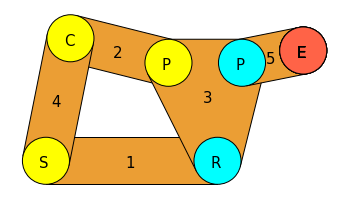}}{{\tiny 2D-M434}}
\qquad\subsubfloat{\includegraphics[width=0.05\textwidth]{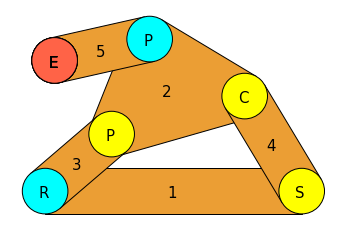}}{{\tiny 2D-M435}}
\qquad\subsubfloat{\includegraphics[width=0.05\textwidth]{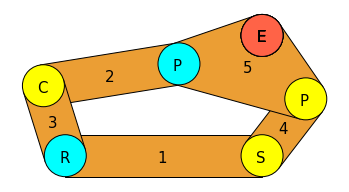}}{{\tiny 2D-M436}}
\qquad\subsubfloat{\includegraphics[width=0.05\textwidth]{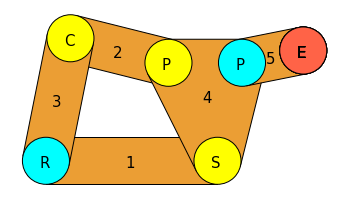}}{{\tiny 2D-M437}}
\qquad\subsubfloat{\includegraphics[width=0.05\textwidth]{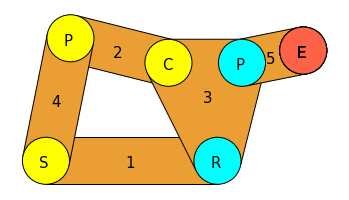}}{{\tiny 2D-M438}}
\qquad\subsubfloat{\includegraphics[width=0.05\textwidth]{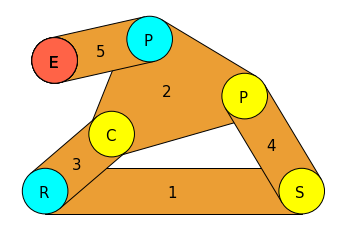}}{{\tiny 2D-M439}}
\qquad\subsubfloat{\includegraphics[width=0.05\textwidth]{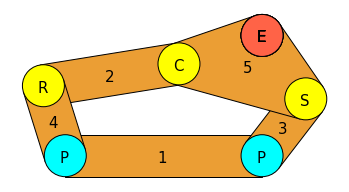}}{{\tiny 2D-M440}}
\qquad\subsubfloat{\includegraphics[width=0.05\textwidth]{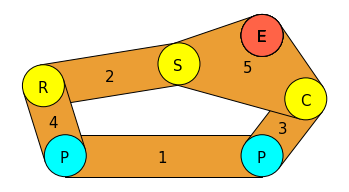}}{{\tiny 2D-M441}}
\qquad\subsubfloat{\includegraphics[width=0.05\textwidth]{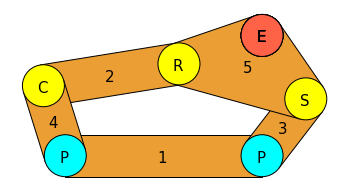}}{{\tiny 2D-M442}}
\qquad\subsubfloat{\includegraphics[width=0.05\textwidth]{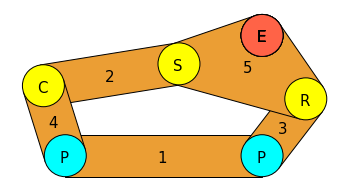}}{{\tiny 2D-M443}}
\qquad\subsubfloat{\includegraphics[width=0.05\textwidth]{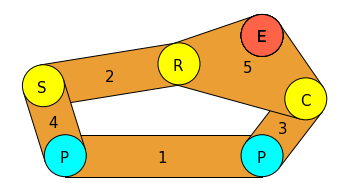}}{{\tiny 2D-M444}}
\qquad\subsubfloat{\includegraphics[width=0.05\textwidth]{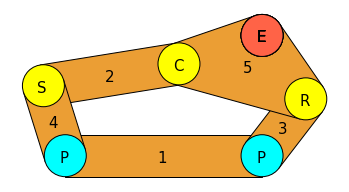}}{{\tiny 2D-M445}}
\qquad\subsubfloat{\includegraphics[width=0.05\textwidth]{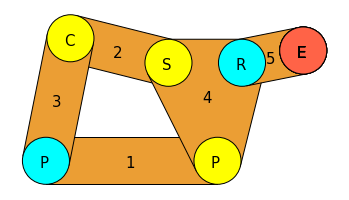}}{{\tiny 2D-M446}}
\qquad\subsubfloat{\includegraphics[width=0.05\textwidth]{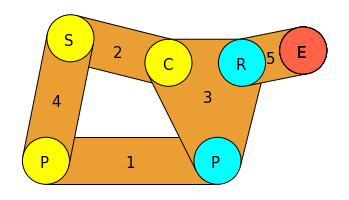}}{{\tiny 2D-M447}}
\qquad\subsubfloat{\includegraphics[width=0.05\textwidth]{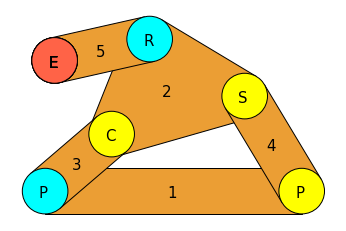}}{{\tiny 2D-M448}}
\qquad\subsubfloat{\includegraphics[width=0.05\textwidth]{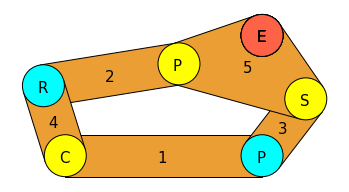}}{{\tiny 2D-M449}}
\qquad\subsubfloat{\includegraphics[width=0.05\textwidth]{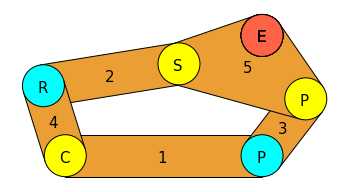}}{{\tiny 2D-M450}}
\qquad\subsubfloat{\includegraphics[width=0.05\textwidth]{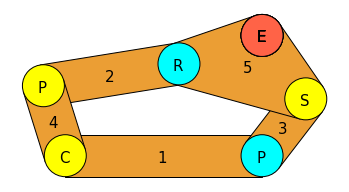}}{{\tiny 2D-M451}}
\qquad\subsubfloat{\includegraphics[width=0.05\textwidth]{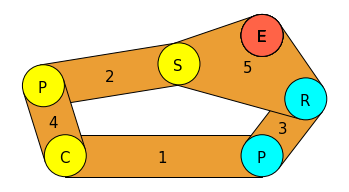}}{{\tiny 2D-M452}}
\qquad\subsubfloat{\includegraphics[width=0.05\textwidth]{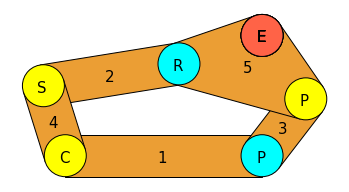}}{{\tiny 2D-M453}}
\qquad\subsubfloat{\includegraphics[width=0.05\textwidth]{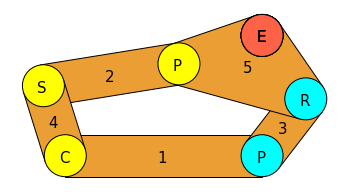}}{{\tiny 2D-M454}}
\qquad\subsubfloat{\includegraphics[width=0.05\textwidth]{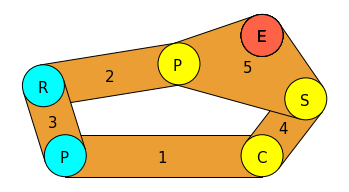}}{{\tiny 2D-M455}}
\qquad\subsubfloat{\includegraphics[width=0.05\textwidth]{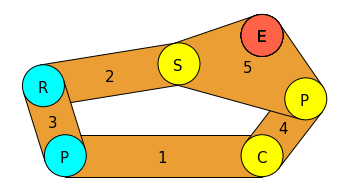}}{{\tiny 2D-M456}}
\qquad\subsubfloat{\includegraphics[width=0.05\textwidth]{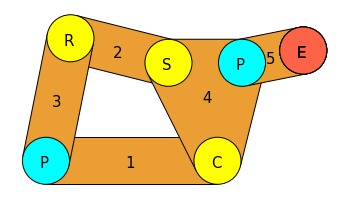}}{{\tiny 2D-M457}}
\qquad\subsubfloat{\includegraphics[width=0.05\textwidth]{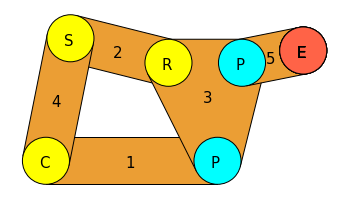}}{{\tiny 2D-M458}}
\qquad\subsubfloat{\includegraphics[width=0.05\textwidth]{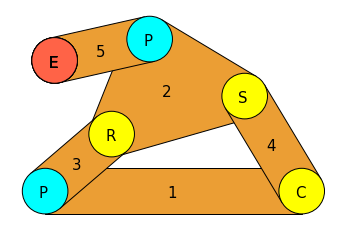}}{{\tiny 2D-M459}}
\qquad\subsubfloat{\includegraphics[width=0.05\textwidth]{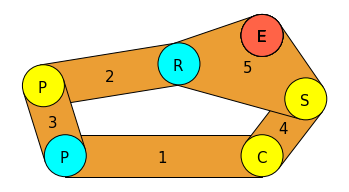}}{{\tiny 2D-M460}}
\qquad\subsubfloat{\includegraphics[width=0.05\textwidth]{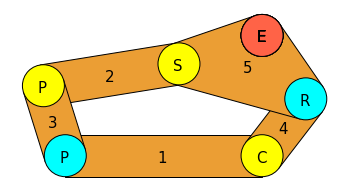}}{{\tiny 2D-M461}}
\qquad\subsubfloat{\includegraphics[width=0.05\textwidth]{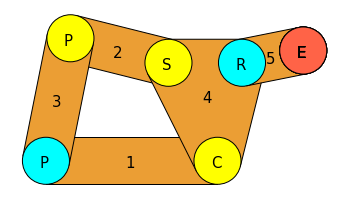}}{{\tiny 2D-M462}}
\qquad\subsubfloat{\includegraphics[width=0.05\textwidth]{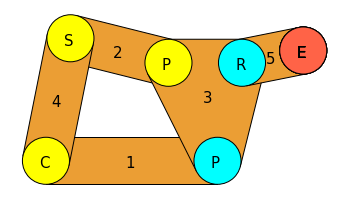}}{{\tiny 2D-M463}}
\qquad\subsubfloat{\includegraphics[width=0.05\textwidth]{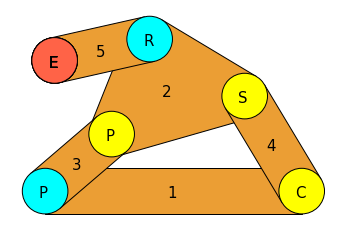}}{{\tiny 2D-M464}}
\qquad\subsubfloat{\includegraphics[width=0.05\textwidth]{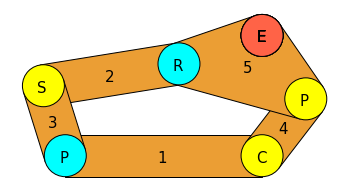}}{{\tiny 2D-M465}}
\qquad\subsubfloat{\includegraphics[width=0.05\textwidth]{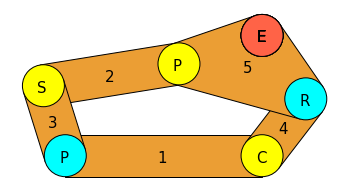}}{{\tiny 2D-M466}}
\qquad\subsubfloat{\includegraphics[width=0.05\textwidth]{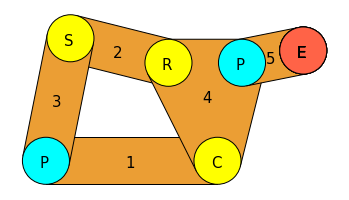}}{{\tiny 2D-M467}}
\qquad\subsubfloat{\includegraphics[width=0.05\textwidth]{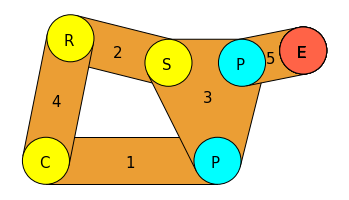}}{{\tiny 2D-M468}}
\qquad\subsubfloat{\includegraphics[width=0.05\textwidth]{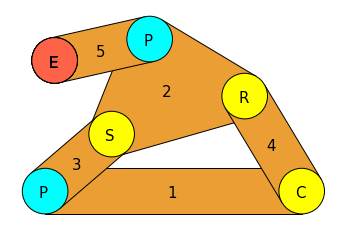}}{{\tiny 2D-M469}}
\qquad\subsubfloat{\includegraphics[width=0.05\textwidth]{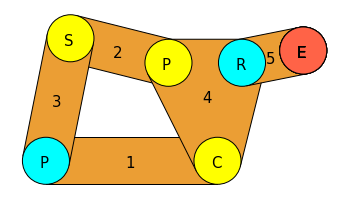}}{{\tiny 2D-M470}}
\qquad\subsubfloat{\includegraphics[width=0.05\textwidth]{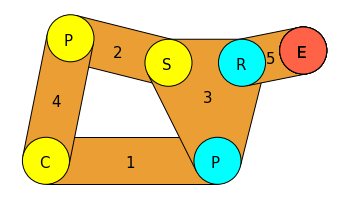}}{{\tiny 2D-M471}}
\qquad\subsubfloat{\includegraphics[width=0.05\textwidth]{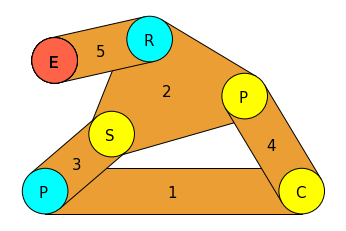}}{{\tiny 2D-M472}}
\qquad\subsubfloat{\includegraphics[width=0.05\textwidth]{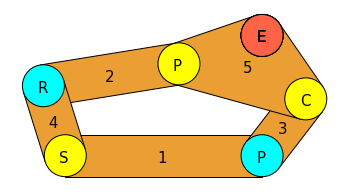}}{{\tiny 2D-M473}}
\qquad\subsubfloat{\includegraphics[width=0.05\textwidth]{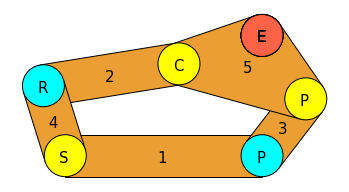}}{{\tiny 2D-M474}}
\qquad\subsubfloat{\includegraphics[width=0.05\textwidth]{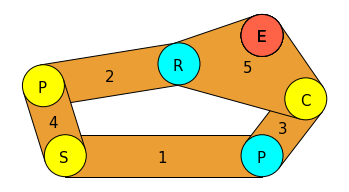}}{{\tiny 2D-M475}}
\qquad\subsubfloat{\includegraphics[width=0.05\textwidth]{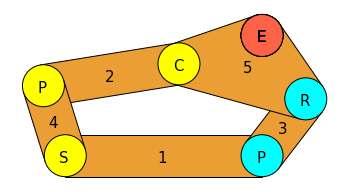}}{{\tiny 2D-M476}}
\qquad\subsubfloat{\includegraphics[width=0.05\textwidth]{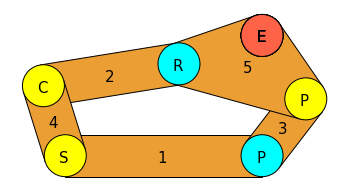}}{{\tiny 2D-M477}}
\qquad\subsubfloat{\includegraphics[width=0.05\textwidth]{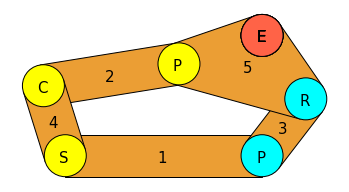}}{{\tiny 2D-M478}}
\qquad\subsubfloat{\includegraphics[width=0.05\textwidth]{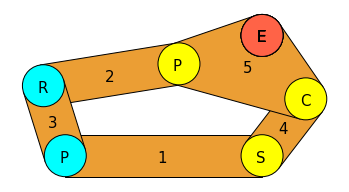}}{{\tiny 2D-M479}}
\qquad\subsubfloat{\includegraphics[width=0.05\textwidth]{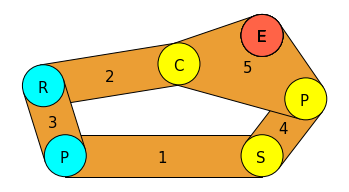}}{{\tiny 2D-M480}}
\qquad\subsubfloat{\includegraphics[width=0.05\textwidth]{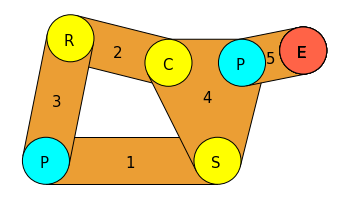}}{{\tiny 2D-M481}}
\qquad\subsubfloat{\includegraphics[width=0.05\textwidth]{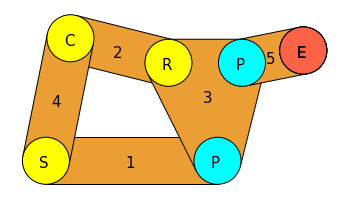}}{{\tiny 2D-M482}}
\qquad\subsubfloat{\includegraphics[width=0.05\textwidth]{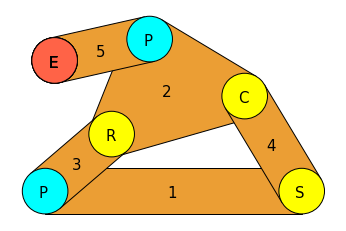}}{{\tiny 2D-M483}}
\qquad\subsubfloat{\includegraphics[width=0.05\textwidth]{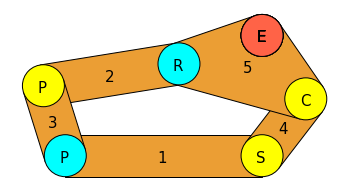}}{{\tiny 2D-M484}}
\qquad\subsubfloat{\includegraphics[width=0.05\textwidth]{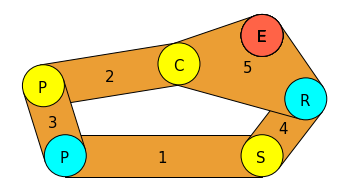}}{{\tiny 2D-M485}}
\qquad\subsubfloat{\includegraphics[width=0.05\textwidth]{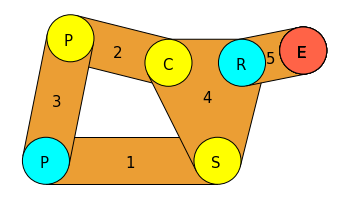}}{{\tiny 2D-M486}}
\qquad\subsubfloat{\includegraphics[width=0.05\textwidth]{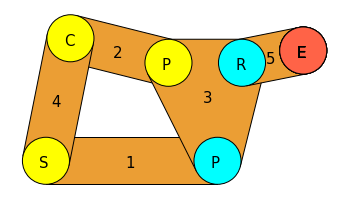}}{{\tiny 2D-M487}}
\qquad\subsubfloat{\includegraphics[width=0.05\textwidth]{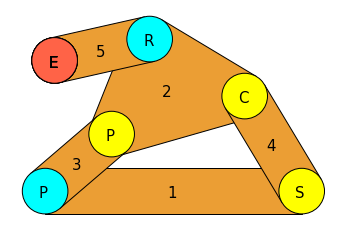}}{{\tiny 2D-M488}}
\qquad\subsubfloat{\includegraphics[width=0.05\textwidth]{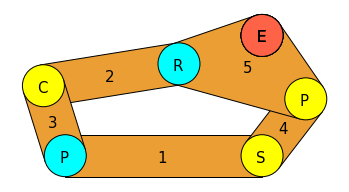}}{{\tiny 2D-M489}}
\qquad\subsubfloat{\includegraphics[width=0.05\textwidth]{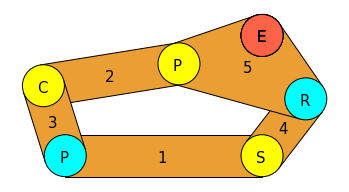}}{{\tiny 2D-M490}}
\qquad\subsubfloat{\includegraphics[width=0.05\textwidth]{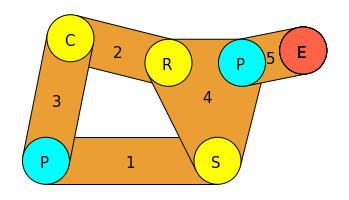}}{{\tiny 2D-M491}}
\qquad\subsubfloat{\includegraphics[width=0.05\textwidth]{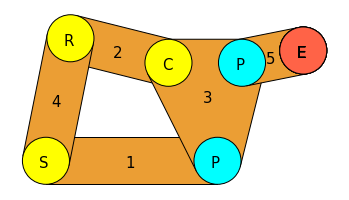}}{{\tiny 2D-M492}}
\qquad\subsubfloat{\includegraphics[width=0.05\textwidth]{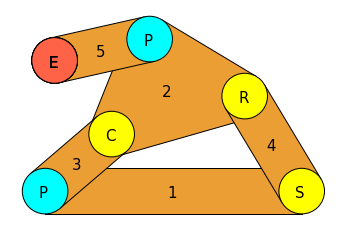}}{{\tiny 2D-M493}}
\qquad\subsubfloat{\includegraphics[width=0.05\textwidth]{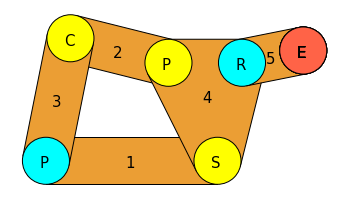}}{{\tiny 2D-M494}}
\qquad\subsubfloat{\includegraphics[width=0.05\textwidth]{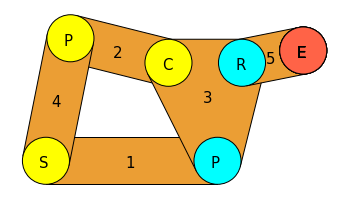}}{{\tiny 2D-M495}}  
\qquad\subsubfloat{\includegraphics[width=0.05\textwidth]{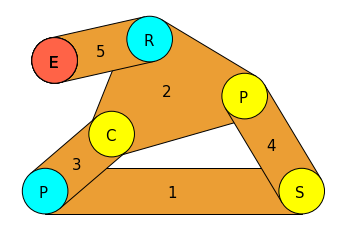}}{{\tiny 2D-M496}}
\qquad\subsubfloat{\includegraphics[width=0.05\textwidth]{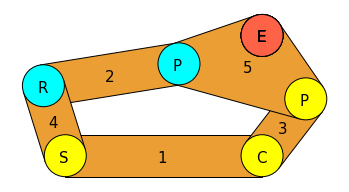}}{{\tiny 2D-M497}}
\qquad\subsubfloat{\includegraphics[width=0.05\textwidth]{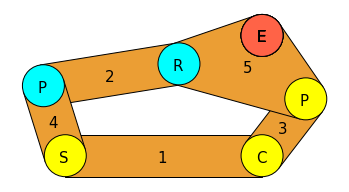}}{{\tiny 2D-M498}}
\qquad\subsubfloat{\includegraphics[width=0.05\textwidth]{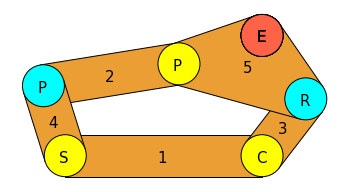}}{{\tiny 2D-M499}}
\qquad\subsubfloat{\includegraphics[width=0.05\textwidth]{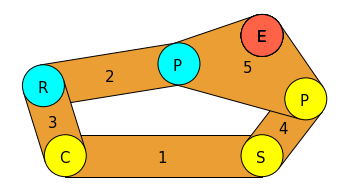}}{{\tiny 2D-M500}}
\qquad\subsubfloat{\includegraphics[width=0.05\textwidth]{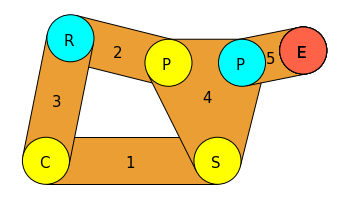}}{{\tiny 2D-M501}}
\qquad\subsubfloat{\includegraphics[width=0.05\textwidth]{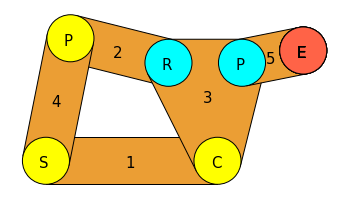}}{{\tiny 2D-M502}}
\qquad\subsubfloat{\includegraphics[width=0.05\textwidth]{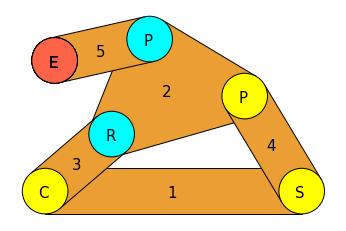}}{{\tiny 2D-M503}}
\qquad\subsubfloat{\includegraphics[width=0.05\textwidth]{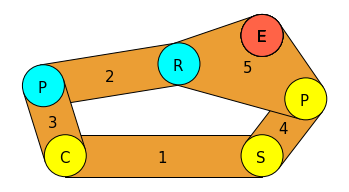}}{{\tiny 2D-M504}}
\qquad\subsubfloat{\includegraphics[width=0.05\textwidth]{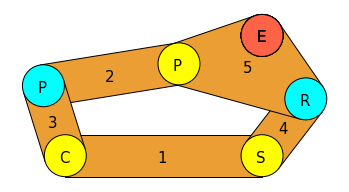}}{{\tiny 2D-M505}}
\qquad\subsubfloat{\includegraphics[width=0.05\textwidth]{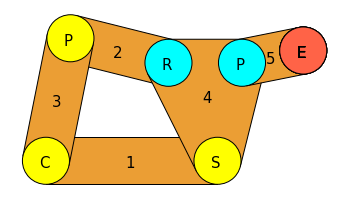}}{{\tiny 2D-M506}}
\qquad\subsubfloat{\includegraphics[width=0.05\textwidth]{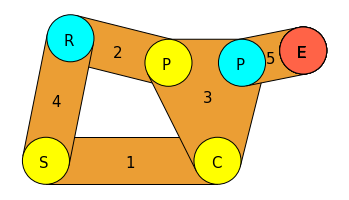}}{{\tiny 2D-M507}}
\qquad\subsubfloat{\includegraphics[width=0.05\textwidth]{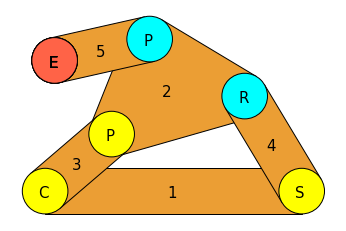}}{{\tiny 2D-M508}}
\qquad\subsubfloat{\includegraphics[width=0.05\textwidth]{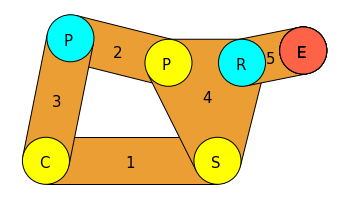}}{{\tiny 2D-M509}}
\qquad\subsubfloat{\includegraphics[width=0.05\textwidth]{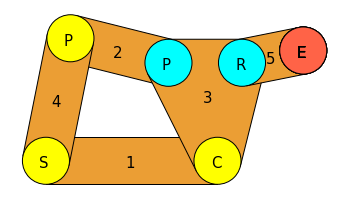}}{{\tiny 2D-M510}}
\qquad\subsubfloat{\includegraphics[width=0.05\textwidth]{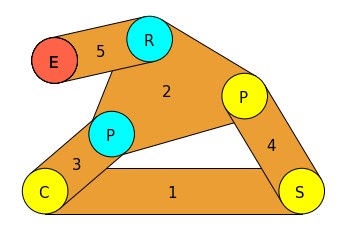}}{{\tiny 2D-M511}}
\qquad\subsubfloat{\includegraphics[width=0.05\textwidth]{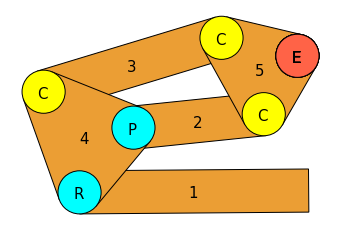}}{{\tiny 2D-M512}}
\qquad\subsubfloat{\includegraphics[width=0.05\textwidth]{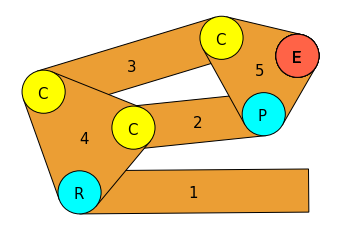}}{{\tiny 2D-M513}}
\qquad\subsubfloat{\includegraphics[width=0.05\textwidth]{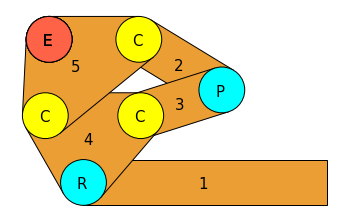}}{{\tiny 2D-M514}}
\qquad\subsubfloat{\includegraphics[width=0.05\textwidth]{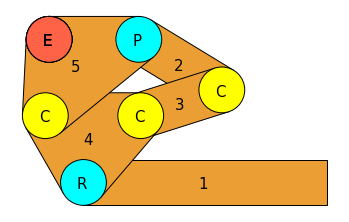}}{{\tiny 2D-M515}}
\qquad\subsubfloat{\includegraphics[width=0.05\textwidth]{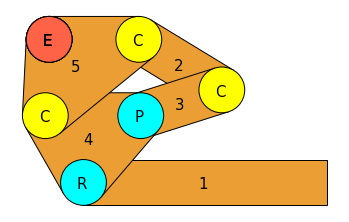}}{{\tiny 2D-M516}}
\qquad\subsubfloat{\includegraphics[width=0.05\textwidth]{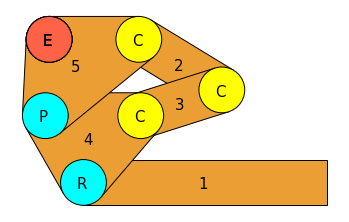}}{{\tiny 2D-M517}}
\qquad\subsubfloat{\includegraphics[width=0.05\textwidth]{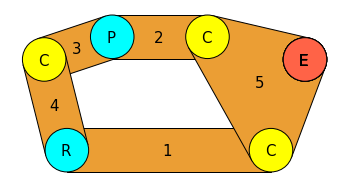}}{{\tiny 2D-M518}}
\qquad\subsubfloat{\includegraphics[width=0.05\textwidth]{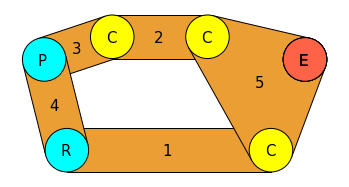}}{{\tiny 2D-M519}}
\qquad\subsubfloat{\includegraphics[width=0.05\textwidth]{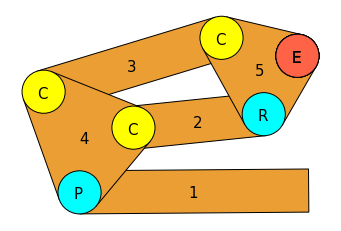}}{{\tiny 2D-M520}}
\qquad\subsubfloat{\includegraphics[width=0.05\textwidth]{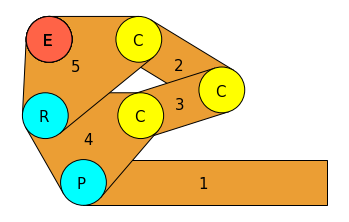}}{{\tiny 2D-M521}}
\qquad\subsubfloat{\includegraphics[width=0.05\textwidth]{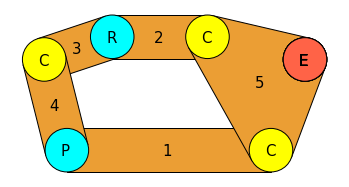}}{{\tiny 2D-M522}}
\qquad\subsubfloat{\includegraphics[width=0.05\textwidth]{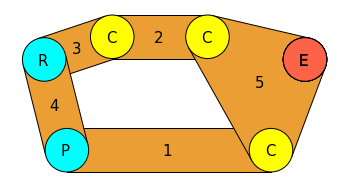}}{{\tiny 2D-M523}}
\qquad\subsubfloat{\includegraphics[width=0.05\textwidth]{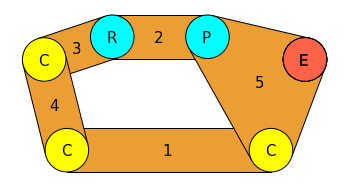}}{{\tiny 2D-M524}}
\qquad\subsubfloat{\includegraphics[width=0.05\textwidth]{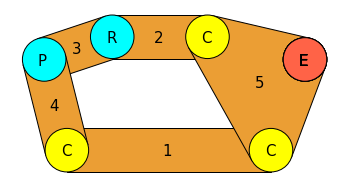}}{{\tiny 2D-M525}}
\qquad\subsubfloat{\includegraphics[width=0.05\textwidth]{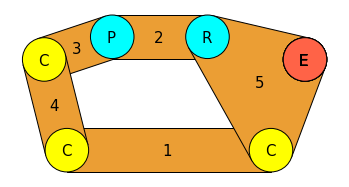}}{{\tiny 2D-M526}}
\qquad\subsubfloat{\includegraphics[width=0.05\textwidth]{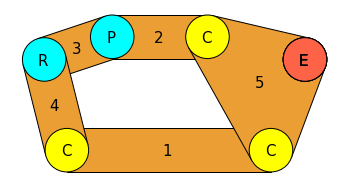}}{{\tiny 2D-M527}}
\qquad\subsubfloat{\includegraphics[width=0.05\textwidth]{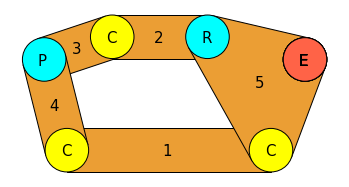}}{{\tiny 2D-M528}}

      \end{minipage}
    \end{subfigure}
    \caption{Schematic diagrams of 2-DOF Manipulators (Contd.)}
    \end{figure}

\begin{figure}[H]\ContinuedFloat
  \centering
  \begin{subfigure}{\columnwidth}
    \begin{minipage}{\textwidth}\footnotesize
    \centering

\subsubfloat{\includegraphics[width=0.05\textwidth]{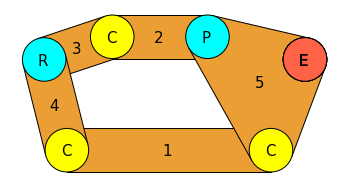}}{{\tiny 2D-M529}}
\qquad\subsubfloat{\includegraphics[width=0.05\textwidth]{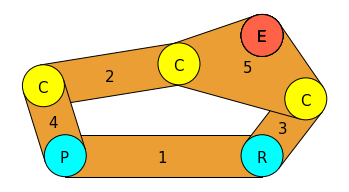}}{{\tiny 2D-M530}}
\qquad\subsubfloat{\includegraphics[width=0.05\textwidth]{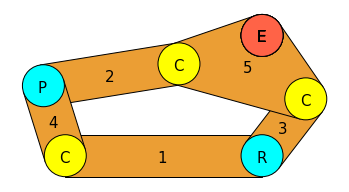}}{{\tiny 2D-M531}}
\qquad\subsubfloat{\includegraphics[width=0.05\textwidth]{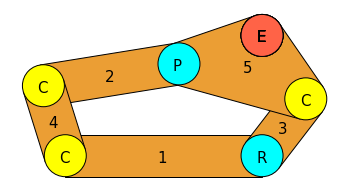}}{{\tiny 2D-M532}}
\qquad\subsubfloat{\includegraphics[width=0.05\textwidth]{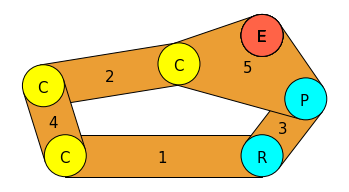}}{{\tiny 2D-M533}}
\qquad\subsubfloat{\includegraphics[width=0.05\textwidth]{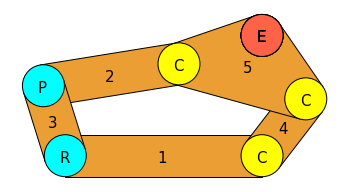}}{{\tiny 2D-M534}}
\qquad\subsubfloat{\includegraphics[width=0.05\textwidth]{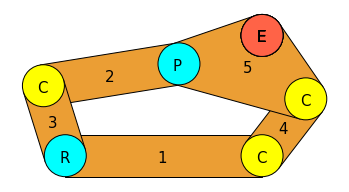}}{{\tiny 2D-M535}}
\qquad  \subsubfloat{\includegraphics[width=0.05\textwidth]{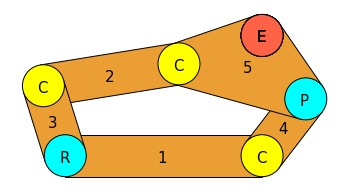}}{{\tiny 2D-M536}}
\qquad\subsubfloat{\includegraphics[width=0.05\textwidth]{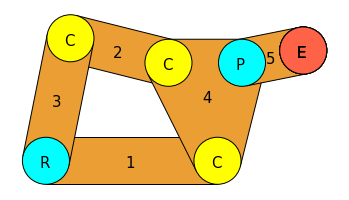}}{{\tiny 2D-M537}}
\qquad\subsubfloat{\includegraphics[width=0.05\textwidth]{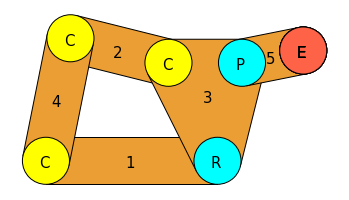}}{{\tiny 2D-M538}}
\qquad\subsubfloat{\includegraphics[width=0.05\textwidth]{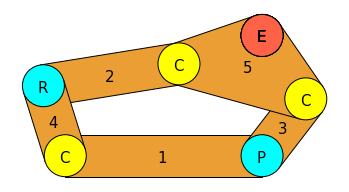}}{{\tiny 2D-M539}}
\qquad\subsubfloat{\includegraphics[width=0.05\textwidth]{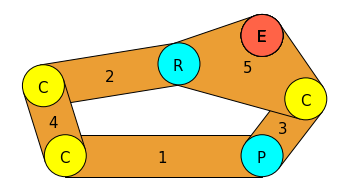}}{{\tiny 2D-M540}}
\qquad\subsubfloat{\includegraphics[width=0.05\textwidth]{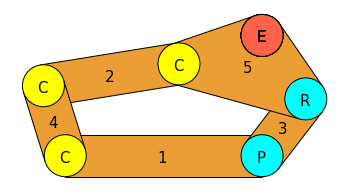}}{{\tiny 2D-M541}}
\qquad\subsubfloat{\includegraphics[width=0.05\textwidth]{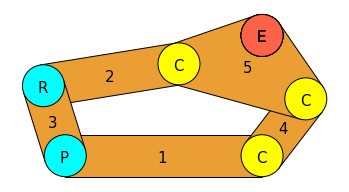}}{{\tiny 2D-M542}}
\qquad\subsubfloat{\includegraphics[width=0.05\textwidth]{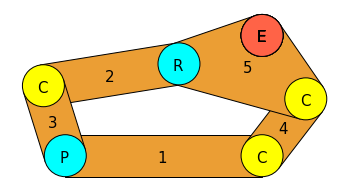}}{{\tiny 2D-M543}}
\qquad\subsubfloat{\includegraphics[width=0.05\textwidth]{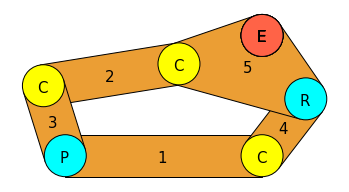}}{{\tiny 2D-M544}}
\qquad\subsubfloat{\includegraphics[width=0.05\textwidth]{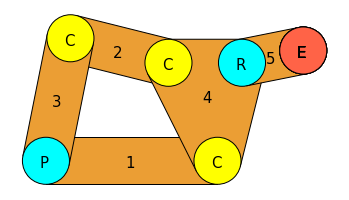}}{{\tiny 2D-M545}}
\qquad\subsubfloat{\includegraphics[width=0.05\textwidth]{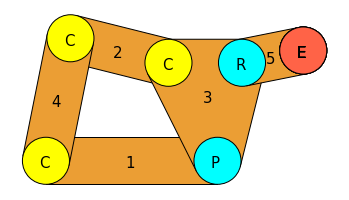}}{{\tiny 2D-M546}}
\qquad\subsubfloat{\includegraphics[width=0.05\textwidth]{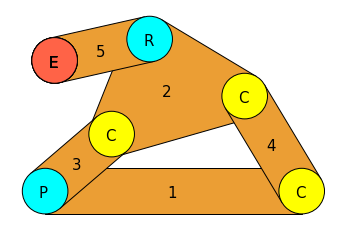}}{{\tiny 2D-M547}}
\qquad\subsubfloat{\includegraphics[width=0.05\textwidth]{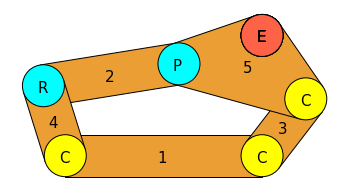}}{{\tiny 2D-M548}}
\qquad\subsubfloat{\includegraphics[width=0.05\textwidth]{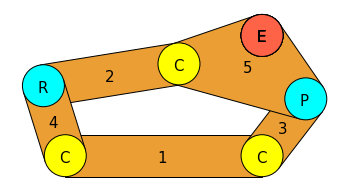}}{{\tiny 2D-M549}}
\qquad\subsubfloat{\includegraphics[width=0.05\textwidth]{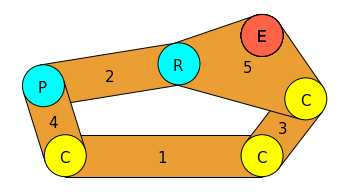}}{{\tiny 2D-M550}}
\qquad\subsubfloat{\includegraphics[width=0.05\textwidth]{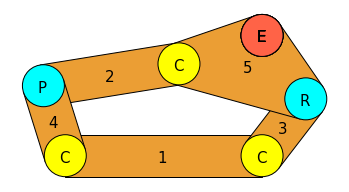}}{{\tiny 2D-M551}}
\qquad\subsubfloat{\includegraphics[width=0.05\textwidth]{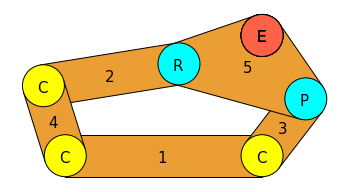}}{{\tiny 2D-M552}}
\qquad\subsubfloat{\includegraphics[width=0.05\textwidth]{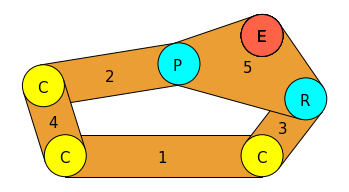}}{{\tiny 2D-M553}}
\qquad\subsubfloat{\includegraphics[width=0.05\textwidth]{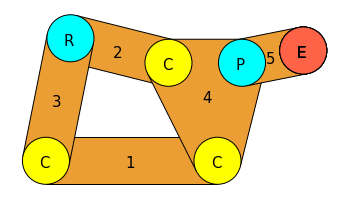}}{{\tiny 2D-M554}}
\qquad\subsubfloat{\includegraphics[width=0.05\textwidth]{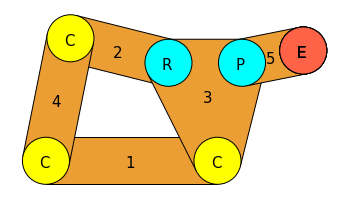}}{{\tiny 2D-M555}}
\qquad\subsubfloat{\includegraphics[width=0.05\textwidth]{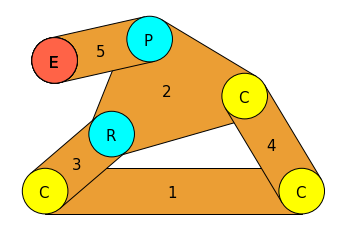}}{{\tiny 2D-M556}}
\qquad\subsubfloat{\includegraphics[width=0.05\textwidth]{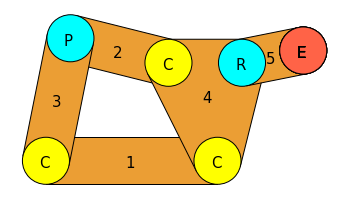}}{{\tiny 2D-M557}}
\qquad\subsubfloat{\includegraphics[width=0.05\textwidth]{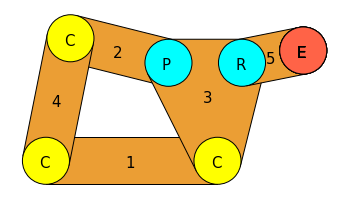}}{{\tiny 2D-M558}}
\qquad\subsubfloat{\includegraphics[width=0.05\textwidth]{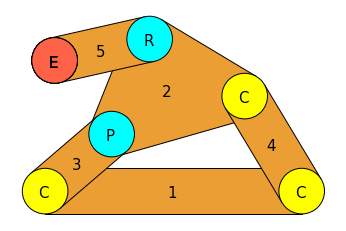}}{{\tiny 2D-M559}}
\qquad\subsubfloat{\includegraphics[width=0.05\textwidth]{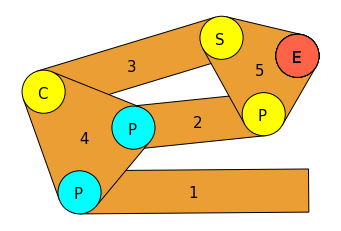}}{{\tiny 2D-M560}}
\qquad\subsubfloat{\includegraphics[width=0.05\textwidth]{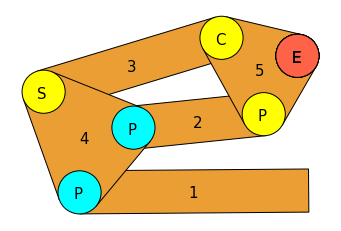}}{{\tiny 2D-M561}}
\qquad\subsubfloat{\includegraphics[width=0.05\textwidth]{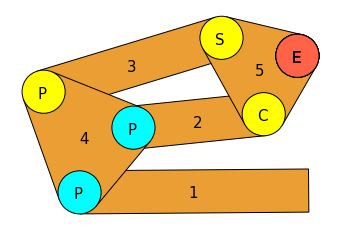}}{{\tiny 2D-M562}}
\qquad\subsubfloat{\includegraphics[width=0.05\textwidth]{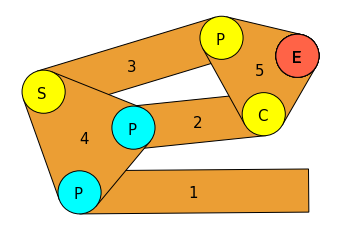}}{{\tiny 2D-M563}}
\qquad\subsubfloat{\includegraphics[width=0.05\textwidth]{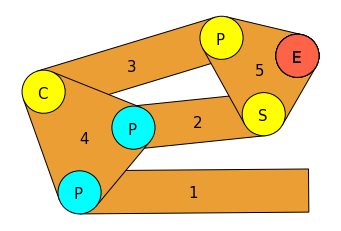}}{{\tiny 2D-M564}}
\qquad\subsubfloat{\includegraphics[width=0.05\textwidth]{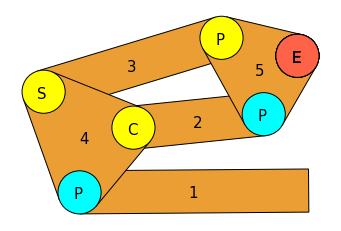}}{{\tiny 2D-M565}}
\qquad\subsubfloat{\includegraphics[width=0.05\textwidth]{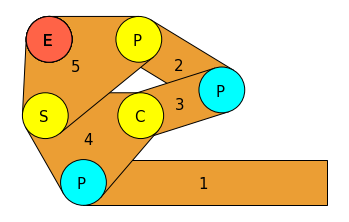}}{{\tiny 2D-M566}}
\qquad\subsubfloat{\includegraphics[width=0.05\textwidth]{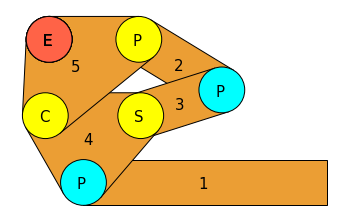}}{{\tiny 2D-M567}}
\qquad\subsubfloat{\includegraphics[width=0.05\textwidth]{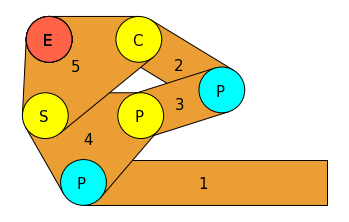}}{{\tiny 2D-M568}}
\qquad\subsubfloat{\includegraphics[width=0.05\textwidth]{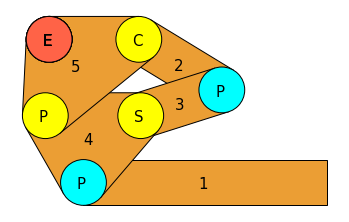}}{{\tiny 2D-M569}}
\qquad\subsubfloat{\includegraphics[width=0.05\textwidth]{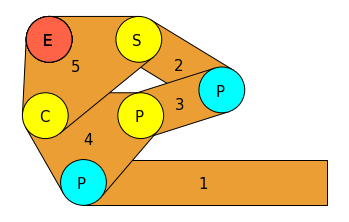}}{{\tiny 2D-M570}}
\qquad\subsubfloat{\includegraphics[width=0.05\textwidth]{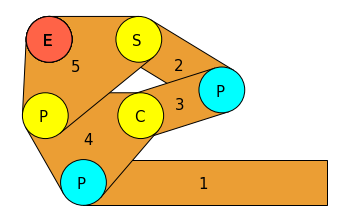}}{{\tiny 2D-M571}}
\qquad\subsubfloat{\includegraphics[width=0.05\textwidth]{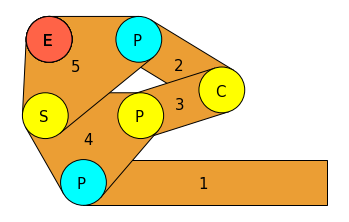}}{{\tiny 2D-M572}}
\qquad\subsubfloat{\includegraphics[width=0.05\textwidth]{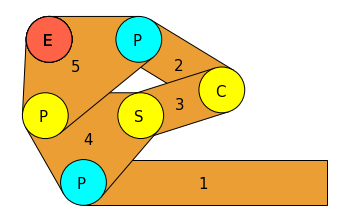}}{{\tiny 2D-M573}}
\qquad\subsubfloat{\includegraphics[width=0.05\textwidth]{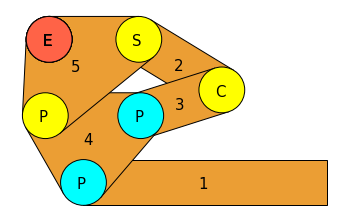}}{{\tiny 2D-M574}}
\qquad\subsubfloat{\includegraphics[width=0.05\textwidth]{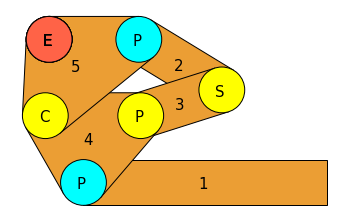}}{{\tiny 2D-M575}}
\qquad\subsubfloat{\includegraphics[width=0.05\textwidth]{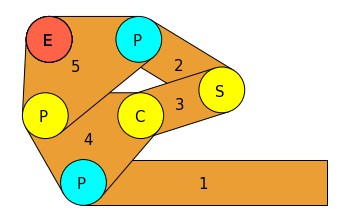}}{{\tiny 2D-M576}}
\qquad\subsubfloat{\includegraphics[width=0.05\textwidth]{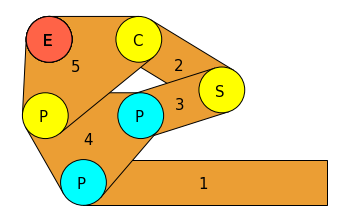}}{{\tiny 2D-M577}}
\qquad\subsubfloat{\includegraphics[width=0.05\textwidth]{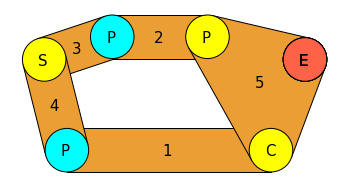}}{{\tiny 2D-M578}}
\qquad\subsubfloat{\includegraphics[width=0.05\textwidth]{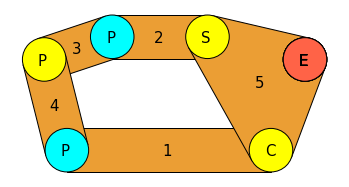}}{{\tiny 2D-M579}}
\qquad\subsubfloat{\includegraphics[width=0.05\textwidth]{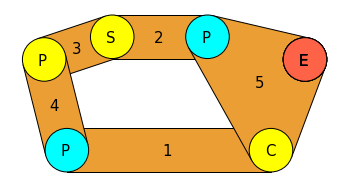}}{{\tiny 2D-M580}}
\qquad\subsubfloat{\includegraphics[width=0.05\textwidth]{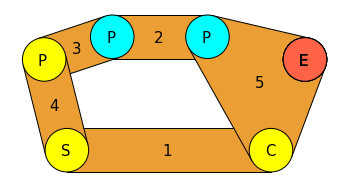}}{{\tiny 2D-M581}}
\qquad\subsubfloat{\includegraphics[width=0.05\textwidth]{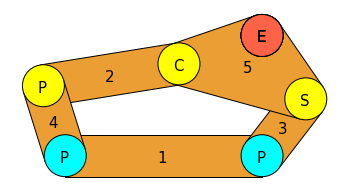}}{{\tiny 2D-M582}}
\qquad\subsubfloat{\includegraphics[width=0.05\textwidth]{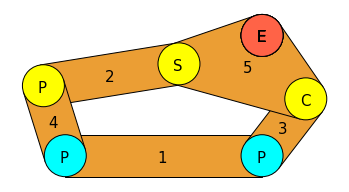}}{{\tiny 2D-M583}}
\qquad\subsubfloat{\includegraphics[width=0.05\textwidth]{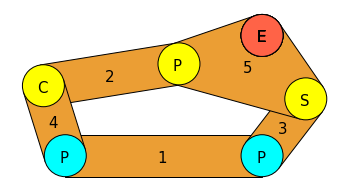}}{{\tiny 2D-M584}}
\qquad\subsubfloat{\includegraphics[width=0.05\textwidth]{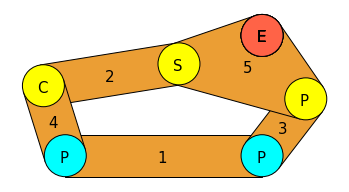}}{{\tiny 2D-M585}}
\qquad\subsubfloat{\includegraphics[width=0.05\textwidth]{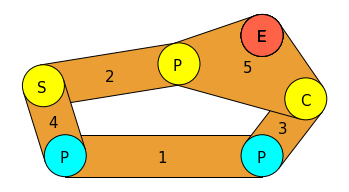}}{{\tiny 2D-M586}}
\qquad\subsubfloat{\includegraphics[width=0.05\textwidth]{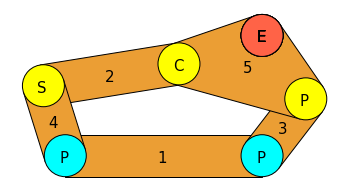}}{{\tiny 2D-M587}}
\qquad\subsubfloat{\includegraphics[width=0.05\textwidth]{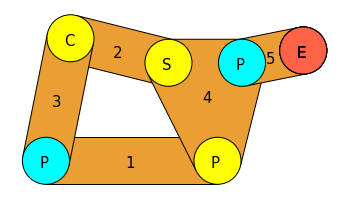}}{{\tiny 2D-M588}}
\qquad\subsubfloat{\includegraphics[width=0.05\textwidth]{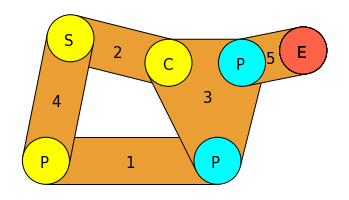}}{{\tiny 2D-M589}}
\qquad\subsubfloat{\includegraphics[width=0.05\textwidth]{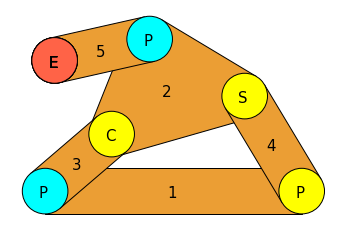}}{{\tiny 2D-M590}}
\qquad\subsubfloat{\includegraphics[width=0.05\textwidth]{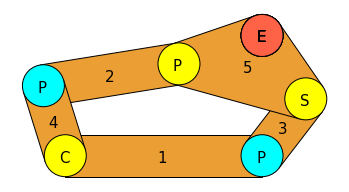}}{{\tiny 2D-M591}}
\qquad\subsubfloat{\includegraphics[width=0.05\textwidth]{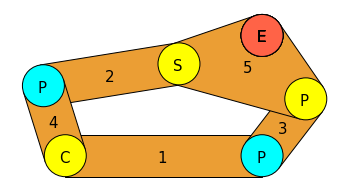}}{{\tiny 2D-M592}}
\qquad\subsubfloat{\includegraphics[width=0.05\textwidth]{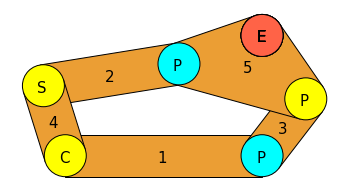}}{{\tiny 2D-M593}}
\qquad\subsubfloat{\includegraphics[width=0.05\textwidth]{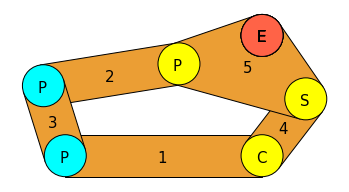}}{{\tiny 2D-M594}}
\qquad\subsubfloat{\includegraphics[width=0.05\textwidth]{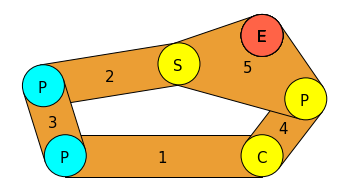}}{{\tiny 2D-M595}}
\qquad\subsubfloat{\includegraphics[width=0.05\textwidth]{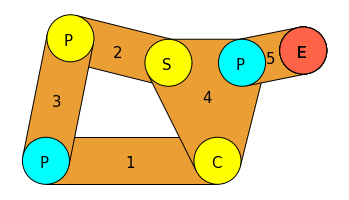}}{{\tiny 2D-M596}}
\qquad\subsubfloat{\includegraphics[width=0.05\textwidth]{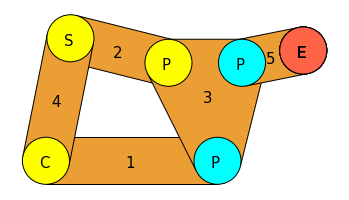}}{{\tiny 2D-M597}}
\qquad\subsubfloat{\includegraphics[width=0.05\textwidth]{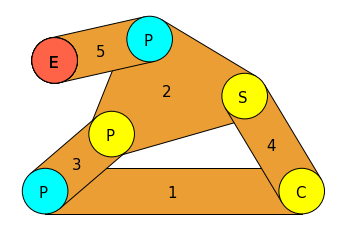}}{{\tiny 2D-M598}}
\qquad\subsubfloat{\includegraphics[width=0.05\textwidth]{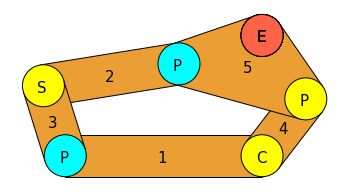}}{{\tiny 2D-M599}}
\qquad\subsubfloat{\includegraphics[width=0.05\textwidth]{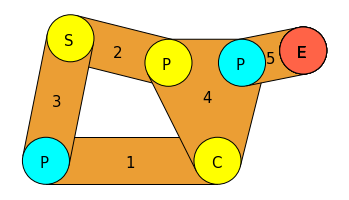}}{{\tiny 2D-M600}}
\qquad\subsubfloat{\includegraphics[width=0.05\textwidth]{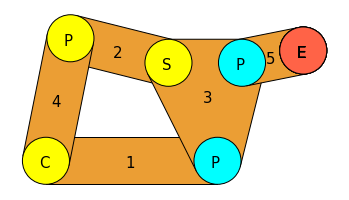}}{{\tiny 2D-M601}}
\qquad\subsubfloat{\includegraphics[width=0.05\textwidth]{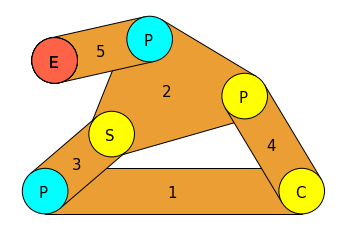}}{{\tiny 2D-M602}}
\qquad\subsubfloat{\includegraphics[width=0.05\textwidth]{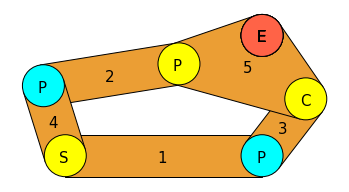}}{{\tiny 2D-M603}}
\qquad\subsubfloat{\includegraphics[width=0.05\textwidth]{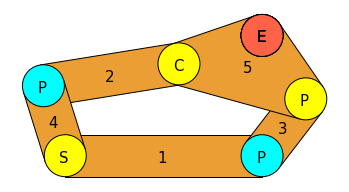}}{{\tiny 2D-M604}}
\qquad\subsubfloat{\includegraphics[width=0.05\textwidth]{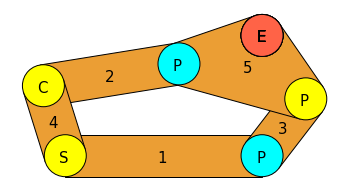}}{{\tiny 2D-M605}}
\qquad\subsubfloat{\includegraphics[width=0.05\textwidth]{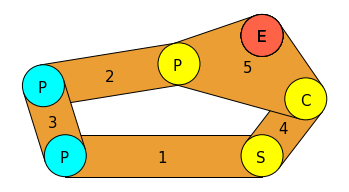}}{{\tiny 2D-M606}}
\qquad\subsubfloat{\includegraphics[width=0.05\textwidth]{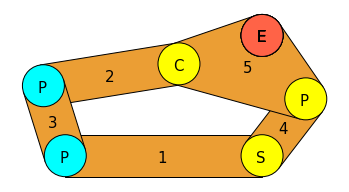}}{{\tiny 2D-M607}}
\qquad\subsubfloat{\includegraphics[width=0.05\textwidth]{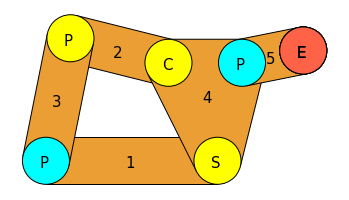}}{{\tiny 2D-M608}}
\qquad\subsubfloat{\includegraphics[width=0.05\textwidth]{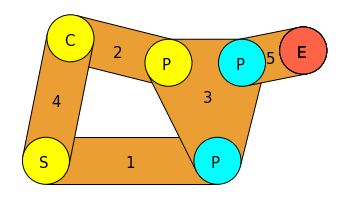}}{{\tiny 2D-M609}}
\qquad\subsubfloat{\includegraphics[width=0.05\textwidth]{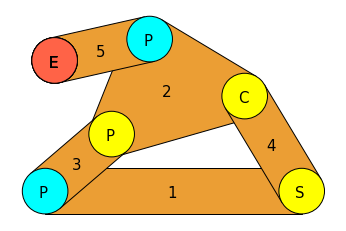}}{{\tiny 2D-M610}}
\qquad\subsubfloat{\includegraphics[width=0.05\textwidth]{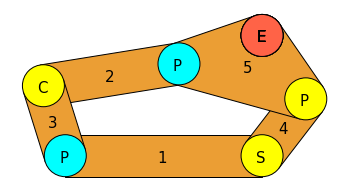}}{{\tiny 2D-M611}}
\qquad\subsubfloat{\includegraphics[width=0.05\textwidth]{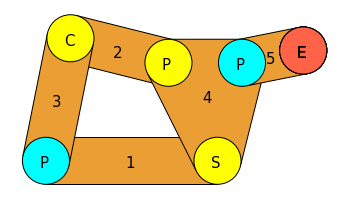}}{{\tiny 2D-M612}}
\qquad\subsubfloat{\includegraphics[width=0.05\textwidth]{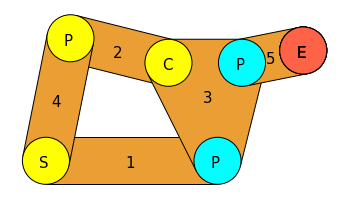}}{{\tiny 2D-M613}}
\qquad\subsubfloat{\includegraphics[width=0.05\textwidth]{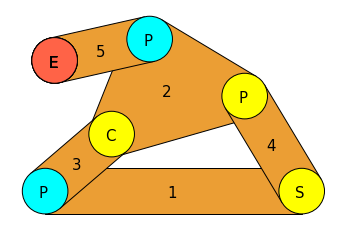}}{{\tiny 2D-M614}}
\qquad\subsubfloat{\includegraphics[width=0.05\textwidth]{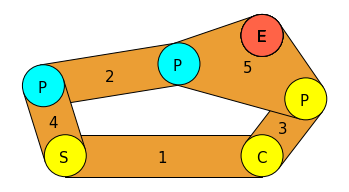}}{{\tiny 2D-M615}}
\qquad\subsubfloat{\includegraphics[width=0.05\textwidth]{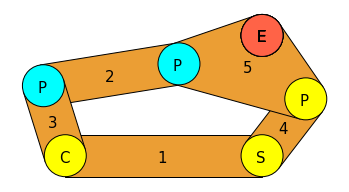}}{{\tiny 2D-M616}}
\qquad\subsubfloat{\includegraphics[width=0.05\textwidth]{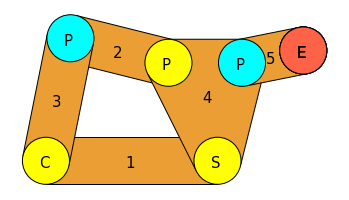}}{{\tiny 2D-M617}}
\qquad\subsubfloat{\includegraphics[width=0.05\textwidth]{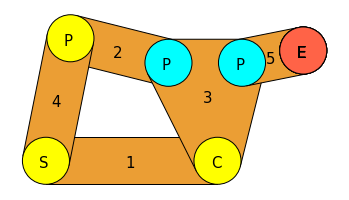}}{{\tiny 2D-M618}}
\qquad\subsubfloat{\includegraphics[width=0.05\textwidth]{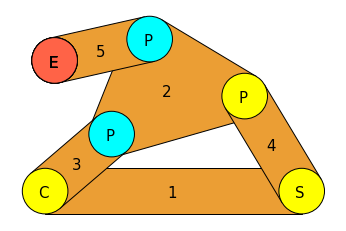}}{{\tiny 2D-M619}}
\qquad\subsubfloat{\includegraphics[width=0.05\textwidth]{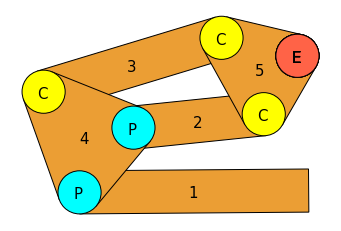}}{{\tiny 2D-M620}}
\qquad\subsubfloat{\includegraphics[width=0.05\textwidth]{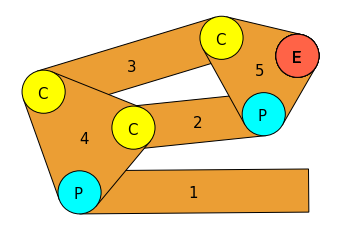}}{{\tiny 2D-M621}}
\qquad\subsubfloat{\includegraphics[width=0.05\textwidth]{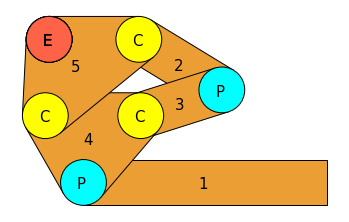}}{{\tiny 2D-M622}}
\qquad\subsubfloat{\includegraphics[width=0.05\textwidth]{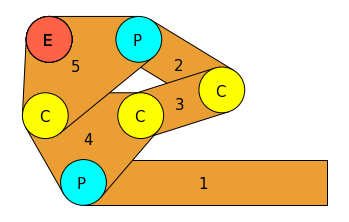}}{{\tiny 2D-M623}}
\qquad\subsubfloat{\includegraphics[width=0.05\textwidth]{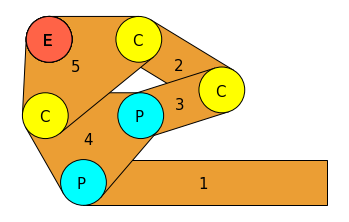}}{{\tiny 2D-M624}}
\qquad\subsubfloat{\includegraphics[width=0.05\textwidth]{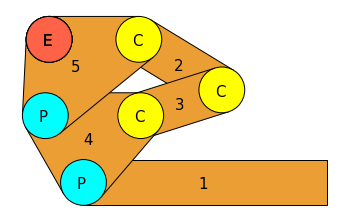}}{{\tiny 2D-M625}}
\qquad\subsubfloat{\includegraphics[width=0.05\textwidth]{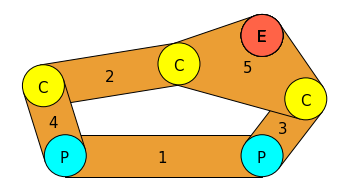}}{{\tiny 2D-M626}}
\qquad\subsubfloat{\includegraphics[width=0.05\textwidth]{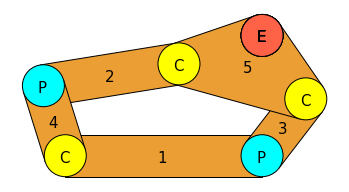}}{{\tiny 2D-M627}}
\qquad\subsubfloat{\includegraphics[width=0.05\textwidth]{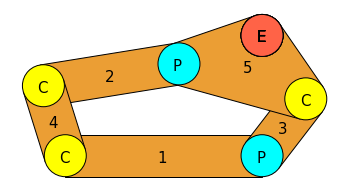}}{{\tiny 2D-M628}}
\qquad\subsubfloat{\includegraphics[width=0.05\textwidth]{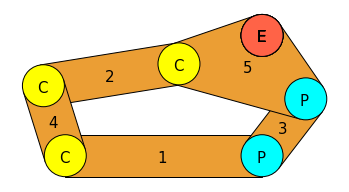}}{{\tiny 2D-M629}}
\qquad\subsubfloat{\includegraphics[width=0.05\textwidth]{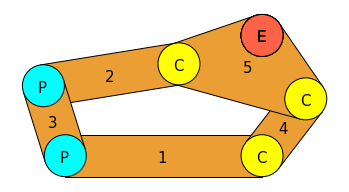}}{{\tiny 2D-M630}}
\qquad\subsubfloat{\includegraphics[width=0.05\textwidth]{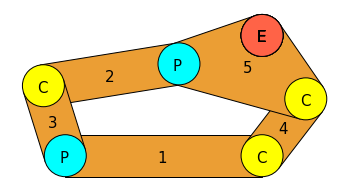}}{{\tiny 2D-M631}}
\qquad\subsubfloat{\includegraphics[width=0.05\textwidth]{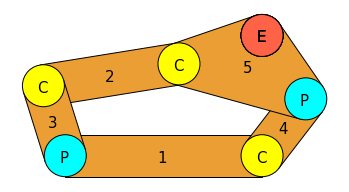}}{{\tiny 2D-M632}}
\qquad\subsubfloat{\includegraphics[width=0.05\textwidth]{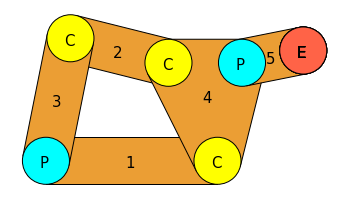}}{{\tiny 2D-M633}}
\qquad\subsubfloat{\includegraphics[width=0.05\textwidth]{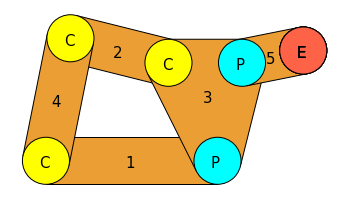}}{{\tiny 2D-M634}}
\qquad\subsubfloat{\includegraphics[width=0.05\textwidth]{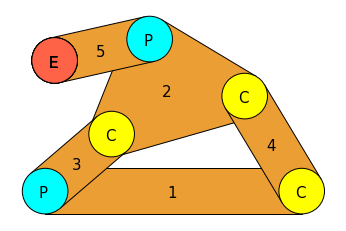}}{{\tiny 2D-M635}}
\qquad\subsubfloat{\includegraphics[width=0.05\textwidth]{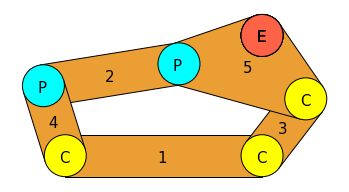}}{{\tiny 2D-M636}}
\qquad\subsubfloat{\includegraphics[width=0.05\textwidth]{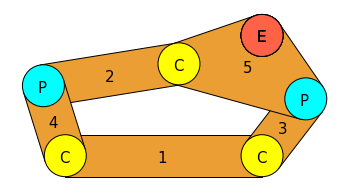}}{{\tiny 2D-M637}}
\qquad\subsubfloat{\includegraphics[width=0.05\textwidth]{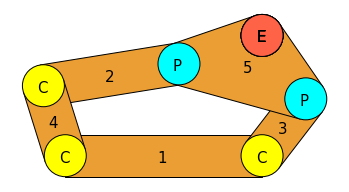}}{{\tiny 2D-M638}}
\qquad\subsubfloat{\includegraphics[width=0.05\textwidth]{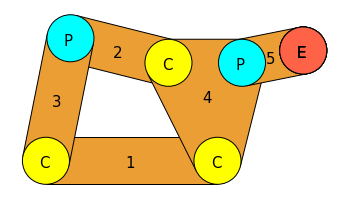}}{{\tiny 2D-M639}}
\qquad\subsubfloat{\includegraphics[width=0.05\textwidth]{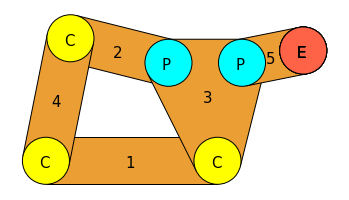}}{{\tiny 2D-M640}}
\qquad\subsubfloat{\includegraphics[width=0.05\textwidth]{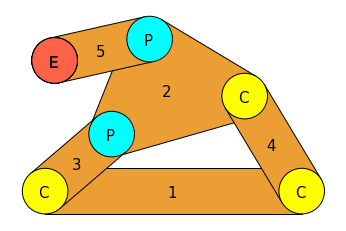}}{{\tiny 2D-M641}}
\qquad\subsubfloat{\includegraphics[width=0.05\textwidth]{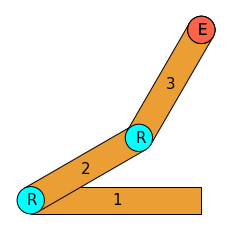}}{{\tiny 2D-M642}}
\qquad\subsubfloat{\includegraphics[width=0.05\textwidth]{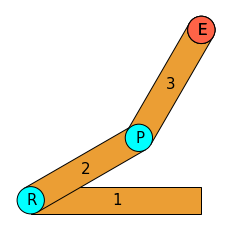}}{{\tiny 2D-M643}}
\qquad\subsubfloat{\includegraphics[width=0.05\textwidth]{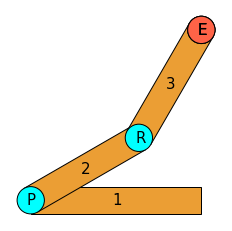}}{{\tiny 2D-M644}}
\qquad\subsubfloat{\includegraphics[width=0.05\textwidth]{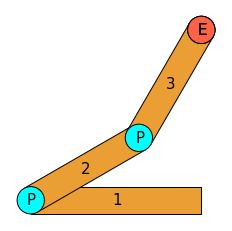}}{{\tiny 2D-M645}}

    \end{minipage}
  \end{subfigure}
  \caption{Schematic diagrams of 2-DOF Manipulators (Contd.)}
  \end{figure}

\begin{figure}[H]
\centering
\begin{subfigure}{\columnwidth}
  \begin{minipage}{\textwidth}\footnotesize
  \centering
\subsubfloat{\includegraphics[width=0.05\textwidth]{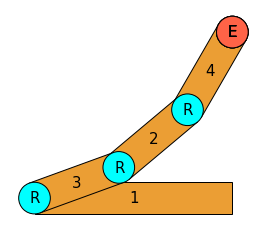}}{{\tiny 3D-M1}}
\qquad\subsubfloat{\includegraphics[width=0.05\textwidth]{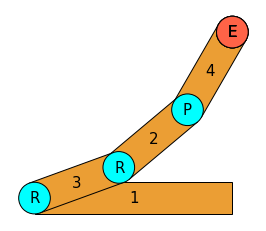}}{{\tiny 3D-M2}}
\qquad\subsubfloat{\includegraphics[width=0.05\textwidth]{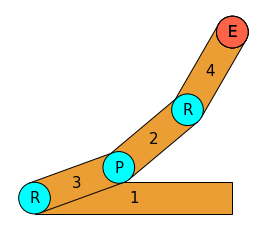}}{{\tiny 3D-M3}}
\qquad\subsubfloat{\includegraphics[width=0.05\textwidth]{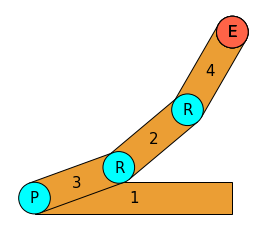}}{{\tiny 3D-M4}}
\qquad\subsubfloat{\includegraphics[width=0.05\textwidth]{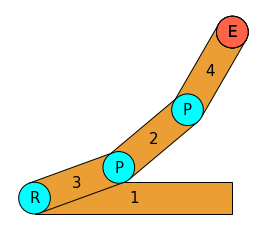}}{{\tiny 3D-M5}}
\qquad\subsubfloat{\includegraphics[width=0.05\textwidth]{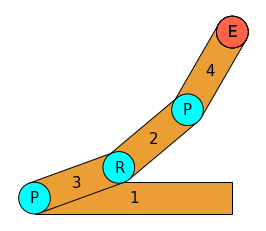}}{{\tiny 3D-M6}}
\qquad\subsubfloat{\includegraphics[width=0.05\textwidth]{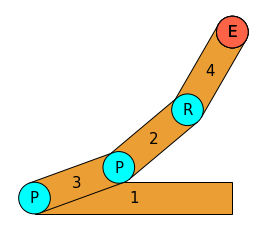}}{{\tiny 3D-M7}}
\qquad\subsubfloat{\includegraphics[width=0.05\textwidth]{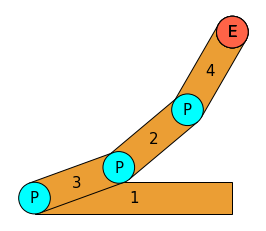}}{{\tiny 3D-M8}}

  \end{minipage}
\end{subfigure}
\caption{Schematic diagrams of 3-DOF Manipulators}
\end{figure}

\begin{figure}[H]
\centering
\begin{subfigure}{\columnwidth}
  \begin{minipage}{\textwidth}\footnotesize
  \centering
\subsubfloat{\includegraphics[width=0.05\textwidth]{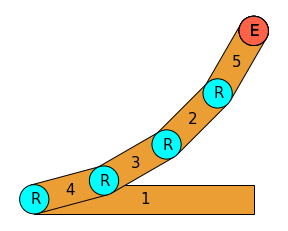}}{{\tiny 4D-M1}}
\qquad\subsubfloat{\includegraphics[width=0.05\textwidth]{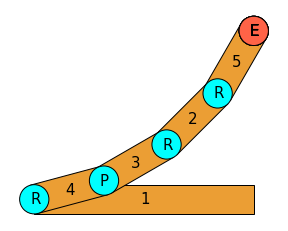}}{{\tiny 4D-M2}}
\qquad\subsubfloat{\includegraphics[width=0.05\textwidth]{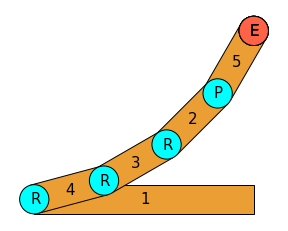}}{{\tiny 4D-M3}}
\qquad\subsubfloat{\includegraphics[width=0.05\textwidth]{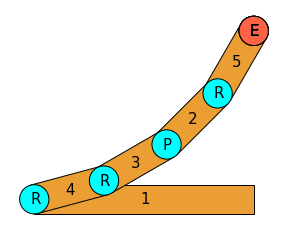}}{{\tiny 4D-M4}}
\qquad\subsubfloat{\includegraphics[width=0.05\textwidth]{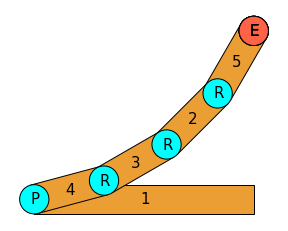}}{{\tiny 4D-M5}}
\qquad\subsubfloat{\includegraphics[width=0.05\textwidth]{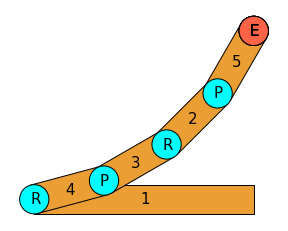}}{{\tiny 4D-M6}}
\qquad\subsubfloat{\includegraphics[width=0.05\textwidth]{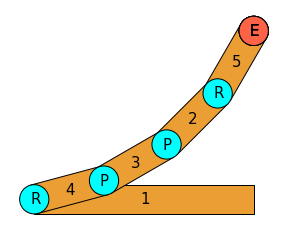}}{{\tiny 4D-M7}}
\qquad\subsubfloat{\includegraphics[width=0.05\textwidth]{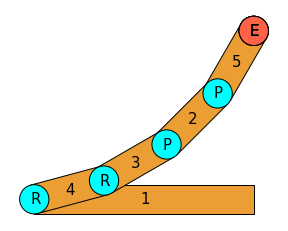}}{{\tiny 4D-M8}}
\qquad\subsubfloat{\includegraphics[width=0.05\textwidth]{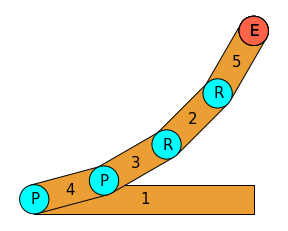}}{{\tiny 4D-M9}}
\qquad\subsubfloat{\includegraphics[width=0.05\textwidth]{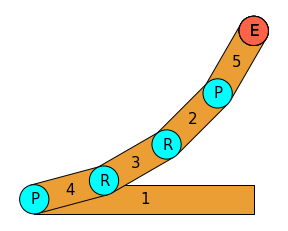}}{{\tiny 4D-M10}}
\qquad\subsubfloat{\includegraphics[width=0.05\textwidth]{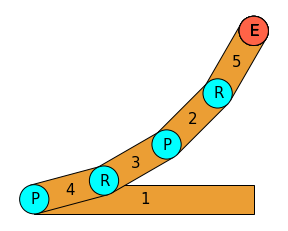}}{{\tiny 4D-M11}}
\qquad\subsubfloat{\includegraphics[width=0.05\textwidth]{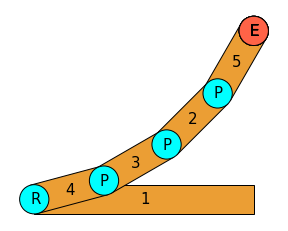}}{{\tiny 4D-M12}}
\qquad\subsubfloat{\includegraphics[width=0.05\textwidth]{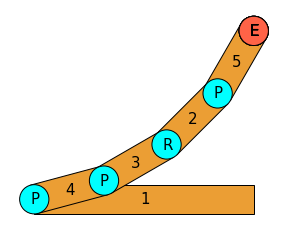}}{{\tiny 4D-M13}}
\qquad\subsubfloat{\includegraphics[width=0.05\textwidth]{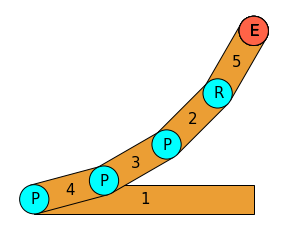}}{{\tiny 4D-M14}}
\qquad\subsubfloat{\includegraphics[width=0.05\textwidth]{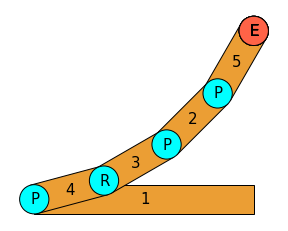}}{{\tiny 4D-M15}}

  \end{minipage}
\end{subfigure}
\caption{Schematic diagrams of 4-DOF Manipulators}
\end{figure}
