# Supplementary material for: Dimensional synthesis of spatial manipulators for velocity and force transmission for operation around a specified task point
Source: arXiv:2210.04446 source file (2022-10-10)
Supplement: Supplementary file 2 [file AppendixB.tex]

% Appendix Template

\chapter{Force-transformation matrix of five-link revolute-type parallel manipulator} % Main appendix title

\label{AppendixB} % Change X to a consecutive letter; for referencing this appendix elsewhere, use \ref{AppendixX}

\lhead{Appendix B. \emph{Force-transformation matrix of five-link revolute-type parallel manipulator}} % Change X to a consecutive letter; this is for the header on each page - perhaps a shortened title

\begin{figure}[hb]
  \centering
  \includegraphics[width=0.4\linewidth]{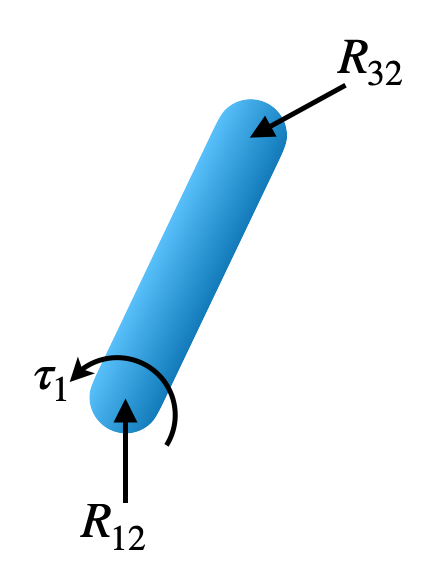}
  \caption{Freebody diagram of the second link}
  \label{fig8}
\end{figure}

The free-body diagram of the second link is shown in the figure \ref{fig8}. From the figure, we have
\[
\vec{R}_{12}+\vec{R}_{32}=0
\implies \vec{R}_{32} = -\vec{R}_{12}
\]
and
\[
\vec{\tau}_{1}-\vec{l}_2 \times \vec{R}_{32}=0
\implies \vec{\tau}_{1} = \vec{l}_2 \times \vec{R}_{12}
\]
\begin{align}
\therefore \tau_1=l_2 \left( R_{12y}\cos{\theta}_2 - R_{12x}\sin{\theta}_2 \right)
 \label{app2eq1}
\end{align}

\begin{figure}[hb]
  \centering
  \includegraphics[width=0.7\linewidth]{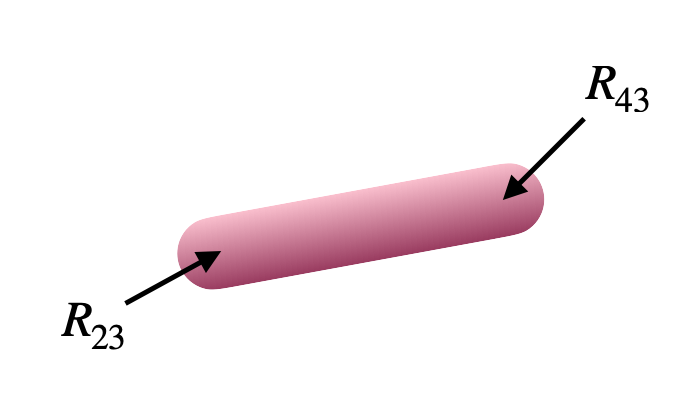}
  \caption{Freebody diagram of the third link}
  \label{fig9}
\end{figure}

The free-body diagram of the third link is shown in the figure \ref{fig9}. From the figure, we have
\[
\vec{R}_{23}+\vec{R}_{43}=0
\implies \vec{R}_{43} = -\vec{R}_{23} = \vec{R}_{32} = -\vec{R}_{12}
\]
and
\[
\vec{l}_3 \times \vec{R}_{43}=0
\implies \vec{l}_3 \times \vec{R}_{12} = 0
\]
\begin{align}
\therefore l_3 \left( R_{12y}\cos{\theta}_3 - R_{12x}\sin{\theta}_3 \right) = 0
 \label{app2eq2}
\end{align}

\begin{figure}[hb]
  \centering
  \includegraphics[width=1.0\linewidth]{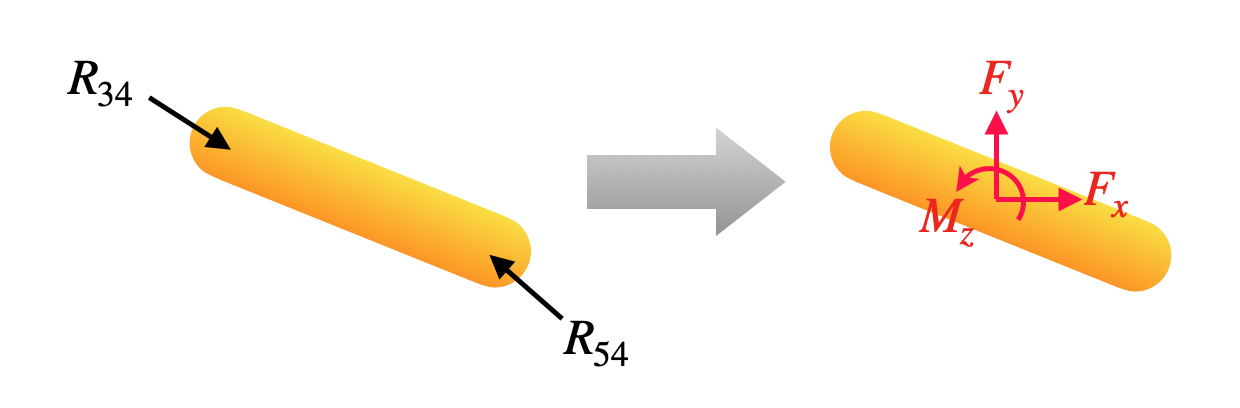}
  \caption{Freebody diagram of the fourth link}
  \label{fig10}
\end{figure}

The free-body diagram of the fourth link is shown in the figure \ref{fig10}. From the figure, we have
\[
\vec{R}_{34}+\vec{R}_{54}=\vec{F}
\implies \vec{R}_{54} = \vec{F} - \vec{R}_{34} = \vec{F} + \vec{R}_{43} = \vec{F} - \vec{R}_{12}
\]
and
\[
\vec{l}_4 \times \vec{R}_{54}=\frac{\vec{l}_4}{2} \times \vec{F} + \vec{M}
\implies \vec{l}_4 \times \left(\vec{F} - \vec{R}_{12}\right)=\frac{\vec{l}_4}{2} \times \vec{F} + \vec{M}
\]
\[
\implies \vec{M} - \frac{\vec{l}_4}{2} \times \vec{F} + \vec{l}_4 \times \vec{R}_{12} = 0
\]
\begin{align}
\therefore M_z - \frac{l_4}{2}\left(F_y\cos{\theta}_4-F_x\sin{\theta}_4\right)+l_4\left(R_{12y}\cos{\theta}_4-R_{12x}\sin{\theta}_4\right) = 0
 \label{app2eq3}
\end{align}

\begin{figure}[hb]
  \centering
  \includegraphics[width=0.4\linewidth]{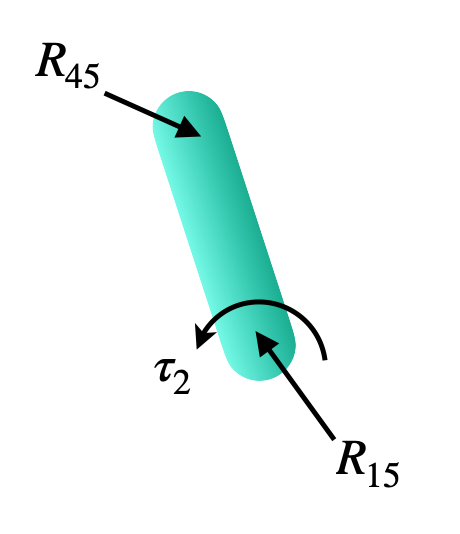}
  \caption{Freebody diagram of the fifth link}
  \label{fig11}
\end{figure}

The free-body diagram of the fifth link is shown in the figure \ref{fig11}. From the figure, we have
\[
\vec{R}_{45}+\vec{R}_{15}=0
\implies \vec{R}_{15} = -\vec{R}_{45} = \vec{R}_{54} = \vec{F} - \vec{R}_{12}
\]
and
\[
\vec{\tau}_2 + \vec{l}_5 \times \vec{R}_{15}=0
\implies \vec{\tau}_2 + \vec{l}_5 \times \left( \vec{F} - \vec{R}_{12} \right) = 0
\]
\[
\implies \vec{\tau}_2 = \vec{l}_5 \times \left( \vec{R}_{12} - \vec{F} \right) = 0
\]
\begin{align}
\therefore \tau_2 = l_5 \left[ \left(R_{12y}-F_y\right)\cos{\theta}_5 - \left(R_{12x}-F_x\right)\sin{\theta}_5 \right]
 \label{app2eq4}
\end{align}

From equation \ref{app2eq2} and equation \ref{app2eq3},
\[
\begin{bmatrix} -l_3 \sin{\theta}_3 & l_3 \cos{\theta}_3 \\ -l_4 \sin{\theta}_4 & l_4 \cos{\theta}_4 \end{bmatrix} \begin{Bmatrix} R_{12x} \\ R_{12y} \end{Bmatrix} = \begin{bmatrix} 0 & 0 & 0 \\ -\frac{l_4}{2}\sin{\theta}_4 & \frac{l_4}{2}\cos{\theta}_4 & -1 \end{bmatrix} \begin{Bmatrix} F_x \\ F_y \\ M_z \end{Bmatrix}
\]
\[
\Rightarrow \begin{Bmatrix} R_{12x} \\ R_{12y} \end{Bmatrix} = \begin{bmatrix} -l_3 \sin{\theta}_3 & l_3 \cos{\theta}_3 \\ -l_4 \sin{\theta}_4 & l_4 \cos{\theta}_4 \end{bmatrix}^{-1} \begin{bmatrix} 0 & 0 & 0 \\ -\frac{l_4}{2}\sin{\theta}_4 & \frac{l_4}{2}\cos{\theta}_4 & -1 \end{bmatrix} \begin{Bmatrix} F_x \\ F_y \\ M_z \end{Bmatrix}
\]
\[
\Rightarrow \begin{Bmatrix} R_{12x} \\ R_{12y} \end{Bmatrix} = \frac{1}{l_3l_4\sin{\left(\theta_4 - \theta_3\right)}}\begin{bmatrix} l_4 \cos{\theta}_4 & -l_3 \cos{\theta}_3 \\ l_4 \sin{\theta}_4 & -l_3 \sin{\theta}_3 \end{bmatrix} \begin{bmatrix} 0 & 0 & 0 \\ -\frac{l_4}{2}\sin{\theta}_4 & \frac{l_4}{2}\cos{\theta}_4 & -1 \end{bmatrix} \begin{Bmatrix} F_x \\ F_y \\ M_z \end{Bmatrix}
\]
\begin{align}
\Rightarrow \begin{Bmatrix} R_{12x} \\ R_{12y} \end{Bmatrix} = \begin{bmatrix} \frac{\cos{\theta}_3\sin{\theta}_4}{2\sin{\left(\theta_4 - \theta_3\right)}} & -\frac{\cos{\theta}_3\cos{\theta}_4}{2\sin{\left(\theta_4 - \theta_3\right)}} & \frac{\cos{\theta}_3}{l_4\sin{\left(\theta_4 - \theta_3\right)}} \\ \frac{\sin{\theta}_3\sin{\theta}_4}{2\sin{\left(\theta_4 - \theta_3\right)}} & -\frac{\sin{\theta}_3\cos{\theta}_4}{2\sin{\left(\theta_4 - \theta_3\right)}} & \frac{\sin{\theta}_3}{l_4\sin{\left(\theta_4 - \theta_3\right)}} \end{bmatrix} \begin{Bmatrix} F_x \\ F_y \\ M_z \end{Bmatrix}
 \label{app2eq5}
\end{align}

From equation \ref{app2eq1} and equation \ref{app2eq4},
\[
\Rightarrow \begin{Bmatrix} \tau_1 \\ \tau_2 \end{Bmatrix} = \begin{bmatrix} -l_2\sin{\theta}_2 & l_2\cos{\theta}_2 \\ -l_5\sin{\theta}_5 & l_5\cos{\theta}_5 \end{bmatrix} \begin{Bmatrix} R_{12x} \\ R_{12y} \end{Bmatrix} + \begin{bmatrix} 0 & 0 & 0 \\ l_5\sin{\theta}_5 & -l_5\cos{\theta}_5 & 0 \end{bmatrix} \begin{Bmatrix} F_x \\ F_y \\ M_z \end{Bmatrix}
\]
By using equation \ref{app2eq5},
\newline
\resizebox{\textwidth}{!}{$\Rightarrow \begin{Bmatrix} \tau_1 \\ \tau_2 \end{Bmatrix} = \begin{bmatrix} -l_2\sin{\theta}_2 & l_2\cos{\theta}_2 \\ -l_5\sin{\theta}_5 & l_5\cos{\theta}_5 \end{bmatrix} \begin{bmatrix} \frac{\cos{\theta}_3\sin{\theta}_4}{2\sin{\left(\theta_4 - \theta_3\right)}} & -\frac{\cos{\theta}_3\cos{\theta}_4}{2\sin{\left(\theta_4 - \theta_3\right)}} & \frac{\cos{\theta}_3}{l_4\sin{\left(\theta_4 - \theta_3\right)}} \\ \frac{\sin{\theta}_3\sin{\theta}_4}{2\sin{\left(\theta_4 - \theta_3\right)}} & -\frac{\sin{\theta}_3\cos{\theta}_4}{2\sin{\left(\theta_4 - \theta_3\right)}} & \frac{\sin{\theta}_3}{l_4\sin{\left(\theta_4 - \theta_3\right)}} \end{bmatrix} \begin{Bmatrix} F_x \\ F_y \\ M_z \end{Bmatrix} + \begin{bmatrix} 0 & 0 & 0 \\ l_5\sin{\theta}_5 & -l_5\cos{\theta}_5 & 0 \end{bmatrix} \begin{Bmatrix} F_x \\ F_y \\ M_z \end{Bmatrix}$}
\newline
\resizebox{\textwidth}{!}{$\Rightarrow \begin{Bmatrix} \tau_1 \\ \tau_2 \end{Bmatrix} = \begin{bmatrix} \frac{l_{2} \sin{\left(\theta_2 \right)} \sin{\left(\theta_4 \right)} \cos{\left(\theta_3 \right)}}{2 \sin{\left(\theta_3 - \theta_4 \right)}} - \frac{l_{2} \sin{\left(\theta_3 \right)} \sin{\left(\theta_4 \right)} \cos{\left(\theta_2 \right)}}{2 \sin{\left(\theta_3 - \theta_4 \right)}} & - \frac{l_{2} \sin{\left(\theta_2 \right)} \cos{\left(\theta_3 \right)} \cos{\left(\theta_4 \right)}}{2 \sin{\left(\theta_3 - \theta_4 \right)}} + \frac{l_{2} \sin{\left(\theta_3 \right)} \cos{\left(\theta_2 \right)} \cos{\left(\theta_4 \right)}}{2 \sin{\left(\theta_3 - \theta_4 \right)}} & \frac{l_{2} \sin{\left(\theta_2 \right)} \cos{\left(\theta_3 \right)}}{l_{4} \sin{\left(\theta_3 - \theta_4 \right)}} - \frac{l_{2} \sin{\left(\theta_3 \right)} \cos{\left(\theta_2 \right)}}{l_{4} \sin{\left(\theta_3 - \theta_4 \right)}}\\l_{5} \left(\frac{\sin{\left(\theta_4 \right)} \cos{\left(\theta_3 \right)}}{2 \sin{\left(\theta_3 - \theta_4 \right)}} + 1\right) \sin{\left(\theta_5 \right)} - \frac{l_{5} \sin{\left(\theta_3 \right)} \sin{\left(\theta_4 \right)} \cos{\left(\theta_5 \right)}}{2 \sin{\left(\theta_3 - \theta_4 \right)}} & - l_{5} \left(- \frac{\sin{\left(\theta_3 \right)} \cos{\left(\theta_4 \right)}}{2 \sin{\left(\theta_3 - \theta_4 \right)}} + 1\right) \cos{\left(\theta_5 \right)} - \frac{l_{5} \sin{\left(\theta_5 \right)} \cos{\left(\theta_3 \right)} \cos{\left(\theta_4 \right)}}{2 \sin{\left(\theta_3 - \theta_4 \right)}} & - \frac{l_{5} \sin{\left(\theta_3 \right)} \cos{\left(\theta_5 \right)}}{l_{4} \sin{\left(\theta_3 - \theta_4 \right)}} + \frac{l_{5} \sin{\left(\theta_5 \right)} \cos{\left(\theta_3 \right)}}{l_{4} \sin{\left(\theta_3 - \theta_4 \right)}} \end{bmatrix} \begin{Bmatrix} F_x \\ F_y \\ M_z \end{Bmatrix}$}
\newline
\resizebox{\textwidth}{!}{$\Rightarrow \begin{Bmatrix} \tau_1 \\ \tau_2 \end{Bmatrix} = \begin{bmatrix} \frac{l_{2} \sin{\left(\theta_4 \right)} \sin{\left(\theta_2 - \theta_3 \right)}}{2 \sin{\left(\theta_3 - \theta_4 \right)}} & - \frac{l_{2} \sin{\left(\theta_2 - \theta_3 \right)} \cos{\left(\theta_4 \right)}}{2 \sin{\left(\theta_3 - \theta_4 \right)}} & \frac{l_{2} \sin{\left(\theta_2 - \theta_3 \right)}}{l_{4} \sin{\left(\theta_3 - \theta_4 \right)}}\\\frac{l_{5} \left(\frac{\cos{\left(- \theta_3 + \theta_4 + \theta_5 \right)}}{2} - \cos{\left(\theta_3 - \theta_4 + \theta_5 \right)} + \frac{\cos{\left(\theta_3 + \theta_4 - \theta_5 \right)}}{2}\right)}{2 \sin{\left(\theta_3 - \theta_4 \right)}} & \frac{l_{5} \left(\frac{\sin{\left(- \theta_3 + \theta_4 + \theta_5 \right)}}{2} - \sin{\left(\theta_3 - \theta_4 + \theta_5 \right)} + \frac{\sin{\left(\theta_3 + \theta_4 - \theta_5 \right)}}{2}\right)}{2 \sin{\left(\theta_3 - \theta_4 \right)}} & - \frac{l_{5} \sin{\left(\theta_3 - \theta_5 \right)}}{l_{4} \sin{\left(\theta_3 - \theta_4 \right)}} \end{bmatrix} \begin{Bmatrix} F_x \\ F_y \\ M_z \end{Bmatrix}$}
\[
\Rightarrow \begin{Bmatrix} \tau_1 \\ \tau_2 \end{Bmatrix} = \left[J\right]^T \begin{Bmatrix} F_x \\ F_y \\ M_z \end{Bmatrix}
\]
where
\newline
\resizebox{\textwidth}{!}{$\left[J\right] = \begin{bmatrix} \frac{l_{2} \sin{\left(\theta_4 \right)} \sin{\left(\theta_2 - \theta_3 \right)}}{2 \sin{\left(\theta_3 - \theta_4 \right)}} & \frac{l_{5} \left(\frac{\cos{\left(- \theta_3 + \theta_4 + \theta_5 \right)}}{2} - \cos{\left(\theta_3 - \theta_4 + \theta_5 \right)} + \frac{\cos{\left(\theta_3 + \theta_4 - \theta_5 \right)}}{2}\right)}{2 \sin{\left(\theta_3 - \theta_4 \right)}}\\- \frac{l_{2} \sin{\left(\theta_2 - \theta_3 \right)} \cos{\left(\theta_4 \right)}}{2 \sin{\left(\theta_3 - \theta_4 \right)}} & \frac{l_{5} \left(\frac{\sin{\left(- \theta_3 + \theta_4 + \theta_5 \right)}}{2} - \sin{\left(\theta_3 - \theta_4 + \theta_5 \right)} + \frac{\sin{\left(\theta_3 + \theta_4 - \theta_5 \right)}}{2}\right)}{2 \sin{\left(\theta_3 - \theta_4 \right)}}\\\frac{l_{2} \sin{\left(\theta_2 - \theta_3 \right)}}{l_{4} \sin{\left(\theta_3 - \theta_4 \right)}} & - \frac{l_{5} \sin{\left(\theta_3 - \theta_5 \right)}}{l_{4} \sin{\left(\theta_3 - \theta_4 \right)}} \end{bmatrix}$}
