# Supplementary material for: Dimensional synthesis of spatial manipulators for velocity and force transmission for operation around a specified task point
Source: arXiv:2210.04446 source file (2022-10-10)
Supplement: Supplementary file 3 [file AppendixD.tex]

% Appendix Template

%\chapter{Results of optimisation for manipulators of of DOF 2} % Main appendix title

\label{AppendixD} % Change X to a consecutive letter; for referencing this appendix elsewhere, use \ref{AppendixX}

%\lhead{Appendix D. \emph{Results of optimisation for manipulators of of DOF 2}} % Change X to a consecutive letter; this is for the header on each page - perhaps a shortened title
%\subsection{Class 1} \label{appendix_five_1_1}
\section*{Appendix B}
\subsection*{Results of optimisation}
\begingroup\makeatletter\def\f@size{4}\check@mathfonts
\subsubsection*{For manipulators of DOF 1}

{\tiny 1D-M1:}   $\hat{n}_{13}=0.0\hat{i}+0.0\hat{j}+1.0\hat{k}$,\;\;\;$\hat{n}_{14}=0.02\hat{i}-0.52\hat{j}+0.85\hat{k}$,\;\;\;$\hat{n}_{23}=0.75\hat{i}-0.51\hat{j}+0.42\hat{k}$,\;\;\;$\vec{r}_{13}=10.0\hat{i}+0.0\hat{j}+0.53\hat{k}$,\;\;\;$\vec{r}_{14}=10.0\hat{i}+0.0\hat{j}+10.0\hat{k}$,\;\;\;$\vec{r}_{23}=0.0\hat{i}+0.0\hat{j}+0.0\hat{k}$,\;\;\;$\vec{r}_{24}=10.0\hat{i}+10.0\hat{j}+10.0\hat{k}$.

{\tiny 1D-M2:}   $\hat{n}_{13}=0.58\hat{i}+0.58\hat{j}-0.58\hat{k}$,\;\;\;$\hat{n}_{14}=0.0\hat{i}+0.77\hat{j}+0.63\hat{k}$,\;\;\;$\hat{n}_{24}=0.29\hat{i}+0.95\hat{j}-0.09\hat{k}$,\;\;\;$\vec{r}_{13}=0.0\hat{i}+10.0\hat{j}+0.0\hat{k}$,\;\;\;$\vec{r}_{14}=0.0\hat{i}+0.0\hat{j}+10.0\hat{k}$,\;\;\;$\vec{r}_{23}=10.0\hat{i}+0.0\hat{j}+0.0\hat{k}$,\;\;\;$\vec{r}_{24}=0.0\hat{i}+10.0\hat{j}+10.0\hat{k}$.

{\tiny 1D-M3:}   $\hat{n}_{13}=-0.03\hat{i}-0.71\hat{j}-0.71\hat{k}$,\;\;\;$\hat{n}_{14}=0.71\hat{i}-0.68\hat{j}-0.18\hat{k}$,\;\;\;$\hat{n}_{23}=-0.82\hat{i}-0.37\hat{j}+0.44\hat{k}$,\;\;\;$\vec{r}_{13}=10.0\hat{i}+10.0\hat{j}+0.0\hat{k}$,\;\;\;$\vec{r}_{14}=0.0\hat{i}+0.0\hat{j}+0.0\hat{k}$,\;\;\;$\vec{r}_{23}=10.0\hat{i}+0.0\hat{j}+0.0\hat{k}$,\;\;\;$\vec{r}_{24}=0.0\hat{i}+10.0\hat{j}+10.0\hat{k}$.

{\tiny 1D-M4:}   $\hat{n}_{13}=-0.0\hat{i}+0.0\hat{j}-1.0\hat{k}$,\;\;\;$\hat{n}_{14}=-0.58\hat{i}-0.8\hat{j}+0.15\hat{k}$,\;\;\;$\hat{n}_{24}=0.53\hat{i}+0.6\hat{j}+0.6\hat{k}$,\;\;\;$\vec{r}_{13}=10.0\hat{i}+0.0\hat{j}+10.0\hat{k}$,\;\;\;$\vec{r}_{14}=10.0\hat{i}+0.0\hat{j}+10.0\hat{k}$,\;\;\;$\vec{r}_{23}=0.0\hat{i}+10.0\hat{j}+10.0\hat{k}$,\;\;\;$\vec{r}_{24}=10.0\hat{i}+10.0\hat{j}+0.0\hat{k}$.

{\tiny 1D-M5:}   $\hat{n}_{13}=-0.08\hat{i}+0.46\hat{j}+0.89\hat{k}$,\;\;\;$\hat{n}_{23}=0.61\hat{i}-0.33\hat{j}+0.72\hat{k}$,\;\;\;$\hat{n}_{24}=0.79\hat{i}-0.58\hat{j}-0.19\hat{k}$,\;\;\;$\vec{r}_{13}=0.0\hat{i}+10.0\hat{j}+10.0\hat{k}$,\;\;\;$\vec{r}_{14}=10.0\hat{i}+10.0\hat{j}+0.0\hat{k}$,\;\;\;$\vec{r}_{23}=10.0\hat{i}+0.0\hat{j}+10.0\hat{k}$,\;\;\;$\vec{r}_{24}=0.0\hat{i}+0.0\hat{j}+0.0\hat{k}$.

{\tiny 1D-M6:}   $\hat{n}_{13}=0.0\hat{i}+0.37\hat{j}+0.93\hat{k}$,\;\;\;$\hat{n}_{23}=0.33\hat{i}-0.66\hat{j}+0.67\hat{k}$,\;\;\;$\hat{n}_{24}=0.84\hat{i}-0.53\hat{j}-0.09\hat{k}$,\;\;\;$\vec{r}_{13}=0.0\hat{i}+10.0\hat{j}+10.0\hat{k}$,\;\;\;$\vec{r}_{14}=10.0\hat{i}+10.0\hat{j}+10.0\hat{k}$,\;\;\;$\vec{r}_{23}=0.0\hat{i}+0.0\hat{j}+0.0\hat{k}$,\;\;\;$\vec{r}_{24}=10.0\hat{i}+10.0\hat{j}+0.0\hat{k}$.

{\tiny 1D-M7:}   $\hat{n}_{13}=-0.21\hat{i}-0.95\hat{j}-0.24\hat{k}$,\;\;\;$\hat{n}_{14}=0.41\hat{i}-0.48\hat{j}-0.78\hat{k}$,\;\;\;$\hat{n}_{23}=-0.17\hat{i}-0.96\hat{j}+0.24\hat{k}$,\;\;\;$\vec{r}_{13}=5.38\hat{i}+6.86\hat{j}+4.63\hat{k}$,\;\;\;$\vec{r}_{14}=0.0\hat{i}+10.0\hat{j}+10.0\hat{k}$,\;\;\;$\vec{r}_{23}=6.61\hat{i}+5.26\hat{j}+5.64\hat{k}$,\;\;\;$\vec{r}_{24}=5.08\hat{i}+5.88\hat{j}+3.64\hat{k}$.

{\tiny 1D-M8:}   $\hat{n}_{13}=-0.72\hat{i}-0.39\hat{j}+0.57\hat{k}$,\;\;\;$\hat{n}_{14}=0.31\hat{i}-0.9\hat{j}+0.29\hat{k}$,\;\;\;$\hat{n}_{24}=-0.04\hat{i}-1.0\hat{j}+0.06\hat{k}$,\;\;\;$\vec{r}_{13}=6.43\hat{i}+4.57\hat{j}+5.96\hat{k}$,\;\;\;$\vec{r}_{14}=0.0\hat{i}+0.0\hat{j}+0.0\hat{k}$,\;\;\;$\vec{r}_{23}=3.69\hat{i}+6.29\hat{j}+5.5\hat{k}$,\;\;\;$\vec{r}_{24}=5.32\hat{i}+3.65\hat{j}+6.36\hat{k}$.

{\tiny 1D-M9:}   $\hat{n}_{13}=0.44\hat{i}+0.64\hat{j}+0.63\hat{k}$,\;\;\;$\hat{n}_{23}=0.15\hat{i}+0.42\hat{j}-0.9\hat{k}$,\;\;\;$\hat{n}_{24}=0.5\hat{i}+0.61\hat{j}-0.62\hat{k}$,\;\;\;$\vec{r}_{13}=0.0\hat{i}+10.0\hat{j}+10.0\hat{k}$,\;\;\;$\vec{r}_{14}=10.0\hat{i}+0.0\hat{j}+10.0\hat{k}$,\;\;\;$\vec{r}_{23}=10.0\hat{i}+10.0\hat{j}+10.0\hat{k}$,\;\;\;$\vec{r}_{24}=0.0\hat{i}+0.0\hat{j}+0.0\hat{k}$.

{\tiny 1D-M10:}\label{result_1_10}   $\hat{n}_{14}=0.0\hat{i}+0.0\hat{j}-1.0\hat{k}$,\;\;\;$\hat{n}_{23}=0.04\hat{i}-0.71\hat{j}+0.7\hat{k}$,\;\;\;$\hat{n}_{24}=-0.84\hat{i}-0.49\hat{j}-0.25\hat{k}$,\;\;\;$\vec{r}_{13}=3.76\hat{i}+5.51\hat{j}+5.34\hat{k}$,\;\;\;$\vec{r}_{14}=10.0\hat{i}+0.0\hat{j}+1.6\hat{k}$,\;\;\;$\vec{r}_{23}=4.11\hat{i}+6.4\hat{j}+4.81\hat{k}$,\;\;\;$\vec{r}_{24}=4.67\hat{i}+3.62\hat{j}+5.9\hat{k}$.

{\tiny 1D-M11:}   $\hat{n}_{14}=0.16\hat{i}-0.66\hat{j}+0.74\hat{k}$,\;\;\;$\hat{n}_{23}=0.89\hat{i}-0.47\hat{j}-0.02\hat{k}$,\;\;\;$\hat{n}_{24}=-0.96\hat{i}-0.28\hat{j}-0.02\hat{k}$,\;\;\;$\vec{r}_{13}=2.15\hat{i}+6.75\hat{j}+2.1\hat{k}$,\;\;\;$\vec{r}_{14}=10.0\hat{i}+10.0\hat{j}+10.0\hat{k}$,\;\;\;$\vec{r}_{23}=1.36\hat{i}+8.7\hat{j}+7.55\hat{k}$,\;\;\;$\vec{r}_{24}=4.88\hat{i}+4.39\hat{j}+4.5\hat{k}$.

{\tiny 1D-M12:}   $\hat{n}_{14}=-0.0\hat{i}+0.0\hat{j}+1.0\hat{k}$,\;\;\;$\hat{n}_{23}=0.0\hat{i}+0.76\hat{j}-0.65\hat{k}$,\;\;\;$\hat{n}_{24}=0.21\hat{i}-0.79\hat{j}-0.58\hat{k}$,\;\;\;$\vec{r}_{13}=0.0\hat{i}+0.0\hat{j}+10.0\hat{k}$,\;\;\;$\vec{r}_{14}=0.0\hat{i}+10.0\hat{j}+2.63\hat{k}$,\;\;\;$\vec{r}_{23}=10.0\hat{i}+10.0\hat{j}+10.0\hat{k}$,\;\;\;$\vec{r}_{24}=10.0\hat{i}+10.0\hat{j}+0.0\hat{k}$.

{\tiny 1D-M13:}   $\hat{n}_{12}=-0.82\hat{i}-0.54\hat{j}+0.19\hat{k}$,\;\;\;$\hat{n}_{13}=0.82\hat{i}+0.0\hat{j}-0.57\hat{k}$,\;\;\;$\hat{n}_{24}=0.03\hat{i}-0.82\hat{j}-0.57\hat{k}$,\;\;\;$\vec{r}_{12}=10.0\hat{i}+0.0\hat{j}+10.0\hat{k}$,\;\;\;$\vec{r}_{13}=0.0\hat{i}+0.0\hat{j}+0.0\hat{k}$,\;\;\;$\vec{r}_{24}=0.0\hat{i}+10.0\hat{j}+10.0\hat{k}$,\;\;\;$\vec{r}_{34}=10.0\hat{i}+0.0\hat{j}+0.0\hat{k}$.

{\tiny 1D-M14:}   $\hat{n}_{12}=0.59\hat{i}-0.79\hat{j}-0.17\hat{k}$,\;\;\;$\hat{n}_{13}=0.55\hat{i}+0.02\hat{j}+0.84\hat{k}$,\;\;\;$\hat{n}_{24}=0.58\hat{i}-0.57\hat{j}-0.59\hat{k}$,\;\;\;$\vec{r}_{12}=0.0\hat{i}+0.0\hat{j}+10.0\hat{k}$,\;\;\;$\vec{r}_{13}=0.0\hat{i}+0.0\hat{j}+10.0\hat{k}$,\;\;\;$\vec{r}_{24}=10.0\hat{i}+0.0\hat{j}+0.0\hat{k}$,\;\;\;$\vec{r}_{34}=10.0\hat{i}+10.0\hat{j}+10.0\hat{k}$.

{\tiny 1D-M15:}   $\hat{n}_{12}=0.0\hat{i}+0.71\hat{j}-0.71\hat{k}$,\;\;\;$\hat{n}_{13}=0.88\hat{i}-0.37\hat{j}-0.3\hat{k}$,\;\;\;$\hat{n}_{34}=-0.0\hat{i}+0.69\hat{j}-0.73\hat{k}$,\;\;\;$\vec{r}_{12}=0.0\hat{i}+10.0\hat{j}+0.0\hat{k}$,\;\;\;$\vec{r}_{13}=0.0\hat{i}+0.0\hat{j}+0.0\hat{k}$,\;\;\;$\vec{r}_{24}=10.0\hat{i}+10.0\hat{j}+10.0\hat{k}$,\;\;\;$\vec{r}_{34}=10.0\hat{i}+0.0\hat{j}+10.0\hat{k}$.

{\tiny 1D-M16:}   $\hat{n}_{12}=0.0\hat{i}+0.0\hat{j}-1.0\hat{k}$,\;\;\;$\hat{n}_{24}=-0.58\hat{i}+0.58\hat{j}+0.58\hat{k}$,\;\;\;$\hat{n}_{34}=-0.0\hat{i}+0.0\hat{j}-1.0\hat{k}$,\;\;\;$\vec{r}_{12}=10.0\hat{i}+10.0\hat{j}+0.0\hat{k}$,\;\;\;$\vec{r}_{13}=0.0\hat{i}+0.0\hat{j}+0.0\hat{k}$,\;\;\;$\vec{r}_{24}=0.0\hat{i}+10.0\hat{j}+10.0\hat{k}$,\;\;\;$\vec{r}_{34}=10.0\hat{i}+10.0\hat{j}+0.45\hat{k}$.

{\tiny 1D-M17:}   $\hat{n}_{12}=0.47\hat{i}-0.44\hat{j}+0.77\hat{k}$,\;\;\;$\hat{n}_{24}=0.11\hat{i}+0.39\hat{j}+0.92\hat{k}$,\;\;\;$\hat{n}_{34}=0.69\hat{i}-0.19\hat{j}-0.69\hat{k}$,\;\;\;$\vec{r}_{12}=0.0\hat{i}+10.0\hat{j}+0.0\hat{k}$,\;\;\;$\vec{r}_{13}=0.0\hat{i}+10.0\hat{j}+10.0\hat{k}$,\;\;\;$\vec{r}_{24}=10.0\hat{i}+10.0\hat{j}+0.0\hat{k}$,\;\;\;$\vec{r}_{34}=0.0\hat{i}+0.0\hat{j}+0.0\hat{k}$.

{\tiny 1D-M18:}   $\hat{n}_{12}=0.08\hat{i}-0.58\hat{j}+0.81\hat{k}$,\;\;\;$\hat{n}_{24}=0.45\hat{i}-0.53\hat{j}+0.72\hat{k}$,\;\;\;$\hat{n}_{34}=0.39\hat{i}-0.82\hat{j}-0.42\hat{k}$,\;\;\;$\vec{r}_{12}=10.0\hat{i}+10.0\hat{j}+10.0\hat{k}$,\;\;\;$\vec{r}_{13}=0.0\hat{i}+0.0\hat{j}+10.0\hat{k}$,\;\;\;$\vec{r}_{24}=0.0\hat{i}+10.0\hat{j}+0.0\hat{k}$,\;\;\;$\vec{r}_{34}=10.0\hat{i}+10.0\hat{j}+0.0\hat{k}$.

{\tiny 1D-M19:}   $\hat{n}_{13}=0.58\hat{i}+0.58\hat{j}+0.58\hat{k}$,\;\;\;$\hat{n}_{14}=-0.63\hat{i}-0.77\hat{j}-0.08\hat{k}$,\;\;\;$\vec{r}_{13}=10.0\hat{i}+10.0\hat{j}+0.0\hat{k}$,\;\;\;$\vec{r}_{14}=0.0\hat{i}+10.0\hat{j}+0.0\hat{k}$,\;\;\;$\vec{r}_{23}=0.0\hat{i}+10.0\hat{j}+10.0\hat{k}$,\;\;\;$\vec{r}_{24}=10.0\hat{i}+0.0\hat{j}+10.0\hat{k}$.

{\tiny 1D-M20:}   $\hat{n}_{14}=-0.62\hat{i}+0.73\hat{j}-0.29\hat{k}$,\;\;\;$\hat{n}_{24}=0.59\hat{i}-0.56\hat{j}+0.58\hat{k}$,\;\;\;$\vec{r}_{13}=4.05\hat{i}+6.66\hat{j}+3.38\hat{k}$,\;\;\;$\vec{r}_{14}=10.0\hat{i}+10.0\hat{j}+10.0\hat{k}$,\;\;\;$\vec{r}_{23}=4.38\hat{i}+5.09\hat{j}+3.57\hat{k}$,\;\;\;$\vec{r}_{24}=6.45\hat{i}+6.22\hat{j}+5.3\hat{k}$.

{\tiny 1D-M21:}   $\hat{n}_{12}=0.78\hat{i}-0.25\hat{j}-0.58\hat{k}$,\;\;\;$\hat{n}_{24}=-0.0\hat{i}+0.71\hat{j}-0.71\hat{k}$,\;\;\;$\vec{r}_{12}=10.0\hat{i}+10.0\hat{j}+10.0\hat{k}$,\;\;\;$\vec{r}_{13}=10.0\hat{i}+10.0\hat{j}+10.0\hat{k}$,\;\;\;$\vec{r}_{24}=10.0\hat{i}+0.0\hat{j}+10.0\hat{k}$,\;\;\;$\vec{r}_{34}=0.0\hat{i}+0.0\hat{j}+0.0\hat{k}$.

{\tiny 1D-M22:}   $\hat{n}_{13}=0.58\hat{i}+0.58\hat{j}+0.58\hat{k}$,\;\;\;$\hat{n}_{14}=0.0\hat{i}+1.0\hat{j}-0.0\hat{k}$,\;\;\;$\hat{n}_{23}=0.0\hat{i}+0.0\hat{j}+1.0\hat{k}$,\;\;\;$\vec{r}_{13}=10.0\hat{i}+10.0\hat{j}+0.0\hat{k}$,\;\;\;$\vec{r}_{23}=0.0\hat{i}+10.0\hat{j}+5.3\hat{k}$,\;\;\;$\vec{r}_{24}=10.0\hat{i}+0.0\hat{j}+10.0\hat{k}$.

{\tiny 1D-M23:}   $\hat{n}_{13}=0.77\hat{i}+0.0\hat{j}-0.64\hat{k}$,\;\;\;$\hat{n}_{14}=0.0\hat{i}+0.0\hat{j}-1.0\hat{k}$,\;\;\;$\hat{n}_{24}=-0.0\hat{i}+0.92\hat{j}-0.38\hat{k}$,\;\;\;$\vec{r}_{13}=10.0\hat{i}+0.0\hat{j}+0.0\hat{k}$,\;\;\;$\vec{r}_{23}=0.0\hat{i}+0.0\hat{j}+0.0\hat{k}$,\;\;\;$\vec{r}_{24}=10.0\hat{i}+10.0\hat{j}+10.0\hat{k}$.

{\tiny 1D-M24:}   $\hat{n}_{13}=0.0\hat{i}+0.71\hat{j}-0.71\hat{k}$,\;\;\;$\hat{n}_{14}=0.82\hat{i}-0.41\hat{j}-0.41\hat{k}$,\;\;\;$\hat{n}_{23}=-0.58\hat{i}-0.58\hat{j}-0.58\hat{k}$,\;\;\;$\vec{r}_{13}=10.0\hat{i}+10.0\hat{j}+10.0\hat{k}$,\;\;\;$\vec{r}_{14}=10.0\hat{i}+10.0\hat{j}+10.0\hat{k}$,\;\;\;$\vec{r}_{24}=0.0\hat{i}+0.0\hat{j}+0.0\hat{k}$.

{\tiny 1D-M25:}   $\hat{n}_{13}=0.16\hat{i}+0.61\hat{j}-0.77\hat{k}$,\;\;\;$\hat{n}_{14}=-0.8\hat{i}+0.54\hat{j}+0.26\hat{k}$,\;\;\;$\hat{n}_{24}=0.58\hat{i}+0.58\hat{j}+0.58\hat{k}$,\;\;\;$\vec{r}_{13}=0.0\hat{i}+0.0\hat{j}+0.0\hat{k}$,\;\;\;$\vec{r}_{14}=0.0\hat{i}+0.0\hat{j}+0.0\hat{k}$,\;\;\;$\vec{r}_{23}=10.0\hat{i}+10.0\hat{j}+10.0\hat{k}$.

{\tiny 1D-M26:}   $\hat{n}_{13}=-0.0\hat{i}+0.56\hat{j}+0.83\hat{k}$,\;\;\;$\hat{n}_{23}=-0.58\hat{i}+0.56\hat{j}-0.59\hat{k}$,\;\;\;$\hat{n}_{24}=0.81\hat{i}+0.46\hat{j}-0.36\hat{k}$,\;\;\;$\vec{r}_{13}=0.0\hat{i}+0.0\hat{j}+10.0\hat{k}$,\;\;\;$\vec{r}_{14}=10.0\hat{i}+0.0\hat{j}+0.0\hat{k}$,\;\;\;$\vec{r}_{24}=0.0\hat{i}+10.0\hat{j}+10.0\hat{k}$.

{\tiny 1D-M27:}   $\hat{n}_{13}=0.0\hat{i}-0.0\hat{j}+1.0\hat{k}$,\;\;\;$\hat{n}_{23}=-0.17\hat{i}-0.6\hat{j}+0.78\hat{k}$,\;\;\;$\hat{n}_{24}=-0.58\hat{i}-0.58\hat{j}-0.58\hat{k}$,\;\;\;$\vec{r}_{13}=10.0\hat{i}+10.0\hat{j}+2.83\hat{k}$,\;\;\;$\vec{r}_{14}=10.0\hat{i}+10.0\hat{j}+10.0\hat{k}$,\;\;\;$\vec{r}_{23}=0.0\hat{i}+0.0\hat{j}+0.0\hat{k}$.

{\tiny 1D-M28:}   $\hat{n}_{13}=-0.08\hat{i}-0.95\hat{j}-0.3\hat{k}$,\;\;\;$\hat{n}_{14}=0.0\hat{i}+0.0\hat{j}+1.0\hat{k}$,\;\;\;$\hat{n}_{23}=-0.31\hat{i}-0.44\hat{j}+0.84\hat{k}$,\;\;\;$\vec{r}_{14}=10.0\hat{i}+0.0\hat{j}+7.16\hat{k}$,\;\;\;$\vec{r}_{23}=4.62\hat{i}+3.55\hat{j}+4.57\hat{k}$,\;\;\;$\vec{r}_{24}=5.36\hat{i}+4.87\hat{j}+4.55\hat{k}$.

{\tiny 1D-M29:}   $\hat{n}_{13}=0.94\hat{i}-0.34\hat{j}-0.08\hat{k}$,\;\;\;$\hat{n}_{14}=0.36\hat{i}+0.32\hat{j}+0.88\hat{k}$,\;\;\;$\hat{n}_{24}=0.14\hat{i}-0.99\hat{j}-0.03\hat{k}$,\;\;\;$\vec{r}_{14}=10.0\hat{i}+10.0\hat{j}+0.0\hat{k}$,\;\;\;$\vec{r}_{23}=6.04\hat{i}+4.16\hat{j}+5.3\hat{k}$,\;\;\;$\vec{r}_{24}=3.09\hat{i}+4.06\hat{j}+2.83\hat{k}$.

{\tiny 1D-M30:}   $\hat{n}_{13}=0.0\hat{i}+0.53\hat{j}-0.85\hat{k}$,\;\;\;$\hat{n}_{14}=0.04\hat{i}+0.85\hat{j}-0.53\hat{k}$,\;\;\;$\hat{n}_{23}=-0.59\hat{i}+0.2\hat{j}+0.79\hat{k}$,\;\;\;$\vec{r}_{14}=0.0\hat{i}+0.0\hat{j}+0.0\hat{k}$,\;\;\;$\vec{r}_{23}=10.0\hat{i}+0.0\hat{j}+0.0\hat{k}$,\;\;\;$\vec{r}_{24}=0.0\hat{i}+10.0\hat{j}+10.0\hat{k}$.

{\tiny 1D-M31:}   $\hat{n}_{13}=0.58\hat{i}+0.58\hat{j}-0.58\hat{k}$,\;\;\;$\hat{n}_{14}=0.61\hat{i}+0.72\hat{j}+0.33\hat{k}$,\;\;\;$\hat{n}_{24}=-0.74\hat{i}+0.66\hat{j}-0.08\hat{k}$,\;\;\;$\vec{r}_{14}=0.0\hat{i}+0.0\hat{j}+10.0\hat{k}$,\;\;\;$\vec{r}_{23}=10.0\hat{i}+10.0\hat{j}+0.0\hat{k}$,\;\;\;$\vec{r}_{24}=0.0\hat{i}+0.0\hat{j}+10.0\hat{k}$.

{\tiny 1D-M32:}   $\hat{n}_{13}=0.49\hat{i}-0.6\hat{j}-0.63\hat{k}$,\;\;\;$\hat{n}_{23}=0.71\hat{i}+0.25\hat{j}-0.65\hat{k}$,\;\;\;$\hat{n}_{24}=-0.85\hat{i}-0.47\hat{j}-0.22\hat{k}$,\;\;\;$\vec{r}_{14}=0.0\hat{i}+10.0\hat{j}+10.0\hat{k}$,\;\;\;$\vec{r}_{23}=0.0\hat{i}+0.0\hat{j}+0.0\hat{k}$,\;\;\;$\vec{r}_{24}=10.0\hat{i}+0.0\hat{j}+10.0\hat{k}$.

{\tiny 1D-M33:}   $\hat{n}_{13}=-0.66\hat{i}-0.58\hat{j}+0.49\hat{k}$,\;\;\;$\hat{n}_{23}=0.25\hat{i}+0.44\hat{j}+0.86\hat{k}$,\;\;\;$\hat{n}_{24}=-0.63\hat{i}+0.22\hat{j}+0.75\hat{k}$,\;\;\;$\vec{r}_{14}=0.0\hat{i}+10.0\hat{j}+10.0\hat{k}$,\;\;\;$\vec{r}_{23}=10.0\hat{i}+10.0\hat{j}+0.0\hat{k}$,\;\;\;$\vec{r}_{24}=0.0\hat{i}+0.0\hat{j}+0.0\hat{k}$.

{\tiny 1D-M34:}   $\hat{n}_{13}=-0.74\hat{i}-0.6\hat{j}-0.29\hat{k}$,\;\;\;$\hat{n}_{14}=-0.62\hat{i}-0.35\hat{j}-0.7\hat{k}$,\;\;\;$\hat{n}_{23}=0.27\hat{i}-0.91\hat{j}-0.32\hat{k}$,\;\;\;$\vec{r}_{13}=1.42\hat{i}+3.47\hat{j}+4.31\hat{k}$,\;\;\;$\vec{r}_{14}=0.0\hat{i}+0.0\hat{j}+10.0\hat{k}$,\;\;\;$\vec{r}_{24}=4.36\hat{i}+8.23\hat{j}+4.01\hat{k}$.

{\tiny 1D-M35:}   $\hat{n}_{13}=-0.42\hat{i}-0.91\hat{j}-0.01\hat{k}$,\;\;\;$\hat{n}_{14}=0.43\hat{i}+0.25\hat{j}+0.87\hat{k}$,\;\;\;$\hat{n}_{24}=-0.22\hat{i}-0.98\hat{j}-0.01\hat{k}$,\;\;\;$\vec{r}_{13}=4.89\hat{i}+4.28\hat{j}+3.84\hat{k}$,\;\;\;$\vec{r}_{14}=10.0\hat{i}+10.0\hat{j}+0.0\hat{k}$,\;\;\;$\vec{r}_{23}=4.55\hat{i}+6.12\hat{j}+6.81\hat{k}$.

{\tiny 1D-M36:}   $\hat{n}_{13}=-0.44\hat{i}-0.72\hat{j}-0.53\hat{k}$,\;\;\;$\hat{n}_{14}=0.83\hat{i}+0.56\hat{j}+0.02\hat{k}$,\;\;\;$\hat{n}_{23}=0.53\hat{i}+0.17\hat{j}+0.83\hat{k}$,\;\;\;$\vec{r}_{13}=4.07\hat{i}+7.49\hat{j}+8.26\hat{k}$,\;\;\;$\vec{r}_{23}=7.9\hat{i}+3.19\hat{j}+5.34\hat{k}$,\;\;\;$\vec{r}_{24}=0.9\hat{i}+1.12\hat{j}+1.36\hat{k}$.

{\tiny 1D-M37:}   $\hat{n}_{13}=0.01\hat{i}-0.41\hat{j}-0.91\hat{k}$,\;\;\;$\hat{n}_{14}=0.75\hat{i}+0.56\hat{j}-0.35\hat{k}$,\;\;\;$\hat{n}_{24}=0.01\hat{i}+0.03\hat{j}-1.0\hat{k}$,\;\;\;$\vec{r}_{13}=8.51\hat{i}+5.61\hat{j}+9.3\hat{k}$,\;\;\;$\vec{r}_{23}=6.97\hat{i}+5.83\hat{j}+8.15\hat{k}$,\;\;\;$\vec{r}_{24}=8.79\hat{i}+9.89\hat{j}+0.01\hat{k}$.

{\tiny 1D-M38:}   $\hat{n}_{13}=0.61\hat{i}-0.54\hat{j}-0.58\hat{k}$,\;\;\;$\hat{n}_{23}=0.04\hat{i}-0.37\hat{j}-0.93\hat{k}$,\;\;\;$\hat{n}_{24}=0.2\hat{i}-0.61\hat{j}+0.77\hat{k}$,\;\;\;$\vec{r}_{13}=0.0\hat{i}+10.0\hat{j}+10.0\hat{k}$,\;\;\;$\vec{r}_{14}=10.0\hat{i}+10.0\hat{j}+0.0\hat{k}$,\;\;\;$\vec{r}_{23}=10.0\hat{i}+0.0\hat{j}+0.0\hat{k}$.

{\tiny 1D-M39:}   $\hat{n}_{13}=-0.95\hat{i}-0.16\hat{j}-0.27\hat{k}$,\;\;\;$\hat{n}_{23}=0.0\hat{i}+0.7\hat{j}+0.72\hat{k}$,\;\;\;$\hat{n}_{24}=0.0\hat{i}+0.9\hat{j}-0.45\hat{k}$,\;\;\;$\vec{r}_{13}=10.0\hat{i}+0.0\hat{j}+10.0\hat{k}$,\;\;\;$\vec{r}_{14}=0.0\hat{i}+10.0\hat{j}+0.0\hat{k}$,\;\;\;$\vec{r}_{24}=10.0\hat{i}+10.0\hat{j}+10.0\hat{k}$.

{\tiny 1D-M40:}   $\hat{n}_{14}=0.16\hat{i}+0.79\hat{j}-0.6\hat{k}$,\;\;\;$\hat{n}_{23}=-0.6\hat{i}-0.8\hat{j}-0.08\hat{k}$,\;\;\;$\hat{n}_{24}=0.64\hat{i}-0.67\hat{j}-0.37\hat{k}$,\;\;\;$\vec{r}_{13}=1.1\hat{i}+4.9\hat{j}+2.13\hat{k}$,\;\;\;$\vec{r}_{14}=0.0\hat{i}+0.0\hat{j}+0.0\hat{k}$,\;\;\;$\vec{r}_{24}=2.1\hat{i}+1.07\hat{j}+6.29\hat{k}$.

{\tiny 1D-M41:}   $\hat{n}_{14}=-0.38\hat{i}+0.38\hat{j}+0.84\hat{k}$,\;\;\;$\hat{n}_{23}=-0.1\hat{i}-0.91\hat{j}+0.41\hat{k}$,\;\;\;$\hat{n}_{24}=0.15\hat{i}-0.92\hat{j}-0.37\hat{k}$,\;\;\;$\vec{r}_{13}=2.65\hat{i}+4.93\hat{j}+7.29\hat{k}$,\;\;\;$\vec{r}_{14}=10.0\hat{i}+0.0\hat{j}+0.0\hat{k}$,\;\;\;$\vec{r}_{23}=5.5\hat{i}+6.06\hat{j}+4.36\hat{k}$.

{\tiny 1D-M42:}   $\hat{n}_{14}=0.03\hat{i}+0.04\hat{j}-1.0\hat{k}$,\;\;\;$\hat{n}_{23}=0.33\hat{i}+0.27\hat{j}-0.9\hat{k}$,\;\;\;$\hat{n}_{24}=0.54\hat{i}+0.31\hat{j}-0.78\hat{k}$,\;\;\;$\vec{r}_{13}=6.21\hat{i}+5.74\hat{j}+0.52\hat{k}$,\;\;\;$\vec{r}_{23}=9.31\hat{i}+7.29\hat{j}+7.38\hat{k}$,\;\;\;$\vec{r}_{24}=0.63\hat{i}+8.6\hat{j}+9.34\hat{k}$.

{\tiny 1D-M43:}   $\hat{n}_{14}=-0.04\hat{i}-0.47\hat{j}-0.88\hat{k}$,\;\;\;$\hat{n}_{23}=0.88\hat{i}+0.43\hat{j}-0.18\hat{k}$,\;\;\;$\hat{n}_{24}=0.26\hat{i}-0.36\hat{j}-0.9\hat{k}$,\;\;\;$\vec{r}_{13}=1.34\hat{i}+0.31\hat{j}+9.39\hat{k}$,\;\;\;$\vec{r}_{23}=3.01\hat{i}+2.96\hat{j}+3.33\hat{k}$,\;\;\;$\vec{r}_{24}=4.67\hat{i}+6.48\hat{j}+0.25\hat{k}$.

{\tiny 1D-M44:}   $\hat{n}_{14}=-0.44\hat{i}-0.37\hat{j}+0.82\hat{k}$,\;\;\;$\hat{n}_{23}=0.69\hat{i}-0.73\hat{j}+0.04\hat{k}$,\;\;\;$\hat{n}_{24}=0.58\hat{i}+0.58\hat{j}+0.58\hat{k}$,\;\;\;$\vec{r}_{13}=10.0\hat{i}+10.0\hat{j}+10.0\hat{k}$,\;\;\;$\vec{r}_{14}=0.0\hat{i}+0.0\hat{j}+0.0\hat{k}$,\;\;\;$\vec{r}_{23}=0.0\hat{i}+0.0\hat{j}+0.0\hat{k}$.

{\tiny 1D-M45:}   $\hat{n}_{14}=-0.8\hat{i}-0.26\hat{j}-0.54\hat{k}$,\;\;\;$\hat{n}_{23}=0.58\hat{i}-0.58\hat{j}-0.58\hat{k}$,\;\;\;$\hat{n}_{24}=0.17\hat{i}+0.78\hat{j}-0.61\hat{k}$,\;\;\;$\vec{r}_{13}=0.0\hat{i}+10.0\hat{j}+0.0\hat{k}$,\;\;\;$\vec{r}_{14}=10.0\hat{i}+0.0\hat{j}+10.0\hat{k}$,\;\;\;$\vec{r}_{24}=10.0\hat{i}+0.0\hat{j}+10.0\hat{k}$.

{\tiny 1D-M46:}   $\hat{n}_{12}=-0.15\hat{i}+0.71\hat{j}-0.68\hat{k}$,\;\;\;$\hat{n}_{13}=-0.42\hat{i}-0.63\hat{j}-0.66\hat{k}$,\;\;\;$\hat{n}_{24}=-0.75\hat{i}+0.29\hat{j}+0.59\hat{k}$,\;\;\;$\vec{r}_{12}=0.0\hat{i}+10.0\hat{j}+0.0\hat{k}$,\;\;\;$\vec{r}_{24}=0.0\hat{i}+0.0\hat{j}+0.0\hat{k}$,\;\;\;$\vec{r}_{34}=10.0\hat{i}+10.0\hat{j}+10.0\hat{k}$.

{\tiny 1D-M47:}   $\hat{n}_{12}=-0.47\hat{i}+0.81\hat{j}-0.34\hat{k}$,\;\;\;$\hat{n}_{13}=-0.58\hat{i}-0.58\hat{j}-0.58\hat{k}$,\;\;\;$\hat{n}_{34}=0.67\hat{i}+0.08\hat{j}-0.74\hat{k}$,\;\;\;$\vec{r}_{12}=10.0\hat{i}+10.0\hat{j}+10.0\hat{k}$,\;\;\;$\vec{r}_{24}=0.0\hat{i}+0.0\hat{j}+0.0\hat{k}$,\;\;\;$\vec{r}_{34}=10.0\hat{i}+10.0\hat{j}+10.0\hat{k}$.

{\tiny 1D-M48:}   $\hat{n}_{12}=-0.78\hat{i}+0.61\hat{j}-0.14\hat{k}$,\;\;\;$\hat{n}_{13}=-0.0\hat{i}+0.0\hat{j}+1.0\hat{k}$,\;\;\;$\hat{n}_{24}=-0.71\hat{i}-0.61\hat{j}+0.34\hat{k}$,\;\;\;$\vec{r}_{12}=10.0\hat{i}+10.0\hat{j}+0.0\hat{k}$,\;\;\;$\vec{r}_{13}=0.0\hat{i}+0.0\hat{j}+1.46\hat{k}$,\;\;\;$\vec{r}_{34}=10.0\hat{i}+10.0\hat{j}+10.0\hat{k}$.

{\tiny 1D-M49:}   $\hat{n}_{12}=-0.0\hat{i}+0.94\hat{j}-0.34\hat{k}$,\;\;\;$\hat{n}_{13}=0.0\hat{i}+0.0\hat{j}-1.0\hat{k}$,\;\;\;$\hat{n}_{34}=-0.73\hat{i}+0.69\hat{j}-0.0\hat{k}$,\;\;\;$\vec{r}_{12}=10.0\hat{i}+0.0\hat{j}+10.0\hat{k}$,\;\;\;$\vec{r}_{13}=10.0\hat{i}+0.0\hat{j}+4.77\hat{k}$,\;\;\;$\vec{r}_{24}=0.0\hat{i}+10.0\hat{j}+0.0\hat{k}$.

{\tiny 1D-M50:}   $\hat{n}_{12}=0.82\hat{i}-0.44\hat{j}+0.36\hat{k}$,\;\;\;$\hat{n}_{24}=-0.58\hat{i}-0.6\hat{j}+0.55\hat{k}$,\;\;\;$\hat{n}_{34}=0.0\hat{i}+0.57\hat{j}+0.82\hat{k}$,\;\;\;$\vec{r}_{12}=10.0\hat{i}+10.0\hat{j}+0.0\hat{k}$,\;\;\;$\vec{r}_{13}=0.0\hat{i}+0.0\hat{j}+10.0\hat{k}$,\;\;\;$\vec{r}_{34}=10.0\hat{i}+10.0\hat{j}+0.0\hat{k}$.

{\tiny 1D-M51:}   $\hat{n}_{12}=-0.0\hat{i}+0.62\hat{j}-0.78\hat{k}$,\;\;\;$\hat{n}_{24}=-0.79\hat{i}+0.53\hat{j}+0.31\hat{k}$,\;\;\;$\hat{n}_{34}=0.77\hat{i}+0.44\hat{j}+0.47\hat{k}$,\;\;\;$\vec{r}_{12}=10.0\hat{i}+0.0\hat{j}+10.0\hat{k}$,\;\;\;$\vec{r}_{13}=10.0\hat{i}+10.0\hat{j}+10.0\hat{k}$,\;\;\;$\vec{r}_{24}=0.0\hat{i}+0.0\hat{j}+0.0\hat{k}$.

{\tiny 1D-M52:}   $\hat{n}_{12}=0.69\hat{i}+0.51\hat{j}+0.52\hat{k}$,\;\;\;$\hat{n}_{13}=-0.91\hat{i}-0.28\hat{j}-0.3\hat{k}$,\;\;\;$\hat{n}_{24}=-0.0\hat{i}+0.69\hat{j}-0.72\hat{k}$,\;\;\;$\vec{r}_{13}=10.0\hat{i}+0.0\hat{j}+10.0\hat{k}$,\;\;\;$\vec{r}_{24}=10.0\hat{i}+10.0\hat{j}+10.0\hat{k}$,\;\;\;$\vec{r}_{34}=0.0\hat{i}+0.0\hat{j}+0.0\hat{k}$.

{\tiny 1D-M53:}   $\hat{n}_{12}=0.61\hat{i}-0.05\hat{j}+0.79\hat{k}$,\;\;\;$\hat{n}_{13}=-0.65\hat{i}-0.37\hat{j}-0.66\hat{k}$,\;\;\;$\hat{n}_{34}=-0.61\hat{i}+0.5\hat{j}+0.61\hat{k}$,\;\;\;$\vec{r}_{13}=10.0\hat{i}+10.0\hat{j}+0.0\hat{k}$,\;\;\;$\vec{r}_{24}=0.0\hat{i}+10.0\hat{j}+10.0\hat{k}$,\;\;\;$\vec{r}_{34}=0.0\hat{i}+0.0\hat{j}+0.0\hat{k}$.

{\tiny 1D-M54:}   $\hat{n}_{12}=-0.86\hat{i}+0.41\hat{j}-0.3\hat{k}$,\;\;\;$\hat{n}_{24}=-0.6\hat{i}-0.48\hat{j}+0.64\hat{k}$,\;\;\;$\hat{n}_{34}=-0.68\hat{i}+0.26\hat{j}-0.69\hat{k}$,\;\;\;$\vec{r}_{13}=10.0\hat{i}+10.0\hat{j}+10.0\hat{k}$,\;\;\;$\vec{r}_{24}=10.0\hat{i}+0.0\hat{j}+0.0\hat{k}$,\;\;\;$\vec{r}_{34}=0.0\hat{i}+10.0\hat{j}+0.0\hat{k}$.

{\tiny 1D-M55:}   $\hat{n}_{12}=-0.0\hat{i}+0.75\hat{j}+0.66\hat{k}$,\;\;\;$\hat{n}_{24}=-0.96\hat{i}+0.16\hat{j}+0.22\hat{k}$,\;\;\;$\hat{n}_{34}=-0.0\hat{i}+0.71\hat{j}-0.7\hat{k}$,\;\;\;$\vec{r}_{13}=0.0\hat{i}+10.0\hat{j}+0.0\hat{k}$,\;\;\;$\vec{r}_{24}=10.0\hat{i}+10.0\hat{j}+10.0\hat{k}$,\;\;\;$\vec{r}_{34}=10.0\hat{i}+0.0\hat{j}+10.0\hat{k}$.

{\tiny 1D-M56:}   $\hat{n}_{12}=-0.74\hat{i}+0.08\hat{j}+0.66\hat{k}$,\;\;\;$\hat{n}_{24}=0.77\hat{i}-0.64\hat{j}-0.02\hat{k}$,\;\;\;$\hat{n}_{34}=0.58\hat{i}+0.58\hat{j}+0.58\hat{k}$,\;\;\;$\vec{r}_{12}=0.0\hat{i}+0.0\hat{j}+0.0\hat{k}$,\;\;\;$\vec{r}_{13}=10.0\hat{i}+10.0\hat{j}+10.0\hat{k}$,\;\;\;$\vec{r}_{24}=10.0\hat{i}+10.0\hat{j}+10.0\hat{k}$.

{\tiny 1D-M57:}   $\hat{n}_{12}=0.0\hat{i}+0.79\hat{j}-0.61\hat{k}$,\;\;\;$\hat{n}_{24}=0.6\hat{i}+0.48\hat{j}+0.63\hat{k}$,\;\;\;$\hat{n}_{34}=0.0\hat{i}+0.57\hat{j}+0.82\hat{k}$,\;\;\;$\vec{r}_{12}=10.0\hat{i}+10.0\hat{j}+10.0\hat{k}$,\;\;\;$\vec{r}_{13}=0.0\hat{i}+0.0\hat{j}+0.0\hat{k}$,\;\;\;$\vec{r}_{34}=10.0\hat{i}+10.0\hat{j}+0.0\hat{k}$.

{\tiny 1D-M58:}   $\hat{n}_{13}=0.71\hat{i}-0.71\hat{j}+0.0\hat{k}$,\;\;\;$\hat{n}_{14}=0.58\hat{i}+0.58\hat{j}-0.58\hat{k}$,\;\;\;$\vec{r}_{13}=0.0\hat{i}+0.0\hat{j}+0.0\hat{k}$,\;\;\;$\vec{r}_{23}=10.0\hat{i}+10.0\hat{j}+0.0\hat{k}$,\;\;\;$\vec{r}_{24}=0.0\hat{i}+0.0\hat{j}+10.0\hat{k}$.

{\tiny 1D-M59:}   $\hat{n}_{13}=0.57\hat{i}-0.61\hat{j}-0.55\hat{k}$,\;\;\;$\hat{n}_{14}=-0.63\hat{i}-0.66\hat{j}-0.41\hat{k}$,\;\;\;$\vec{r}_{14}=10.0\hat{i}+0.0\hat{j}+0.0\hat{k}$,\;\;\;$\vec{r}_{23}=1.65\hat{i}+1.14\hat{j}+3.04\hat{k}$,\;\;\;$\vec{r}_{24}=3.29\hat{i}+6.44\hat{j}+8.8\hat{k}$.

{\tiny 1D-M60:}   $\hat{n}_{14}=0.62\hat{i}-0.06\hat{j}+0.78\hat{k}$,\;\;\;$\hat{n}_{24}=-0.71\hat{i}-0.53\hat{j}+0.46\hat{k}$,\;\;\;$\vec{r}_{13}=7.06\hat{i}+6.93\hat{j}+6.95\hat{k}$,\;\;\;$\vec{r}_{14}=0.0\hat{i}+10.0\hat{j}+0.0\hat{k}$,\;\;\;$\vec{r}_{23}=2.75\hat{i}+2.12\hat{j}+7.47\hat{k}$.

{\tiny 1D-M61:}   $\hat{n}_{14}=-0.32\hat{i}-0.19\hat{j}+0.93\hat{k}$,\;\;\;$\hat{n}_{24}=-0.61\hat{i}+0.79\hat{j}-0.08\hat{k}$,\;\;\;$\vec{r}_{13}=5.17\hat{i}+7.03\hat{j}+1.54\hat{k}$,\;\;\;$\vec{r}_{23}=9.53\hat{i}+5.41\hat{j}+6.8\hat{k}$,\;\;\;$\vec{r}_{24}=0.37\hat{i}+8.09\hat{j}+7.49\hat{k}$.

{\tiny 1D-M62:}   $\hat{n}_{12}=0.28\hat{i}+0.64\hat{j}+0.71\hat{k}$,\;\;\;$\hat{n}_{24}=0.0\hat{i}+0.52\hat{j}+0.85\hat{k}$,\;\;\;$\vec{r}_{12}=0.0\hat{i}+0.0\hat{j}+10.0\hat{k}$,\;\;\;$\vec{r}_{13}=10.0\hat{i}+0.0\hat{j}+10.0\hat{k}$,\;\;\;$\vec{r}_{34}=0.0\hat{i}+10.0\hat{j}+0.0\hat{k}$.

{\tiny 1D-M63:}   $\hat{n}_{12}=-0.46\hat{i}-0.43\hat{j}+0.78\hat{k}$,\;\;\;$\hat{n}_{24}=-0.07\hat{i}-0.66\hat{j}-0.75\hat{k}$,\;\;\;$\vec{r}_{13}=0.0\hat{i}+10.0\hat{j}+10.0\hat{k}$,\;\;\;$\vec{r}_{24}=10.0\hat{i}+10.0\hat{j}+0.0\hat{k}$,\;\;\;$\vec{r}_{34}=10.0\hat{i}+0.0\hat{j}+0.0\hat{k}$.

{\tiny 1D-M64:}   $\hat{n}_{13}=-0.23\hat{i}+0.23\hat{j}-0.95\hat{k}$,\;\;\;$\hat{n}_{14}=-0.71\hat{i}-0.71\hat{j}+0.0\hat{k}$,\;\;\;$\hat{n}_{23}=0.59\hat{i}-0.59\hat{j}+0.55\hat{k}$,\;\;\;$\hat{n}_{24}=0.43\hat{i}-0.43\hat{j}-0.8\hat{k}$,\;\;\;$\vec{r}_{13}=10.0\hat{i}+0.0\hat{j}+10.0\hat{k}$,\;\;\;$\vec{r}_{14}=5.01\hat{i}+5.01\hat{j}+5.01\hat{k}$,\;\;\;$\vec{r}_{23}=0.0\hat{i}+10.0\hat{j}+0.0\hat{k}$,\;\;\;$\vec{r}_{24}=0.0\hat{i}+10.0\hat{j}+10.0\hat{k}$.

{\tiny 1D-M65:}\label{result_1_65}   $\hat{n}_{13}=0.31\hat{i}-0.63\hat{j}+0.71\hat{k}$,\;\;\;$\hat{n}_{14}=-0.62\hat{i}-0.02\hat{j}-0.78\hat{k}$,\;\;\;$\hat{n}_{23}=-0.89\hat{i}-0.46\hat{j}-0.01\hat{k}$,\;\;\;$\hat{n}_{24}=0.33\hat{i}-0.63\hat{j}-0.7\hat{k}$,\;\;\;$\vec{r}_{13}=5.12\hat{i}+4.88\hat{j}+5.02\hat{k}$,\;\;\;$\vec{r}_{14}=10.0\hat{i}+10.0\hat{j}+0.0\hat{k}$,\;\;\;$\vec{r}_{23}=4.82\hat{i}+4.82\hat{j}+4.97\hat{k}$,\;\;\;$\vec{r}_{24}=4.86\hat{i}+5.18\hat{j}+4.92\hat{k}$.

{\tiny 1D-M66:}   $\hat{n}_{13}=0.61\hat{i}-0.61\hat{j}+0.51\hat{k}$,\;\;\;$\hat{n}_{14}=-0.71\hat{i}-0.71\hat{j}-0.0\hat{k}$,\;\;\;$\hat{n}_{23}=-0.59\hat{i}+0.59\hat{j}+0.56\hat{k}$,\;\;\;$\hat{n}_{24}=0.31\hat{i}-0.31\hat{j}-0.9\hat{k}$,\;\;\;$\vec{r}_{13}=10.0\hat{i}+0.0\hat{j}+10.0\hat{k}$,\;\;\;$\vec{r}_{14}=5.06\hat{i}+5.03\hat{j}+5.17\hat{k}$,\;\;\;$\vec{r}_{23}=10.0\hat{i}+0.0\hat{j}+0.0\hat{k}$,\;\;\;$\vec{r}_{24}=0.0\hat{i}+10.0\hat{j}+10.0\hat{k}$.

{\tiny 1D-M67:}   $\hat{n}_{13}=-0.58\hat{i}+0.8\hat{j}-0.16\hat{k}$,\;\;\;$\hat{n}_{14}=0.0\hat{i}-0.0\hat{j}+1.0\hat{k}$,\;\;\;$\hat{n}_{23}=-0.86\hat{i}-0.52\hat{j}+0.03\hat{k}$,\;\;\;$\hat{n}_{24}=-0.44\hat{i}-0.89\hat{j}-0.05\hat{k}$,\;\;\;$\vec{r}_{13}=10.0\hat{i}+10.0\hat{j}+0.0\hat{k}$,\;\;\;$\vec{r}_{14}=0.0\hat{i}+0.0\hat{j}+3.07\hat{k}$,\;\;\;$\vec{r}_{23}=0.0\hat{i}+10.0\hat{j}+10.0\hat{k}$,\;\;\;$\vec{r}_{24}=10.0\hat{i}+0.0\hat{j}+0.0\hat{k}$.

{\tiny 1D-M68:}   $\hat{n}_{12}=0.34\hat{i}-0.89\hat{j}+0.31\hat{k}$,\;\;\;$\hat{n}_{13}=0.56\hat{i}+0.34\hat{j}-0.76\hat{k}$,\;\;\;$\hat{n}_{24}=-0.0\hat{i}+0.82\hat{j}+0.57\hat{k}$,\;\;\;$\hat{n}_{34}=-0.85\hat{i}+0.27\hat{j}-0.44\hat{k}$,\;\;\;$\vec{r}_{12}=10.0\hat{i}+10.0\hat{j}+10.0\hat{k}$,\;\;\;$\vec{r}_{13}=0.0\hat{i}+10.0\hat{j}+10.0\hat{k}$,\;\;\;$\vec{r}_{24}=10.0\hat{i}+0.0\hat{j}+0.0\hat{k}$,\;\;\;$\vec{r}_{34}=10.0\hat{i}+10.0\hat{j}+0.0\hat{k}$.

{\tiny 1D-M69:}   $\hat{n}_{12}=-0.0\hat{i}+0.77\hat{j}+0.64\hat{k}$,\;\;\;$\hat{n}_{13}=0.55\hat{i}-0.44\hat{j}+0.71\hat{k}$,\;\;\;$\hat{n}_{24}=-0.79\hat{i}+0.61\hat{j}+0.1\hat{k}$,\;\;\;$\hat{n}_{34}=-0.82\hat{i}-0.32\hat{j}+0.48\hat{k}$,\;\;\;$\vec{r}_{12}=10.0\hat{i}+0.0\hat{j}+0.0\hat{k}$,\;\;\;$\vec{r}_{13}=10.0\hat{i}+10.0\hat{j}+0.0\hat{k}$,\;\;\;$\vec{r}_{24}=10.0\hat{i}+10.0\hat{j}+10.0\hat{k}$,\;\;\;$\vec{r}_{34}=10.0\hat{i}+0.0\hat{j}+0.0\hat{k}$.

{\tiny 1D-M70:}   $\hat{n}_{13}=-0.58\hat{i}+0.58\hat{j}+0.58\hat{k}$,\;\;\;$\hat{n}_{14}=0.58\hat{i}-0.58\hat{j}-0.58\hat{k}$,\;\;\;$\hat{n}_{23}=-0.05\hat{i}+0.68\hat{j}-0.73\hat{k}$,\;\;\;$\vec{r}_{23}=10.0\hat{i}+0.0\hat{j}+10.0\hat{k}$,\;\;\;$\vec{r}_{24}=0.0\hat{i}+10.0\hat{j}+0.0\hat{k}$.

{\tiny 1D-M71:}   $\hat{n}_{13}=-0.58\hat{i}-0.58\hat{j}+0.58\hat{k}$,\;\;\;$\hat{n}_{14}=0.58\hat{i}+0.58\hat{j}-0.58\hat{k}$,\;\;\;$\hat{n}_{24}=-0.12\hat{i}+0.76\hat{j}+0.64\hat{k}$,\;\;\;$\vec{r}_{23}=10.0\hat{i}+10.0\hat{j}+0.0\hat{k}$,\;\;\;$\vec{r}_{24}=0.0\hat{i}+0.0\hat{j}+10.0\hat{k}$.

{\tiny 1D-M72:}   $\hat{n}_{13}=-0.21\hat{i}-0.79\hat{j}+0.58\hat{k}$,\;\;\;$\hat{n}_{14}=0.21\hat{i}+0.79\hat{j}-0.58\hat{k}$,\;\;\;$\hat{n}_{23}=-0.58\hat{i}+0.58\hat{j}+0.58\hat{k}$,\;\;\;$\vec{r}_{14}=0.0\hat{i}+10.0\hat{j}+0.0\hat{k}$,\;\;\;$\vec{r}_{24}=10.0\hat{i}+0.0\hat{j}+10.0\hat{k}$.

{\tiny 1D-M73:}   $\hat{n}_{13}=-0.3\hat{i}+0.81\hat{j}-0.51\hat{k}$,\;\;\;$\hat{n}_{14}=-0.3\hat{i}+0.81\hat{j}-0.51\hat{k}$,\;\;\;$\hat{n}_{24}=0.58\hat{i}+0.58\hat{j}+0.58\hat{k}$,\;\;\;$\vec{r}_{14}=0.0\hat{i}+0.0\hat{j}+0.0\hat{k}$,\;\;\;$\vec{r}_{23}=10.0\hat{i}+10.0\hat{j}+10.0\hat{k}$.

{\tiny 1D-M74:}   $\hat{n}_{13}=-0.62\hat{i}-0.77\hat{j}-0.15\hat{k}$,\;\;\;$\hat{n}_{23}=-0.58\hat{i}+0.58\hat{j}-0.58\hat{k}$,\;\;\;$\hat{n}_{24}=0.53\hat{i}-0.27\hat{j}-0.8\hat{k}$,\;\;\;$\vec{r}_{14}=10.0\hat{i}+0.0\hat{j}+0.0\hat{k}$,\;\;\;$\vec{r}_{24}=0.0\hat{i}+10.0\hat{j}+10.0\hat{k}$.

{\tiny 1D-M75:}   $\hat{n}_{13}=0.0\hat{i}-0.71\hat{j}+0.71\hat{k}$,\;\;\;$\hat{n}_{23}=-0.82\hat{i}+0.41\hat{j}+0.41\hat{k}$,\;\;\;$\hat{n}_{24}=0.58\hat{i}+0.58\hat{j}+0.58\hat{k}$,\;\;\;$\vec{r}_{14}=0.0\hat{i}+0.0\hat{j}+0.0\hat{k}$,\;\;\;$\vec{r}_{23}=10.0\hat{i}+10.0\hat{j}+10.0\hat{k}$.

{\tiny 1D-M76:}   $\hat{n}_{13}=-0.42\hat{i}-0.11\hat{j}-0.9\hat{k}$,\;\;\;$\hat{n}_{14}=-0.55\hat{i}-0.55\hat{j}+0.63\hat{k}$,\;\;\;$\hat{n}_{23}=-0.4\hat{i}-0.63\hat{j}-0.66\hat{k}$,\;\;\;$\vec{r}_{13}=6.6\hat{i}+0.48\hat{j}+3.49\hat{k}$,\;\;\;$\vec{r}_{24}=4.51\hat{i}+2.41\hat{j}+7.15\hat{k}$.

{\tiny 1D-M77:}   $\hat{n}_{13}=0.68\hat{i}+0.58\hat{j}+0.45\hat{k}$,\;\;\;$\hat{n}_{14}=-0.84\hat{i}+0.51\hat{j}+0.16\hat{k}$,\;\;\;$\hat{n}_{24}=0.09\hat{i}+0.07\hat{j}-0.99\hat{k}$,\;\;\;$\vec{r}_{13}=5.88\hat{i}+3.66\hat{j}+8.07\hat{k}$,\;\;\;$\vec{r}_{23}=5.04\hat{i}+4.9\hat{j}+8.77\hat{k}$.

{\tiny 1D-M78:}   $\hat{n}_{13}=-0.82\hat{i}+0.41\hat{j}+0.41\hat{k}$,\;\;\;$\hat{n}_{23}=0.0\hat{i}-0.71\hat{j}+0.71\hat{k}$,\;\;\;$\hat{n}_{24}=-0.58\hat{i}-0.58\hat{j}-0.58\hat{k}$,\;\;\;$\vec{r}_{13}=0.0\hat{i}+0.0\hat{j}+0.0\hat{k}$,\;\;\;$\vec{r}_{14}=10.0\hat{i}+10.0\hat{j}+10.0\hat{k}$.

{\tiny 1D-M79:}   $\hat{n}_{14}=-0.3\hat{i}-0.22\hat{j}+0.93\hat{k}$,\;\;\;$\hat{n}_{23}=0.35\hat{i}+0.04\hat{j}-0.93\hat{k}$,\;\;\;$\hat{n}_{24}=0.17\hat{i}-0.24\hat{j}+0.96\hat{k}$,\;\;\;$\vec{r}_{13}=1.22\hat{i}+2.68\hat{j}+2.58\hat{k}$,\;\;\;$\vec{r}_{24}=3.32\hat{i}+1.52\hat{j}+3.48\hat{k}$.

{\tiny 1D-M80:}   $\hat{n}_{14}=-0.07\hat{i}+0.16\hat{j}+0.99\hat{k}$,\;\;\;$\hat{n}_{23}=0.48\hat{i}-0.66\hat{j}+0.58\hat{k}$,\;\;\;$\hat{n}_{24}=0.04\hat{i}+0.14\hat{j}+0.99\hat{k}$,\;\;\;$\vec{r}_{13}=3.42\hat{i}+7.36\hat{j}+7.95\hat{k}$,\;\;\;$\vec{r}_{23}=5.45\hat{i}+6.86\hat{j}+8.94\hat{k}$.

{\tiny 1D-M81:}   $\hat{n}_{14}=-0.66\hat{i}+0.09\hat{j}+0.75\hat{k}$,\;\;\;$\hat{n}_{23}=-0.66\hat{i}+0.09\hat{j}+0.75\hat{k}$,\;\;\;$\hat{n}_{24}=-0.58\hat{i}+0.58\hat{j}-0.58\hat{k}$,\;\;\;$\vec{r}_{13}=10.0\hat{i}+0.0\hat{j}+0.0\hat{k}$,\;\;\;$\vec{r}_{14}=0.0\hat{i}+10.0\hat{j}+10.0\hat{k}$.

{\tiny 1D-M82:}   $\hat{n}_{12}=-0.67\hat{i}+0.45\hat{j}+0.59\hat{k}$,\;\;\;$\hat{n}_{13}=0.55\hat{i}-0.61\hat{j}-0.57\hat{k}$,\;\;\;$\hat{n}_{24}=0.53\hat{i}-0.27\hat{j}+0.8\hat{k}$,\;\;\;$\vec{r}_{24}=0.0\hat{i}+10.0\hat{j}+0.0\hat{k}$,\;\;\;$\vec{r}_{34}=10.0\hat{i}+0.0\hat{j}+10.0\hat{k}$.

{\tiny 1D-M83:}   $\hat{n}_{12}=-0.0\hat{i}+0.0\hat{j}-1.0\hat{k}$,\;\;\;$\hat{n}_{13}=0.0\hat{i}+0.0\hat{j}+1.0\hat{k}$,\;\;\;$\hat{n}_{24}=0.71\hat{i}+0.71\hat{j}+0.0\hat{k}$,\;\;\;$\vec{r}_{13}=10.0\hat{i}+10.0\hat{j}+9.32\hat{k}$,\;\;\;$\vec{r}_{34}=0.0\hat{i}+0.0\hat{j}+0.29\hat{k}$.

{\tiny 1D-M84:}   $\hat{n}_{12}=-0.57\hat{i}-0.49\hat{j}-0.66\hat{k}$,\;\;\;$\hat{n}_{13}=-0.82\hat{i}+0.41\hat{j}+0.41\hat{k}$,\;\;\;$\hat{n}_{34}=0.58\hat{i}+0.6\hat{j}+0.56\hat{k}$,\;\;\;$\vec{r}_{13}=10.0\hat{i}+10.0\hat{j}+10.0\hat{k}$,\;\;\;$\vec{r}_{24}=0.0\hat{i}+0.0\hat{j}+0.0\hat{k}$.

{\tiny 1D-M85:}   $\hat{n}_{12}=-0.77\hat{i}-0.61\hat{j}-0.16\hat{k}$,\;\;\;$\hat{n}_{24}=0.58\hat{i}-0.58\hat{j}-0.58\hat{k}$,\;\;\;$\hat{n}_{34}=0.01\hat{i}-0.7\hat{j}+0.71\hat{k}$,\;\;\;$\vec{r}_{13}=0.0\hat{i}+10.0\hat{j}+0.0\hat{k}$,\;\;\;$\vec{r}_{34}=10.0\hat{i}+0.0\hat{j}+10.0\hat{k}$.

{\tiny 1D-M86:}   $\hat{n}_{12}=0.58\hat{i}-0.81\hat{j}-0.0\hat{k}$,\;\;\;$\hat{n}_{24}=0.0\hat{i}-0.0\hat{j}-1.0\hat{k}$,\;\;\;$\hat{n}_{34}=0.75\hat{i}-0.66\hat{j}+0.0\hat{k}$,\;\;\;$\vec{r}_{13}=0.0\hat{i}+10.0\hat{j}+1.51\hat{k}$,\;\;\;$\vec{r}_{24}=10.0\hat{i}+0.0\hat{j}+6.87\hat{k}$.

{\tiny 1D-M87:}   $\hat{n}_{12}=-0.82\hat{i}+0.41\hat{j}-0.41\hat{k}$,\;\;\;$\hat{n}_{24}=-0.58\hat{i}-0.64\hat{j}+0.51\hat{k}$,\;\;\;$\hat{n}_{34}=-0.58\hat{i}-0.55\hat{j}+0.6\hat{k}$,\;\;\;$\vec{r}_{12}=10.0\hat{i}+10.0\hat{j}+0.0\hat{k}$,\;\;\;$\vec{r}_{13}=0.0\hat{i}+0.0\hat{j}+10.0\hat{k}$.

{\tiny 1D-M88:}   $\hat{n}_{13}=-0.58\hat{i}+0.58\hat{j}-0.58\hat{k}$,\;\;\;$\hat{n}_{14}=0.58\hat{i}-0.58\hat{j}+0.58\hat{k}$,\;\;\;$\vec{r}_{23}=0.0\hat{i}+10.0\hat{j}+10.0\hat{k}$,\;\;\;$\vec{r}_{24}=10.0\hat{i}+0.0\hat{j}+0.0\hat{k}$.

{\tiny 1D-M89:}   $\hat{n}_{14}=0.0\hat{i}-0.36\hat{j}-0.93\hat{k}$,\;\;\;$\hat{n}_{24}=-0.72\hat{i}-0.26\hat{j}-0.64\hat{k}$,\;\;\;$\vec{r}_{13}=8.34\hat{i}+6.1\hat{j}+5.75\hat{k}$,\;\;\;$\vec{r}_{23}=3.26\hat{i}+4.56\hat{j}+7.14\hat{k}$.

{\tiny 1D-M90:}   $\hat{n}_{12}=0.0\hat{i}+0.0\hat{j}+1.0\hat{k}$,\;\;\;$\hat{n}_{24}=-0.0\hat{i}+0.92\hat{j}+0.38\hat{k}$,\;\;\;$\vec{r}_{13}=10.0\hat{i}+10.0\hat{j}+10.0\hat{k}$,\;\;\;$\vec{r}_{34}=0.0\hat{i}+0.0\hat{j}+0.0\hat{k}$.

{\tiny 1D-M91:}   $\hat{n}_{13}=-0.24\hat{i}-0.85\hat{j}+0.47\hat{k}$,\;\;\;$\hat{n}_{14}=-0.24\hat{i}-0.85\hat{j}+0.47\hat{k}$,\;\;\;$\hat{n}_{23}=-0.35\hat{i}-0.37\hat{j}-0.86\hat{k}$,\;\;\;$\hat{n}_{24}=0.91\hat{i}-0.37\hat{j}-0.21\hat{k}$,\;\;\;$\vec{r}_{14}=4.82\hat{i}+5.35\hat{j}+4.24\hat{k}$,\;\;\;$\vec{r}_{23}=5.77\hat{i}+5.14\hat{j}+4.2\hat{k}$,\;\;\;$\vec{r}_{24}=5.35\hat{i}+5.81\hat{j}+5.53\hat{k}$.

{\tiny 1D-M92:}   $\hat{n}_{13}=-0.05\hat{i}-0.21\hat{j}+0.98\hat{k}$,\;\;\;$\hat{n}_{14}=0.19\hat{i}+0.29\hat{j}-0.94\hat{k}$,\;\;\;$\hat{n}_{23}=0.16\hat{i}+0.12\hat{j}+0.98\hat{k}$,\;\;\;$\hat{n}_{24}=-0.72\hat{i}-0.67\hat{j}+0.2\hat{k}$,\;\;\;$\vec{r}_{13}=8.59\hat{i}+9.74\hat{j}+5.71\hat{k}$,\;\;\;$\vec{r}_{23}=9.97\hat{i}+5.54\hat{j}+5.15\hat{k}$,\;\;\;$\vec{r}_{24}=3.31\hat{i}+4.3\hat{j}+4.92\hat{k}$.

{\tiny 1D-M93:}   $\hat{n}_{13}=-0.63\hat{i}+0.17\hat{j}+0.75\hat{k}$,\;\;\;$\hat{n}_{14}=0.76\hat{i}-0.05\hat{j}+0.65\hat{k}$,\;\;\;$\hat{n}_{23}=0.76\hat{i}-0.05\hat{j}+0.65\hat{k}$,\;\;\;$\hat{n}_{24}=-0.14\hat{i}-0.98\hat{j}+0.1\hat{k}$,\;\;\;$\vec{r}_{13}=5.68\hat{i}+5.82\hat{j}+5.13\hat{k}$,\;\;\;$\vec{r}_{14}=4.08\hat{i}+5.92\hat{j}+4.4\hat{k}$,\;\;\;$\vec{r}_{24}=5.36\hat{i}+5.32\hat{j}+5.78\hat{k}$.

{\tiny 1D-M94:}   $\hat{n}_{13}=0.4\hat{i}-0.48\hat{j}+0.78\hat{k}$,\;\;\;$\hat{n}_{14}=0.26\hat{i}-0.75\hat{j}-0.61\hat{k}$,\;\;\;$\hat{n}_{23}=-0.88\hat{i}-0.45\hat{j}+0.18\hat{k}$,\;\;\;$\hat{n}_{24}=0.26\hat{i}-0.75\hat{j}-0.61\hat{k}$,\;\;\;$\vec{r}_{13}=4.92\hat{i}+4.88\hat{j}+5.04\hat{k}$,\;\;\;$\vec{r}_{14}=4.81\hat{i}+4.88\hat{j}+4.88\hat{k}$,\;\;\;$\vec{r}_{23}=4.93\hat{i}+4.88\hat{j}+5.07\hat{k}$.

{\tiny 1D-M95:}   $\hat{n}_{12}=-0.89\hat{i}-0.29\hat{j}-0.36\hat{k}$,\;\;\;$\hat{n}_{13}=0.66\hat{i}+0.57\hat{j}+0.49\hat{k}$,\;\;\;$\hat{n}_{24}=-0.16\hat{i}-0.53\hat{j}+0.83\hat{k}$,\;\;\;$\hat{n}_{34}=-0.73\hat{i}+0.63\hat{j}+0.26\hat{k}$,\;\;\;$\vec{r}_{13}=4.73\hat{i}+4.26\hat{j}+4.77\hat{k}$,\;\;\;$\vec{r}_{24}=5.36\hat{i}+5.47\hat{j}+4.87\hat{k}$,\;\;\;$\vec{r}_{34}=4.74\hat{i}+5.76\hat{j}+4.86\hat{k}$.

{\tiny 1D-M96:}   $\hat{n}_{12}=-0.52\hat{i}-0.13\hat{j}+0.84\hat{k}$,\;\;\;$\hat{n}_{13}=0.7\hat{i}-0.64\hat{j}+0.33\hat{k}$,\;\;\;$\hat{n}_{24}=-0.18\hat{i}-0.95\hat{j}-0.26\hat{k}$,\;\;\;$\hat{n}_{34}=-0.49\hat{i}-0.76\hat{j}-0.42\hat{k}$,\;\;\;$\vec{r}_{12}=3.53\hat{i}+7.37\hat{j}+5.85\hat{k}$,\;\;\;$\vec{r}_{13}=7.27\hat{i}+7.33\hat{j}+2.16\hat{k}$,\;\;\;$\vec{r}_{34}=3.23\hat{i}+6.27\hat{j}+4.91\hat{k}$.

\subsubsection*{For manipulators of DOF 2}
\input{contentfolder/mechanisms2/result/dof2/result2_full}
\subsubsection*{For manipulators of DOF 3}

{\tiny 3D-M1:}\label{result_3_1}   $\hat{n}_{13}=-0.71\hat{i}+0.11\hat{j}-0.7\hat{k}$,\;\;\;$\hat{n}_{23}=-0.0\hat{i}+0.58\hat{j}-0.81\hat{k}$,\;\;\;$\hat{n}_{24}=0.82\hat{i}-0.46\hat{j}-0.34\hat{k}$,\;\;\;$\vec{r}_{13}=10.0\hat{i}+10.0\hat{j}+0.0\hat{k}$,\;\;\;$\vec{r}_{23}=10.0\hat{i}+0.0\hat{j}+10.0\hat{k}$,\;\;\;$\vec{r}_{24}=10.0\hat{i}+10.0\hat{j}+10.0\hat{k}$.

{\tiny 3D-M2:}   $\hat{n}_{13}=-0.8\hat{i}+0.33\hat{j}+0.49\hat{k}$,\;\;\;$\hat{n}_{23}=-0.17\hat{i}+0.67\hat{j}-0.73\hat{k}$,\;\;\;$\hat{n}_{24}=-0.57\hat{i}-0.67\hat{j}-0.48\hat{k}$,\;\;\;$\vec{r}_{13}=10.0\hat{i}+10.0\hat{j}+10.0\hat{k}$,\;\;\;$\vec{r}_{23}=10.0\hat{i}+10.0\hat{j}+10.0\hat{k}$.

{\tiny 3D-M3:}   $\hat{n}_{13}=-0.8\hat{i}+0.58\hat{j}+0.14\hat{k}$,\;\;\;$\hat{n}_{23}=-0.74\hat{i}-0.51\hat{j}-0.43\hat{k}$,\;\;\;$\hat{n}_{24}=0.51\hat{i}+0.16\hat{j}+0.84\hat{k}$,\;\;\;$\vec{r}_{13}=10.0\hat{i}+10.0\hat{j}+10.0\hat{k}$,\;\;\;$\vec{r}_{24}=10.0\hat{i}+10.0\hat{j}+0.0\hat{k}$.

{\tiny 3D-M4:}   $\hat{n}_{13}=-0.57\hat{i}-0.67\hat{j}-0.48\hat{k}$,\;\;\;$\hat{n}_{23}=-0.31\hat{i}-0.36\hat{j}-0.88\hat{k}$,\;\;\;$\hat{n}_{24}=0.76\hat{i}-0.65\hat{j}+0.0\hat{k}$,\;\;\;$\vec{r}_{23}=10.0\hat{i}+10.0\hat{j}+0.0\hat{k}$,\;\;\;$\vec{r}_{24}=10.0\hat{i}+10.0\hat{j}+10.0\hat{k}$.

{\tiny 3D-M5:}   $\hat{n}_{13}=0.5\hat{i}+0.18\hat{j}+0.85\hat{k}$,\;\;\;$\hat{n}_{23}=-0.76\hat{i}-0.61\hat{j}-0.24\hat{k}$,\;\;\;$\hat{n}_{24}=0.03\hat{i}+0.33\hat{j}-0.94\hat{k}$,\;\;\;$\vec{r}_{13}=10.0\hat{i}+10.0\hat{j}+0.0\hat{k}$.

{\tiny 3D-M6:}   $\hat{n}_{13}=-0.6\hat{i}-0.76\hat{j}-0.26\hat{k}$,\;\;\;$\hat{n}_{23}=0.26\hat{i}+0.4\hat{j}+0.88\hat{k}$,\;\;\;$\hat{n}_{24}=-0.21\hat{i}-0.17\hat{j}+0.96\hat{k}$,\;\;\;$\vec{r}_{23}=10.0\hat{i}+10.0\hat{j}+0.0\hat{k}$.

{\tiny 3D-M7:}   $\hat{n}_{13}=-0.54\hat{i}-0.83\hat{j}+0.12\hat{k}$,\;\;\;$\hat{n}_{23}=0.18\hat{i}-0.26\hat{j}-0.95\hat{k}$,\;\;\;$\hat{n}_{24}=-0.04\hat{i}-0.56\hat{j}-0.83\hat{k}$,\;\;\;$\vec{r}_{24}=10.0\hat{i}+10.0\hat{j}+0.0\hat{k}$.

{\tiny 3D-M8:}\label{result_3_8}   $\hat{n}_{13}=0.41\hat{i}+0.89\hat{j}-0.2\hat{k}$,\;\;\;$\hat{n}_{23}=-0.62\hat{i}+0.11\hat{j}-0.78\hat{k}$,\;\;\;$\hat{n}_{24}=-0.67\hat{i}+0.44\hat{j}+0.59\hat{k}$.

\subsubsection*{For manipulators of DOF 4}

{\tiny 4D-M1:}\label{result_4_1}   $\hat{n}_{14}=-0.29\hat{i}+0.57\hat{j}-0.77\hat{k}$,\;\;\;$\hat{n}_{23}=0.75\hat{i}-0.53\hat{j}+0.4\hat{k}$,\;\;\;$\hat{n}_{25}=-0.34\hat{i}+0.83\hat{j}-0.45\hat{k}$,\;\;\;$\hat{n}_{34}=-0.72\hat{i}+0.12\hat{j}+0.69\hat{k}$,\;\;\;$\vec{r}_{14}=10.0\hat{i}+0.0\hat{j}+10.0\hat{k}$,\;\;\;$\vec{r}_{23}=10.0\hat{i}+10.0\hat{j}+0.0\hat{k}$,\;\;\;$\vec{r}_{25}=0.0\hat{i}+0.0\hat{j}+0.0\hat{k}$,\;\;\;$\vec{r}_{34}=10.0\hat{i}+10.0\hat{j}+10.0\hat{k}$.

{\tiny 4D-M2:}   $\hat{n}_{14}=0.82\hat{i}+0.49\hat{j}+0.3\hat{k}$,\;\;\;$\hat{n}_{23}=-0.39\hat{i}-0.47\hat{j}-0.79\hat{k}$,\;\;\;$\hat{n}_{25}=-0.42\hat{i}-0.85\hat{j}-0.32\hat{k}$,\;\;\;$\hat{n}_{34}=0.57\hat{i}+0.69\hat{j}+0.45\hat{k}$,\;\;\;$\vec{r}_{14}=10.0\hat{i}+0.0\hat{j}+10.0\hat{k}$,\;\;\;$\vec{r}_{23}=10.0\hat{i}+10.0\hat{j}+0.0\hat{k}$,\;\;\;$\vec{r}_{25}=0.0\hat{i}+10.0\hat{j}+10.0\hat{k}$.

{\tiny 4D-M3:}   $\hat{n}_{14}=0.39\hat{i}+0.47\hat{j}-0.79\hat{k}$,\;\;\;$\hat{n}_{23}=-0.42\hat{i}-0.85\hat{j}+0.32\hat{k}$,\;\;\;$\hat{n}_{25}=-0.57\hat{i}-0.69\hat{j}+0.45\hat{k}$,\;\;\;$\hat{n}_{34}=0.82\hat{i}+0.49\hat{j}-0.3\hat{k}$,\;\;\;$\vec{r}_{14}=10.0\hat{i}+10.0\hat{j}+10.0\hat{k}$,\;\;\;$\vec{r}_{23}=0.0\hat{i}+10.0\hat{j}+0.0\hat{k}$,\;\;\;$\vec{r}_{34}=10.0\hat{i}+0.0\hat{j}+0.0\hat{k}$.

{\tiny 4D-M4:}   $\hat{n}_{14}=0.42\hat{i}+0.85\hat{j}-0.32\hat{k}$,\;\;\;$\hat{n}_{23}=-0.57\hat{i}-0.69\hat{j}+0.45\hat{k}$,\;\;\;$\hat{n}_{25}=-0.39\hat{i}-0.47\hat{j}+0.79\hat{k}$,\;\;\;$\hat{n}_{34}=0.82\hat{i}+0.49\hat{j}-0.3\hat{k}$,\;\;\;$\vec{r}_{14}=0.0\hat{i}+10.0\hat{j}+0.0\hat{k}$,\;\;\;$\vec{r}_{25}=10.0\hat{i}+10.0\hat{j}+10.0\hat{k}$,\;\;\;$\vec{r}_{34}=10.0\hat{i}+0.0\hat{j}+0.0\hat{k}$.

{\tiny 4D-M5:}   $\hat{n}_{14}=-0.57\hat{i}-0.69\hat{j}-0.45\hat{k}$,\;\;\;$\hat{n}_{23}=0.42\hat{i}+0.85\hat{j}+0.32\hat{k}$,\;\;\;$\hat{n}_{25}=0.82\hat{i}+0.49\hat{j}+0.3\hat{k}$,\;\;\;$\hat{n}_{34}=-0.39\hat{i}-0.47\hat{j}-0.79\hat{k}$,\;\;\;$\vec{r}_{23}=0.0\hat{i}+10.0\hat{j}+10.0\hat{k}$,\;\;\;$\vec{r}_{25}=10.0\hat{i}+0.0\hat{j}+10.0\hat{k}$,\;\;\;$\vec{r}_{34}=10.0\hat{i}+10.0\hat{j}+0.0\hat{k}$.

{\tiny 4D-M6:}   $\hat{n}_{14}=-0.54\hat{i}-0.84\hat{j}-0.08\hat{k}$,\;\;\;$\hat{n}_{23}=-0.68\hat{i}-0.7\hat{j}-0.22\hat{k}$,\;\;\;$\hat{n}_{25}=0.62\hat{i}-0.53\hat{j}+0.59\hat{k}$,\;\;\;$\hat{n}_{34}=-0.58\hat{i}-0.81\hat{j}-0.12\hat{k}$,\;\;\;$\vec{r}_{14}=0.0\hat{i}+10.0\hat{j}+10.0\hat{k}$,\;\;\;$\vec{r}_{23}=10.0\hat{i}+0.0\hat{j}+0.0\hat{k}$.

{\tiny 4D-M7:}   $\hat{n}_{14}=0.54\hat{i}+0.84\hat{j}-0.08\hat{k}$,\;\;\;$\hat{n}_{23}=-0.05\hat{i}+0.94\hat{j}+0.34\hat{k}$,\;\;\;$\hat{n}_{25}=-0.68\hat{i}-0.7\hat{j}+0.22\hat{k}$,\;\;\;$\hat{n}_{34}=0.84\hat{i}+0.22\hat{j}-0.49\hat{k}$,\;\;\;$\vec{r}_{14}=0.0\hat{i}+10.0\hat{j}+0.0\hat{k}$,\;\;\;$\vec{r}_{25}=10.0\hat{i}+0.0\hat{j}+10.0\hat{k}$.

{\tiny 4D-M8:}   $\hat{n}_{14}=0.54\hat{i}+0.84\hat{j}-0.08\hat{k}$,\;\;\;$\hat{n}_{23}=-0.26\hat{i}+0.85\hat{j}+0.46\hat{k}$,\;\;\;$\hat{n}_{25}=-0.8\hat{i}-0.46\hat{j}+0.38\hat{k}$,\;\;\;$\hat{n}_{34}=-0.68\hat{i}-0.7\hat{j}+0.22\hat{k}$,\;\;\;$\vec{r}_{14}=0.0\hat{i}+10.0\hat{j}+0.0\hat{k}$,\;\;\;$\vec{r}_{34}=10.0\hat{i}+0.0\hat{j}+10.0\hat{k}$.

{\tiny 4D-M9:}   $\hat{n}_{14}=-0.08\hat{i}-0.96\hat{j}-0.27\hat{k}$,\;\;\;$\hat{n}_{23}=0.54\hat{i}+0.84\hat{j}-0.08\hat{k}$,\;\;\;$\hat{n}_{25}=-0.68\hat{i}-0.7\hat{j}+0.22\hat{k}$,\;\;\;$\hat{n}_{34}=-0.84\hat{i}-0.08\hat{j}+0.53\hat{k}$,\;\;\;$\vec{r}_{23}=0.0\hat{i}+10.0\hat{j}+0.0\hat{k}$,\;\;\;$\vec{r}_{25}=10.0\hat{i}+0.0\hat{j}+10.0\hat{k}$.

{\tiny 4D-M10:}   $\hat{n}_{14}=-0.63\hat{i}-0.76\hat{j}-0.17\hat{k}$,\;\;\;$\hat{n}_{23}=-0.54\hat{i}-0.84\hat{j}-0.08\hat{k}$,\;\;\;$\hat{n}_{25}=-0.56\hat{i}+0.59\hat{j}-0.57\hat{k}$,\;\;\;$\hat{n}_{34}=-0.68\hat{i}-0.7\hat{j}-0.22\hat{k}$,\;\;\;$\vec{r}_{23}=0.0\hat{i}+10.0\hat{j}+10.0\hat{k}$,\;\;\;$\vec{r}_{34}=10.0\hat{i}+0.0\hat{j}+0.0\hat{k}$.

{\tiny 4D-M11:}   $\hat{n}_{14}=-0.32\hat{i}+0.81\hat{j}-0.49\hat{k}$,\;\;\;$\hat{n}_{23}=0.78\hat{i}+0.52\hat{j}+0.35\hat{k}$,\;\;\;$\hat{n}_{25}=-0.68\hat{i}-0.7\hat{j}-0.22\hat{k}$,\;\;\;$\hat{n}_{34}=0.54\hat{i}+0.84\hat{j}+0.08\hat{k}$,\;\;\;$\vec{r}_{25}=10.0\hat{i}+0.0\hat{j}+0.0\hat{k}$,\;\;\;$\vec{r}_{34}=0.0\hat{i}+10.0\hat{j}+10.0\hat{k}$.

{\tiny 4D-M12:}   $\hat{n}_{14}=0.09\hat{i}-1.0\hat{j}+0.05\hat{k}$,\;\;\;$\hat{n}_{23}=0.67\hat{i}+0.35\hat{j}+0.66\hat{k}$,\;\;\;$\hat{n}_{25}=0.01\hat{i}-0.88\hat{j}+0.47\hat{k}$,\;\;\;$\hat{n}_{34}=-0.75\hat{i}+0.31\hat{j}+0.59\hat{k}$,\;\;\;$\vec{r}_{14}=4.0\hat{i}+2.99\hat{j}+5.94\hat{k}$.

{\tiny 4D-M13:}\label{result_4_13}   $\hat{n}_{14}=-0.94\hat{i}-0.18\hat{j}-0.29\hat{k}$,\;\;\;$\hat{n}_{23}=0.32\hat{i}-0.95\hat{j}+0.01\hat{k}$,\;\;\;$\hat{n}_{25}=-0.03\hat{i}-0.8\hat{j}+0.59\hat{k}$,\;\;\;$\hat{n}_{34}=0.34\hat{i}-0.57\hat{j}-0.75\hat{k}$,\;\;\;$\vec{r}_{23}=7.59\hat{i}+3.33\hat{j}+4.0\hat{k}$.

{\tiny 4D-M14:}   $\hat{n}_{14}=-0.38\hat{i}-0.54\hat{j}-0.75\hat{k}$,\;\;\;$\hat{n}_{23}=-0.54\hat{i}-0.53\hat{j}+0.65\hat{k}$,\;\;\;$\hat{n}_{25}=0.34\hat{i}-0.93\hat{j}-0.12\hat{k}$,\;\;\;$\hat{n}_{34}=0.75\hat{i}-0.65\hat{j}+0.1\hat{k}$,\;\;\;$\vec{r}_{25}=3.55\hat{i}+6.33\hat{j}+6.15\hat{k}$.

{\tiny 4D-M15:}   $\hat{n}_{14}=-0.19\hat{i}-0.68\hat{j}-0.71\hat{k}$,\;\;\;$\hat{n}_{23}=0.56\hat{i}-0.67\hat{j}+0.49\hat{k}$,\;\;\;$\hat{n}_{25}=-0.8\hat{i}-0.3\hat{j}+0.51\hat{k}$,\;\;\;$\hat{n}_{34}=0.84\hat{i}-0.54\hat{j}+0.05\hat{k}$,\;\;\;$\vec{r}_{34}=3.99\hat{i}+5.66\hat{j}+6.62\hat{k}$.
\endgroup
