# Supplementary material for: Dimensional synthesis of spatial manipulators for velocity and force transmission for operation around a specified task point
Source: arXiv:2210.04446 source file (2022-10-10)
Supplement: Supplementary file 4 [file AppendixG.tex]

% Appendix Template

\chapter{Relation between force-transmission matrix and velocity-transmission matrix} % Main appendix title

\label{AppendixG} % Change X to a consecutive letter; for referencing this appendix elsewhere, use \ref{AppendixX}

\lhead{Appendix G. \emph{Relation between force-transmission matrix and velocity-transmission matrix}} % Change X to a consecutive letter; this is for the header on each page - perhaps a shortened title

The mapping of joint velocities to end-effector velocities is given by the equation
\begin{equation}
  \label{eq:vel_jacobian}
  v=J\dot{\theta}.
\end{equation}

For a robotic system of negligible frictional power losses that transfers forces from the joint forces/torques to the end-effector forces, the total power remains conserved. This is given by equation \eqref{eq:power_joints_and_endeffector}.

\begin{equation}
  \label{eq:power_joints_and_endeffector}
  P=F^Tv=\tau^T \dot{\theta}
\end{equation}

By putting equation \eqref{eq:vel_jacobian} in equation \eqref{eq:power_joints_and_endeffector},

\begin{equation}
  F^Tv=\tau^T \dot{\theta}
\end{equation}

\begin{equation}
  \Rightarrow F^TJ\dot{\theta}=\tau^T \dot{\theta}
\end{equation}

\begin{equation}
  \Rightarrow F^TJ=\tau^T
\end{equation}

\begin{equation}
  \Rightarrow \tau^T=J^TF
\end{equation}

Thus, the force-transformation matrix is exactly the transpose of the velocity-transformation matrix.
