# Supplementary material for: Dimensional synthesis of spatial manipulators for velocity and force transmission for operation around a specified task point
Source: arXiv:2210.04446 source file (2022-10-10)
Supplement: Supplementary file 5 [file AppendixH.tex]

\chapter{Optimisation Method} % Main appendix title

\label{AppendixH} % Change X to a consecutive letter; for referencing this appendix elsewhere, use \ref{AppendixX}

\lhead{Appendix H. \emph{Optimisation Method}} % Change X to a consecutive letter; this is for the header on each page - perhaps a shortened title

\section{Optimisation Method used in this study}

MATLAB Optimisation Toolbox is used to perform optimisation in this study. The \emph{fmincon} command is used in MATLAB with default options. The default method that the command uses for this kind of optimisation problems is \emph{interior-point} with BFGS approximation of Hessian.

\subsection{Problem}
Minimise

$$f(\mathbf{x})$$

Subject to

$$\begin{matrix}g_i(\mathbf{x})\leq0 \\ h_j(\mathbf{x})=0\end{matrix}$$

The idea of interior-point method is to have a barrier function such that the initial point is pressurised to stay within the interior of the feasible region during the iterations before finally converging to a local minimum point. One such barrier function is logarithmic function. And the inequality constraints are converted to equality constrains by introducing additional (slack) variables. This modifies the optimisation problem, as shown below.

\subsection{Modified problem}
Minimise

$$f(\mathbf{x})-c\sum_{i} \log_e{\left(s_i\right)}$$

Subject to

$$\begin{matrix}g_i(\mathbf{x})+s_i=0 \\ h_j(\mathbf{x})=0 \\ s_i\geq0 \end{matrix}$$

where $c$ is the barrier parameter.

\subsection{Lagrangian}
The Lagrangian of the problem can be formulated as show below.

$$\mathcal{L}\left(x,s,\lambda,\mu \right) = f(\mathbf{x})-c\sum_{i} \log_e{\left(s_i\right)}+\lambda^T h(x)+\mu^T \left(g(x)+s\right)$$

The goal is to find a point that vanishes the gradient of Lagrangian.

\subsection{Gradient of Lagrangian}

$$\nabla_x \mathcal{L} = \nabla_x f+\lambda^T \nabla_x h+\mu^T \nabla_x g$$

$$\nabla_s \mathcal{L} = -c\sum_{i} \left(\frac{1}{s_i}\right) +\mu_i = -c\mathbf{S}^{-1}e+\mu$$

$$\nabla_{\lambda} \mathcal{L} = h$$

$$\nabla_{\mu} \mathcal{L} = g+s$$

where $S=\text{diag}\left(s_1,s_2,...\right)$ and $e=\left(1,1,...\right)^T$.

\subsection{Newton's Method}

Setting the gradient of Lagrangian to zero gives

$$F(x,s,\lambda,\mu)=\begin{Bmatrix} \nabla_x f+\lambda^T \nabla_x h+\mu^T \nabla_x g \\ -ce+\mathbf{S}\mu \\ h \\ g+s \end{Bmatrix}=0$$

By using Newton's method,

$$\begin{Bmatrix} x_{n+1}-x_{n} \\ s_{n+1}-s_{n} \\ \lambda_{n+1}-\lambda_{n} \\ \mu_{n+1}-\mu_{n} \end{Bmatrix}=\begin{Bmatrix} \Delta x\\ \Delta s \\ \Delta \lambda \\ \Delta \mu \end{Bmatrix}=-\left(\nabla F^{-1}\right) F$$

where

% $$\nabla F=\begin{bmatrix}\nabla_{x}F_1 & \nabla_{s}F_1 & \nabla_{\lambda}F_1 & \nabla_{\mu}F_1 \\ \nabla_{x}F_2 & \nabla_{s}F_2 & \nabla_{\lambda}F_2 & \nabla_{\lambda}F_2 \\ \nabla_{x}F_3 & \nabla_{s}F_3 & \nabla_{\lambda}F_3 & \nabla_{\lambda}F_3 \\ \nabla_{x}F_4 & \nabla_{s}F_4 & \nabla_{\lambda}F_4 & \nabla_{\lambda}F_4 \end{bmatrix}$$

% $$\Rightarrow \nabla F=\begin{bmatrix}\nabla_{xx}L & 0 & \nabla_{x}h^T & \nabla_{x}g^T \\ 0 & M & 0 & S \\ \nabla_{x}h & 0 & 0 & 0 \\ \nabla_{x}g^T & -I & 0 & 0 \end{bmatrix}$$

$$\nabla F=\begin{bmatrix}\nabla_{xx}\mathcal{L} & 0 & \nabla_{x}h^T & \nabla_{x}g^T \\ 0 & M & 0 & S \\ \nabla_{x}h & 0 & 0 & 0 \\ \nabla_{x}g & -I & 0 & 0 \end{bmatrix}$$

where $\nabla_{xx}\mathcal{L}=\nabla_{xx} f+\lambda^T \nabla_{xx} h+\mu^T \nabla_{xx} g$ and $M=\text{diag}\left(\mu_1,\mu_2,...\right)$.

\subsection{Descent direction}

Descent direction $d=\{d_x,d_s,d_{\lambda},d_{\mu} \}^T$ can be given by solving the system

$$\begin{bmatrix}\nabla_{xx}\mathcal{L} & 0 & \nabla_{x}h^T & \nabla_{x}g^T \\ 0 & M & 0 & S \\ \nabla_{x}h & 0 & 0 & 0 \\ \nabla_{x}g & -I & 0 & 0 \end{bmatrix}\begin{Bmatrix} d_x \\ d_s \\ d_{\lambda} \\ d_{\mu} \end{Bmatrix}=-\begin{Bmatrix} \nabla_x f+\lambda^T \nabla_x h+\mu^T \nabla_x g \\ -ce+\mathbf{S}\mu \\ h \\ g+s \end{Bmatrix}$$

\subsection{Hessian approximation (BFGS)}

The Hessian $\nabla_{xx} \mathcal{L}$ of the Lagrangian can be approximated at each step by using the BFGS formula

$$H_{k+1}=H_k+\frac{y_ky_k^T}{y_k^Ts_k}+\frac{H_ks_ks_k^TH_k}{s_k^TH_ks_k},$$

where $s_k=x_{k+1}-x_k$ and $y_k=\nabla f(x_{k+1})-\nabla f(x_k)$.

\subsection{Line search}

$$\begin{Bmatrix} x_{n+1} \\ s_{n+1} \end{Bmatrix}=\begin{Bmatrix} x_{n} \\ s_{n} \end{Bmatrix} + \alpha_s \begin{Bmatrix} d_x \\ d_s \end{Bmatrix} $$

$$\begin{Bmatrix} \lambda_{n+1} \\ \mu_{n+1} \end{Bmatrix}=\begin{Bmatrix} \lambda_{n} \\ \mu_{n} \end{Bmatrix} + \alpha_{\mu} \begin{Bmatrix} d_{\lambda} \\ d_{\mu} \end{Bmatrix} $$

$$\alpha_s^{\text{max}}=\text{max}\{\alpha\in (0,1]: s+\alpha d_s \geq (1-\tau)s\}$$

$$\alpha_\mu^{\text{max}}=\text{max}\{\alpha\in (0,1]: \mu+\alpha d_\mu \geq (1-\tau)s\}$$
