# Supplementary material for: Dimensional synthesis of spatial manipulators for velocity and force transmission for operation around a specified task point
Source: arXiv:2210.04446 source file (2022-10-10)
Supplement: Supplementary file 6 [file classappendix10.tex]

\subsection{Class 10} \label{appendix_five_2_1}
2D-M560:

$\hat{n}_{14}=-0.13\hat{i}+0.58\hat{j}-0.8\hat{k}$,\;\;\;$\hat{n}_{24}=0.71\hat{i}-0.71\hat{j}+0.0\hat{k}$,\;\;\;$\hat{n}_{25}=-0.0\hat{i}+0.0\hat{j}+1.0\hat{k}$,\;\;\;$\hat{n}_{34}=-0.6\hat{i}+0.6\hat{j}+0.53\hat{k}$,\newline
$\vec{r}_{34}=10.0\hat{i}+0.0\hat{j}+0.0\hat{k}$,\;\;\;$\vec{r}_{35}=0.0\hat{i}+10.0\hat{j}+10.0\hat{k}$.

2D-M561:

$\hat{n}_{14}=0.0\hat{i}+0.0\hat{j}-1.0\hat{k}$,\;\;\;$\hat{n}_{24}=0.0\hat{i}+0.0\hat{j}+1.0\hat{k}$,\;\;\;$\hat{n}_{25}=-0.69\hat{i}+0.56\hat{j}+0.46\hat{k}$,\;\;\;$\hat{n}_{35}=0.0\hat{i}+0.82\hat{j}-0.57\hat{k}$,\newline
$\vec{r}_{34}=10.0\hat{i}+0.0\hat{j}+10.0\hat{k}$,\;\;\;$\vec{r}_{35}=0.0\hat{i}+10.0\hat{j}+0.0\hat{k}$.

2D-M562:

$\hat{n}_{14}=-0.08\hat{i}-0.71\hat{j}+0.7\hat{k}$,\;\;\;$\hat{n}_{24}=-0.48\hat{i}+0.68\hat{j}+0.55\hat{k}$,\;\;\;$\hat{n}_{25}=0.53\hat{i}-0.27\hat{j}+0.8\hat{k}$,\;\;\;$\hat{n}_{34}=0.6\hat{i}-0.55\hat{j}-0.58\hat{k}$,\newline
$\vec{r}_{25}=10.0\hat{i}+0.0\hat{j}+10.0\hat{k}$,\;\;\;$\vec{r}_{35}=0.0\hat{i}+10.0\hat{j}+0.0\hat{k}$.

2D-M563:

$\hat{n}_{14}=-0.03\hat{i}+0.77\hat{j}+0.64\hat{k}$,\;\;\;$\hat{n}_{24}=-0.37\hat{i}+0.56\hat{j}-0.74\hat{k}$,\;\;\;$\hat{n}_{25}=-0.93\hat{i}-0.17\hat{j}+0.33\hat{k}$,\;\;\;$\hat{n}_{35}=0.0\hat{i}+0.69\hat{j}-0.72\hat{k}$,\newline
$\vec{r}_{25}=0.0\hat{i}+10.0\hat{j}+10.0\hat{k}$,\;\;\;$\vec{r}_{34}=10.0\hat{i}+0.0\hat{j}+0.0\hat{k}$.

2D-M564:

$\hat{n}_{14}=-0.26\hat{i}+0.79\hat{j}+0.56\hat{k}$,\;\;\;$\hat{n}_{24}=-0.57\hat{i}-0.64\hat{j}+0.51\hat{k}$,\;\;\;$\hat{n}_{34}=0.82\hat{i}-0.41\hat{j}+0.41\hat{k}$,\;\;\;$\hat{n}_{35}=-0.58\hat{i}-0.56\hat{j}+0.59\hat{k}$,\newline
$\vec{r}_{25}=10.0\hat{i}+10.0\hat{j}+0.0\hat{k}$,\;\;\;$\vec{r}_{34}=0.0\hat{i}+0.0\hat{j}+10.0\hat{k}$.

2D-M565:

$\hat{n}_{14}=-0.0\hat{i}+0.0\hat{j}+1.0\hat{k}$,\;\;\;$\hat{n}_{24}=-0.0\hat{i}-0.0\hat{j}+1.0\hat{k}$,\;\;\;$\hat{n}_{25}=0.67\hat{i}+0.74\hat{j}-0.0\hat{k}$,\;\;\;$\hat{n}_{35}=-0.72\hat{i}-0.7\hat{j}+0.0\hat{k}$,\newline
$\vec{r}_{24}=10.0\hat{i}+10.0\hat{j}+1.02\hat{k}$,\;\;\;$\vec{r}_{34}=0.0\hat{i}+0.0\hat{j}+9.32\hat{k}$.

2D-M566:

$\hat{n}_{14}=-0.0\hat{i}-0.91\hat{j}-0.42\hat{k}$,\;\;\;$\hat{n}_{23}=-0.0\hat{i}+0.0\hat{j}+1.0\hat{k}$,\;\;\;$\hat{n}_{25}=-0.59\hat{i}+0.7\hat{j}+0.39\hat{k}$,\;\;\;$\hat{n}_{34}=-0.76\hat{i}-0.65\hat{j}+0.02\hat{k}$,\newline
$\vec{r}_{34}=0.0\hat{i}+10.0\hat{j}+0.0\hat{k}$,\;\;\;$\vec{r}_{45}=10.0\hat{i}+0.0\hat{j}+10.0\hat{k}$.

2D-M567:

$\hat{n}_{14}=0.27\hat{i}+0.67\hat{j}-0.69\hat{k}$,\;\;\;$\hat{n}_{23}=-0.01\hat{i}-0.71\hat{j}-0.7\hat{k}$,\;\;\;$\hat{n}_{25}=0.58\hat{i}-0.58\hat{j}+0.58\hat{k}$,\;\;\;$\hat{n}_{45}=0.01\hat{i}+0.71\hat{j}+0.7\hat{k}$,\newline
$\vec{r}_{34}=10.0\hat{i}+0.0\hat{j}+0.0\hat{k}$,\;\;\;$\vec{r}_{45}=0.0\hat{i}+10.0\hat{j}+10.0\hat{k}$.

2D-M568:

$\hat{n}_{14}=-0.64\hat{i}+0.57\hat{j}-0.52\hat{k}$,\;\;\;$\hat{n}_{23}=-0.0\hat{i}+0.71\hat{j}+0.71\hat{k}$,\;\;\;$\hat{n}_{25}=0.82\hat{i}-0.41\hat{j}+0.41\hat{k}$,\;\;\;$\hat{n}_{34}=-0.58\hat{i}-0.58\hat{j}+0.58\hat{k}$,\newline
$\vec{r}_{25}=0.0\hat{i}+0.0\hat{j}+10.0\hat{k}$,\;\;\;$\vec{r}_{45}=10.0\hat{i}+10.0\hat{j}+0.0\hat{k}$.

2D-M569:

$\hat{n}_{14}=-0.01\hat{i}+0.7\hat{j}-0.71\hat{k}$,\;\;\;$\hat{n}_{23}=0.58\hat{i}-0.58\hat{j}-0.58\hat{k}$,\;\;\;$\hat{n}_{25}=0.21\hat{i}+0.79\hat{j}-0.58\hat{k}$,\;\;\;$\hat{n}_{45}=0.58\hat{i}-0.58\hat{j}-0.58\hat{k}$,\newline
$\vec{r}_{25}=0.0\hat{i}+10.0\hat{j}+0.0\hat{k}$,\;\;\;$\vec{r}_{34}=10.0\hat{i}+0.0\hat{j}+10.0\hat{k}$.

2D-M570:

$\hat{n}_{14}=0.98\hat{i}-0.12\hat{j}+0.13\hat{k}$,\;\;\;$\hat{n}_{23}=-0.0\hat{i}+0.7\hat{j}+0.71\hat{k}$,\;\;\;$\hat{n}_{34}=0.58\hat{i}-0.58\hat{j}+0.58\hat{k}$,\;\;\;$\hat{n}_{45}=0.0\hat{i}-0.7\hat{j}-0.71\hat{k}$,\newline
$\vec{r}_{25}=10.0\hat{i}+0.0\hat{j}+0.0\hat{k}$,\;\;\;$\vec{r}_{45}=0.0\hat{i}+10.0\hat{j}+10.0\hat{k}$.

2D-M571:

$\hat{n}_{14}=-0.05\hat{i}+1.0\hat{j}+0.0\hat{k}$,\;\;\;$\hat{n}_{23}=-0.0\hat{i}+0.0\hat{j}+1.0\hat{k}$,\;\;\;$\hat{n}_{34}=0.63\hat{i}+0.63\hat{j}-0.46\hat{k}$,\;\;\;$\hat{n}_{45}=0.0\hat{i}+0.0\hat{j}-1.0\hat{k}$,\newline
$\vec{r}_{25}=10.0\hat{i}+10.0\hat{j}+10.0\hat{k}$,\;\;\;$\vec{r}_{34}=0.0\hat{i}+0.0\hat{j}+0.0\hat{k}$.

2D-M572:

$\hat{n}_{14}=-0.68\hat{i}+0.34\hat{j}+0.64\hat{k}$,\;\;\;$\hat{n}_{23}=0.53\hat{i}-0.27\hat{j}-0.8\hat{k}$,\;\;\;$\hat{n}_{25}=0.62\hat{i}+0.77\hat{j}+0.15\hat{k}$,\;\;\;$\hat{n}_{34}=-0.58\hat{i}+0.58\hat{j}-0.58\hat{k}$,\newline
$\vec{r}_{23}=10.0\hat{i}+0.0\hat{j}+0.0\hat{k}$,\;\;\;$\vec{r}_{45}=0.0\hat{i}+10.0\hat{j}+10.0\hat{k}$.

2D-M573:

$\hat{n}_{14}=-0.65\hat{i}+0.76\hat{j}-0.0\hat{k}$,\;\;\;$\hat{n}_{23}=0.6\hat{i}-0.6\hat{j}-0.53\hat{k}$,\;\;\;$\hat{n}_{25}=-0.38\hat{i}+0.38\hat{j}-0.85\hat{k}$,\;\;\;$\hat{n}_{45}=-0.0\hat{i}+0.0\hat{j}+1.0\hat{k}$,\newline
$\vec{r}_{23}=0.0\hat{i}+10.0\hat{j}+10.0\hat{k}$,\;\;\;$\vec{r}_{34}=10.0\hat{i}+0.0\hat{j}+0.0\hat{k}$.

2D-M574:

$\hat{n}_{14}=-0.45\hat{i}-0.89\hat{j}-0.0\hat{k}$,\;\;\;$\hat{n}_{23}=0.63\hat{i}-0.63\hat{j}-0.46\hat{k}$,\;\;\;$\hat{n}_{34}=-0.0\hat{i}-0.0\hat{j}-1.0\hat{k}$,\;\;\;$\hat{n}_{45}=0.0\hat{i}+0.0\hat{j}+1.0\hat{k}$,\newline
$\vec{r}_{23}=0.0\hat{i}+10.0\hat{j}+10.0\hat{k}$,\;\;\;$\vec{r}_{25}=10.0\hat{i}+0.0\hat{j}+0.0\hat{k}$.

2D-M575:

$\hat{n}_{14}=-0.0\hat{i}+0.71\hat{j}-0.71\hat{k}$,\;\;\;$\hat{n}_{25}=-1.0\hat{i}+0.0\hat{j}-0.0\hat{k}$,\;\;\;$\hat{n}_{34}=-0.0\hat{i}+0.71\hat{j}+0.71\hat{k}$,\;\;\;$\hat{n}_{45}=0.93\hat{i}-0.25\hat{j}-0.25\hat{k}$,\newline
$\vec{r}_{23}=0.0\hat{i}+0.0\hat{j}+0.0\hat{k}$,\;\;\;$\vec{r}_{45}=10.0\hat{i}+10.0\hat{j}+10.0\hat{k}$.

2D-M576:

$\hat{n}_{14}=-0.95\hat{i}-0.23\hat{j}-0.23\hat{k}$,\;\;\;$\hat{n}_{25}=0.36\hat{i}+0.66\hat{j}-0.66\hat{k}$,\;\;\;$\hat{n}_{34}=-0.93\hat{i}+0.25\hat{j}-0.25\hat{k}$,\;\;\;$\hat{n}_{45}=-0.0\hat{i}+0.71\hat{j}-0.71\hat{k}$,\newline
$\vec{r}_{23}=0.0\hat{i}+0.0\hat{j}+10.0\hat{k}$,\;\;\;$\vec{r}_{34}=10.0\hat{i}+10.0\hat{j}+0.0\hat{k}$.

2D-M577:

$\hat{n}_{14}=0.15\hat{i}-0.85\hat{j}-0.51\hat{k}$,\;\;\;$\hat{n}_{25}=0.8\hat{i}+0.33\hat{j}+0.5\hat{k}$,\;\;\;$\hat{n}_{34}=0.0\hat{i}-0.0\hat{j}+1.0\hat{k}$,\;\;\;$\hat{n}_{45}=-0.0\hat{i}+0.52\hat{j}-0.86\hat{k}$,\newline
$\vec{r}_{23}=0.0\hat{i}+0.0\hat{j}+10.0\hat{k}$,\;\;\;$\vec{r}_{25}=10.0\hat{i}+10.0\hat{j}+0.0\hat{k}$.

2D-M578:

$\hat{n}_{14}=0.19\hat{i}+0.77\hat{j}-0.61\hat{k}$,\;\;\;$\hat{n}_{15}=-0.84\hat{i}+0.09\hat{j}-0.54\hat{k}$,\;\;\;$\hat{n}_{23}=0.98\hat{i}-0.15\hat{j}+0.12\hat{k}$,\;\;\;$\hat{n}_{25}=0.0\hat{i}+0.62\hat{j}+0.78\hat{k}$,\newline
$\vec{r}_{15}=0.0\hat{i}+10.0\hat{j}+0.0\hat{k}$,\;\;\;$\vec{r}_{34}=10.0\hat{i}+0.0\hat{j}+10.0\hat{k}$.

2D-M579:

$\hat{n}_{14}=-0.81\hat{i}-0.27\hat{j}+0.52\hat{k}$,\;\;\;$\hat{n}_{15}=0.0\hat{i}+0.75\hat{j}+0.66\hat{k}$,\;\;\;$\hat{n}_{23}=0.12\hat{i}+0.8\hat{j}+0.59\hat{k}$,\;\;\;$\hat{n}_{34}=-0.58\hat{i}+0.54\hat{j}-0.61\hat{k}$,\newline
$\vec{r}_{15}=0.0\hat{i}+10.0\hat{j}+10.0\hat{k}$,\;\;\;$\vec{r}_{25}=10.0\hat{i}+0.0\hat{j}+0.0\hat{k}$.

2D-M580:

$\hat{n}_{14}=-0.49\hat{i}+0.81\hat{j}-0.32\hat{k}$,\;\;\;$\hat{n}_{15}=0.82\hat{i}-0.41\hat{j}-0.41\hat{k}$,\;\;\;$\hat{n}_{25}=0.65\hat{i}+0.1\hat{j}-0.75\hat{k}$,\;\;\;$\hat{n}_{34}=-0.58\hat{i}-0.58\hat{j}-0.58\hat{k}$,\newline
$\vec{r}_{15}=10.0\hat{i}+10.0\hat{j}+10.0\hat{k}$,\;\;\;$\vec{r}_{23}=0.0\hat{i}+0.0\hat{j}+0.0\hat{k}$.

2D-M581:

$\hat{n}_{15}=0.53\hat{i}-0.27\hat{j}+0.8\hat{k}$,\;\;\;$\hat{n}_{23}=0.82\hat{i}+0.42\hat{j}+0.4\hat{k}$,\;\;\;$\hat{n}_{25}=-0.01\hat{i}+0.7\hat{j}-0.71\hat{k}$,\;\;\;$\hat{n}_{34}=0.58\hat{i}-0.58\hat{j}-0.58\hat{k}$,\newline
$\vec{r}_{14}=0.0\hat{i}+10.0\hat{j}+0.0\hat{k}$,\;\;\;$\vec{r}_{15}=10.0\hat{i}+0.0\hat{j}+10.0\hat{k}$.

2D-M582:

$\hat{n}_{13}=0.23\hat{i}-0.75\hat{j}-0.62\hat{k}$,\;\;\;$\hat{n}_{14}=0.0\hat{i}-0.71\hat{j}+0.71\hat{k}$,\;\;\;$\hat{n}_{24}=0.58\hat{i}+0.58\hat{j}+0.58\hat{k}$,\;\;\;$\hat{n}_{25}=-0.82\hat{i}+0.41\hat{j}+0.41\hat{k}$,\newline
$\vec{r}_{25}=0.0\hat{i}+0.0\hat{j}+0.0\hat{k}$,\;\;\;$\vec{r}_{35}=10.0\hat{i}+10.0\hat{j}+10.0\hat{k}$.

2D-M583:

$\hat{n}_{13}=-0.67\hat{i}+0.45\hat{j}+0.59\hat{k}$,\;\;\;$\hat{n}_{14}=-0.53\hat{i}+0.27\hat{j}-0.8\hat{k}$,\;\;\;$\hat{n}_{24}=0.56\hat{i}-0.6\hat{j}-0.57\hat{k}$,\;\;\;$\hat{n}_{35}=-0.53\hat{i}+0.27\hat{j}-0.8\hat{k}$,\newline
$\vec{r}_{25}=10.0\hat{i}+0.0\hat{j}+10.0\hat{k}$,\;\;\;$\vec{r}_{35}=0.0\hat{i}+10.0\hat{j}+0.0\hat{k}$.

2D-M584:

$\hat{n}_{13}=-0.25\hat{i}-0.55\hat{j}+0.8\hat{k}$,\;\;\;$\hat{n}_{14}=-0.82\hat{i}-0.38\hat{j}-0.43\hat{k}$,\;\;\;$\hat{n}_{24}=0.0\hat{i}+0.75\hat{j}-0.66\hat{k}$,\;\;\;$\hat{n}_{25}=-0.58\hat{i}+0.54\hat{j}+0.61\hat{k}$,\newline
$\vec{r}_{24}=10.0\hat{i}+0.0\hat{j}+10.0\hat{k}$,\;\;\;$\vec{r}_{35}=0.0\hat{i}+10.0\hat{j}+0.0\hat{k}$.

2D-M585:

$\hat{n}_{13}=-0.02\hat{i}+0.7\hat{j}-0.72\hat{k}$,\;\;\;$\hat{n}_{14}=0.58\hat{i}-0.58\hat{j}-0.58\hat{k}$,\;\;\;$\hat{n}_{24}=0.8\hat{i}+0.52\hat{j}+0.28\hat{k}$,\;\;\;$\hat{n}_{35}=0.58\hat{i}-0.58\hat{j}-0.58\hat{k}$,\newline
$\vec{r}_{24}=0.0\hat{i}+10.0\hat{j}+0.0\hat{k}$,\;\;\;$\vec{r}_{25}=10.0\hat{i}+0.0\hat{j}+10.0\hat{k}$.

2D-M586:

$\hat{n}_{13}=-0.57\hat{i}-0.49\hat{j}+0.66\hat{k}$,\;\;\;$\hat{n}_{14}=0.82\hat{i}-0.41\hat{j}+0.41\hat{k}$,\;\;\;$\hat{n}_{25}=-0.58\hat{i}-0.59\hat{j}+0.56\hat{k}$,\;\;\;$\hat{n}_{35}=0.82\hat{i}-0.41\hat{j}+0.41\hat{k}$,\newline
$\vec{r}_{24}=10.0\hat{i}+10.0\hat{j}+0.0\hat{k}$,\;\;\;$\vec{r}_{35}=0.0\hat{i}+0.0\hat{j}+10.0\hat{k}$.

2D-M587:

$\hat{n}_{13}=-0.05\hat{i}+0.71\hat{j}+0.71\hat{k}$,\;\;\;$\hat{n}_{14}=-0.36\hat{i}-0.66\hat{j}+0.66\hat{k}$,\;\;\;$\hat{n}_{25}=0.93\hat{i}-0.25\hat{j}+0.25\hat{k}$,\;\;\;$\hat{n}_{35}=-0.0\hat{i}+0.71\hat{j}-0.71\hat{k}$,\newline
$\vec{r}_{24}=0.0\hat{i}+0.0\hat{j}+10.0\hat{k}$,\;\;\;$\vec{r}_{25}=10.0\hat{i}+10.0\hat{j}+0.0\hat{k}$.

2D-M588:

$\hat{n}_{13}=0.36\hat{i}+0.66\hat{j}+0.66\hat{k}$,\;\;\;$\hat{n}_{14}=-0.0\hat{i}+0.71\hat{j}+0.71\hat{k}$,\;\;\;$\hat{n}_{23}=-0.93\hat{i}+0.25\hat{j}+0.25\hat{k}$,\;\;\;$\hat{n}_{45}=-0.05\hat{i}-0.71\hat{j}+0.71\hat{k}$,\newline
$\vec{r}_{23}=0.0\hat{i}+0.0\hat{j}+0.0\hat{k}$,\;\;\;$\vec{r}_{24}=10.0\hat{i}+10.0\hat{j}+10.0\hat{k}$.

2D-M589:

$\hat{n}_{13}=0.97\hat{i}-0.11\hat{j}+0.2\hat{k}$,\;\;\;$\hat{n}_{14}=0.71\hat{i}-0.7\hat{j}+0.1\hat{k}$,\;\;\;$\hat{n}_{23}=0.48\hat{i}-0.87\hat{j}+0.06\hat{k}$,\;\;\;$\hat{n}_{35}=-0.19\hat{i}-0.87\hat{j}+0.45\hat{k}$,\newline
$\vec{r}_{23}=4.03\hat{i}+6.0\hat{j}+5.93\hat{k}$,\;\;\;$\vec{r}_{24}=6.07\hat{i}+6.19\hat{j}+4.65\hat{k}$.

2D-M590:

$\hat{n}_{13}=0.57\hat{i}+0.49\hat{j}+0.66\hat{k}$,\;\;\;$\hat{n}_{14}=-0.58\hat{i}-0.59\hat{j}-0.56\hat{k}$,\;\;\;$\hat{n}_{23}=0.82\hat{i}-0.41\hat{j}-0.41\hat{k}$,\;\;\;$\hat{n}_{25}=0.26\hat{i}-0.84\hat{j}+0.47\hat{k}$,\newline
$\vec{r}_{23}=0.0\hat{i}+0.0\hat{j}+0.0\hat{k}$,\;\;\;$\vec{r}_{24}=10.0\hat{i}+10.0\hat{j}+10.0\hat{k}$.

2D-M591:

$\hat{n}_{13}=-0.0\hat{i}+0.0\hat{j}+1.0\hat{k}$,\;\;\;$\hat{n}_{14}=-0.53\hat{i}+0.27\hat{j}-0.8\hat{k}$,\;\;\;$\hat{n}_{24}=-0.62\hat{i}-0.77\hat{j}+0.15\hat{k}$,\;\;\;$\hat{n}_{25}=-0.58\hat{i}+0.58\hat{j}+0.58\hat{k}$,\newline
$\vec{r}_{14}=10.0\hat{i}+0.0\hat{j}+10.0\hat{k}$,\;\;\;$\vec{r}_{35}=0.0\hat{i}+10.0\hat{j}+0.0\hat{k}$.

2D-M592:

$\hat{n}_{13}=0.76\hat{i}+0.65\hat{j}-0.0\hat{k}$,\;\;\;$\hat{n}_{14}=0.63\hat{i}+0.63\hat{j}-0.46\hat{k}$,\;\;\;$\hat{n}_{24}=-0.0\hat{i}-0.0\hat{j}+1.0\hat{k}$,\;\;\;$\hat{n}_{35}=0.0\hat{i}+0.0\hat{j}-1.0\hat{k}$,\newline
$\vec{r}_{14}=0.0\hat{i}+0.0\hat{j}+0.0\hat{k}$,\;\;\;$\vec{r}_{25}=10.0\hat{i}+10.0\hat{j}+10.0\hat{k}$.

2D-M593:

$\hat{n}_{13}=0.03\hat{i}+0.87\hat{j}+0.49\hat{k}$,\;\;\;$\hat{n}_{14}=0.55\hat{i}-0.55\hat{j}-0.63\hat{k}$,\;\;\;$\hat{n}_{25}=-0.0\hat{i}-0.0\hat{j}+1.0\hat{k}$,\;\;\;$\hat{n}_{35}=-0.45\hat{i}+0.45\hat{j}-0.77\hat{k}$,\newline
$\vec{r}_{14}=10.0\hat{i}+0.0\hat{j}+0.0\hat{k}$,\;\;\;$\vec{r}_{24}=0.0\hat{i}+10.0\hat{j}+10.0\hat{k}$.

2D-M594:

$\hat{n}_{13}=0.01\hat{i}+0.7\hat{j}-0.71\hat{k}$,\;\;\;$\hat{n}_{14}=0.47\hat{i}+0.35\hat{j}-0.81\hat{k}$,\;\;\;$\hat{n}_{23}=-0.82\hat{i}+0.42\hat{j}+0.4\hat{k}$,\;\;\;$\hat{n}_{25}=-0.58\hat{i}-0.58\hat{j}-0.58\hat{k}$,\newline
$\vec{r}_{14}=0.0\hat{i}+0.0\hat{j}+0.0\hat{k}$,\;\;\;$\vec{r}_{45}=10.0\hat{i}+10.0\hat{j}+10.0\hat{k}$.

2D-M595:

$\hat{n}_{13}=0.58\hat{i}-0.82\hat{j}+0.0\hat{k}$,\;\;\;$\hat{n}_{14}=-0.34\hat{i}+0.47\hat{j}+0.81\hat{k}$,\;\;\;$\hat{n}_{23}=-0.0\hat{i}+0.0\hat{j}+1.0\hat{k}$,\;\;\;$\hat{n}_{45}=0.6\hat{i}-0.56\hat{j}+0.57\hat{k}$,\newline
$\vec{r}_{14}=0.0\hat{i}+10.0\hat{j}+10.0\hat{k}$,\;\;\;$\vec{r}_{25}=10.0\hat{i}+0.0\hat{j}+0.0\hat{k}$.

2D-M596:

$\hat{n}_{13}=-0.81\hat{i}-0.48\hat{j}-0.33\hat{k}$,\;\;\;$\hat{n}_{14}=-0.81\hat{i}-0.48\hat{j}-0.33\hat{k}$,\;\;\;$\hat{n}_{23}=0.58\hat{i}-0.58\hat{j}-0.58\hat{k}$,\;\;\;$\hat{n}_{45}=-0.06\hat{i}+0.64\hat{j}-0.77\hat{k}$,\newline
$\vec{r}_{14}=10.0\hat{i}+0.0\hat{j}+10.0\hat{k}$,\;\;\;$\vec{r}_{24}=0.0\hat{i}+10.0\hat{j}+0.0\hat{k}$.

2D-M597:

$\hat{n}_{13}=-0.84\hat{i}-0.37\hat{j}+0.41\hat{k}$,\;\;\;$\hat{n}_{14}=-0.13\hat{i}-0.99\hat{j}-0.01\hat{k}$,\;\;\;$\hat{n}_{23}=-0.19\hat{i}-0.98\hat{j}-0.03\hat{k}$,\;\;\;$\hat{n}_{35}=0.32\hat{i}-0.93\hat{j}-0.17\hat{k}$,\newline
$\vec{r}_{14}=5.77\hat{i}+4.06\hat{j}+3.99\hat{k}$,\;\;\;$\vec{r}_{24}=5.34\hat{i}+4.63\hat{j}+6.04\hat{k}$.

2D-M598:

$\hat{n}_{13}=-0.71\hat{i}+0.71\hat{j}-0.0\hat{k}$,\;\;\;$\hat{n}_{14}=-0.07\hat{i}-0.67\hat{j}+0.74\hat{k}$,\;\;\;$\hat{n}_{23}=0.58\hat{i}+0.58\hat{j}+0.58\hat{k}$,\;\;\;$\hat{n}_{25}=0.0\hat{i}-0.0\hat{j}-1.0\hat{k}$,\newline
$\vec{r}_{14}=10.0\hat{i}+10.0\hat{j}+10.0\hat{k}$,\;\;\;$\vec{r}_{24}=0.0\hat{i}+0.0\hat{j}+0.0\hat{k}$.

2D-M599:

$\hat{n}_{13}=0.65\hat{i}+0.55\hat{j}-0.53\hat{k}$,\;\;\;$\hat{n}_{14}=0.0\hat{i}-0.0\hat{j}+1.0\hat{k}$,\;\;\;$\hat{n}_{25}=-0.4\hat{i}-0.34\hat{j}-0.85\hat{k}$,\;\;\;$\hat{n}_{45}=0.7\hat{i}+0.71\hat{j}-0.0\hat{k}$,\newline
$\vec{r}_{14}=10.0\hat{i}+10.0\hat{j}+2.98\hat{k}$,\;\;\;$\vec{r}_{23}=0.0\hat{i}+0.0\hat{j}+5.77\hat{k}$.

2D-M600:

$\hat{n}_{13}=-0.21\hat{i}+0.58\hat{j}-0.79\hat{k}$,\;\;\;$\hat{n}_{14}=0.21\hat{i}-0.58\hat{j}+0.79\hat{k}$,\;\;\;$\hat{n}_{24}=-0.58\hat{i}+0.58\hat{j}+0.58\hat{k}$,\;\;\;$\hat{n}_{45}=-0.01\hat{i}+0.81\hat{j}+0.59\hat{k}$,\newline
$\vec{r}_{14}=0.0\hat{i}+10.0\hat{j}+0.0\hat{k}$,\;\;\;$\vec{r}_{23}=10.0\hat{i}+0.0\hat{j}+10.0\hat{k}$.

2D-M601:

$\hat{n}_{13}=-0.77\hat{i}-0.63\hat{j}-0.12\hat{k}$,\;\;\;$\hat{n}_{14}=-0.82\hat{i}-0.58\hat{j}-0.04\hat{k}$,\;\;\;$\hat{n}_{24}=0.35\hat{i}-0.91\hat{j}+0.22\hat{k}$,\;\;\;$\hat{n}_{35}=0.63\hat{i}-0.77\hat{j}+0.03\hat{k}$,\newline
$\vec{r}_{14}=4.03\hat{i}+4.08\hat{j}+4.09\hat{k}$,\;\;\;$\vec{r}_{23}=4.01\hat{i}+5.96\hat{j}+5.94\hat{k}$.

2D-M602:

$\hat{n}_{13}=0.57\hat{i}+0.49\hat{j}-0.66\hat{k}$,\;\;\;$\hat{n}_{14}=0.82\hat{i}-0.41\hat{j}+0.41\hat{k}$,\;\;\;$\hat{n}_{24}=0.58\hat{i}+0.59\hat{j}-0.56\hat{k}$,\;\;\;$\hat{n}_{25}=0.57\hat{i}+0.29\hat{j}+0.77\hat{k}$,\newline
$\vec{r}_{14}=10.0\hat{i}+10.0\hat{j}+0.0\hat{k}$,\;\;\;$\vec{r}_{23}=0.0\hat{i}+0.0\hat{j}+10.0\hat{k}$.

2D-M603:

$\hat{n}_{13}=-0.57\hat{i}-0.64\hat{j}+0.51\hat{k}$,\;\;\;$\hat{n}_{24}=0.82\hat{i}-0.41\hat{j}+0.41\hat{k}$,\;\;\;$\hat{n}_{25}=0.58\hat{i}+0.56\hat{j}-0.59\hat{k}$,\;\;\;$\hat{n}_{35}=0.82\hat{i}-0.41\hat{j}+0.41\hat{k}$,\newline
$\vec{r}_{14}=0.0\hat{i}+0.0\hat{j}+10.0\hat{k}$,\;\;\;$\vec{r}_{35}=10.0\hat{i}+10.0\hat{j}+0.0\hat{k}$.

2D-M604:

$\hat{n}_{13}=-0.03\hat{i}+0.71\hat{j}-0.71\hat{k}$,\;\;\;$\hat{n}_{24}=-0.36\hat{i}+0.66\hat{j}+0.66\hat{k}$,\;\;\;$\hat{n}_{25}=0.93\hat{i}+0.25\hat{j}+0.25\hat{k}$,\;\;\;$\hat{n}_{35}=0.0\hat{i}+0.71\hat{j}+0.71\hat{k}$,\newline
$\vec{r}_{14}=0.0\hat{i}+10.0\hat{j}+0.0\hat{k}$,\;\;\;$\vec{r}_{25}=10.0\hat{i}+0.0\hat{j}+10.0\hat{k}$.

2D-M605:

$\hat{n}_{13}=0.04\hat{i}+0.71\hat{j}+0.71\hat{k}$,\;\;\;$\hat{n}_{24}=0.93\hat{i}+0.25\hat{j}-0.25\hat{k}$,\;\;\;$\hat{n}_{25}=-0.36\hat{i}+0.66\hat{j}-0.66\hat{k}$,\;\;\;$\hat{n}_{35}=0.0\hat{i}+0.71\hat{j}-0.71\hat{k}$,\newline
$\vec{r}_{14}=0.0\hat{i}+10.0\hat{j}+10.0\hat{k}$,\;\;\;$\vec{r}_{24}=10.0\hat{i}+0.0\hat{j}+0.0\hat{k}$.

2D-M606:

$\hat{n}_{13}=0.82\hat{i}+0.38\hat{j}+0.44\hat{k}$,\;\;\;$\hat{n}_{23}=-0.04\hat{i}-0.72\hat{j}+0.69\hat{k}$,\;\;\;$\hat{n}_{25}=-0.58\hat{i}+0.58\hat{j}+0.58\hat{k}$,\;\;\;$\hat{n}_{45}=-0.07\hat{i}+0.67\hat{j}-0.74\hat{k}$,\newline
$\vec{r}_{14}=10.0\hat{i}+0.0\hat{j}+10.0\hat{k}$,\;\;\;$\vec{r}_{45}=0.0\hat{i}+10.0\hat{j}+0.0\hat{k}$.

2D-M607:

$\hat{n}_{13}=-0.02\hat{i}+0.65\hat{j}+0.76\hat{k}$,\;\;\;$\hat{n}_{23}=1.0\hat{i}+0.0\hat{j}+0.02\hat{k}$,\;\;\;$\hat{n}_{25}=0.01\hat{i}+0.76\hat{j}-0.65\hat{k}$,\;\;\;$\hat{n}_{45}=-0.58\hat{i}-0.53\hat{j}-0.62\hat{k}$,\newline
$\vec{r}_{14}=0.0\hat{i}+0.0\hat{j}+0.0\hat{k}$,\;\;\;$\vec{r}_{25}=10.0\hat{i}+10.0\hat{j}+10.0\hat{k}$.

2D-M608:

$\hat{n}_{13}=0.0\hat{i}+0.0\hat{j}+1.0\hat{k}$,\;\;\;$\hat{n}_{23}=-0.59\hat{i}+0.7\hat{j}+0.39\hat{k}$,\;\;\;$\hat{n}_{24}=0.76\hat{i}+0.65\hat{j}-0.02\hat{k}$,\;\;\;$\hat{n}_{45}=-0.1\hat{i}-0.92\hat{j}-0.39\hat{k}$,\newline
$\vec{r}_{14}=10.0\hat{i}+0.0\hat{j}+10.0\hat{k}$,\;\;\;$\vec{r}_{24}=0.0\hat{i}+10.0\hat{j}+0.0\hat{k}$.

2D-M609:

$\hat{n}_{13}=0.79\hat{i}+0.27\hat{j}+0.55\hat{k}$,\;\;\;$\hat{n}_{23}=-0.11\hat{i}-0.98\hat{j}+0.18\hat{k}$,\;\;\;$\hat{n}_{24}=-0.02\hat{i}-0.99\hat{j}+0.11\hat{k}$,\;\;\;$\hat{n}_{35}=-0.6\hat{i}+0.19\hat{j}+0.77\hat{k}$,\newline
$\vec{r}_{14}=3.89\hat{i}+5.76\hat{j}+4.46\hat{k}$,\;\;\;$\vec{r}_{24}=3.89\hat{i}+5.39\hat{j}+6.11\hat{k}$.

2D-M610:

$\hat{n}_{13}=0.45\hat{i}+0.36\hat{j}+0.81\hat{k}$,\;\;\;$\hat{n}_{23}=-0.58\hat{i}-0.58\hat{j}+0.58\hat{k}$,\;\;\;$\hat{n}_{24}=-0.33\hat{i}-0.48\hat{j}-0.81\hat{k}$,\;\;\;$\hat{n}_{25}=-0.44\hat{i}-0.71\hat{j}+0.56\hat{k}$,\newline
$\vec{r}_{14}=0.0\hat{i}+0.0\hat{j}+10.0\hat{k}$,\;\;\;$\vec{r}_{24}=10.0\hat{i}+10.0\hat{j}+0.0\hat{k}$.

2D-M611:

$\hat{n}_{13}=0.37\hat{i}-0.93\hat{j}-0.0\hat{k}$,\;\;\;$\hat{n}_{23}=0.93\hat{i}+0.37\hat{j}+0.05\hat{k}$,\;\;\;$\hat{n}_{25}=0.0\hat{i}-0.0\hat{j}+1.0\hat{k}$,\;\;\;$\hat{n}_{45}=0.0\hat{i}+0.79\hat{j}+0.61\hat{k}$,\newline
$\vec{r}_{14}=10.0\hat{i}+0.0\hat{j}+10.0\hat{k}$,\;\;\;$\vec{r}_{23}=0.0\hat{i}+10.0\hat{j}+0.0\hat{k}$.

2D-M612:

$\hat{n}_{13}=-0.82\hat{i}-0.38\hat{j}-0.43\hat{k}$,\;\;\;$\hat{n}_{23}=0.0\hat{i}+0.75\hat{j}-0.66\hat{k}$,\;\;\;$\hat{n}_{24}=-0.58\hat{i}+0.54\hat{j}+0.61\hat{k}$,\;\;\;$\hat{n}_{45}=0.41\hat{i}+0.36\hat{j}-0.84\hat{k}$,\newline
$\vec{r}_{14}=0.0\hat{i}+10.0\hat{j}+0.0\hat{k}$,\;\;\;$\vec{r}_{23}=10.0\hat{i}+0.0\hat{j}+10.0\hat{k}$.

2D-M613:

$\hat{n}_{13}=0.76\hat{i}-0.62\hat{j}-0.18\hat{k}$,\;\;\;$\hat{n}_{23}=-0.09\hat{i}-0.83\hat{j}-0.56\hat{k}$,\;\;\;$\hat{n}_{24}=0.21\hat{i}-0.89\hat{j}+0.4\hat{k}$,\;\;\;$\hat{n}_{35}=-0.55\hat{i}-0.77\hat{j}+0.33\hat{k}$,\newline
$\vec{r}_{14}=6.72\hat{i}+5.99\hat{j}+6.41\hat{k}$,\;\;\;$\vec{r}_{23}=3.54\hat{i}+3.37\hat{j}+3.29\hat{k}$.

2D-M614:

$\hat{n}_{13}=0.75\hat{i}-0.5\hat{j}+0.43\hat{k}$,\;\;\;$\hat{n}_{23}=-0.13\hat{i}+0.52\hat{j}+0.84\hat{k}$,\;\;\;$\hat{n}_{24}=-0.61\hat{i}+0.71\hat{j}-0.35\hat{k}$,\;\;\;$\hat{n}_{25}=-0.0\hat{i}+0.0\hat{j}-1.0\hat{k}$,\newline
$\vec{r}_{14}=10.0\hat{i}+0.0\hat{j}+0.0\hat{k}$,\;\;\;$\vec{r}_{23}=0.0\hat{i}+10.0\hat{j}+10.0\hat{k}$.

2D-M615:

$\hat{n}_{13}=0.83\hat{i}+0.22\hat{j}+0.52\hat{k}$,\;\;\;$\hat{n}_{24}=0.89\hat{i}+0.46\hat{j}+0.0\hat{k}$,\;\;\;$\hat{n}_{25}=-0.0\hat{i}+0.0\hat{j}+1.0\hat{k}$,\;\;\;$\hat{n}_{35}=-0.0\hat{i}+0.58\hat{j}-0.82\hat{k}$,\newline
$\vec{r}_{13}=10.0\hat{i}+10.0\hat{j}+0.0\hat{k}$,\;\;\;$\vec{r}_{14}=0.0\hat{i}+0.0\hat{j}+10.0\hat{k}$.

2D-M616:

$\hat{n}_{13}=-0.56\hat{i}+0.63\hat{j}+0.54\hat{k}$,\;\;\;$\hat{n}_{23}=-0.56\hat{i}-0.77\hat{j}+0.31\hat{k}$,\;\;\;$\hat{n}_{25}=0.61\hat{i}-0.13\hat{j}+0.78\hat{k}$,\;\;\;$\hat{n}_{45}=0.0\hat{i}-0.0\hat{j}-1.0\hat{k}$,\newline
$\vec{r}_{13}=0.0\hat{i}+10.0\hat{j}+10.0\hat{k}$,\;\;\;$\vec{r}_{14}=10.0\hat{i}+0.0\hat{j}+0.0\hat{k}$.

2D-M617:

$\hat{n}_{13}=-0.82\hat{i}+0.41\hat{j}+0.41\hat{k}$,\;\;\;$\hat{n}_{23}=-0.0\hat{i}+0.71\hat{j}-0.71\hat{k}$,\;\;\;$\hat{n}_{24}=-0.58\hat{i}-0.58\hat{j}-0.58\hat{k}$,\;\;\;$\hat{n}_{45}=-0.03\hat{i}+0.78\hat{j}+0.63\hat{k}$,\newline
$\vec{r}_{13}=0.0\hat{i}+0.0\hat{j}+0.0\hat{k}$,\;\;\;$\vec{r}_{14}=10.0\hat{i}+10.0\hat{j}+10.0\hat{k}$.

2D-M618:

$\hat{n}_{13}=-0.7\hat{i}+0.71\hat{j}-0.01\hat{k}$,\;\;\;$\hat{n}_{23}=0.7\hat{i}-0.71\hat{j}+0.01\hat{k}$,\;\;\;$\hat{n}_{24}=-0.58\hat{i}-0.58\hat{j}-0.58\hat{k}$,\;\;\;$\hat{n}_{35}=0.01\hat{i}-0.0\hat{j}-1.0\hat{k}$,\newline
$\vec{r}_{13}=10.0\hat{i}+10.0\hat{j}+10.0\hat{k}$,\;\;\;$\vec{r}_{14}=0.0\hat{i}+0.0\hat{j}+0.0\hat{k}$.

2D-M619:

$\hat{n}_{13}=-0.46\hat{i}-0.21\hat{j}-0.86\hat{k}$,\;\;\;$\hat{n}_{23}=-0.58\hat{i}-0.67\hat{j}+0.47\hat{k}$,\;\;\;$\hat{n}_{24}=-0.7\hat{i}-0.63\hat{j}+0.33\hat{k}$,\;\;\;$\hat{n}_{25}=0.0\hat{i}+0.0\hat{j}-1.0\hat{k}$,\newline
$\vec{r}_{13}=10.0\hat{i}+10.0\hat{j}+0.0\hat{k}$,\;\;\;$\vec{r}_{14}=0.0\hat{i}+0.0\hat{j}+10.0\hat{k}$.
