# Supplementary material for: Dimensional synthesis of spatial manipulators for velocity and force transmission for operation around a specified task point
Source: arXiv:2210.04446 source file (2022-10-10)
Supplement: Supplementary file 7 [file classappendix11.tex]

\subsection{Class 11} \label{appendix_five_2_1}
2D-M620:

$\hat{n}_{14}=-0.28\hat{i}-0.96\hat{j}+0.04\hat{k}$,\;\;\;$\hat{n}_{24}=0.96\hat{i}-0.28\hat{j}+0.07\hat{k}$,\;\;\;$\hat{n}_{25}=-0.18\hat{i}-0.76\hat{j}-0.63\hat{k}$,\;\;\;$\hat{n}_{34}=-0.8\hat{i}-0.26\hat{j}+0.54\hat{k}$,\newline
$\hat{n}_{35}=0.57\hat{i}-0.6\hat{j}+0.56\hat{k}$,\;\;\;$\vec{r}_{25}=5.33\hat{i}+4.37\hat{j}+4.5\hat{k}$,\;\;\;$\vec{r}_{34}=5.5\hat{i}+5.08\hat{j}+4.04\hat{k}$,\;\;\;$\vec{r}_{35}=5.23\hat{i}+5.61\hat{j}+4.85\hat{k}$.

2D-M621:

$\hat{n}_{14}=-0.12\hat{i}-0.92\hat{j}-0.37\hat{k}$,\;\;\;$\hat{n}_{24}=-0.05\hat{i}-0.64\hat{j}+0.76\hat{k}$,\;\;\;$\hat{n}_{25}=0.99\hat{i}-0.12\hat{j}-0.04\hat{k}$,\;\;\;$\hat{n}_{34}=-0.54\hat{i}-0.63\hat{j}-0.56\hat{k}$,\newline
$\hat{n}_{35}=0.84\hat{i}-0.44\hat{j}-0.32\hat{k}$,\;\;\;$\vec{r}_{24}=5.61\hat{i}+4.52\hat{j}+4.72\hat{k}$,\;\;\;$\vec{r}_{34}=5.32\hat{i}+4.61\hat{j}+5.69\hat{k}$,\;\;\;$\vec{r}_{35}=5.68\hat{i}+4.49\hat{j}+4.87\hat{k}$.

2D-M622:

$\hat{n}_{14}=0.13\hat{i}-0.96\hat{j}+0.26\hat{k}$,\;\;\;$\hat{n}_{23}=-0.74\hat{i}-0.27\hat{j}-0.62\hat{k}$,\;\;\;$\hat{n}_{25}=-0.55\hat{i}-0.3\hat{j}+0.78\hat{k}$,\;\;\;$\hat{n}_{34}=0.39\hat{i}-0.92\hat{j}-0.07\hat{k}$,\newline
$\hat{n}_{45}=0.74\hat{i}+0.27\hat{j}+0.62\hat{k}$,\;\;\;$\vec{r}_{25}=5.57\hat{i}+2.78\hat{j}+5.57\hat{k}$,\;\;\;$\vec{r}_{34}=5.22\hat{i}+5.68\hat{j}+5.16\hat{k}$,\;\;\;$\vec{r}_{45}=4.79\hat{i}+5.09\hat{j}+5.42\hat{k}$.

2D-M623:

$\hat{n}_{14}=-0.62\hat{i}-0.79\hat{j}+0.02\hat{k}$,\;\;\;$\hat{n}_{23}=-0.19\hat{i}-0.57\hat{j}-0.8\hat{k}$,\;\;\;$\hat{n}_{25}=0.76\hat{i}-0.59\hat{j}+0.25\hat{k}$,\;\;\;$\hat{n}_{34}=-0.62\hat{i}-0.56\hat{j}+0.55\hat{k}$,\newline
$\hat{n}_{45}=0.76\hat{i}-0.59\hat{j}+0.25\hat{k}$,\;\;\;$\vec{r}_{23}=5.03\hat{i}+5.53\hat{j}+5.53\hat{k}$,\;\;\;$\vec{r}_{34}=5.47\hat{i}+5.5\hat{j}+5.13\hat{k}$,\;\;\;$\vec{r}_{45}=4.75\hat{i}+4.83\hat{j}+4.97\hat{k}$.

2D-M624:

$\hat{n}_{14}=0.28\hat{i}-0.95\hat{j}-0.15\hat{k}$,\;\;\;$\hat{n}_{23}=-0.65\hat{i}+0.36\hat{j}-0.67\hat{k}$,\;\;\;$\hat{n}_{25}=0.0\hat{i}-0.88\hat{j}-0.47\hat{k}$,\;\;\;$\hat{n}_{34}=-0.76\hat{i}-0.31\hat{j}+0.57\hat{k}$,\newline
$\hat{n}_{45}=0.76\hat{i}+0.31\hat{j}-0.57\hat{k}$,\;\;\;$\vec{r}_{23}=5.46\hat{i}+4.8\hat{j}+4.59\hat{k}$,\;\;\;$\vec{r}_{25}=5.47\hat{i}+5.47\hat{j}+5.46\hat{k}$,\;\;\;$\vec{r}_{45}=5.41\hat{i}+4.87\hat{j}+4.83\hat{k}$.

2D-M625:

$\hat{n}_{14}=-0.82\hat{i}-0.53\hat{j}+0.21\hat{k}$,\;\;\;$\hat{n}_{23}=-0.72\hat{i}-0.55\hat{j}-0.43\hat{k}$,\;\;\;$\hat{n}_{25}=0.13\hat{i}-0.71\hat{j}+0.69\hat{k}$,\;\;\;$\hat{n}_{34}=0.68\hat{i}-0.44\hat{j}-0.58\hat{k}$,\newline
$\hat{n}_{45}=0.55\hat{i}-0.83\hat{j}+0.08\hat{k}$,\;\;\;$\vec{r}_{23}=5.29\hat{i}+5.23\hat{j}+4.71\hat{k}$,\;\;\;$\vec{r}_{25}=5.24\hat{i}+4.87\hat{j}+4.94\hat{k}$,\;\;\;$\vec{r}_{34}=5.27\hat{i}+4.71\hat{j}+4.75\hat{k}$.

2D-M626:

$\hat{n}_{13}=0.92\hat{i}-0.21\hat{j}-0.34\hat{k}$,\;\;\;$\hat{n}_{14}=0.0\hat{i}+0.85\hat{j}-0.53\hat{k}$,\;\;\;$\hat{n}_{24}=-0.7\hat{i}+0.38\hat{j}+0.61\hat{k}$,\;\;\;$\hat{n}_{25}=0.72\hat{i}+0.37\hat{j}+0.59\hat{k}$,\newline
$\hat{n}_{35}=-0.0\hat{i}+0.85\hat{j}-0.53\hat{k}$,\;\;\;$\vec{r}_{24}=5.1\hat{i}+5.02\hat{j}+4.88\hat{k}$,\;\;\;$\vec{r}_{25}=4.98\hat{i}+4.97\hat{j}+4.7\hat{k}$,\;\;\;$\vec{r}_{35}=5.0\hat{i}+5.34\hat{j}+4.97\hat{k}$.

2D-M627:

$\hat{n}_{13}=-0.3\hat{i}-0.95\hat{j}+0.01\hat{k}$,\;\;\;$\hat{n}_{14}=-0.14\hat{i}-0.97\hat{j}+0.21\hat{k}$,\;\;\;$\hat{n}_{24}=0.76\hat{i}-0.24\hat{j}-0.61\hat{k}$,\;\;\;$\hat{n}_{25}=0.64\hat{i}+0.07\hat{j}+0.77\hat{k}$,\newline
$\hat{n}_{35}=-0.76\hat{i}+0.24\hat{j}+0.61\hat{k}$,\;\;\;$\vec{r}_{14}=4.84\hat{i}+5.25\hat{j}+5.19\hat{k}$,\;\;\;$\vec{r}_{25}=4.92\hat{i}+4.76\hat{j}+4.77\hat{k}$,\;\;\;$\vec{r}_{35}=5.12\hat{i}+4.84\hat{j}+5.2\hat{k}$.

2D-M628:

$\hat{n}_{13}=0.29\hat{i}-0.93\hat{j}-0.21\hat{k}$,\;\;\;$\hat{n}_{14}=0.37\hat{i}-0.59\hat{j}+0.72\hat{k}$,\;\;\;$\hat{n}_{24}=0.12\hat{i}-0.74\hat{j}-0.67\hat{k}$,\;\;\;$\hat{n}_{25}=-0.92\hat{i}-0.33\hat{j}+0.2\hat{k}$,\newline
$\hat{n}_{35}=-0.92\hat{i}-0.33\hat{j}+0.2\hat{k}$,\;\;\;$\vec{r}_{14}=6.32\hat{i}+6.38\hat{j}+4.93\hat{k}$,\;\;\;$\vec{r}_{24}=6.43\hat{i}+6.16\hat{j}+4.07\hat{k}$,\;\;\;$\vec{r}_{35}=6.02\hat{i}+5.53\hat{j}+6.45\hat{k}$.

2D-M629:

$\hat{n}_{13}=0.74\hat{i}-0.68\hat{j}+0.01\hat{k}$,\;\;\;$\hat{n}_{14}=-0.89\hat{i}-0.36\hat{j}+0.27\hat{k}$,\;\;\;$\hat{n}_{24}=0.12\hat{i}-0.77\hat{j}-0.62\hat{k}$,\;\;\;$\hat{n}_{25}=0.43\hat{i}-0.52\hat{j}+0.73\hat{k}$,\newline
$\hat{n}_{35}=-0.68\hat{i}-0.74\hat{j}-0.01\hat{k}$,\;\;\;$\vec{r}_{14}=5.03\hat{i}+4.8\hat{j}+5.77\hat{k}$,\;\;\;$\vec{r}_{24}=5.76\hat{i}+4.26\hat{j}+5.22\hat{k}$,\;\;\;$\vec{r}_{25}=4.62\hat{i}+4.42\hat{j}+4.9\hat{k}$.

2D-M630:

$\hat{n}_{13}=0.8\hat{i}-0.38\hat{j}-0.46\hat{k}$,\;\;\;$\hat{n}_{14}=-0.48\hat{i}+0.78\hat{j}-0.4\hat{k}$,\;\;\;$\hat{n}_{23}=0.09\hat{i}-0.68\hat{j}+0.73\hat{k}$,\;\;\;$\hat{n}_{25}=0.59\hat{i}+0.62\hat{j}+0.51\hat{k}$,\newline
$\hat{n}_{45}=0.65\hat{i}+0.01\hat{j}-0.76\hat{k}$,\;\;\;$\vec{r}_{14}=4.7\hat{i}+5.66\hat{j}+4.83\hat{k}$,\;\;\;$\vec{r}_{25}=6.03\hat{i}+5.58\hat{j}+4.55\hat{k}$,\;\;\;$\vec{r}_{45}=4.74\hat{i}+5.38\hat{j}+4.36\hat{k}$.

2D-M631:

$\hat{n}_{13}=-0.6\hat{i}-0.75\hat{j}+0.26\hat{k}$,\;\;\;$\hat{n}_{14}=0.13\hat{i}-0.83\hat{j}-0.54\hat{k}$,\;\;\;$\hat{n}_{23}=0.68\hat{i}-0.32\hat{j}+0.66\hat{k}$,\;\;\;$\hat{n}_{25}=0.41\hat{i}-0.57\hat{j}-0.71\hat{k}$,\newline
$\hat{n}_{45}=-0.72\hat{i}-0.45\hat{j}+0.52\hat{k}$,\;\;\;$\vec{r}_{14}=4.8\hat{i}+5.04\hat{j}+5.14\hat{k}$,\;\;\;$\vec{r}_{23}=4.8\hat{i}+5.08\hat{j}+5.19\hat{k}$,\;\;\;$\vec{r}_{45}=4.8\hat{i}+4.92\hat{j}+5.14\hat{k}$.

2D-M632:

$\hat{n}_{13}=-0.55\hat{i}+0.61\hat{j}+0.57\hat{k}$,\;\;\;$\hat{n}_{14}=0.55\hat{i}-0.61\hat{j}-0.57\hat{k}$,\;\;\;$\hat{n}_{23}=0.66\hat{i}-0.1\hat{j}+0.74\hat{k}$,\;\;\;$\hat{n}_{25}=-0.51\hat{i}-0.79\hat{j}+0.35\hat{k}$,\newline
$\hat{n}_{45}=0.82\hat{i}+0.25\hat{j}+0.52\hat{k}$,\;\;\;$\vec{r}_{14}=5.03\hat{i}+5.08\hat{j}+4.43\hat{k}$,\;\;\;$\vec{r}_{23}=4.96\hat{i}+4.92\hat{j}+4.61\hat{k}$,\;\;\;$\vec{r}_{25}=4.99\hat{i}+5.5\hat{j}+4.97\hat{k}$.

2D-M633:

$\hat{n}_{13}=-0.22\hat{i}-0.66\hat{j}+0.71\hat{k}$,\;\;\;$\hat{n}_{14}=-0.22\hat{i}-0.66\hat{j}+0.71\hat{k}$,\;\;\;$\hat{n}_{23}=-0.94\hat{i}-0.06\hat{j}-0.34\hat{k}$,\;\;\;$\hat{n}_{24}=0.27\hat{i}-0.74\hat{j}-0.61\hat{k}$,\newline
$\hat{n}_{45}=0.43\hat{i}-0.72\hat{j}-0.54\hat{k}$,\;\;\;$\vec{r}_{14}=5.81\hat{i}+4.94\hat{j}+5.59\hat{k}$,\;\;\;$\vec{r}_{23}=5.82\hat{i}+5.62\hat{j}+5.68\hat{k}$,\;\;\;$\vec{r}_{24}=5.41\hat{i}+5.81\hat{j}+4.83\hat{k}$.

2D-M634:

$\hat{n}_{13}=-0.36\hat{i}-0.72\hat{j}-0.59\hat{k}$,\;\;\;$\hat{n}_{14}=-0.83\hat{i}-0.54\hat{j}+0.1\hat{k}$,\;\;\;$\hat{n}_{23}=0.14\hat{i}-0.98\hat{j}+0.1\hat{k}$,\;\;\;$\hat{n}_{24}=-0.05\hat{i}-0.98\hat{j}-0.19\hat{k}$,\newline
$\hat{n}_{35}=0.91\hat{i}-0.41\hat{j}-0.05\hat{k}$,\;\;\;$\vec{r}_{14}=5.41\hat{i}+6.3\hat{j}+5.72\hat{k}$,\;\;\;$\vec{r}_{23}=6.29\hat{i}+4.07\hat{j}+4.39\hat{k}$,\;\;\;$\vec{r}_{24}=4.55\hat{i}+5.87\hat{j}+5.73\hat{k}$.

2D-M635:

$\hat{n}_{13}=-0.64\hat{i}-0.34\hat{j}+0.68\hat{k}$,\;\;\;$\hat{n}_{14}=0.82\hat{i}-0.35\hat{j}-0.45\hat{k}$,\;\;\;$\hat{n}_{23}=-0.56\hat{i}-0.4\hat{j}-0.73\hat{k}$,\;\;\;$\hat{n}_{24}=-0.08\hat{i}-0.85\hat{j}+0.52\hat{k}$,\newline
$\hat{n}_{25}=0.53\hat{i}-0.84\hat{j}+0.08\hat{k}$,\;\;\;$\vec{r}_{14}=5.14\hat{i}+4.94\hat{j}+4.73\hat{k}$,\;\;\;$\vec{r}_{23}=4.92\hat{i}+4.92\hat{j}+5.18\hat{k}$,\;\;\;$\vec{r}_{24}=5.28\hat{i}+5.07\hat{j}+4.34\hat{k}$.

2D-M636:

$\hat{n}_{13}=0.71\hat{i}+0.58\hat{j}+0.41\hat{k}$,\;\;\;$\hat{n}_{14}=0.1\hat{i}-0.65\hat{j}+0.75\hat{k}$,\;\;\;$\hat{n}_{24}=0.92\hat{i}-0.23\hat{j}-0.32\hat{k}$,\;\;\;$\hat{n}_{25}=-0.38\hat{i}-0.72\hat{j}-0.58\hat{k}$,\newline
$\hat{n}_{35}=-0.7\hat{i}+0.49\hat{j}+0.52\hat{k}$,\;\;\;$\vec{r}_{13}=5.53\hat{i}+4.39\hat{j}+5.47\hat{k}$,\;\;\;$\vec{r}_{14}=5.67\hat{i}+4.41\hat{j}+5.69\hat{k}$,\;\;\;$\vec{r}_{35}=4.4\hat{i}+5.62\hat{j}+4.11\hat{k}$.

2D-M637:

$\hat{n}_{13}=-0.23\hat{i}-0.83\hat{j}+0.51\hat{k}$,\;\;\;$\hat{n}_{14}=0.39\hat{i}-0.56\hat{j}-0.74\hat{k}$,\;\;\;$\hat{n}_{24}=-0.23\hat{i}-0.83\hat{j}+0.51\hat{k}$,\;\;\;$\hat{n}_{25}=0.89\hat{i}+0.03\hat{j}+0.45\hat{k}$,\newline
$\hat{n}_{35}=-0.97\hat{i}+0.18\hat{j}-0.14\hat{k}$,\;\;\;$\vec{r}_{13}=3.21\hat{i}+4.86\hat{j}+5.67\hat{k}$,\;\;\;$\vec{r}_{14}=5.98\hat{i}+4.92\hat{j}+3.95\hat{k}$,\;\;\;$\vec{r}_{25}=5.09\hat{i}+4.22\hat{j}+5.31\hat{k}$.

2D-M638:

$\hat{n}_{13}=0.38\hat{i}-0.92\hat{j}+0.12\hat{k}$,\;\;\;$\hat{n}_{14}=0.47\hat{i}+0.08\hat{j}-0.88\hat{k}$,\;\;\;$\hat{n}_{24}=-0.79\hat{i}-0.4\hat{j}-0.46\hat{k}$,\;\;\;$\hat{n}_{25}=0.38\hat{i}-0.92\hat{j}+0.12\hat{k}$,\newline
$\hat{n}_{35}=-0.91\hat{i}-0.35\hat{j}+0.22\hat{k}$,\;\;\;$\vec{r}_{13}=5.58\hat{i}+5.48\hat{j}+5.37\hat{k}$,\;\;\;$\vec{r}_{14}=5.7\hat{i}+4.44\hat{j}+4.83\hat{k}$,\;\;\;$\vec{r}_{24}=4.21\hat{i}+5.3\hat{j}+5.78\hat{k}$.

2D-M639:

$\hat{n}_{13}=0.77\hat{i}-0.16\hat{j}+0.62\hat{k}$,\;\;\;$\hat{n}_{14}=0.42\hat{i}-0.6\hat{j}-0.68\hat{k}$,\;\;\;$\hat{n}_{23}=0.42\hat{i}-0.6\hat{j}-0.68\hat{k}$,\;\;\;$\hat{n}_{24}=-0.48\hat{i}-0.79\hat{j}+0.4\hat{k}$,\newline
$\hat{n}_{45}=-0.6\hat{i}-0.75\hat{j}+0.29\hat{k}$,\;\;\;$\vec{r}_{13}=4.51\hat{i}+5.52\hat{j}+4.98\hat{k}$,\;\;\;$\vec{r}_{14}=4.46\hat{i}+5.27\hat{j}+5.44\hat{k}$,\;\;\;$\vec{r}_{24}=4.6\hat{i}+5.54\hat{j}+5.22\hat{k}$.

2D-M640:

$\hat{n}_{13}=0.83\hat{i}-0.46\hat{j}+0.31\hat{k}$,\;\;\;$\hat{n}_{14}=-0.21\hat{i}-0.78\hat{j}-0.6\hat{k}$,\;\;\;$\hat{n}_{23}=0.83\hat{i}-0.46\hat{j}+0.31\hat{k}$,\;\;\;$\hat{n}_{24}=-0.51\hat{i}-0.43\hat{j}+0.74\hat{k}$,\newline
$\hat{n}_{35}=-0.5\hat{i}-0.86\hat{j}+0.06\hat{k}$,\;\;\;$\vec{r}_{13}=4.66\hat{i}+5.31\hat{j}+5.3\hat{k}$,\;\;\;$\vec{r}_{14}=4.67\hat{i}+5.05\hat{j}+4.71\hat{k}$,\;\;\;$\vec{r}_{24}=5.26\hat{i}+4.83\hat{j}+4.96\hat{k}$.

2D-M641:

$\hat{n}_{13}=-0.59\hat{i}-0.49\hat{j}+0.64\hat{k}$,\;\;\;$\hat{n}_{14}=0.81\hat{i}-0.38\hat{j}+0.45\hat{k}$,\;\;\;$\hat{n}_{23}=0.69\hat{i}-0.72\hat{j}+0.08\hat{k}$,\;\;\;$\hat{n}_{24}=-0.02\hat{i}-0.78\hat{j}-0.62\hat{k}$,\newline
$\hat{n}_{25}=-0.72\hat{i}-0.68\hat{j}+0.09\hat{k}$,\;\;\;$\vec{r}_{13}=5.42\hat{i}+5.52\hat{j}+5.21\hat{k}$,\;\;\;$\vec{r}_{14}=5.48\hat{i}+4.49\hat{j}+5.19\hat{k}$,\;\;\;$\vec{r}_{24}=5.53\hat{i}+5.39\hat{j}+5.46\hat{k}$.
