# Supplementary material for: Dimensional synthesis of spatial manipulators for velocity and force transmission for operation around a specified task point
Source: arXiv:2210.04446 source file (2022-10-10)
Supplement: Supplementary file 8 [file classappendix3.tex]

\subsection{Class 3} \label{appendix_five_2_1}
{\tiny 2D-M21:}

$\hat{n}_{14}=0.0\hat{i}+0.86\hat{j}+0.51\hat{k}$,\;\;\;$\hat{n}_{24}=-0.68\hat{i}+0.06\hat{j}-0.73\hat{k}$,\;\;\;$\hat{n}_{25}=0.58\hat{i}-0.58\hat{j}-0.58\hat{k}$,\;\;\;$\vec{r}_{14}=0.0\hat{i}+10.0\hat{j}+10.0\hat{k}$,\newline
$\vec{r}_{34}=0.0\hat{i}+10.0\hat{j}+0.0\hat{k}$,\;\;\;$\vec{r}_{35}=10.0\hat{i}+0.0\hat{j}+10.0\hat{k}$.

{\tiny 2D-M22:}

$\hat{n}_{14}=0.0\hat{i}+0.0\hat{j}-1.0\hat{k}$,\;\;\;$\hat{n}_{25}=0.0\hat{i}+0.0\hat{j}+1.0\hat{k}$,\;\;\;$\hat{n}_{45}=0.0\hat{i}+0.62\hat{j}+0.79\hat{k}$,\;\;\;$\vec{r}_{14}=10.0\hat{i}+10.0\hat{j}+0.03\hat{k}$,\newline
$\vec{r}_{23}=10.0\hat{i}+0.0\hat{j}+10.0\hat{k}$,\;\;\;$\vec{r}_{34}=0.0\hat{i}+10.0\hat{j}+0.0\hat{k}$.

{\tiny 2D-M23:}

$\hat{n}_{14}=0.0\hat{i}+0.79\hat{j}+0.61\hat{k}$,\;\;\;$\hat{n}_{34}=0.58\hat{i}-0.58\hat{j}-0.58\hat{k}$,\;\;\;$\hat{n}_{45}=0.0\hat{i}+0.73\hat{j}+0.69\hat{k}$,\;\;\;$\vec{r}_{14}=0.0\hat{i}+10.0\hat{j}+10.0\hat{k}$,\newline
$\vec{r}_{23}=10.0\hat{i}+0.0\hat{j}+10.0\hat{k}$,\;\;\;$\vec{r}_{25}=0.0\hat{i}+10.0\hat{j}+0.0\hat{k}$.

{\tiny 2D-M24:}

$\hat{n}_{14}=0.21\hat{i}+0.81\hat{j}+0.55\hat{k}$,\;\;\;$\hat{n}_{24}=-0.0\hat{i}+0.0\hat{j}+1.0\hat{k}$,\;\;\;$\hat{n}_{25}=0.0\hat{i}+0.0\hat{j}-1.0\hat{k}$,\;\;\;$\vec{r}_{24}=0.0\hat{i}+10.0\hat{j}+3.96\hat{k}$,\newline
$\vec{r}_{34}=0.0\hat{i}+0.0\hat{j}+0.0\hat{k}$,\;\;\;$\vec{r}_{35}=10.0\hat{i}+10.0\hat{j}+10.0\hat{k}$.

{\tiny 2D-M25:}

$\hat{n}_{14}=0.0\hat{i}+0.0\hat{j}-1.0\hat{k}$,\;\;\;$\hat{n}_{24}=-0.58\hat{i}+0.58\hat{j}+0.58\hat{k}$,\;\;\;$\hat{n}_{25}=0.26\hat{i}-0.46\hat{j}+0.85\hat{k}$,\;\;\;$\vec{r}_{25}=10.0\hat{i}+0.0\hat{j}+10.0\hat{k}$,\newline
$\vec{r}_{34}=10.0\hat{i}+0.0\hat{j}+10.0\hat{k}$,\;\;\;$\vec{r}_{35}=0.0\hat{i}+10.0\hat{j}+0.0\hat{k}$.

{\tiny 2D-M26:}

$\hat{n}_{14}=-0.0\hat{i}+1.0\hat{j}-0.0\hat{k}$,\;\;\;$\hat{n}_{25}=-0.71\hat{i}+0.71\hat{j}+0.0\hat{k}$,\;\;\;$\hat{n}_{45}=0.0\hat{i}+0.0\hat{j}-1.0\hat{k}$,\;\;\;$\vec{r}_{23}=0.0\hat{i}+0.0\hat{j}+0.0\hat{k}$,\newline
$\vec{r}_{25}=10.0\hat{i}+10.0\hat{j}+0.0\hat{k}$,\;\;\;$\vec{r}_{34}=10.0\hat{i}+10.0\hat{j}+10.0\hat{k}$.

{\tiny 2D-M27:}

$\hat{n}_{14}=-0.1\hat{i}-0.04\hat{j}+0.99\hat{k}$,\;\;\;$\hat{n}_{25}=-0.73\hat{i}-0.61\hat{j}+0.31\hat{k}$,\;\;\;$\hat{n}_{45}=-0.27\hat{i}-0.4\hat{j}-0.88\hat{k}$,\;\;\;$\vec{r}_{23}=5.31\hat{i}+4.46\hat{j}+4.41\hat{k}$,\newline
$\vec{r}_{34}=4.99\hat{i}+4.55\hat{j}+5.58\hat{k}$,\;\;\;$\vec{r}_{45}=10.0\hat{i}+10.0\hat{j}+0.0\hat{k}$.

{\tiny 2D-M28:}

$\hat{n}_{14}=-0.0\hat{i}+1.0\hat{j}-0.0\hat{k}$,\;\;\;$\hat{n}_{34}=-0.71\hat{i}+0.71\hat{j}-0.0\hat{k}$,\;\;\;$\hat{n}_{45}=-0.0\hat{i}+0.0\hat{j}-1.0\hat{k}$,\;\;\;$\vec{r}_{23}=0.0\hat{i}+0.0\hat{j}+0.0\hat{k}$,\newline
$\vec{r}_{25}=10.0\hat{i}+10.0\hat{j}+10.0\hat{k}$,\;\;\;$\vec{r}_{34}=10.0\hat{i}+10.0\hat{j}+0.0\hat{k}$.

{\tiny 2D-M29:}

$\hat{n}_{14}=0.52\hat{i}-0.5\hat{j}+0.69\hat{k}$,\;\;\;$\hat{n}_{34}=-0.13\hat{i}-0.58\hat{j}+0.81\hat{k}$,\;\;\;$\hat{n}_{45}=-0.25\hat{i}+0.91\hat{j}-0.35\hat{k}$,\;\;\;$\vec{r}_{23}=3.3\hat{i}+3.38\hat{j}+6.5\hat{k}$,\newline
$\vec{r}_{25}=4.87\hat{i}+6.69\hat{j}+6.68\hat{k}$,\;\;\;$\vec{r}_{45}=0.0\hat{i}+0.0\hat{j}+0.0\hat{k}$.

{\tiny 2D-M30:}

$\hat{n}_{13}=0.81\hat{i}-0.38\hat{j}-0.44\hat{k}$,\;\;\;$\hat{n}_{14}=0.58\hat{i}-0.58\hat{j}-0.58\hat{k}$,\;\;\;$\hat{n}_{35}=0.58\hat{i}-0.58\hat{j}-0.58\hat{k}$,\;\;\;$\vec{r}_{13}=10.0\hat{i}+10.0\hat{j}+10.0\hat{k}$,\newline
$\vec{r}_{24}=0.0\hat{i}+10.0\hat{j}+0.0\hat{k}$,\;\;\;$\vec{r}_{25}=10.0\hat{i}+0.0\hat{j}+10.0\hat{k}$.

{\tiny 2D-M31:}

$\hat{n}_{13}=0.0\hat{i}+0.71\hat{j}-0.71\hat{k}$,\;\;\;$\hat{n}_{14}=0.01\hat{i}+0.71\hat{j}-0.7\hat{k}$,\;\;\;$\hat{n}_{45}=-0.58\hat{i}+0.58\hat{j}+0.58\hat{k}$,\;\;\;$\vec{r}_{13}=0.0\hat{i}+0.0\hat{j}+0.0\hat{k}$,\newline
$\vec{r}_{23}=10.0\hat{i}+0.0\hat{j}+10.0\hat{k}$,\;\;\;$\vec{r}_{25}=0.0\hat{i}+10.0\hat{j}+0.0\hat{k}$.

{\tiny 2D-M32:}

$\hat{n}_{13}=0.09\hat{i}-0.77\hat{j}+0.63\hat{k}$,\;\;\;$\hat{n}_{14}=0.21\hat{i}-0.82\hat{j}+0.53\hat{k}$,\;\;\;$\hat{n}_{45}=-0.82\hat{i}-0.45\hat{j}-0.36\hat{k}$,\;\;\;$\vec{r}_{13}=6.51\hat{i}+3.35\hat{j}+4.18\hat{k}$,\newline
$\vec{r}_{23}=4.5\hat{i}+6.92\hat{j}+6.91\hat{k}$,\;\;\;$\vec{r}_{24}=4.66\hat{i}+4.14\hat{j}+6.71\hat{k}$.

{\tiny 2D-M33:}

$\hat{n}_{13}=-0.7\hat{i}+0.01\hat{j}+0.72\hat{k}$,\;\;\;$\hat{n}_{14}=0.0\hat{i}+0.71\hat{j}-0.71\hat{k}$,\;\;\;$\hat{n}_{35}=-0.0\hat{i}+0.54\hat{j}+0.84\hat{k}$,\;\;\;$\vec{r}_{13}=10.0\hat{i}+10.0\hat{j}+10.0\hat{k}$,\newline
$\vec{r}_{23}=10.0\hat{i}+0.0\hat{j}+0.0\hat{k}$,\;\;\;$\vec{r}_{24}=0.0\hat{i}+10.0\hat{j}+10.0\hat{k}$.

{\tiny 2D-M34:}

$\hat{n}_{13}=-0.0\hat{i}+0.71\hat{j}-0.71\hat{k}$,\;\;\;$\hat{n}_{14}=-0.58\hat{i}-0.58\hat{j}-0.58\hat{k}$,\;\;\;$\hat{n}_{35}=0.04\hat{i}-0.73\hat{j}+0.68\hat{k}$,\;\;\;$\vec{r}_{24}=10.0\hat{i}+10.0\hat{j}+10.0\hat{k}$,\newline
$\vec{r}_{25}=0.0\hat{i}+0.0\hat{j}+0.0\hat{k}$,\;\;\;$\vec{r}_{35}=0.0\hat{i}+10.0\hat{j}+0.0\hat{k}$.

{\tiny 2D-M35:}

$\hat{n}_{13}=-0.58\hat{i}+0.58\hat{j}-0.58\hat{k}$,\;\;\;$\hat{n}_{14}=0.0\hat{i}+0.71\hat{j}-0.71\hat{k}$,\;\;\;$\hat{n}_{45}=-0.08\hat{i}+0.62\hat{j}-0.78\hat{k}$,\;\;\;$\vec{r}_{23}=10.0\hat{i}+0.0\hat{j}+0.0\hat{k}$,\newline
$\vec{r}_{24}=0.0\hat{i}+10.0\hat{j}+10.0\hat{k}$,\;\;\;$\vec{r}_{45}=10.0\hat{i}+10.0\hat{j}+10.0\hat{k}$.
