# Supplementary material for: Dimensional synthesis of spatial manipulators for velocity and force transmission for operation around a specified task point
Source: arXiv:2210.04446 source file (2022-10-10)
Supplement: Supplementary file 9 [file classappendix5.tex]

\subsection{Class 5} \label{appendix_five_2_1}
{\tiny 2D-M41:}

$\hat{n}_{14}=0.81\hat{i}-0.55\hat{j}+0.2\hat{k}$,\;\;\;$\hat{n}_{24}=-0.0\hat{i}+0.51\hat{j}+0.86\hat{k}$,\;\;\;$\hat{n}_{25}=-0.32\hat{i}+0.65\hat{j}-0.69\hat{k}$,\;\;\;$\hat{n}_{34}=0.36\hat{i}-0.31\hat{j}-0.88\hat{k}$,\newline
$\vec{r}_{14}=10.0\hat{i}+10.0\hat{j}+0.0\hat{k}$,\;\;\;$\vec{r}_{24}=10.0\hat{i}+10.0\hat{j}+0.0\hat{k}$,\;\;\;$\vec{r}_{25}=10.0\hat{i}+0.0\hat{j}+10.0\hat{k}$,\;\;\;$\vec{r}_{34}=10.0\hat{i}+10.0\hat{j}+10.0\hat{k}$,\newline
$\vec{r}_{35}=0.0\hat{i}+0.0\hat{j}+0.0\hat{k}$.

{\tiny 2D-M42:}

$\hat{n}_{14}=0.0\hat{i}+0.95\hat{j}-0.3\hat{k}$,\;\;\;$\hat{n}_{24}=-0.0\hat{i}+0.0\hat{j}-1.0\hat{k}$,\;\;\;$\hat{n}_{25}=0.62\hat{i}-0.68\hat{j}+0.4\hat{k}$,\;\;\;$\hat{n}_{35}=0.8\hat{i}+0.57\hat{j}-0.2\hat{k}$,\newline
$\vec{r}_{14}=0.0\hat{i}+0.0\hat{j}+0.0\hat{k}$,\;\;\;$\vec{r}_{24}=10.0\hat{i}+10.0\hat{j}+1.2\hat{k}$,\;\;\;$\vec{r}_{25}=10.0\hat{i}+10.0\hat{j}+0.0\hat{k}$,\;\;\;$\vec{r}_{34}=0.0\hat{i}+0.0\hat{j}+0.0\hat{k}$,\newline
$\vec{r}_{35}=10.0\hat{i}+0.0\hat{j}+10.0\hat{k}$.

{\tiny 2D-M43:}

$\hat{n}_{14}=0.68\hat{i}+0.56\hat{j}-0.47\hat{k}$,\;\;\;$\hat{n}_{24}=-0.42\hat{i}-0.62\hat{j}+0.66\hat{k}$,\;\;\;$\hat{n}_{25}=0.14\hat{i}+0.82\hat{j}-0.55\hat{k}$,\;\;\;$\hat{n}_{34}=-0.0\hat{i}+0.84\hat{j}+0.54\hat{k}$,\newline
$\vec{r}_{14}=0.0\hat{i}+10.0\hat{j}+10.0\hat{k}$,\;\;\;$\vec{r}_{24}=0.0\hat{i}+0.0\hat{j}+0.0\hat{k}$,\;\;\;$\vec{r}_{25}=10.0\hat{i}+0.0\hat{j}+10.0\hat{k}$,\;\;\;$\vec{r}_{34}=10.0\hat{i}+0.0\hat{j}+0.0\hat{k}$,\newline
$\vec{r}_{35}=0.0\hat{i}+10.0\hat{j}+10.0\hat{k}$.

{\tiny 2D-M44:}

$\hat{n}_{14}=0.7\hat{i}-0.1\hat{j}+0.7\hat{k}$,\;\;\;$\hat{n}_{24}=0.74\hat{i}-0.18\hat{j}+0.65\hat{k}$,\;\;\;$\hat{n}_{25}=-0.87\hat{i}-0.07\hat{j}-0.48\hat{k}$,\;\;\;$\hat{n}_{35}=-0.19\hat{i}-0.59\hat{j}+0.78\hat{k}$,\newline
$\vec{r}_{14}=10.0\hat{i}+0.0\hat{j}+10.0\hat{k}$,\;\;\;$\vec{r}_{24}=10.0\hat{i}+10.0\hat{j}+0.0\hat{k}$,\;\;\;$\vec{r}_{25}=10.0\hat{i}+0.0\hat{j}+10.0\hat{k}$,\;\;\;$\vec{r}_{34}=0.0\hat{i}+0.0\hat{j}+0.0\hat{k}$,\newline
$\vec{r}_{35}=10.0\hat{i}+10.0\hat{j}+10.0\hat{k}$.

{\tiny 2D-M45:}

$\hat{n}_{14}=-0.4\hat{i}-0.28\hat{j}+0.87\hat{k}$,\;\;\;$\hat{n}_{24}=0.63\hat{i}+0.63\hat{j}+0.46\hat{k}$,\;\;\;$\hat{n}_{34}=0.84\hat{i}-0.2\hat{j}-0.5\hat{k}$,\;\;\;$\hat{n}_{35}=0.12\hat{i}-0.64\hat{j}+0.76\hat{k}$,\newline
$\vec{r}_{14}=10.0\hat{i}+10.0\hat{j}+10.0\hat{k}$,\;\;\;$\vec{r}_{24}=10.0\hat{i}+0.0\hat{j}+0.0\hat{k}$,\;\;\;$\vec{r}_{25}=0.0\hat{i}+10.0\hat{j}+0.0\hat{k}$,\;\;\;$\vec{r}_{34}=10.0\hat{i}+10.0\hat{j}+10.0\hat{k}$,\newline
$\vec{r}_{35}=10.0\hat{i}+0.0\hat{j}+10.0\hat{k}$.

{\tiny 2D-M46:}

$\hat{n}_{14}=-0.62\hat{i}-0.71\hat{j}-0.32\hat{k}$,\;\;\;$\hat{n}_{24}=0.58\hat{i}+0.71\hat{j}+0.39\hat{k}$,\;\;\;$\hat{n}_{25}=0.55\hat{i}-0.12\hat{j}+0.83\hat{k}$,\;\;\;$\hat{n}_{35}=0.13\hat{i}-0.7\hat{j}+0.7\hat{k}$,\newline
$\vec{r}_{14}=0.0\hat{i}+10.0\hat{j}+0.0\hat{k}$,\;\;\;$\vec{r}_{24}=10.0\hat{i}+0.0\hat{j}+10.0\hat{k}$,\;\;\;$\vec{r}_{25}=0.0\hat{i}+0.0\hat{j}+10.0\hat{k}$,\;\;\;$\vec{r}_{34}=0.0\hat{i}+10.0\hat{j}+0.0\hat{k}$,\newline
$\vec{r}_{35}=10.0\hat{i}+10.0\hat{j}+10.0\hat{k}$.

{\tiny 2D-M47:}

$\hat{n}_{14}=0.82\hat{i}-0.53\hat{j}-0.24\hat{k}$,\;\;\;$\hat{n}_{23}=-0.0\hat{i}+0.85\hat{j}-0.52\hat{k}$,\;\;\;$\hat{n}_{25}=0.0\hat{i}+0.0\hat{j}+1.0\hat{k}$,\;\;\;$\hat{n}_{34}=0.38\hat{i}+0.92\hat{j}+0.0\hat{k}$,\newline
$\vec{r}_{14}=10.0\hat{i}+10.0\hat{j}+10.0\hat{k}$,\;\;\;$\vec{r}_{23}=0.0\hat{i}+10.0\hat{j}+0.0\hat{k}$,\;\;\;$\vec{r}_{25}=10.0\hat{i}+10.0\hat{j}+9.45\hat{k}$,\;\;\;$\vec{r}_{34}=10.0\hat{i}+0.0\hat{j}+10.0\hat{k}$,\newline
$\vec{r}_{45}=0.0\hat{i}+10.0\hat{j}+10.0\hat{k}$.

{\tiny 2D-M48:}

$\hat{n}_{14}=0.0\hat{i}+0.0\hat{j}+1.0\hat{k}$,\;\;\;$\hat{n}_{23}=-0.64\hat{i}+0.64\hat{j}-0.43\hat{k}$,\;\;\;$\hat{n}_{25}=0.09\hat{i}-0.7\hat{j}+0.7\hat{k}$,\;\;\;$\hat{n}_{45}=-0.49\hat{i}+0.5\hat{j}+0.72\hat{k}$,\newline
$\vec{r}_{14}=10.0\hat{i}+0.0\hat{j}+10.0\hat{k}$,\;\;\;$\vec{r}_{23}=10.0\hat{i}+10.0\hat{j}+0.0\hat{k}$,\;\;\;$\vec{r}_{25}=10.0\hat{i}+0.0\hat{j}+10.0\hat{k}$,\;\;\;$\vec{r}_{34}=0.0\hat{i}+0.0\hat{j}+0.0\hat{k}$,\newline
$\vec{r}_{45}=10.0\hat{i}+10.0\hat{j}+10.0\hat{k}$.

{\tiny 2D-M49:}

$\hat{n}_{14}=0.82\hat{i}+0.55\hat{j}-0.11\hat{k}$,\;\;\;$\hat{n}_{23}=0.0\hat{i}+0.58\hat{j}+0.81\hat{k}$,\;\;\;$\hat{n}_{25}=0.67\hat{i}-0.3\hat{j}+0.67\hat{k}$,\;\;\;$\hat{n}_{34}=-0.71\hat{i}+0.0\hat{j}+0.71\hat{k}$,\newline
$\vec{r}_{14}=10.0\hat{i}+0.0\hat{j}+10.0\hat{k}$,\;\;\;$\vec{r}_{23}=10.0\hat{i}+0.0\hat{j}+0.0\hat{k}$,\;\;\;$\vec{r}_{25}=0.0\hat{i}+0.0\hat{j}+0.0\hat{k}$,\;\;\;$\vec{r}_{34}=0.0\hat{i}+10.0\hat{j}+10.0\hat{k}$,\newline
$\vec{r}_{45}=10.0\hat{i}+0.0\hat{j}+0.0\hat{k}$.

{\tiny 2D-M50:}

$\hat{n}_{14}=-0.3\hat{i}+0.61\hat{j}+0.73\hat{k}$,\;\;\;$\hat{n}_{23}=0.77\hat{i}+0.62\hat{j}-0.15\hat{k}$,\;\;\;$\hat{n}_{25}=-0.53\hat{i}-0.06\hat{j}-0.85\hat{k}$,\;\;\;$\hat{n}_{45}=-0.49\hat{i}-0.54\hat{j}+0.68\hat{k}$,\newline
$\vec{r}_{14}=0.0\hat{i}+10.0\hat{j}+10.0\hat{k}$,\;\;\;$\vec{r}_{23}=0.0\hat{i}+10.0\hat{j}+10.0\hat{k}$,\;\;\;$\vec{r}_{25}=0.0\hat{i}+10.0\hat{j}+0.0\hat{k}$,\;\;\;$\vec{r}_{34}=10.0\hat{i}+0.0\hat{j}+0.0\hat{k}$,\newline
$\vec{r}_{45}=10.0\hat{i}+10.0\hat{j}+10.0\hat{k}$.

{\tiny 2D-M51:}

$\hat{n}_{14}=0.28\hat{i}-0.63\hat{j}+0.72\hat{k}$,\;\;\;$\hat{n}_{23}=-0.0\hat{i}+0.0\hat{j}+1.0\hat{k}$,\;\;\;$\hat{n}_{34}=0.71\hat{i}-0.71\hat{j}-0.0\hat{k}$,\;\;\;$\hat{n}_{45}=-0.37\hat{i}-0.37\hat{j}-0.85\hat{k}$,\newline
$\vec{r}_{14}=0.0\hat{i}+10.0\hat{j}+0.0\hat{k}$,\;\;\;$\vec{r}_{23}=10.0\hat{i}+10.0\hat{j}+0.0\hat{k}$,\;\;\;$\vec{r}_{25}=0.0\hat{i}+0.0\hat{j}+0.0\hat{k}$,\;\;\;$\vec{r}_{34}=10.0\hat{i}+10.0\hat{j}+10.0\hat{k}$,\newline
$\vec{r}_{45}=10.0\hat{i}+10.0\hat{j}+0.0\hat{k}$.

{\tiny 2D-M52:}

$\hat{n}_{14}=-0.72\hat{i}+0.08\hat{j}-0.69\hat{k}$,\;\;\;$\hat{n}_{23}=-0.59\hat{i}-0.19\hat{j}-0.78\hat{k}$,\;\;\;$\hat{n}_{34}=-0.0\hat{i}+0.8\hat{j}-0.6\hat{k}$,\;\;\;$\hat{n}_{45}=0.58\hat{i}+0.17\hat{j}+0.8\hat{k}$,\newline
$\vec{r}_{14}=10.0\hat{i}+0.0\hat{j}+10.0\hat{k}$,\;\;\;$\vec{r}_{23}=10.0\hat{i}+10.0\hat{j}+0.0\hat{k}$,\;\;\;$\vec{r}_{25}=0.0\hat{i}+0.0\hat{j}+10.0\hat{k}$,\;\;\;$\vec{r}_{34}=0.0\hat{i}+10.0\hat{j}+0.0\hat{k}$,\newline
$\vec{r}_{45}=10.0\hat{i}+10.0\hat{j}+0.0\hat{k}$.

{\tiny 2D-M53:}

$\hat{n}_{14}=0.25\hat{i}+0.41\hat{j}+0.88\hat{k}$,\;\;\;$\hat{n}_{23}=-0.0\hat{i}+0.21\hat{j}-0.98\hat{k}$,\;\;\;$\hat{n}_{25}=0.66\hat{i}-0.62\hat{j}+0.43\hat{k}$,\;\;\;$\hat{n}_{34}=-0.64\hat{i}+0.56\hat{j}+0.52\hat{k}$,\newline
$\vec{r}_{14}=10.0\hat{i}+10.0\hat{j}+0.0\hat{k}$,\;\;\;$\vec{r}_{23}=0.0\hat{i}+0.0\hat{j}+0.0\hat{k}$,\;\;\;$\vec{r}_{25}=0.0\hat{i}+10.0\hat{j}+0.0\hat{k}$,\;\;\;$\vec{r}_{34}=0.0\hat{i}+10.0\hat{j}+10.0\hat{k}$,\newline
$\vec{r}_{45}=10.0\hat{i}+10.0\hat{j}+0.0\hat{k}$.

{\tiny 2D-M54:}

$\hat{n}_{14}=0.41\hat{i}+0.67\hat{j}+0.61\hat{k}$,\;\;\;$\hat{n}_{23}=0.66\hat{i}+0.6\hat{j}-0.46\hat{k}$,\;\;\;$\hat{n}_{25}=0.71\hat{i}-0.71\hat{j}+0.02\hat{k}$,\;\;\;$\hat{n}_{45}=-0.69\hat{i}+0.72\hat{j}-0.04\hat{k}$,\newline
$\vec{r}_{14}=10.0\hat{i}+0.0\hat{j}+0.0\hat{k}$,\;\;\;$\vec{r}_{23}=0.0\hat{i}+0.0\hat{j}+0.0\hat{k}$,\;\;\;$\vec{r}_{25}=0.0\hat{i}+0.0\hat{j}+10.0\hat{k}$,\;\;\;$\vec{r}_{34}=10.0\hat{i}+10.0\hat{j}+10.0\hat{k}$,\newline
$\vec{r}_{45}=0.0\hat{i}+0.0\hat{j}+10.0\hat{k}$.

{\tiny 2D-M55:}

$\hat{n}_{14}=0.0\hat{i}+0.58\hat{j}+0.81\hat{k}$,\;\;\;$\hat{n}_{23}=-0.46\hat{i}+0.48\hat{j}+0.75\hat{k}$,\;\;\;$\hat{n}_{34}=0.9\hat{i}-0.44\hat{j}-0.0\hat{k}$,\;\;\;$\hat{n}_{45}=-0.7\hat{i}+0.11\hat{j}-0.7\hat{k}$,\newline
$\vec{r}_{14}=10.0\hat{i}+10.0\hat{j}+0.0\hat{k}$,\;\;\;$\vec{r}_{23}=0.0\hat{i}+0.0\hat{j}+10.0\hat{k}$,\;\;\;$\vec{r}_{25}=10.0\hat{i}+10.0\hat{j}+0.0\hat{k}$,\;\;\;$\vec{r}_{34}=10.0\hat{i}+10.0\hat{j}+10.0\hat{k}$,\newline
$\vec{r}_{45}=10.0\hat{i}+0.0\hat{j}+10.0\hat{k}$.

{\tiny 2D-M56:}

$\hat{n}_{14}=0.82\hat{i}-0.52\hat{j}+0.25\hat{k}$,\;\;\;$\hat{n}_{25}=0.0\hat{i}-0.71\hat{j}-0.71\hat{k}$,\;\;\;$\hat{n}_{34}=0.0\hat{i}+0.71\hat{j}+0.71\hat{k}$,\;\;\;$\hat{n}_{45}=-0.93\hat{i}-0.25\hat{j}+0.25\hat{k}$,\newline
$\vec{r}_{14}=10.0\hat{i}+10.0\hat{j}+0.0\hat{k}$,\;\;\;$\vec{r}_{23}=10.0\hat{i}+0.0\hat{j}+0.0\hat{k}$,\;\;\;$\vec{r}_{25}=0.0\hat{i}+9.98\hat{j}+10.0\hat{k}$,\;\;\;$\vec{r}_{34}=10.0\hat{i}+10.0\hat{j}+0.0\hat{k}$,\newline
$\vec{r}_{45}=0.0\hat{i}+10.0\hat{j}+10.0\hat{k}$.

{\tiny 2D-M57:}

$\hat{n}_{14}=-0.7\hat{i}+0.09\hat{j}+0.71\hat{k}$,\;\;\;$\hat{n}_{25}=0.6\hat{i}+0.6\hat{j}-0.54\hat{k}$,\;\;\;$\hat{n}_{34}=-0.68\hat{i}+0.67\hat{j}-0.3\hat{k}$,\;\;\;$\hat{n}_{45}=-0.72\hat{i}-0.5\hat{j}+0.48\hat{k}$,\newline
$\vec{r}_{14}=10.0\hat{i}+10.0\hat{j}+10.0\hat{k}$,\;\;\;$\vec{r}_{23}=0.0\hat{i}+10.0\hat{j}+0.0\hat{k}$,\;\;\;$\vec{r}_{25}=10.0\hat{i}+0.0\hat{j}+0.0\hat{k}$,\;\;\;$\vec{r}_{34}=10.0\hat{i}+10.0\hat{j}+10.0\hat{k}$,\newline
$\vec{r}_{45}=10.0\hat{i}+0.0\hat{j}+0.0\hat{k}$.

{\tiny 2D-M58:}

$\hat{n}_{14}=-0.0\hat{i}+0.85\hat{j}+0.52\hat{k}$,\;\;\;$\hat{n}_{25}=0.34\hat{i}-0.23\hat{j}+0.91\hat{k}$,\;\;\;$\hat{n}_{34}=-0.48\hat{i}-0.73\hat{j}+0.48\hat{k}$,\;\;\;$\hat{n}_{45}=-0.76\hat{i}-0.64\hat{j}-0.01\hat{k}$,\newline
$\vec{r}_{14}=0.0\hat{i}+0.0\hat{j}+10.0\hat{k}$,\;\;\;$\vec{r}_{23}=0.0\hat{i}+10.0\hat{j}+10.0\hat{k}$,\;\;\;$\vec{r}_{25}=10.0\hat{i}+0.0\hat{j}+10.0\hat{k}$,\;\;\;$\vec{r}_{34}=0.0\hat{i}+0.0\hat{j}+0.0\hat{k}$,\newline
$\vec{r}_{45}=10.0\hat{i}+0.0\hat{j}+0.0\hat{k}$.

{\tiny 2D-M59:}

$\hat{n}_{14}=-0.79\hat{i}-0.21\hat{j}+0.58\hat{k}$,\;\;\;$\hat{n}_{15}=-0.4\hat{i}-0.12\hat{j}+0.91\hat{k}$,\;\;\;$\hat{n}_{23}=-0.63\hat{i}-0.63\hat{j}-0.46\hat{k}$,\;\;\;$\hat{n}_{25}=0.0\hat{i}+0.71\hat{j}+0.71\hat{k}$,\newline
$\vec{r}_{14}=0.0\hat{i}+10.0\hat{j}+10.0\hat{k}$,\;\;\;$\vec{r}_{15}=10.0\hat{i}+10.0\hat{j}+10.0\hat{k}$,\;\;\;$\vec{r}_{23}=0.0\hat{i}+10.0\hat{j}+0.0\hat{k}$,\;\;\;$\vec{r}_{25}=0.0\hat{i}+0.0\hat{j}+10.0\hat{k}$,\newline
$\vec{r}_{34}=10.0\hat{i}+0.0\hat{j}+0.0\hat{k}$.

{\tiny 2D-M60:}

$\hat{n}_{14}=0.8\hat{i}-0.54\hat{j}+0.26\hat{k}$,\;\;\;$\hat{n}_{15}=0.35\hat{i}+0.91\hat{j}-0.21\hat{k}$,\;\;\;$\hat{n}_{23}=0.0\hat{i}+0.71\hat{j}+0.71\hat{k}$,\;\;\;$\hat{n}_{34}=-0.16\hat{i}-0.62\hat{j}-0.77\hat{k}$,\newline
$\vec{r}_{14}=10.0\hat{i}+10.0\hat{j}+0.0\hat{k}$,\;\;\;$\vec{r}_{15}=0.0\hat{i}+10.0\hat{j}+10.0\hat{k}$,\;\;\;$\vec{r}_{23}=10.0\hat{i}+0.0\hat{j}+0.0\hat{k}$,\;\;\;$\vec{r}_{25}=0.0\hat{i}+0.0\hat{j}+10.0\hat{k}$,\newline
$\vec{r}_{34}=10.0\hat{i}+10.0\hat{j}+0.0\hat{k}$.

{\tiny 2D-M61:}

$\hat{n}_{14}=-0.67\hat{i}-0.3\hat{j}-0.67\hat{k}$,\;\;\;$\hat{n}_{15}=0.0\hat{i}-0.0\hat{j}+1.0\hat{k}$,\;\;\;$\hat{n}_{25}=0.3\hat{i}+0.67\hat{j}+0.67\hat{k}$,\;\;\;$\hat{n}_{34}=0.71\hat{i}-0.71\hat{j}+0.0\hat{k}$,\newline
$\vec{r}_{14}=10.0\hat{i}+0.0\hat{j}+10.0\hat{k}$,\;\;\;$\vec{r}_{15}=0.0\hat{i}+0.0\hat{j}+7.65\hat{k}$,\;\;\;$\vec{r}_{23}=10.0\hat{i}+10.0\hat{j}+0.0\hat{k}$,\;\;\;$\vec{r}_{25}=0.0\hat{i}+10.0\hat{j}+10.0\hat{k}$,\newline
$\vec{r}_{34}=0.0\hat{i}+0.0\hat{j}+10.0\hat{k}$.

{\tiny 2D-M62:}

$\hat{n}_{14}=0.81\hat{i}-0.54\hat{j}-0.24\hat{k}$,\;\;\;$\hat{n}_{23}=-0.37\hat{i}-0.15\hat{j}-0.91\hat{k}$,\;\;\;$\hat{n}_{25}=0.26\hat{i}+0.72\hat{j}-0.64\hat{k}$,\;\;\;$\hat{n}_{34}=-0.48\hat{i}-0.06\hat{j}+0.88\hat{k}$,\newline
$\vec{r}_{14}=0.0\hat{i}+10.0\hat{j}+10.0\hat{k}$,\;\;\;$\vec{r}_{15}=10.0\hat{i}+10.0\hat{j}+10.0\hat{k}$,\;\;\;$\vec{r}_{23}=10.0\hat{i}+10.0\hat{j}+0.0\hat{k}$,\;\;\;$\vec{r}_{25}=0.0\hat{i}+10.0\hat{j}+0.0\hat{k}$,\newline
$\vec{r}_{34}=10.0\hat{i}+0.0\hat{j}+0.0\hat{k}$.

{\tiny 2D-M63:}

$\hat{n}_{14}=0.68\hat{i}+0.52\hat{j}+0.52\hat{k}$,\;\;\;$\hat{n}_{23}=0.84\hat{i}+0.1\hat{j}-0.53\hat{k}$,\;\;\;$\hat{n}_{25}=0.0\hat{i}+0.0\hat{j}+1.0\hat{k}$,\;\;\;$\hat{n}_{34}=-0.0\hat{i}+0.16\hat{j}-0.99\hat{k}$,\newline
$\vec{r}_{14}=0.0\hat{i}+0.0\hat{j}+10.0\hat{k}$,\;\;\;$\vec{r}_{15}=10.0\hat{i}+0.0\hat{j}+0.0\hat{k}$,\;\;\;$\vec{r}_{23}=10.0\hat{i}+0.0\hat{j}+0.0\hat{k}$,\;\;\;$\vec{r}_{25}=10.0\hat{i}+10.0\hat{j}+1.8\hat{k}$,\newline
$\vec{r}_{34}=0.0\hat{i}+10.0\hat{j}+0.0\hat{k}$.

{\tiny 2D-M64:}

$\hat{n}_{14}=0.0\hat{i}+0.0\hat{j}+1.0\hat{k}$,\;\;\;$\hat{n}_{23}=-0.88\hat{i}+0.23\hat{j}-0.42\hat{k}$,\;\;\;$\hat{n}_{25}=0.47\hat{i}-0.32\hat{j}+0.82\hat{k}$,\;\;\;$\hat{n}_{34}=-0.7\hat{i}-0.67\hat{j}-0.26\hat{k}$,\newline
$\vec{r}_{14}=0.0\hat{i}+10.0\hat{j}+10.0\hat{k}$,\;\;\;$\vec{r}_{15}=10.0\hat{i}+0.0\hat{j}+10.0\hat{k}$,\;\;\;$\vec{r}_{23}=10.0\hat{i}+10.0\hat{j}+0.0\hat{k}$,\;\;\;$\vec{r}_{25}=10.0\hat{i}+0.0\hat{j}+10.0\hat{k}$,\newline
$\vec{r}_{34}=0.0\hat{i}+10.0\hat{j}+10.0\hat{k}$.

{\tiny 2D-M65:}

$\hat{n}_{14}=0.31\hat{i}-0.9\hat{j}+0.32\hat{k}$,\;\;\;$\hat{n}_{23}=0.77\hat{i}+0.37\hat{j}-0.51\hat{k}$,\;\;\;$\hat{n}_{25}=0.32\hat{i}+0.66\hat{j}+0.68\hat{k}$,\;\;\;$\hat{n}_{34}=0.13\hat{i}-0.63\hat{j}-0.76\hat{k}$,\newline
$\vec{r}_{14}=10.0\hat{i}+10.0\hat{j}+0.0\hat{k}$,\;\;\;$\vec{r}_{15}=10.0\hat{i}+0.0\hat{j}+0.0\hat{k}$,\;\;\;$\vec{r}_{23}=10.0\hat{i}+0.0\hat{j}+10.0\hat{k}$,\;\;\;$\vec{r}_{25}=10.0\hat{i}+0.0\hat{j}+0.0\hat{k}$,\newline
$\vec{r}_{34}=0.0\hat{i}+10.0\hat{j}+10.0\hat{k}$.

{\tiny 2D-M66:}

$\hat{n}_{15}=-0.0\hat{i}+0.86\hat{j}+0.51\hat{k}$,\;\;\;$\hat{n}_{23}=0.7\hat{i}-0.7\hat{j}+0.17\hat{k}$,\;\;\;$\hat{n}_{25}=-0.71\hat{i}+0.5\hat{j}+0.5\hat{k}$,\;\;\;$\hat{n}_{34}=-0.15\hat{i}-0.62\hat{j}-0.77\hat{k}$,\newline
$\vec{r}_{14}=0.0\hat{i}+0.0\hat{j}+10.0\hat{k}$,\;\;\;$\vec{r}_{15}=0.0\hat{i}+10.0\hat{j}+10.0\hat{k}$,\;\;\;$\vec{r}_{23}=10.0\hat{i}+10.0\hat{j}+10.0\hat{k}$,\;\;\;$\vec{r}_{25}=10.0\hat{i}+0.0\hat{j}+0.0\hat{k}$,\newline
$\vec{r}_{34}=10.0\hat{i}+10.0\hat{j}+0.0\hat{k}$.

{\tiny 2D-M67:}

$\hat{n}_{13}=0.14\hat{i}+0.99\hat{j}+0.0\hat{k}$,\;\;\;$\hat{n}_{14}=0.39\hat{i}+0.52\hat{j}-0.76\hat{k}$,\;\;\;$\hat{n}_{24}=0.79\hat{i}+0.57\hat{j}-0.23\hat{k}$,\;\;\;$\hat{n}_{25}=-0.61\hat{i}-0.01\hat{j}-0.79\hat{k}$,\newline
$\vec{r}_{13}=0.0\hat{i}+10.0\hat{j}+0.0\hat{k}$,\;\;\;$\vec{r}_{14}=10.0\hat{i}+10.0\hat{j}+10.0\hat{k}$,\;\;\;$\vec{r}_{24}=10.0\hat{i}+0.0\hat{j}+0.0\hat{k}$,\;\;\;$\vec{r}_{25}=10.0\hat{i}+0.0\hat{j}+10.0\hat{k}$,\newline
$\vec{r}_{35}=0.0\hat{i}+10.0\hat{j}+10.0\hat{k}$.

{\tiny 2D-M68:}

$\hat{n}_{13}=0.61\hat{i}+0.15\hat{j}-0.78\hat{k}$,\;\;\;$\hat{n}_{14}=0.57\hat{i}-0.22\hat{j}+0.79\hat{k}$,\;\;\;$\hat{n}_{24}=0.42\hat{i}+0.64\hat{j}-0.64\hat{k}$,\;\;\;$\hat{n}_{35}=-0.52\hat{i}-0.82\hat{j}-0.24\hat{k}$,\newline
$\vec{r}_{13}=10.0\hat{i}+10.0\hat{j}+10.0\hat{k}$,\;\;\;$\vec{r}_{14}=10.0\hat{i}+0.0\hat{j}+10.0\hat{k}$,\;\;\;$\vec{r}_{24}=10.0\hat{i}+10.0\hat{j}+10.0\hat{k}$,\;\;\;$\vec{r}_{25}=0.0\hat{i}+10.0\hat{j}+0.0\hat{k}$,\newline
$\vec{r}_{35}=10.0\hat{i}+0.0\hat{j}+0.0\hat{k}$.

{\tiny 2D-M69:}

$\hat{n}_{13}=0.69\hat{i}-0.03\hat{j}+0.72\hat{k}$,\;\;\;$\hat{n}_{14}=-0.33\hat{i}+0.9\hat{j}+0.29\hat{k}$,\;\;\;$\hat{n}_{24}=-0.51\hat{i}-0.85\hat{j}+0.12\hat{k}$,\;\;\;$\hat{n}_{25}=0.34\hat{i}+0.69\hat{j}-0.64\hat{k}$,\newline
$\vec{r}_{13}=10.0\hat{i}+0.0\hat{j}+10.0\hat{k}$,\;\;\;$\vec{r}_{14}=10.0\hat{i}+10.0\hat{j}+0.0\hat{k}$,\;\;\;$\vec{r}_{24}=10.0\hat{i}+0.0\hat{j}+0.0\hat{k}$,\;\;\;$\vec{r}_{25}=10.0\hat{i}+10.0\hat{j}+10.0\hat{k}$,\newline
$\vec{r}_{35}=0.0\hat{i}+10.0\hat{j}+0.0\hat{k}$.

{\tiny 2D-M70:}

$\hat{n}_{13}=-0.0\hat{i}+0.0\hat{j}-1.0\hat{k}$,\;\;\;$\hat{n}_{14}=0.6\hat{i}+0.54\hat{j}+0.6\hat{k}$,\;\;\;$\hat{n}_{24}=-0.67\hat{i}-0.3\hat{j}+0.68\hat{k}$,\;\;\;$\hat{n}_{35}=0.6\hat{i}+0.49\hat{j}+0.64\hat{k}$,\newline
$\vec{r}_{13}=10.0\hat{i}+0.0\hat{j}+2.68\hat{k}$,\;\;\;$\vec{r}_{14}=0.0\hat{i}+0.0\hat{j}+10.0\hat{k}$,\;\;\;$\vec{r}_{24}=10.0\hat{i}+0.0\hat{j}+0.0\hat{k}$,\;\;\;$\vec{r}_{25}=0.0\hat{i}+10.0\hat{j}+0.0\hat{k}$,\newline
$\vec{r}_{35}=0.0\hat{i}+0.0\hat{j}+10.0\hat{k}$.

{\tiny 2D-M71:}

$\hat{n}_{13}=-0.0\hat{i}+0.68\hat{j}-0.74\hat{k}$,\;\;\;$\hat{n}_{14}=0.7\hat{i}-0.18\hat{j}+0.7\hat{k}$,\;\;\;$\hat{n}_{25}=-0.15\hat{i}+0.7\hat{j}-0.7\hat{k}$,\;\;\;$\hat{n}_{35}=0.5\hat{i}+0.78\hat{j}+0.37\hat{k}$,\newline
$\vec{r}_{13}=10.0\hat{i}+10.0\hat{j}+10.0\hat{k}$,\;\;\;$\vec{r}_{14}=10.0\hat{i}+10.0\hat{j}+0.0\hat{k}$,\;\;\;$\vec{r}_{24}=10.0\hat{i}+0.0\hat{j}+10.0\hat{k}$,\;\;\;$\vec{r}_{25}=0.0\hat{i}+0.0\hat{j}+0.0\hat{k}$,\newline
$\vec{r}_{35}=0.0\hat{i}+10.0\hat{j}+0.0\hat{k}$.

{\tiny 2D-M72:}

$\hat{n}_{13}=0.81\hat{i}-0.4\hat{j}+0.42\hat{k}$,\;\;\;$\hat{n}_{14}=-0.0\hat{i}+0.73\hat{j}+0.68\hat{k}$,\;\;\;$\hat{n}_{25}=0.95\hat{i}+0.13\hat{j}-0.29\hat{k}$,\;\;\;$\hat{n}_{35}=0.03\hat{i}+0.76\hat{j}+0.65\hat{k}$,\newline
$\vec{r}_{13}=10.0\hat{i}+10.0\hat{j}+0.0\hat{k}$,\;\;\;$\vec{r}_{14}=0.0\hat{i}+0.0\hat{j}+10.0\hat{k}$,\;\;\;$\vec{r}_{24}=0.0\hat{i}+10.0\hat{j}+10.0\hat{k}$,\;\;\;$\vec{r}_{25}=10.0\hat{i}+0.0\hat{j}+0.0\hat{k}$,\newline
$\vec{r}_{35}=0.0\hat{i}+0.0\hat{j}+10.0\hat{k}$.

{\tiny 2D-M73:}

$\hat{n}_{13}=0.0\hat{i}+0.05\hat{j}-1.0\hat{k}$,\;\;\;$\hat{n}_{14}=0.71\hat{i}-0.05\hat{j}+0.7\hat{k}$,\;\;\;$\hat{n}_{23}=-0.59\hat{i}+0.46\hat{j}+0.67\hat{k}$,\;\;\;$\hat{n}_{45}=0.0\hat{i}-0.86\hat{j}-0.51\hat{k}$,\newline
$\vec{r}_{13}=10.0\hat{i}+0.0\hat{j}+10.0\hat{k}$,\;\;\;$\vec{r}_{14}=10.0\hat{i}+0.0\hat{j}+10.0\hat{k}$,\;\;\;$\vec{r}_{23}=0.0\hat{i}+0.0\hat{j}+10.0\hat{k}$,\;\;\;$\vec{r}_{24}=10.0\hat{i}+10.0\hat{j}+0.0\hat{k}$,\newline
$\vec{r}_{45}=0.0\hat{i}+0.0\hat{j}+10.0\hat{k}$.

{\tiny 2D-M74:}

$\hat{n}_{13}=0.0\hat{i}-0.0\hat{j}+1.0\hat{k}$,\;\;\;$\hat{n}_{14}=-0.02\hat{i}-0.9\hat{j}+0.43\hat{k}$,\;\;\;$\hat{n}_{23}=-0.94\hat{i}-0.11\hat{j}-0.33\hat{k}$,\;\;\;$\hat{n}_{35}=-0.87\hat{i}-0.5\hat{j}+0.0\hat{k}$,\newline
$\vec{r}_{13}=10.0\hat{i}+0.0\hat{j}+0.0\hat{k}$,\;\;\;$\vec{r}_{14}=7.25\hat{i}+5.1\hat{j}+3.87\hat{k}$,\;\;\;$\vec{r}_{23}=8.61\hat{i}+8.77\hat{j}+6.23\hat{k}$,\;\;\;$\vec{r}_{24}=1.63\hat{i}+6.13\hat{j}+3.88\hat{k}$,\newline
$\vec{r}_{35}=10.0\hat{i}+0.0\hat{j}+10.0\hat{k}$.

{\tiny 2D-M75:}

$\hat{n}_{13}=0.05\hat{i}+0.55\hat{j}-0.83\hat{k}$,\;\;\;$\hat{n}_{14}=0.65\hat{i}-0.39\hat{j}-0.65\hat{k}$,\;\;\;$\hat{n}_{23}=0.0\hat{i}+0.25\hat{j}-0.97\hat{k}$,\;\;\;$\hat{n}_{25}=0.48\hat{i}-0.37\hat{j}-0.8\hat{k}$,\newline
$\vec{r}_{13}=10.0\hat{i}+10.0\hat{j}+10.0\hat{k}$,\;\;\;$\vec{r}_{14}=10.0\hat{i}+0.0\hat{j}+0.0\hat{k}$,\;\;\;$\vec{r}_{23}=0.0\hat{i}+0.0\hat{j}+0.0\hat{k}$,\;\;\;$\vec{r}_{24}=10.0\hat{i}+10.0\hat{j}+10.0\hat{k}$,\newline
$\vec{r}_{25}=0.0\hat{i}+10.0\hat{j}+10.0\hat{k}$.

{\tiny 2D-M76:}

$\hat{n}_{13}=0.7\hat{i}-0.14\hat{j}-0.7\hat{k}$,\;\;\;$\hat{n}_{14}=-0.52\hat{i}+0.82\hat{j}+0.25\hat{k}$,\;\;\;$\hat{n}_{24}=0.22\hat{i}-0.18\hat{j}-0.96\hat{k}$,\;\;\;$\hat{n}_{25}=0.36\hat{i}-0.63\hat{j}+0.69\hat{k}$,\newline
$\vec{r}_{13}=10.0\hat{i}+0.0\hat{j}+0.0\hat{k}$,\;\;\;$\vec{r}_{14}=0.0\hat{i}+0.0\hat{j}+10.0\hat{k}$,\;\;\;$\vec{r}_{24}=10.0\hat{i}+0.0\hat{j}+0.0\hat{k}$,\;\;\;$\vec{r}_{25}=0.0\hat{i}+10.0\hat{j}+0.0\hat{k}$,\newline
$\vec{r}_{35}=10.0\hat{i}+10.0\hat{j}+10.0\hat{k}$.

{\tiny 2D-M77:}

$\hat{n}_{13}=0.73\hat{i}+0.15\hat{j}-0.67\hat{k}$,\;\;\;$\hat{n}_{14}=-0.91\hat{i}+0.3\hat{j}-0.28\hat{k}$,\;\;\;$\hat{n}_{24}=-0.47\hat{i}-0.47\hat{j}-0.75\hat{k}$,\;\;\;$\hat{n}_{35}=-0.0\hat{i}+0.67\hat{j}+0.74\hat{k}$,\newline
$\vec{r}_{13}=0.0\hat{i}+0.0\hat{j}+0.0\hat{k}$,\;\;\;$\vec{r}_{14}=10.0\hat{i}+10.0\hat{j}+0.0\hat{k}$,\;\;\;$\vec{r}_{24}=10.0\hat{i}+0.0\hat{j}+10.0\hat{k}$,\;\;\;$\vec{r}_{25}=0.0\hat{i}+10.0\hat{j}+10.0\hat{k}$,\newline
$\vec{r}_{35}=10.0\hat{i}+0.0\hat{j}+0.0\hat{k}$.

{\tiny 2D-M78:}

$\hat{n}_{13}=-0.67\hat{i}-0.6\hat{j}+0.44\hat{k}$,\;\;\;$\hat{n}_{14}=-0.71\hat{i}-0.18\hat{j}-0.68\hat{k}$,\;\;\;$\hat{n}_{25}=-0.0\hat{i}+0.0\hat{j}-1.0\hat{k}$,\;\;\;$\hat{n}_{35}=-0.67\hat{i}+0.49\hat{j}+0.56\hat{k}$,\newline
$\vec{r}_{13}=0.0\hat{i}+10.0\hat{j}+10.0\hat{k}$,\;\;\;$\vec{r}_{14}=0.0\hat{i}+0.0\hat{j}+10.0\hat{k}$,\;\;\;$\vec{r}_{24}=10.0\hat{i}+0.0\hat{j}+0.0\hat{k}$,\;\;\;$\vec{r}_{25}=0.0\hat{i}+10.0\hat{j}+9.99\hat{k}$,\newline
$\vec{r}_{35}=10.0\hat{i}+10.0\hat{j}+10.0\hat{k}$.

{\tiny 2D-M79:}

$\hat{n}_{13}=0.0\hat{i}+0.62\hat{j}-0.78\hat{k}$,\;\;\;$\hat{n}_{14}=0.43\hat{i}-0.88\hat{j}+0.22\hat{k}$,\;\;\;$\hat{n}_{23}=0.0\hat{i}+0.0\hat{j}-1.0\hat{k}$,\;\;\;$\hat{n}_{25}=0.77\hat{i}+0.12\hat{j}-0.62\hat{k}$,\newline
$\vec{r}_{13}=10.0\hat{i}+10.0\hat{j}+10.0\hat{k}$,\;\;\;$\vec{r}_{14}=0.0\hat{i}+0.0\hat{j}+0.0\hat{k}$,\;\;\;$\vec{r}_{23}=0.0\hat{i}+10.0\hat{j}+0.0\hat{k}$,\;\;\;$\vec{r}_{25}=10.0\hat{i}+0.0\hat{j}+0.0\hat{k}$,\newline
$\vec{r}_{45}=0.0\hat{i}+10.0\hat{j}+10.0\hat{k}$.

{\tiny 2D-M80:}

$\hat{n}_{13}=0.04\hat{i}-0.71\hat{j}-0.71\hat{k}$,\;\;\;$\hat{n}_{14}=-0.86\hat{i}-0.35\hat{j}+0.38\hat{k}$,\;\;\;$\hat{n}_{23}=0.81\hat{i}-0.31\hat{j}+0.5\hat{k}$,\;\;\;$\hat{n}_{45}=0.01\hat{i}-0.72\hat{j}-0.69\hat{k}$,\newline
$\vec{r}_{13}=0.0\hat{i}+10.0\hat{j}+10.0\hat{k}$,\;\;\;$\vec{r}_{14}=0.0\hat{i}+10.0\hat{j}+10.0\hat{k}$,\;\;\;$\vec{r}_{23}=0.0\hat{i}+0.0\hat{j}+10.0\hat{k}$,\;\;\;$\vec{r}_{25}=10.0\hat{i}+10.0\hat{j}+0.0\hat{k}$,\newline
$\vec{r}_{45}=0.0\hat{i}+0.0\hat{j}+10.0\hat{k}$.

{\tiny 2D-M81:}

$\hat{n}_{13}=-0.0\hat{i}+0.87\hat{j}-0.5\hat{k}$,\;\;\;$\hat{n}_{14}=0.0\hat{i}+0.28\hat{j}+0.96\hat{k}$,\;\;\;$\hat{n}_{23}=-0.49\hat{i}-0.73\hat{j}-0.49\hat{k}$,\;\;\;$\hat{n}_{45}=-0.08\hat{i}+0.55\hat{j}+0.83\hat{k}$,\newline
$\vec{r}_{13}=10.0\hat{i}+10.0\hat{j}+10.0\hat{k}$,\;\;\;$\vec{r}_{14}=0.0\hat{i}+10.0\hat{j}+10.0\hat{k}$,\;\;\;$\vec{r}_{23}=10.0\hat{i}+10.0\hat{j}+0.0\hat{k}$,\;\;\;$\vec{r}_{24}=10.0\hat{i}+0.0\hat{j}+10.0\hat{k}$,\newline
$\vec{r}_{45}=10.0\hat{i}+0.0\hat{j}+0.0\hat{k}$.

{\tiny 2D-M82:}

$\hat{n}_{13}=-0.51\hat{i}+0.31\hat{j}+0.8\hat{k}$,\;\;\;$\hat{n}_{14}=-0.04\hat{i}-0.6\hat{j}-0.8\hat{k}$,\;\;\;$\hat{n}_{23}=0.37\hat{i}-0.47\hat{j}-0.8\hat{k}$,\;\;\;$\hat{n}_{35}=-0.02\hat{i}+0.6\hat{j}-0.8\hat{k}$,\newline
$\vec{r}_{13}=0.0\hat{i}+10.0\hat{j}+10.0\hat{k}$,\;\;\;$\vec{r}_{14}=4.5\hat{i}+2.54\hat{j}+7.9\hat{k}$,\;\;\;$\vec{r}_{23}=8.09\hat{i}+8.34\hat{j}+4.68\hat{k}$,\;\;\;$\vec{r}_{24}=9.23\hat{i}+8.25\hat{j}+1.09\hat{k}$,\newline
$\vec{r}_{35}=10.0\hat{i}+10.0\hat{j}+10.0\hat{k}$.

{\tiny 2D-M83:}

$\hat{n}_{13}=0.0\hat{i}+0.58\hat{j}-0.81\hat{k}$,\;\;\;$\hat{n}_{14}=0.79\hat{i}-0.21\hat{j}+0.58\hat{k}$,\;\;\;$\hat{n}_{23}=0.58\hat{i}+0.58\hat{j}-0.58\hat{k}$,\;\;\;$\hat{n}_{25}=-0.82\hat{i}+0.47\hat{j}+0.33\hat{k}$,\newline
$\vec{r}_{13}=10.0\hat{i}+10.0\hat{j}+10.0\hat{k}$,\;\;\;$\vec{r}_{14}=0.0\hat{i}+10.0\hat{j}+0.0\hat{k}$,\;\;\;$\vec{r}_{23}=10.0\hat{i}+0.0\hat{j}+0.0\hat{k}$,\;\;\;$\vec{r}_{24}=10.0\hat{i}+10.0\hat{j}+10.0\hat{k}$,\newline
$\vec{r}_{25}=10.0\hat{i}+10.0\hat{j}+10.0\hat{k}$.

{\tiny 2D-M84:}

$\hat{n}_{13}=0.0\hat{i}+0.0\hat{j}-1.0\hat{k}$,\;\;\;$\hat{n}_{14}=0.48\hat{i}+0.77\hat{j}+0.43\hat{k}$,\;\;\;$\hat{n}_{25}=0.71\hat{i}-0.0\hat{j}+0.7\hat{k}$,\;\;\;$\hat{n}_{45}=0.5\hat{i}+0.61\hat{j}-0.62\hat{k}$,\newline
$\vec{r}_{13}=10.0\hat{i}+0.0\hat{j}+10.0\hat{k}$,\;\;\;$\vec{r}_{14}=10.0\hat{i}+0.0\hat{j}+0.0\hat{k}$,\;\;\;$\vec{r}_{23}=0.0\hat{i}+10.0\hat{j}+0.0\hat{k}$,\;\;\;$\vec{r}_{25}=10.0\hat{i}+10.0\hat{j}+0.0\hat{k}$,\newline
$\vec{r}_{45}=10.0\hat{i}+10.0\hat{j}+10.0\hat{k}$.

{\tiny 2D-M85:}

$\hat{n}_{13}=-0.65\hat{i}+0.65\hat{j}-0.4\hat{k}$,\;\;\;$\hat{n}_{14}=-0.48\hat{i}+0.45\hat{j}+0.75\hat{k}$,\;\;\;$\hat{n}_{24}=0.63\hat{i}+0.46\hat{j}+0.63\hat{k}$,\;\;\;$\hat{n}_{45}=0.01\hat{i}+0.58\hat{j}-0.81\hat{k}$,\newline
$\vec{r}_{13}=10.0\hat{i}+10.0\hat{j}+10.0\hat{k}$,\;\;\;$\vec{r}_{14}=10.0\hat{i}+0.0\hat{j}+0.0\hat{k}$,\;\;\;$\vec{r}_{23}=0.0\hat{i}+0.0\hat{j}+10.0\hat{k}$,\;\;\;$\vec{r}_{24}=0.0\hat{i}+10.0\hat{j}+0.0\hat{k}$,\newline
$\vec{r}_{45}=10.0\hat{i}+0.0\hat{j}+10.0\hat{k}$.

{\tiny 2D-M86:}

$\hat{n}_{13}=-0.16\hat{i}-0.63\hat{j}-0.76\hat{k}$,\;\;\;$\hat{n}_{14}=-0.22\hat{i}-0.92\hat{j}+0.34\hat{k}$,\;\;\;$\hat{n}_{24}=1.0\hat{i}-0.08\hat{j}-0.01\hat{k}$,\;\;\;$\hat{n}_{35}=-0.71\hat{i}+0.1\hat{j}+0.7\hat{k}$,\newline
$\vec{r}_{13}=10.0\hat{i}+0.0\hat{j}+0.0\hat{k}$,\;\;\;$\vec{r}_{14}=7.61\hat{i}+1.62\hat{j}+8.23\hat{k}$,\;\;\;$\vec{r}_{23}=1.68\hat{i}+5.11\hat{j}+6.63\hat{k}$,\;\;\;$\vec{r}_{24}=5.61\hat{i}+4.8\hat{j}+3.36\hat{k}$,\newline
$\vec{r}_{35}=10.0\hat{i}+10.0\hat{j}+10.0\hat{k}$.

{\tiny 2D-M87:}

$\hat{n}_{13}=0.66\hat{i}-0.66\hat{j}+0.36\hat{k}$,\;\;\;$\hat{n}_{14}=0.52\hat{i}-0.42\hat{j}-0.75\hat{k}$,\;\;\;$\hat{n}_{24}=0.12\hat{i}-0.71\hat{j}+0.7\hat{k}$,\;\;\;$\hat{n}_{25}=0.68\hat{i}+0.16\hat{j}+0.72\hat{k}$,\newline
$\vec{r}_{13}=0.0\hat{i}+0.0\hat{j}+10.0\hat{k}$,\;\;\;$\vec{r}_{14}=0.0\hat{i}+0.0\hat{j}+0.0\hat{k}$,\;\;\;$\vec{r}_{23}=10.0\hat{i}+10.0\hat{j}+10.0\hat{k}$,\;\;\;$\vec{r}_{24}=0.0\hat{i}+10.0\hat{j}+0.0\hat{k}$,\newline
$\vec{r}_{25}=0.0\hat{i}+10.0\hat{j}+0.0\hat{k}$.

{\tiny 2D-M88:}

$\hat{n}_{13}=0.0\hat{i}+0.62\hat{j}-0.79\hat{k}$,\;\;\;$\hat{n}_{24}=0.82\hat{i}+0.42\hat{j}+0.39\hat{k}$,\;\;\;$\hat{n}_{25}=0.0\hat{i}-0.7\hat{j}+0.71\hat{k}$,\;\;\;$\hat{n}_{35}=-0.0\hat{i}+0.7\hat{j}-0.72\hat{k}$,\newline
$\vec{r}_{13}=10.0\hat{i}+10.0\hat{j}+10.0\hat{k}$,\;\;\;$\vec{r}_{14}=10.0\hat{i}+0.0\hat{j}+10.0\hat{k}$,\;\;\;$\vec{r}_{24}=0.0\hat{i}+10.0\hat{j}+0.0\hat{k}$,\;\;\;$\vec{r}_{25}=10.0\hat{i}+10.0\hat{j}+10.0\hat{k}$,\newline
$\vec{r}_{35}=0.0\hat{i}+0.0\hat{j}+0.0\hat{k}$.

{\tiny 2D-M89:}

$\hat{n}_{13}=-0.0\hat{i}-0.58\hat{j}-0.82\hat{k}$,\;\;\;$\hat{n}_{24}=0.65\hat{i}-0.54\hat{j}-0.54\hat{k}$,\;\;\;$\hat{n}_{25}=0.0\hat{i}+0.38\hat{j}-0.92\hat{k}$,\;\;\;$\hat{n}_{35}=-0.58\hat{i}+0.51\hat{j}+0.63\hat{k}$,\newline
$\vec{r}_{13}=10.0\hat{i}+10.0\hat{j}+0.0\hat{k}$,\;\;\;$\vec{r}_{14}=10.0\hat{i}+10.0\hat{j}+0.0\hat{k}$,\;\;\;$\vec{r}_{24}=0.0\hat{i}+10.0\hat{j}+10.0\hat{k}$,\;\;\;$\vec{r}_{25}=0.0\hat{i}+0.0\hat{j}+0.0\hat{k}$,\newline
$\vec{r}_{35}=0.0\hat{i}+10.0\hat{j}+10.0\hat{k}$.

{\tiny 2D-M90:}

$\hat{n}_{13}=0.71\hat{i}-0.1\hat{j}+0.7\hat{k}$,\;\;\;$\hat{n}_{24}=0.3\hat{i}+0.67\hat{j}-0.67\hat{k}$,\;\;\;$\hat{n}_{25}=0.0\hat{i}-0.71\hat{j}-0.71\hat{k}$,\;\;\;$\hat{n}_{35}=-0.03\hat{i}+0.68\hat{j}+0.73\hat{k}$,\newline
$\vec{r}_{13}=10.0\hat{i}+0.0\hat{j}+10.0\hat{k}$,\;\;\;$\vec{r}_{14}=0.0\hat{i}+0.0\hat{j}+10.0\hat{k}$,\;\;\;$\vec{r}_{24}=0.0\hat{i}+10.0\hat{j}+10.0\hat{k}$,\;\;\;$\vec{r}_{25}=10.0\hat{i}+10.0\hat{j}+0.0\hat{k}$,\newline
$\vec{r}_{35}=10.0\hat{i}+10.0\hat{j}+0.0\hat{k}$.

{\tiny 2D-M91:}

$\hat{n}_{13}=-0.85\hat{i}+0.47\hat{j}-0.25\hat{k}$,\;\;\;$\hat{n}_{23}=-0.0\hat{i}+0.0\hat{j}+1.0\hat{k}$,\;\;\;$\hat{n}_{25}=-0.13\hat{i}-0.63\hat{j}-0.76\hat{k}$,\;\;\;$\hat{n}_{45}=-0.33\hat{i}-0.9\hat{j}+0.29\hat{k}$,\newline
$\vec{r}_{13}=10.0\hat{i}+10.0\hat{j}+0.0\hat{k}$,\;\;\;$\vec{r}_{14}=0.0\hat{i}+0.0\hat{j}+10.0\hat{k}$,\;\;\;$\vec{r}_{23}=0.0\hat{i}+0.0\hat{j}+10.0\hat{k}$,\;\;\;$\vec{r}_{25}=10.0\hat{i}+10.0\hat{j}+0.0\hat{k}$,\newline
$\vec{r}_{45}=0.0\hat{i}+10.0\hat{j}+10.0\hat{k}$.

{\tiny 2D-M92:}

$\hat{n}_{13}=0.0\hat{i}+0.0\hat{j}-1.0\hat{k}$,\;\;\;$\hat{n}_{23}=0.25\hat{i}-0.44\hat{j}-0.86\hat{k}$,\;\;\;$\hat{n}_{25}=0.41\hat{i}+0.2\hat{j}-0.89\hat{k}$,\;\;\;$\hat{n}_{45}=0.75\hat{i}-0.65\hat{j}+0.11\hat{k}$,\newline
$\vec{r}_{13}=0.0\hat{i}+10.0\hat{j}+9.97\hat{k}$,\;\;\;$\vec{r}_{14}=0.0\hat{i}+0.0\hat{j}+10.0\hat{k}$,\;\;\;$\vec{r}_{23}=10.0\hat{i}+0.0\hat{j}+0.0\hat{k}$,\;\;\;$\vec{r}_{25}=10.0\hat{i}+10.0\hat{j}+10.0\hat{k}$,\newline
$\vec{r}_{45}=10.0\hat{i}+10.0\hat{j}+0.0\hat{k}$.

{\tiny 2D-M93:}

$\hat{n}_{13}=-0.32\hat{i}+0.6\hat{j}-0.74\hat{k}$,\;\;\;$\hat{n}_{23}=-0.71\hat{i}-0.71\hat{j}+0.0\hat{k}$,\;\;\;$\hat{n}_{24}=0.33\hat{i}-0.33\hat{j}-0.89\hat{k}$,\;\;\;$\hat{n}_{45}=-0.29\hat{i}-0.38\hat{j}+0.88\hat{k}$,\newline
$\vec{r}_{13}=0.0\hat{i}+10.0\hat{j}+0.0\hat{k}$,\;\;\;$\vec{r}_{14}=0.0\hat{i}+10.0\hat{j}+0.0\hat{k}$,\;\;\;$\vec{r}_{23}=10.0\hat{i}+0.0\hat{j}+10.0\hat{k}$,\;\;\;$\vec{r}_{24}=10.0\hat{i}+0.0\hat{j}+0.0\hat{k}$,\newline
$\vec{r}_{45}=10.0\hat{i}+10.0\hat{j}+10.0\hat{k}$.

{\tiny 2D-M94:}

$\hat{n}_{13}=0.6\hat{i}-0.11\hat{j}+0.79\hat{k}$,\;\;\;$\hat{n}_{23}=0.13\hat{i}-0.76\hat{j}-0.63\hat{k}$,\;\;\;$\hat{n}_{24}=-0.28\hat{i}+0.27\hat{j}+0.92\hat{k}$,\;\;\;$\hat{n}_{35}=0.13\hat{i}-0.65\hat{j}+0.75\hat{k}$,\newline
$\vec{r}_{13}=0.0\hat{i}+10.0\hat{j}+0.0\hat{k}$,\;\;\;$\vec{r}_{14}=6.57\hat{i}+7.46\hat{j}+8.53\hat{k}$,\;\;\;$\vec{r}_{23}=7.76\hat{i}+9.05\hat{j}+0.95\hat{k}$,\;\;\;$\vec{r}_{24}=8.61\hat{i}+8.08\hat{j}+6.19\hat{k}$,\newline
$\vec{r}_{35}=10.0\hat{i}+10.0\hat{j}+10.0\hat{k}$.

{\tiny 2D-M95:}

$\hat{n}_{13}=0.82\hat{i}-0.38\hat{j}+0.42\hat{k}$,\;\;\;$\hat{n}_{23}=0.58\hat{i}+0.6\hat{j}+0.56\hat{k}$,\;\;\;$\hat{n}_{24}=0.77\hat{i}-0.22\hat{j}-0.6\hat{k}$,\;\;\;$\hat{n}_{25}=0.3\hat{i}-0.62\hat{j}-0.73\hat{k}$,\newline
$\vec{r}_{13}=10.0\hat{i}+10.0\hat{j}+0.0\hat{k}$,\;\;\;$\vec{r}_{14}=0.0\hat{i}+0.0\hat{j}+10.0\hat{k}$,\;\;\;$\vec{r}_{23}=0.0\hat{i}+10.0\hat{j}+0.0\hat{k}$,\;\;\;$\vec{r}_{24}=10.0\hat{i}+0.0\hat{j}+0.0\hat{k}$,\newline
$\vec{r}_{25}=0.0\hat{i}+10.0\hat{j}+10.0\hat{k}$.

{\tiny 2D-M96:}

$\hat{n}_{13}=0.07\hat{i}-0.81\hat{j}+0.58\hat{k}$,\;\;\;$\hat{n}_{23}=0.35\hat{i}-0.92\hat{j}+0.15\hat{k}$,\;\;\;$\hat{n}_{25}=-0.39\hat{i}-0.83\hat{j}-0.39\hat{k}$,\;\;\;$\hat{n}_{45}=0.75\hat{i}-0.47\hat{j}+0.47\hat{k}$,\newline
$\vec{r}_{13}=0.0\hat{i}+10.0\hat{j}+0.0\hat{k}$,\;\;\;$\vec{r}_{14}=0.0\hat{i}+10.0\hat{j}+0.0\hat{k}$,\;\;\;$\vec{r}_{23}=0.0\hat{i}+0.0\hat{j}+10.0\hat{k}$,\;\;\;$\vec{r}_{25}=0.0\hat{i}+10.0\hat{j}+10.0\hat{k}$,\newline
$\vec{r}_{45}=10.0\hat{i}+10.0\hat{j}+10.0\hat{k}$.

{\tiny 2D-M97:}

$\hat{n}_{13}=-0.69\hat{i}-0.36\hat{j}+0.63\hat{k}$,\;\;\;$\hat{n}_{23}=-0.0\hat{i}+0.36\hat{j}+0.93\hat{k}$,\;\;\;$\hat{n}_{24}=-0.67\hat{i}-0.35\hat{j}+0.65\hat{k}$,\;\;\;$\hat{n}_{45}=0.9\hat{i}+0.28\hat{j}+0.33\hat{k}$,\newline
$\vec{r}_{13}=10.0\hat{i}+10.0\hat{j}+10.0\hat{k}$,\;\;\;$\vec{r}_{14}=0.0\hat{i}+10.0\hat{j}+10.0\hat{k}$,\;\;\;$\vec{r}_{23}=10.0\hat{i}+0.0\hat{j}+0.0\hat{k}$,\;\;\;$\vec{r}_{24}=0.0\hat{i}+0.0\hat{j}+0.0\hat{k}$,\newline
$\vec{r}_{45}=10.0\hat{i}+0.0\hat{j}+10.0\hat{k}$.

{\tiny 2D-M98:}

$\hat{n}_{13}=0.67\hat{i}+0.12\hat{j}+0.73\hat{k}$,\;\;\;$\hat{n}_{23}=0.83\hat{i}+0.3\hat{j}+0.48\hat{k}$,\;\;\;$\hat{n}_{24}=-0.87\hat{i}+0.24\hat{j}+0.43\hat{k}$,\;\;\;$\hat{n}_{35}=-0.17\hat{i}+0.67\hat{j}-0.73\hat{k}$,\newline
$\vec{r}_{13}=0.0\hat{i}+10.0\hat{j}+0.0\hat{k}$,\;\;\;$\vec{r}_{14}=3.35\hat{i}+7.41\hat{j}+8.14\hat{k}$,\;\;\;$\vec{r}_{23}=2.65\hat{i}+5.33\hat{j}+4.37\hat{k}$,\;\;\;$\vec{r}_{24}=1.81\hat{i}+5.97\hat{j}+8.77\hat{k}$,\newline
$\vec{r}_{35}=10.0\hat{i}+10.0\hat{j}+10.0\hat{k}$.

{\tiny 2D-M99:}

$\hat{n}_{13}=0.48\hat{i}+0.77\hat{j}-0.42\hat{k}$,\;\;\;$\hat{n}_{23}=-0.7\hat{i}-0.56\hat{j}+0.44\hat{k}$,\;\;\;$\hat{n}_{24}=0.64\hat{i}-0.64\hat{j}-0.42\hat{k}$,\;\;\;$\hat{n}_{25}=-0.0\hat{i}+0.48\hat{j}-0.88\hat{k}$,\newline
$\vec{r}_{13}=10.0\hat{i}+0.0\hat{j}+10.0\hat{k}$,\;\;\;$\vec{r}_{14}=0.0\hat{i}+0.0\hat{j}+0.0\hat{k}$,\;\;\;$\vec{r}_{23}=0.0\hat{i}+10.0\hat{j}+10.0\hat{k}$,\;\;\;$\vec{r}_{24}=10.0\hat{i}+10.0\hat{j}+0.0\hat{k}$,\newline
$\vec{r}_{25}=10.0\hat{i}+10.0\hat{j}+10.0\hat{k}$.

{\tiny 2D-M100:}

$\hat{n}_{13}=0.86\hat{i}-0.36\hat{j}+0.36\hat{k}$,\;\;\;$\hat{n}_{24}=0.81\hat{i}+0.47\hat{j}-0.34\hat{k}$,\;\;\;$\hat{n}_{25}=-0.05\hat{i}+0.71\hat{j}+0.71\hat{k}$,\;\;\;$\hat{n}_{35}=0.0\hat{i}+0.69\hat{j}+0.73\hat{k}$,\newline
$\vec{r}_{13}=10.0\hat{i}+10.0\hat{j}+0.0\hat{k}$,\;\;\;$\vec{r}_{14}=0.0\hat{i}+10.0\hat{j}+10.0\hat{k}$,\;\;\;$\vec{r}_{24}=10.0\hat{i}+0.0\hat{j}+0.0\hat{k}$,\;\;\;$\vec{r}_{25}=10.0\hat{i}+10.0\hat{j}+0.0\hat{k}$,\newline
$\vec{r}_{35}=10.0\hat{i}+0.0\hat{j}+0.0\hat{k}$.

{\tiny 2D-M101:}

$\hat{n}_{13}=-0.5\hat{i}-0.83\hat{j}-0.24\hat{k}$,\;\;\;$\hat{n}_{23}=-0.08\hat{i}-0.53\hat{j}-0.84\hat{k}$,\;\;\;$\hat{n}_{25}=0.0\hat{i}+0.97\hat{j}+0.26\hat{k}$,\;\;\;$\hat{n}_{45}=-0.83\hat{i}-0.4\hat{j}-0.4\hat{k}$,\newline
$\vec{r}_{13}=10.0\hat{i}+0.0\hat{j}+10.0\hat{k}$,\;\;\;$\vec{r}_{14}=10.0\hat{i}+10.0\hat{j}+0.0\hat{k}$,\;\;\;$\vec{r}_{23}=10.0\hat{i}+10.0\hat{j}+0.0\hat{k}$,\;\;\;$\vec{r}_{25}=0.0\hat{i}+10.0\hat{j}+10.0\hat{k}$,\newline
$\vec{r}_{45}=0.0\hat{i}+10.0\hat{j}+10.0\hat{k}$.

{\tiny 2D-M102:}

$\hat{n}_{13}=0.97\hat{i}+0.01\hat{j}-0.26\hat{k}$,\;\;\;$\hat{n}_{23}=-0.58\hat{i}-0.36\hat{j}-0.73\hat{k}$,\;\;\;$\hat{n}_{24}=0.48\hat{i}-0.52\hat{j}-0.71\hat{k}$,\;\;\;$\hat{n}_{45}=0.34\hat{i}-0.57\hat{j}+0.75\hat{k}$,\newline
$\vec{r}_{13}=0.0\hat{i}+10.0\hat{j}+10.0\hat{k}$,\;\;\;$\vec{r}_{14}=10.0\hat{i}+10.0\hat{j}+0.0\hat{k}$,\;\;\;$\vec{r}_{23}=0.0\hat{i}+10.0\hat{j}+0.0\hat{k}$,\;\;\;$\vec{r}_{24}=0.0\hat{i}+0.0\hat{j}+0.0\hat{k}$,\newline
$\vec{r}_{45}=0.0\hat{i}+10.0\hat{j}+0.0\hat{k}$.

{\tiny 2D-M103:}

$\hat{n}_{13}=-0.86\hat{i}-0.27\hat{j}+0.44\hat{k}$,\;\;\;$\hat{n}_{23}=0.0\hat{i}+0.71\hat{j}-0.71\hat{k}$,\;\;\;$\hat{n}_{24}=0.68\hat{i}-0.68\hat{j}+0.25\hat{k}$,\;\;\;$\hat{n}_{35}=0.69\hat{i}+0.27\hat{j}-0.67\hat{k}$,\newline
$\vec{r}_{13}=0.0\hat{i}+0.0\hat{j}+0.0\hat{k}$,\;\;\;$\vec{r}_{14}=10.0\hat{i}+10.0\hat{j}+10.0\hat{k}$,\;\;\;$\vec{r}_{23}=0.0\hat{i}+10.0\hat{j}+0.0\hat{k}$,\;\;\;$\vec{r}_{24}=0.0\hat{i}+0.0\hat{j}+10.0\hat{k}$,\newline
$\vec{r}_{35}=0.0\hat{i}+10.0\hat{j}+10.0\hat{k}$.

{\tiny 2D-M104:}

$\hat{n}_{13}=-0.0\hat{i}+0.69\hat{j}-0.72\hat{k}$,\;\;\;$\hat{n}_{23}=-0.0\hat{i}+0.99\hat{j}+0.14\hat{k}$,\;\;\;$\hat{n}_{24}=0.0\hat{i}+0.39\hat{j}+0.92\hat{k}$,\;\;\;$\hat{n}_{25}=-0.82\hat{i}+0.51\hat{j}-0.26\hat{k}$,\newline
$\vec{r}_{13}=10.0\hat{i}+10.0\hat{j}+10.0\hat{k}$,\;\;\;$\vec{r}_{14}=10.0\hat{i}+0.0\hat{j}+0.0\hat{k}$,\;\;\;$\vec{r}_{23}=10.0\hat{i}+10.0\hat{j}+0.0\hat{k}$,\;\;\;$\vec{r}_{24}=0.0\hat{i}+10.0\hat{j}+10.0\hat{k}$,\newline
$\vec{r}_{25}=10.0\hat{i}+10.0\hat{j}+0.0\hat{k}$.
