# Supplementary material for: Dimensional synthesis of spatial manipulators for velocity and force transmission for operation around a specified task point
Source: arXiv:2210.04446 source file (2022-10-10)
Supplement: Supplementary file 10 [file classappendix6.tex]

\subsection{Class 6} \label{appendix_five_2_1}
{\tiny 2D-M105:}

$\hat{n}_{14}=-0.0\hat{i}+0.56\hat{j}-0.83\hat{k}$,\;\;\;$\hat{n}_{24}=-0.35\hat{i}+0.49\hat{j}+0.8\hat{k}$,\;\;\;$\hat{n}_{25}=-0.58\hat{i}+0.59\hat{j}+0.56\hat{k}$,\;\;\;$\hat{n}_{34}=-0.73\hat{i}-0.67\hat{j}-0.13\hat{k}$,\newline
$\vec{r}_{14}=10.0\hat{i}+10.0\hat{j}+10.0\hat{k}$,\;\;\;$\vec{r}_{24}=0.0\hat{i}+10.0\hat{j}+10.0\hat{k}$,\;\;\;$\vec{r}_{34}=0.0\hat{i}+10.0\hat{j}+0.0\hat{k}$,\;\;\;$\vec{r}_{35}=10.0\hat{i}+0.0\hat{j}+10.0\hat{k}$.

{\tiny 2D-M106:}

$\hat{n}_{14}=-0.0\hat{i}+0.0\hat{j}-1.0\hat{k}$,\;\;\;$\hat{n}_{24}=-0.82\hat{i}-0.08\hat{j}+0.56\hat{k}$,\;\;\;$\hat{n}_{25}=0.6\hat{i}-0.61\hat{j}+0.53\hat{k}$,\;\;\;$\hat{n}_{35}=-0.0\hat{i}+0.61\hat{j}+0.8\hat{k}$,\newline
$\vec{r}_{14}=10.0\hat{i}+10.0\hat{j}+0.01\hat{k}$,\;\;\;$\vec{r}_{24}=10.0\hat{i}+0.0\hat{j}+0.0\hat{k}$,\;\;\;$\vec{r}_{34}=0.0\hat{i}+10.0\hat{j}+10.0\hat{k}$,\;\;\;$\vec{r}_{35}=10.0\hat{i}+0.0\hat{j}+0.0\hat{k}$.

{\tiny 2D-M107:}

$\hat{n}_{14}=0.53\hat{i}-0.74\hat{j}-0.41\hat{k}$,\;\;\;$\hat{n}_{24}=0.69\hat{i}+0.12\hat{j}+0.72\hat{k}$,\;\;\;$\hat{n}_{25}=-0.6\hat{i}+0.75\hat{j}+0.3\hat{k}$,\;\;\;$\hat{n}_{34}=-0.63\hat{i}-0.48\hat{j}+0.62\hat{k}$,\newline
$\vec{r}_{14}=10.0\hat{i}+10.0\hat{j}+0.0\hat{k}$,\;\;\;$\vec{r}_{24}=0.0\hat{i}+10.0\hat{j}+0.0\hat{k}$,\;\;\;$\vec{r}_{25}=10.0\hat{i}+10.0\hat{j}+0.0\hat{k}$,\;\;\;$\vec{r}_{35}=0.0\hat{i}+0.0\hat{j}+10.0\hat{k}$.

{\tiny 2D-M108:}

$\hat{n}_{14}=0.0\hat{i}+0.64\hat{j}-0.77\hat{k}$,\;\;\;$\hat{n}_{24}=-0.0\hat{i}+0.71\hat{j}+0.71\hat{k}$,\;\;\;$\hat{n}_{25}=-0.74\hat{i}+0.55\hat{j}-0.4\hat{k}$,\;\;\;$\hat{n}_{35}=-0.54\hat{i}-0.58\hat{j}+0.61\hat{k}$,\newline
$\vec{r}_{14}=10.0\hat{i}+10.0\hat{j}+10.0\hat{k}$,\;\;\;$\vec{r}_{24}=10.0\hat{i}+0.0\hat{j}+0.0\hat{k}$,\;\;\;$\vec{r}_{25}=10.0\hat{i}+10.0\hat{j}+0.0\hat{k}$,\;\;\;$\vec{r}_{34}=0.0\hat{i}+0.0\hat{j}+10.0\hat{k}$.

{\tiny 2D-M109:}

$\hat{n}_{14}=0.08\hat{i}-0.62\hat{j}+0.78\hat{k}$,\;\;\;$\hat{n}_{24}=0.0\hat{i}+0.67\hat{j}+0.75\hat{k}$,\;\;\;$\hat{n}_{34}=0.58\hat{i}+0.57\hat{j}-0.59\hat{k}$,\;\;\;$\hat{n}_{35}=-0.82\hat{i}+0.38\hat{j}-0.43\hat{k}$,\newline
$\vec{r}_{14}=10.0\hat{i}+10.0\hat{j}+10.0\hat{k}$,\;\;\;$\vec{r}_{24}=10.0\hat{i}+0.0\hat{j}+0.0\hat{k}$,\;\;\;$\vec{r}_{25}=10.0\hat{i}+10.0\hat{j}+0.0\hat{k}$,\;\;\;$\vec{r}_{35}=0.0\hat{i}+0.0\hat{j}+10.0\hat{k}$.

{\tiny 2D-M110:}

$\hat{n}_{14}=0.82\hat{i}+0.06\hat{j}+0.57\hat{k}$,\;\;\;$\hat{n}_{24}=-0.35\hat{i}-0.66\hat{j}+0.66\hat{k}$,\;\;\;$\hat{n}_{34}=-0.7\hat{i}+0.01\hat{j}-0.72\hat{k}$,\;\;\;$\hat{n}_{35}=-0.58\hat{i}+0.58\hat{j}+0.57\hat{k}$,\newline
$\vec{r}_{14}=10.0\hat{i}+0.0\hat{j}+10.0\hat{k}$,\;\;\;$\vec{r}_{24}=10.0\hat{i}+10.0\hat{j}+10.0\hat{k}$,\;\;\;$\vec{r}_{25}=0.0\hat{i}+10.0\hat{j}+0.0\hat{k}$,\;\;\;$\vec{r}_{34}=10.0\hat{i}+0.0\hat{j}+10.0\hat{k}$.

{\tiny 2D-M111:}

$\hat{n}_{14}=-0.11\hat{i}+0.79\hat{j}+0.6\hat{k}$,\;\;\;$\hat{n}_{24}=0.65\hat{i}-0.33\hat{j}-0.68\hat{k}$,\;\;\;$\hat{n}_{25}=0.66\hat{i}-0.07\hat{j}+0.75\hat{k}$,\;\;\;$\hat{n}_{34}=0.11\hat{i}+0.99\hat{j}-0.08\hat{k}$,\newline
$\vec{r}_{14}=0.0\hat{i}+10.0\hat{j}+10.0\hat{k}$,\;\;\;$\vec{r}_{25}=0.0\hat{i}+10.0\hat{j}+0.0\hat{k}$,\;\;\;$\vec{r}_{34}=10.0\hat{i}+0.0\hat{j}+10.0\hat{k}$,\;\;\;$\vec{r}_{35}=10.0\hat{i}+10.0\hat{j}+0.0\hat{k}$.

{\tiny 2D-M112:}

$\hat{n}_{14}=0.32\hat{i}+0.93\hat{j}+0.17\hat{k}$,\;\;\;$\hat{n}_{24}=0.48\hat{i}-0.75\hat{j}+0.45\hat{k}$,\;\;\;$\hat{n}_{25}=0.0\hat{i}+0.65\hat{j}-0.76\hat{k}$,\;\;\;$\hat{n}_{35}=0.19\hat{i}+0.7\hat{j}+0.69\hat{k}$,\newline
$\vec{r}_{14}=0.0\hat{i}+10.0\hat{j}+10.0\hat{k}$,\;\;\;$\vec{r}_{25}=0.0\hat{i}+10.0\hat{j}+0.0\hat{k}$,\;\;\;$\vec{r}_{34}=0.0\hat{i}+10.0\hat{j}+10.0\hat{k}$,\;\;\;$\vec{r}_{35}=10.0\hat{i}+0.0\hat{j}+0.0\hat{k}$.

{\tiny 2D-M113:}

$\hat{n}_{14}=0.8\hat{i}-0.48\hat{j}-0.35\hat{k}$,\;\;\;$\hat{n}_{24}=-0.0\hat{i}+0.7\hat{j}+0.71\hat{k}$,\;\;\;$\hat{n}_{25}=0.95\hat{i}-0.22\hat{j}-0.2\hat{k}$,\;\;\;$\hat{n}_{35}=-0.36\hat{i}+0.36\hat{j}-0.86\hat{k}$,\newline
$\vec{r}_{14}=0.0\hat{i}+0.0\hat{j}+0.0\hat{k}$,\;\;\;$\vec{r}_{25}=0.0\hat{i}+0.0\hat{j}+0.0\hat{k}$,\;\;\;$\vec{r}_{34}=10.0\hat{i}+10.0\hat{j}+10.0\hat{k}$,\;\;\;$\vec{r}_{35}=0.0\hat{i}+0.0\hat{j}+10.0\hat{k}$.

{\tiny 2D-M114:}

$\hat{n}_{14}=-0.69\hat{i}+0.71\hat{j}+0.17\hat{k}$,\;\;\;$\hat{n}_{24}=-0.54\hat{i}+0.63\hat{j}-0.56\hat{k}$,\;\;\;$\hat{n}_{34}=0.71\hat{i}+0.7\hat{j}-0.12\hat{k}$,\;\;\;$\hat{n}_{35}=-0.0\hat{i}+0.0\hat{j}-1.0\hat{k}$,\newline
$\vec{r}_{14}=10.0\hat{i}+10.0\hat{j}+0.0\hat{k}$,\;\;\;$\vec{r}_{25}=0.0\hat{i}+10.0\hat{j}+10.0\hat{k}$,\;\;\;$\vec{r}_{34}=10.0\hat{i}+0.0\hat{j}+0.0\hat{k}$,\;\;\;$\vec{r}_{35}=10.0\hat{i}+10.0\hat{j}+10.0\hat{k}$.

{\tiny 2D-M115:}

$\hat{n}_{14}=0.0\hat{i}+0.0\hat{j}+1.0\hat{k}$,\;\;\;$\hat{n}_{24}=0.57\hat{i}+0.27\hat{j}-0.77\hat{k}$,\;\;\;$\hat{n}_{25}=0.0\hat{i}+0.86\hat{j}-0.51\hat{k}$,\;\;\;$\hat{n}_{35}=-0.62\hat{i}-0.62\hat{j}-0.48\hat{k}$,\newline
$\vec{r}_{14}=10.0\hat{i}+10.0\hat{j}+9.95\hat{k}$,\;\;\;$\vec{r}_{24}=10.0\hat{i}+10.0\hat{j}+10.0\hat{k}$,\;\;\;$\vec{r}_{25}=0.0\hat{i}+10.0\hat{j}+0.0\hat{k}$,\;\;\;$\vec{r}_{34}=0.0\hat{i}+0.0\hat{j}+0.0\hat{k}$.

{\tiny 2D-M116:}

$\hat{n}_{14}=0.76\hat{i}-0.61\hat{j}+0.24\hat{k}$,\;\;\;$\hat{n}_{24}=0.01\hat{i}+0.7\hat{j}-0.71\hat{k}$,\;\;\;$\hat{n}_{25}=-0.58\hat{i}-0.58\hat{j}-0.58\hat{k}$,\;\;\;$\hat{n}_{35}=0.82\hat{i}-0.41\hat{j}-0.4\hat{k}$,\newline
$\vec{r}_{14}=0.0\hat{i}+0.0\hat{j}+10.0\hat{k}$,\;\;\;$\vec{r}_{24}=0.0\hat{i}+0.0\hat{j}+0.0\hat{k}$,\;\;\;$\vec{r}_{34}=10.0\hat{i}+10.0\hat{j}+10.0\hat{k}$,\;\;\;$\vec{r}_{35}=0.0\hat{i}+0.0\hat{j}+0.0\hat{k}$.

{\tiny 2D-M117:}

$\hat{n}_{14}=0.23\hat{i}-0.48\hat{j}-0.85\hat{k}$,\;\;\;$\hat{n}_{23}=-0.94\hat{i}-0.33\hat{j}+0.03\hat{k}$,\;\;\;$\hat{n}_{25}=-0.61\hat{i}+0.57\hat{j}-0.55\hat{k}$,\;\;\;$\hat{n}_{34}=0.0\hat{i}+0.69\hat{j}+0.72\hat{k}$,\newline
$\vec{r}_{14}=10.0\hat{i}+0.0\hat{j}+0.0\hat{k}$,\;\;\;$\vec{r}_{23}=10.0\hat{i}+0.0\hat{j}+10.0\hat{k}$,\;\;\;$\vec{r}_{34}=0.0\hat{i}+10.0\hat{j}+10.0\hat{k}$,\;\;\;$\vec{r}_{45}=10.0\hat{i}+0.0\hat{j}+0.0\hat{k}$.

{\tiny 2D-M118:}

$\hat{n}_{14}=0.02\hat{i}+0.57\hat{j}-0.82\hat{k}$,\;\;\;$\hat{n}_{23}=0.65\hat{i}-0.75\hat{j}-0.1\hat{k}$,\;\;\;$\hat{n}_{25}=-0.58\hat{i}-0.58\hat{j}+0.58\hat{k}$,\;\;\;$\hat{n}_{45}=-0.49\hat{i}-0.32\hat{j}-0.81\hat{k}$,\newline
$\vec{r}_{14}=10.0\hat{i}+10.0\hat{j}+10.0\hat{k}$,\;\;\;$\vec{r}_{23}=0.0\hat{i}+0.0\hat{j}+10.0\hat{k}$,\;\;\;$\vec{r}_{34}=10.0\hat{i}+10.0\hat{j}+0.0\hat{k}$,\;\;\;$\vec{r}_{45}=0.0\hat{i}+0.0\hat{j}+10.0\hat{k}$.

{\tiny 2D-M119:}

$\hat{n}_{14}=-0.0\hat{i}+0.58\hat{j}+0.81\hat{k}$,\;\;\;$\hat{n}_{23}=-0.78\hat{i}+0.01\hat{j}-0.62\hat{k}$,\;\;\;$\hat{n}_{25}=-0.41\hat{i}+0.82\hat{j}+0.41\hat{k}$,\;\;\;$\hat{n}_{34}=0.58\hat{i}+0.58\hat{j}-0.58\hat{k}$,\newline
$\vec{r}_{14}=10.0\hat{i}+0.0\hat{j}+0.0\hat{k}$,\;\;\;$\vec{r}_{23}=0.0\hat{i}+0.0\hat{j}+10.0\hat{k}$,\;\;\;$\vec{r}_{25}=10.0\hat{i}+10.0\hat{j}+0.0\hat{k}$,\;\;\;$\vec{r}_{45}=0.0\hat{i}+0.0\hat{j}+10.0\hat{k}$.

{\tiny 2D-M120:}

$\hat{n}_{14}=0.31\hat{i}+0.36\hat{j}+0.88\hat{k}$,\;\;\;$\hat{n}_{23}=-0.82\hat{i}-0.4\hat{j}+0.4\hat{k}$,\;\;\;$\hat{n}_{25}=0.83\hat{i}+0.37\hat{j}-0.41\hat{k}$,\;\;\;$\hat{n}_{45}=0.0\hat{i}+0.0\hat{j}+1.0\hat{k}$,\newline
$\vec{r}_{14}=10.0\hat{i}+10.0\hat{j}+0.0\hat{k}$,\;\;\;$\vec{r}_{23}=10.0\hat{i}+0.0\hat{j}+10.0\hat{k}$,\;\;\;$\vec{r}_{25}=0.0\hat{i}+10.0\hat{j}+10.0\hat{k}$,\;\;\;$\vec{r}_{34}=0.0\hat{i}+0.0\hat{j}+0.0\hat{k}$.

{\tiny 2D-M121:}

$\hat{n}_{14}=0.9\hat{i}+0.39\hat{j}-0.18\hat{k}$,\;\;\;$\hat{n}_{23}=-0.0\hat{i}+0.71\hat{j}+0.71\hat{k}$,\;\;\;$\hat{n}_{34}=-0.0\hat{i}+0.71\hat{j}-0.71\hat{k}$,\;\;\;$\hat{n}_{45}=-0.93\hat{i}+0.25\hat{j}-0.25\hat{k}$,\newline
$\vec{r}_{14}=10.0\hat{i}+0.0\hat{j}+0.0\hat{k}$,\;\;\;$\vec{r}_{23}=10.0\hat{i}+0.0\hat{j}+0.0\hat{k}$,\;\;\;$\vec{r}_{25}=0.0\hat{i}+0.0\hat{j}+10.0\hat{k}$,\;\;\;$\vec{r}_{45}=10.0\hat{i}+10.0\hat{j}+0.0\hat{k}$.

{\tiny 2D-M122:}

$\hat{n}_{14}=-0.66\hat{i}+0.15\hat{j}+0.74\hat{k}$,\;\;\;$\hat{n}_{23}=-0.0\hat{i}+0.71\hat{j}-0.71\hat{k}$,\;\;\;$\hat{n}_{34}=0.63\hat{i}+0.55\hat{j}+0.55\hat{k}$,\;\;\;$\hat{n}_{45}=0.77\hat{i}-0.45\hat{j}-0.45\hat{k}$,\newline
$\vec{r}_{14}=10.0\hat{i}+0.0\hat{j}+0.0\hat{k}$,\;\;\;$\vec{r}_{23}=0.0\hat{i}+0.0\hat{j}+0.0\hat{k}$,\;\;\;$\vec{r}_{25}=10.0\hat{i}+0.0\hat{j}+10.0\hat{k}$,\;\;\;$\vec{r}_{34}=0.0\hat{i}+10.0\hat{j}+0.0\hat{k}$.

{\tiny 2D-M123:}

$\hat{n}_{14}=0.61\hat{i}+0.04\hat{j}+0.79\hat{k}$,\;\;\;$\hat{n}_{23}=-0.58\hat{i}-0.58\hat{j}+0.58\hat{k}$,\;\;\;$\hat{n}_{25}=0.42\hat{i}-0.89\hat{j}-0.2\hat{k}$,\;\;\;$\hat{n}_{34}=0.15\hat{i}+0.62\hat{j}+0.77\hat{k}$,\newline
$\vec{r}_{14}=10.0\hat{i}+10.0\hat{j}+0.0\hat{k}$,\;\;\;$\vec{r}_{25}=0.0\hat{i}+0.0\hat{j}+10.0\hat{k}$,\;\;\;$\vec{r}_{34}=10.0\hat{i}+10.0\hat{j}+0.0\hat{k}$,\;\;\;$\vec{r}_{45}=0.0\hat{i}+0.0\hat{j}+10.0\hat{k}$.

{\tiny 2D-M124:}

$\hat{n}_{14}=0.25\hat{i}-0.67\hat{j}-0.7\hat{k}$,\;\;\;$\hat{n}_{23}=0.58\hat{i}+0.58\hat{j}-0.58\hat{k}$,\;\;\;$\hat{n}_{25}=0.0\hat{i}-0.0\hat{j}-1.0\hat{k}$,\;\;\;$\hat{n}_{45}=-0.71\hat{i}+0.71\hat{j}-0.0\hat{k}$,\newline
$\vec{r}_{14}=0.0\hat{i}+10.0\hat{j}+10.0\hat{k}$,\;\;\;$\vec{r}_{25}=10.0\hat{i}+10.0\hat{j}+10.0\hat{k}$,\;\;\;$\vec{r}_{34}=0.0\hat{i}+0.0\hat{j}+10.0\hat{k}$,\;\;\;$\vec{r}_{45}=10.0\hat{i}+10.0\hat{j}+0.0\hat{k}$.

{\tiny 2D-M125:}

$\hat{n}_{14}=0.0\hat{i}+0.0\hat{j}-1.0\hat{k}$,\;\;\;$\hat{n}_{23}=0.58\hat{i}-0.58\hat{j}+0.58\hat{k}$,\;\;\;$\hat{n}_{25}=-0.41\hat{i}-0.82\hat{j}-0.4\hat{k}$,\;\;\;$\hat{n}_{34}=0.31\hat{i}-0.6\hat{j}-0.73\hat{k}$,\newline
$\vec{r}_{14}=10.0\hat{i}+10.0\hat{j}+0.67\hat{k}$,\;\;\;$\vec{r}_{25}=10.0\hat{i}+0.0\hat{j}+0.0\hat{k}$,\;\;\;$\vec{r}_{34}=0.0\hat{i}+10.0\hat{j}+10.0\hat{k}$,\;\;\;$\vec{r}_{45}=0.0\hat{i}+10.0\hat{j}+10.0\hat{k}$.

{\tiny 2D-M126:}

$\hat{n}_{14}=0.43\hat{i}-0.74\hat{j}-0.52\hat{k}$,\;\;\;$\hat{n}_{23}=0.07\hat{i}-0.94\hat{j}+0.33\hat{k}$,\;\;\;$\hat{n}_{25}=0.07\hat{i}-0.83\hat{j}+0.55\hat{k}$,\;\;\;$\hat{n}_{45}=0.02\hat{i}+0.87\hat{j}+0.5\hat{k}$,\newline
$\vec{r}_{14}=10.0\hat{i}+10.0\hat{j}+0.0\hat{k}$,\;\;\;$\vec{r}_{25}=4.06\hat{i}+3.92\hat{j}+4.65\hat{k}$,\;\;\;$\vec{r}_{34}=5.03\hat{i}+4.27\hat{j}+5.76\hat{k}$,\;\;\;$\vec{r}_{45}=0.0\hat{i}+10.0\hat{j}+10.0\hat{k}$.

{\tiny 2D-M127:}

$\hat{n}_{14}=-0.0\hat{i}+0.59\hat{j}+0.81\hat{k}$,\;\;\;$\hat{n}_{23}=0.0\hat{i}+0.72\hat{j}-0.7\hat{k}$,\;\;\;$\hat{n}_{34}=-0.82\hat{i}-0.45\hat{j}+0.37\hat{k}$,\;\;\;$\hat{n}_{45}=-0.06\hat{i}+0.7\hat{j}+0.71\hat{k}$,\newline
$\vec{r}_{14}=10.0\hat{i}+0.0\hat{j}+0.0\hat{k}$,\;\;\;$\vec{r}_{25}=0.0\hat{i}+10.0\hat{j}+10.0\hat{k}$,\;\;\;$\vec{r}_{34}=10.0\hat{i}+0.0\hat{j}+0.0\hat{k}$,\;\;\;$\vec{r}_{45}=10.0\hat{i}+10.0\hat{j}+0.0\hat{k}$.

{\tiny 2D-M128:}

$\hat{n}_{14}=-0.0\hat{i}+0.86\hat{j}+0.51\hat{k}$,\;\;\;$\hat{n}_{23}=-0.2\hat{i}-0.95\hat{j}+0.24\hat{k}$,\;\;\;$\hat{n}_{34}=0.58\hat{i}-0.81\hat{j}-0.05\hat{k}$,\;\;\;$\hat{n}_{45}=-0.59\hat{i}+0.15\hat{j}-0.8\hat{k}$,\newline
$\vec{r}_{14}=0.0\hat{i}+0.0\hat{j}+10.0\hat{k}$,\;\;\;$\vec{r}_{25}=6.36\hat{i}+5.69\hat{j}+8.17\hat{k}$,\;\;\;$\vec{r}_{34}=6.17\hat{i}+5.22\hat{j}+2.99\hat{k}$,\;\;\;$\vec{r}_{45}=0.0\hat{i}+10.0\hat{j}+0.0\hat{k}$.

{\tiny 2D-M129:}

$\hat{n}_{14}=-0.71\hat{i}+0.09\hat{j}+0.7\hat{k}$,\;\;\;$\hat{n}_{23}=-0.0\hat{i}+0.0\hat{j}-1.0\hat{k}$,\;\;\;$\hat{n}_{25}=0.56\hat{i}+0.67\hat{j}+0.49\hat{k}$,\;\;\;$\hat{n}_{34}=0.71\hat{i}-0.71\hat{j}-0.0\hat{k}$,\newline
$\vec{r}_{14}=10.0\hat{i}+0.0\hat{j}+0.0\hat{k}$,\;\;\;$\vec{r}_{23}=0.0\hat{i}+10.0\hat{j}+0.0\hat{k}$,\;\;\;$\vec{r}_{25}=10.0\hat{i}+0.0\hat{j}+0.0\hat{k}$,\;\;\;$\vec{r}_{45}=10.0\hat{i}+0.0\hat{j}+0.0\hat{k}$.

{\tiny 2D-M130:}

$\hat{n}_{14}=-0.53\hat{i}+0.27\hat{j}+0.8\hat{k}$,\;\;\;$\hat{n}_{23}=-0.9\hat{i}+0.11\hat{j}-0.41\hat{k}$,\;\;\;$\hat{n}_{25}=-0.67\hat{i}-0.67\hat{j}-0.34\hat{k}$,\;\;\;$\hat{n}_{45}=-0.0\hat{i}+0.0\hat{j}+1.0\hat{k}$,\newline
$\vec{r}_{14}=0.0\hat{i}+10.0\hat{j}+10.0\hat{k}$,\;\;\;$\vec{r}_{23}=0.0\hat{i}+0.0\hat{j}+10.0\hat{k}$,\;\;\;$\vec{r}_{25}=10.0\hat{i}+0.0\hat{j}+0.0\hat{k}$,\;\;\;$\vec{r}_{34}=0.0\hat{i}+10.0\hat{j}+0.0\hat{k}$.

{\tiny 2D-M131:}

$\hat{n}_{14}=-0.09\hat{i}-0.53\hat{j}+0.84\hat{k}$,\;\;\;$\hat{n}_{23}=0.7\hat{i}+0.38\hat{j}-0.61\hat{k}$,\;\;\;$\hat{n}_{25}=-0.69\hat{i}+0.11\hat{j}-0.72\hat{k}$,\;\;\;$\hat{n}_{34}=-0.81\hat{i}+0.56\hat{j}-0.15\hat{k}$,\newline
$\vec{r}_{14}=10.0\hat{i}+10.0\hat{j}+10.0\hat{k}$,\;\;\;$\vec{r}_{23}=10.0\hat{i}+0.0\hat{j}+0.0\hat{k}$,\;\;\;$\vec{r}_{34}=0.0\hat{i}+0.0\hat{j}+10.0\hat{k}$,\;\;\;$\vec{r}_{45}=10.0\hat{i}+10.0\hat{j}+10.0\hat{k}$.

{\tiny 2D-M132:}

$\hat{n}_{14}=0.01\hat{i}+0.86\hat{j}-0.51\hat{k}$,\;\;\;$\hat{n}_{23}=0.41\hat{i}-0.89\hat{j}-0.2\hat{k}$,\;\;\;$\hat{n}_{25}=0.09\hat{i}-0.99\hat{j}+0.07\hat{k}$,\;\;\;$\hat{n}_{45}=0.43\hat{i}-0.74\hat{j}+0.51\hat{k}$,\newline
$\vec{r}_{14}=0.0\hat{i}+10.0\hat{j}+0.0\hat{k}$,\;\;\;$\vec{r}_{23}=2.99\hat{i}+6.07\hat{j}+3.02\hat{k}$,\;\;\;$\vec{r}_{34}=6.84\hat{i}+4.37\hat{j}+3.84\hat{k}$,\;\;\;$\vec{r}_{45}=10.0\hat{i}+10.0\hat{j}+10.0\hat{k}$.

{\tiny 2D-M133:}

$\hat{n}_{14}=0.81\hat{i}-0.36\hat{j}+0.46\hat{k}$,\;\;\;$\hat{n}_{23}=0.9\hat{i}+0.31\hat{j}-0.31\hat{k}$,\;\;\;$\hat{n}_{34}=-0.0\hat{i}+0.71\hat{j}+0.71\hat{k}$,\;\;\;$\hat{n}_{45}=-0.44\hat{i}+0.64\hat{j}-0.64\hat{k}$,\newline
$\vec{r}_{14}=10.0\hat{i}+10.0\hat{j}+0.0\hat{k}$,\;\;\;$\vec{r}_{23}=10.0\hat{i}+0.0\hat{j}+0.0\hat{k}$,\;\;\;$\vec{r}_{25}=0.0\hat{i}+10.0\hat{j}+10.0\hat{k}$,\;\;\;$\vec{r}_{34}=0.0\hat{i}+0.0\hat{j}+10.0\hat{k}$.

{\tiny 2D-M134:}

$\hat{n}_{14}=0.38\hat{i}+0.67\hat{j}+0.64\hat{k}$,\;\;\;$\hat{n}_{23}=0.04\hat{i}-0.98\hat{j}+0.18\hat{k}$,\;\;\;$\hat{n}_{34}=0.65\hat{i}-0.75\hat{j}-0.17\hat{k}$,\;\;\;$\hat{n}_{45}=0.7\hat{i}-0.1\hat{j}-0.7\hat{k}$,\newline
$\vec{r}_{14}=10.0\hat{i}+0.0\hat{j}+0.0\hat{k}$,\;\;\;$\vec{r}_{23}=5.69\hat{i}+5.22\hat{j}+4.09\hat{k}$,\;\;\;$\vec{r}_{25}=3.77\hat{i}+3.77\hat{j}+3.8\hat{k}$,\;\;\;$\vec{r}_{45}=10.0\hat{i}+10.0\hat{j}+10.0\hat{k}$.

{\tiny 2D-M135:}

$\hat{n}_{14}=-0.13\hat{i}+0.65\hat{j}-0.75\hat{k}$,\;\;\;$\hat{n}_{25}=-0.6\hat{i}+0.78\hat{j}+0.18\hat{k}$,\;\;\;$\hat{n}_{34}=-0.58\hat{i}-0.58\hat{j}+0.58\hat{k}$,\;\;\;$\hat{n}_{45}=0.56\hat{i}+0.24\hat{j}+0.8\hat{k}$,\newline
$\vec{r}_{14}=10.0\hat{i}+10.0\hat{j}+10.0\hat{k}$,\;\;\;$\vec{r}_{23}=10.0\hat{i}+10.0\hat{j}+0.0\hat{k}$,\;\;\;$\vec{r}_{25}=0.0\hat{i}+0.0\hat{j}+10.0\hat{k}$,\;\;\;$\vec{r}_{45}=0.0\hat{i}+0.0\hat{j}+10.0\hat{k}$.

{\tiny 2D-M136:}

$\hat{n}_{14}=-0.0\hat{i}+0.57\hat{j}-0.82\hat{k}$,\;\;\;$\hat{n}_{25}=0.69\hat{i}-0.69\hat{j}-0.22\hat{k}$,\;\;\;$\hat{n}_{34}=0.87\hat{i}+0.21\hat{j}+0.45\hat{k}$,\;\;\;$\hat{n}_{45}=-0.0\hat{i}+0.56\hat{j}-0.83\hat{k}$,\newline
$\vec{r}_{14}=10.0\hat{i}+10.0\hat{j}+10.0\hat{k}$,\;\;\;$\vec{r}_{23}=0.0\hat{i}+0.0\hat{j}+10.0\hat{k}$,\;\;\;$\vec{r}_{25}=10.0\hat{i}+10.0\hat{j}+10.0\hat{k}$,\;\;\;$\vec{r}_{34}=10.0\hat{i}+10.0\hat{j}+0.0\hat{k}$.

{\tiny 2D-M137:}

$\hat{n}_{14}=-0.43\hat{i}-0.25\hat{j}-0.87\hat{k}$,\;\;\;$\hat{n}_{25}=-0.58\hat{i}+0.58\hat{j}-0.58\hat{k}$,\;\;\;$\hat{n}_{34}=-0.0\hat{i}+0.0\hat{j}-1.0\hat{k}$,\;\;\;$\hat{n}_{45}=-0.71\hat{i}-0.71\hat{j}-0.0\hat{k}$,\newline
$\vec{r}_{14}=10.0\hat{i}+10.0\hat{j}+0.0\hat{k}$,\;\;\;$\vec{r}_{23}=0.0\hat{i}+10.0\hat{j}+10.0\hat{k}$,\;\;\;$\vec{r}_{34}=10.0\hat{i}+0.0\hat{j}+0.0\hat{k}$,\;\;\;$\vec{r}_{45}=10.0\hat{i}+0.0\hat{j}+0.0\hat{k}$.

{\tiny 2D-M138:}

$\hat{n}_{14}=0.17\hat{i}-0.5\hat{j}-0.85\hat{k}$,\;\;\;$\hat{n}_{25}=-0.79\hat{i}-0.49\hat{j}-0.37\hat{k}$,\;\;\;$\hat{n}_{34}=-0.35\hat{i}-0.79\hat{j}+0.51\hat{k}$,\;\;\;$\hat{n}_{45}=0.77\hat{i}-0.23\hat{j}+0.6\hat{k}$,\newline
$\vec{r}_{14}=10.0\hat{i}+0.0\hat{j}+0.0\hat{k}$,\;\;\;$\vec{r}_{23}=6.47\hat{i}+3.98\hat{j}+5.17\hat{k}$,\;\;\;$\vec{r}_{34}=9.55\hat{i}+4.3\hat{j}+5.0\hat{k}$,\;\;\;$\vec{r}_{45}=10.0\hat{i}+10.0\hat{j}+0.0\hat{k}$.

{\tiny 2D-M139:}

$\hat{n}_{14}=-0.0\hat{i}+0.67\hat{j}-0.74\hat{k}$,\;\;\;$\hat{n}_{25}=0.54\hat{i}-0.14\hat{j}+0.83\hat{k}$,\;\;\;$\hat{n}_{34}=0.17\hat{i}-0.7\hat{j}-0.7\hat{k}$,\;\;\;$\hat{n}_{45}=0.63\hat{i}+0.7\hat{j}-0.34\hat{k}$,\newline
$\vec{r}_{14}=0.0\hat{i}+0.0\hat{j}+0.0\hat{k}$,\;\;\;$\vec{r}_{23}=0.0\hat{i}+0.0\hat{j}+10.0\hat{k}$,\;\;\;$\vec{r}_{25}=10.0\hat{i}+10.0\hat{j}+0.0\hat{k}$,\;\;\;$\vec{r}_{34}=10.0\hat{i}+0.0\hat{j}+0.0\hat{k}$.

{\tiny 2D-M140:}

$\hat{n}_{14}=-0.0\hat{i}+0.0\hat{j}-1.0\hat{k}$,\;\;\;$\hat{n}_{25}=0.39\hat{i}+0.27\hat{j}+0.88\hat{k}$,\;\;\;$\hat{n}_{34}=-0.19\hat{i}-0.77\hat{j}+0.6\hat{k}$,\;\;\;$\hat{n}_{45}=0.0\hat{i}+0.74\hat{j}-0.67\hat{k}$,\newline
$\vec{r}_{14}=10.0\hat{i}+10.0\hat{j}+9.9\hat{k}$,\;\;\;$\vec{r}_{23}=4.36\hat{i}+0.9\hat{j}+3.84\hat{k}$,\;\;\;$\vec{r}_{25}=7.17\hat{i}+1.16\hat{j}+6.63\hat{k}$,\;\;\;$\vec{r}_{45}=0.0\hat{i}+10.0\hat{j}+0.0\hat{k}$.

{\tiny 2D-M141:}

$\hat{n}_{14}=-0.38\hat{i}+0.38\hat{j}+0.84\hat{k}$,\;\;\;$\hat{n}_{15}=0.93\hat{i}-0.2\hat{j}-0.3\hat{k}$,\;\;\;$\hat{n}_{23}=0.0\hat{i}+0.95\hat{j}+0.31\hat{k}$,\;\;\;$\hat{n}_{25}=-0.0\hat{i}+0.74\hat{j}+0.67\hat{k}$,\newline
$\vec{r}_{14}=0.0\hat{i}+0.0\hat{j}+10.0\hat{k}$,\;\;\;$\vec{r}_{15}=0.0\hat{i}+0.0\hat{j}+0.0\hat{k}$,\;\;\;$\vec{r}_{23}=10.0\hat{i}+0.0\hat{j}+0.0\hat{k}$,\;\;\;$\vec{r}_{34}=10.0\hat{i}+10.0\hat{j}+10.0\hat{k}$.

{\tiny 2D-M142:}

$\hat{n}_{14}=0.71\hat{i}-0.71\hat{j}+0.0\hat{k}$,\;\;\;$\hat{n}_{15}=0.82\hat{i}-0.41\hat{j}+0.41\hat{k}$,\;\;\;$\hat{n}_{23}=0.0\hat{i}+0.0\hat{j}-1.0\hat{k}$,\;\;\;$\hat{n}_{34}=-0.58\hat{i}-0.58\hat{j}+0.58\hat{k}$,\newline
$\vec{r}_{14}=10.0\hat{i}+10.0\hat{j}+0.0\hat{k}$,\;\;\;$\vec{r}_{15}=10.0\hat{i}+10.0\hat{j}+0.0\hat{k}$,\;\;\;$\vec{r}_{23}=10.0\hat{i}+10.0\hat{j}+8.6\hat{k}$,\;\;\;$\vec{r}_{25}=0.0\hat{i}+0.0\hat{j}+10.0\hat{k}$.

{\tiny 2D-M143:}

$\hat{n}_{14}=-0.19\hat{i}+0.78\hat{j}+0.6\hat{k}$,\;\;\;$\hat{n}_{15}=-0.71\hat{i}+0.69\hat{j}-0.14\hat{k}$,\;\;\;$\hat{n}_{23}=-0.68\hat{i}-0.7\hat{j}+0.21\hat{k}$,\;\;\;$\hat{n}_{25}=0.79\hat{i}-0.24\hat{j}+0.56\hat{k}$,\newline
$\vec{r}_{14}=10.0\hat{i}+10.0\hat{j}+0.0\hat{k}$,\;\;\;$\vec{r}_{15}=10.0\hat{i}+10.0\hat{j}+10.0\hat{k}$,\;\;\;$\vec{r}_{25}=10.0\hat{i}+10.0\hat{j}+0.0\hat{k}$,\;\;\;$\vec{r}_{34}=0.0\hat{i}+0.0\hat{j}+10.0\hat{k}$.

{\tiny 2D-M144:}

$\hat{n}_{14}=0.24\hat{i}+0.8\hat{j}+0.56\hat{k}$,\;\;\;$\hat{n}_{15}=-0.0\hat{i}+0.0\hat{j}-1.0\hat{k}$,\;\;\;$\hat{n}_{23}=-0.65\hat{i}+0.74\hat{j}-0.15\hat{k}$,\;\;\;$\hat{n}_{34}=0.9\hat{i}-0.31\hat{j}-0.31\hat{k}$,\newline
$\vec{r}_{14}=0.0\hat{i}+10.0\hat{j}+10.0\hat{k}$,\;\;\;$\vec{r}_{15}=0.0\hat{i}+10.0\hat{j}+9.72\hat{k}$,\;\;\;$\vec{r}_{25}=10.0\hat{i}+0.0\hat{j}+0.0\hat{k}$,\;\;\;$\vec{r}_{34}=0.0\hat{i}+0.0\hat{j}+10.0\hat{k}$.

{\tiny 2D-M145:}

$\hat{n}_{14}=0.28\hat{i}-0.8\hat{j}-0.53\hat{k}$,\;\;\;$\hat{n}_{15}=0.69\hat{i}-0.71\hat{j}-0.14\hat{k}$,\;\;\;$\hat{n}_{25}=0.77\hat{i}-0.15\hat{j}+0.62\hat{k}$,\;\;\;$\hat{n}_{34}=0.7\hat{i}+0.68\hat{j}-0.21\hat{k}$,\newline
$\vec{r}_{14}=0.0\hat{i}+0.0\hat{j}+10.0\hat{k}$,\;\;\;$\vec{r}_{15}=0.0\hat{i}+0.0\hat{j}+0.0\hat{k}$,\;\;\;$\vec{r}_{23}=10.0\hat{i}+10.0\hat{j}+0.0\hat{k}$,\;\;\;$\vec{r}_{25}=0.0\hat{i}+0.0\hat{j}+10.0\hat{k}$.

{\tiny 2D-M146:}

$\hat{n}_{14}=0.69\hat{i}+0.02\hat{j}+0.72\hat{k}$,\;\;\;$\hat{n}_{15}=0.82\hat{i}-0.41\hat{j}+0.41\hat{k}$,\;\;\;$\hat{n}_{25}=-0.58\hat{i}-0.58\hat{j}+0.58\hat{k}$,\;\;\;$\hat{n}_{34}=0.43\hat{i}-0.82\hat{j}-0.39\hat{k}$,\newline
$\vec{r}_{14}=10.0\hat{i}+10.0\hat{j}+0.0\hat{k}$,\;\;\;$\vec{r}_{15}=10.0\hat{i}+10.0\hat{j}+0.0\hat{k}$,\;\;\;$\vec{r}_{23}=0.0\hat{i}+0.0\hat{j}+10.0\hat{k}$,\;\;\;$\vec{r}_{34}=10.0\hat{i}+10.0\hat{j}+0.0\hat{k}$.

{\tiny 2D-M147:}

$\hat{n}_{14}=-0.44\hat{i}-0.86\hat{j}-0.26\hat{k}$,\;\;\;$\hat{n}_{23}=-0.36\hat{i}+0.55\hat{j}-0.76\hat{k}$,\;\;\;$\hat{n}_{25}=0.55\hat{i}-0.62\hat{j}-0.56\hat{k}$,\;\;\;$\hat{n}_{34}=0.54\hat{i}-0.25\hat{j}+0.81\hat{k}$,\newline
$\vec{r}_{14}=0.0\hat{i}+10.0\hat{j}+10.0\hat{k}$,\;\;\;$\vec{r}_{15}=0.0\hat{i}+10.0\hat{j}+0.0\hat{k}$,\;\;\;$\vec{r}_{23}=0.0\hat{i}+10.0\hat{j}+0.0\hat{k}$,\;\;\;$\vec{r}_{34}=10.0\hat{i}+0.0\hat{j}+10.0\hat{k}$.

{\tiny 2D-M148:}

$\hat{n}_{14}=0.92\hat{i}+0.25\hat{j}-0.3\hat{k}$,\;\;\;$\hat{n}_{23}=0.14\hat{i}+0.63\hat{j}+0.77\hat{k}$,\;\;\;$\hat{n}_{25}=-0.06\hat{i}+0.68\hat{j}+0.73\hat{k}$,\;\;\;$\hat{n}_{34}=0.59\hat{i}-0.57\hat{j}+0.57\hat{k}$,\newline
$\vec{r}_{14}=0.0\hat{i}+0.0\hat{j}+0.0\hat{k}$,\;\;\;$\vec{r}_{15}=10.0\hat{i}+0.0\hat{j}+0.0\hat{k}$,\;\;\;$\vec{r}_{23}=10.0\hat{i}+0.0\hat{j}+0.0\hat{k}$,\;\;\;$\vec{r}_{25}=0.0\hat{i}+10.0\hat{j}+10.0\hat{k}$.

{\tiny 2D-M149:}

$\hat{n}_{14}=-0.36\hat{i}+0.55\hat{j}-0.76\hat{k}$,\;\;\;$\hat{n}_{23}=0.55\hat{i}-0.62\hat{j}-0.56\hat{k}$,\;\;\;$\hat{n}_{25}=0.44\hat{i}+0.86\hat{j}+0.26\hat{k}$,\;\;\;$\hat{n}_{34}=-0.54\hat{i}+0.25\hat{j}-0.81\hat{k}$,\newline
$\vec{r}_{14}=0.0\hat{i}+10.0\hat{j}+0.0\hat{k}$,\;\;\;$\vec{r}_{15}=0.0\hat{i}+10.0\hat{j}+0.0\hat{k}$,\;\;\;$\vec{r}_{25}=0.0\hat{i}+10.0\hat{j}+10.0\hat{k}$,\;\;\;$\vec{r}_{34}=10.0\hat{i}+0.0\hat{j}+10.0\hat{k}$.

{\tiny 2D-M150:}

$\hat{n}_{14}=-0.23\hat{i}+0.48\hat{j}-0.85\hat{k}$,\;\;\;$\hat{n}_{23}=-0.61\hat{i}+0.57\hat{j}+0.55\hat{k}$,\;\;\;$\hat{n}_{25}=0.0\hat{i}+0.69\hat{j}-0.72\hat{k}$,\;\;\;$\hat{n}_{34}=-0.94\hat{i}-0.33\hat{j}-0.03\hat{k}$,\newline
$\vec{r}_{14}=10.0\hat{i}+0.0\hat{j}+10.0\hat{k}$,\;\;\;$\vec{r}_{15}=10.0\hat{i}+0.0\hat{j}+10.0\hat{k}$,\;\;\;$\vec{r}_{25}=0.0\hat{i}+10.0\hat{j}+0.0\hat{k}$,\;\;\;$\vec{r}_{34}=10.0\hat{i}+0.0\hat{j}+0.0\hat{k}$.

{\tiny 2D-M151:}

$\hat{n}_{14}=0.61\hat{i}-0.2\hat{j}-0.77\hat{k}$,\;\;\;$\hat{n}_{23}=0.34\hat{i}-0.46\hat{j}-0.82\hat{k}$,\;\;\;$\hat{n}_{25}=0.8\hat{i}+0.48\hat{j}+0.36\hat{k}$,\;\;\;$\hat{n}_{34}=0.62\hat{i}-0.55\hat{j}+0.56\hat{k}$,\newline
$\vec{r}_{14}=10.0\hat{i}+0.0\hat{j}+0.0\hat{k}$,\;\;\;$\vec{r}_{15}=10.0\hat{i}+0.0\hat{j}+0.0\hat{k}$,\;\;\;$\vec{r}_{23}=0.0\hat{i}+10.0\hat{j}+10.0\hat{k}$,\;\;\;$\vec{r}_{25}=10.0\hat{i}+0.0\hat{j}+10.0\hat{k}$.

{\tiny 2D-M152:}

$\hat{n}_{14}=0.66\hat{i}-0.45\hat{j}-0.6\hat{k}$,\;\;\;$\hat{n}_{23}=-0.5\hat{i}+0.8\hat{j}-0.33\hat{k}$,\;\;\;$\hat{n}_{25}=-0.0\hat{i}+0.0\hat{j}-1.0\hat{k}$,\;\;\;$\hat{n}_{34}=0.29\hat{i}+0.06\hat{j}-0.95\hat{k}$,\newline
$\vec{r}_{14}=0.0\hat{i}+10.0\hat{j}+10.0\hat{k}$,\;\;\;$\vec{r}_{15}=10.0\hat{i}+10.0\hat{j}+10.0\hat{k}$,\;\;\;$\vec{r}_{23}=0.0\hat{i}+10.0\hat{j}+0.0\hat{k}$,\;\;\;$\vec{r}_{34}=10.0\hat{i}+0.0\hat{j}+0.0\hat{k}$.

{\tiny 2D-M153:}

$\hat{n}_{14}=-0.06\hat{i}+0.99\hat{j}-0.11\hat{k}$,\;\;\;$\hat{n}_{24}=0.0\hat{i}+0.86\hat{j}-0.5\hat{k}$,\;\;\;$\hat{n}_{25}=-0.68\hat{i}-0.73\hat{j}+0.1\hat{k}$,\;\;\;$\hat{n}_{34}=0.0\hat{i}+0.56\hat{j}+0.83\hat{k}$,\newline
$\vec{r}_{24}=10.0\hat{i}+10.0\hat{j}+10.0\hat{k}$,\;\;\;$\vec{r}_{25}=10.0\hat{i}+0.0\hat{j}+10.0\hat{k}$,\;\;\;$\vec{r}_{34}=10.0\hat{i}+0.0\hat{j}+0.0\hat{k}$,\;\;\;$\vec{r}_{35}=0.0\hat{i}+10.0\hat{j}+0.0\hat{k}$.

{\tiny 2D-M154:}

$\hat{n}_{14}=0.49\hat{i}+0.46\hat{j}-0.74\hat{k}$,\;\;\;$\hat{n}_{24}=-0.0\hat{i}+0.29\hat{j}+0.96\hat{k}$,\;\;\;$\hat{n}_{25}=-0.55\hat{i}-0.55\hat{j}+0.63\hat{k}$,\;\;\;$\hat{n}_{35}=0.46\hat{i}-0.88\hat{j}-0.05\hat{k}$,\newline
$\vec{r}_{24}=10.0\hat{i}+10.0\hat{j}+0.0\hat{k}$,\;\;\;$\vec{r}_{25}=0.0\hat{i}+10.0\hat{j}+0.0\hat{k}$,\;\;\;$\vec{r}_{34}=10.0\hat{i}+0.0\hat{j}+0.0\hat{k}$,\;\;\;$\vec{r}_{35}=10.0\hat{i}+10.0\hat{j}+10.0\hat{k}$.

{\tiny 2D-M155:}

$\hat{n}_{14}=0.0\hat{i}+0.71\hat{j}-0.7\hat{k}$,\;\;\;$\hat{n}_{24}=-0.0\hat{i}+0.66\hat{j}-0.75\hat{k}$,\;\;\;$\hat{n}_{25}=0.9\hat{i}+0.28\hat{j}+0.34\hat{k}$,\;\;\;$\hat{n}_{34}=0.0\hat{i}+0.71\hat{j}-0.7\hat{k}$,\newline
$\vec{r}_{24}=0.0\hat{i}+0.0\hat{j}+0.0\hat{k}$,\;\;\;$\vec{r}_{25}=0.0\hat{i}+10.0\hat{j}+0.0\hat{k}$,\;\;\;$\vec{r}_{34}=10.0\hat{i}+10.0\hat{j}+10.0\hat{k}$,\;\;\;$\vec{r}_{35}=10.0\hat{i}+0.0\hat{j}+10.0\hat{k}$.

{\tiny 2D-M156:}

$\hat{n}_{14}=-0.0\hat{i}-0.0\hat{j}-1.0\hat{k}$,\;\;\;$\hat{n}_{24}=0.0\hat{i}+0.73\hat{j}-0.68\hat{k}$,\;\;\;$\hat{n}_{25}=-0.57\hat{i}-0.66\hat{j}-0.5\hat{k}$,\;\;\;$\hat{n}_{35}=0.08\hat{i}-0.7\hat{j}+0.7\hat{k}$,\newline
$\vec{r}_{24}=0.0\hat{i}+0.0\hat{j}+0.0\hat{k}$,\;\;\;$\vec{r}_{25}=10.0\hat{i}+0.0\hat{j}+10.0\hat{k}$,\;\;\;$\vec{r}_{34}=0.0\hat{i}+10.0\hat{j}+0.0\hat{k}$,\;\;\;$\vec{r}_{35}=10.0\hat{i}+10.0\hat{j}+10.0\hat{k}$.

{\tiny 2D-M157:}

$\hat{n}_{14}=-0.0\hat{i}+0.64\hat{j}-0.76\hat{k}$,\;\;\;$\hat{n}_{24}=0.0\hat{i}+0.71\hat{j}-0.71\hat{k}$,\;\;\;$\hat{n}_{34}=-0.91\hat{i}+0.32\hat{j}+0.27\hat{k}$,\;\;\;$\hat{n}_{35}=-0.0\hat{i}+0.69\hat{j}-0.72\hat{k}$,\newline
$\vec{r}_{24}=0.0\hat{i}+10.0\hat{j}+0.0\hat{k}$,\;\;\;$\vec{r}_{25}=10.0\hat{i}+10.0\hat{j}+10.0\hat{k}$,\;\;\;$\vec{r}_{34}=0.0\hat{i}+0.0\hat{j}+0.0\hat{k}$,\;\;\;$\vec{r}_{35}=10.0\hat{i}+0.0\hat{j}+10.0\hat{k}$.

{\tiny 2D-M158:}

$\hat{n}_{14}=0.0\hat{i}+0.92\hat{j}+0.4\hat{k}$,\;\;\;$\hat{n}_{24}=0.15\hat{i}+0.34\hat{j}+0.93\hat{k}$,\;\;\;$\hat{n}_{25}=0.44\hat{i}+0.4\hat{j}-0.81\hat{k}$,\;\;\;$\hat{n}_{35}=-0.49\hat{i}-0.72\hat{j}-0.49\hat{k}$,\newline
$\vec{r}_{24}=0.0\hat{i}+10.0\hat{j}+10.0\hat{k}$,\;\;\;$\vec{r}_{25}=10.0\hat{i}+10.0\hat{j}+10.0\hat{k}$,\;\;\;$\vec{r}_{34}=10.0\hat{i}+0.0\hat{j}+10.0\hat{k}$,\;\;\;$\vec{r}_{35}=10.0\hat{i}+10.0\hat{j}+0.0\hat{k}$.

{\tiny 2D-M159:}

$\hat{n}_{14}=-0.03\hat{i}+0.83\hat{j}+0.56\hat{k}$,\;\;\;$\hat{n}_{23}=0.54\hat{i}+0.67\hat{j}+0.51\hat{k}$,\;\;\;$\hat{n}_{25}=-0.58\hat{i}-0.62\hat{j}+0.53\hat{k}$,\;\;\;$\hat{n}_{34}=0.0\hat{i}+0.1\hat{j}-1.0\hat{k}$,\newline
$\vec{r}_{23}=10.0\hat{i}+10.0\hat{j}+0.0\hat{k}$,\;\;\;$\vec{r}_{25}=10.0\hat{i}+10.0\hat{j}+10.0\hat{k}$,\;\;\;$\vec{r}_{34}=10.0\hat{i}+0.0\hat{j}+10.0\hat{k}$,\;\;\;$\vec{r}_{45}=0.0\hat{i}+10.0\hat{j}+0.0\hat{k}$.

{\tiny 2D-M160:}

$\hat{n}_{14}=-0.24\hat{i}-0.94\hat{j}+0.26\hat{k}$,\;\;\;$\hat{n}_{23}=0.65\hat{i}-0.65\hat{j}+0.41\hat{k}$,\;\;\;$\hat{n}_{25}=0.11\hat{i}-0.7\hat{j}+0.7\hat{k}$,\;\;\;$\hat{n}_{45}=-0.51\hat{i}+0.46\hat{j}+0.73\hat{k}$,\newline
$\vec{r}_{23}=10.0\hat{i}+10.0\hat{j}+0.0\hat{k}$,\;\;\;$\vec{r}_{25}=10.0\hat{i}+0.0\hat{j}+10.0\hat{k}$,\;\;\;$\vec{r}_{34}=0.0\hat{i}+0.0\hat{j}+0.0\hat{k}$,\;\;\;$\vec{r}_{45}=10.0\hat{i}+10.0\hat{j}+10.0\hat{k}$.

{\tiny 2D-M161:}

$\hat{n}_{14}=-0.0\hat{i}+0.0\hat{j}-1.0\hat{k}$,\;\;\;$\hat{n}_{23}=0.14\hat{i}+0.36\hat{j}+0.92\hat{k}$,\;\;\;$\hat{n}_{25}=0.0\hat{i}+0.48\hat{j}-0.88\hat{k}$,\;\;\;$\hat{n}_{34}=0.66\hat{i}+0.34\hat{j}-0.67\hat{k}$,\newline
$\vec{r}_{23}=10.0\hat{i}+10.0\hat{j}+0.0\hat{k}$,\;\;\;$\vec{r}_{25}=0.0\hat{i}+10.0\hat{j}+0.0\hat{k}$,\;\;\;$\vec{r}_{34}=10.0\hat{i}+0.0\hat{j}+0.0\hat{k}$,\;\;\;$\vec{r}_{45}=10.0\hat{i}+10.0\hat{j}+10.0\hat{k}$.

{\tiny 2D-M162:}

$\hat{n}_{14}=0.16\hat{i}+0.5\hat{j}-0.85\hat{k}$,\;\;\;$\hat{n}_{23}=0.65\hat{i}-0.38\hat{j}+0.65\hat{k}$,\;\;\;$\hat{n}_{25}=-0.0\hat{i}+0.5\hat{j}-0.86\hat{k}$,\;\;\;$\hat{n}_{45}=0.72\hat{i}-0.35\hat{j}+0.6\hat{k}$,\newline
$\vec{r}_{23}=0.0\hat{i}+0.0\hat{j}+10.0\hat{k}$,\;\;\;$\vec{r}_{25}=10.0\hat{i}+10.0\hat{j}+10.0\hat{k}$,\;\;\;$\vec{r}_{34}=0.0\hat{i}+10.0\hat{j}+0.0\hat{k}$,\;\;\;$\vec{r}_{45}=0.0\hat{i}+0.0\hat{j}+10.0\hat{k}$.

{\tiny 2D-M163:}

$\hat{n}_{14}=-0.0\hat{i}+0.64\hat{j}+0.77\hat{k}$,\;\;\;$\hat{n}_{23}=-0.0\hat{i}+0.98\hat{j}+0.22\hat{k}$,\;\;\;$\hat{n}_{34}=0.67\hat{i}-0.3\hat{j}+0.67\hat{k}$,\;\;\;$\hat{n}_{45}=0.0\hat{i}+0.49\hat{j}-0.87\hat{k}$,\newline
$\vec{r}_{23}=0.0\hat{i}+0.0\hat{j}+10.0\hat{k}$,\;\;\;$\vec{r}_{25}=0.0\hat{i}+10.0\hat{j}+0.0\hat{k}$,\;\;\;$\vec{r}_{34}=0.0\hat{i}+0.0\hat{j}+10.0\hat{k}$,\;\;\;$\vec{r}_{45}=10.0\hat{i}+10.0\hat{j}+10.0\hat{k}$.

{\tiny 2D-M164:}

$\hat{n}_{14}=0.55\hat{i}+0.44\hat{j}+0.71\hat{k}$,\;\;\;$\hat{n}_{23}=0.71\hat{i}-0.71\hat{j}-0.07\hat{k}$,\;\;\;$\hat{n}_{34}=0.63\hat{i}+0.74\hat{j}-0.24\hat{k}$,\;\;\;$\hat{n}_{45}=-0.73\hat{i}+0.68\hat{j}+0.1\hat{k}$,\newline
$\vec{r}_{23}=0.0\hat{i}+0.0\hat{j}+10.0\hat{k}$,\;\;\;$\vec{r}_{25}=10.0\hat{i}+10.0\hat{j}+10.0\hat{k}$,\;\;\;$\vec{r}_{34}=0.0\hat{i}+0.0\hat{j}+0.0\hat{k}$,\;\;\;$\vec{r}_{45}=0.0\hat{i}+0.0\hat{j}+0.0\hat{k}$.

{\tiny 2D-M165:}

$\hat{n}_{14}=-0.98\hat{i}-0.16\hat{j}+0.1\hat{k}$,\;\;\;$\hat{n}_{23}=-0.32\hat{i}-0.84\hat{j}+0.43\hat{k}$,\;\;\;$\hat{n}_{25}=0.74\hat{i}+0.36\hat{j}-0.57\hat{k}$,\;\;\;$\hat{n}_{34}=-0.73\hat{i}+0.65\hat{j}+0.21\hat{k}$,\newline
$\vec{r}_{23}=10.0\hat{i}+10.0\hat{j}+10.0\hat{k}$,\;\;\;$\vec{r}_{25}=0.0\hat{i}+10.0\hat{j}+0.0\hat{k}$,\;\;\;$\vec{r}_{34}=10.0\hat{i}+10.0\hat{j}+0.0\hat{k}$,\;\;\;$\vec{r}_{45}=0.0\hat{i}+0.0\hat{j}+0.0\hat{k}$.

{\tiny 2D-M166:}

$\hat{n}_{14}=0.44\hat{i}+0.11\hat{j}-0.89\hat{k}$,\;\;\;$\hat{n}_{23}=0.0\hat{i}+0.86\hat{j}-0.52\hat{k}$,\;\;\;$\hat{n}_{25}=-0.62\hat{i}+0.14\hat{j}+0.77\hat{k}$,\;\;\;$\hat{n}_{45}=-0.0\hat{i}+0.54\hat{j}-0.84\hat{k}$,\newline
$\vec{r}_{23}=10.0\hat{i}+10.0\hat{j}+10.0\hat{k}$,\;\;\;$\vec{r}_{25}=0.0\hat{i}+10.0\hat{j}+10.0\hat{k}$,\;\;\;$\vec{r}_{34}=10.0\hat{i}+0.0\hat{j}+0.0\hat{k}$,\;\;\;$\vec{r}_{45}=0.0\hat{i}+10.0\hat{j}+0.0\hat{k}$.

{\tiny 2D-M167:}

$\hat{n}_{14}=-0.83\hat{i}+0.47\hat{j}+0.3\hat{k}$,\;\;\;$\hat{n}_{23}=-0.67\hat{i}-0.68\hat{j}-0.31\hat{k}$,\;\;\;$\hat{n}_{34}=-0.6\hat{i}+0.6\hat{j}+0.53\hat{k}$,\;\;\;$\hat{n}_{45}=0.67\hat{i}-0.57\hat{j}-0.48\hat{k}$,\newline
$\vec{r}_{23}=0.0\hat{i}+10.0\hat{j}+10.0\hat{k}$,\;\;\;$\vec{r}_{25}=10.0\hat{i}+10.0\hat{j}+0.0\hat{k}$,\;\;\;$\vec{r}_{34}=0.0\hat{i}+0.0\hat{j}+0.0\hat{k}$,\;\;\;$\vec{r}_{45}=0.0\hat{i}+0.0\hat{j}+0.0\hat{k}$.

{\tiny 2D-M168:}

$\hat{n}_{14}=-0.0\hat{i}+0.74\hat{j}+0.67\hat{k}$,\;\;\;$\hat{n}_{25}=0.6\hat{i}-0.54\hat{j}-0.6\hat{k}$,\;\;\;$\hat{n}_{34}=-0.64\hat{i}-0.54\hat{j}-0.54\hat{k}$,\;\;\;$\hat{n}_{45}=-0.0\hat{i}+0.45\hat{j}-0.89\hat{k}$,\newline
$\vec{r}_{23}=0.0\hat{i}+10.0\hat{j}+10.0\hat{k}$,\;\;\;$\vec{r}_{25}=0.0\hat{i}+0.0\hat{j}+0.0\hat{k}$,\;\;\;$\vec{r}_{34}=10.0\hat{i}+10.0\hat{j}+0.0\hat{k}$,\;\;\;$\vec{r}_{45}=10.0\hat{i}+0.0\hat{j}+10.0\hat{k}$.

{\tiny 2D-M169:}

$\hat{n}_{14}=-0.49\hat{i}-0.87\hat{j}-0.08\hat{k}$,\;\;\;$\hat{n}_{25}=0.41\hat{i}+0.91\hat{j}+0.0\hat{k}$,\;\;\;$\hat{n}_{34}=0.49\hat{i}+0.53\hat{j}+0.69\hat{k}$,\;\;\;$\hat{n}_{45}=-0.0\hat{i}+0.68\hat{j}-0.74\hat{k}$,\newline
$\vec{r}_{23}=0.0\hat{i}+10.0\hat{j}+0.0\hat{k}$,\;\;\;$\vec{r}_{25}=0.0\hat{i}+10.0\hat{j}+10.0\hat{k}$,\;\;\;$\vec{r}_{34}=10.0\hat{i}+0.0\hat{j}+10.0\hat{k}$,\;\;\;$\vec{r}_{45}=10.0\hat{i}+10.0\hat{j}+10.0\hat{k}$.

{\tiny 2D-M170:}

$\hat{n}_{14}=-0.0\hat{i}+0.0\hat{j}-1.0\hat{k}$,\;\;\;$\hat{n}_{25}=0.36\hat{i}+0.86\hat{j}-0.37\hat{k}$,\;\;\;$\hat{n}_{34}=-0.0\hat{i}+0.92\hat{j}-0.39\hat{k}$,\;\;\;$\hat{n}_{45}=-0.0\hat{i}-0.0\hat{j}-1.0\hat{k}$,\newline
$\vec{r}_{23}=0.0\hat{i}+10.0\hat{j}+10.0\hat{k}$,\;\;\;$\vec{r}_{25}=10.0\hat{i}+0.0\hat{j}+10.0\hat{k}$,\;\;\;$\vec{r}_{34}=0.0\hat{i}+0.0\hat{j}+0.0\hat{k}$,\;\;\;$\vec{r}_{45}=10.0\hat{i}+10.0\hat{j}+10.0\hat{k}$.

{\tiny 2D-M171:}

$\hat{n}_{14}=-0.0\hat{i}+0.75\hat{j}+0.66\hat{k}$,\;\;\;$\hat{n}_{15}=0.92\hat{i}-0.07\hat{j}+0.39\hat{k}$,\;\;\;$\hat{n}_{23}=-0.0\hat{i}+0.0\hat{j}-1.0\hat{k}$,\;\;\;$\hat{n}_{25}=0.0\hat{i}+0.75\hat{j}+0.66\hat{k}$,\newline
$\vec{r}_{15}=0.0\hat{i}+0.0\hat{j}+10.0\hat{k}$,\;\;\;$\vec{r}_{23}=0.0\hat{i}+10.0\hat{j}+0.48\hat{k}$,\;\;\;$\vec{r}_{25}=10.0\hat{i}+0.0\hat{j}+0.0\hat{k}$,\;\;\;$\vec{r}_{34}=10.0\hat{i}+10.0\hat{j}+0.0\hat{k}$.

{\tiny 2D-M172:}

$\hat{n}_{14}=0.58\hat{i}+0.58\hat{j}+0.58\hat{k}$,\;\;\;$\hat{n}_{15}=0.0\hat{i}+0.39\hat{j}+0.92\hat{k}$,\;\;\;$\hat{n}_{23}=0.0\hat{i}+0.77\hat{j}-0.63\hat{k}$,\;\;\;$\hat{n}_{34}=-0.8\hat{i}+0.28\hat{j}+0.52\hat{k}$,\newline
$\vec{r}_{15}=0.0\hat{i}+10.0\hat{j}+10.0\hat{k}$,\;\;\;$\vec{r}_{23}=0.0\hat{i}+0.0\hat{j}+0.0\hat{k}$,\;\;\;$\vec{r}_{25}=10.0\hat{i}+10.0\hat{j}+10.0\hat{k}$,\;\;\;$\vec{r}_{34}=0.0\hat{i}+0.0\hat{j}+0.0\hat{k}$.

{\tiny 2D-M173:}

$\hat{n}_{14}=0.48\hat{i}+0.68\hat{j}-0.55\hat{k}$,\;\;\;$\hat{n}_{15}=0.02\hat{i}+0.84\hat{j}-0.55\hat{k}$,\;\;\;$\hat{n}_{25}=0.61\hat{i}-0.78\hat{j}-0.17\hat{k}$,\;\;\;$\hat{n}_{34}=0.0\hat{i}+0.35\hat{j}-0.94\hat{k}$,\newline
$\vec{r}_{15}=0.0\hat{i}+10.0\hat{j}+0.0\hat{k}$,\;\;\;$\vec{r}_{23}=0.0\hat{i}+0.0\hat{j}+10.0\hat{k}$,\;\;\;$\vec{r}_{25}=10.0\hat{i}+10.0\hat{j}+0.0\hat{k}$,\;\;\;$\vec{r}_{34}=10.0\hat{i}+10.0\hat{j}+10.0\hat{k}$.

{\tiny 2D-M174:}

$\hat{n}_{14}=0.52\hat{i}-0.77\hat{j}+0.38\hat{k}$,\;\;\;$\hat{n}_{23}=0.4\hat{i}-0.7\hat{j}+0.59\hat{k}$,\;\;\;$\hat{n}_{25}=0.7\hat{i}-0.62\hat{j}-0.34\hat{k}$,\;\;\;$\hat{n}_{34}=0.81\hat{i}+0.29\hat{j}-0.51\hat{k}$,\newline
$\vec{r}_{15}=10.0\hat{i}+10.0\hat{j}+10.0\hat{k}$,\;\;\;$\vec{r}_{23}=10.0\hat{i}+10.0\hat{j}+0.0\hat{k}$,\;\;\;$\vec{r}_{25}=0.0\hat{i}+0.0\hat{j}+10.0\hat{k}$,\;\;\;$\vec{r}_{34}=10.0\hat{i}+0.0\hat{j}+0.0\hat{k}$.

{\tiny 2D-M175:}

$\hat{n}_{14}=-0.99\hat{i}+0.16\hat{j}+0.04\hat{k}$,\;\;\;$\hat{n}_{23}=0.8\hat{i}-0.15\hat{j}-0.58\hat{k}$,\;\;\;$\hat{n}_{25}=-0.12\hat{i}-0.53\hat{j}-0.84\hat{k}$,\;\;\;$\hat{n}_{34}=-0.83\hat{i}-0.55\hat{j}-0.09\hat{k}$,\newline
$\vec{r}_{15}=10.0\hat{i}+0.0\hat{j}+0.0\hat{k}$,\;\;\;$\vec{r}_{23}=0.0\hat{i}+0.0\hat{j}+0.0\hat{k}$,\;\;\;$\vec{r}_{25}=0.0\hat{i}+10.0\hat{j}+10.0\hat{k}$,\;\;\;$\vec{r}_{34}=10.0\hat{i}+0.0\hat{j}+10.0\hat{k}$.

{\tiny 2D-M176:}

$\hat{n}_{14}=0.0\hat{i}-0.0\hat{j}+1.0\hat{k}$,\;\;\;$\hat{n}_{23}=-0.95\hat{i}+0.17\hat{j}+0.25\hat{k}$,\;\;\;$\hat{n}_{25}=-0.0\hat{i}+0.22\hat{j}+0.97\hat{k}$,\;\;\;$\hat{n}_{34}=-0.02\hat{i}-0.78\hat{j}+0.63\hat{k}$,\newline
$\vec{r}_{15}=0.0\hat{i}+10.0\hat{j}+0.0\hat{k}$,\;\;\;$\vec{r}_{23}=10.0\hat{i}+10.0\hat{j}+10.0\hat{k}$,\;\;\;$\vec{r}_{25}=0.0\hat{i}+10.0\hat{j}+10.0\hat{k}$,\;\;\;$\vec{r}_{34}=10.0\hat{i}+0.0\hat{j}+10.0\hat{k}$.

{\tiny 2D-M177:}

$\hat{n}_{14}=0.68\hat{i}+0.71\hat{j}-0.19\hat{k}$,\;\;\;$\hat{n}_{23}=-0.0\hat{i}+0.51\hat{j}-0.86\hat{k}$,\;\;\;$\hat{n}_{25}=0.0\hat{i}+0.26\hat{j}-0.97\hat{k}$,\;\;\;$\hat{n}_{34}=0.0\hat{i}+0.0\hat{j}-1.0\hat{k}$,\newline
$\vec{r}_{14}=0.0\hat{i}+0.0\hat{j}+0.0\hat{k}$,\;\;\;$\vec{r}_{15}=10.0\hat{i}+0.0\hat{j}+10.0\hat{k}$,\;\;\;$\vec{r}_{23}=10.0\hat{i}+10.0\hat{j}+10.0\hat{k}$,\;\;\;$\vec{r}_{25}=0.0\hat{i}+0.0\hat{j}+0.0\hat{k}$.

{\tiny 2D-M178:}

$\hat{n}_{14}=-0.0\hat{i}+0.71\hat{j}-0.71\hat{k}$,\;\;\;$\hat{n}_{23}=-0.0\hat{i}+0.0\hat{j}+1.0\hat{k}$,\;\;\;$\hat{n}_{25}=0.58\hat{i}-0.58\hat{j}-0.58\hat{k}$,\;\;\;$\hat{n}_{34}=-0.87\hat{i}-0.5\hat{j}+0.0\hat{k}$,\newline
$\vec{r}_{14}=0.0\hat{i}+10.0\hat{j}+0.0\hat{k}$,\;\;\;$\vec{r}_{15}=10.0\hat{i}+0.0\hat{j}+10.0\hat{k}$,\;\;\;$\vec{r}_{23}=10.0\hat{i}+0.0\hat{j}+0.58\hat{k}$,\;\;\;$\vec{r}_{34}=10.0\hat{i}+0.0\hat{j}+10.0\hat{k}$.

{\tiny 2D-M179:}

$\hat{n}_{14}=-0.9\hat{i}-0.44\hat{j}+0.04\hat{k}$,\;\;\;$\hat{n}_{23}=0.0\hat{i}+0.76\hat{j}+0.65\hat{k}$,\;\;\;$\hat{n}_{25}=-0.0\hat{i}+0.0\hat{j}+1.0\hat{k}$,\;\;\;$\hat{n}_{34}=0.34\hat{i}+0.93\hat{j}-0.14\hat{k}$,\newline
$\vec{r}_{14}=10.0\hat{i}+0.0\hat{j}+10.0\hat{k}$,\;\;\;$\vec{r}_{15}=0.0\hat{i}+10.0\hat{j}+0.0\hat{k}$,\;\;\;$\vec{r}_{25}=10.0\hat{i}+10.0\hat{j}+0.02\hat{k}$,\;\;\;$\vec{r}_{34}=0.0\hat{i}+10.0\hat{j}+0.0\hat{k}$.

{\tiny 2D-M180:}

$\hat{n}_{15}=0.92\hat{i}-0.1\hat{j}+0.38\hat{k}$,\;\;\;$\hat{n}_{23}=0.82\hat{i}-0.39\hat{j}+0.42\hat{k}$,\;\;\;$\hat{n}_{25}=0.0\hat{i}+0.71\hat{j}+0.71\hat{k}$,\;\;\;$\hat{n}_{34}=-0.0\hat{i}+0.68\hat{j}-0.74\hat{k}$,\newline
$\vec{r}_{14}=10.0\hat{i}+10.0\hat{j}+0.0\hat{k}$,\;\;\;$\vec{r}_{15}=0.0\hat{i}+0.0\hat{j}+10.0\hat{k}$,\;\;\;$\vec{r}_{23}=0.0\hat{i}+0.0\hat{j}+10.0\hat{k}$,\;\;\;$\vec{r}_{25}=0.0\hat{i}+10.0\hat{j}+10.0\hat{k}$.

{\tiny 2D-M181:}

$\hat{n}_{15}=-0.71\hat{i}-0.23\hat{j}-0.67\hat{k}$,\;\;\;$\hat{n}_{23}=-0.69\hat{i}+0.02\hat{j}-0.72\hat{k}$,\;\;\;$\hat{n}_{25}=0.68\hat{i}-0.21\hat{j}-0.7\hat{k}$,\;\;\;$\hat{n}_{34}=0.43\hat{i}+0.82\hat{j}-0.39\hat{k}$,\newline
$\vec{r}_{14}=0.0\hat{i}+10.0\hat{j}+0.0\hat{k}$,\;\;\;$\vec{r}_{15}=0.0\hat{i}+0.0\hat{j}+10.0\hat{k}$,\;\;\;$\vec{r}_{23}=10.0\hat{i}+0.0\hat{j}+10.0\hat{k}$,\;\;\;$\vec{r}_{34}=10.0\hat{i}+0.0\hat{j}+10.0\hat{k}$.

{\tiny 2D-M182:}

$\hat{n}_{15}=-0.62\hat{i}-0.69\hat{j}-0.38\hat{k}$,\;\;\;$\hat{n}_{23}=-0.71\hat{i}+0.67\hat{j}-0.22\hat{k}$,\;\;\;$\hat{n}_{25}=0.78\hat{i}+0.17\hat{j}-0.61\hat{k}$,\;\;\;$\hat{n}_{34}=-0.25\hat{i}-0.8\hat{j}-0.55\hat{k}$,\newline
$\vec{r}_{14}=10.0\hat{i}+0.0\hat{j}+0.0\hat{k}$,\;\;\;$\vec{r}_{15}=0.0\hat{i}+10.0\hat{j}+0.0\hat{k}$,\;\;\;$\vec{r}_{25}=0.0\hat{i}+10.0\hat{j}+10.0\hat{k}$,\;\;\;$\vec{r}_{34}=0.0\hat{i}+10.0\hat{j}+10.0\hat{k}$.

{\tiny 2D-M183:}

$\hat{n}_{13}=-0.61\hat{i}-0.5\hat{j}+0.61\hat{k}$,\;\;\;$\hat{n}_{14}=-0.64\hat{i}+0.77\hat{j}+0.05\hat{k}$,\;\;\;$\hat{n}_{24}=-0.58\hat{i}-0.58\hat{j}-0.57\hat{k}$,\;\;\;$\hat{n}_{25}=0.72\hat{i}-0.69\hat{j}-0.03\hat{k}$,\newline
$\vec{r}_{13}=0.0\hat{i}+10.0\hat{j}+10.0\hat{k}$,\;\;\;$\vec{r}_{14}=0.0\hat{i}+0.0\hat{j}+0.0\hat{k}$,\;\;\;$\vec{r}_{25}=10.0\hat{i}+10.0\hat{j}+10.0\hat{k}$,\;\;\;$\vec{r}_{35}=0.0\hat{i}+0.0\hat{j}+0.0\hat{k}$.

{\tiny 2D-M184:}

$\hat{n}_{13}=-0.88\hat{i}-0.06\hat{j}+0.48\hat{k}$,\;\;\;$\hat{n}_{14}=0.48\hat{i}+0.33\hat{j}-0.81\hat{k}$,\;\;\;$\hat{n}_{24}=-0.55\hat{i}-0.59\hat{j}-0.59\hat{k}$,\;\;\;$\hat{n}_{35}=-0.64\hat{i}+0.75\hat{j}-0.19\hat{k}$,\newline
$\vec{r}_{13}=10.0\hat{i}+0.0\hat{j}+0.0\hat{k}$,\;\;\;$\vec{r}_{14}=0.0\hat{i}+0.0\hat{j}+0.0\hat{k}$,\;\;\;$\vec{r}_{25}=10.0\hat{i}+10.0\hat{j}+10.0\hat{k}$,\;\;\;$\vec{r}_{35}=0.0\hat{i}+0.0\hat{j}+0.0\hat{k}$.

{\tiny 2D-M185:}

$\hat{n}_{13}=-0.62\hat{i}+0.62\hat{j}-0.49\hat{k}$,\;\;\;$\hat{n}_{14}=0.66\hat{i}-0.03\hat{j}-0.75\hat{k}$,\;\;\;$\hat{n}_{24}=0.72\hat{i}-0.03\hat{j}-0.69\hat{k}$,\;\;\;$\hat{n}_{25}=-0.58\hat{i}-0.57\hat{j}-0.58\hat{k}$,\newline
$\vec{r}_{13}=0.0\hat{i}+0.0\hat{j}+10.0\hat{k}$,\;\;\;$\vec{r}_{14}=10.0\hat{i}+10.0\hat{j}+10.0\hat{k}$,\;\;\;$\vec{r}_{24}=0.0\hat{i}+0.0\hat{j}+0.0\hat{k}$,\;\;\;$\vec{r}_{35}=10.0\hat{i}+10.0\hat{j}+10.0\hat{k}$.

{\tiny 2D-M186:}

$\hat{n}_{13}=-0.26\hat{i}+0.46\hat{j}-0.85\hat{k}$,\;\;\;$\hat{n}_{14}=-0.66\hat{i}-0.53\hat{j}+0.53\hat{k}$,\;\;\;$\hat{n}_{24}=0.27\hat{i}+0.88\hat{j}-0.39\hat{k}$,\;\;\;$\hat{n}_{35}=-0.0\hat{i}-0.0\hat{j}+1.0\hat{k}$,\newline
$\vec{r}_{13}=10.0\hat{i}+0.0\hat{j}+10.0\hat{k}$,\;\;\;$\vec{r}_{14}=10.0\hat{i}+0.0\hat{j}+10.0\hat{k}$,\;\;\;$\vec{r}_{24}=10.0\hat{i}+10.0\hat{j}+10.0\hat{k}$,\;\;\;$\vec{r}_{25}=0.0\hat{i}+0.0\hat{j}+0.0\hat{k}$.

{\tiny 2D-M187:}

$\hat{n}_{13}=0.72\hat{i}-0.48\hat{j}+0.5\hat{k}$,\;\;\;$\hat{n}_{14}=0.8\hat{i}-0.25\hat{j}-0.55\hat{k}$,\;\;\;$\hat{n}_{25}=0.14\hat{i}+0.67\hat{j}+0.73\hat{k}$,\;\;\;$\hat{n}_{35}=-0.07\hat{i}+0.73\hat{j}-0.68\hat{k}$,\newline
$\vec{r}_{13}=10.0\hat{i}+10.0\hat{j}+0.0\hat{k}$,\;\;\;$\vec{r}_{14}=10.0\hat{i}+10.0\hat{j}+10.0\hat{k}$,\;\;\;$\vec{r}_{24}=0.0\hat{i}+0.0\hat{j}+0.0\hat{k}$,\;\;\;$\vec{r}_{35}=10.0\hat{i}+0.0\hat{j}+10.0\hat{k}$.

{\tiny 2D-M188:}

$\hat{n}_{13}=0.0\hat{i}+0.5\hat{j}-0.86\hat{k}$,\;\;\;$\hat{n}_{14}=-0.67\hat{i}+0.67\hat{j}+0.34\hat{k}$,\;\;\;$\hat{n}_{25}=0.9\hat{i}+0.11\hat{j}-0.41\hat{k}$,\;\;\;$\hat{n}_{35}=0.0\hat{i}+0.0\hat{j}+1.0\hat{k}$,\newline
$\vec{r}_{13}=10.0\hat{i}+0.0\hat{j}+10.0\hat{k}$,\;\;\;$\vec{r}_{14}=10.0\hat{i}+10.0\hat{j}+0.0\hat{k}$,\;\;\;$\vec{r}_{24}=0.0\hat{i}+0.0\hat{j}+0.0\hat{k}$,\;\;\;$\vec{r}_{25}=0.0\hat{i}+10.0\hat{j}+10.0\hat{k}$.

{\tiny 2D-M189:}

$\hat{n}_{13}=0.65\hat{i}-0.65\hat{j}-0.38\hat{k}$,\;\;\;$\hat{n}_{14}=-0.71\hat{i}+0.61\hat{j}+0.35\hat{k}$,\;\;\;$\hat{n}_{23}=-0.0\hat{i}+0.87\hat{j}+0.5\hat{k}$,\;\;\;$\hat{n}_{45}=-0.0\hat{i}+0.84\hat{j}+0.55\hat{k}$,\newline
$\vec{r}_{13}=10.0\hat{i}+10.0\hat{j}+10.0\hat{k}$,\;\;\;$\vec{r}_{14}=10.0\hat{i}+10.0\hat{j}+10.0\hat{k}$,\;\;\;$\vec{r}_{23}=10.0\hat{i}+0.0\hat{j}+0.0\hat{k}$,\;\;\;$\vec{r}_{24}=0.0\hat{i}+0.0\hat{j}+10.0\hat{k}$.

{\tiny 2D-M190:}

$\hat{n}_{13}=0.02\hat{i}-0.58\hat{j}-0.82\hat{k}$,\;\;\;$\hat{n}_{14}=-0.84\hat{i}-0.33\hat{j}+0.44\hat{k}$,\;\;\;$\hat{n}_{23}=-0.13\hat{i}-0.9\hat{j}+0.42\hat{k}$,\;\;\;$\hat{n}_{35}=-0.36\hat{i}+0.37\hat{j}-0.86\hat{k}$,\newline
$\vec{r}_{13}=10.0\hat{i}+0.0\hat{j}+0.0\hat{k}$,\;\;\;$\vec{r}_{14}=2.49\hat{i}+4.03\hat{j}+6.6\hat{k}$,\;\;\;$\vec{r}_{23}=2.43\hat{i}+3.38\hat{j}+6.05\hat{k}$,\;\;\;$\vec{r}_{24}=3.44\hat{i}+3.7\hat{j}+2.4\hat{k}$.

{\tiny 2D-M191:}

$\hat{n}_{13}=0.0\hat{i}+0.0\hat{j}+1.0\hat{k}$,\;\;\;$\hat{n}_{14}=-0.0\hat{i}+0.67\hat{j}-0.74\hat{k}$,\;\;\;$\hat{n}_{23}=-0.88\hat{i}-0.3\hat{j}-0.36\hat{k}$,\;\;\;$\hat{n}_{25}=0.0\hat{i}+0.0\hat{j}-1.0\hat{k}$,\newline
$\vec{r}_{13}=10.0\hat{i}+10.0\hat{j}+10.0\hat{k}$,\;\;\;$\vec{r}_{14}=10.0\hat{i}+10.0\hat{j}+10.0\hat{k}$,\;\;\;$\vec{r}_{23}=10.0\hat{i}+0.0\hat{j}+10.0\hat{k}$,\;\;\;$\vec{r}_{24}=0.0\hat{i}+0.0\hat{j}+0.0\hat{k}$.

{\tiny 2D-M192:}

$\hat{n}_{13}=0.04\hat{i}+0.71\hat{j}+0.71\hat{k}$,\;\;\;$\hat{n}_{14}=0.0\hat{i}+0.48\hat{j}+0.88\hat{k}$,\;\;\;$\hat{n}_{24}=0.7\hat{i}+0.23\hat{j}-0.67\hat{k}$,\;\;\;$\hat{n}_{25}=0.89\hat{i}+0.46\hat{j}+0.03\hat{k}$,\newline
$\vec{r}_{13}=0.0\hat{i}+0.0\hat{j}+10.0\hat{k}$,\;\;\;$\vec{r}_{24}=10.0\hat{i}+10.0\hat{j}+10.0\hat{k}$,\;\;\;$\vec{r}_{25}=0.0\hat{i}+10.0\hat{j}+0.0\hat{k}$,\;\;\;$\vec{r}_{35}=10.0\hat{i}+0.0\hat{j}+0.0\hat{k}$.

{\tiny 2D-M193:}

$\hat{n}_{13}=-0.0\hat{i}+0.51\hat{j}+0.86\hat{k}$,\;\;\;$\hat{n}_{14}=-0.0\hat{i}-0.0\hat{j}+1.0\hat{k}$,\;\;\;$\hat{n}_{24}=-0.62\hat{i}-0.48\hat{j}+0.62\hat{k}$,\;\;\;$\hat{n}_{35}=0.0\hat{i}+0.0\hat{j}+1.0\hat{k}$,\newline
$\vec{r}_{13}=0.0\hat{i}+0.0\hat{j}+10.0\hat{k}$,\;\;\;$\vec{r}_{24}=10.0\hat{i}+10.0\hat{j}+10.0\hat{k}$,\;\;\;$\vec{r}_{25}=10.0\hat{i}+0.0\hat{j}+0.0\hat{k}$,\;\;\;$\vec{r}_{35}=0.0\hat{i}+10.0\hat{j}+0.0\hat{k}$.

{\tiny 2D-M194:}

$\hat{n}_{13}=-0.68\hat{i}-0.73\hat{j}+0.06\hat{k}$,\;\;\;$\hat{n}_{14}=-0.46\hat{i}-0.83\hat{j}+0.31\hat{k}$,\;\;\;$\hat{n}_{24}=0.49\hat{i}+0.05\hat{j}+0.87\hat{k}$,\;\;\;$\hat{n}_{25}=-0.33\hat{i}+0.62\hat{j}-0.71\hat{k}$,\newline
$\vec{r}_{13}=0.0\hat{i}+10.0\hat{j}+0.0\hat{k}$,\;\;\;$\vec{r}_{24}=10.0\hat{i}+10.0\hat{j}+0.0\hat{k}$,\;\;\;$\vec{r}_{25}=0.0\hat{i}+0.0\hat{j}+0.0\hat{k}$,\;\;\;$\vec{r}_{35}=10.0\hat{i}+0.0\hat{j}+10.0\hat{k}$.

{\tiny 2D-M195:}

$\hat{n}_{13}=0.0\hat{i}+0.53\hat{j}+0.85\hat{k}$,\;\;\;$\hat{n}_{14}=-0.76\hat{i}+0.63\hat{j}-0.19\hat{k}$,\;\;\;$\hat{n}_{24}=-0.15\hat{i}-0.45\hat{j}-0.88\hat{k}$,\;\;\;$\hat{n}_{35}=0.64\hat{i}+0.46\hat{j}-0.61\hat{k}$,\newline
$\vec{r}_{13}=10.0\hat{i}+0.0\hat{j}+0.0\hat{k}$,\;\;\;$\vec{r}_{24}=0.0\hat{i}+10.0\hat{j}+10.0\hat{k}$,\;\;\;$\vec{r}_{25}=10.0\hat{i}+0.0\hat{j}+10.0\hat{k}$,\;\;\;$\vec{r}_{35}=0.0\hat{i}+0.0\hat{j}+0.0\hat{k}$.

{\tiny 2D-M196:}

$\hat{n}_{13}=-0.38\hat{i}-0.4\hat{j}-0.83\hat{k}$,\;\;\;$\hat{n}_{14}=0.72\hat{i}+0.0\hat{j}+0.69\hat{k}$,\;\;\;$\hat{n}_{25}=-0.7\hat{i}-0.08\hat{j}+0.7\hat{k}$,\;\;\;$\hat{n}_{35}=0.56\hat{i}+0.54\hat{j}+0.63\hat{k}$,\newline
$\vec{r}_{13}=10.0\hat{i}+10.0\hat{j}+0.0\hat{k}$,\;\;\;$\vec{r}_{24}=10.0\hat{i}+0.0\hat{j}+0.0\hat{k}$,\;\;\;$\vec{r}_{25}=10.0\hat{i}+10.0\hat{j}+10.0\hat{k}$,\;\;\;$\vec{r}_{35}=0.0\hat{i}+10.0\hat{j}+10.0\hat{k}$.

{\tiny 2D-M197:}

$\hat{n}_{13}=-0.17\hat{i}+0.74\hat{j}+0.65\hat{k}$,\;\;\;$\hat{n}_{14}=0.79\hat{i}-0.59\hat{j}-0.16\hat{k}$,\;\;\;$\hat{n}_{25}=0.31\hat{i}+0.6\hat{j}-0.74\hat{k}$,\;\;\;$\hat{n}_{35}=-0.53\hat{i}-0.57\hat{j}-0.63\hat{k}$,\newline
$\vec{r}_{13}=0.0\hat{i}+10.0\hat{j}+10.0\hat{k}$,\;\;\;$\vec{r}_{24}=10.0\hat{i}+0.0\hat{j}+0.0\hat{k}$,\;\;\;$\vec{r}_{25}=0.0\hat{i}+10.0\hat{j}+0.0\hat{k}$,\;\;\;$\vec{r}_{35}=0.0\hat{i}+0.0\hat{j}+10.0\hat{k}$.

{\tiny 2D-M198:}

$\hat{n}_{13}=-0.78\hat{i}+0.61\hat{j}-0.08\hat{k}$,\;\;\;$\hat{n}_{14}=-0.68\hat{i}-0.51\hat{j}+0.52\hat{k}$,\;\;\;$\hat{n}_{23}=0.02\hat{i}+0.69\hat{j}+0.72\hat{k}$,\;\;\;$\hat{n}_{25}=-0.9\hat{i}-0.27\hat{j}+0.33\hat{k}$,\newline
$\vec{r}_{13}=10.0\hat{i}+10.0\hat{j}+0.0\hat{k}$,\;\;\;$\vec{r}_{23}=0.0\hat{i}+0.0\hat{j}+10.0\hat{k}$,\;\;\;$\vec{r}_{25}=0.0\hat{i}+10.0\hat{j}+10.0\hat{k}$,\;\;\;$\vec{r}_{45}=10.0\hat{i}+10.0\hat{j}+0.0\hat{k}$.

{\tiny 2D-M199:}

$\hat{n}_{13}=-1.0\hat{i}+0.02\hat{j}-0.02\hat{k}$,\;\;\;$\hat{n}_{14}=-0.0\hat{i}+0.0\hat{j}+1.0\hat{k}$,\;\;\;$\hat{n}_{23}=0.0\hat{i}+0.46\hat{j}-0.89\hat{k}$,\;\;\;$\hat{n}_{45}=0.09\hat{i}+0.72\hat{j}+0.69\hat{k}$,\newline
$\vec{r}_{13}=0.0\hat{i}+0.0\hat{j}+0.0\hat{k}$,\;\;\;$\vec{r}_{23}=0.0\hat{i}+10.0\hat{j}+0.0\hat{k}$,\;\;\;$\vec{r}_{25}=10.0\hat{i}+0.0\hat{j}+10.0\hat{k}$,\;\;\;$\vec{r}_{45}=10.0\hat{i}+10.0\hat{j}+0.0\hat{k}$.

{\tiny 2D-M200:}

$\hat{n}_{13}=0.66\hat{i}-0.03\hat{j}+0.75\hat{k}$,\;\;\;$\hat{n}_{14}=0.0\hat{i}+0.0\hat{j}+1.0\hat{k}$,\;\;\;$\hat{n}_{23}=0.51\hat{i}-0.45\hat{j}+0.73\hat{k}$,\;\;\;$\hat{n}_{25}=0.0\hat{i}+0.72\hat{j}+0.7\hat{k}$,\newline
$\vec{r}_{13}=10.0\hat{i}+10.0\hat{j}+0.0\hat{k}$,\;\;\;$\vec{r}_{23}=0.0\hat{i}+0.0\hat{j}+10.0\hat{k}$,\;\;\;$\vec{r}_{25}=0.0\hat{i}+10.0\hat{j}+10.0\hat{k}$,\;\;\;$\vec{r}_{45}=10.0\hat{i}+10.0\hat{j}+0.0\hat{k}$.

{\tiny 2D-M201:}

$\hat{n}_{13}=-0.45\hat{i}+0.37\hat{j}-0.82\hat{k}$,\;\;\;$\hat{n}_{14}=0.0\hat{i}+0.0\hat{j}+1.0\hat{k}$,\;\;\;$\hat{n}_{23}=0.06\hat{i}+0.57\hat{j}+0.82\hat{k}$,\;\;\;$\hat{n}_{45}=0.0\hat{i}+0.44\hat{j}-0.9\hat{k}$,\newline
$\vec{r}_{13}=10.0\hat{i}+0.0\hat{j}+10.0\hat{k}$,\;\;\;$\vec{r}_{23}=0.0\hat{i}+0.0\hat{j}+10.0\hat{k}$,\;\;\;$\vec{r}_{25}=0.0\hat{i}+10.0\hat{j}+0.0\hat{k}$,\;\;\;$\vec{r}_{45}=10.0\hat{i}+0.0\hat{j}+10.0\hat{k}$.

{\tiny 2D-M202:}

$\hat{n}_{13}=0.58\hat{i}-0.58\hat{j}-0.58\hat{k}$,\;\;\;$\hat{n}_{14}=-0.65\hat{i}+0.11\hat{j}-0.76\hat{k}$,\;\;\;$\hat{n}_{23}=-0.5\hat{i}-0.81\hat{j}+0.31\hat{k}$,\;\;\;$\hat{n}_{45}=0.13\hat{i}-0.77\hat{j}-0.62\hat{k}$,\newline
$\vec{r}_{13}=10.0\hat{i}+10.0\hat{j}+0.0\hat{k}$,\;\;\;$\vec{r}_{23}=0.0\hat{i}+10.0\hat{j}+10.0\hat{k}$,\;\;\;$\vec{r}_{24}=0.0\hat{i}+0.0\hat{j}+0.0\hat{k}$,\;\;\;$\vec{r}_{45}=0.0\hat{i}+10.0\hat{j}+10.0\hat{k}$.

{\tiny 2D-M203:}

$\hat{n}_{13}=-0.0\hat{i}+0.86\hat{j}+0.51\hat{k}$,\;\;\;$\hat{n}_{14}=-0.89\hat{i}-0.4\hat{j}-0.2\hat{k}$,\;\;\;$\hat{n}_{23}=-0.51\hat{i}-0.77\hat{j}-0.37\hat{k}$,\;\;\;$\hat{n}_{35}=0.83\hat{i}+0.55\hat{j}+0.11\hat{k}$,\newline
$\vec{r}_{13}=0.0\hat{i}+0.0\hat{j}+10.0\hat{k}$,\;\;\;$\vec{r}_{23}=5.28\hat{i}+4.6\hat{j}+5.29\hat{k}$,\;\;\;$\vec{r}_{24}=5.29\hat{i}+5.38\hat{j}+4.64\hat{k}$,\;\;\;$\vec{r}_{35}=10.0\hat{i}+0.0\hat{j}+0.0\hat{k}$.

{\tiny 2D-M204:}

$\hat{n}_{13}=-0.0\hat{i}+0.0\hat{j}-1.0\hat{k}$,\;\;\;$\hat{n}_{14}=-0.68\hat{i}+0.43\hat{j}-0.59\hat{k}$,\;\;\;$\hat{n}_{23}=0.58\hat{i}+0.78\hat{j}+0.22\hat{k}$,\;\;\;$\hat{n}_{25}=0.66\hat{i}-0.02\hat{j}+0.75\hat{k}$,\newline
$\vec{r}_{13}=0.0\hat{i}+0.0\hat{j}+6.32\hat{k}$,\;\;\;$\vec{r}_{23}=10.0\hat{i}+0.0\hat{j}+0.0\hat{k}$,\;\;\;$\vec{r}_{24}=0.0\hat{i}+10.0\hat{j}+10.0\hat{k}$,\;\;\;$\vec{r}_{25}=10.0\hat{i}+10.0\hat{j}+0.0\hat{k}$.

{\tiny 2D-M205:}

$\hat{n}_{13}=-0.0\hat{i}+0.81\hat{j}-0.59\hat{k}$,\;\;\;$\hat{n}_{14}=-0.51\hat{i}-0.48\hat{j}+0.71\hat{k}$,\;\;\;$\hat{n}_{25}=-0.76\hat{i}-0.0\hat{j}-0.65\hat{k}$,\;\;\;$\hat{n}_{45}=0.72\hat{i}+0.22\hat{j}+0.66\hat{k}$,\newline
$\vec{r}_{13}=0.0\hat{i}+10.0\hat{j}+0.0\hat{k}$,\;\;\;$\vec{r}_{23}=10.0\hat{i}+0.0\hat{j}+10.0\hat{k}$,\;\;\;$\vec{r}_{25}=0.0\hat{i}+0.0\hat{j}+10.0\hat{k}$,\;\;\;$\vec{r}_{45}=10.0\hat{i}+10.0\hat{j}+0.0\hat{k}$.

{\tiny 2D-M206:}

$\hat{n}_{13}=-0.0\hat{i}+0.41\hat{j}+0.91\hat{k}$,\;\;\;$\hat{n}_{14}=-0.14\hat{i}+0.59\hat{j}+0.79\hat{k}$,\;\;\;$\hat{n}_{25}=0.0\hat{i}+0.81\hat{j}+0.58\hat{k}$,\;\;\;$\hat{n}_{45}=-0.6\hat{i}+0.18\hat{j}-0.77\hat{k}$,\newline
$\vec{r}_{13}=10.0\hat{i}+0.0\hat{j}+0.0\hat{k}$,\;\;\;$\vec{r}_{23}=0.0\hat{i}+10.0\hat{j}+0.0\hat{k}$,\;\;\;$\vec{r}_{25}=0.0\hat{i}+0.0\hat{j}+10.0\hat{k}$,\;\;\;$\vec{r}_{45}=10.0\hat{i}+0.0\hat{j}+10.0\hat{k}$.

{\tiny 2D-M207:}

$\hat{n}_{13}=-0.58\hat{i}+0.58\hat{j}-0.58\hat{k}$,\;\;\;$\hat{n}_{14}=0.11\hat{i}-0.65\hat{j}-0.76\hat{k}$,\;\;\;$\hat{n}_{24}=0.81\hat{i}+0.5\hat{j}-0.31\hat{k}$,\;\;\;$\hat{n}_{45}=-0.06\hat{i}+0.56\hat{j}+0.83\hat{k}$,\newline
$\vec{r}_{13}=10.0\hat{i}+10.0\hat{j}+0.0\hat{k}$,\;\;\;$\vec{r}_{23}=0.0\hat{i}+0.0\hat{j}+0.0\hat{k}$,\;\;\;$\vec{r}_{24}=10.0\hat{i}+0.0\hat{j}+10.0\hat{k}$,\;\;\;$\vec{r}_{45}=10.0\hat{i}+0.0\hat{j}+0.0\hat{k}$.

{\tiny 2D-M208:}

$\hat{n}_{13}=0.36\hat{i}+0.64\hat{j}+0.68\hat{k}$,\;\;\;$\hat{n}_{14}=-0.01\hat{i}-0.52\hat{j}+0.85\hat{k}$,\;\;\;$\hat{n}_{24}=0.52\hat{i}+0.04\hat{j}+0.85\hat{k}$,\;\;\;$\hat{n}_{35}=0.81\hat{i}+0.05\hat{j}-0.58\hat{k}$,\newline
$\vec{r}_{13}=0.0\hat{i}+0.0\hat{j}+10.0\hat{k}$,\;\;\;$\vec{r}_{23}=5.3\hat{i}+4.88\hat{j}+5.01\hat{k}$,\;\;\;$\vec{r}_{24}=3.68\hat{i}+4.58\hat{j}+4.75\hat{k}$,\;\;\;$\vec{r}_{35}=10.0\hat{i}+0.0\hat{j}+0.0\hat{k}$.

{\tiny 2D-M209:}

$\hat{n}_{13}=-0.7\hat{i}-0.01\hat{j}-0.71\hat{k}$,\;\;\;$\hat{n}_{14}=0.58\hat{i}+0.58\hat{j}-0.58\hat{k}$,\;\;\;$\hat{n}_{24}=0.42\hat{i}-0.82\hat{j}-0.4\hat{k}$,\;\;\;$\hat{n}_{25}=0.01\hat{i}-0.58\hat{j}+0.82\hat{k}$,\newline
$\vec{r}_{13}=0.0\hat{i}+0.0\hat{j}+10.0\hat{k}$,\;\;\;$\vec{r}_{23}=10.0\hat{i}+10.0\hat{j}+0.0\hat{k}$,\;\;\;$\vec{r}_{24}=0.0\hat{i}+0.0\hat{j}+10.0\hat{k}$,\;\;\;$\vec{r}_{25}=10.0\hat{i}+0.0\hat{j}+10.0\hat{k}$.

{\tiny 2D-M210:}

$\hat{n}_{13}=-0.7\hat{i}-0.7\hat{j}-0.15\hat{k}$,\;\;\;$\hat{n}_{14}=0.46\hat{i}-0.36\hat{j}-0.81\hat{k}$,\;\;\;$\hat{n}_{24}=0.35\hat{i}-0.4\hat{j}-0.85\hat{k}$,\;\;\;$\hat{n}_{25}=0.58\hat{i}-0.57\hat{j}+0.58\hat{k}$,\newline
$\vec{r}_{13}=0.0\hat{i}+10.0\hat{j}+0.0\hat{k}$,\;\;\;$\vec{r}_{14}=0.0\hat{i}+10.0\hat{j}+10.0\hat{k}$,\;\;\;$\vec{r}_{24}=10.0\hat{i}+0.0\hat{j}+0.0\hat{k}$,\;\;\;$\vec{r}_{35}=10.0\hat{i}+0.0\hat{j}+0.0\hat{k}$.

{\tiny 2D-M211:}

$\hat{n}_{13}=-0.0\hat{i}+0.59\hat{j}+0.81\hat{k}$,\;\;\;$\hat{n}_{14}=0.62\hat{i}+0.35\hat{j}+0.7\hat{k}$,\;\;\;$\hat{n}_{24}=-0.0\hat{i}+0.0\hat{j}-1.0\hat{k}$,\;\;\;$\hat{n}_{35}=-0.04\hat{i}+0.83\hat{j}-0.56\hat{k}$,\newline
$\vec{r}_{13}=10.0\hat{i}+0.0\hat{j}+0.0\hat{k}$,\;\;\;$\vec{r}_{14}=10.0\hat{i}+10.0\hat{j}+0.0\hat{k}$,\;\;\;$\vec{r}_{24}=10.0\hat{i}+0.0\hat{j}+8.83\hat{k}$,\;\;\;$\vec{r}_{25}=0.0\hat{i}+10.0\hat{j}+10.0\hat{k}$.

{\tiny 2D-M212:}

$\hat{n}_{13}=0.47\hat{i}+0.0\hat{j}+0.88\hat{k}$,\;\;\;$\hat{n}_{14}=-0.94\hat{i}-0.04\hat{j}-0.35\hat{k}$,\;\;\;$\hat{n}_{24}=-0.0\hat{i}+0.22\hat{j}-0.98\hat{k}$,\;\;\;$\hat{n}_{25}=0.66\hat{i}+0.54\hat{j}-0.52\hat{k}$,\newline
$\vec{r}_{13}=0.0\hat{i}+0.0\hat{j}+10.0\hat{k}$,\;\;\;$\vec{r}_{14}=10.0\hat{i}+10.0\hat{j}+0.0\hat{k}$,\;\;\;$\vec{r}_{25}=0.0\hat{i}+10.0\hat{j}+10.0\hat{k}$,\;\;\;$\vec{r}_{35}=10.0\hat{i}+0.0\hat{j}+10.0\hat{k}$.

{\tiny 2D-M213:}

$\hat{n}_{13}=-0.57\hat{i}-0.42\hat{j}+0.71\hat{k}$,\;\;\;$\hat{n}_{14}=-0.88\hat{i}+0.45\hat{j}+0.18\hat{k}$,\;\;\;$\hat{n}_{24}=-0.82\hat{i}+0.36\hat{j}-0.45\hat{k}$,\;\;\;$\hat{n}_{35}=-0.13\hat{i}+0.77\hat{j}-0.62\hat{k}$,\newline
$\vec{r}_{13}=0.0\hat{i}+0.0\hat{j}+0.0\hat{k}$,\;\;\;$\vec{r}_{14}=3.57\hat{i}+2.56\hat{j}+7.35\hat{k}$,\;\;\;$\vec{r}_{25}=2.49\hat{i}+4.52\hat{j}+2.78\hat{k}$,\;\;\;$\vec{r}_{35}=0.0\hat{i}+10.0\hat{j}+0.0\hat{k}$.

{\tiny 2D-M214:}

$\hat{n}_{13}=0.0\hat{i}+0.0\hat{j}-1.0\hat{k}$,\;\;\;$\hat{n}_{14}=0.57\hat{i}+0.52\hat{j}+0.63\hat{k}$,\;\;\;$\hat{n}_{25}=-0.71\hat{i}+0.71\hat{j}+0.01\hat{k}$,\;\;\;$\hat{n}_{35}=-0.43\hat{i}-0.46\hat{j}+0.77\hat{k}$,\newline
$\vec{r}_{13}=10.0\hat{i}+10.0\hat{j}+0.0\hat{k}$,\;\;\;$\vec{r}_{14}=0.0\hat{i}+0.0\hat{j}+10.0\hat{k}$,\;\;\;$\vec{r}_{24}=10.0\hat{i}+10.0\hat{j}+0.0\hat{k}$,\;\;\;$\vec{r}_{25}=0.0\hat{i}+0.0\hat{j}+0.0\hat{k}$.

{\tiny 2D-M215:}

$\hat{n}_{13}=0.46\hat{i}-0.33\hat{j}-0.83\hat{k}$,\;\;\;$\hat{n}_{14}=-0.64\hat{i}+0.67\hat{j}+0.37\hat{k}$,\;\;\;$\hat{n}_{25}=0.79\hat{i}-0.55\hat{j}+0.25\hat{k}$,\;\;\;$\hat{n}_{35}=-0.71\hat{i}+0.12\hat{j}+0.69\hat{k}$,\newline
$\vec{r}_{13}=10.0\hat{i}+0.0\hat{j}+0.0\hat{k}$,\;\;\;$\vec{r}_{14}=8.26\hat{i}+4.82\hat{j}+7.98\hat{k}$,\;\;\;$\vec{r}_{24}=7.31\hat{i}+1.36\hat{j}+7.25\hat{k}$,\;\;\;$\vec{r}_{35}=10.0\hat{i}+10.0\hat{j}+10.0\hat{k}$.

{\tiny 2D-M216:}

$\hat{n}_{13}=0.68\hat{i}-0.08\hat{j}-0.73\hat{k}$,\;\;\;$\hat{n}_{14}=0.0\hat{i}+0.0\hat{j}-1.0\hat{k}$,\;\;\;$\hat{n}_{23}=0.72\hat{i}-0.69\hat{j}+0.05\hat{k}$,\;\;\;$\hat{n}_{25}=-0.82\hat{i}-0.52\hat{j}+0.24\hat{k}$,\newline
$\vec{r}_{13}=10.0\hat{i}+10.0\hat{j}+10.0\hat{k}$,\;\;\;$\vec{r}_{14}=0.0\hat{i}+0.0\hat{j}+5.72\hat{k}$,\;\;\;$\vec{r}_{23}=0.0\hat{i}+0.0\hat{j}+10.0\hat{k}$,\;\;\;$\vec{r}_{45}=10.0\hat{i}+10.0\hat{j}+0.0\hat{k}$.

{\tiny 2D-M217:}

$\hat{n}_{13}=0.0\hat{i}+0.0\hat{j}-1.0\hat{k}$,\;\;\;$\hat{n}_{14}=-0.81\hat{i}-0.41\hat{j}-0.42\hat{k}$,\;\;\;$\hat{n}_{23}=0.43\hat{i}-0.64\hat{j}-0.64\hat{k}$,\;\;\;$\hat{n}_{45}=-0.01\hat{i}-0.7\hat{j}+0.72\hat{k}$,\newline
$\vec{r}_{13}=10.0\hat{i}+10.0\hat{j}+0.2\hat{k}$,\;\;\;$\vec{r}_{14}=0.0\hat{i}+0.0\hat{j}+10.0\hat{k}$,\;\;\;$\vec{r}_{23}=0.0\hat{i}+0.0\hat{j}+10.0\hat{k}$,\;\;\;$\vec{r}_{25}=10.0\hat{i}+0.0\hat{j}+0.0\hat{k}$.

{\tiny 2D-M218:}

$\hat{n}_{13}=0.78\hat{i}+0.17\hat{j}-0.6\hat{k}$,\;\;\;$\hat{n}_{14}=0.02\hat{i}-0.83\hat{j}-0.56\hat{k}$,\;\;\;$\hat{n}_{23}=-0.64\hat{i}-0.64\hat{j}-0.43\hat{k}$,\;\;\;$\hat{n}_{45}=-0.87\hat{i}-0.24\hat{j}+0.44\hat{k}$,\newline
$\vec{r}_{13}=0.0\hat{i}+10.0\hat{j}+10.0\hat{k}$,\;\;\;$\vec{r}_{14}=0.0\hat{i}+0.0\hat{j}+10.0\hat{k}$,\;\;\;$\vec{r}_{23}=0.0\hat{i}+10.0\hat{j}+0.0\hat{k}$,\;\;\;$\vec{r}_{24}=10.0\hat{i}+0.0\hat{j}+0.0\hat{k}$.

{\tiny 2D-M219:}

$\hat{n}_{13}=0.67\hat{i}+0.26\hat{j}-0.69\hat{k}$,\;\;\;$\hat{n}_{14}=-0.92\hat{i}-0.37\hat{j}+0.13\hat{k}$,\;\;\;$\hat{n}_{23}=-0.26\hat{i}-0.91\hat{j}-0.31\hat{k}$,\;\;\;$\hat{n}_{35}=0.68\hat{i}+0.46\hat{j}+0.57\hat{k}$,\newline
$\vec{r}_{13}=0.0\hat{i}+0.0\hat{j}+0.0\hat{k}$,\;\;\;$\vec{r}_{14}=2.68\hat{i}+4.94\hat{j}+6.84\hat{k}$,\;\;\;$\vec{r}_{23}=8.18\hat{i}+7.07\hat{j}+1.99\hat{k}$,\;\;\;$\vec{r}_{24}=8.1\hat{i}+8.25\hat{j}+5.88\hat{k}$.

{\tiny 2D-M220:}

$\hat{n}_{13}=-0.52\hat{i}+0.15\hat{j}-0.84\hat{k}$,\;\;\;$\hat{n}_{14}=0.0\hat{i}+0.91\hat{j}+0.41\hat{k}$,\;\;\;$\hat{n}_{23}=-0.63\hat{i}-0.54\hat{j}+0.56\hat{k}$,\;\;\;$\hat{n}_{25}=0.0\hat{i}+0.0\hat{j}+1.0\hat{k}$,\newline
$\vec{r}_{13}=0.0\hat{i}+10.0\hat{j}+0.0\hat{k}$,\;\;\;$\vec{r}_{14}=0.0\hat{i}+10.0\hat{j}+10.0\hat{k}$,\;\;\;$\vec{r}_{23}=10.0\hat{i}+0.0\hat{j}+10.0\hat{k}$,\;\;\;$\vec{r}_{24}=0.0\hat{i}+0.0\hat{j}+0.0\hat{k}$.

{\tiny 2D-M221:}

$\hat{n}_{13}=-0.0\hat{i}+0.43\hat{j}-0.9\hat{k}$,\;\;\;$\hat{n}_{14}=0.54\hat{i}+0.68\hat{j}+0.49\hat{k}$,\;\;\;$\hat{n}_{23}=0.0\hat{i}+0.0\hat{j}+1.0\hat{k}$,\;\;\;$\hat{n}_{25}=0.62\hat{i}-0.52\hat{j}+0.59\hat{k}$,\newline
$\vec{r}_{13}=10.0\hat{i}+10.0\hat{j}+10.0\hat{k}$,\;\;\;$\vec{r}_{14}=0.0\hat{i}+0.0\hat{j}+10.0\hat{k}$,\;\;\;$\vec{r}_{25}=0.0\hat{i}+10.0\hat{j}+0.0\hat{k}$,\;\;\;$\vec{r}_{45}=10.0\hat{i}+10.0\hat{j}+0.0\hat{k}$.

{\tiny 2D-M222:}

$\hat{n}_{13}=-0.0\hat{i}+0.97\hat{j}-0.24\hat{k}$,\;\;\;$\hat{n}_{14}=0.0\hat{i}+0.6\hat{j}-0.8\hat{k}$,\;\;\;$\hat{n}_{23}=-0.52\hat{i}+0.75\hat{j}+0.41\hat{k}$,\;\;\;$\hat{n}_{45}=-0.82\hat{i}-0.0\hat{j}-0.58\hat{k}$,\newline
$\vec{r}_{13}=0.0\hat{i}+10.0\hat{j}+0.0\hat{k}$,\;\;\;$\vec{r}_{14}=0.0\hat{i}+10.0\hat{j}+0.0\hat{k}$,\;\;\;$\vec{r}_{25}=10.0\hat{i}+0.0\hat{j}+10.0\hat{k}$,\;\;\;$\vec{r}_{45}=0.0\hat{i}+0.0\hat{j}+10.0\hat{k}$.

{\tiny 2D-M223:}

$\hat{n}_{13}=0.8\hat{i}+0.54\hat{j}-0.26\hat{k}$,\;\;\;$\hat{n}_{14}=-0.17\hat{i}+0.61\hat{j}+0.78\hat{k}$,\;\;\;$\hat{n}_{23}=-0.58\hat{i}+0.58\hat{j}-0.58\hat{k}$,\;\;\;$\hat{n}_{45}=0.81\hat{i}-0.44\hat{j}-0.39\hat{k}$,\newline
$\vec{r}_{13}=0.0\hat{i}+10.0\hat{j}+10.0\hat{k}$,\;\;\;$\vec{r}_{14}=0.0\hat{i}+10.0\hat{j}+10.0\hat{k}$,\;\;\;$\vec{r}_{24}=10.0\hat{i}+0.0\hat{j}+0.0\hat{k}$,\;\;\;$\vec{r}_{45}=0.0\hat{i}+0.0\hat{j}+0.0\hat{k}$.

{\tiny 2D-M224:}

$\hat{n}_{13}=-0.69\hat{i}-0.5\hat{j}-0.52\hat{k}$,\;\;\;$\hat{n}_{14}=-0.91\hat{i}-0.41\hat{j}+0.11\hat{k}$,\;\;\;$\hat{n}_{23}=0.87\hat{i}+0.46\hat{j}+0.2\hat{k}$,\;\;\;$\hat{n}_{35}=-0.03\hat{i}+0.87\hat{j}-0.5\hat{k}$,\newline
$\vec{r}_{13}=0.0\hat{i}+10.0\hat{j}+0.0\hat{k}$,\;\;\;$\vec{r}_{14}=3.02\hat{i}+5.79\hat{j}+6.14\hat{k}$,\;\;\;$\vec{r}_{24}=3.41\hat{i}+5.22\hat{j}+4.98\hat{k}$,\;\;\;$\vec{r}_{35}=0.0\hat{i}+0.0\hat{j}+0.0\hat{k}$.

{\tiny 2D-M225:}

$\hat{n}_{13}=-0.0\hat{i}+0.61\hat{j}+0.8\hat{k}$,\;\;\;$\hat{n}_{14}=-0.99\hat{i}-0.07\hat{j}+0.1\hat{k}$,\;\;\;$\hat{n}_{23}=0.0\hat{i}+0.71\hat{j}-0.7\hat{k}$,\;\;\;$\hat{n}_{25}=-0.82\hat{i}+0.52\hat{j}-0.25\hat{k}$,\newline
$\vec{r}_{13}=10.0\hat{i}+0.0\hat{j}+0.0\hat{k}$,\;\;\;$\vec{r}_{14}=10.0\hat{i}+0.0\hat{j}+0.0\hat{k}$,\;\;\;$\vec{r}_{24}=0.0\hat{i}+0.0\hat{j}+10.0\hat{k}$,\;\;\;$\vec{r}_{25}=10.0\hat{i}+10.0\hat{j}+0.0\hat{k}$.

{\tiny 2D-M226:}

$\hat{n}_{13}=0.62\hat{i}+0.62\hat{j}+0.47\hat{k}$,\;\;\;$\hat{n}_{14}=0.79\hat{i}+0.24\hat{j}-0.56\hat{k}$,\;\;\;$\hat{n}_{25}=-0.0\hat{i}+0.71\hat{j}+0.71\hat{k}$,\;\;\;$\hat{n}_{45}=0.59\hat{i}-0.52\hat{j}+0.62\hat{k}$,\newline
$\vec{r}_{13}=0.0\hat{i}+10.0\hat{j}+0.0\hat{k}$,\;\;\;$\vec{r}_{14}=0.0\hat{i}+10.0\hat{j}+10.0\hat{k}$,\;\;\;$\vec{r}_{23}=10.0\hat{i}+0.0\hat{j}+0.0\hat{k}$,\;\;\;$\vec{r}_{25}=0.0\hat{i}+0.0\hat{j}+10.0\hat{k}$.

{\tiny 2D-M227:}

$\hat{n}_{13}=0.0\hat{i}+0.0\hat{j}-1.0\hat{k}$,\;\;\;$\hat{n}_{14}=-0.62\hat{i}-0.79\hat{j}-0.02\hat{k}$,\;\;\;$\hat{n}_{25}=0.0\hat{i}+0.0\hat{j}-1.0\hat{k}$,\;\;\;$\hat{n}_{45}=-0.79\hat{i}-0.61\hat{j}+0.03\hat{k}$,\newline
$\vec{r}_{13}=10.0\hat{i}+0.0\hat{j}+4.83\hat{k}$,\;\;\;$\vec{r}_{14}=0.0\hat{i}+10.0\hat{j}+10.0\hat{k}$,\;\;\;$\vec{r}_{23}=0.0\hat{i}+10.0\hat{j}+0.0\hat{k}$,\;\;\;$\vec{r}_{45}=10.0\hat{i}+0.0\hat{j}+10.0\hat{k}$.

{\tiny 2D-M228:}

$\hat{n}_{13}=-0.58\hat{i}+0.58\hat{j}-0.58\hat{k}$,\;\;\;$\hat{n}_{14}=-0.8\hat{i}-0.25\hat{j}+0.55\hat{k}$,\;\;\;$\hat{n}_{24}=-0.58\hat{i}+0.58\hat{j}-0.58\hat{k}$,\;\;\;$\hat{n}_{45}=0.05\hat{i}-0.93\hat{j}-0.36\hat{k}$,\newline
$\vec{r}_{13}=10.0\hat{i}+10.0\hat{j}+10.0\hat{k}$,\;\;\;$\vec{r}_{14}=10.0\hat{i}+10.0\hat{j}+10.0\hat{k}$,\;\;\;$\vec{r}_{23}=0.0\hat{i}+10.0\hat{j}+0.0\hat{k}$,\;\;\;$\vec{r}_{24}=0.0\hat{i}+0.0\hat{j}+10.0\hat{k}$.

{\tiny 2D-M229:}

$\hat{n}_{13}=0.07\hat{i}+0.61\hat{j}+0.79\hat{k}$,\;\;\;$\hat{n}_{14}=-0.63\hat{i}-0.46\hat{j}-0.63\hat{k}$,\;\;\;$\hat{n}_{24}=0.71\hat{i}+0.0\hat{j}-0.71\hat{k}$,\;\;\;$\hat{n}_{35}=0.3\hat{i}+0.07\hat{j}+0.95\hat{k}$,\newline
$\vec{r}_{13}=10.0\hat{i}+0.0\hat{j}+0.0\hat{k}$,\;\;\;$\vec{r}_{14}=10.0\hat{i}+0.0\hat{j}+0.0\hat{k}$,\;\;\;$\vec{r}_{23}=0.0\hat{i}+10.0\hat{j}+10.0\hat{k}$,\;\;\;$\vec{r}_{24}=0.0\hat{i}+0.0\hat{j}+0.0\hat{k}$.

{\tiny 2D-M230:}

$\hat{n}_{13}=0.5\hat{i}+0.61\hat{j}+0.61\hat{k}$,\;\;\;$\hat{n}_{14}=-0.03\hat{i}-0.73\hat{j}+0.69\hat{k}$,\;\;\;$\hat{n}_{24}=-0.0\hat{i}+0.43\hat{j}-0.9\hat{k}$,\;\;\;$\hat{n}_{25}=0.21\hat{i}+0.04\hat{j}+0.98\hat{k}$,\newline
$\vec{r}_{13}=0.0\hat{i}+0.0\hat{j}+10.0\hat{k}$,\;\;\;$\vec{r}_{14}=10.0\hat{i}+10.0\hat{j}+10.0\hat{k}$,\;\;\;$\vec{r}_{23}=10.0\hat{i}+0.0\hat{j}+0.0\hat{k}$,\;\;\;$\vec{r}_{24}=0.0\hat{i}+10.0\hat{j}+0.0\hat{k}$.

{\tiny 2D-M231:}

$\hat{n}_{13}=0.0\hat{i}+0.71\hat{j}-0.71\hat{k}$,\;\;\;$\hat{n}_{14}=-0.75\hat{i}-0.43\hat{j}+0.51\hat{k}$,\;\;\;$\hat{n}_{24}=0.0\hat{i}-0.0\hat{j}+1.0\hat{k}$,\;\;\;$\hat{n}_{45}=-0.67\hat{i}+0.05\hat{j}+0.74\hat{k}$,\newline
$\vec{r}_{13}=0.0\hat{i}+10.0\hat{j}+0.0\hat{k}$,\;\;\;$\vec{r}_{14}=0.0\hat{i}+0.0\hat{j}+0.0\hat{k}$,\;\;\;$\vec{r}_{23}=10.0\hat{i}+10.0\hat{j}+10.0\hat{k}$,\;\;\;$\vec{r}_{45}=10.0\hat{i}+10.0\hat{j}+10.0\hat{k}$.

{\tiny 2D-M232:}

$\hat{n}_{13}=-0.5\hat{i}-0.18\hat{j}-0.85\hat{k}$,\;\;\;$\hat{n}_{14}=-0.45\hat{i}+0.89\hat{j}+0.01\hat{k}$,\;\;\;$\hat{n}_{24}=-0.13\hat{i}+0.94\hat{j}-0.33\hat{k}$,\;\;\;$\hat{n}_{35}=0.05\hat{i}-0.83\hat{j}+0.56\hat{k}$,\newline
$\vec{r}_{13}=10.0\hat{i}+10.0\hat{j}+0.0\hat{k}$,\;\;\;$\vec{r}_{14}=7.26\hat{i}+2.37\hat{j}+4.72\hat{k}$,\;\;\;$\vec{r}_{23}=0.91\hat{i}+0.23\hat{j}+9.74\hat{k}$,\;\;\;$\vec{r}_{35}=0.0\hat{i}+10.0\hat{j}+0.0\hat{k}$.

{\tiny 2D-M233:}

$\hat{n}_{13}=-0.0\hat{i}+0.71\hat{j}-0.71\hat{k}$,\;\;\;$\hat{n}_{14}=-0.44\hat{i}+0.36\hat{j}-0.83\hat{k}$,\;\;\;$\hat{n}_{24}=-0.53\hat{i}+0.64\hat{j}+0.56\hat{k}$,\;\;\;$\hat{n}_{25}=0.0\hat{i}+0.44\hat{j}-0.9\hat{k}$,\newline
$\vec{r}_{13}=10.0\hat{i}+10.0\hat{j}+10.0\hat{k}$,\;\;\;$\vec{r}_{14}=10.0\hat{i}+0.0\hat{j}+10.0\hat{k}$,\;\;\;$\vec{r}_{23}=0.0\hat{i}+10.0\hat{j}+0.0\hat{k}$,\;\;\;$\vec{r}_{25}=10.0\hat{i}+0.0\hat{j}+10.0\hat{k}$.

{\tiny 2D-M234:}

$\hat{n}_{13}=-0.75\hat{i}+0.66\hat{j}+0.01\hat{k}$,\;\;\;$\hat{n}_{24}=0.0\hat{i}+0.0\hat{j}+1.0\hat{k}$,\;\;\;$\hat{n}_{25}=-0.56\hat{i}-0.56\hat{j}-0.61\hat{k}$,\;\;\;$\hat{n}_{35}=-0.69\hat{i}+0.72\hat{j}-0.03\hat{k}$,\newline
$\vec{r}_{13}=10.0\hat{i}+10.0\hat{j}+0.0\hat{k}$,\;\;\;$\vec{r}_{14}=10.0\hat{i}+10.0\hat{j}+10.0\hat{k}$,\;\;\;$\vec{r}_{24}=0.0\hat{i}+0.0\hat{j}+0.0\hat{k}$,\;\;\;$\vec{r}_{35}=0.0\hat{i}+0.0\hat{j}+0.0\hat{k}$.

{\tiny 2D-M235:}

$\hat{n}_{13}=0.31\hat{i}-0.6\hat{j}-0.73\hat{k}$,\;\;\;$\hat{n}_{24}=0.63\hat{i}+0.55\hat{j}+0.55\hat{k}$,\;\;\;$\hat{n}_{25}=-0.0\hat{i}+0.19\hat{j}-0.98\hat{k}$,\;\;\;$\hat{n}_{35}=0.71\hat{i}-0.69\hat{j}-0.13\hat{k}$,\newline
$\vec{r}_{13}=0.0\hat{i}+10.0\hat{j}+10.0\hat{k}$,\;\;\;$\vec{r}_{14}=10.0\hat{i}+0.0\hat{j}+0.0\hat{k}$,\;\;\;$\vec{r}_{24}=0.0\hat{i}+0.0\hat{j}+10.0\hat{k}$,\;\;\;$\vec{r}_{25}=0.0\hat{i}+10.0\hat{j}+0.0\hat{k}$.

{\tiny 2D-M236:}

$\hat{n}_{13}=-0.0\hat{i}+0.69\hat{j}-0.72\hat{k}$,\;\;\;$\hat{n}_{24}=0.51\hat{i}-0.63\hat{j}-0.59\hat{k}$,\;\;\;$\hat{n}_{25}=0.79\hat{i}+0.56\hat{j}+0.23\hat{k}$,\;\;\;$\hat{n}_{35}=-0.29\hat{i}+0.5\hat{j}-0.82\hat{k}$,\newline
$\vec{r}_{13}=0.0\hat{i}+0.0\hat{j}+0.0\hat{k}$,\;\;\;$\vec{r}_{14}=10.0\hat{i}+0.0\hat{j}+10.0\hat{k}$,\;\;\;$\vec{r}_{25}=0.0\hat{i}+10.0\hat{j}+0.0\hat{k}$,\;\;\;$\vec{r}_{35}=0.0\hat{i}+10.0\hat{j}+0.0\hat{k}$.

{\tiny 2D-M237:}

$\hat{n}_{13}=-0.17\hat{i}+0.67\hat{j}-0.72\hat{k}$,\;\;\;$\hat{n}_{24}=0.19\hat{i}-0.97\hat{j}+0.15\hat{k}$,\;\;\;$\hat{n}_{25}=-0.93\hat{i}-0.33\hat{j}+0.15\hat{k}$,\;\;\;$\hat{n}_{35}=-0.71\hat{i}+0.1\hat{j}+0.7\hat{k}$,\newline
$\vec{r}_{13}=10.0\hat{i}+10.0\hat{j}+10.0\hat{k}$,\;\;\;$\vec{r}_{14}=2.89\hat{i}+3.46\hat{j}+8.02\hat{k}$,\;\;\;$\vec{r}_{25}=3.92\hat{i}+1.58\hat{j}+8.22\hat{k}$,\;\;\;$\vec{r}_{35}=10.0\hat{i}+0.0\hat{j}+0.0\hat{k}$.

{\tiny 2D-M238:}

$\hat{n}_{13}=0.53\hat{i}+0.67\hat{j}-0.51\hat{k}$,\;\;\;$\hat{n}_{24}=-0.0\hat{i}+0.83\hat{j}-0.55\hat{k}$,\;\;\;$\hat{n}_{25}=-0.76\hat{i}-0.0\hat{j}-0.65\hat{k}$,\;\;\;$\hat{n}_{35}=0.58\hat{i}-0.45\hat{j}-0.68\hat{k}$,\newline
$\vec{r}_{13}=10.0\hat{i}+0.0\hat{j}+10.0\hat{k}$,\;\;\;$\vec{r}_{14}=10.0\hat{i}+0.0\hat{j}+10.0\hat{k}$,\;\;\;$\vec{r}_{24}=0.0\hat{i}+10.0\hat{j}+0.0\hat{k}$,\;\;\;$\vec{r}_{25}=0.0\hat{i}+0.0\hat{j}+10.0\hat{k}$.

{\tiny 2D-M239:}

$\hat{n}_{13}=-0.02\hat{i}+0.57\hat{j}-0.82\hat{k}$,\;\;\;$\hat{n}_{24}=0.47\hat{i}-0.88\hat{j}-0.02\hat{k}$,\;\;\;$\hat{n}_{25}=0.02\hat{i}-0.98\hat{j}+0.18\hat{k}$,\;\;\;$\hat{n}_{35}=0.68\hat{i}+0.54\hat{j}+0.5\hat{k}$,\newline
$\vec{r}_{13}=10.0\hat{i}+0.0\hat{j}+10.0\hat{k}$,\;\;\;$\vec{r}_{14}=5.13\hat{i}+6.46\hat{j}+3.38\hat{k}$,\;\;\;$\vec{r}_{24}=2.82\hat{i}+5.36\hat{j}+3.17\hat{k}$,\;\;\;$\vec{r}_{35}=0.0\hat{i}+10.0\hat{j}+0.0\hat{k}$.

{\tiny 2D-M240:}

$\hat{n}_{13}=-0.69\hat{i}-0.54\hat{j}+0.49\hat{k}$,\;\;\;$\hat{n}_{23}=0.22\hat{i}-0.69\hat{j}-0.69\hat{k}$,\;\;\;$\hat{n}_{25}=-0.58\hat{i}-0.58\hat{j}+0.57\hat{k}$,\;\;\;$\hat{n}_{45}=-0.78\hat{i}+0.2\hat{j}-0.6\hat{k}$,\newline
$\vec{r}_{13}=0.0\hat{i}+10.0\hat{j}+10.0\hat{k}$,\;\;\;$\vec{r}_{14}=0.0\hat{i}+0.0\hat{j}+10.0\hat{k}$,\;\;\;$\vec{r}_{23}=10.0\hat{i}+10.0\hat{j}+0.0\hat{k}$,\;\;\;$\vec{r}_{45}=10.0\hat{i}+10.0\hat{j}+0.0\hat{k}$.

{\tiny 2D-M241:}

$\hat{n}_{13}=-0.03\hat{i}+0.84\hat{j}-0.55\hat{k}$,\;\;\;$\hat{n}_{23}=0.0\hat{i}+0.0\hat{j}-1.0\hat{k}$,\;\;\;$\hat{n}_{25}=-0.47\hat{i}-0.59\hat{j}+0.66\hat{k}$,\;\;\;$\hat{n}_{45}=0.0\hat{i}+0.66\hat{j}+0.75\hat{k}$,\newline
$\vec{r}_{13}=0.0\hat{i}+10.0\hat{j}+0.0\hat{k}$,\;\;\;$\vec{r}_{14}=10.0\hat{i}+0.0\hat{j}+10.0\hat{k}$,\;\;\;$\vec{r}_{23}=10.0\hat{i}+10.0\hat{j}+0.0\hat{k}$,\;\;\;$\vec{r}_{25}=0.0\hat{i}+0.0\hat{j}+0.0\hat{k}$.

{\tiny 2D-M242:}

$\hat{n}_{13}=-0.72\hat{i}+0.05\hat{j}-0.69\hat{k}$,\;\;\;$\hat{n}_{23}=-0.71\hat{i}+0.01\hat{j}-0.7\hat{k}$,\;\;\;$\hat{n}_{24}=-0.6\hat{i}-0.54\hat{j}+0.59\hat{k}$,\;\;\;$\hat{n}_{45}=0.27\hat{i}+0.43\hat{j}+0.86\hat{k}$,\newline
$\vec{r}_{13}=0.0\hat{i}+0.0\hat{j}+10.0\hat{k}$,\;\;\;$\vec{r}_{14}=10.0\hat{i}+0.0\hat{j}+10.0\hat{k}$,\;\;\;$\vec{r}_{23}=10.0\hat{i}+10.0\hat{j}+0.0\hat{k}$,\;\;\;$\vec{r}_{24}=0.0\hat{i}+10.0\hat{j}+0.0\hat{k}$.

{\tiny 2D-M243:}

$\hat{n}_{13}=-0.45\hat{i}-0.23\hat{j}-0.86\hat{k}$,\;\;\;$\hat{n}_{23}=-0.13\hat{i}-0.92\hat{j}+0.37\hat{k}$,\;\;\;$\hat{n}_{24}=-0.94\hat{i}-0.18\hat{j}-0.29\hat{k}$,\;\;\;$\hat{n}_{35}=0.37\hat{i}+0.14\hat{j}+0.92\hat{k}$,\newline
$\vec{r}_{13}=10.0\hat{i}+10.0\hat{j}+0.0\hat{k}$,\;\;\;$\vec{r}_{14}=5.12\hat{i}+5.39\hat{j}+4.42\hat{k}$,\;\;\;$\vec{r}_{23}=5.78\hat{i}+4.24\hat{j}+5.07\hat{k}$,\;\;\;$\vec{r}_{24}=5.54\hat{i}+5.62\hat{j}+5.4\hat{k}$.

{\tiny 2D-M244:}

$\hat{n}_{13}=0.22\hat{i}+0.43\hat{j}+0.87\hat{k}$,\;\;\;$\hat{n}_{23}=0.57\hat{i}-0.58\hat{j}+0.58\hat{k}$,\;\;\;$\hat{n}_{24}=0.58\hat{i}-0.21\hat{j}-0.79\hat{k}$,\;\;\;$\hat{n}_{25}=0.14\hat{i}+0.37\hat{j}+0.92\hat{k}$,\newline
$\vec{r}_{13}=10.0\hat{i}+10.0\hat{j}+0.0\hat{k}$,\;\;\;$\vec{r}_{14}=0.0\hat{i}+0.0\hat{j}+10.0\hat{k}$,\;\;\;$\vec{r}_{23}=0.0\hat{i}+10.0\hat{j}+0.0\hat{k}$,\;\;\;$\vec{r}_{24}=10.0\hat{i}+10.0\hat{j}+10.0\hat{k}$.

{\tiny 2D-M245:}

$\hat{n}_{13}=0.0\hat{i}+0.69\hat{j}-0.72\hat{k}$,\;\;\;$\hat{n}_{23}=-0.64\hat{i}+0.56\hat{j}+0.53\hat{k}$,\;\;\;$\hat{n}_{25}=-0.81\hat{i}+0.41\hat{j}+0.41\hat{k}$,\;\;\;$\hat{n}_{45}=0.7\hat{i}+0.49\hat{j}+0.52\hat{k}$,\newline
$\vec{r}_{13}=0.0\hat{i}+10.0\hat{j}+0.0\hat{k}$,\;\;\;$\vec{r}_{14}=10.0\hat{i}+0.0\hat{j}+10.0\hat{k}$,\;\;\;$\vec{r}_{25}=10.0\hat{i}+10.0\hat{j}+10.0\hat{k}$,\;\;\;$\vec{r}_{45}=0.0\hat{i}+10.0\hat{j}+0.0\hat{k}$.

{\tiny 2D-M246:}

$\hat{n}_{13}=0.0\hat{i}+0.49\hat{j}+0.87\hat{k}$,\;\;\;$\hat{n}_{23}=0.55\hat{i}+0.63\hat{j}+0.55\hat{k}$,\;\;\;$\hat{n}_{25}=0.69\hat{i}+0.04\hat{j}-0.73\hat{k}$,\;\;\;$\hat{n}_{45}=0.0\hat{i}+0.91\hat{j}-0.42\hat{k}$,\newline
$\vec{r}_{13}=10.0\hat{i}+10.0\hat{j}+0.0\hat{k}$,\;\;\;$\vec{r}_{14}=10.0\hat{i}+10.0\hat{j}+10.0\hat{k}$,\;\;\;$\vec{r}_{25}=0.0\hat{i}+0.0\hat{j}+0.0\hat{k}$,\;\;\;$\vec{r}_{45}=0.0\hat{i}+0.0\hat{j}+0.0\hat{k}$.

{\tiny 2D-M247:}

$\hat{n}_{13}=0.43\hat{i}-0.44\hat{j}+0.79\hat{k}$,\;\;\;$\hat{n}_{23}=0.71\hat{i}-0.71\hat{j}+0.0\hat{k}$,\;\;\;$\hat{n}_{24}=-0.0\hat{i}-0.0\hat{j}+1.0\hat{k}$,\;\;\;$\hat{n}_{45}=0.0\hat{i}+0.58\hat{j}-0.81\hat{k}$,\newline
$\vec{r}_{13}=0.0\hat{i}+10.0\hat{j}+0.0\hat{k}$,\;\;\;$\vec{r}_{14}=0.0\hat{i}+10.0\hat{j}+0.0\hat{k}$,\;\;\;$\vec{r}_{24}=10.0\hat{i}+0.0\hat{j}+0.0\hat{k}$,\;\;\;$\vec{r}_{45}=10.0\hat{i}+10.0\hat{j}+10.0\hat{k}$.

{\tiny 2D-M248:}

$\hat{n}_{13}=0.05\hat{i}+0.84\hat{j}+0.54\hat{k}$,\;\;\;$\hat{n}_{23}=-0.23\hat{i}-0.91\hat{j}+0.33\hat{k}$,\;\;\;$\hat{n}_{24}=0.26\hat{i}-0.96\hat{j}-0.03\hat{k}$,\;\;\;$\hat{n}_{35}=-0.63\hat{i}+0.73\hat{j}-0.26\hat{k}$,\newline
$\vec{r}_{13}=0.0\hat{i}+0.0\hat{j}+10.0\hat{k}$,\;\;\;$\vec{r}_{14}=4.95\hat{i}+3.34\hat{j}+4.38\hat{k}$,\;\;\;$\vec{r}_{24}=3.26\hat{i}+3.75\hat{j}+6.05\hat{k}$,\;\;\;$\vec{r}_{35}=10.0\hat{i}+10.0\hat{j}+10.0\hat{k}$.

{\tiny 2D-M249:}

$\hat{n}_{13}=0.0\hat{i}+0.77\hat{j}-0.64\hat{k}$,\;\;\;$\hat{n}_{23}=0.5\hat{i}-0.5\hat{j}+0.71\hat{k}$,\;\;\;$\hat{n}_{24}=0.0\hat{i}+0.77\hat{j}+0.64\hat{k}$,\;\;\;$\hat{n}_{25}=0.54\hat{i}+0.67\hat{j}-0.51\hat{k}$,\newline
$\vec{r}_{13}=10.0\hat{i}+10.0\hat{j}+10.0\hat{k}$,\;\;\;$\vec{r}_{14}=0.0\hat{i}+10.0\hat{j}+10.0\hat{k}$,\;\;\;$\vec{r}_{24}=10.0\hat{i}+0.0\hat{j}+0.0\hat{k}$,\;\;\;$\vec{r}_{25}=10.0\hat{i}+0.0\hat{j}+10.0\hat{k}$.

{\tiny 2D-M250:}

$\hat{n}_{13}=0.52\hat{i}-0.84\hat{j}+0.15\hat{k}$,\;\;\;$\hat{n}_{23}=-0.73\hat{i}+0.01\hat{j}+0.69\hat{k}$,\;\;\;$\hat{n}_{25}=0.0\hat{i}+0.85\hat{j}-0.53\hat{k}$,\;\;\;$\hat{n}_{45}=-0.57\hat{i}-0.51\hat{j}-0.64\hat{k}$,\newline
$\vec{r}_{13}=0.0\hat{i}+0.0\hat{j}+10.0\hat{k}$,\;\;\;$\vec{r}_{14}=0.0\hat{i}+0.0\hat{j}+0.0\hat{k}$,\;\;\;$\vec{r}_{23}=10.0\hat{i}+10.0\hat{j}+10.0\hat{k}$,\;\;\;$\vec{r}_{25}=0.0\hat{i}+10.0\hat{j}+0.0\hat{k}$.

{\tiny 2D-M251:}

$\hat{n}_{13}=-0.33\hat{i}+0.54\hat{j}-0.78\hat{k}$,\;\;\;$\hat{n}_{23}=0.04\hat{i}+0.73\hat{j}-0.68\hat{k}$,\;\;\;$\hat{n}_{25}=0.2\hat{i}+0.67\hat{j}+0.72\hat{k}$,\;\;\;$\hat{n}_{45}=-0.65\hat{i}-0.65\hat{j}-0.38\hat{k}$,\newline
$\vec{r}_{13}=0.0\hat{i}+0.0\hat{j}+0.0\hat{k}$,\;\;\;$\vec{r}_{14}=0.0\hat{i}+10.0\hat{j}+0.0\hat{k}$,\;\;\;$\vec{r}_{23}=10.0\hat{i}+10.0\hat{j}+10.0\hat{k}$,\;\;\;$\vec{r}_{45}=10.0\hat{i}+0.0\hat{j}+0.0\hat{k}$.

{\tiny 2D-M252:}

$\hat{n}_{13}=-0.0\hat{i}+0.64\hat{j}-0.77\hat{k}$,\;\;\;$\hat{n}_{23}=0.52\hat{i}-0.71\hat{j}-0.47\hat{k}$,\;\;\;$\hat{n}_{24}=-0.08\hat{i}-0.68\hat{j}+0.73\hat{k}$,\;\;\;$\hat{n}_{45}=-0.0\hat{i}+0.0\hat{j}+1.0\hat{k}$,\newline
$\vec{r}_{13}=10.0\hat{i}+0.0\hat{j}+10.0\hat{k}$,\;\;\;$\vec{r}_{14}=10.0\hat{i}+10.0\hat{j}+10.0\hat{k}$,\;\;\;$\vec{r}_{23}=0.0\hat{i}+0.0\hat{j}+0.0\hat{k}$,\;\;\;$\vec{r}_{24}=0.0\hat{i}+10.0\hat{j}+0.0\hat{k}$.

{\tiny 2D-M253:}

$\hat{n}_{13}=0.63\hat{i}+0.02\hat{j}-0.78\hat{k}$,\;\;\;$\hat{n}_{23}=0.91\hat{i}+0.23\hat{j}+0.35\hat{k}$,\;\;\;$\hat{n}_{24}=0.88\hat{i}+0.24\hat{j}+0.42\hat{k}$,\;\;\;$\hat{n}_{35}=-0.18\hat{i}-0.57\hat{j}-0.8\hat{k}$,\newline
$\vec{r}_{13}=10.0\hat{i}+10.0\hat{j}+10.0\hat{k}$,\;\;\;$\vec{r}_{14}=6.56\hat{i}+4.75\hat{j}+6.38\hat{k}$,\;\;\;$\vec{r}_{23}=6.53\hat{i}+2.55\hat{j}+7.74\hat{k}$,\;\;\;$\vec{r}_{24}=5.03\hat{i}+4.39\hat{j}+6.92\hat{k}$.

{\tiny 2D-M254:}

$\hat{n}_{13}=-0.42\hat{i}-0.76\hat{j}-0.5\hat{k}$,\;\;\;$\hat{n}_{23}=0.37\hat{i}+0.8\hat{j}+0.47\hat{k}$,\;\;\;$\hat{n}_{24}=-0.68\hat{i}+0.68\hat{j}-0.27\hat{k}$,\;\;\;$\hat{n}_{25}=0.85\hat{i}+0.17\hat{j}+0.5\hat{k}$,\newline
$\vec{r}_{13}=0.0\hat{i}+10.0\hat{j}+10.0\hat{k}$,\;\;\;$\vec{r}_{14}=0.0\hat{i}+0.0\hat{j}+10.0\hat{k}$,\;\;\;$\vec{r}_{23}=10.0\hat{i}+10.0\hat{j}+0.0\hat{k}$,\;\;\;$\vec{r}_{24}=10.0\hat{i}+10.0\hat{j}+10.0\hat{k}$.

{\tiny 2D-M255:}

$\hat{n}_{13}=-0.0\hat{i}+0.0\hat{j}+1.0\hat{k}$,\;\;\;$\hat{n}_{23}=0.76\hat{i}+0.63\hat{j}+0.14\hat{k}$,\;\;\;$\hat{n}_{24}=-0.57\hat{i}+0.55\hat{j}+0.61\hat{k}$,\;\;\;$\hat{n}_{45}=0.0\hat{i}+0.64\hat{j}+0.77\hat{k}$,\newline
$\vec{r}_{13}=10.0\hat{i}+10.0\hat{j}+0.0\hat{k}$,\;\;\;$\vec{r}_{14}=0.0\hat{i}+10.0\hat{j}+0.0\hat{k}$,\;\;\;$\vec{r}_{23}=10.0\hat{i}+0.0\hat{j}+10.0\hat{k}$,\;\;\;$\vec{r}_{45}=10.0\hat{i}+10.0\hat{j}+0.0\hat{k}$.

{\tiny 2D-M256:}

$\hat{n}_{13}=0.01\hat{i}+0.58\hat{j}-0.81\hat{k}$,\;\;\;$\hat{n}_{23}=0.88\hat{i}+0.31\hat{j}+0.37\hat{k}$,\;\;\;$\hat{n}_{24}=-0.8\hat{i}+0.07\hat{j}+0.59\hat{k}$,\;\;\;$\hat{n}_{35}=0.82\hat{i}-0.48\hat{j}-0.32\hat{k}$,\newline
$\vec{r}_{13}=10.0\hat{i}+0.0\hat{j}+10.0\hat{k}$,\;\;\;$\vec{r}_{14}=3.41\hat{i}+1.17\hat{j}+1.95\hat{k}$,\;\;\;$\vec{r}_{23}=6.6\hat{i}+8.7\hat{j}+2.72\hat{k}$,\;\;\;$\vec{r}_{35}=10.0\hat{i}+10.0\hat{j}+10.0\hat{k}$.

{\tiny 2D-M257:}

$\hat{n}_{13}=0.57\hat{i}+0.14\hat{j}+0.81\hat{k}$,\;\;\;$\hat{n}_{23}=0.64\hat{i}-0.74\hat{j}-0.2\hat{k}$,\;\;\;$\hat{n}_{24}=0.42\hat{i}+0.74\hat{j}-0.52\hat{k}$,\;\;\;$\hat{n}_{25}=-0.0\hat{i}+0.61\hat{j}+0.79\hat{k}$,\newline
$\vec{r}_{13}=0.0\hat{i}+10.0\hat{j}+0.0\hat{k}$,\;\;\;$\vec{r}_{14}=10.0\hat{i}+10.0\hat{j}+0.0\hat{k}$,\;\;\;$\vec{r}_{23}=0.0\hat{i}+0.0\hat{j}+10.0\hat{k}$,\;\;\;$\vec{r}_{25}=10.0\hat{i}+0.0\hat{j}+0.0\hat{k}$.

{\tiny 2D-M258:}

$\hat{n}_{13}=0.64\hat{i}+0.35\hat{j}-0.68\hat{k}$,\;\;\;$\hat{n}_{14}=0.66\hat{i}-0.05\hat{j}-0.75\hat{k}$,\;\;\;$\hat{n}_{24}=0.82\hat{i}-0.57\hat{j}-0.1\hat{k}$,\;\;\;$\hat{n}_{25}=-0.0\hat{i}+0.0\hat{j}-1.0\hat{k}$,\newline
$\vec{r}_{14}=10.0\hat{i}+0.0\hat{j}+0.0\hat{k}$,\;\;\;$\vec{r}_{24}=0.0\hat{i}+10.0\hat{j}+10.0\hat{k}$,\;\;\;$\vec{r}_{25}=10.0\hat{i}+10.0\hat{j}+0.76\hat{k}$,\;\;\;$\vec{r}_{35}=0.0\hat{i}+0.0\hat{j}+10.0\hat{k}$.

{\tiny 2D-M259:}

$\hat{n}_{13}=-0.1\hat{i}+0.76\hat{j}+0.64\hat{k}$,\;\;\;$\hat{n}_{14}=-0.93\hat{i}+0.38\hat{j}+0.02\hat{k}$,\;\;\;$\hat{n}_{24}=0.48\hat{i}-0.74\hat{j}-0.48\hat{k}$,\;\;\;$\hat{n}_{35}=0.68\hat{i}+0.44\hat{j}+0.59\hat{k}$,\newline
$\vec{r}_{14}=10.0\hat{i}+10.0\hat{j}+0.0\hat{k}$,\;\;\;$\vec{r}_{24}=0.0\hat{i}+0.0\hat{j}+0.0\hat{k}$,\;\;\;$\vec{r}_{25}=0.0\hat{i}+10.0\hat{j}+10.0\hat{k}$,\;\;\;$\vec{r}_{35}=10.0\hat{i}+0.0\hat{j}+10.0\hat{k}$.

{\tiny 2D-M260:}

$\hat{n}_{13}=-0.97\hat{i}+0.07\hat{j}-0.25\hat{k}$,\;\;\;$\hat{n}_{14}=-0.89\hat{i}+0.46\hat{j}+0.01\hat{k}$,\;\;\;$\hat{n}_{25}=0.11\hat{i}+0.76\hat{j}-0.64\hat{k}$,\;\;\;$\hat{n}_{35}=-0.59\hat{i}-0.52\hat{j}+0.62\hat{k}$,\newline
$\vec{r}_{14}=0.0\hat{i}+0.0\hat{j}+0.0\hat{k}$,\;\;\;$\vec{r}_{24}=10.0\hat{i}+0.0\hat{j}+10.0\hat{k}$,\;\;\;$\vec{r}_{25}=0.0\hat{i}+10.0\hat{j}+0.0\hat{k}$,\;\;\;$\vec{r}_{35}=0.0\hat{i}+10.0\hat{j}+10.0\hat{k}$.

{\tiny 2D-M261:}

$\hat{n}_{13}=0.0\hat{i}+0.49\hat{j}-0.87\hat{k}$,\;\;\;$\hat{n}_{14}=-0.03\hat{i}+0.4\hat{j}-0.91\hat{k}$,\;\;\;$\hat{n}_{23}=-0.0\hat{i}+0.6\hat{j}-0.8\hat{k}$,\;\;\;$\hat{n}_{25}=-0.64\hat{i}+0.54\hat{j}+0.54\hat{k}$,\newline
$\vec{r}_{14}=10.0\hat{i}+10.0\hat{j}+10.0\hat{k}$,\;\;\;$\vec{r}_{23}=10.0\hat{i}+10.0\hat{j}+10.0\hat{k}$,\;\;\;$\vec{r}_{25}=10.0\hat{i}+0.0\hat{j}+0.0\hat{k}$,\;\;\;$\vec{r}_{45}=0.0\hat{i}+0.0\hat{j}+10.0\hat{k}$.

{\tiny 2D-M262:}

$\hat{n}_{13}=0.84\hat{i}-0.32\hat{j}-0.44\hat{k}$,\;\;\;$\hat{n}_{14}=0.6\hat{i}-0.43\hat{j}+0.68\hat{k}$,\;\;\;$\hat{n}_{23}=0.79\hat{i}+0.56\hat{j}+0.23\hat{k}$,\;\;\;$\hat{n}_{45}=0.06\hat{i}-0.82\hat{j}+0.57\hat{k}$,\newline
$\vec{r}_{14}=10.0\hat{i}+0.0\hat{j}+10.0\hat{k}$,\;\;\;$\vec{r}_{23}=10.0\hat{i}+0.0\hat{j}+10.0\hat{k}$,\;\;\;$\vec{r}_{25}=0.0\hat{i}+10.0\hat{j}+0.0\hat{k}$,\;\;\;$\vec{r}_{45}=0.0\hat{i}+0.0\hat{j}+0.0\hat{k}$.

{\tiny 2D-M263:}

$\hat{n}_{13}=-0.0\hat{i}+0.0\hat{j}-1.0\hat{k}$,\;\;\;$\hat{n}_{14}=0.0\hat{i}+0.73\hat{j}+0.69\hat{k}$,\;\;\;$\hat{n}_{23}=0.0\hat{i}-0.0\hat{j}-1.0\hat{k}$,\;\;\;$\hat{n}_{45}=0.0\hat{i}+0.65\hat{j}+0.76\hat{k}$,\newline
$\vec{r}_{14}=0.0\hat{i}+10.0\hat{j}+10.0\hat{k}$,\;\;\;$\vec{r}_{23}=10.0\hat{i}+10.0\hat{j}+8.19\hat{k}$,\;\;\;$\vec{r}_{24}=0.0\hat{i}+0.0\hat{j}+0.0\hat{k}$,\;\;\;$\vec{r}_{45}=10.0\hat{i}+10.0\hat{j}+0.0\hat{k}$.

{\tiny 2D-M264:}

$\hat{n}_{13}=-0.33\hat{i}-0.07\hat{j}-0.94\hat{k}$,\;\;\;$\hat{n}_{14}=-0.99\hat{i}-0.15\hat{j}+0.02\hat{k}$,\;\;\;$\hat{n}_{23}=-0.57\hat{i}-0.81\hat{j}-0.17\hat{k}$,\;\;\;$\hat{n}_{35}=0.35\hat{i}+0.65\hat{j}-0.67\hat{k}$,\newline
$\vec{r}_{14}=5.08\hat{i}+4.91\hat{j}+5.17\hat{k}$,\;\;\;$\vec{r}_{23}=4.91\hat{i}+5.3\hat{j}+4.76\hat{k}$,\;\;\;$\vec{r}_{24}=5.32\hat{i}+5.1\hat{j}+5.01\hat{k}$,\;\;\;$\vec{r}_{35}=0.0\hat{i}+0.0\hat{j}+0.0\hat{k}$.

{\tiny 2D-M265:}

$\hat{n}_{13}=0.31\hat{i}+0.52\hat{j}+0.8\hat{k}$,\;\;\;$\hat{n}_{14}=-0.0\hat{i}+0.24\hat{j}+0.97\hat{k}$,\;\;\;$\hat{n}_{23}=-0.65\hat{i}-0.39\hat{j}+0.65\hat{k}$,\;\;\;$\hat{n}_{25}=0.26\hat{i}+0.41\hat{j}+0.88\hat{k}$,\newline
$\vec{r}_{14}=0.0\hat{i}+10.0\hat{j}+10.0\hat{k}$,\;\;\;$\vec{r}_{23}=10.0\hat{i}+10.0\hat{j}+10.0\hat{k}$,\;\;\;$\vec{r}_{24}=10.0\hat{i}+0.0\hat{j}+0.0\hat{k}$,\;\;\;$\vec{r}_{25}=10.0\hat{i}+10.0\hat{j}+0.0\hat{k}$.

{\tiny 2D-M266:}

$\hat{n}_{13}=0.0\hat{i}+0.73\hat{j}-0.69\hat{k}$,\;\;\;$\hat{n}_{14}=0.53\hat{i}-0.66\hat{j}-0.53\hat{k}$,\;\;\;$\hat{n}_{25}=0.76\hat{i}+0.64\hat{j}-0.13\hat{k}$,\;\;\;$\hat{n}_{45}=0.78\hat{i}+0.63\hat{j}-0.01\hat{k}$,\newline
$\vec{r}_{14}=10.0\hat{i}+0.0\hat{j}+0.0\hat{k}$,\;\;\;$\vec{r}_{23}=0.0\hat{i}+10.0\hat{j}+10.0\hat{k}$,\;\;\;$\vec{r}_{25}=10.0\hat{i}+0.0\hat{j}+0.0\hat{k}$,\;\;\;$\vec{r}_{45}=10.0\hat{i}+0.0\hat{j}+10.0\hat{k}$.

{\tiny 2D-M267:}

$\hat{n}_{13}=0.0\hat{i}-0.71\hat{j}-0.71\hat{k}$,\;\;\;$\hat{n}_{14}=0.53\hat{i}+0.6\hat{j}+0.6\hat{k}$,\;\;\;$\hat{n}_{24}=-0.0\hat{i}-0.71\hat{j}+0.71\hat{k}$,\;\;\;$\hat{n}_{45}=0.24\hat{i}+0.42\hat{j}-0.88\hat{k}$,\newline
$\vec{r}_{14}=0.0\hat{i}+10.0\hat{j}+0.0\hat{k}$,\;\;\;$\vec{r}_{23}=10.0\hat{i}+0.0\hat{j}+10.0\hat{k}$,\;\;\;$\vec{r}_{24}=0.0\hat{i}+0.0\hat{j}+0.0\hat{k}$,\;\;\;$\vec{r}_{45}=10.0\hat{i}+10.0\hat{j}+10.0\hat{k}$.

{\tiny 2D-M268:}

$\hat{n}_{13}=-0.03\hat{i}+0.34\hat{j}-0.94\hat{k}$,\;\;\;$\hat{n}_{14}=-0.09\hat{i}-0.97\hat{j}-0.23\hat{k}$,\;\;\;$\hat{n}_{24}=0.91\hat{i}-0.36\hat{j}-0.21\hat{k}$,\;\;\;$\hat{n}_{35}=0.11\hat{i}+0.51\hat{j}-0.85\hat{k}$,\newline
$\vec{r}_{14}=4.96\hat{i}+5.0\hat{j}+5.04\hat{k}$,\;\;\;$\vec{r}_{23}=4.9\hat{i}+4.92\hat{j}+5.09\hat{k}$,\;\;\;$\vec{r}_{24}=6.07\hat{i}+5.07\hat{j}+5.07\hat{k}$,\;\;\;$\vec{r}_{35}=10.0\hat{i}+10.0\hat{j}+10.0\hat{k}$.

{\tiny 2D-M269:}

$\hat{n}_{13}=-0.58\hat{i}+0.17\hat{j}-0.8\hat{k}$,\;\;\;$\hat{n}_{14}=0.7\hat{i}+0.02\hat{j}+0.71\hat{k}$,\;\;\;$\hat{n}_{24}=0.0\hat{i}-0.0\hat{j}+1.0\hat{k}$,\;\;\;$\hat{n}_{25}=-0.31\hat{i}+0.72\hat{j}-0.62\hat{k}$,\newline
$\vec{r}_{14}=10.0\hat{i}+10.0\hat{j}+0.0\hat{k}$,\;\;\;$\vec{r}_{23}=0.0\hat{i}+10.0\hat{j}+10.0\hat{k}$,\;\;\;$\vec{r}_{24}=10.0\hat{i}+0.0\hat{j}+5.51\hat{k}$,\;\;\;$\vec{r}_{25}=10.0\hat{i}+10.0\hat{j}+10.0\hat{k}$.

{\tiny 2D-M270:}

$\hat{n}_{13}=-0.0\hat{i}+0.0\hat{j}+1.0\hat{k}$,\;\;\;$\hat{n}_{24}=0.0\hat{i}+0.02\hat{j}+1.0\hat{k}$,\;\;\;$\hat{n}_{25}=0.62\hat{i}-0.48\hat{j}-0.62\hat{k}$,\;\;\;$\hat{n}_{35}=0.85\hat{i}-0.48\hat{j}+0.22\hat{k}$,\newline
$\vec{r}_{14}=0.0\hat{i}+0.0\hat{j}+0.0\hat{k}$,\;\;\;$\vec{r}_{24}=10.0\hat{i}+10.0\hat{j}+0.0\hat{k}$,\;\;\;$\vec{r}_{25}=0.0\hat{i}+10.0\hat{j}+10.0\hat{k}$,\;\;\;$\vec{r}_{35}=10.0\hat{i}+10.0\hat{j}+0.0\hat{k}$.

{\tiny 2D-M271:}

$\hat{n}_{13}=0.0\hat{i}+0.94\hat{j}-0.35\hat{k}$,\;\;\;$\hat{n}_{24}=-0.71\hat{i}+0.71\hat{j}+0.01\hat{k}$,\;\;\;$\hat{n}_{25}=0.61\hat{i}+0.64\hat{j}-0.46\hat{k}$,\;\;\;$\hat{n}_{35}=-0.72\hat{i}+0.69\hat{j}+0.02\hat{k}$,\newline
$\vec{r}_{14}=0.0\hat{i}+0.0\hat{j}+0.0\hat{k}$,\;\;\;$\vec{r}_{24}=10.0\hat{i}+10.0\hat{j}+0.0\hat{k}$,\;\;\;$\vec{r}_{25}=10.0\hat{i}+10.0\hat{j}+10.0\hat{k}$,\;\;\;$\vec{r}_{35}=10.0\hat{i}+10.0\hat{j}+0.0\hat{k}$.

{\tiny 2D-M272:}

$\hat{n}_{13}=0.27\hat{i}+0.68\hat{j}+0.68\hat{k}$,\;\;\;$\hat{n}_{24}=-0.88\hat{i}+0.48\hat{j}+0.01\hat{k}$,\;\;\;$\hat{n}_{25}=0.12\hat{i}+0.76\hat{j}+0.64\hat{k}$,\;\;\;$\hat{n}_{35}=0.68\hat{i}+0.44\hat{j}+0.59\hat{k}$,\newline
$\vec{r}_{14}=0.0\hat{i}+10.0\hat{j}+10.0\hat{k}$,\;\;\;$\vec{r}_{24}=10.0\hat{i}+10.0\hat{j}+0.0\hat{k}$,\;\;\;$\vec{r}_{25}=10.0\hat{i}+0.0\hat{j}+0.0\hat{k}$,\;\;\;$\vec{r}_{35}=10.0\hat{i}+0.0\hat{j}+10.0\hat{k}$.

{\tiny 2D-M273:}

$\hat{n}_{13}=0.79\hat{i}-0.46\hat{j}+0.4\hat{k}$,\;\;\;$\hat{n}_{23}=-0.93\hat{i}-0.37\hat{j}+0.1\hat{k}$,\;\;\;$\hat{n}_{25}=-0.59\hat{i}+0.55\hat{j}+0.59\hat{k}$,\;\;\;$\hat{n}_{45}=-0.59\hat{i}+0.2\hat{j}-0.78\hat{k}$,\newline
$\vec{r}_{14}=0.0\hat{i}+0.0\hat{j}+0.0\hat{k}$,\;\;\;$\vec{r}_{23}=10.0\hat{i}+0.0\hat{j}+0.0\hat{k}$,\;\;\;$\vec{r}_{25}=0.0\hat{i}+10.0\hat{j}+10.0\hat{k}$,\;\;\;$\vec{r}_{45}=10.0\hat{i}+10.0\hat{j}+0.0\hat{k}$.

{\tiny 2D-M274:}

$\hat{n}_{13}=-0.0\hat{i}+0.95\hat{j}+0.31\hat{k}$,\;\;\;$\hat{n}_{23}=-0.06\hat{i}+0.26\hat{j}+0.96\hat{k}$,\;\;\;$\hat{n}_{25}=0.0\hat{i}+0.31\hat{j}-0.95\hat{k}$,\;\;\;$\hat{n}_{45}=-0.64\hat{i}+0.43\hat{j}+0.64\hat{k}$,\newline
$\vec{r}_{14}=10.0\hat{i}+10.0\hat{j}+10.0\hat{k}$,\;\;\;$\vec{r}_{23}=10.0\hat{i}+0.0\hat{j}+0.0\hat{k}$,\;\;\;$\vec{r}_{25}=0.0\hat{i}+0.0\hat{j}+0.0\hat{k}$,\;\;\;$\vec{r}_{45}=10.0\hat{i}+0.0\hat{j}+0.0\hat{k}$.

{\tiny 2D-M275:}

$\hat{n}_{13}=-0.77\hat{i}-0.46\hat{j}-0.44\hat{k}$,\;\;\;$\hat{n}_{23}=0.78\hat{i}-0.61\hat{j}+0.14\hat{k}$,\;\;\;$\hat{n}_{24}=-0.43\hat{i}-0.13\hat{j}+0.89\hat{k}$,\;\;\;$\hat{n}_{45}=-0.7\hat{i}+0.1\hat{j}-0.71\hat{k}$,\newline
$\vec{r}_{14}=10.0\hat{i}+10.0\hat{j}+0.0\hat{k}$,\;\;\;$\vec{r}_{23}=0.0\hat{i}+0.0\hat{j}+10.0\hat{k}$,\;\;\;$\vec{r}_{24}=0.0\hat{i}+0.0\hat{j}+0.0\hat{k}$,\;\;\;$\vec{r}_{45}=10.0\hat{i}+0.0\hat{j}+10.0\hat{k}$.

{\tiny 2D-M276:}

$\hat{n}_{13}=0.28\hat{i}+0.29\hat{j}+0.91\hat{k}$,\;\;\;$\hat{n}_{23}=0.67\hat{i}+0.73\hat{j}+0.16\hat{k}$,\;\;\;$\hat{n}_{24}=-0.52\hat{i}-0.26\hat{j}-0.81\hat{k}$,\;\;\;$\hat{n}_{35}=-0.33\hat{i}-0.35\hat{j}-0.88\hat{k}$,\newline
$\vec{r}_{14}=4.74\hat{i}+4.95\hat{j}+5.1\hat{k}$,\;\;\;$\vec{r}_{23}=6.26\hat{i}+5.85\hat{j}+6.44\hat{k}$,\;\;\;$\vec{r}_{24}=4.75\hat{i}+4.71\hat{j}+5.03\hat{k}$,\;\;\;$\vec{r}_{35}=10.0\hat{i}+10.0\hat{j}+0.0\hat{k}$.

{\tiny 2D-M277:}

$\hat{n}_{13}=0.0\hat{i}+0.0\hat{j}-1.0\hat{k}$,\;\;\;$\hat{n}_{23}=0.58\hat{i}+0.58\hat{j}-0.58\hat{k}$,\;\;\;$\hat{n}_{24}=-0.0\hat{i}+0.0\hat{j}-1.0\hat{k}$,\;\;\;$\hat{n}_{25}=0.0\hat{i}+0.5\hat{j}+0.86\hat{k}$,\newline
$\vec{r}_{14}=0.0\hat{i}+10.0\hat{j}+10.0\hat{k}$,\;\;\;$\vec{r}_{23}=0.0\hat{i}+0.0\hat{j}+0.0\hat{k}$,\;\;\;$\vec{r}_{24}=10.0\hat{i}+0.0\hat{j}+0.0\hat{k}$,\;\;\;$\vec{r}_{25}=10.0\hat{i}+0.0\hat{j}+0.0\hat{k}$.

{\tiny 2D-M278:}

$\hat{n}_{13}=-0.0\hat{i}+0.6\hat{j}-0.8\hat{k}$,\;\;\;$\hat{n}_{23}=0.52\hat{i}-0.72\hat{j}-0.46\hat{k}$,\;\;\;$\hat{n}_{25}=0.0\hat{i}+0.0\hat{j}-1.0\hat{k}$,\;\;\;$\hat{n}_{45}=-0.47\hat{i}+0.63\hat{j}-0.63\hat{k}$,\newline
$\vec{r}_{14}=10.0\hat{i}+10.0\hat{j}+10.0\hat{k}$,\;\;\;$\vec{r}_{23}=0.0\hat{i}+0.0\hat{j}+10.0\hat{k}$,\;\;\;$\vec{r}_{25}=10.0\hat{i}+0.0\hat{j}+0.0\hat{k}$,\;\;\;$\vec{r}_{45}=0.0\hat{i}+10.0\hat{j}+0.0\hat{k}$.

{\tiny 2D-M279:}

$\hat{n}_{13}=-0.97\hat{i}-0.25\hat{j}+0.0\hat{k}$,\;\;\;$\hat{n}_{23}=-0.0\hat{i}+0.0\hat{j}+1.0\hat{k}$,\;\;\;$\hat{n}_{24}=-0.64\hat{i}+0.57\hat{j}+0.52\hat{k}$,\;\;\;$\hat{n}_{45}=0.73\hat{i}-0.14\hat{j}+0.67\hat{k}$,\newline
$\vec{r}_{14}=10.0\hat{i}+10.0\hat{j}+0.0\hat{k}$,\;\;\;$\vec{r}_{23}=0.0\hat{i}+0.0\hat{j}+10.0\hat{k}$,\;\;\;$\vec{r}_{24}=0.0\hat{i}+10.0\hat{j}+10.0\hat{k}$,\;\;\;$\vec{r}_{45}=10.0\hat{i}+10.0\hat{j}+0.0\hat{k}$.

{\tiny 2D-M280:}

$\hat{n}_{13}=0.72\hat{i}+0.46\hat{j}-0.52\hat{k}$,\;\;\;$\hat{n}_{23}=0.57\hat{i}-0.76\hat{j}-0.32\hat{k}$,\;\;\;$\hat{n}_{24}=-0.19\hat{i}-0.67\hat{j}-0.72\hat{k}$,\;\;\;$\hat{n}_{35}=0.65\hat{i}-0.72\hat{j}-0.23\hat{k}$,\newline
$\vec{r}_{14}=6.07\hat{i}+5.03\hat{j}+3.9\hat{k}$,\;\;\;$\vec{r}_{23}=6.94\hat{i}+7.02\hat{j}+2.92\hat{k}$,\;\;\;$\vec{r}_{24}=2.83\hat{i}+3.65\hat{j}+7.09\hat{k}$,\;\;\;$\vec{r}_{35}=10.0\hat{i}+10.0\hat{j}+0.0\hat{k}$.

{\tiny 2D-M281:}

$\hat{n}_{13}=-0.58\hat{i}-0.36\hat{j}+0.73\hat{k}$,\;\;\;$\hat{n}_{23}=0.0\hat{i}+0.9\hat{j}+0.45\hat{k}$,\;\;\;$\hat{n}_{24}=-0.8\hat{i}+0.0\hat{j}-0.6\hat{k}$,\;\;\;$\hat{n}_{25}=-0.0\hat{i}+0.0\hat{j}+1.0\hat{k}$,\newline
$\vec{r}_{14}=10.0\hat{i}+10.0\hat{j}+0.0\hat{k}$,\;\;\;$\vec{r}_{23}=0.0\hat{i}+0.0\hat{j}+10.0\hat{k}$,\;\;\;$\vec{r}_{24}=0.0\hat{i}+10.0\hat{j}+0.0\hat{k}$,\;\;\;$\vec{r}_{25}=0.0\hat{i}+10.0\hat{j}+6.03\hat{k}$.

{\tiny 2D-M282:}

$\hat{n}_{13}=0.82\hat{i}+0.52\hat{j}-0.25\hat{k}$,\;\;\;$\hat{n}_{24}=-0.69\hat{i}-0.22\hat{j}+0.69\hat{k}$,\;\;\;$\hat{n}_{25}=0.01\hat{i}+0.71\hat{j}+0.7\hat{k}$,\;\;\;$\hat{n}_{35}=-0.57\hat{i}+0.65\hat{j}-0.51\hat{k}$,\newline
$\vec{r}_{13}=10.0\hat{i}+0.0\hat{j}+0.0\hat{k}$,\;\;\;$\vec{r}_{14}=0.0\hat{i}+10.0\hat{j}+10.0\hat{k}$,\;\;\;$\vec{r}_{24}=0.0\hat{i}+0.0\hat{j}+0.0\hat{k}$,\;\;\;$\vec{r}_{25}=10.0\hat{i}+0.0\hat{j}+0.0\hat{k}$.

{\tiny 2D-M283:}

$\hat{n}_{13}=0.2\hat{i}+0.9\hat{j}-0.38\hat{k}$,\;\;\;$\hat{n}_{24}=0.0\hat{i}+0.38\hat{j}-0.92\hat{k}$,\;\;\;$\hat{n}_{25}=-0.0\hat{i}+0.0\hat{j}-1.0\hat{k}$,\;\;\;$\hat{n}_{35}=0.0\hat{i}+0.89\hat{j}+0.46\hat{k}$,\newline
$\vec{r}_{13}=10.0\hat{i}+10.0\hat{j}+10.0\hat{k}$,\;\;\;$\vec{r}_{14}=0.0\hat{i}+10.0\hat{j}+0.0\hat{k}$,\;\;\;$\vec{r}_{24}=10.0\hat{i}+0.0\hat{j}+10.0\hat{k}$,\;\;\;$\vec{r}_{35}=10.0\hat{i}+10.0\hat{j}+0.0\hat{k}$.

{\tiny 2D-M284:}

$\hat{n}_{13}=-0.79\hat{i}-0.19\hat{j}+0.59\hat{k}$,\;\;\;$\hat{n}_{24}=0.58\hat{i}-0.5\hat{j}+0.64\hat{k}$,\;\;\;$\hat{n}_{25}=-0.0\hat{i}+0.8\hat{j}+0.6\hat{k}$,\;\;\;$\hat{n}_{35}=-0.75\hat{i}-0.19\hat{j}+0.64\hat{k}$,\newline
$\vec{r}_{13}=10.0\hat{i}+0.0\hat{j}+0.0\hat{k}$,\;\;\;$\vec{r}_{14}=0.0\hat{i}+10.0\hat{j}+10.0\hat{k}$,\;\;\;$\vec{r}_{25}=10.0\hat{i}+0.0\hat{j}+0.0\hat{k}$,\;\;\;$\vec{r}_{35}=0.0\hat{i}+0.0\hat{j}+0.0\hat{k}$.

{\tiny 2D-M285:}

$\hat{n}_{13}=0.0\hat{i}+0.82\hat{j}-0.58\hat{k}$,\;\;\;$\hat{n}_{23}=0.82\hat{i}-0.21\hat{j}+0.54\hat{k}$,\;\;\;$\hat{n}_{25}=-0.0\hat{i}+0.66\hat{j}-0.75\hat{k}$,\;\;\;$\hat{n}_{45}=0.97\hat{i}-0.24\hat{j}-0.07\hat{k}$,\newline
$\vec{r}_{13}=0.0\hat{i}+0.0\hat{j}+0.0\hat{k}$,\;\;\;$\vec{r}_{14}=0.0\hat{i}+10.0\hat{j}+0.0\hat{k}$,\;\;\;$\vec{r}_{23}=10.0\hat{i}+10.0\hat{j}+0.0\hat{k}$,\;\;\;$\vec{r}_{25}=10.0\hat{i}+0.0\hat{j}+10.0\hat{k}$.

{\tiny 2D-M286:}

$\hat{n}_{13}=-0.43\hat{i}+0.84\hat{j}+0.32\hat{k}$,\;\;\;$\hat{n}_{23}=0.25\hat{i}-0.57\hat{j}-0.78\hat{k}$,\;\;\;$\hat{n}_{25}=0.0\hat{i}+0.0\hat{j}+1.0\hat{k}$,\;\;\;$\hat{n}_{45}=0.77\hat{i}+0.45\hat{j}+0.45\hat{k}$,\newline
$\vec{r}_{13}=0.0\hat{i}+10.0\hat{j}+10.0\hat{k}$,\;\;\;$\vec{r}_{14}=10.0\hat{i}+10.0\hat{j}+0.0\hat{k}$,\;\;\;$\vec{r}_{23}=10.0\hat{i}+0.0\hat{j}+0.0\hat{k}$,\;\;\;$\vec{r}_{45}=0.0\hat{i}+10.0\hat{j}+10.0\hat{k}$.

{\tiny 2D-M287:}

$\hat{n}_{13}=-0.79\hat{i}+0.51\hat{j}+0.34\hat{k}$,\;\;\;$\hat{n}_{23}=0.08\hat{i}+0.56\hat{j}+0.82\hat{k}$,\;\;\;$\hat{n}_{24}=-0.65\hat{i}+0.37\hat{j}-0.67\hat{k}$,\;\;\;$\hat{n}_{45}=-0.0\hat{i}+0.0\hat{j}+1.0\hat{k}$,\newline
$\vec{r}_{13}=10.0\hat{i}+10.0\hat{j}+10.0\hat{k}$,\;\;\;$\vec{r}_{14}=0.0\hat{i}+0.0\hat{j}+10.0\hat{k}$,\;\;\;$\vec{r}_{23}=10.0\hat{i}+0.0\hat{j}+0.0\hat{k}$,\;\;\;$\vec{r}_{24}=0.0\hat{i}+10.0\hat{j}+0.0\hat{k}$.

{\tiny 2D-M288:}

$\hat{n}_{13}=-0.53\hat{i}-0.53\hat{j}-0.67\hat{k}$,\;\;\;$\hat{n}_{23}=-0.62\hat{i}-0.62\hat{j}+0.48\hat{k}$,\;\;\;$\hat{n}_{24}=0.0\hat{i}+0.0\hat{j}+1.0\hat{k}$,\;\;\;$\hat{n}_{35}=-0.18\hat{i}+0.9\hat{j}-0.4\hat{k}$,\newline
$\vec{r}_{13}=10.0\hat{i}+0.0\hat{j}+10.0\hat{k}$,\;\;\;$\vec{r}_{14}=0.0\hat{i}+10.0\hat{j}+0.0\hat{k}$,\;\;\;$\vec{r}_{23}=10.0\hat{i}+0.0\hat{j}+0.0\hat{k}$,\;\;\;$\vec{r}_{24}=10.0\hat{i}+10.0\hat{j}+0.29\hat{k}$.

{\tiny 2D-M289:}

$\hat{n}_{13}=0.0\hat{i}+0.27\hat{j}+0.96\hat{k}$,\;\;\;$\hat{n}_{23}=-0.53\hat{i}+0.18\hat{j}-0.83\hat{k}$,\;\;\;$\hat{n}_{24}=0.64\hat{i}-0.42\hat{j}+0.64\hat{k}$,\;\;\;$\hat{n}_{25}=-0.0\hat{i}+0.0\hat{j}+1.0\hat{k}$,\newline
$\vec{r}_{13}=10.0\hat{i}+10.0\hat{j}+0.0\hat{k}$,\;\;\;$\vec{r}_{14}=0.0\hat{i}+0.0\hat{j}+10.0\hat{k}$,\;\;\;$\vec{r}_{23}=0.0\hat{i}+10.0\hat{j}+0.0\hat{k}$,\;\;\;$\vec{r}_{24}=0.0\hat{i}+10.0\hat{j}+0.0\hat{k}$.

{\tiny 2D-M290:}

$\hat{n}_{13}=0.22\hat{i}+0.8\hat{j}+0.56\hat{k}$,\;\;\;$\hat{n}_{23}=0.51\hat{i}+0.62\hat{j}-0.59\hat{k}$,\;\;\;$\hat{n}_{24}=-0.54\hat{i}+0.58\hat{j}-0.61\hat{k}$,\;\;\;$\hat{n}_{45}=0.23\hat{i}-0.69\hat{j}-0.69\hat{k}$,\newline
$\vec{r}_{13}=10.0\hat{i}+0.0\hat{j}+0.0\hat{k}$,\;\;\;$\vec{r}_{14}=0.0\hat{i}+10.0\hat{j}+10.0\hat{k}$,\;\;\;$\vec{r}_{23}=10.0\hat{i}+10.0\hat{j}+10.0\hat{k}$,\;\;\;$\vec{r}_{45}=10.0\hat{i}+10.0\hat{j}+0.0\hat{k}$.

{\tiny 2D-M291:}

$\hat{n}_{13}=0.36\hat{i}+0.81\hat{j}-0.46\hat{k}$,\;\;\;$\hat{n}_{23}=0.73\hat{i}+0.06\hat{j}+0.68\hat{k}$,\;\;\;$\hat{n}_{24}=-0.58\hat{i}+0.58\hat{j}+0.58\hat{k}$,\;\;\;$\hat{n}_{35}=-0.24\hat{i}-0.74\hat{j}+0.63\hat{k}$,\newline
$\vec{r}_{13}=0.0\hat{i}+10.0\hat{j}+0.0\hat{k}$,\;\;\;$\vec{r}_{14}=10.0\hat{i}+0.0\hat{j}+10.0\hat{k}$,\;\;\;$\vec{r}_{23}=0.0\hat{i}+10.0\hat{j}+0.0\hat{k}$,\;\;\;$\vec{r}_{35}=0.0\hat{i}+0.0\hat{j}+0.0\hat{k}$.

{\tiny 2D-M292:}

$\hat{n}_{13}=-0.37\hat{i}-0.55\hat{j}-0.74\hat{k}$,\;\;\;$\hat{n}_{23}=-0.72\hat{i}+0.69\hat{j}-0.07\hat{k}$,\;\;\;$\hat{n}_{24}=-0.6\hat{i}-0.6\hat{j}+0.53\hat{k}$,\;\;\;$\hat{n}_{25}=-0.81\hat{i}-0.57\hat{j}+0.15\hat{k}$,\newline
$\vec{r}_{13}=10.0\hat{i}+10.0\hat{j}+0.0\hat{k}$,\;\;\;$\vec{r}_{14}=0.0\hat{i}+0.0\hat{j}+10.0\hat{k}$,\;\;\;$\vec{r}_{23}=10.0\hat{i}+10.0\hat{j}+10.0\hat{k}$,\;\;\;$\vec{r}_{25}=10.0\hat{i}+0.0\hat{j}+10.0\hat{k}$.

{\tiny 2D-M293:}

$\hat{n}_{13}=0.71\hat{i}+0.0\hat{j}-0.71\hat{k}$,\;\;\;$\hat{n}_{23}=-0.58\hat{i}-0.58\hat{j}-0.58\hat{k}$,\;\;\;$\hat{n}_{25}=-0.67\hat{i}+0.05\hat{j}+0.74\hat{k}$,\;\;\;$\hat{n}_{45}=0.41\hat{i}-0.82\hat{j}+0.41\hat{k}$,\newline
$\vec{r}_{13}=0.0\hat{i}+0.0\hat{j}+0.0\hat{k}$,\;\;\;$\vec{r}_{14}=10.0\hat{i}+10.0\hat{j}+10.0\hat{k}$,\;\;\;$\vec{r}_{25}=10.0\hat{i}+10.0\hat{j}+10.0\hat{k}$,\;\;\;$\vec{r}_{45}=0.0\hat{i}+0.0\hat{j}+0.0\hat{k}$.

{\tiny 2D-M294:}

$\hat{n}_{13}=-0.37\hat{i}+0.44\hat{j}-0.82\hat{k}$,\;\;\;$\hat{n}_{23}=0.58\hat{i}-0.58\hat{j}-0.58\hat{k}$,\;\;\;$\hat{n}_{24}=-0.0\hat{i}+0.0\hat{j}+1.0\hat{k}$,\;\;\;$\hat{n}_{45}=0.71\hat{i}-0.11\hat{j}-0.7\hat{k}$,\newline
$\vec{r}_{13}=0.0\hat{i}+10.0\hat{j}+0.0\hat{k}$,\;\;\;$\vec{r}_{14}=10.0\hat{i}+0.0\hat{j}+10.0\hat{k}$,\;\;\;$\vec{r}_{24}=10.0\hat{i}+0.0\hat{j}+0.0\hat{k}$,\;\;\;$\vec{r}_{45}=10.0\hat{i}+10.0\hat{j}+10.0\hat{k}$.

{\tiny 2D-M295:}

$\hat{n}_{13}=0.71\hat{i}-0.71\hat{j}+0.0\hat{k}$,\;\;\;$\hat{n}_{23}=0.58\hat{i}+0.58\hat{j}-0.58\hat{k}$,\;\;\;$\hat{n}_{24}=0.0\hat{i}-0.0\hat{j}+1.0\hat{k}$,\;\;\;$\hat{n}_{35}=0.25\hat{i}-0.67\hat{j}-0.7\hat{k}$,\newline
$\vec{r}_{13}=0.0\hat{i}+0.0\hat{j}+10.0\hat{k}$,\;\;\;$\vec{r}_{14}=10.0\hat{i}+10.0\hat{j}+0.0\hat{k}$,\;\;\;$\vec{r}_{24}=0.0\hat{i}+0.0\hat{j}+0.58\hat{k}$,\;\;\;$\vec{r}_{35}=0.0\hat{i}+10.0\hat{j}+10.0\hat{k}$.

{\tiny 2D-M296:}

$\hat{n}_{13}=0.7\hat{i}-0.01\hat{j}+0.72\hat{k}$,\;\;\;$\hat{n}_{23}=-0.58\hat{i}+0.58\hat{j}+0.57\hat{k}$,\;\;\;$\hat{n}_{24}=0.35\hat{i}+0.66\hat{j}-0.66\hat{k}$,\;\;\;$\hat{n}_{25}=-0.61\hat{i}+0.09\hat{j}-0.79\hat{k}$,\newline
$\vec{r}_{13}=10.0\hat{i}+0.0\hat{j}+10.0\hat{k}$,\;\;\;$\vec{r}_{14}=0.0\hat{i}+10.0\hat{j}+0.0\hat{k}$,\;\;\;$\vec{r}_{24}=10.0\hat{i}+10.0\hat{j}+10.0\hat{k}$,\;\;\;$\vec{r}_{25}=0.0\hat{i}+10.0\hat{j}+0.0\hat{k}$.
