# Supplementary material for: Dimensional synthesis of spatial manipulators for velocity and force transmission for operation around a specified task point
Source: arXiv:2210.04446 source file (2022-10-10)
Supplement: Supplementary file 11 [file classappendix7.tex]

\subsection{Class 7} \label{appendix_five_2_1}
{\tiny 2D-M297:}

$\hat{n}_{14}=-0.0\hat{i}+0.62\hat{j}+0.78\hat{k}$,\;\;\;$\hat{n}_{24}=-0.0\hat{i}+0.3\hat{j}-0.95\hat{k}$,\;\;\;$\hat{n}_{25}=-0.0\hat{i}+0.92\hat{j}-0.4\hat{k}$,\;\;\;$\hat{n}_{34}=0.71\hat{i}+0.23\hat{j}+0.67\hat{k}$,\newline
$\hat{n}_{35}=-0.73\hat{i}+0.34\hat{j}+0.59\hat{k}$,\;\;\;$\vec{r}_{14}=10.0\hat{i}+0.0\hat{j}+0.0\hat{k}$,\;\;\;$\vec{r}_{24}=10.0\hat{i}+0.0\hat{j}+10.0\hat{k}$,\;\;\;$\vec{r}_{25}=0.0\hat{i}+10.0\hat{j}+0.0\hat{k}$,\newline
$\vec{r}_{34}=0.0\hat{i}+10.0\hat{j}+0.0\hat{k}$,\;\;\;$\vec{r}_{35}=10.0\hat{i}+10.0\hat{j}+10.0\hat{k}$.

{\tiny 2D-M298:}

$\hat{n}_{14}=-0.47\hat{i}-0.21\hat{j}+0.86\hat{k}$,\;\;\;$\hat{n}_{24}=0.09\hat{i}-0.59\hat{j}-0.8\hat{k}$,\;\;\;$\hat{n}_{25}=0.78\hat{i}+0.14\hat{j}+0.61\hat{k}$,\;\;\;$\hat{n}_{34}=0.79\hat{i}+0.46\hat{j}-0.39\hat{k}$,\newline
$\hat{n}_{35}=-0.59\hat{i}+0.63\hat{j}-0.51\hat{k}$,\;\;\;$\vec{r}_{14}=10.0\hat{i}+10.0\hat{j}+10.0\hat{k}$,\;\;\;$\vec{r}_{24}=0.0\hat{i}+10.0\hat{j}+10.0\hat{k}$,\;\;\;$\vec{r}_{25}=10.0\hat{i}+0.0\hat{j}+10.0\hat{k}$,\newline
$\vec{r}_{34}=10.0\hat{i}+0.0\hat{j}+0.0\hat{k}$,\;\;\;$\vec{r}_{35}=10.0\hat{i}+10.0\hat{j}+0.0\hat{k}$.

{\tiny 2D-M299:}

$\hat{n}_{14}=0.57\hat{i}+0.67\hat{j}+0.48\hat{k}$,\;\;\;$\hat{n}_{23}=0.58\hat{i}+0.56\hat{j}-0.58\hat{k}$,\;\;\;$\hat{n}_{25}=0.23\hat{i}+0.94\hat{j}-0.23\hat{k}$,\;\;\;$\hat{n}_{34}=0.42\hat{i}-0.8\hat{j}-0.42\hat{k}$,\newline
$\hat{n}_{45}=-0.71\hat{i}-0.0\hat{j}-0.71\hat{k}$,\;\;\;$\vec{r}_{14}=10.0\hat{i}+0.0\hat{j}+0.0\hat{k}$,\;\;\;$\vec{r}_{23}=0.0\hat{i}+10.0\hat{j}+0.0\hat{k}$,\;\;\;$\vec{r}_{25}=10.0\hat{i}+0.0\hat{j}+10.0\hat{k}$,\newline
$\vec{r}_{34}=10.0\hat{i}+10.0\hat{j}+0.0\hat{k}$,\;\;\;$\vec{r}_{45}=5.33\hat{i}+2.14\hat{j}+5.86\hat{k}$.

{\tiny 2D-M300:}

$\hat{n}_{14}=0.77\hat{i}+0.04\hat{j}-0.64\hat{k}$,\;\;\;$\hat{n}_{23}=-0.58\hat{i}-0.56\hat{j}-0.58\hat{k}$,\;\;\;$\hat{n}_{25}=-0.42\hat{i}+0.8\hat{j}-0.42\hat{k}$,\;\;\;$\hat{n}_{34}=-0.23\hat{i}-0.94\hat{j}-0.23\hat{k}$,\newline
$\hat{n}_{45}=0.71\hat{i}+0.0\hat{j}-0.71\hat{k}$,\;\;\;$\vec{r}_{14}=0.0\hat{i}+0.0\hat{j}+0.0\hat{k}$,\;\;\;$\vec{r}_{23}=10.0\hat{i}+0.0\hat{j}+0.0\hat{k}$,\;\;\;$\vec{r}_{25}=0.0\hat{i}+0.0\hat{j}+0.0\hat{k}$,\newline
$\vec{r}_{34}=0.0\hat{i}+10.0\hat{j}+10.0\hat{k}$,\;\;\;$\vec{r}_{45}=4.56\hat{i}+5.47\hat{j}+4.32\hat{k}$.

{\tiny 2D-M301:}

$\hat{n}_{14}=0.13\hat{i}-0.65\hat{j}-0.75\hat{k}$,\;\;\;$\hat{n}_{23}=0.98\hat{i}-0.18\hat{j}-0.08\hat{k}$,\;\;\;$\hat{n}_{25}=-0.19\hat{i}-0.78\hat{j}-0.59\hat{k}$,\;\;\;$\hat{n}_{34}=-0.04\hat{i}-0.59\hat{j}+0.8\hat{k}$,\newline
$\hat{n}_{45}=0.55\hat{i}-0.24\hat{j}+0.8\hat{k}$,\;\;\;$\vec{r}_{14}=10.0\hat{i}+10.0\hat{j}+0.0\hat{k}$,\;\;\;$\vec{r}_{23}=5.39\hat{i}+4.79\hat{j}+5.38\hat{k}$,\;\;\;$\vec{r}_{25}=4.53\hat{i}+5.13\hat{j}+7.95\hat{k}$,\newline
$\vec{r}_{34}=5.37\hat{i}+4.62\hat{j}+5.27\hat{k}$,\;\;\;$\vec{r}_{45}=0.0\hat{i}+10.0\hat{j}+0.0\hat{k}$.

{\tiny 2D-M302:}

$\hat{n}_{14}=-0.6\hat{i}-0.79\hat{j}-0.16\hat{k}$,\;\;\;$\hat{n}_{15}=-0.59\hat{i}-0.79\hat{j}-0.16\hat{k}$,\;\;\;$\hat{n}_{23}=0.71\hat{i}-0.43\hat{j}-0.55\hat{k}$,\;\;\;$\hat{n}_{25}=0.64\hat{i}-0.58\hat{j}+0.5\hat{k}$,\newline
$\hat{n}_{34}=0.45\hat{i}-0.17\hat{j}-0.88\hat{k}$,\;\;\;$\vec{r}_{14}=6.47\hat{i}+3.62\hat{j}+4.11\hat{k}$,\;\;\;$\vec{r}_{15}=0.0\hat{i}+10.0\hat{j}+0.0\hat{k}$,\;\;\;$\vec{r}_{23}=0.0\hat{i}+10.0\hat{j}+10.0\hat{k}$,\newline
$\vec{r}_{25}=0.0\hat{i}+10.0\hat{j}+0.0\hat{k}$,\;\;\;$\vec{r}_{34}=10.0\hat{i}+0.0\hat{j}+0.0\hat{k}$.

{\tiny 2D-M303:}

$\hat{n}_{14}=-0.05\hat{i}-0.76\hat{j}+0.65\hat{k}$,\;\;\;$\hat{n}_{15}=-0.8\hat{i}-0.35\hat{j}-0.49\hat{k}$,\;\;\;$\hat{n}_{23}=0.42\hat{i}-0.91\hat{j}+0.04\hat{k}$,\;\;\;$\hat{n}_{25}=0.78\hat{i}+0.38\hat{j}+0.5\hat{k}$,\newline
$\hat{n}_{34}=-0.5\hat{i}-0.12\hat{j}+0.86\hat{k}$,\;\;\;$\vec{r}_{14}=10.0\hat{i}+0.0\hat{j}+10.0\hat{k}$,\;\;\;$\vec{r}_{15}=10.0\hat{i}+0.0\hat{j}+10.0\hat{k}$,\;\;\;$\vec{r}_{23}=10.0\hat{i}+10.0\hat{j}+0.0\hat{k}$,\newline
$\vec{r}_{25}=4.09\hat{i}+6.24\hat{j}+6.18\hat{k}$,\;\;\;$\vec{r}_{34}=0.0\hat{i}+10.0\hat{j}+10.0\hat{k}$.

{\tiny 2D-M304:}

$\hat{n}_{14}=-0.11\hat{i}+0.76\hat{j}-0.64\hat{k}$,\;\;\;$\hat{n}_{15}=0.11\hat{i}-0.76\hat{j}+0.64\hat{k}$,\;\;\;$\hat{n}_{23}=-0.89\hat{i}+0.22\hat{j}+0.4\hat{k}$,\;\;\;$\hat{n}_{25}=0.49\hat{i}+0.6\hat{j}+0.63\hat{k}$,\newline
$\hat{n}_{34}=0.56\hat{i}-0.49\hat{j}-0.67\hat{k}$,\;\;\;$\vec{r}_{14}=4.93\hat{i}+5.16\hat{j}+4.85\hat{k}$,\;\;\;$\vec{r}_{15}=0.0\hat{i}+10.0\hat{j}+0.0\hat{k}$,\;\;\;$\vec{r}_{23}=0.0\hat{i}+0.0\hat{j}+0.0\hat{k}$,\newline
$\vec{r}_{25}=10.0\hat{i}+0.0\hat{j}+10.0\hat{k}$,\;\;\;$\vec{r}_{34}=10.0\hat{i}+10.0\hat{j}+10.0\hat{k}$.

{\tiny 2D-M305:}

$\hat{n}_{14}=-0.9\hat{i}-0.42\hat{j}-0.11\hat{k}$,\;\;\;$\hat{n}_{15}=0.34\hat{i}-0.6\hat{j}-0.72\hat{k}$,\;\;\;$\hat{n}_{23}=0.63\hat{i}+0.73\hat{j}-0.26\hat{k}$,\;\;\;$\hat{n}_{25}=-0.36\hat{i}+0.57\hat{j}+0.74\hat{k}$,\newline
$\hat{n}_{34}=-0.27\hat{i}+0.69\hat{j}-0.67\hat{k}$,\;\;\;$\vec{r}_{14}=0.0\hat{i}+10.0\hat{j}+10.0\hat{k}$,\;\;\;$\vec{r}_{15}=10.0\hat{i}+10.0\hat{j}+0.0\hat{k}$,\;\;\;$\vec{r}_{23}=10.0\hat{i}+0.0\hat{j}+0.0\hat{k}$,\newline
$\vec{r}_{25}=4.72\hat{i}+4.85\hat{j}+4.83\hat{k}$,\;\;\;$\vec{r}_{34}=10.0\hat{i}+10.0\hat{j}+10.0\hat{k}$.

{\tiny 2D-M306:}

$\hat{n}_{14}=-0.8\hat{i}-0.47\hat{j}-0.37\hat{k}$,\;\;\;$\hat{n}_{15}=0.05\hat{i}-0.66\hat{j}+0.75\hat{k}$,\;\;\;$\hat{n}_{23}=0.0\hat{i}+0.68\hat{j}-0.74\hat{k}$,\;\;\;$\hat{n}_{25}=0.56\hat{i}-0.59\hat{j}-0.57\hat{k}$,\newline
$\hat{n}_{34}=0.95\hat{i}-0.24\hat{j}-0.22\hat{k}$,\;\;\;$\vec{r}_{14}=10.0\hat{i}+0.0\hat{j}+10.0\hat{k}$,\;\;\;$\vec{r}_{15}=10.0\hat{i}+10.0\hat{j}+10.0\hat{k}$,\;\;\;$\vec{r}_{23}=0.0\hat{i}+10.0\hat{j}+0.0\hat{k}$,\newline
$\vec{r}_{25}=10.0\hat{i}+10.0\hat{j}+10.0\hat{k}$,\;\;\;$\vec{r}_{34}=0.0\hat{i}+0.0\hat{j}+0.0\hat{k}$.

{\tiny 2D-M307:}

$\hat{n}_{14}=0.49\hat{i}+0.66\hat{j}-0.57\hat{k}$,\;\;\;$\hat{n}_{15}=-0.04\hat{i}-0.63\hat{j}-0.77\hat{k}$,\;\;\;$\hat{n}_{23}=0.89\hat{i}-0.36\hat{j}+0.26\hat{k}$,\;\;\;$\hat{n}_{25}=0.56\hat{i}-0.66\hat{j}+0.51\hat{k}$,\newline
$\hat{n}_{34}=-0.0\hat{i}+0.63\hat{j}+0.77\hat{k}$,\;\;\;$\vec{r}_{14}=10.0\hat{i}+0.0\hat{j}+0.0\hat{k}$,\;\;\;$\vec{r}_{15}=10.0\hat{i}+0.0\hat{j}+0.0\hat{k}$,\;\;\;$\vec{r}_{23}=0.0\hat{i}+0.0\hat{j}+10.0\hat{k}$,\newline
$\vec{r}_{25}=10.0\hat{i}+10.0\hat{j}+0.0\hat{k}$,\;\;\;$\vec{r}_{34}=0.0\hat{i}+10.0\hat{j}+10.0\hat{k}$.

{\tiny 2D-M308:}

$\hat{n}_{13}=-0.7\hat{i}-0.05\hat{j}-0.72\hat{k}$,\;\;\;$\hat{n}_{14}=-0.56\hat{i}-0.56\hat{j}+0.61\hat{k}$,\;\;\;$\hat{n}_{24}=-0.29\hat{i}-0.9\hat{j}+0.34\hat{k}$,\;\;\;$\hat{n}_{25}=-0.61\hat{i}+0.49\hat{j}+0.63\hat{k}$,\newline
$\hat{n}_{35}=0.73\hat{i}+0.02\hat{j}+0.68\hat{k}$,\;\;\;$\vec{r}_{13}=0.0\hat{i}+10.0\hat{j}+0.0\hat{k}$,\;\;\;$\vec{r}_{14}=10.0\hat{i}+0.0\hat{j}+10.0\hat{k}$,\;\;\;$\vec{r}_{24}=0.0\hat{i}+10.0\hat{j}+0.0\hat{k}$,\newline
$\vec{r}_{25}=0.0\hat{i}+0.0\hat{j}+10.0\hat{k}$,\;\;\;$\vec{r}_{35}=10.0\hat{i}+0.0\hat{j}+10.0\hat{k}$.

{\tiny 2D-M309:}

$\hat{n}_{13}=0.02\hat{i}-0.75\hat{j}+0.66\hat{k}$,\;\;\;$\hat{n}_{14}=0.8\hat{i}+0.4\hat{j}+0.44\hat{k}$,\;\;\;$\hat{n}_{24}=-0.94\hat{i}+0.25\hat{j}+0.21\hat{k}$,\;\;\;$\hat{n}_{25}=0.56\hat{i}-0.61\hat{j}-0.56\hat{k}$,\newline
$\hat{n}_{35}=-0.05\hat{i}-0.69\hat{j}+0.72\hat{k}$,\;\;\;$\vec{r}_{13}=0.0\hat{i}+10.0\hat{j}+0.0\hat{k}$,\;\;\;$\vec{r}_{14}=0.0\hat{i}+10.0\hat{j}+0.0\hat{k}$,\;\;\;$\vec{r}_{24}=10.0\hat{i}+10.0\hat{j}+10.0\hat{k}$,\newline
$\vec{r}_{25}=0.0\hat{i}+0.0\hat{j}+0.0\hat{k}$,\;\;\;$\vec{r}_{35}=10.0\hat{i}+0.0\hat{j}+10.0\hat{k}$.

{\tiny 2D-M310:}

$\hat{n}_{13}=-0.0\hat{i}-0.0\hat{j}-1.0\hat{k}$,\;\;\;$\hat{n}_{14}=-0.57\hat{i}-0.82\hat{j}+0.04\hat{k}$,\;\;\;$\hat{n}_{24}=0.0\hat{i}-0.0\hat{j}-1.0\hat{k}$,\;\;\;$\hat{n}_{25}=-0.83\hat{i}+0.06\hat{j}-0.56\hat{k}$,\newline
$\hat{n}_{35}=-0.8\hat{i}+0.61\hat{j}-0.01\hat{k}$,\;\;\;$\vec{r}_{13}=0.0\hat{i}+10.0\hat{j}+2.36\hat{k}$,\;\;\;$\vec{r}_{14}=0.0\hat{i}+0.0\hat{j}+0.0\hat{k}$,\;\;\;$\vec{r}_{24}=10.0\hat{i}+10.0\hat{j}+2.5\hat{k}$,\newline
$\vec{r}_{25}=0.0\hat{i}+0.0\hat{j}+10.0\hat{k}$,\;\;\;$\vec{r}_{35}=10.0\hat{i}+10.0\hat{j}+0.0\hat{k}$.

{\tiny 2D-M311:}

$\hat{n}_{13}=0.71\hat{i}-0.09\hat{j}-0.7\hat{k}$,\;\;\;$\hat{n}_{14}=-0.48\hat{i}-0.86\hat{j}-0.2\hat{k}$,\;\;\;$\hat{n}_{24}=-0.91\hat{i}-0.42\hat{j}+0.03\hat{k}$,\;\;\;$\hat{n}_{25}=0.47\hat{i}-0.89\hat{j}-0.02\hat{k}$,\newline
$\hat{n}_{35}=-0.0\hat{i}-0.0\hat{j}-1.0\hat{k}$,\;\;\;$\vec{r}_{13}=10.0\hat{i}+0.0\hat{j}+0.0\hat{k}$,\;\;\;$\vec{r}_{14}=5.44\hat{i}+1.75\hat{j}+1.53\hat{k}$,\;\;\;$\vec{r}_{24}=3.06\hat{i}+6.64\hat{j}+4.6\hat{k}$,\newline
$\vec{r}_{25}=4.99\hat{i}+1.52\hat{j}+1.51\hat{k}$,\;\;\;$\vec{r}_{35}=10.0\hat{i}+10.0\hat{j}+7.73\hat{k}$.

{\tiny 2D-M312:}

$\hat{n}_{13}=-0.54\hat{i}+0.76\hat{j}+0.37\hat{k}$,\;\;\;$\hat{n}_{14}=0.44\hat{i}+0.54\hat{j}+0.72\hat{k}$,\;\;\;$\hat{n}_{23}=0.14\hat{i}+0.63\hat{j}-0.76\hat{k}$,\;\;\;$\hat{n}_{25}=-0.34\hat{i}-0.72\hat{j}+0.61\hat{k}$,\newline
$\hat{n}_{45}=-0.88\hat{i}+0.47\hat{j}+0.12\hat{k}$,\;\;\;$\vec{r}_{13}=10.0\hat{i}+10.0\hat{j}+0.0\hat{k}$,\;\;\;$\vec{r}_{14}=10.0\hat{i}+0.0\hat{j}+10.0\hat{k}$,\;\;\;$\vec{r}_{23}=10.0\hat{i}+10.0\hat{j}+10.0\hat{k}$,\newline
$\vec{r}_{25}=0.0\hat{i}+0.0\hat{j}+0.0\hat{k}$,\;\;\;$\vec{r}_{45}=0.0\hat{i}+0.0\hat{j}+0.0\hat{k}$.

{\tiny 2D-M313:}

$\hat{n}_{13}=-0.79\hat{i}+0.17\hat{j}-0.59\hat{k}$,\;\;\;$\hat{n}_{14}=-0.42\hat{i}+0.66\hat{j}+0.62\hat{k}$,\;\;\;$\hat{n}_{23}=-0.32\hat{i}+0.5\hat{j}-0.8\hat{k}$,\;\;\;$\hat{n}_{25}=0.84\hat{i}-0.0\hat{j}-0.54\hat{k}$,\newline
$\hat{n}_{45}=0.73\hat{i}+0.68\hat{j}-0.09\hat{k}$,\;\;\;$\vec{r}_{13}=0.0\hat{i}+0.0\hat{j}+10.0\hat{k}$,\;\;\;$\vec{r}_{14}=0.0\hat{i}+0.0\hat{j}+10.0\hat{k}$,\;\;\;$\vec{r}_{23}=10.0\hat{i}+10.0\hat{j}+10.0\hat{k}$,\newline
$\vec{r}_{25}=10.0\hat{i}+0.0\hat{j}+0.0\hat{k}$,\;\;\;$\vec{r}_{45}=0.0\hat{i}+10.0\hat{j}+0.0\hat{k}$.

{\tiny 2D-M314:}

$\hat{n}_{13}=0.9\hat{i}-0.42\hat{j}+0.06\hat{k}$,\;\;\;$\hat{n}_{14}=-0.0\hat{i}+0.0\hat{j}-1.0\hat{k}$,\;\;\;$\hat{n}_{23}=-0.83\hat{i}-0.54\hat{j}+0.11\hat{k}$,\;\;\;$\hat{n}_{25}=0.51\hat{i}-0.85\hat{j}+0.09\hat{k}$,\newline
$\hat{n}_{45}=-0.0\hat{i}+0.34\hat{j}+0.94\hat{k}$,\;\;\;$\vec{r}_{13}=0.0\hat{i}+0.0\hat{j}+10.0\hat{k}$,\;\;\;$\vec{r}_{14}=10.0\hat{i}+10.0\hat{j}+2.38\hat{k}$,\;\;\;$\vec{r}_{23}=10.0\hat{i}+0.0\hat{j}+0.0\hat{k}$,\newline
$\vec{r}_{25}=10.0\hat{i}+10.0\hat{j}+0.0\hat{k}$,\;\;\;$\vec{r}_{45}=0.0\hat{i}+0.0\hat{j}+10.0\hat{k}$.

{\tiny 2D-M315:}

$\hat{n}_{13}=0.0\hat{i}+0.61\hat{j}-0.79\hat{k}$,\;\;\;$\hat{n}_{14}=-0.41\hat{i}-0.02\hat{j}-0.91\hat{k}$,\;\;\;$\hat{n}_{23}=-0.26\hat{i}-0.67\hat{j}+0.69\hat{k}$,\;\;\;$\hat{n}_{24}=-0.92\hat{i}-0.37\hat{j}-0.1\hat{k}$,\newline
$\hat{n}_{35}=0.0\hat{i}+0.83\hat{j}-0.56\hat{k}$,\;\;\;$\vec{r}_{13}=10.0\hat{i}+10.0\hat{j}+10.0\hat{k}$,\;\;\;$\vec{r}_{14}=4.86\hat{i}+5.62\hat{j}+6.15\hat{k}$,\;\;\;$\vec{r}_{23}=5.03\hat{i}+4.98\hat{j}+5.21\hat{k}$,\newline
$\vec{r}_{24}=5.31\hat{i}+5.28\hat{j}+4.75\hat{k}$,\;\;\;$\vec{r}_{35}=0.0\hat{i}+10.0\hat{j}+0.0\hat{k}$.

{\tiny 2D-M316:}

$\hat{n}_{13}=-0.83\hat{i}-0.08\hat{j}+0.55\hat{k}$,\;\;\;$\hat{n}_{14}=-0.31\hat{i}+0.77\hat{j}+0.56\hat{k}$,\;\;\;$\hat{n}_{23}=0.93\hat{i}+0.36\hat{j}+0.05\hat{k}$,\;\;\;$\hat{n}_{24}=0.28\hat{i}-0.5\hat{j}+0.82\hat{k}$,\newline
$\hat{n}_{25}=-0.51\hat{i}+0.74\hat{j}-0.43\hat{k}$,\;\;\;$\vec{r}_{13}=0.0\hat{i}+0.0\hat{j}+0.0\hat{k}$,\;\;\;$\vec{r}_{14}=0.0\hat{i}+10.0\hat{j}+10.0\hat{k}$,\;\;\;$\vec{r}_{23}=10.0\hat{i}+0.0\hat{j}+10.0\hat{k}$,\newline
$\vec{r}_{24}=0.0\hat{i}+10.0\hat{j}+0.0\hat{k}$,\;\;\;$\vec{r}_{25}=10.0\hat{i}+10.0\hat{j}+10.0\hat{k}$.

{\tiny 2D-M317:}

$\hat{n}_{13}=-0.6\hat{i}+0.68\hat{j}+0.42\hat{k}$,\;\;\;$\hat{n}_{14}=0.18\hat{i}+0.62\hat{j}-0.76\hat{k}$,\;\;\;$\hat{n}_{24}=0.41\hat{i}+0.5\hat{j}-0.76\hat{k}$,\;\;\;$\hat{n}_{25}=0.91\hat{i}-0.38\hat{j}+0.17\hat{k}$,\newline
$\hat{n}_{35}=-0.74\hat{i}-0.37\hat{j}-0.56\hat{k}$,\;\;\;$\vec{r}_{13}=10.0\hat{i}+10.0\hat{j}+10.0\hat{k}$,\;\;\;$\vec{r}_{14}=0.0\hat{i}+0.0\hat{j}+0.0\hat{k}$,\;\;\;$\vec{r}_{24}=10.0\hat{i}+10.0\hat{j}+10.0\hat{k}$,\newline
$\vec{r}_{25}=10.0\hat{i}+10.0\hat{j}+0.0\hat{k}$,\;\;\;$\vec{r}_{35}=10.0\hat{i}+0.0\hat{j}+10.0\hat{k}$.

{\tiny 2D-M318:}

$\hat{n}_{13}=0.84\hat{i}-0.16\hat{j}-0.52\hat{k}$,\;\;\;$\hat{n}_{14}=0.55\hat{i}+0.26\hat{j}+0.79\hat{k}$,\;\;\;$\hat{n}_{24}=-0.0\hat{i}+0.94\hat{j}+0.35\hat{k}$,\;\;\;$\hat{n}_{25}=0.0\hat{i}+0.93\hat{j}-0.36\hat{k}$,\newline
$\hat{n}_{35}=0.78\hat{i}+0.04\hat{j}-0.62\hat{k}$,\;\;\;$\vec{r}_{13}=10.0\hat{i}+0.0\hat{j}+0.0\hat{k}$,\;\;\;$\vec{r}_{14}=0.0\hat{i}+0.0\hat{j}+10.0\hat{k}$,\;\;\;$\vec{r}_{24}=10.0\hat{i}+0.0\hat{j}+0.0\hat{k}$,\newline
$\vec{r}_{25}=10.0\hat{i}+10.0\hat{j}+10.0\hat{k}$,\;\;\;$\vec{r}_{35}=0.0\hat{i}+10.0\hat{j}+10.0\hat{k}$.

{\tiny 2D-M319:}

$\hat{n}_{13}=0.85\hat{i}+0.13\hat{j}-0.51\hat{k}$,\;\;\;$\hat{n}_{14}=0.51\hat{i}-0.51\hat{j}+0.69\hat{k}$,\;\;\;$\hat{n}_{24}=0.13\hat{i}+0.87\hat{j}+0.47\hat{k}$,\;\;\;$\hat{n}_{25}=-0.3\hat{i}-0.53\hat{j}-0.79\hat{k}$,\newline
$\hat{n}_{35}=-0.88\hat{i}-0.4\hat{j}+0.26\hat{k}$,\;\;\;$\vec{r}_{13}=0.0\hat{i}+0.0\hat{j}+0.0\hat{k}$,\;\;\;$\vec{r}_{14}=0.0\hat{i}+0.0\hat{j}+0.0\hat{k}$,\;\;\;$\vec{r}_{24}=0.0\hat{i}+10.0\hat{j}+10.0\hat{k}$,\newline
$\vec{r}_{25}=10.0\hat{i}+0.0\hat{j}+0.0\hat{k}$,\;\;\;$\vec{r}_{35}=10.0\hat{i}+0.0\hat{j}+10.0\hat{k}$.
