# Supplementary material for: Dimensional synthesis of spatial manipulators for velocity and force transmission for operation around a specified task point
Source: arXiv:2210.04446 source file (2022-10-10)
Supplement: Supplementary file 12 [file classappendix8.tex]

\subsection{Class 8} \label{appendix_five_2_1}
{\tiny 2D-M320:}

$\hat{n}_{14}=-0.2\hat{i}+0.68\hat{j}-0.71\hat{k}$,\;\;\;$\hat{n}_{24}=-0.35\hat{i}+0.47\hat{j}-0.81\hat{k}$,\;\;\;$\hat{n}_{25}=0.58\hat{i}-0.58\hat{j}-0.58\hat{k}$,\;\;\;$\hat{n}_{34}=-0.16\hat{i}+0.61\hat{j}-0.77\hat{k}$,\newline
$\vec{r}_{14}=10.0\hat{i}+10.0\hat{j}+10.0\hat{k}$,\;\;\;$\vec{r}_{34}=10.0\hat{i}+0.0\hat{j}+10.0\hat{k}$,\;\;\;$\vec{r}_{35}=0.0\hat{i}+10.0\hat{j}+0.0\hat{k}$.

{\tiny 2D-M321:}

$\hat{n}_{14}=0.63\hat{i}+0.7\hat{j}+0.33\hat{k}$,\;\;\;$\hat{n}_{24}=0.78\hat{i}+0.6\hat{j}+0.18\hat{k}$,\;\;\;$\hat{n}_{25}=-0.58\hat{i}+0.58\hat{j}+0.58\hat{k}$,\;\;\;$\hat{n}_{35}=-0.37\hat{i}+0.45\hat{j}-0.82\hat{k}$,\newline
$\vec{r}_{14}=0.0\hat{i}+10.0\hat{j}+0.0\hat{k}$,\;\;\;$\vec{r}_{34}=10.0\hat{i}+0.0\hat{j}+10.0\hat{k}$,\;\;\;$\vec{r}_{35}=0.0\hat{i}+10.0\hat{j}+0.0\hat{k}$.

{\tiny 2D-M322:}

$\hat{n}_{14}=0.0\hat{i}+0.71\hat{j}-0.7\hat{k}$,\;\;\;$\hat{n}_{24}=0.0\hat{i}+0.7\hat{j}-0.71\hat{k}$,\;\;\;$\hat{n}_{25}=-0.22\hat{i}+0.64\hat{j}+0.73\hat{k}$,\;\;\;$\hat{n}_{34}=0.52\hat{i}-0.51\hat{j}+0.69\hat{k}$,\newline
$\vec{r}_{14}=10.0\hat{i}+10.0\hat{j}+10.0\hat{k}$,\;\;\;$\vec{r}_{25}=10.0\hat{i}+0.0\hat{j}+0.0\hat{k}$,\;\;\;$\vec{r}_{35}=0.0\hat{i}+10.0\hat{j}+10.0\hat{k}$.

{\tiny 2D-M323:}

$\hat{n}_{14}=0.0\hat{i}+0.68\hat{j}-0.74\hat{k}$,\;\;\;$\hat{n}_{24}=0.0\hat{i}+0.72\hat{j}-0.69\hat{k}$,\;\;\;$\hat{n}_{25}=-0.78\hat{i}-0.61\hat{j}-0.14\hat{k}$,\;\;\;$\hat{n}_{35}=-0.37\hat{i}+0.74\hat{j}-0.56\hat{k}$,\newline
$\vec{r}_{14}=0.0\hat{i}+10.0\hat{j}+0.0\hat{k}$,\;\;\;$\vec{r}_{25}=0.0\hat{i}+10.0\hat{j}+10.0\hat{k}$,\;\;\;$\vec{r}_{34}=10.0\hat{i}+0.0\hat{j}+0.0\hat{k}$.

{\tiny 2D-M324:}

$\hat{n}_{14}=-0.17\hat{i}-0.47\hat{j}-0.87\hat{k}$,\;\;\;$\hat{n}_{24}=0.31\hat{i}+0.57\hat{j}+0.76\hat{k}$,\;\;\;$\hat{n}_{34}=0.95\hat{i}-0.17\hat{j}-0.26\hat{k}$,\;\;\;$\hat{n}_{35}=-0.0\hat{i}+0.71\hat{j}+0.71\hat{k}$,\newline
$\vec{r}_{14}=10.0\hat{i}+10.0\hat{j}+0.0\hat{k}$,\;\;\;$\vec{r}_{25}=0.0\hat{i}+0.0\hat{j}+0.0\hat{k}$,\;\;\;$\vec{r}_{34}=10.0\hat{i}+10.0\hat{j}+10.0\hat{k}$.

{\tiny 2D-M325:}

$\hat{n}_{14}=0.0\hat{i}+0.63\hat{j}-0.77\hat{k}$,\;\;\;$\hat{n}_{24}=-0.16\hat{i}-0.89\hat{j}-0.42\hat{k}$,\;\;\;$\hat{n}_{25}=-0.0\hat{i}+0.0\hat{j}+1.0\hat{k}$,\;\;\;$\hat{n}_{35}=0.58\hat{i}-0.42\hat{j}+0.7\hat{k}$,\newline
$\vec{r}_{14}=10.0\hat{i}+10.0\hat{j}+10.0\hat{k}$,\;\;\;$\vec{r}_{24}=10.0\hat{i}+0.0\hat{j}+0.0\hat{k}$,\;\;\;$\vec{r}_{34}=0.0\hat{i}+10.0\hat{j}+10.0\hat{k}$.

{\tiny 2D-M326:}

$\hat{n}_{14}=-0.04\hat{i}+0.56\hat{j}-0.82\hat{k}$,\;\;\;$\hat{n}_{23}=-0.0\hat{i}+0.71\hat{j}-0.71\hat{k}$,\;\;\;$\hat{n}_{25}=0.58\hat{i}+0.58\hat{j}+0.58\hat{k}$,\;\;\;$\hat{n}_{34}=0.82\hat{i}-0.41\hat{j}-0.41\hat{k}$,\newline
$\vec{r}_{14}=10.0\hat{i}+0.0\hat{j}+10.0\hat{k}$,\;\;\;$\vec{r}_{34}=0.0\hat{i}+0.0\hat{j}+0.0\hat{k}$,\;\;\;$\vec{r}_{45}=10.0\hat{i}+10.0\hat{j}+10.0\hat{k}$.

{\tiny 2D-M327:}

$\hat{n}_{14}=-0.0\hat{i}+0.47\hat{j}-0.88\hat{k}$,\;\;\;$\hat{n}_{23}=0.29\hat{i}+0.47\hat{j}+0.84\hat{k}$,\;\;\;$\hat{n}_{25}=0.58\hat{i}+0.61\hat{j}-0.54\hat{k}$,\;\;\;$\hat{n}_{45}=-0.0\hat{i}+0.66\hat{j}+0.75\hat{k}$,\newline
$\vec{r}_{14}=10.0\hat{i}+10.0\hat{j}+10.0\hat{k}$,\;\;\;$\vec{r}_{34}=0.0\hat{i}+0.0\hat{j}+10.0\hat{k}$,\;\;\;$\vec{r}_{45}=10.0\hat{i}+10.0\hat{j}+0.0\hat{k}$.

{\tiny 2D-M328:}

$\hat{n}_{14}=0.0\hat{i}+0.0\hat{j}+1.0\hat{k}$,\;\;\;$\hat{n}_{23}=0.0\hat{i}+0.68\hat{j}-0.73\hat{k}$,\;\;\;$\hat{n}_{25}=-0.93\hat{i}-0.33\hat{j}-0.15\hat{k}$,\;\;\;$\hat{n}_{34}=0.0\hat{i}+0.73\hat{j}+0.68\hat{k}$,\newline
$\vec{r}_{14}=10.0\hat{i}+0.0\hat{j}+4.15\hat{k}$,\;\;\;$\vec{r}_{25}=10.0\hat{i}+0.0\hat{j}+10.0\hat{k}$,\;\;\;$\vec{r}_{45}=0.0\hat{i}+10.0\hat{j}+0.0\hat{k}$.

{\tiny 2D-M329:}

$\hat{n}_{14}=-0.45\hat{i}-0.89\hat{j}+0.0\hat{k}$,\;\;\;$\hat{n}_{23}=-0.58\hat{i}+0.58\hat{j}-0.58\hat{k}$,\;\;\;$\hat{n}_{25}=0.55\hat{i}+0.8\hat{j}+0.25\hat{k}$,\;\;\;$\hat{n}_{45}=0.58\hat{i}-0.58\hat{j}+0.58\hat{k}$,\newline
$\vec{r}_{14}=0.0\hat{i}+10.0\hat{j}+10.0\hat{k}$,\;\;\;$\vec{r}_{25}=0.0\hat{i}+10.0\hat{j}+10.0\hat{k}$,\;\;\;$\vec{r}_{34}=10.0\hat{i}+0.0\hat{j}+0.0\hat{k}$.

{\tiny 2D-M330:}

$\hat{n}_{14}=0.37\hat{i}-0.39\hat{j}+0.84\hat{k}$,\;\;\;$\hat{n}_{23}=0.0\hat{i}-0.0\hat{j}-1.0\hat{k}$,\;\;\;$\hat{n}_{34}=-0.67\hat{i}+0.67\hat{j}+0.33\hat{k}$,\;\;\;$\hat{n}_{45}=-0.34\hat{i}+0.34\hat{j}-0.88\hat{k}$,\newline
$\vec{r}_{14}=10.0\hat{i}+0.0\hat{j}+10.0\hat{k}$,\;\;\;$\vec{r}_{25}=0.0\hat{i}+10.0\hat{j}+0.0\hat{k}$,\;\;\;$\vec{r}_{45}=10.0\hat{i}+0.0\hat{j}+10.0\hat{k}$.

{\tiny 2D-M331:}

$\hat{n}_{14}=0.9\hat{i}+0.25\hat{j}+0.37\hat{k}$,\;\;\;$\hat{n}_{23}=0.58\hat{i}+0.58\hat{j}+0.58\hat{k}$,\;\;\;$\hat{n}_{34}=0.0\hat{i}+0.71\hat{j}-0.71\hat{k}$,\;\;\;$\hat{n}_{45}=-0.58\hat{i}-0.58\hat{j}-0.58\hat{k}$,\newline
$\vec{r}_{14}=10.0\hat{i}+0.0\hat{j}+10.0\hat{k}$,\;\;\;$\vec{r}_{25}=10.0\hat{i}+10.0\hat{j}+10.0\hat{k}$,\;\;\;$\vec{r}_{34}=0.0\hat{i}+0.0\hat{j}+0.0\hat{k}$.

{\tiny 2D-M332:}

$\hat{n}_{14}=-0.0\hat{i}+0.56\hat{j}+0.83\hat{k}$,\;\;\;$\hat{n}_{23}=-0.78\hat{i}-0.14\hat{j}-0.61\hat{k}$,\;\;\;$\hat{n}_{25}=-0.0\hat{i}+0.87\hat{j}-0.5\hat{k}$,\;\;\;$\hat{n}_{34}=0.58\hat{i}-0.52\hat{j}-0.63\hat{k}$,\newline
$\vec{r}_{14}=10.0\hat{i}+10.0\hat{j}+0.0\hat{k}$,\;\;\;$\vec{r}_{23}=0.0\hat{i}+10.0\hat{j}+0.0\hat{k}$,\;\;\;$\vec{r}_{45}=10.0\hat{i}+0.0\hat{j}+10.0\hat{k}$.

{\tiny 2D-M333:}

$\hat{n}_{14}=-0.79\hat{i}+0.28\hat{j}-0.55\hat{k}$,\;\;\;$\hat{n}_{23}=-0.95\hat{i}+0.21\hat{j}-0.21\hat{k}$,\;\;\;$\hat{n}_{25}=-0.0\hat{i}+0.71\hat{j}-0.71\hat{k}$,\;\;\;$\hat{n}_{45}=-0.0\hat{i}+0.71\hat{j}-0.71\hat{k}$,\newline
$\vec{r}_{14}=10.0\hat{i}+10.0\hat{j}+0.0\hat{k}$,\;\;\;$\vec{r}_{23}=10.0\hat{i}+10.0\hat{j}+0.0\hat{k}$,\;\;\;$\vec{r}_{34}=0.0\hat{i}+0.0\hat{j}+10.0\hat{k}$.

{\tiny 2D-M334:}

$\hat{n}_{14}=0.36\hat{i}+0.32\hat{j}-0.88\hat{k}$,\;\;\;$\hat{n}_{23}=-0.26\hat{i}+0.8\hat{j}+0.54\hat{k}$,\;\;\;$\hat{n}_{34}=0.58\hat{i}+0.58\hat{j}-0.58\hat{k}$,\;\;\;$\hat{n}_{45}=-0.58\hat{i}-0.58\hat{j}+0.58\hat{k}$,\newline
$\vec{r}_{14}=10.0\hat{i}+10.0\hat{j}+10.0\hat{k}$,\;\;\;$\vec{r}_{23}=0.0\hat{i}+0.0\hat{j}+10.0\hat{k}$,\;\;\;$\vec{r}_{25}=10.0\hat{i}+10.0\hat{j}+0.0\hat{k}$.

{\tiny 2D-M335:}

$\hat{n}_{14}=-0.79\hat{i}+0.29\hat{j}+0.54\hat{k}$,\;\;\;$\hat{n}_{25}=0.0\hat{i}+0.71\hat{j}+0.7\hat{k}$,\;\;\;$\hat{n}_{34}=-0.58\hat{i}+0.58\hat{j}-0.58\hat{k}$,\;\;\;$\hat{n}_{45}=-0.0\hat{i}-0.71\hat{j}-0.7\hat{k}$,\newline
$\vec{r}_{14}=10.0\hat{i}+10.0\hat{j}+10.0\hat{k}$,\;\;\;$\vec{r}_{23}=0.0\hat{i}+10.0\hat{j}+10.0\hat{k}$,\;\;\;$\vec{r}_{45}=10.0\hat{i}+0.0\hat{j}+0.0\hat{k}$.

{\tiny 2D-M336:}

$\hat{n}_{14}=-0.81\hat{i}+0.38\hat{j}-0.44\hat{k}$,\;\;\;$\hat{n}_{25}=-0.58\hat{i}+0.58\hat{j}-0.58\hat{k}$,\;\;\;$\hat{n}_{34}=-0.01\hat{i}+0.7\hat{j}+0.71\hat{k}$,\;\;\;$\hat{n}_{45}=0.58\hat{i}-0.58\hat{j}+0.58\hat{k}$,\newline
$\vec{r}_{14}=10.0\hat{i}+10.0\hat{j}+0.0\hat{k}$,\;\;\;$\vec{r}_{23}=10.0\hat{i}+0.0\hat{j}+0.0\hat{k}$,\;\;\;$\vec{r}_{34}=0.0\hat{i}+10.0\hat{j}+10.0\hat{k}$.

{\tiny 2D-M337:}

$\hat{n}_{14}=-0.68\hat{i}-0.53\hat{j}-0.5\hat{k}$,\;\;\;$\hat{n}_{25}=0.57\hat{i}+0.23\hat{j}-0.79\hat{k}$,\;\;\;$\hat{n}_{34}=-0.58\hat{i}-0.58\hat{j}-0.58\hat{k}$,\;\;\;$\hat{n}_{45}=-0.58\hat{i}-0.58\hat{j}-0.58\hat{k}$,\newline
$\vec{r}_{14}=0.0\hat{i}+10.0\hat{j}+0.0\hat{k}$,\;\;\;$\vec{r}_{23}=10.0\hat{i}+10.0\hat{j}+10.0\hat{k}$,\;\;\;$\vec{r}_{25}=0.0\hat{i}+0.0\hat{j}+0.0\hat{k}$.

{\tiny 2D-M338:}

$\hat{n}_{14}=0.0\hat{i}+0.71\hat{j}+0.71\hat{k}$,\;\;\;$\hat{n}_{15}=0.53\hat{i}-0.27\hat{j}-0.8\hat{k}$,\;\;\;$\hat{n}_{23}=-0.0\hat{i}+0.71\hat{j}+0.71\hat{k}$,\;\;\;$\hat{n}_{25}=0.58\hat{i}-0.58\hat{j}+0.58\hat{k}$,\newline
$\vec{r}_{14}=10.0\hat{i}+0.0\hat{j}+0.0\hat{k}$,\;\;\;$\vec{r}_{15}=10.0\hat{i}+0.0\hat{j}+0.0\hat{k}$,\;\;\;$\vec{r}_{34}=0.0\hat{i}+10.0\hat{j}+10.0\hat{k}$.

{\tiny 2D-M339:}

$\hat{n}_{14}=0.81\hat{i}-0.29\hat{j}+0.52\hat{k}$,\;\;\;$\hat{n}_{15}=0.82\hat{i}-0.41\hat{j}+0.41\hat{k}$,\;\;\;$\hat{n}_{23}=-0.81\hat{i}+0.29\hat{j}-0.52\hat{k}$,\;\;\;$\hat{n}_{34}=0.58\hat{i}+0.58\hat{j}-0.58\hat{k}$,\newline
$\vec{r}_{14}=0.0\hat{i}+0.0\hat{j}+10.0\hat{k}$,\;\;\;$\vec{r}_{15}=0.0\hat{i}+0.0\hat{j}+10.0\hat{k}$,\;\;\;$\vec{r}_{25}=10.0\hat{i}+10.0\hat{j}+0.0\hat{k}$.

{\tiny 2D-M340:}

$\hat{n}_{14}=-0.0\hat{i}+0.48\hat{j}+0.87\hat{k}$,\;\;\;$\hat{n}_{15}=-0.74\hat{i}+0.67\hat{j}-0.04\hat{k}$,\;\;\;$\hat{n}_{25}=0.0\hat{i}+0.0\hat{j}-1.0\hat{k}$,\;\;\;$\hat{n}_{34}=-0.63\hat{i}-0.78\hat{j}+0.0\hat{k}$,\newline
$\vec{r}_{14}=10.0\hat{i}+10.0\hat{j}+0.0\hat{k}$,\;\;\;$\vec{r}_{15}=10.0\hat{i}+10.0\hat{j}+10.0\hat{k}$,\;\;\;$\vec{r}_{23}=0.0\hat{i}+0.0\hat{j}+10.0\hat{k}$.

{\tiny 2D-M341:}

$\hat{n}_{14}=0.12\hat{i}+0.81\hat{j}+0.58\hat{k}$,\;\;\;$\hat{n}_{23}=0.0\hat{i}+0.71\hat{j}+0.71\hat{k}$,\;\;\;$\hat{n}_{25}=-0.58\hat{i}-0.58\hat{j}+0.58\hat{k}$,\;\;\;$\hat{n}_{34}=0.82\hat{i}-0.41\hat{j}+0.41\hat{k}$,\newline
$\vec{r}_{14}=5.93\hat{i}+3.77\hat{j}+5.0\hat{k}$,\;\;\;$\vec{r}_{15}=0.0\hat{i}+0.0\hat{j}+10.0\hat{k}$,\;\;\;$\vec{r}_{34}=10.0\hat{i}+10.0\hat{j}+0.0\hat{k}$.

{\tiny 2D-M342:}

$\hat{n}_{14}=0.91\hat{i}+0.32\hat{j}-0.28\hat{k}$,\;\;\;$\hat{n}_{23}=-0.82\hat{i}-0.43\hat{j}+0.38\hat{k}$,\;\;\;$\hat{n}_{25}=0.0\hat{i}+0.66\hat{j}+0.75\hat{k}$,\;\;\;$\hat{n}_{34}=0.58\hat{i}-0.61\hat{j}+0.54\hat{k}$,\newline
$\vec{r}_{14}=4.11\hat{i}+7.58\hat{j}+7.9\hat{k}$,\;\;\;$\vec{r}_{15}=10.0\hat{i}+0.0\hat{j}+0.0\hat{k}$,\;\;\;$\vec{r}_{25}=0.0\hat{i}+10.0\hat{j}+10.0\hat{k}$.

{\tiny 2D-M343:}

$\hat{n}_{14}=0.0\hat{i}+0.0\hat{j}+1.0\hat{k}$,\;\;\;$\hat{n}_{23}=0.85\hat{i}-0.47\hat{j}-0.25\hat{k}$,\;\;\;$\hat{n}_{25}=0.49\hat{i}+0.87\hat{j}+0.0\hat{k}$,\;\;\;$\hat{n}_{34}=-0.0\hat{i}+0.0\hat{j}-1.0\hat{k}$,\newline
$\vec{r}_{14}=0.42\hat{i}+5.85\hat{j}+6.72\hat{k}$,\;\;\;$\vec{r}_{15}=10.0\hat{i}+10.0\hat{j}+10.0\hat{k}$,\;\;\;$\vec{r}_{23}=10.0\hat{i}+0.0\hat{j}+0.0\hat{k}$.

{\tiny 2D-M344:}

$\hat{n}_{14}=-0.1\hat{i}+0.5\hat{j}-0.86\hat{k}$,\;\;\;$\hat{n}_{24}=0.0\hat{i}+0.0\hat{j}+1.0\hat{k}$,\;\;\;$\hat{n}_{25}=0.64\hat{i}-0.33\hat{j}-0.69\hat{k}$,\;\;\;$\hat{n}_{34}=0.0\hat{i}+0.97\hat{j}-0.22\hat{k}$,\newline
$\vec{r}_{24}=0.0\hat{i}+10.0\hat{j}+0.14\hat{k}$,\;\;\;$\vec{r}_{34}=10.0\hat{i}+0.0\hat{j}+10.0\hat{k}$,\;\;\;$\vec{r}_{35}=10.0\hat{i}+10.0\hat{j}+0.0\hat{k}$.

{\tiny 2D-M345:}

$\hat{n}_{14}=0.0\hat{i}+0.03\hat{j}+1.0\hat{k}$,\;\;\;$\hat{n}_{24}=-0.25\hat{i}+0.47\hat{j}+0.85\hat{k}$,\;\;\;$\hat{n}_{25}=-0.58\hat{i}+0.58\hat{j}-0.58\hat{k}$,\;\;\;$\hat{n}_{35}=-0.64\hat{i}+0.13\hat{j}+0.76\hat{k}$,\newline
$\vec{r}_{24}=10.0\hat{i}+0.0\hat{j}+0.0\hat{k}$,\;\;\;$\vec{r}_{34}=10.0\hat{i}+0.0\hat{j}+0.0\hat{k}$,\;\;\;$\vec{r}_{35}=0.0\hat{i}+10.0\hat{j}+10.0\hat{k}$.

{\tiny 2D-M346:}

$\hat{n}_{14}=0.1\hat{i}-0.09\hat{j}+0.99\hat{k}$,\;\;\;$\hat{n}_{24}=-0.0\hat{i}+0.0\hat{j}+1.0\hat{k}$,\;\;\;$\hat{n}_{25}=-0.89\hat{i}+0.44\hat{j}+0.1\hat{k}$,\;\;\;$\hat{n}_{34}=-0.0\hat{i}+0.77\hat{j}+0.64\hat{k}$,\newline
$\vec{r}_{24}=0.0\hat{i}+10.0\hat{j}+5.28\hat{k}$,\;\;\;$\vec{r}_{25}=0.0\hat{i}+0.0\hat{j}+0.0\hat{k}$,\;\;\;$\vec{r}_{35}=10.0\hat{i}+10.0\hat{j}+10.0\hat{k}$.

{\tiny 2D-M347:}

$\hat{n}_{14}=-0.0\hat{i}-0.0\hat{j}+1.0\hat{k}$,\;\;\;$\hat{n}_{24}=0.31\hat{i}+0.36\hat{j}-0.88\hat{k}$,\;\;\;$\hat{n}_{25}=0.81\hat{i}-0.47\hat{j}-0.35\hat{k}$,\;\;\;$\hat{n}_{35}=0.58\hat{i}+0.58\hat{j}+0.58\hat{k}$,\newline
$\vec{r}_{24}=10.0\hat{i}+10.0\hat{j}+10.0\hat{k}$,\;\;\;$\vec{r}_{25}=0.0\hat{i}+0.0\hat{j}+0.0\hat{k}$,\;\;\;$\vec{r}_{34}=10.0\hat{i}+10.0\hat{j}+10.0\hat{k}$.

{\tiny 2D-M348:}

$\hat{n}_{14}=0.32\hat{i}-0.67\hat{j}-0.66\hat{k}$,\;\;\;$\hat{n}_{24}=0.82\hat{i}+0.42\hat{j}+0.39\hat{k}$,\;\;\;$\hat{n}_{34}=0.58\hat{i}-0.58\hat{j}-0.58\hat{k}$,\;\;\;$\hat{n}_{35}=-0.02\hat{i}+0.7\hat{j}-0.72\hat{k}$,\newline
$\vec{r}_{24}=10.0\hat{i}+0.0\hat{j}+10.0\hat{k}$,\;\;\;$\vec{r}_{25}=0.0\hat{i}+10.0\hat{j}+0.0\hat{k}$,\;\;\;$\vec{r}_{35}=10.0\hat{i}+0.0\hat{j}+10.0\hat{k}$.

{\tiny 2D-M349:}

$\hat{n}_{14}=0.52\hat{i}+0.01\hat{j}-0.85\hat{k}$,\;\;\;$\hat{n}_{24}=-0.71\hat{i}+0.06\hat{j}-0.71\hat{k}$,\;\;\;$\hat{n}_{34}=0.25\hat{i}-0.67\hat{j}-0.7\hat{k}$,\;\;\;$\hat{n}_{35}=-0.03\hat{i}+0.71\hat{j}-0.7\hat{k}$,\newline
$\vec{r}_{24}=0.0\hat{i}+10.0\hat{j}+0.0\hat{k}$,\;\;\;$\vec{r}_{25}=0.0\hat{i}+0.0\hat{j}+10.0\hat{k}$,\;\;\;$\vec{r}_{34}=10.0\hat{i}+0.0\hat{j}+0.0\hat{k}$.

{\tiny 2D-M350:}

$\hat{n}_{14}=0.25\hat{i}+0.21\hat{j}+0.94\hat{k}$,\;\;\;$\hat{n}_{24}=0.59\hat{i}+0.57\hat{j}+0.58\hat{k}$,\;\;\;$\hat{n}_{25}=-0.37\hat{i}-0.31\hat{j}-0.88\hat{k}$,\;\;\;$\hat{n}_{34}=-0.78\hat{i}+0.6\hat{j}+0.19\hat{k}$,\newline
$\vec{r}_{25}=10.0\hat{i}+10.0\hat{j}+0.0\hat{k}$,\;\;\;$\vec{r}_{34}=0.0\hat{i}+0.0\hat{j}+0.0\hat{k}$,\;\;\;$\vec{r}_{35}=10.0\hat{i}+10.0\hat{j}+10.0\hat{k}$.

{\tiny 2D-M351:}

$\hat{n}_{14}=-0.12\hat{i}+0.83\hat{j}+0.55\hat{k}$,\;\;\;$\hat{n}_{24}=-0.58\hat{i}-0.6\hat{j}-0.55\hat{k}$,\;\;\;$\hat{n}_{25}=0.82\hat{i}-0.41\hat{j}-0.41\hat{k}$,\;\;\;$\hat{n}_{35}=-0.04\hat{i}+0.66\hat{j}-0.75\hat{k}$,\newline
$\vec{r}_{25}=10.0\hat{i}+10.0\hat{j}+10.0\hat{k}$,\;\;\;$\vec{r}_{34}=0.0\hat{i}+0.0\hat{j}+0.0\hat{k}$,\;\;\;$\vec{r}_{35}=10.0\hat{i}+10.0\hat{j}+10.0\hat{k}$.

{\tiny 2D-M352:}

$\hat{n}_{14}=0.01\hat{i}+0.02\hat{j}+1.0\hat{k}$,\;\;\;$\hat{n}_{24}=0.58\hat{i}+0.58\hat{j}-0.58\hat{k}$,\;\;\;$\hat{n}_{25}=-0.71\hat{i}+0.7\hat{j}-0.01\hat{k}$,\;\;\;$\hat{n}_{35}=0.4\hat{i}+0.41\hat{j}+0.82\hat{k}$,\newline
$\vec{r}_{25}=0.0\hat{i}+0.0\hat{j}+10.0\hat{k}$,\;\;\;$\vec{r}_{34}=10.0\hat{i}+10.0\hat{j}+0.0\hat{k}$,\;\;\;$\vec{r}_{35}=0.0\hat{i}+0.0\hat{j}+10.0\hat{k}$.

{\tiny 2D-M353:}

$\hat{n}_{14}=-0.45\hat{i}+0.89\hat{j}+0.04\hat{k}$,\;\;\;$\hat{n}_{24}=-0.62\hat{i}+0.44\hat{j}+0.65\hat{k}$,\;\;\;$\hat{n}_{34}=0.27\hat{i}+0.77\hat{j}-0.58\hat{k}$,\;\;\;$\hat{n}_{35}=-0.71\hat{i}-0.14\hat{j}-0.69\hat{k}$,\newline
$\vec{r}_{25}=0.0\hat{i}+10.0\hat{j}+0.0\hat{k}$,\;\;\;$\vec{r}_{34}=10.0\hat{i}+0.0\hat{j}+10.0\hat{k}$,\;\;\;$\vec{r}_{35}=0.0\hat{i}+0.0\hat{j}+10.0\hat{k}$.

{\tiny 2D-M354:}

$\hat{n}_{14}=0.02\hat{i}+0.98\hat{j}+0.19\hat{k}$,\;\;\;$\hat{n}_{24}=0.0\hat{i}+0.68\hat{j}-0.73\hat{k}$,\;\;\;$\hat{n}_{25}=-0.78\hat{i}+0.27\hat{j}+0.56\hat{k}$,\;\;\;$\hat{n}_{35}=0.58\hat{i}+0.49\hat{j}+0.65\hat{k}$,\newline
$\vec{r}_{24}=0.0\hat{i}+0.0\hat{j}+0.0\hat{k}$,\;\;\;$\vec{r}_{25}=10.0\hat{i}+0.0\hat{j}+0.0\hat{k}$,\;\;\;$\vec{r}_{34}=10.0\hat{i}+10.0\hat{j}+10.0\hat{k}$.

{\tiny 2D-M355:}

$\hat{n}_{14}=0.0\hat{i}+0.0\hat{j}+1.0\hat{k}$,\;\;\;$\hat{n}_{24}=0.71\hat{i}+0.71\hat{j}-0.0\hat{k}$,\;\;\;$\hat{n}_{25}=0.58\hat{i}-0.58\hat{j}+0.58\hat{k}$,\;\;\;$\hat{n}_{35}=-0.0\hat{i}+0.0\hat{j}-1.0\hat{k}$,\newline
$\vec{r}_{24}=0.0\hat{i}+10.0\hat{j}+10.0\hat{k}$,\;\;\;$\vec{r}_{34}=10.0\hat{i}+0.0\hat{j}+0.0\hat{k}$,\;\;\;$\vec{r}_{35}=0.0\hat{i}+10.0\hat{j}+9.99\hat{k}$.

{\tiny 2D-M356:}

$\hat{n}_{14}=0.68\hat{i}-0.52\hat{j}-0.52\hat{k}$,\;\;\;$\hat{n}_{23}=0.37\hat{i}-0.92\hat{j}-0.17\hat{k}$,\;\;\;$\hat{n}_{25}=-0.57\hat{i}-0.6\hat{j}+0.57\hat{k}$,\;\;\;$\hat{n}_{34}=0.69\hat{i}+0.02\hat{j}+0.72\hat{k}$,\newline
$\vec{r}_{23}=0.0\hat{i}+0.0\hat{j}+0.0\hat{k}$,\;\;\;$\vec{r}_{34}=10.0\hat{i}+10.0\hat{j}+0.0\hat{k}$,\;\;\;$\vec{r}_{45}=0.0\hat{i}+0.0\hat{j}+10.0\hat{k}$.

{\tiny 2D-M357:}

$\hat{n}_{14}=-0.04\hat{i}+0.91\hat{j}+0.41\hat{k}$,\;\;\;$\hat{n}_{23}=0.0\hat{i}+0.62\hat{j}+0.78\hat{k}$,\;\;\;$\hat{n}_{25}=-0.0\hat{i}-0.0\hat{j}+1.0\hat{k}$,\;\;\;$\hat{n}_{45}=0.89\hat{i}+0.1\hat{j}-0.44\hat{k}$,\newline
$\vec{r}_{23}=0.0\hat{i}+10.0\hat{j}+10.0\hat{k}$,\;\;\;$\vec{r}_{34}=10.0\hat{i}+0.0\hat{j}+0.0\hat{k}$,\;\;\;$\vec{r}_{45}=10.0\hat{i}+10.0\hat{j}+10.0\hat{k}$.

{\tiny 2D-M358:}

$\hat{n}_{14}=0.25\hat{i}+0.09\hat{j}+0.96\hat{k}$,\;\;\;$\hat{n}_{23}=-0.0\hat{i}+0.49\hat{j}+0.87\hat{k}$,\;\;\;$\hat{n}_{25}=-0.79\hat{i}-0.58\hat{j}+0.2\hat{k}$,\;\;\;$\hat{n}_{34}=0.57\hat{i}-0.56\hat{j}+0.6\hat{k}$,\newline
$\vec{r}_{23}=10.0\hat{i}+10.0\hat{j}+0.0\hat{k}$,\;\;\;$\vec{r}_{25}=0.0\hat{i}+10.0\hat{j}+10.0\hat{k}$,\;\;\;$\vec{r}_{45}=10.0\hat{i}+0.0\hat{j}+0.0\hat{k}$.

{\tiny 2D-M359:}

$\hat{n}_{14}=0.37\hat{i}-0.62\hat{j}-0.7\hat{k}$,\;\;\;$\hat{n}_{23}=0.71\hat{i}+0.0\hat{j}+0.71\hat{k}$,\;\;\;$\hat{n}_{25}=-0.55\hat{i}+0.63\hat{j}+0.55\hat{k}$,\;\;\;$\hat{n}_{45}=-0.45\hat{i}-0.77\hat{j}+0.45\hat{k}$,\newline
$\vec{r}_{23}=10.0\hat{i}+0.0\hat{j}+10.0\hat{k}$,\;\;\;$\vec{r}_{25}=0.0\hat{i}+0.0\hat{j}+10.0\hat{k}$,\;\;\;$\vec{r}_{34}=10.0\hat{i}+10.0\hat{j}+0.0\hat{k}$.

{\tiny 2D-M360:}

$\hat{n}_{14}=0.0\hat{i}+0.28\hat{j}+0.96\hat{k}$,\;\;\;$\hat{n}_{23}=0.25\hat{i}-0.55\hat{j}-0.8\hat{k}$,\;\;\;$\hat{n}_{34}=0.58\hat{i}-0.58\hat{j}+0.58\hat{k}$,\;\;\;$\hat{n}_{45}=-0.78\hat{i}-0.6\hat{j}+0.18\hat{k}$,\newline
$\vec{r}_{23}=0.0\hat{i}+10.0\hat{j}+10.0\hat{k}$,\;\;\;$\vec{r}_{25}=10.0\hat{i}+0.0\hat{j}+0.0\hat{k}$,\;\;\;$\vec{r}_{45}=0.0\hat{i}+10.0\hat{j}+10.0\hat{k}$.

{\tiny 2D-M361:}

$\hat{n}_{14}=-0.65\hat{i}+0.76\hat{j}+0.0\hat{k}$,\;\;\;$\hat{n}_{23}=0.53\hat{i}+0.66\hat{j}-0.53\hat{k}$,\;\;\;$\hat{n}_{34}=0.88\hat{i}+0.27\hat{j}-0.39\hat{k}$,\;\;\;$\hat{n}_{45}=-0.0\hat{i}+0.0\hat{j}-1.0\hat{k}$,\newline
$\vec{r}_{23}=10.0\hat{i}+0.0\hat{j}+0.0\hat{k}$,\;\;\;$\vec{r}_{25}=10.0\hat{i}+10.0\hat{j}+10.0\hat{k}$,\;\;\;$\vec{r}_{34}=0.0\hat{i}+0.0\hat{j}+0.0\hat{k}$.

{\tiny 2D-M362:}

$\hat{n}_{14}=-0.01\hat{i}+0.17\hat{j}-0.99\hat{k}$,\;\;\;$\hat{n}_{23}=-0.0\hat{i}+0.74\hat{j}-0.67\hat{k}$,\;\;\;$\hat{n}_{25}=0.0\hat{i}+0.0\hat{j}-1.0\hat{k}$,\;\;\;$\hat{n}_{34}=0.93\hat{i}-0.37\hat{j}+0.05\hat{k}$,\newline
$\vec{r}_{25}=0.0\hat{i}+10.0\hat{j}+9.3\hat{k}$,\;\;\;$\vec{r}_{34}=0.0\hat{i}+0.0\hat{j}+10.0\hat{k}$,\;\;\;$\vec{r}_{45}=10.0\hat{i}+10.0\hat{j}+0.0\hat{k}$.

{\tiny 2D-M363:}

$\hat{n}_{14}=0.01\hat{i}+0.68\hat{j}-0.73\hat{k}$,\;\;\;$\hat{n}_{23}=0.0\hat{i}+0.71\hat{j}+0.71\hat{k}$,\;\;\;$\hat{n}_{25}=0.0\hat{i}-0.71\hat{j}+0.71\hat{k}$,\;\;\;$\hat{n}_{45}=-0.93\hat{i}-0.25\hat{j}-0.25\hat{k}$,\newline
$\vec{r}_{25}=10.0\hat{i}+0.0\hat{j}+10.0\hat{k}$,\;\;\;$\vec{r}_{34}=0.0\hat{i}+10.0\hat{j}+0.0\hat{k}$,\;\;\;$\vec{r}_{45}=10.0\hat{i}+0.0\hat{j}+10.0\hat{k}$.

{\tiny 2D-M364:}

$\hat{n}_{14}=-0.5\hat{i}-0.58\hat{j}-0.64\hat{k}$,\;\;\;$\hat{n}_{23}=0.71\hat{i}+0.71\hat{j}+0.0\hat{k}$,\;\;\;$\hat{n}_{25}=-0.0\hat{i}+0.0\hat{j}+1.0\hat{k}$,\;\;\;$\hat{n}_{34}=-0.0\hat{i}+0.0\hat{j}+1.0\hat{k}$,\newline
$\vec{r}_{25}=0.0\hat{i}+0.0\hat{j}+0.0\hat{k}$,\;\;\;$\vec{r}_{34}=10.0\hat{i}+10.0\hat{j}+5.83\hat{k}$,\;\;\;$\vec{r}_{45}=10.0\hat{i}+10.0\hat{j}+10.0\hat{k}$.

{\tiny 2D-M365:}

$\hat{n}_{14}=0.26\hat{i}+0.45\hat{j}+0.85\hat{k}$,\;\;\;$\hat{n}_{23}=-0.62\hat{i}-0.78\hat{j}-0.0\hat{k}$,\;\;\;$\hat{n}_{25}=-0.13\hat{i}-0.95\hat{j}+0.3\hat{k}$,\;\;\;$\hat{n}_{45}=-0.44\hat{i}-0.24\hat{j}+0.87\hat{k}$,\newline
$\vec{r}_{25}=6.53\hat{i}+5.84\hat{j}+4.67\hat{k}$,\;\;\;$\vec{r}_{34}=5.22\hat{i}+3.7\hat{j}+6.69\hat{k}$,\;\;\;$\vec{r}_{45}=10.0\hat{i}+10.0\hat{j}+10.0\hat{k}$.

{\tiny 2D-M366:}

$\hat{n}_{14}=-0.31\hat{i}+0.95\hat{j}-0.06\hat{k}$,\;\;\;$\hat{n}_{23}=-0.0\hat{i}+0.63\hat{j}+0.77\hat{k}$,\;\;\;$\hat{n}_{34}=0.0\hat{i}+0.96\hat{j}+0.29\hat{k}$,\;\;\;$\hat{n}_{45}=-0.85\hat{i}-0.1\hat{j}+0.52\hat{k}$,\newline
$\vec{r}_{25}=0.0\hat{i}+0.0\hat{j}+0.0\hat{k}$,\;\;\;$\vec{r}_{34}=0.0\hat{i}+10.0\hat{j}+10.0\hat{k}$,\;\;\;$\vec{r}_{45}=10.0\hat{i}+10.0\hat{j}+10.0\hat{k}$.

{\tiny 2D-M367:}

$\hat{n}_{14}=-0.1\hat{i}+0.0\hat{j}-1.0\hat{k}$,\;\;\;$\hat{n}_{23}=0.0\hat{i}+0.71\hat{j}-0.71\hat{k}$,\;\;\;$\hat{n}_{34}=0.95\hat{i}+0.21\hat{j}-0.21\hat{k}$,\;\;\;$\hat{n}_{45}=-0.24\hat{i}-0.42\hat{j}+0.88\hat{k}$,\newline
$\vec{r}_{25}=0.0\hat{i}+10.0\hat{j}+10.0\hat{k}$,\;\;\;$\vec{r}_{34}=10.0\hat{i}+0.0\hat{j}+0.0\hat{k}$,\;\;\;$\vec{r}_{45}=10.0\hat{i}+10.0\hat{j}+10.0\hat{k}$.

{\tiny 2D-M368:}

$\hat{n}_{14}=-0.5\hat{i}+0.75\hat{j}+0.44\hat{k}$,\;\;\;$\hat{n}_{23}=-0.59\hat{i}-0.19\hat{j}-0.79\hat{k}$,\;\;\;$\hat{n}_{25}=0.59\hat{i}-0.68\hat{j}-0.44\hat{k}$,\;\;\;$\hat{n}_{34}=-0.59\hat{i}-0.56\hat{j}+0.58\hat{k}$,\newline
$\vec{r}_{23}=0.0\hat{i}+0.0\hat{j}+10.0\hat{k}$,\;\;\;$\vec{r}_{25}=10.0\hat{i}+10.0\hat{j}+10.0\hat{k}$,\;\;\;$\vec{r}_{45}=10.0\hat{i}+10.0\hat{j}+0.0\hat{k}$.

{\tiny 2D-M369:}

$\hat{n}_{14}=0.04\hat{i}+0.72\hat{j}+0.69\hat{k}$,\;\;\;$\hat{n}_{23}=-0.9\hat{i}-0.31\hat{j}+0.31\hat{k}$,\;\;\;$\hat{n}_{25}=0.0\hat{i}+0.71\hat{j}+0.71\hat{k}$,\;\;\;$\hat{n}_{45}=-0.44\hat{i}+0.64\hat{j}-0.64\hat{k}$,\newline
$\vec{r}_{23}=10.0\hat{i}+0.0\hat{j}+0.0\hat{k}$,\;\;\;$\vec{r}_{25}=0.0\hat{i}+0.0\hat{j}+10.0\hat{k}$,\;\;\;$\vec{r}_{34}=0.0\hat{i}+10.0\hat{j}+10.0\hat{k}$.

{\tiny 2D-M370:}

$\hat{n}_{14}=-0.25\hat{i}+0.84\hat{j}+0.49\hat{k}$,\;\;\;$\hat{n}_{23}=-0.79\hat{i}-0.56\hat{j}-0.24\hat{k}$,\;\;\;$\hat{n}_{25}=0.58\hat{i}-0.58\hat{j}-0.58\hat{k}$,\;\;\;$\hat{n}_{34}=0.82\hat{i}+0.56\hat{j}-0.13\hat{k}$,\newline
$\vec{r}_{23}=0.0\hat{i}+10.0\hat{j}+0.0\hat{k}$,\;\;\;$\vec{r}_{34}=10.0\hat{i}+0.0\hat{j}+10.0\hat{k}$,\;\;\;$\vec{r}_{45}=10.0\hat{i}+0.0\hat{j}+10.0\hat{k}$.

{\tiny 2D-M371:}

$\hat{n}_{14}=-0.41\hat{i}+0.2\hat{j}+0.89\hat{k}$,\;\;\;$\hat{n}_{23}=0.0\hat{i}-0.74\hat{j}-0.67\hat{k}$,\;\;\;$\hat{n}_{25}=-0.02\hat{i}-0.11\hat{j}+0.99\hat{k}$,\;\;\;$\hat{n}_{45}=-0.0\hat{i}-0.0\hat{j}+1.0\hat{k}$,\newline
$\vec{r}_{23}=3.16\hat{i}+2.97\hat{j}+6.41\hat{k}$,\;\;\;$\vec{r}_{34}=3.07\hat{i}+6.34\hat{j}+6.83\hat{k}$,\;\;\;$\vec{r}_{45}=0.0\hat{i}+10.0\hat{j}+4.66\hat{k}$.

{\tiny 2D-M372:}

$\hat{n}_{14}=-0.72\hat{i}-0.7\hat{j}+0.01\hat{k}$,\;\;\;$\hat{n}_{23}=0.55\hat{i}-0.55\hat{j}-0.63\hat{k}$,\;\;\;$\hat{n}_{34}=-0.71\hat{i}-0.71\hat{j}-0.0\hat{k}$,\;\;\;$\hat{n}_{45}=0.45\hat{i}-0.45\hat{j}+0.77\hat{k}$,\newline
$\vec{r}_{23}=0.0\hat{i}+10.0\hat{j}+10.0\hat{k}$,\;\;\;$\vec{r}_{25}=10.0\hat{i}+0.0\hat{j}+0.0\hat{k}$,\;\;\;$\vec{r}_{34}=0.0\hat{i}+10.0\hat{j}+0.0\hat{k}$.

{\tiny 2D-M373:}

$\hat{n}_{14}=0.62\hat{i}+0.59\hat{j}-0.52\hat{k}$,\;\;\;$\hat{n}_{23}=-0.13\hat{i}-0.8\hat{j}+0.59\hat{k}$,\;\;\;$\hat{n}_{34}=-0.02\hat{i}-0.94\hat{j}+0.35\hat{k}$,\;\;\;$\hat{n}_{45}=0.51\hat{i}-0.74\hat{j}-0.43\hat{k}$,\newline
$\vec{r}_{23}=3.72\hat{i}+3.44\hat{j}+4.97\hat{k}$,\;\;\;$\vec{r}_{25}=6.54\hat{i}+6.37\hat{j}+3.86\hat{k}$,\;\;\;$\vec{r}_{45}=10.0\hat{i}+10.0\hat{j}+0.0\hat{k}$.

{\tiny 2D-M374:}

$\hat{n}_{14}=0.06\hat{i}+0.93\hat{j}-0.37\hat{k}$,\;\;\;$\hat{n}_{25}=-0.63\hat{i}+0.76\hat{j}+0.13\hat{k}$,\;\;\;$\hat{n}_{34}=0.58\hat{i}+0.58\hat{j}-0.58\hat{k}$,\;\;\;$\hat{n}_{45}=0.52\hat{i}+0.29\hat{j}+0.81\hat{k}$,\newline
$\vec{r}_{23}=0.0\hat{i}+0.0\hat{j}+10.0\hat{k}$,\;\;\;$\vec{r}_{25}=10.0\hat{i}+10.0\hat{j}+0.0\hat{k}$,\;\;\;$\vec{r}_{45}=10.0\hat{i}+10.0\hat{j}+0.0\hat{k}$.

{\tiny 2D-M375:}

$\hat{n}_{14}=-0.74\hat{i}-0.3\hat{j}-0.6\hat{k}$,\;\;\;$\hat{n}_{25}=-0.71\hat{i}+0.71\hat{j}+0.0\hat{k}$,\;\;\;$\hat{n}_{34}=-0.55\hat{i}-0.55\hat{j}-0.63\hat{k}$,\;\;\;$\hat{n}_{45}=-0.45\hat{i}-0.45\hat{j}+0.77\hat{k}$,\newline
$\vec{r}_{23}=10.0\hat{i}+10.0\hat{j}+0.0\hat{k}$,\;\;\;$\vec{r}_{25}=0.0\hat{i}+0.0\hat{j}+0.0\hat{k}$,\;\;\;$\vec{r}_{34}=0.0\hat{i}+0.0\hat{j}+10.0\hat{k}$.

{\tiny 2D-M376:}

$\hat{n}_{14}=0.08\hat{i}+0.11\hat{j}-0.99\hat{k}$,\;\;\;$\hat{n}_{25}=0.57\hat{i}-0.48\hat{j}+0.66\hat{k}$,\;\;\;$\hat{n}_{34}=0.0\hat{i}+0.0\hat{j}+1.0\hat{k}$,\;\;\;$\hat{n}_{45}=-0.0\hat{i}+0.83\hat{j}+0.55\hat{k}$,\newline
$\vec{r}_{23}=10.0\hat{i}+0.0\hat{j}+0.0\hat{k}$,\;\;\;$\vec{r}_{34}=0.0\hat{i}+10.0\hat{j}+0.01\hat{k}$,\;\;\;$\vec{r}_{45}=0.0\hat{i}+10.0\hat{j}+10.0\hat{k}$.

{\tiny 2D-M377:}

$\hat{n}_{14}=0.14\hat{i}-0.01\hat{j}-0.99\hat{k}$,\;\;\;$\hat{n}_{25}=-1.0\hat{i}+0.03\hat{j}-0.02\hat{k}$,\;\;\;$\hat{n}_{34}=0.56\hat{i}-0.83\hat{j}-0.06\hat{k}$,\;\;\;$\hat{n}_{45}=0.14\hat{i}-0.52\hat{j}+0.84\hat{k}$,\newline
$\vec{r}_{23}=3.17\hat{i}+3.41\hat{j}+4.4\hat{k}$,\;\;\;$\vec{r}_{34}=7.03\hat{i}+7.38\hat{j}+5.37\hat{k}$,\;\;\;$\vec{r}_{45}=10.0\hat{i}+0.0\hat{j}+10.0\hat{k}$.

{\tiny 2D-M378:}

$\hat{n}_{14}=0.0\hat{i}+0.0\hat{j}+1.0\hat{k}$,\;\;\;$\hat{n}_{25}=0.43\hat{i}+0.46\hat{j}-0.78\hat{k}$,\;\;\;$\hat{n}_{34}=-0.62\hat{i}+0.48\hat{j}-0.62\hat{k}$,\;\;\;$\hat{n}_{45}=-0.11\hat{i}-0.92\hat{j}-0.37\hat{k}$,\newline
$\vec{r}_{23}=10.0\hat{i}+0.0\hat{j}+10.0\hat{k}$,\;\;\;$\vec{r}_{25}=0.0\hat{i}+0.0\hat{j}+0.0\hat{k}$,\;\;\;$\vec{r}_{34}=10.0\hat{i}+10.0\hat{j}+0.0\hat{k}$.

{\tiny 2D-M379:}

$\hat{n}_{14}=-0.75\hat{i}-0.41\hat{j}-0.53\hat{k}$,\;\;\;$\hat{n}_{25}=0.13\hat{i}-0.82\hat{j}+0.55\hat{k}$,\;\;\;$\hat{n}_{34}=-0.29\hat{i}-0.73\hat{j}-0.61\hat{k}$,\;\;\;$\hat{n}_{45}=0.65\hat{i}-0.72\hat{j}+0.23\hat{k}$,\newline
$\vec{r}_{23}=6.7\hat{i}+6.71\hat{j}+3.56\hat{k}$,\;\;\;$\vec{r}_{25}=3.87\hat{i}+6.71\hat{j}+6.83\hat{k}$,\;\;\;$\vec{r}_{45}=10.0\hat{i}+10.0\hat{j}+10.0\hat{k}$.

{\tiny 2D-M380:}

$\hat{n}_{14}=-0.0\hat{i}-0.0\hat{j}-1.0\hat{k}$,\;\;\;$\hat{n}_{15}=-0.0\hat{i}+0.57\hat{j}-0.82\hat{k}$,\;\;\;$\hat{n}_{23}=-0.39\hat{i}-0.43\hat{j}+0.82\hat{k}$,\;\;\;$\hat{n}_{25}=-0.64\hat{i}-0.7\hat{j}-0.31\hat{k}$,\newline
$\vec{r}_{15}=10.0\hat{i}+10.0\hat{j}+10.0\hat{k}$,\;\;\;$\vec{r}_{23}=10.0\hat{i}+10.0\hat{j}+10.0\hat{k}$,\;\;\;$\vec{r}_{34}=0.0\hat{i}+0.0\hat{j}+0.0\hat{k}$.

{\tiny 2D-M381:}

$\hat{n}_{14}=-0.61\hat{i}-0.61\hat{j}+0.51\hat{k}$,\;\;\;$\hat{n}_{15}=-0.18\hat{i}+0.76\hat{j}-0.62\hat{k}$,\;\;\;$\hat{n}_{23}=0.0\hat{i}-0.0\hat{j}+1.0\hat{k}$,\;\;\;$\hat{n}_{34}=0.14\hat{i}+0.55\hat{j}+0.82\hat{k}$,\newline
$\vec{r}_{15}=0.0\hat{i}+10.0\hat{j}+0.0\hat{k}$,\;\;\;$\vec{r}_{23}=0.0\hat{i}+0.0\hat{j}+9.59\hat{k}$,\;\;\;$\vec{r}_{25}=10.0\hat{i}+10.0\hat{j}+10.0\hat{k}$.

{\tiny 2D-M382:}

$\hat{n}_{14}=-0.41\hat{i}-0.41\hat{j}-0.82\hat{k}$,\;\;\;$\hat{n}_{15}=-0.82\hat{i}+0.41\hat{j}-0.41\hat{k}$,\;\;\;$\hat{n}_{23}=0.58\hat{i}+0.58\hat{j}-0.58\hat{k}$,\;\;\;$\hat{n}_{25}=-0.0\hat{i}+0.0\hat{j}-1.0\hat{k}$,\newline
$\vec{r}_{15}=0.0\hat{i}+0.0\hat{j}+10.0\hat{k}$,\;\;\;$\vec{r}_{25}=0.0\hat{i}+0.0\hat{j}+0.56\hat{k}$,\;\;\;$\vec{r}_{34}=10.0\hat{i}+10.0\hat{j}+0.0\hat{k}$.

{\tiny 2D-M383:}

$\hat{n}_{14}=0.53\hat{i}-0.85\hat{j}-0.0\hat{k}$,\;\;\;$\hat{n}_{15}=-0.68\hat{i}+0.51\hat{j}-0.52\hat{k}$,\;\;\;$\hat{n}_{23}=-0.0\hat{i}+0.0\hat{j}-1.0\hat{k}$,\;\;\;$\hat{n}_{34}=0.0\hat{i}+0.53\hat{j}-0.85\hat{k}$,\newline
$\vec{r}_{15}=10.0\hat{i}+0.0\hat{j}+10.0\hat{k}$,\;\;\;$\vec{r}_{25}=0.0\hat{i}+10.0\hat{j}+0.0\hat{k}$,\;\;\;$\vec{r}_{34}=10.0\hat{i}+0.0\hat{j}+10.0\hat{k}$.

{\tiny 2D-M384:}

$\hat{n}_{14}=0.0\hat{i}+0.71\hat{j}+0.71\hat{k}$,\;\;\;$\hat{n}_{15}=0.82\hat{i}-0.41\hat{j}+0.41\hat{k}$,\;\;\;$\hat{n}_{25}=-0.0\hat{i}+0.71\hat{j}+0.71\hat{k}$,\;\;\;$\hat{n}_{34}=-0.58\hat{i}-0.58\hat{j}+0.58\hat{k}$,\newline
$\vec{r}_{15}=10.0\hat{i}+10.0\hat{j}+0.0\hat{k}$,\;\;\;$\vec{r}_{23}=0.0\hat{i}+0.0\hat{j}+10.0\hat{k}$,\;\;\;$\vec{r}_{25}=10.0\hat{i}+10.0\hat{j}+0.0\hat{k}$.

{\tiny 2D-M385:}

$\hat{n}_{14}=0.0\hat{i}-0.0\hat{j}+1.0\hat{k}$,\;\;\;$\hat{n}_{15}=-0.0\hat{i}+0.0\hat{j}+1.0\hat{k}$,\;\;\;$\hat{n}_{25}=-0.71\hat{i}+0.71\hat{j}+0.0\hat{k}$,\;\;\;$\hat{n}_{34}=-0.41\hat{i}+0.41\hat{j}+0.82\hat{k}$,\newline
$\vec{r}_{15}=0.0\hat{i}+10.0\hat{j}+0.26\hat{k}$,\;\;\;$\vec{r}_{23}=10.0\hat{i}+0.0\hat{j}+0.0\hat{k}$,\;\;\;$\vec{r}_{34}=0.0\hat{i}+10.0\hat{j}+10.0\hat{k}$.

{\tiny 2D-M386:}

$\hat{n}_{14}=-0.62\hat{i}-0.77\hat{j}+0.15\hat{k}$,\;\;\;$\hat{n}_{23}=0.73\hat{i}+0.62\hat{j}-0.28\hat{k}$,\;\;\;$\hat{n}_{25}=-0.58\hat{i}+0.58\hat{j}+0.58\hat{k}$,\;\;\;$\hat{n}_{34}=-0.53\hat{i}+0.27\hat{j}-0.8\hat{k}$,\newline
$\vec{r}_{15}=10.0\hat{i}+0.0\hat{j}+10.0\hat{k}$,\;\;\;$\vec{r}_{23}=6.72\hat{i}+3.59\hat{j}+6.36\hat{k}$,\;\;\;$\vec{r}_{34}=0.0\hat{i}+10.0\hat{j}+0.0\hat{k}$.

{\tiny 2D-M387:}

$\hat{n}_{14}=0.0\hat{i}-0.71\hat{j}-0.71\hat{k}$,\;\;\;$\hat{n}_{23}=-0.08\hat{i}+0.62\hat{j}+0.78\hat{k}$,\;\;\;$\hat{n}_{25}=0.82\hat{i}-0.41\hat{j}+0.41\hat{k}$,\;\;\;$\hat{n}_{34}=-0.58\hat{i}-0.58\hat{j}+0.58\hat{k}$,\newline
$\vec{r}_{15}=10.0\hat{i}+10.0\hat{j}+0.0\hat{k}$,\;\;\;$\vec{r}_{23}=5.96\hat{i}+4.18\hat{j}+6.17\hat{k}$,\;\;\;$\vec{r}_{25}=0.0\hat{i}+0.0\hat{j}+10.0\hat{k}$.

{\tiny 2D-M388:}

$\hat{n}_{14}=0.0\hat{i}+0.71\hat{j}+0.71\hat{k}$,\;\;\;$\hat{n}_{23}=-0.58\hat{i}-0.58\hat{j}+0.58\hat{k}$,\;\;\;$\hat{n}_{25}=-0.12\hat{i}-0.81\hat{j}-0.58\hat{k}$,\;\;\;$\hat{n}_{34}=0.82\hat{i}-0.41\hat{j}+0.41\hat{k}$,\newline
$\vec{r}_{15}=0.0\hat{i}+0.0\hat{j}+10.0\hat{k}$,\;\;\;$\vec{r}_{25}=3.34\hat{i}+2.57\hat{j}+6.67\hat{k}$,\;\;\;$\vec{r}_{34}=10.0\hat{i}+10.0\hat{j}+0.0\hat{k}$.

{\tiny 2D-M389:}

$\hat{n}_{14}=-0.82\hat{i}+0.43\hat{j}-0.39\hat{k}$,\;\;\;$\hat{n}_{23}=0.58\hat{i}+0.61\hat{j}-0.54\hat{k}$,\;\;\;$\hat{n}_{25}=-0.0\hat{i}+0.67\hat{j}+0.74\hat{k}$,\;\;\;$\hat{n}_{34}=-0.82\hat{i}+0.43\hat{j}-0.38\hat{k}$,\newline
$\vec{r}_{15}=10.0\hat{i}+10.0\hat{j}+0.0\hat{k}$,\;\;\;$\vec{r}_{25}=0.0\hat{i}+0.0\hat{j}+10.0\hat{k}$,\;\;\;$\vec{r}_{34}=3.03\hat{i}+6.87\hat{j}+5.52\hat{k}$.

{\tiny 2D-M390:}

$\hat{n}_{14}=-0.82\hat{i}-0.38\hat{j}+0.43\hat{k}$,\;\;\;$\hat{n}_{23}=0.0\hat{i}+0.75\hat{j}+0.66\hat{k}$,\;\;\;$\hat{n}_{25}=-0.69\hat{i}-0.48\hat{j}+0.54\hat{k}$,\;\;\;$\hat{n}_{34}=-0.58\hat{i}+0.54\hat{j}-0.61\hat{k}$,\newline
$\vec{r}_{15}=0.0\hat{i}+10.0\hat{j}+10.0\hat{k}$,\;\;\;$\vec{r}_{23}=10.0\hat{i}+0.0\hat{j}+0.0\hat{k}$,\;\;\;$\vec{r}_{25}=3.66\hat{i}+6.37\hat{j}+4.46\hat{k}$.

{\tiny 2D-M391:}

$\hat{n}_{14}=-0.0\hat{i}+0.0\hat{j}-1.0\hat{k}$,\;\;\;$\hat{n}_{23}=-0.94\hat{i}-0.28\hat{j}+0.18\hat{k}$,\;\;\;$\hat{n}_{25}=0.0\hat{i}+0.88\hat{j}-0.48\hat{k}$,\;\;\;$\hat{n}_{34}=0.12\hat{i}-0.78\hat{j}-0.61\hat{k}$,\newline
$\vec{r}_{15}=0.0\hat{i}+10.0\hat{j}+10.0\hat{k}$,\;\;\;$\vec{r}_{23}=10.0\hat{i}+0.0\hat{j}+0.0\hat{k}$,\;\;\;$\vec{r}_{34}=1.2\hat{i}+1.39\hat{j}+9.93\hat{k}$.

{\tiny 2D-M392:}

$\hat{n}_{14}=-0.76\hat{i}-0.65\hat{j}-0.02\hat{k}$,\;\;\;$\hat{n}_{23}=-0.37\hat{i}+0.39\hat{j}+0.84\hat{k}$,\;\;\;$\hat{n}_{25}=-0.0\hat{i}+0.0\hat{j}-1.0\hat{k}$,\;\;\;$\hat{n}_{34}=0.59\hat{i}-0.7\hat{j}+0.39\hat{k}$,\newline
$\vec{r}_{14}=0.0\hat{i}+10.0\hat{j}+10.0\hat{k}$,\;\;\;$\vec{r}_{15}=10.0\hat{i}+0.0\hat{j}+0.0\hat{k}$,\;\;\;$\vec{r}_{23}=4.57\hat{i}+7.23\hat{j}+6.35\hat{k}$.

{\tiny 2D-M393:}

$\hat{n}_{14}=0.76\hat{i}+0.65\hat{j}+0.02\hat{k}$,\;\;\;$\hat{n}_{23}=0.0\hat{i}+0.0\hat{j}-1.0\hat{k}$,\;\;\;$\hat{n}_{25}=0.37\hat{i}-0.39\hat{j}-0.84\hat{k}$,\;\;\;$\hat{n}_{34}=0.59\hat{i}-0.7\hat{j}+0.39\hat{k}$,\newline
$\vec{r}_{14}=0.0\hat{i}+10.0\hat{j}+10.0\hat{k}$,\;\;\;$\vec{r}_{15}=10.0\hat{i}+0.0\hat{j}+0.0\hat{k}$,\;\;\;$\vec{r}_{25}=6.29\hat{i}+5.68\hat{j}+2.58\hat{k}$.

{\tiny 2D-M394:}

$\hat{n}_{14}=-0.34\hat{i}+0.88\hat{j}+0.33\hat{k}$,\;\;\;$\hat{n}_{23}=-0.93\hat{i}-0.35\hat{j}-0.0\hat{k}$,\;\;\;$\hat{n}_{25}=0.0\hat{i}+0.0\hat{j}+1.0\hat{k}$,\;\;\;$\hat{n}_{34}=-0.66\hat{i}+0.03\hat{j}-0.75\hat{k}$,\newline
$\vec{r}_{14}=0.0\hat{i}+10.0\hat{j}+10.0\hat{k}$,\;\;\;$\vec{r}_{15}=10.0\hat{i}+10.0\hat{j}+0.0\hat{k}$,\;\;\;$\vec{r}_{34}=4.97\hat{i}+5.13\hat{j}+4.93\hat{k}$.

{\tiny 2D-M395:}

$\hat{n}_{15}=-0.82\hat{i}+0.41\hat{j}-0.41\hat{k}$,\;\;\;$\hat{n}_{23}=-0.07\hat{i}+0.74\hat{j}+0.67\hat{k}$,\;\;\;$\hat{n}_{25}=-0.07\hat{i}+0.74\hat{j}+0.67\hat{k}$,\;\;\;$\hat{n}_{34}=-0.58\hat{i}-0.58\hat{j}+0.58\hat{k}$,\newline
$\vec{r}_{14}=0.0\hat{i}+0.0\hat{j}+10.0\hat{k}$,\;\;\;$\vec{r}_{15}=10.0\hat{i}+10.0\hat{j}+0.0\hat{k}$,\;\;\;$\vec{r}_{23}=10.0\hat{i}+10.0\hat{j}+0.0\hat{k}$.

{\tiny 2D-M396:}

$\hat{n}_{15}=-0.82\hat{i}+0.41\hat{j}+0.41\hat{k}$,\;\;\;$\hat{n}_{23}=0.56\hat{i}+0.23\hat{j}-0.79\hat{k}$,\;\;\;$\hat{n}_{25}=0.56\hat{i}+0.23\hat{j}-0.79\hat{k}$,\;\;\;$\hat{n}_{34}=0.58\hat{i}+0.58\hat{j}+0.58\hat{k}$,\newline
$\vec{r}_{14}=10.0\hat{i}+10.0\hat{j}+10.0\hat{k}$,\;\;\;$\vec{r}_{15}=0.0\hat{i}+0.0\hat{j}+0.0\hat{k}$,\;\;\;$\vec{r}_{25}=0.0\hat{i}+0.0\hat{j}+0.0\hat{k}$.

{\tiny 2D-M397:}

$\hat{n}_{15}=0.0\hat{i}+0.28\hat{j}+0.96\hat{k}$,\;\;\;$\hat{n}_{23}=0.0\hat{i}+0.19\hat{j}+0.98\hat{k}$,\;\;\;$\hat{n}_{25}=-0.74\hat{i}+0.65\hat{j}-0.17\hat{k}$,\;\;\;$\hat{n}_{34}=-0.5\hat{i}+0.31\hat{j}-0.81\hat{k}$,\newline
$\vec{r}_{14}=10.0\hat{i}+0.0\hat{j}+10.0\hat{k}$,\;\;\;$\vec{r}_{15}=0.0\hat{i}+10.0\hat{j}+10.0\hat{k}$,\;\;\;$\vec{r}_{34}=0.0\hat{i}+10.0\hat{j}+0.0\hat{k}$.

{\tiny 2D-M398:}

$\hat{n}_{13}=-0.0\hat{i}+0.58\hat{j}-0.81\hat{k}$,\;\;\;$\hat{n}_{14}=0.0\hat{i}+0.0\hat{j}+1.0\hat{k}$,\;\;\;$\hat{n}_{24}=-0.61\hat{i}-0.69\hat{j}-0.4\hat{k}$,\;\;\;$\hat{n}_{25}=-0.79\hat{i}+0.59\hat{j}+0.18\hat{k}$,\newline
$\vec{r}_{13}=10.0\hat{i}+10.0\hat{j}+10.0\hat{k}$,\;\;\;$\vec{r}_{25}=10.0\hat{i}+10.0\hat{j}+10.0\hat{k}$,\;\;\;$\vec{r}_{35}=0.0\hat{i}+0.0\hat{j}+0.0\hat{k}$.

{\tiny 2D-M399:}

$\hat{n}_{13}=-0.72\hat{i}+0.59\hat{j}-0.37\hat{k}$,\;\;\;$\hat{n}_{14}=0.0\hat{i}+0.85\hat{j}-0.52\hat{k}$,\;\;\;$\hat{n}_{24}=-0.55\hat{i}-0.51\hat{j}-0.66\hat{k}$,\;\;\;$\hat{n}_{35}=0.08\hat{i}-0.79\hat{j}+0.61\hat{k}$,\newline
$\vec{r}_{13}=10.0\hat{i}+10.0\hat{j}+0.0\hat{k}$,\;\;\;$\vec{r}_{25}=10.0\hat{i}+10.0\hat{j}+10.0\hat{k}$,\;\;\;$\vec{r}_{35}=0.0\hat{i}+0.0\hat{j}+0.0\hat{k}$.

{\tiny 2D-M400:}

$\hat{n}_{13}=0.42\hat{i}-0.4\hat{j}-0.82\hat{k}$,\;\;\;$\hat{n}_{14}=-0.0\hat{i}+0.0\hat{j}-1.0\hat{k}$,\;\;\;$\hat{n}_{24}=0.65\hat{i}+0.76\hat{j}-0.04\hat{k}$,\;\;\;$\hat{n}_{25}=-0.71\hat{i}+0.59\hat{j}-0.39\hat{k}$,\newline
$\vec{r}_{13}=10.0\hat{i}+0.0\hat{j}+0.0\hat{k}$,\;\;\;$\vec{r}_{24}=10.0\hat{i}+0.0\hat{j}+0.0\hat{k}$,\;\;\;$\vec{r}_{35}=0.0\hat{i}+10.0\hat{j}+10.0\hat{k}$.

2D-M401:

$\hat{n}_{13}=-0.73\hat{i}-0.62\hat{j}+0.28\hat{k}$,\;\;\;$\hat{n}_{14}=0.58\hat{i}-0.58\hat{j}-0.58\hat{k}$,\;\;\;$\hat{n}_{24}=0.0\hat{i}+0.71\hat{j}-0.71\hat{k}$,\;\;\;$\hat{n}_{35}=0.58\hat{i}-0.58\hat{j}-0.58\hat{k}$,\newline
$\vec{r}_{13}=10.0\hat{i}+0.0\hat{j}+10.0\hat{k}$,\;\;\;$\vec{r}_{24}=0.0\hat{i}+10.0\hat{j}+0.0\hat{k}$,\;\;\;$\vec{r}_{25}=10.0\hat{i}+0.0\hat{j}+10.0\hat{k}$.

2D-M402:

$\hat{n}_{13}=0.0\hat{i}+0.48\hat{j}-0.88\hat{k}$,\;\;\;$\hat{n}_{14}=-0.0\hat{i}-0.0\hat{j}-1.0\hat{k}$,\;\;\;$\hat{n}_{25}=0.62\hat{i}-0.72\hat{j}-0.32\hat{k}$,\;\;\;$\hat{n}_{35}=0.17\hat{i}-0.47\hat{j}+0.87\hat{k}$,\newline
$\vec{r}_{13}=10.0\hat{i}+0.0\hat{j}+10.0\hat{k}$,\;\;\;$\vec{r}_{24}=10.0\hat{i}+0.0\hat{j}+10.0\hat{k}$,\;\;\;$\vec{r}_{35}=0.0\hat{i}+10.0\hat{j}+0.0\hat{k}$.

2D-M403:

$\hat{n}_{13}=-0.0\hat{i}+0.82\hat{j}+0.57\hat{k}$,\;\;\;$\hat{n}_{14}=-0.0\hat{i}+0.72\hat{j}+0.69\hat{k}$,\;\;\;$\hat{n}_{25}=0.95\hat{i}-0.25\hat{j}-0.18\hat{k}$,\;\;\;$\hat{n}_{35}=-0.0\hat{i}+0.73\hat{j}+0.68\hat{k}$,\newline
$\vec{r}_{13}=0.0\hat{i}+0.0\hat{j}+10.0\hat{k}$,\;\;\;$\vec{r}_{24}=0.0\hat{i}+0.0\hat{j}+0.0\hat{k}$,\;\;\;$\vec{r}_{25}=10.0\hat{i}+10.0\hat{j}+10.0\hat{k}$.

2D-M404:

$\hat{n}_{13}=-0.11\hat{i}+0.58\hat{j}+0.81\hat{k}$,\;\;\;$\hat{n}_{14}=0.56\hat{i}+0.64\hat{j}-0.52\hat{k}$,\;\;\;$\hat{n}_{23}=0.58\hat{i}+0.54\hat{j}-0.61\hat{k}$,\;\;\;$\hat{n}_{25}=-0.81\hat{i}+0.39\hat{j}-0.44\hat{k}$,\newline
$\vec{r}_{13}=0.0\hat{i}+10.0\hat{j}+10.0\hat{k}$,\;\;\;$\vec{r}_{25}=0.0\hat{i}+0.0\hat{j}+10.0\hat{k}$,\;\;\;$\vec{r}_{45}=10.0\hat{i}+10.0\hat{j}+0.0\hat{k}$.

2D-M405:

$\hat{n}_{13}=0.0\hat{i}+0.0\hat{j}+1.0\hat{k}$,\;\;\;$\hat{n}_{14}=-0.48\hat{i}+0.53\hat{j}-0.7\hat{k}$,\;\;\;$\hat{n}_{23}=-0.59\hat{i}+0.52\hat{j}-0.62\hat{k}$,\;\;\;$\hat{n}_{45}=-0.0\hat{i}+0.8\hat{j}+0.6\hat{k}$,\newline
$\vec{r}_{13}=10.0\hat{i}+0.0\hat{j}+6.19\hat{k}$,\;\;\;$\vec{r}_{25}=0.0\hat{i}+10.0\hat{j}+10.0\hat{k}$,\;\;\;$\vec{r}_{45}=10.0\hat{i}+0.0\hat{j}+0.0\hat{k}$.

2D-M406:

$\hat{n}_{13}=0.67\hat{i}-0.34\hat{j}-0.66\hat{k}$,\;\;\;$\hat{n}_{14}=-0.27\hat{i}-0.83\hat{j}-0.48\hat{k}$,\;\;\;$\hat{n}_{23}=-0.38\hat{i}+0.86\hat{j}-0.33\hat{k}$,\;\;\;$\hat{n}_{25}=0.0\hat{i}+0.0\hat{j}-1.0\hat{k}$,\newline
$\vec{r}_{13}=0.0\hat{i}+10.0\hat{j}+10.0\hat{k}$,\;\;\;$\vec{r}_{23}=0.0\hat{i}+10.0\hat{j}+0.0\hat{k}$,\;\;\;$\vec{r}_{45}=10.0\hat{i}+10.0\hat{j}+10.0\hat{k}$.

2D-M407:

$\hat{n}_{13}=0.67\hat{i}+0.67\hat{j}-0.31\hat{k}$,\;\;\;$\hat{n}_{14}=0.8\hat{i}+0.6\hat{j}-0.0\hat{k}$,\;\;\;$\hat{n}_{23}=0.0\hat{i}+0.91\hat{j}-0.42\hat{k}$,\;\;\;$\hat{n}_{45}=-0.0\hat{i}+0.0\hat{j}-1.0\hat{k}$,\newline
$\vec{r}_{13}=0.0\hat{i}+10.0\hat{j}+10.0\hat{k}$,\;\;\;$\vec{r}_{23}=0.0\hat{i}+0.0\hat{j}+0.0\hat{k}$,\;\;\;$\vec{r}_{25}=10.0\hat{i}+0.0\hat{j}+10.0\hat{k}$.

2D-M408:

$\hat{n}_{13}=0.69\hat{i}-0.21\hat{j}+0.69\hat{k}$,\;\;\;$\hat{n}_{14}=-0.59\hat{i}-0.71\hat{j}+0.38\hat{k}$,\;\;\;$\hat{n}_{23}=0.0\hat{i}+0.47\hat{j}+0.88\hat{k}$,\;\;\;$\hat{n}_{45}=0.33\hat{i}+0.21\hat{j}+0.92\hat{k}$,\newline
$\vec{r}_{13}=0.0\hat{i}+10.0\hat{j}+0.0\hat{k}$,\;\;\;$\vec{r}_{23}=10.0\hat{i}+10.0\hat{j}+0.0\hat{k}$,\;\;\;$\vec{r}_{24}=0.0\hat{i}+0.0\hat{j}+10.0\hat{k}$.

2D-M409:

$\hat{n}_{13}=-0.8\hat{i}-0.57\hat{j}+0.16\hat{k}$,\;\;\;$\hat{n}_{14}=0.17\hat{i}-0.72\hat{j}+0.67\hat{k}$,\;\;\;$\hat{n}_{23}=0.04\hat{i}-0.93\hat{j}+0.37\hat{k}$,\;\;\;$\hat{n}_{35}=-0.46\hat{i}+0.71\hat{j}+0.53\hat{k}$,\newline
$\vec{r}_{13}=10.0\hat{i}+0.0\hat{j}+10.0\hat{k}$,\;\;\;$\vec{r}_{23}=6.94\hat{i}+4.88\hat{j}+3.97\hat{k}$,\;\;\;$\vec{r}_{24}=2.96\hat{i}+7.08\hat{j}+6.42\hat{k}$.

2D-M410:

$\hat{n}_{13}=-0.83\hat{i}-0.55\hat{j}+0.1\hat{k}$,\;\;\;$\hat{n}_{14}=0.53\hat{i}-0.48\hat{j}+0.7\hat{k}$,\;\;\;$\hat{n}_{23}=0.17\hat{i}-0.62\hat{j}-0.76\hat{k}$,\;\;\;$\hat{n}_{25}=0.69\hat{i}-0.72\hat{j}-0.07\hat{k}$,\newline
$\vec{r}_{13}=10.0\hat{i}+0.0\hat{j}+10.0\hat{k}$,\;\;\;$\vec{r}_{23}=0.0\hat{i}+10.0\hat{j}+10.0\hat{k}$,\;\;\;$\vec{r}_{24}=10.0\hat{i}+0.0\hat{j}+0.0\hat{k}$.

2D-M411:

$\hat{n}_{13}=-0.0\hat{i}+0.68\hat{j}-0.73\hat{k}$,\;\;\;$\hat{n}_{14}=0.36\hat{i}+0.72\hat{j}+0.59\hat{k}$,\;\;\;$\hat{n}_{25}=-0.0\hat{i}+0.69\hat{j}+0.73\hat{k}$,\;\;\;$\hat{n}_{45}=0.93\hat{i}-0.26\hat{j}-0.24\hat{k}$,\newline
$\vec{r}_{13}=10.0\hat{i}+10.0\hat{j}+10.0\hat{k}$,\;\;\;$\vec{r}_{23}=0.0\hat{i}+0.0\hat{j}+0.0\hat{k}$,\;\;\;$\vec{r}_{45}=10.0\hat{i}+10.0\hat{j}+10.0\hat{k}$.

2D-M412:

$\hat{n}_{13}=-0.58\hat{i}-0.58\hat{j}-0.58\hat{k}$,\;\;\;$\hat{n}_{14}=-0.77\hat{i}-0.48\hat{j}-0.43\hat{k}$,\;\;\;$\hat{n}_{25}=0.81\hat{i}-0.31\hat{j}-0.5\hat{k}$,\;\;\;$\hat{n}_{45}=-0.11\hat{i}+0.76\hat{j}-0.65\hat{k}$,\newline
$\vec{r}_{13}=0.0\hat{i}+10.0\hat{j}+0.0\hat{k}$,\;\;\;$\vec{r}_{23}=0.0\hat{i}+0.0\hat{j}+10.0\hat{k}$,\;\;\;$\vec{r}_{25}=10.0\hat{i}+0.0\hat{j}+0.0\hat{k}$.

2D-M413:

$\hat{n}_{13}=0.71\hat{i}-0.71\hat{j}-0.0\hat{k}$,\;\;\;$\hat{n}_{14}=0.7\hat{i}+0.7\hat{j}+0.16\hat{k}$,\;\;\;$\hat{n}_{24}=0.16\hat{i}+0.16\hat{j}-0.97\hat{k}$,\;\;\;$\hat{n}_{45}=0.0\hat{i}+0.0\hat{j}+1.0\hat{k}$,\newline
$\vec{r}_{13}=0.0\hat{i}+0.0\hat{j}+10.0\hat{k}$,\;\;\;$\vec{r}_{23}=10.0\hat{i}+10.0\hat{j}+0.0\hat{k}$,\;\;\;$\vec{r}_{24}=0.0\hat{i}+0.0\hat{j}+0.0\hat{k}$.

2D-M414:

$\hat{n}_{13}=-0.16\hat{i}+0.51\hat{j}-0.84\hat{k}$,\;\;\;$\hat{n}_{14}=-0.22\hat{i}-0.97\hat{j}-0.01\hat{k}$,\;\;\;$\hat{n}_{24}=-0.74\hat{i}-0.67\hat{j}-0.06\hat{k}$,\;\;\;$\hat{n}_{35}=-0.16\hat{i}+0.1\hat{j}+0.98\hat{k}$,\newline
$\vec{r}_{13}=10.0\hat{i}+0.0\hat{j}+10.0\hat{k}$,\;\;\;$\vec{r}_{23}=4.3\hat{i}+3.55\hat{j}+5.79\hat{k}$,\;\;\;$\vec{r}_{24}=7.0\hat{i}+7.51\hat{j}+6.9\hat{k}$.

2D-M415:

$\hat{n}_{13}=-0.35\hat{i}-0.66\hat{j}+0.66\hat{k}$,\;\;\;$\hat{n}_{14}=0.7\hat{i}-0.71\hat{j}+0.0\hat{k}$,\;\;\;$\hat{n}_{24}=0.0\hat{i}+0.0\hat{j}-1.0\hat{k}$,\;\;\;$\hat{n}_{25}=-0.0\hat{i}-0.0\hat{j}-1.0\hat{k}$,\newline
$\vec{r}_{13}=10.0\hat{i}+10.0\hat{j}+10.0\hat{k}$,\;\;\;$\vec{r}_{23}=0.0\hat{i}+10.0\hat{j}+0.0\hat{k}$,\;\;\;$\vec{r}_{24}=10.0\hat{i}+0.0\hat{j}+5.94\hat{k}$.

2D-M416:

$\hat{n}_{13}=0.0\hat{i}-0.71\hat{j}-0.71\hat{k}$,\;\;\;$\hat{n}_{14}=-0.82\hat{i}+0.41\hat{j}-0.41\hat{k}$,\;\;\;$\hat{n}_{24}=-0.0\hat{i}+0.71\hat{j}+0.71\hat{k}$,\;\;\;$\hat{n}_{25}=0.58\hat{i}+0.58\hat{j}-0.58\hat{k}$,\newline
$\vec{r}_{13}=10.0\hat{i}+10.0\hat{j}+0.0\hat{k}$,\;\;\;$\vec{r}_{14}=10.0\hat{i}+10.0\hat{j}+0.0\hat{k}$,\;\;\;$\vec{r}_{35}=0.0\hat{i}+0.0\hat{j}+10.0\hat{k}$.

2D-M417:

$\hat{n}_{13}=-0.79\hat{i}+0.28\hat{j}+0.55\hat{k}$,\;\;\;$\hat{n}_{14}=-0.93\hat{i}+0.25\hat{j}+0.25\hat{k}$,\;\;\;$\hat{n}_{24}=0.36\hat{i}+0.66\hat{j}+0.66\hat{k}$,\;\;\;$\hat{n}_{35}=-0.0\hat{i}+0.71\hat{j}+0.71\hat{k}$,\newline
$\vec{r}_{13}=10.0\hat{i}+10.0\hat{j}+10.0\hat{k}$,\;\;\;$\vec{r}_{14}=10.0\hat{i}+10.0\hat{j}+10.0\hat{k}$,\;\;\;$\vec{r}_{25}=0.0\hat{i}+0.0\hat{j}+0.0\hat{k}$.

2D-M418:

$\hat{n}_{13}=0.36\hat{i}+0.32\hat{j}+0.88\hat{k}$,\;\;\;$\hat{n}_{14}=-0.66\hat{i}+0.74\hat{j}-0.08\hat{k}$,\;\;\;$\hat{n}_{25}=-0.58\hat{i}-0.58\hat{j}-0.58\hat{k}$,\;\;\;$\hat{n}_{35}=0.58\hat{i}+0.58\hat{j}+0.58\hat{k}$,\newline
$\vec{r}_{13}=10.0\hat{i}+10.0\hat{j}+0.0\hat{k}$,\;\;\;$\vec{r}_{14}=10.0\hat{i}+10.0\hat{j}+10.0\hat{k}$,\;\;\;$\vec{r}_{24}=0.0\hat{i}+0.0\hat{j}+0.0\hat{k}$.

2D-M419:

$\hat{n}_{13}=-0.0\hat{i}+0.8\hat{j}-0.6\hat{k}$,\;\;\;$\hat{n}_{14}=0.0\hat{i}+0.0\hat{j}+1.0\hat{k}$,\;\;\;$\hat{n}_{23}=0.0\hat{i}+0.41\hat{j}-0.91\hat{k}$,\;\;\;$\hat{n}_{25}=0.74\hat{i}+0.67\hat{j}+0.09\hat{k}$,\newline
$\vec{r}_{13}=0.0\hat{i}+0.0\hat{j}+0.0\hat{k}$,\;\;\;$\vec{r}_{14}=10.0\hat{i}+10.0\hat{j}+9.66\hat{k}$,\;\;\;$\vec{r}_{45}=0.0\hat{i}+0.0\hat{j}+0.0\hat{k}$.

2D-M420:

$\hat{n}_{13}=0.0\hat{i}-0.0\hat{j}-1.0\hat{k}$,\;\;\;$\hat{n}_{14}=0.71\hat{i}-0.71\hat{j}+0.0\hat{k}$,\;\;\;$\hat{n}_{23}=-0.61\hat{i}-0.61\hat{j}+0.51\hat{k}$,\;\;\;$\hat{n}_{45}=-0.57\hat{i}-0.57\hat{j}+0.59\hat{k}$,\newline
$\vec{r}_{13}=0.0\hat{i}+0.0\hat{j}+9.49\hat{k}$,\;\;\;$\vec{r}_{14}=0.0\hat{i}+0.0\hat{j}+10.0\hat{k}$,\;\;\;$\vec{r}_{25}=10.0\hat{i}+10.0\hat{j}+0.0\hat{k}$.

2D-M421:

$\hat{n}_{13}=-0.41\hat{i}+0.41\hat{j}+0.82\hat{k}$,\;\;\;$\hat{n}_{14}=-0.71\hat{i}-0.71\hat{j}+0.0\hat{k}$,\;\;\;$\hat{n}_{23}=-0.58\hat{i}+0.58\hat{j}-0.58\hat{k}$,\;\;\;$\hat{n}_{45}=0.0\hat{i}+0.0\hat{j}+1.0\hat{k}$,\newline
$\vec{r}_{13}=0.0\hat{i}+10.0\hat{j}+10.0\hat{k}$,\;\;\;$\vec{r}_{14}=0.0\hat{i}+10.0\hat{j}+10.0\hat{k}$,\;\;\;$\vec{r}_{24}=10.0\hat{i}+0.0\hat{j}+0.0\hat{k}$.

2D-M422:

$\hat{n}_{13}=-0.51\hat{i}+0.32\hat{j}+0.8\hat{k}$,\;\;\;$\hat{n}_{14}=-0.9\hat{i}-0.21\hat{j}-0.39\hat{k}$,\;\;\;$\hat{n}_{23}=-0.48\hat{i}-0.56\hat{j}+0.68\hat{k}$,\;\;\;$\hat{n}_{35}=-0.37\hat{i}+0.25\hat{j}+0.89\hat{k}$,\newline
$\vec{r}_{13}=0.0\hat{i}+10.0\hat{j}+10.0\hat{k}$,\;\;\;$\vec{r}_{14}=4.23\hat{i}+2.59\hat{j}+4.81\hat{k}$,\;\;\;$\vec{r}_{24}=6.61\hat{i}+8.27\hat{j}+8.93\hat{k}$.

2D-M423:

$\hat{n}_{13}=-0.0\hat{i}+0.45\hat{j}+0.9\hat{k}$,\;\;\;$\hat{n}_{14}=0.68\hat{i}-0.71\hat{j}+0.16\hat{k}$,\;\;\;$\hat{n}_{23}=0.49\hat{i}+0.67\hat{j}+0.56\hat{k}$,\;\;\;$\hat{n}_{25}=-0.01\hat{i}+0.25\hat{j}+0.97\hat{k}$,\newline
$\vec{r}_{13}=10.0\hat{i}+10.0\hat{j}+0.0\hat{k}$,\;\;\;$\vec{r}_{14}=10.0\hat{i}+10.0\hat{j}+10.0\hat{k}$,\;\;\;$\vec{r}_{24}=0.0\hat{i}+0.0\hat{j}+0.0\hat{k}$.

2D-M424:

$\hat{n}_{13}=-0.81\hat{i}+0.29\hat{j}-0.51\hat{k}$,\;\;\;$\hat{n}_{14}=-0.0\hat{i}+0.93\hat{j}+0.38\hat{k}$,\;\;\;$\hat{n}_{25}=0.37\hat{i}+0.63\hat{j}-0.68\hat{k}$,\;\;\;$\hat{n}_{45}=-0.0\hat{i}-0.0\hat{j}-1.0\hat{k}$,\newline
$\vec{r}_{13}=10.0\hat{i}+10.0\hat{j}+0.0\hat{k}$,\;\;\;$\vec{r}_{14}=10.0\hat{i}+9.68\hat{j}+0.0\hat{k}$,\;\;\;$\vec{r}_{23}=0.0\hat{i}+0.0\hat{j}+10.0\hat{k}$.

2D-M425:

$\hat{n}_{13}=-0.0\hat{i}+0.0\hat{j}+1.0\hat{k}$,\;\;\;$\hat{n}_{14}=-0.71\hat{i}-0.71\hat{j}-0.0\hat{k}$,\;\;\;$\hat{n}_{24}=0.58\hat{i}-0.58\hat{j}-0.58\hat{k}$,\;\;\;$\hat{n}_{45}=-0.0\hat{i}+0.0\hat{j}+1.0\hat{k}$,\newline
$\vec{r}_{13}=10.0\hat{i}+0.0\hat{j}+0.0\hat{k}$,\;\;\;$\vec{r}_{14}=10.0\hat{i}+0.0\hat{j}+10.0\hat{k}$,\;\;\;$\vec{r}_{23}=0.0\hat{i}+10.0\hat{j}+0.0\hat{k}$.

2D-M426:

$\hat{n}_{13}=-0.32\hat{i}-0.67\hat{j}+0.67\hat{k}$,\;\;\;$\hat{n}_{14}=-0.46\hat{i}-0.88\hat{j}+0.12\hat{k}$,\;\;\;$\hat{n}_{24}=0.28\hat{i}-0.96\hat{j}+0.02\hat{k}$,\;\;\;$\hat{n}_{35}=0.38\hat{i}+0.55\hat{j}-0.74\hat{k}$,\newline
$\vec{r}_{13}=10.0\hat{i}+0.0\hat{j}+10.0\hat{k}$,\;\;\;$\vec{r}_{14}=3.68\hat{i}+6.31\hat{j}+4.84\hat{k}$,\;\;\;$\vec{r}_{23}=3.98\hat{i}+3.51\hat{j}+1.89\hat{k}$.

2D-M427:

$\hat{n}_{13}=-0.0\hat{i}+0.18\hat{j}-0.98\hat{k}$,\;\;\;$\hat{n}_{14}=-0.0\hat{i}+0.83\hat{j}+0.56\hat{k}$,\;\;\;$\hat{n}_{24}=-0.61\hat{i}+0.45\hat{j}-0.66\hat{k}$,\;\;\;$\hat{n}_{25}=0.0\hat{i}+0.0\hat{j}+1.0\hat{k}$,\newline
$\vec{r}_{13}=10.0\hat{i}+0.0\hat{j}+10.0\hat{k}$,\;\;\;$\vec{r}_{14}=10.0\hat{i}+0.0\hat{j}+0.0\hat{k}$,\;\;\;$\vec{r}_{23}=0.0\hat{i}+10.0\hat{j}+10.0\hat{k}$.

2D-M428:

$\hat{n}_{13}=-0.52\hat{i}-0.11\hat{j}-0.85\hat{k}$,\;\;\;$\hat{n}_{24}=0.04\hat{i}-0.63\hat{j}+0.77\hat{k}$,\;\;\;$\hat{n}_{25}=0.59\hat{i}-0.61\hat{j}-0.53\hat{k}$,\;\;\;$\hat{n}_{35}=-0.0\hat{i}+0.65\hat{j}-0.76\hat{k}$,\newline
$\vec{r}_{13}=10.0\hat{i}+10.0\hat{j}+0.0\hat{k}$,\;\;\;$\vec{r}_{14}=10.0\hat{i}+0.0\hat{j}+10.0\hat{k}$,\;\;\;$\vec{r}_{35}=0.0\hat{i}+10.0\hat{j}+0.0\hat{k}$.

2D-M429:

$\hat{n}_{13}=-0.0\hat{i}+0.68\hat{j}-0.73\hat{k}$,\;\;\;$\hat{n}_{24}=-0.0\hat{i}+0.68\hat{j}-0.74\hat{k}$,\;\;\;$\hat{n}_{25}=-0.91\hat{i}+0.14\hat{j}-0.4\hat{k}$,\;\;\;$\hat{n}_{35}=-0.29\hat{i}-0.6\hat{j}+0.74\hat{k}$,\newline
$\vec{r}_{13}=10.0\hat{i}+0.0\hat{j}+10.0\hat{k}$,\;\;\;$\vec{r}_{14}=10.0\hat{i}+10.0\hat{j}+0.0\hat{k}$,\;\;\;$\vec{r}_{25}=0.0\hat{i}+0.0\hat{j}+10.0\hat{k}$.

2D-M430:

$\hat{n}_{13}=0.53\hat{i}-0.27\hat{j}-0.8\hat{k}$,\;\;\;$\hat{n}_{24}=0.0\hat{i}+0.9\hat{j}+0.43\hat{k}$,\;\;\;$\hat{n}_{25}=0.6\hat{i}-0.34\hat{j}+0.72\hat{k}$,\;\;\;$\hat{n}_{35}=0.0\hat{i}-0.0\hat{j}+1.0\hat{k}$,\newline
$\vec{r}_{13}=0.0\hat{i}+10.0\hat{j}+10.0\hat{k}$,\;\;\;$\vec{r}_{14}=10.0\hat{i}+0.0\hat{j}+0.0\hat{k}$,\;\;\;$\vec{r}_{24}=0.0\hat{i}+10.0\hat{j}+10.0\hat{k}$.

2D-M431:

$\hat{n}_{13}=0.82\hat{i}-0.41\hat{j}+0.41\hat{k}$,\;\;\;$\hat{n}_{23}=-0.82\hat{i}+0.41\hat{j}-0.41\hat{k}$,\;\;\;$\hat{n}_{25}=-0.58\hat{i}-0.6\hat{j}+0.55\hat{k}$,\;\;\;$\hat{n}_{45}=0.04\hat{i}-0.66\hat{j}-0.75\hat{k}$,\newline
$\vec{r}_{13}=10.0\hat{i}+10.0\hat{j}+0.0\hat{k}$,\;\;\;$\vec{r}_{14}=0.0\hat{i}+0.0\hat{j}+10.0\hat{k}$,\;\;\;$\vec{r}_{45}=10.0\hat{i}+10.0\hat{j}+0.0\hat{k}$.

2D-M432:

$\hat{n}_{13}=0.68\hat{i}+0.55\hat{j}-0.49\hat{k}$,\;\;\;$\hat{n}_{23}=-0.78\hat{i}-0.54\hat{j}-0.33\hat{k}$,\;\;\;$\hat{n}_{25}=0.42\hat{i}-0.83\hat{j}+0.37\hat{k}$,\;\;\;$\hat{n}_{45}=-0.59\hat{i}-0.56\hat{j}-0.58\hat{k}$,\newline
$\vec{r}_{13}=10.0\hat{i}+0.0\hat{j}+0.0\hat{k}$,\;\;\;$\vec{r}_{14}=0.0\hat{i}+0.0\hat{j}+0.0\hat{k}$,\;\;\;$\vec{r}_{25}=10.0\hat{i}+10.0\hat{j}+10.0\hat{k}$.

2D-M433:

$\hat{n}_{13}=0.26\hat{i}-0.46\hat{j}-0.85\hat{k}$,\;\;\;$\hat{n}_{23}=-0.58\hat{i}+0.58\hat{j}-0.58\hat{k}$,\;\;\;$\hat{n}_{24}=0.2\hat{i}-0.59\hat{j}-0.78\hat{k}$,\;\;\;$\hat{n}_{45}=0.0\hat{i}-0.0\hat{j}-1.0\hat{k}$,\newline
$\vec{r}_{13}=10.0\hat{i}+0.0\hat{j}+0.0\hat{k}$,\;\;\;$\vec{r}_{14}=10.0\hat{i}+0.0\hat{j}+0.0\hat{k}$,\;\;\;$\vec{r}_{24}=0.0\hat{i}+10.0\hat{j}+10.0\hat{k}$.

2D-M434:

$\hat{n}_{13}=0.4\hat{i}+0.67\hat{j}-0.62\hat{k}$,\;\;\;$\hat{n}_{23}=-0.22\hat{i}-0.97\hat{j}-0.01\hat{k}$,\;\;\;$\hat{n}_{24}=0.65\hat{i}-0.76\hat{j}-0.08\hat{k}$,\;\;\;$\hat{n}_{35}=-0.58\hat{i}+0.2\hat{j}+0.79\hat{k}$,\newline
$\vec{r}_{13}=10.0\hat{i}+0.0\hat{j}+10.0\hat{k}$,\;\;\;$\vec{r}_{14}=4.67\hat{i}+5.1\hat{j}+4.86\hat{k}$,\;\;\;$\vec{r}_{24}=5.46\hat{i}+4.73\hat{j}+5.25\hat{k}$.

2D-M435:

$\hat{n}_{13}=0.81\hat{i}-0.22\hat{j}-0.54\hat{k}$,\;\;\;$\hat{n}_{23}=0.58\hat{i}+0.49\hat{j}+0.65\hat{k}$,\;\;\;$\hat{n}_{24}=0.01\hat{i}-0.9\hat{j}+0.44\hat{k}$,\;\;\;$\hat{n}_{25}=-0.0\hat{i}+0.0\hat{j}-1.0\hat{k}$,\newline
$\vec{r}_{13}=0.0\hat{i}+0.0\hat{j}+0.0\hat{k}$,\;\;\;$\vec{r}_{14}=10.0\hat{i}+10.0\hat{j}+10.0\hat{k}$,\;\;\;$\vec{r}_{24}=0.0\hat{i}+0.0\hat{j}+0.0\hat{k}$.

2D-M436:

$\hat{n}_{13}=0.0\hat{i}+0.58\hat{j}-0.81\hat{k}$,\;\;\;$\hat{n}_{23}=0.0\hat{i}+0.71\hat{j}-0.71\hat{k}$,\;\;\;$\hat{n}_{25}=-0.57\hat{i}-0.58\hat{j}-0.58\hat{k}$,\;\;\;$\hat{n}_{45}=0.58\hat{i}+0.58\hat{j}+0.58\hat{k}$,\newline
$\vec{r}_{13}=10.0\hat{i}+10.0\hat{j}+10.0\hat{k}$,\;\;\;$\vec{r}_{14}=10.0\hat{i}+10.0\hat{j}+10.0\hat{k}$,\;\;\;$\vec{r}_{23}=0.0\hat{i}+0.0\hat{j}+0.0\hat{k}$.

2D-M437:

$\hat{n}_{13}=0.63\hat{i}-0.02\hat{j}-0.77\hat{k}$,\;\;\;$\hat{n}_{23}=0.0\hat{i}+0.71\hat{j}+0.71\hat{k}$,\;\;\;$\hat{n}_{24}=-0.58\hat{i}+0.58\hat{j}-0.58\hat{k}$,\;\;\;$\hat{n}_{45}=-0.88\hat{i}+0.35\hat{j}-0.31\hat{k}$,\newline
$\vec{r}_{13}=0.0\hat{i}+10.0\hat{j}+10.0\hat{k}$,\;\;\;$\vec{r}_{14}=0.0\hat{i}+10.0\hat{j}+10.0\hat{k}$,\;\;\;$\vec{r}_{23}=10.0\hat{i}+0.0\hat{j}+0.0\hat{k}$.

2D-M438:

$\hat{n}_{13}=-0.0\hat{i}-0.0\hat{j}-1.0\hat{k}$,\;\;\;$\hat{n}_{23}=-0.04\hat{i}-0.67\hat{j}+0.74\hat{k}$,\;\;\;$\hat{n}_{24}=0.13\hat{i}-0.38\hat{j}+0.92\hat{k}$,\;\;\;$\hat{n}_{35}=0.01\hat{i}+0.0\hat{j}-1.0\hat{k}$,\newline
$\vec{r}_{13}=10.0\hat{i}+0.0\hat{j}+3.41\hat{k}$,\;\;\;$\vec{r}_{14}=4.67\hat{i}+5.79\hat{j}+5.32\hat{k}$,\;\;\;$\vec{r}_{23}=5.13\hat{i}+3.54\hat{j}+6.94\hat{k}$.

2D-M439:

$\hat{n}_{13}=0.17\hat{i}+0.67\hat{j}+0.72\hat{k}$,\;\;\;$\hat{n}_{23}=0.72\hat{i}-0.66\hat{j}+0.23\hat{k}$,\;\;\;$\hat{n}_{24}=-0.51\hat{i}-0.61\hat{j}+0.61\hat{k}$,\;\;\;$\hat{n}_{25}=-0.01\hat{i}+0.61\hat{j}+0.8\hat{k}$,\newline
$\vec{r}_{13}=10.0\hat{i}+0.0\hat{j}+0.0\hat{k}$,\;\;\;$\vec{r}_{14}=0.0\hat{i}+0.0\hat{j}+10.0\hat{k}$,\;\;\;$\vec{r}_{23}=10.0\hat{i}+10.0\hat{j}+0.0\hat{k}$.

2D-M440:

$\hat{n}_{13}=0.0\hat{i}+0.67\hat{j}-0.74\hat{k}$,\;\;\;$\hat{n}_{14}=-0.21\hat{i}+0.03\hat{j}-0.98\hat{k}$,\;\;\;$\hat{n}_{24}=-0.57\hat{i}-0.11\hat{j}+0.82\hat{k}$,\;\;\;$\hat{n}_{25}=-0.49\hat{i}-0.87\hat{j}+0.08\hat{k}$,\newline
$\vec{r}_{24}=10.0\hat{i}+10.0\hat{j}+10.0\hat{k}$,\;\;\;$\vec{r}_{25}=10.0\hat{i}+0.0\hat{j}+0.0\hat{k}$,\;\;\;$\vec{r}_{35}=0.0\hat{i}+10.0\hat{j}+10.0\hat{k}$.

2D-M441:

$\hat{n}_{13}=-0.44\hat{i}-0.65\hat{j}+0.62\hat{k}$,\;\;\;$\hat{n}_{14}=0.0\hat{i}+0.71\hat{j}+0.7\hat{k}$,\;\;\;$\hat{n}_{24}=-0.0\hat{i}+0.71\hat{j}+0.7\hat{k}$,\;\;\;$\hat{n}_{35}=0.06\hat{i}-0.71\hat{j}-0.7\hat{k}$,\newline
$\vec{r}_{24}=0.0\hat{i}+0.0\hat{j}+10.0\hat{k}$,\;\;\;$\vec{r}_{25}=0.0\hat{i}+10.0\hat{j}+10.0\hat{k}$,\;\;\;$\vec{r}_{35}=10.0\hat{i}+10.0\hat{j}+0.0\hat{k}$.

2D-M442:

$\hat{n}_{13}=-0.5\hat{i}-0.62\hat{j}+0.61\hat{k}$,\;\;\;$\hat{n}_{14}=-0.78\hat{i}-0.62\hat{j}+0.04\hat{k}$,\;\;\;$\hat{n}_{24}=-0.52\hat{i}+0.61\hat{j}-0.6\hat{k}$,\;\;\;$\hat{n}_{25}=-0.0\hat{i}+0.78\hat{j}+0.63\hat{k}$,\newline
$\vec{r}_{24}=10.0\hat{i}+10.0\hat{j}+0.0\hat{k}$,\;\;\;$\vec{r}_{25}=10.0\hat{i}+0.0\hat{j}+0.0\hat{k}$,\;\;\;$\vec{r}_{35}=0.0\hat{i}+0.0\hat{j}+10.0\hat{k}$.

2D-M443:

$\hat{n}_{13}=0.0\hat{i}-0.0\hat{j}+1.0\hat{k}$,\;\;\;$\hat{n}_{14}=-0.72\hat{i}-0.68\hat{j}+0.15\hat{k}$,\;\;\;$\hat{n}_{24}=-0.0\hat{i}+0.21\hat{j}+0.98\hat{k}$,\;\;\;$\hat{n}_{35}=0.46\hat{i}-0.61\hat{j}-0.65\hat{k}$,\newline
$\vec{r}_{24}=0.0\hat{i}+0.0\hat{j}+10.0\hat{k}$,\;\;\;$\vec{r}_{25}=10.0\hat{i}+10.0\hat{j}+10.0\hat{k}$,\;\;\;$\vec{r}_{35}=10.0\hat{i}+0.0\hat{j}+0.0\hat{k}$.

2D-M444:

$\hat{n}_{13}=0.0\hat{i}+0.97\hat{j}-0.23\hat{k}$,\;\;\;$\hat{n}_{14}=0.0\hat{i}+0.0\hat{j}+1.0\hat{k}$,\;\;\;$\hat{n}_{25}=-0.37\hat{i}-0.66\hat{j}-0.66\hat{k}$,\;\;\;$\hat{n}_{35}=0.34\hat{i}+0.03\hat{j}-0.94\hat{k}$,\newline
$\vec{r}_{24}=0.0\hat{i}+10.0\hat{j}+10.0\hat{k}$,\;\;\;$\vec{r}_{25}=10.0\hat{i}+10.0\hat{j}+0.0\hat{k}$,\;\;\;$\vec{r}_{35}=10.0\hat{i}+0.0\hat{j}+0.0\hat{k}$.

2D-M445:

$\hat{n}_{13}=-0.0\hat{i}+0.0\hat{j}+1.0\hat{k}$,\;\;\;$\hat{n}_{14}=0.71\hat{i}-0.71\hat{j}+0.0\hat{k}$,\;\;\;$\hat{n}_{25}=0.0\hat{i}-0.0\hat{j}-1.0\hat{k}$,\;\;\;$\hat{n}_{35}=0.5\hat{i}+0.51\hat{j}+0.7\hat{k}$,\newline
$\vec{r}_{24}=10.0\hat{i}+0.0\hat{j}+10.0\hat{k}$,\;\;\;$\vec{r}_{25}=0.0\hat{i}+10.0\hat{j}+0.12\hat{k}$,\;\;\;$\vec{r}_{35}=10.0\hat{i}+10.0\hat{j}+0.0\hat{k}$.

2D-M446:

$\hat{n}_{13}=0.0\hat{i}+0.71\hat{j}-0.71\hat{k}$,\;\;\;$\hat{n}_{14}=-0.44\hat{i}+0.64\hat{j}-0.64\hat{k}$,\;\;\;$\hat{n}_{23}=0.9\hat{i}+0.31\hat{j}-0.31\hat{k}$,\;\;\;$\hat{n}_{45}=-0.81\hat{i}+0.36\hat{j}-0.46\hat{k}$,\newline
$\vec{r}_{23}=0.0\hat{i}+10.0\hat{j}+10.0\hat{k}$,\;\;\;$\vec{r}_{24}=10.0\hat{i}+0.0\hat{j}+0.0\hat{k}$,\;\;\;$\vec{r}_{45}=10.0\hat{i}+10.0\hat{j}+0.0\hat{k}$.

2D-M447:

$\hat{n}_{13}=-0.33\hat{i}-0.07\hat{j}-0.94\hat{k}$,\;\;\;$\hat{n}_{14}=-0.39\hat{i}-0.92\hat{j}+0.03\hat{k}$,\;\;\;$\hat{n}_{23}=-0.34\hat{i}-0.94\hat{j}-0.0\hat{k}$,\;\;\;$\hat{n}_{35}=-0.09\hat{i}-0.53\hat{j}+0.84\hat{k}$,\newline
$\vec{r}_{23}=6.79\hat{i}+4.98\hat{j}+4.77\hat{k}$,\;\;\;$\vec{r}_{24}=4.49\hat{i}+5.46\hat{j}+4.46\hat{k}$,\;\;\;$\vec{r}_{35}=10.0\hat{i}+10.0\hat{j}+10.0\hat{k}$.

2D-M448:

$\hat{n}_{13}=0.0\hat{i}-0.0\hat{j}-1.0\hat{k}$,\;\;\;$\hat{n}_{14}=-0.54\hat{i}-0.58\hat{j}-0.61\hat{k}$,\;\;\;$\hat{n}_{23}=-0.77\hat{i}+0.64\hat{j}+0.07\hat{k}$,\;\;\;$\hat{n}_{25}=-0.56\hat{i}-0.43\hat{j}+0.71\hat{k}$,\newline
$\vec{r}_{23}=0.0\hat{i}+0.0\hat{j}+0.0\hat{k}$,\;\;\;$\vec{r}_{24}=10.0\hat{i}+10.0\hat{j}+10.0\hat{k}$,\;\;\;$\vec{r}_{25}=0.0\hat{i}+0.0\hat{j}+0.0\hat{k}$.

2D-M449:

$\hat{n}_{13}=0.0\hat{i}+0.02\hat{j}-1.0\hat{k}$,\;\;\;$\hat{n}_{14}=0.43\hat{i}+0.38\hat{j}-0.82\hat{k}$,\;\;\;$\hat{n}_{24}=0.0\hat{i}+0.0\hat{j}+1.0\hat{k}$,\;\;\;$\hat{n}_{25}=0.58\hat{i}+0.58\hat{j}+0.58\hat{k}$,\newline
$\vec{r}_{14}=10.0\hat{i}+10.0\hat{j}+10.0\hat{k}$,\;\;\;$\vec{r}_{24}=0.0\hat{i}+0.0\hat{j}+9.97\hat{k}$,\;\;\;$\vec{r}_{35}=0.0\hat{i}+0.0\hat{j}+0.0\hat{k}$.

2D-M450:

$\hat{n}_{13}=0.0\hat{i}+0.0\hat{j}+1.0\hat{k}$,\;\;\;$\hat{n}_{14}=0.55\hat{i}+0.37\hat{j}+0.75\hat{k}$,\;\;\;$\hat{n}_{24}=-0.58\hat{i}-0.57\hat{j}+0.58\hat{k}$,\;\;\;$\hat{n}_{35}=-0.65\hat{i}+0.76\hat{j}+0.06\hat{k}$,\newline
$\vec{r}_{14}=10.0\hat{i}+0.0\hat{j}+10.0\hat{k}$,\;\;\;$\vec{r}_{24}=0.0\hat{i}+0.0\hat{j}+0.0\hat{k}$,\;\;\;$\vec{r}_{25}=0.0\hat{i}+10.0\hat{j}+10.0\hat{k}$.

2D-M451:

$\hat{n}_{13}=-0.0\hat{i}-0.0\hat{j}+1.0\hat{k}$,\;\;\;$\hat{n}_{14}=0.52\hat{i}+0.66\hat{j}+0.54\hat{k}$,\;\;\;$\hat{n}_{24}=0.0\hat{i}+0.81\hat{j}-0.59\hat{k}$,\;\;\;$\hat{n}_{25}=0.0\hat{i}-0.0\hat{j}+1.0\hat{k}$,\newline
$\vec{r}_{14}=10.0\hat{i}+0.0\hat{j}+0.0\hat{k}$,\;\;\;$\vec{r}_{25}=0.0\hat{i}+0.0\hat{j}+9.14\hat{k}$,\;\;\;$\vec{r}_{35}=0.0\hat{i}+10.0\hat{j}+10.0\hat{k}$.

2D-M452:

$\hat{n}_{13}=-0.22\hat{i}-0.25\hat{j}+0.94\hat{k}$,\;\;\;$\hat{n}_{14}=-0.05\hat{i}-0.91\hat{j}+0.41\hat{k}$,\;\;\;$\hat{n}_{24}=-0.13\hat{i}-0.99\hat{j}+0.01\hat{k}$,\;\;\;$\hat{n}_{35}=0.58\hat{i}-0.23\hat{j}-0.78\hat{k}$,\newline
$\vec{r}_{14}=6.43\hat{i}+5.67\hat{j}+3.93\hat{k}$,\;\;\;$\vec{r}_{25}=5.8\hat{i}+5.18\hat{j}+4.73\hat{k}$,\;\;\;$\vec{r}_{35}=10.0\hat{i}+0.0\hat{j}+0.0\hat{k}$.

2D-M453:

$\hat{n}_{13}=0.0\hat{i}+0.0\hat{j}+1.0\hat{k}$,\;\;\;$\hat{n}_{14}=0.57\hat{i}-0.36\hat{j}-0.74\hat{k}$,\;\;\;$\hat{n}_{25}=0.11\hat{i}-0.7\hat{j}+0.7\hat{k}$,\;\;\;$\hat{n}_{35}=0.82\hat{i}+0.51\hat{j}+0.25\hat{k}$,\newline
$\vec{r}_{14}=10.0\hat{i}+10.0\hat{j}+10.0\hat{k}$,\;\;\;$\vec{r}_{24}=0.0\hat{i}+0.0\hat{j}+0.0\hat{k}$,\;\;\;$\vec{r}_{25}=10.0\hat{i}+0.0\hat{j}+10.0\hat{k}$.

2D-M454:

$\hat{n}_{13}=0.73\hat{i}+0.19\hat{j}-0.66\hat{k}$,\;\;\;$\hat{n}_{14}=-0.07\hat{i}-0.92\hat{j}+0.39\hat{k}$,\;\;\;$\hat{n}_{25}=-0.5\hat{i}-0.75\hat{j}+0.43\hat{k}$,\;\;\;$\hat{n}_{35}=-0.82\hat{i}-0.06\hat{j}+0.57\hat{k}$,\newline
$\vec{r}_{14}=3.86\hat{i}+3.2\hat{j}+5.51\hat{k}$,\;\;\;$\vec{r}_{24}=3.91\hat{i}+5.01\hat{j}+4.94\hat{k}$,\;\;\;$\vec{r}_{35}=10.0\hat{i}+0.0\hat{j}+0.0\hat{k}$.

2D-M455:

$\hat{n}_{13}=0.0\hat{i}+0.0\hat{j}+1.0\hat{k}$,\;\;\;$\hat{n}_{14}=-0.34\hat{i}+0.34\hat{j}+0.88\hat{k}$,\;\;\;$\hat{n}_{23}=0.46\hat{i}-0.4\hat{j}-0.79\hat{k}$,\;\;\;$\hat{n}_{25}=-0.67\hat{i}+0.67\hat{j}-0.33\hat{k}$,\newline
$\vec{r}_{14}=10.0\hat{i}+0.0\hat{j}+0.0\hat{k}$,\;\;\;$\vec{r}_{23}=0.0\hat{i}+10.0\hat{j}+10.0\hat{k}$,\;\;\;$\vec{r}_{45}=0.0\hat{i}+10.0\hat{j}+10.0\hat{k}$.

2D-M456:

$\hat{n}_{13}=-0.0\hat{i}+0.0\hat{j}-1.0\hat{k}$,\;\;\;$\hat{n}_{14}=-0.82\hat{i}-0.48\hat{j}-0.31\hat{k}$,\;\;\;$\hat{n}_{23}=0.25\hat{i}-0.55\hat{j}+0.8\hat{k}$,\;\;\;$\hat{n}_{45}=-0.56\hat{i}+0.55\hat{j}+0.62\hat{k}$,\newline
$\vec{r}_{14}=10.0\hat{i}+0.0\hat{j}+10.0\hat{k}$,\;\;\;$\vec{r}_{23}=10.0\hat{i}+0.0\hat{j}+10.0\hat{k}$,\;\;\;$\vec{r}_{25}=0.0\hat{i}+10.0\hat{j}+0.0\hat{k}$.

2D-M457:

$\hat{n}_{13}=0.0\hat{i}+0.81\hat{j}-0.58\hat{k}$,\;\;\;$\hat{n}_{14}=-0.0\hat{i}+0.58\hat{j}+0.81\hat{k}$,\;\;\;$\hat{n}_{23}=0.0\hat{i}+0.71\hat{j}+0.71\hat{k}$,\;\;\;$\hat{n}_{45}=-0.27\hat{i}+0.2\hat{j}+0.94\hat{k}$,\newline
$\vec{r}_{14}=10.0\hat{i}+10.0\hat{j}+0.0\hat{k}$,\;\;\;$\vec{r}_{23}=0.0\hat{i}+0.0\hat{j}+10.0\hat{k}$,\;\;\;$\vec{r}_{24}=10.0\hat{i}+0.0\hat{j}+0.0\hat{k}$.

2D-M458:

$\hat{n}_{13}=-0.71\hat{i}-0.69\hat{j}-0.12\hat{k}$,\;\;\;$\hat{n}_{14}=0.06\hat{i}-0.96\hat{j}+0.26\hat{k}$,\;\;\;$\hat{n}_{23}=-0.31\hat{i}-0.95\hat{j}-0.01\hat{k}$,\;\;\;$\hat{n}_{35}=0.66\hat{i}-0.72\hat{j}+0.22\hat{k}$,\newline
$\vec{r}_{14}=3.78\hat{i}+4.2\hat{j}+4.49\hat{k}$,\;\;\;$\vec{r}_{23}=3.7\hat{i}+4.48\hat{j}+5.93\hat{k}$,\;\;\;$\vec{r}_{24}=5.24\hat{i}+4.23\hat{j}+5.86\hat{k}$.

2D-M459:

$\hat{n}_{13}=0.0\hat{i}+0.0\hat{j}+1.0\hat{k}$,\;\;\;$\hat{n}_{14}=0.86\hat{i}+0.15\hat{j}+0.49\hat{k}$,\;\;\;$\hat{n}_{23}=0.2\hat{i}+0.58\hat{j}-0.79\hat{k}$,\;\;\;$\hat{n}_{25}=0.35\hat{i}+0.93\hat{j}+0.09\hat{k}$,\newline
$\vec{r}_{14}=10.0\hat{i}+0.0\hat{j}+10.0\hat{k}$,\;\;\;$\vec{r}_{23}=10.0\hat{i}+10.0\hat{j}+10.0\hat{k}$,\;\;\;$\vec{r}_{24}=0.0\hat{i}+0.0\hat{j}+0.0\hat{k}$.

2D-M460:

$\hat{n}_{13}=0.61\hat{i}-0.59\hat{j}-0.53\hat{k}$,\;\;\;$\hat{n}_{14}=0.0\hat{i}+0.02\hat{j}-1.0\hat{k}$,\;\;\;$\hat{n}_{23}=0.61\hat{i}+0.77\hat{j}-0.17\hat{k}$,\;\;\;$\hat{n}_{25}=-0.17\hat{i}-0.98\hat{j}+0.06\hat{k}$,\newline
$\vec{r}_{14}=10.0\hat{i}+10.0\hat{j}+10.0\hat{k}$,\;\;\;$\vec{r}_{25}=0.0\hat{i}+10.0\hat{j}+0.0\hat{k}$,\;\;\;$\vec{r}_{45}=0.0\hat{i}+0.0\hat{j}+10.0\hat{k}$.

2D-M461:

$\hat{n}_{13}=0.12\hat{i}+0.65\hat{j}+0.75\hat{k}$,\;\;\;$\hat{n}_{14}=-0.21\hat{i}-0.59\hat{j}-0.78\hat{k}$,\;\;\;$\hat{n}_{23}=-0.65\hat{i}-0.52\hat{j}+0.55\hat{k}$,\;\;\;$\hat{n}_{45}=0.0\hat{i}+0.8\hat{j}+0.59\hat{k}$,\newline
$\vec{r}_{14}=10.0\hat{i}+10.0\hat{j}+0.0\hat{k}$,\;\;\;$\vec{r}_{25}=0.0\hat{i}+0.0\hat{j}+10.0\hat{k}$,\;\;\;$\vec{r}_{45}=0.0\hat{i}+10.0\hat{j}+10.0\hat{k}$.

2D-M462:

$\hat{n}_{13}=-0.0\hat{i}+0.71\hat{j}-0.71\hat{k}$,\;\;\;$\hat{n}_{14}=0.0\hat{i}+0.71\hat{j}-0.71\hat{k}$,\;\;\;$\hat{n}_{23}=0.58\hat{i}+0.58\hat{j}+0.58\hat{k}$,\;\;\;$\hat{n}_{45}=0.79\hat{i}-0.28\hat{j}+0.55\hat{k}$,\newline
$\vec{r}_{14}=0.0\hat{i}+0.0\hat{j}+0.0\hat{k}$,\;\;\;$\vec{r}_{24}=10.0\hat{i}+10.0\hat{j}+10.0\hat{k}$,\;\;\;$\vec{r}_{45}=10.0\hat{i}+10.0\hat{j}+0.0\hat{k}$.

2D-M463:

$\hat{n}_{13}=-0.24\hat{i}+0.33\hat{j}+0.91\hat{k}$,\;\;\;$\hat{n}_{14}=-0.16\hat{i}-0.98\hat{j}-0.1\hat{k}$,\;\;\;$\hat{n}_{23}=-0.52\hat{i}-0.86\hat{j}+0.03\hat{k}$,\;\;\;$\hat{n}_{35}=-0.3\hat{i}+0.44\hat{j}+0.85\hat{k}$,\newline
$\vec{r}_{14}=5.64\hat{i}+4.51\hat{j}+4.3\hat{k}$,\;\;\;$\vec{r}_{24}=5.55\hat{i}+5.55\hat{j}+4.32\hat{k}$,\;\;\;$\vec{r}_{35}=10.0\hat{i}+0.0\hat{j}+0.0\hat{k}$.

2D-M464:

$\hat{n}_{13}=0.67\hat{i}+0.74\hat{j}-0.07\hat{k}$,\;\;\;$\hat{n}_{14}=0.12\hat{i}+0.76\hat{j}-0.64\hat{k}$,\;\;\;$\hat{n}_{23}=-0.58\hat{i}+0.58\hat{j}+0.58\hat{k}$,\;\;\;$\hat{n}_{25}=-0.36\hat{i}-0.32\hat{j}-0.88\hat{k}$,\newline
$\vec{r}_{14}=10.0\hat{i}+0.0\hat{j}+10.0\hat{k}$,\;\;\;$\vec{r}_{24}=0.0\hat{i}+10.0\hat{j}+0.0\hat{k}$,\;\;\;$\vec{r}_{25}=10.0\hat{i}+10.0\hat{j}+0.0\hat{k}$.

2D-M465:

$\hat{n}_{13}=-0.51\hat{i}-0.51\hat{j}-0.7\hat{k}$,\;\;\;$\hat{n}_{14}=-0.89\hat{i}+0.44\hat{j}-0.07\hat{k}$,\;\;\;$\hat{n}_{25}=-0.0\hat{i}+0.0\hat{j}+1.0\hat{k}$,\;\;\;$\hat{n}_{45}=-0.0\hat{i}+0.8\hat{j}+0.61\hat{k}$,\newline
$\vec{r}_{14}=10.0\hat{i}+10.0\hat{j}+10.0\hat{k}$,\;\;\;$\vec{r}_{23}=0.0\hat{i}+0.0\hat{j}+0.0\hat{k}$,\;\;\;$\vec{r}_{25}=10.0\hat{i}+10.0\hat{j}+0.21\hat{k}$.

2D-M466:

$\hat{n}_{13}=0.98\hat{i}-0.13\hat{j}+0.15\hat{k}$,\;\;\;$\hat{n}_{14}=-0.91\hat{i}+0.42\hat{j}+0.04\hat{k}$,\;\;\;$\hat{n}_{25}=-0.0\hat{i}+0.75\hat{j}+0.66\hat{k}$,\;\;\;$\hat{n}_{45}=0.91\hat{i}+0.16\hat{j}-0.38\hat{k}$,\newline
$\vec{r}_{14}=0.0\hat{i}+0.0\hat{j}+0.0\hat{k}$,\;\;\;$\vec{r}_{23}=10.0\hat{i}+10.0\hat{j}+10.0\hat{k}$,\;\;\;$\vec{r}_{45}=10.0\hat{i}+0.0\hat{j}+0.0\hat{k}$.

2D-M467:

$\hat{n}_{13}=-0.28\hat{i}-0.61\hat{j}-0.74\hat{k}$,\;\;\;$\hat{n}_{14}=-0.0\hat{i}+0.26\hat{j}+0.97\hat{k}$,\;\;\;$\hat{n}_{24}=-0.79\hat{i}+0.2\hat{j}+0.58\hat{k}$,\;\;\;$\hat{n}_{45}=-0.01\hat{i}+0.92\hat{j}-0.4\hat{k}$,\newline
$\vec{r}_{14}=10.0\hat{i}+0.0\hat{j}+0.0\hat{k}$,\;\;\;$\vec{r}_{23}=0.0\hat{i}+0.0\hat{j}+0.0\hat{k}$,\;\;\;$\vec{r}_{24}=10.0\hat{i}+10.0\hat{j}+10.0\hat{k}$.

2D-M468:

$\hat{n}_{13}=0.72\hat{i}+0.09\hat{j}+0.69\hat{k}$,\;\;\;$\hat{n}_{14}=-0.05\hat{i}-0.99\hat{j}+0.09\hat{k}$,\;\;\;$\hat{n}_{24}=0.64\hat{i}-0.75\hat{j}+0.16\hat{k}$,\;\;\;$\hat{n}_{35}=0.14\hat{i}-0.99\hat{j}-0.01\hat{k}$,\newline
$\vec{r}_{14}=5.58\hat{i}+5.0\hat{j}+5.4\hat{k}$,\;\;\;$\vec{r}_{23}=4.72\hat{i}+4.21\hat{j}+4.43\hat{k}$,\;\;\;$\vec{r}_{24}=4.1\hat{i}+5.81\hat{j}+5.4\hat{k}$.

2D-M469:

$\hat{n}_{13}=-0.42\hat{i}+0.43\hat{j}+0.8\hat{k}$,\;\;\;$\hat{n}_{14}=0.0\hat{i}+0.25\hat{j}+0.97\hat{k}$,\;\;\;$\hat{n}_{24}=0.51\hat{i}+0.71\hat{j}+0.49\hat{k}$,\;\;\;$\hat{n}_{25}=-0.95\hat{i}-0.14\hat{j}-0.26\hat{k}$,\newline
$\vec{r}_{14}=10.0\hat{i}+0.0\hat{j}+0.0\hat{k}$,\;\;\;$\vec{r}_{23}=0.0\hat{i}+10.0\hat{j}+0.0\hat{k}$,\;\;\;$\vec{r}_{24}=0.0\hat{i}+0.0\hat{j}+10.0\hat{k}$.

2D-M470:

$\hat{n}_{13}=-0.82\hat{i}-0.39\hat{j}-0.42\hat{k}$,\;\;\;$\hat{n}_{14}=0.82\hat{i}+0.39\hat{j}+0.42\hat{k}$,\;\;\;$\hat{n}_{24}=-0.58\hat{i}+0.58\hat{j}+0.58\hat{k}$,\;\;\;$\hat{n}_{45}=0.9\hat{i}+0.27\hat{j}+0.34\hat{k}$,\newline
$\vec{r}_{14}=0.0\hat{i}+10.0\hat{j}+0.0\hat{k}$,\;\;\;$\vec{r}_{23}=10.0\hat{i}+0.0\hat{j}+10.0\hat{k}$,\;\;\;$\vec{r}_{45}=10.0\hat{i}+0.0\hat{j}+10.0\hat{k}$.

2D-M471:

$\hat{n}_{13}=-0.18\hat{i}-0.16\hat{j}+0.97\hat{k}$,\;\;\;$\hat{n}_{14}=-0.93\hat{i}-0.29\hat{j}+0.23\hat{k}$,\;\;\;$\hat{n}_{24}=-0.68\hat{i}-0.67\hat{j}-0.29\hat{k}$,\;\;\;$\hat{n}_{35}=0.28\hat{i}+0.39\hat{j}+0.88\hat{k}$,\newline
$\vec{r}_{14}=3.6\hat{i}+6.7\hat{j}+2.67\hat{k}$,\;\;\;$\vec{r}_{23}=3.29\hat{i}+3.72\hat{j}+2.54\hat{k}$,\;\;\;$\vec{r}_{35}=10.0\hat{i}+10.0\hat{j}+0.0\hat{k}$.

2D-M472:

$\hat{n}_{13}=-0.0\hat{i}+0.0\hat{j}-1.0\hat{k}$,\;\;\;$\hat{n}_{14}=-0.5\hat{i}+0.32\hat{j}-0.81\hat{k}$,\;\;\;$\hat{n}_{24}=-0.57\hat{i}+0.58\hat{j}+0.58\hat{k}$,\;\;\;$\hat{n}_{25}=0.22\hat{i}-0.48\hat{j}-0.85\hat{k}$,\newline
$\vec{r}_{14}=10.0\hat{i}+0.0\hat{j}+10.0\hat{k}$,\;\;\;$\vec{r}_{23}=0.0\hat{i}+10.0\hat{j}+0.0\hat{k}$,\;\;\;$\vec{r}_{25}=10.0\hat{i}+0.0\hat{j}+0.0\hat{k}$.

2D-M473:

$\hat{n}_{13}=-0.0\hat{i}+0.0\hat{j}+1.0\hat{k}$,\;\;\;$\hat{n}_{24}=-0.0\hat{i}+0.07\hat{j}-1.0\hat{k}$,\;\;\;$\hat{n}_{25}=-0.55\hat{i}+0.53\hat{j}-0.65\hat{k}$,\;\;\;$\hat{n}_{35}=0.6\hat{i}+0.79\hat{j}+0.11\hat{k}$,\newline
$\vec{r}_{14}=0.0\hat{i}+10.0\hat{j}+10.0\hat{k}$,\;\;\;$\vec{r}_{24}=10.0\hat{i}+0.0\hat{j}+10.0\hat{k}$,\;\;\;$\vec{r}_{35}=10.0\hat{i}+0.0\hat{j}+0.0\hat{k}$.

2D-M474:

$\hat{n}_{13}=-0.19\hat{i}-0.52\hat{j}-0.84\hat{k}$,\;\;\;$\hat{n}_{24}=-0.0\hat{i}+0.71\hat{j}+0.71\hat{k}$,\;\;\;$\hat{n}_{25}=0.63\hat{i}-0.55\hat{j}+0.55\hat{k}$,\;\;\;$\hat{n}_{35}=-0.77\hat{i}-0.45\hat{j}+0.45\hat{k}$,\newline
$\vec{r}_{14}=10.0\hat{i}+10.0\hat{j}+0.0\hat{k}$,\;\;\;$\vec{r}_{24}=0.0\hat{i}+10.0\hat{j}+10.0\hat{k}$,\;\;\;$\vec{r}_{25}=0.0\hat{i}+0.0\hat{j}+10.0\hat{k}$.

2D-M475:

$\hat{n}_{13}=0.48\hat{i}-0.68\hat{j}-0.55\hat{k}$,\;\;\;$\hat{n}_{24}=-0.6\hat{i}+0.55\hat{j}+0.58\hat{k}$,\;\;\;$\hat{n}_{25}=0.62\hat{i}+0.77\hat{j}-0.15\hat{k}$,\;\;\;$\hat{n}_{35}=0.53\hat{i}-0.27\hat{j}+0.8\hat{k}$,\newline
$\vec{r}_{14}=0.0\hat{i}+10.0\hat{j}+0.0\hat{k}$,\;\;\;$\vec{r}_{25}=10.0\hat{i}+0.0\hat{j}+10.0\hat{k}$,\;\;\;$\vec{r}_{35}=10.0\hat{i}+0.0\hat{j}+10.0\hat{k}$.

2D-M476:

$\hat{n}_{13}=0.25\hat{i}-0.31\hat{j}+0.92\hat{k}$,\;\;\;$\hat{n}_{24}=-0.36\hat{i}-0.58\hat{j}-0.73\hat{k}$,\;\;\;$\hat{n}_{25}=-0.53\hat{i}-0.81\hat{j}-0.26\hat{k}$,\;\;\;$\hat{n}_{35}=0.04\hat{i}-0.6\hat{j}+0.8\hat{k}$,\newline
$\vec{r}_{14}=3.13\hat{i}+7.06\hat{j}+4.74\hat{k}$,\;\;\;$\vec{r}_{25}=3.36\hat{i}+3.16\hat{j}+7.01\hat{k}$,\;\;\;$\vec{r}_{35}=10.0\hat{i}+10.0\hat{j}+10.0\hat{k}$.

2D-M477:

$\hat{n}_{13}=-0.56\hat{i}-0.15\hat{j}-0.82\hat{k}$,\;\;\;$\hat{n}_{24}=-0.55\hat{i}+0.63\hat{j}+0.55\hat{k}$,\;\;\;$\hat{n}_{25}=0.71\hat{i}-0.0\hat{j}+0.71\hat{k}$,\;\;\;$\hat{n}_{35}=-0.45\hat{i}-0.77\hat{j}+0.45\hat{k}$,\newline
$\vec{r}_{14}=10.0\hat{i}+10.0\hat{j}+0.0\hat{k}$,\;\;\;$\vec{r}_{24}=0.0\hat{i}+0.0\hat{j}+10.0\hat{k}$,\;\;\;$\vec{r}_{25}=10.0\hat{i}+0.0\hat{j}+10.0\hat{k}$.

2D-M478:

$\hat{n}_{13}=0.02\hat{i}+0.13\hat{j}-0.99\hat{k}$,\;\;\;$\hat{n}_{24}=-0.36\hat{i}-0.76\hat{j}+0.55\hat{k}$,\;\;\;$\hat{n}_{25}=0.27\hat{i}-0.96\hat{j}-0.11\hat{k}$,\;\;\;$\hat{n}_{35}=-0.18\hat{i}+0.5\hat{j}-0.85\hat{k}$,\newline
$\vec{r}_{14}=4.23\hat{i}+5.03\hat{j}+5.58\hat{k}$,\;\;\;$\vec{r}_{24}=4.93\hat{i}+4.37\hat{j}+4.76\hat{k}$,\;\;\;$\vec{r}_{35}=10.0\hat{i}+0.0\hat{j}+10.0\hat{k}$.

2D-M479:

$\hat{n}_{13}=0.47\hat{i}+0.34\hat{j}-0.81\hat{k}$,\;\;\;$\hat{n}_{23}=-0.0\hat{i}+0.46\hat{j}+0.89\hat{k}$,\;\;\;$\hat{n}_{25}=0.47\hat{i}+0.68\hat{j}+0.56\hat{k}$,\;\;\;$\hat{n}_{45}=-0.68\hat{i}+0.72\hat{j}-0.16\hat{k}$,\newline
$\vec{r}_{14}=10.0\hat{i}+10.0\hat{j}+10.0\hat{k}$,\;\;\;$\vec{r}_{23}=10.0\hat{i}+10.0\hat{j}+0.0\hat{k}$,\;\;\;$\vec{r}_{45}=0.0\hat{i}+0.0\hat{j}+0.0\hat{k}$.

2D-M480:

$\hat{n}_{13}=0.85\hat{i}-0.29\hat{j}-0.44\hat{k}$,\;\;\;$\hat{n}_{23}=0.83\hat{i}+0.44\hat{j}-0.34\hat{k}$,\;\;\;$\hat{n}_{25}=-0.22\hat{i}+0.56\hat{j}-0.8\hat{k}$,\;\;\;$\hat{n}_{45}=-0.56\hat{i}+0.56\hat{j}+0.61\hat{k}$,\newline
$\vec{r}_{14}=10.0\hat{i}+0.0\hat{j}+10.0\hat{k}$,\;\;\;$\vec{r}_{23}=10.0\hat{i}+0.0\hat{j}+0.0\hat{k}$,\;\;\;$\vec{r}_{25}=0.0\hat{i}+10.0\hat{j}+0.0\hat{k}$.

2D-M481:

$\hat{n}_{13}=0.77\hat{i}-0.28\hat{j}-0.57\hat{k}$,\;\;\;$\hat{n}_{23}=0.64\hat{i}-0.74\hat{j}+0.21\hat{k}$,\;\;\;$\hat{n}_{24}=-0.0\hat{i}+0.9\hat{j}-0.44\hat{k}$,\;\;\;$\hat{n}_{45}=-0.0\hat{i}+1.0\hat{j}+0.05\hat{k}$,\newline
$\vec{r}_{14}=0.0\hat{i}+0.0\hat{j}+0.0\hat{k}$,\;\;\;$\vec{r}_{23}=10.0\hat{i}+10.0\hat{j}+0.0\hat{k}$,\;\;\;$\vec{r}_{24}=10.0\hat{i}+0.0\hat{j}+10.0\hat{k}$.

2D-M482:

$\hat{n}_{13}=-0.8\hat{i}-0.4\hat{j}-0.44\hat{k}$,\;\;\;$\hat{n}_{23}=-0.54\hat{i}-0.67\hat{j}+0.51\hat{k}$,\;\;\;$\hat{n}_{24}=0.46\hat{i}-0.89\hat{j}+0.04\hat{k}$,\;\;\;$\hat{n}_{35}=0.58\hat{i}-0.68\hat{j}-0.45\hat{k}$,\newline
$\vec{r}_{14}=2.75\hat{i}+2.95\hat{j}+7.74\hat{k}$,\;\;\;$\vec{r}_{23}=7.76\hat{i}+7.17\hat{j}+2.98\hat{k}$,\;\;\;$\vec{r}_{24}=5.72\hat{i}+2.73\hat{j}+2.31\hat{k}$.

2D-M483:

$\hat{n}_{13}=0.0\hat{i}+0.0\hat{j}+1.0\hat{k}$,\;\;\;$\hat{n}_{23}=-0.0\hat{i}+0.0\hat{j}+1.0\hat{k}$,\;\;\;$\hat{n}_{24}=-0.72\hat{i}-0.0\hat{j}-0.7\hat{k}$,\;\;\;$\hat{n}_{25}=0.97\hat{i}+0.22\hat{j}-0.07\hat{k}$,\newline
$\vec{r}_{14}=10.0\hat{i}+10.0\hat{j}+10.0\hat{k}$,\;\;\;$\vec{r}_{23}=0.0\hat{i}+0.0\hat{j}+0.0\hat{k}$,\;\;\;$\vec{r}_{24}=0.0\hat{i}+10.0\hat{j}+0.0\hat{k}$.

2D-M484:

$\hat{n}_{13}=0.66\hat{i}-0.71\hat{j}-0.26\hat{k}$,\;\;\;$\hat{n}_{23}=-0.59\hat{i}-0.7\hat{j}+0.41\hat{k}$,\;\;\;$\hat{n}_{25}=0.58\hat{i}-0.8\hat{j}-0.13\hat{k}$,\;\;\;$\hat{n}_{45}=-0.16\hat{i}-0.07\hat{j}-0.98\hat{k}$,\newline
$\vec{r}_{14}=0.0\hat{i}+0.0\hat{j}+0.0\hat{k}$,\;\;\;$\vec{r}_{25}=0.0\hat{i}+0.0\hat{j}+10.0\hat{k}$,\;\;\;$\vec{r}_{45}=10.0\hat{i}+10.0\hat{j}+0.0\hat{k}$.

2D-M485:

$\hat{n}_{13}=0.19\hat{i}+0.98\hat{j}+0.0\hat{k}$,\;\;\;$\hat{n}_{23}=0.0\hat{i}+0.0\hat{j}-1.0\hat{k}$,\;\;\;$\hat{n}_{25}=0.92\hat{i}-0.18\hat{j}-0.34\hat{k}$,\;\;\;$\hat{n}_{45}=-0.13\hat{i}+0.76\hat{j}-0.63\hat{k}$,\newline
$\vec{r}_{14}=0.0\hat{i}+0.0\hat{j}+0.0\hat{k}$,\;\;\;$\vec{r}_{25}=0.0\hat{i}+10.0\hat{j}+10.0\hat{k}$,\;\;\;$\vec{r}_{45}=10.0\hat{i}+10.0\hat{j}+10.0\hat{k}$.

2D-M486:

$\hat{n}_{13}=-0.0\hat{i}+0.69\hat{j}-0.72\hat{k}$,\;\;\;$\hat{n}_{23}=0.58\hat{i}+0.58\hat{j}+0.57\hat{k}$,\;\;\;$\hat{n}_{24}=0.82\hat{i}-0.43\hat{j}-0.39\hat{k}$,\;\;\;$\hat{n}_{45}=0.0\hat{i}+0.57\hat{j}-0.82\hat{k}$,\newline
$\vec{r}_{14}=10.0\hat{i}+10.0\hat{j}+10.0\hat{k}$,\;\;\;$\vec{r}_{24}=0.0\hat{i}+0.0\hat{j}+0.0\hat{k}$,\;\;\;$\vec{r}_{45}=10.0\hat{i}+0.0\hat{j}+10.0\hat{k}$.

2D-M487:

$\hat{n}_{13}=0.02\hat{i}-0.35\hat{j}+0.94\hat{k}$,\;\;\;$\hat{n}_{23}=-0.7\hat{i}-0.67\hat{j}+0.25\hat{k}$,\;\;\;$\hat{n}_{24}=-0.84\hat{i}-0.53\hat{j}+0.03\hat{k}$,\;\;\;$\hat{n}_{35}=0.11\hat{i}+0.51\hat{j}-0.85\hat{k}$,\newline
$\vec{r}_{14}=6.14\hat{i}+7.67\hat{j}+6.57\hat{k}$,\;\;\;$\vec{r}_{24}=7.74\hat{i}+4.9\hat{j}+3.93\hat{k}$,\;\;\;$\vec{r}_{35}=10.0\hat{i}+10.0\hat{j}+10.0\hat{k}$.

2D-M488:

$\hat{n}_{13}=-1.0\hat{i}-0.0\hat{j}-0.0\hat{k}$,\;\;\;$\hat{n}_{23}=-0.0\hat{i}+0.71\hat{j}-0.71\hat{k}$,\;\;\;$\hat{n}_{24}=0.93\hat{i}-0.25\hat{j}+0.25\hat{k}$,\;\;\;$\hat{n}_{25}=0.75\hat{i}-0.66\hat{j}+0.02\hat{k}$,\newline
$\vec{r}_{14}=10.0\hat{i}+10.0\hat{j}+0.0\hat{k}$,\;\;\;$\vec{r}_{24}=0.0\hat{i}+0.0\hat{j}+10.0\hat{k}$,\;\;\;$\vec{r}_{25}=10.0\hat{i}+10.0\hat{j}+10.0\hat{k}$.

2D-M489:

$\hat{n}_{13}=-0.59\hat{i}-0.3\hat{j}+0.75\hat{k}$,\;\;\;$\hat{n}_{23}=0.8\hat{i}-0.31\hat{j}+0.51\hat{k}$,\;\;\;$\hat{n}_{25}=0.18\hat{i}-0.55\hat{j}-0.81\hat{k}$,\;\;\;$\hat{n}_{45}=0.56\hat{i}+0.59\hat{j}-0.58\hat{k}$,\newline
$\vec{r}_{14}=10.0\hat{i}+10.0\hat{j}+0.0\hat{k}$,\;\;\;$\vec{r}_{23}=0.0\hat{i}+0.0\hat{j}+10.0\hat{k}$,\;\;\;$\vec{r}_{25}=0.0\hat{i}+10.0\hat{j}+10.0\hat{k}$.

2D-M490:

$\hat{n}_{13}=-0.0\hat{i}+0.72\hat{j}-0.69\hat{k}$,\;\;\;$\hat{n}_{23}=0.78\hat{i}+0.43\hat{j}+0.46\hat{k}$,\;\;\;$\hat{n}_{25}=-0.63\hat{i}+0.55\hat{j}+0.55\hat{k}$,\;\;\;$\hat{n}_{45}=-0.0\hat{i}+0.71\hat{j}-0.7\hat{k}$,\newline
$\vec{r}_{14}=0.0\hat{i}+10.0\hat{j}+0.0\hat{k}$,\;\;\;$\vec{r}_{23}=10.0\hat{i}+0.0\hat{j}+10.0\hat{k}$,\;\;\;$\vec{r}_{45}=10.0\hat{i}+0.0\hat{j}+10.0\hat{k}$.

2D-M491:

$\hat{n}_{13}=-0.39\hat{i}+0.89\hat{j}+0.24\hat{k}$,\;\;\;$\hat{n}_{23}=-0.91\hat{i}-0.34\hat{j}-0.23\hat{k}$,\;\;\;$\hat{n}_{24}=0.0\hat{i}+0.77\hat{j}-0.64\hat{k}$,\;\;\;$\hat{n}_{45}=-0.0\hat{i}+0.0\hat{j}+1.0\hat{k}$,\newline
$\vec{r}_{14}=0.0\hat{i}+0.0\hat{j}+0.0\hat{k}$,\;\;\;$\vec{r}_{23}=10.0\hat{i}+0.0\hat{j}+10.0\hat{k}$,\;\;\;$\vec{r}_{24}=10.0\hat{i}+10.0\hat{j}+10.0\hat{k}$.

2D-M492:

$\hat{n}_{13}=-0.73\hat{i}-0.64\hat{j}-0.26\hat{k}$,\;\;\;$\hat{n}_{23}=0.53\hat{i}-0.85\hat{j}+0.05\hat{k}$,\;\;\;$\hat{n}_{24}=0.65\hat{i}-0.76\hat{j}-0.03\hat{k}$,\;\;\;$\hat{n}_{35}=0.62\hat{i}-0.77\hat{j}+0.16\hat{k}$,\newline
$\vec{r}_{14}=4.11\hat{i}+5.6\hat{j}+4.22\hat{k}$,\;\;\;$\vec{r}_{23}=5.14\hat{i}+5.98\hat{j}+5.75\hat{k}$,\;\;\;$\vec{r}_{24}=5.63\hat{i}+5.96\hat{j}+4.02\hat{k}$.

2D-M493:

$\hat{n}_{13}=0.7\hat{i}+0.36\hat{j}+0.62\hat{k}$,\;\;\;$\hat{n}_{23}=0.29\hat{i}-0.93\hat{j}+0.21\hat{k}$,\;\;\;$\hat{n}_{24}=0.7\hat{i}-0.0\hat{j}-0.71\hat{k}$,\;\;\;$\hat{n}_{25}=0.0\hat{i}+1.0\hat{j}-0.0\hat{k}$,\newline
$\vec{r}_{14}=0.0\hat{i}+0.0\hat{j}+0.0\hat{k}$,\;\;\;$\vec{r}_{23}=10.0\hat{i}+10.0\hat{j}+10.0\hat{k}$,\;\;\;$\vec{r}_{24}=10.0\hat{i}+0.0\hat{j}+0.0\hat{k}$.

2D-M494:

$\hat{n}_{13}=-0.82\hat{i}-0.38\hat{j}+0.43\hat{k}$,\;\;\;$\hat{n}_{23}=0.0\hat{i}+0.75\hat{j}+0.66\hat{k}$,\;\;\;$\hat{n}_{24}=-0.58\hat{i}+0.54\hat{j}-0.61\hat{k}$,\;\;\;$\hat{n}_{45}=0.56\hat{i}-0.74\hat{j}-0.37\hat{k}$,\newline
$\vec{r}_{14}=0.0\hat{i}+10.0\hat{j}+10.0\hat{k}$,\;\;\;$\vec{r}_{23}=10.0\hat{i}+0.0\hat{j}+0.0\hat{k}$,\;\;\;$\vec{r}_{45}=10.0\hat{i}+10.0\hat{j}+0.0\hat{k}$.

2D-M495:

$\hat{n}_{13}=0.64\hat{i}-0.04\hat{j}+0.77\hat{k}$,\;\;\;$\hat{n}_{23}=0.39\hat{i}-0.8\hat{j}-0.45\hat{k}$,\;\;\;$\hat{n}_{24}=0.14\hat{i}-0.86\hat{j}+0.5\hat{k}$,\;\;\;$\hat{n}_{35}=0.33\hat{i}-0.72\hat{j}+0.61\hat{k}$,\newline
$\vec{r}_{14}=4.04\hat{i}+3.89\hat{j}+4.19\hat{k}$,\;\;\;$\vec{r}_{23}=5.86\hat{i}+6.12\hat{j}+4.73\hat{k}$,\;\;\;$\vec{r}_{35}=10.0\hat{i}+10.0\hat{j}+10.0\hat{k}$.

2D-M496:

$\hat{n}_{13}=0.52\hat{i}-0.56\hat{j}-0.65\hat{k}$,\;\;\;$\hat{n}_{23}=0.0\hat{i}+0.76\hat{j}-0.66\hat{k}$,\;\;\;$\hat{n}_{24}=-0.51\hat{i}+0.49\hat{j}+0.71\hat{k}$,\;\;\;$\hat{n}_{25}=0.0\hat{i}+0.77\hat{j}+0.64\hat{k}$,\newline
$\vec{r}_{14}=10.0\hat{i}+0.0\hat{j}+10.0\hat{k}$,\;\;\;$\vec{r}_{23}=0.0\hat{i}+10.0\hat{j}+0.0\hat{k}$,\;\;\;$\vec{r}_{25}=10.0\hat{i}+10.0\hat{j}+0.0\hat{k}$.

2D-M497:

$\hat{n}_{13}=-0.82\hat{i}-0.34\hat{j}-0.46\hat{k}$,\;\;\;$\hat{n}_{24}=0.0\hat{i}+0.64\hat{j}-0.77\hat{k}$,\;\;\;$\hat{n}_{25}=0.0\hat{i}+0.0\hat{j}-1.0\hat{k}$,\;\;\;$\hat{n}_{35}=-0.57\hat{i}+0.55\hat{j}+0.61\hat{k}$,\newline
$\vec{r}_{13}=10.0\hat{i}+0.0\hat{j}+10.0\hat{k}$,\;\;\;$\vec{r}_{14}=0.0\hat{i}+10.0\hat{j}+0.0\hat{k}$,\;\;\;$\vec{r}_{24}=10.0\hat{i}+0.0\hat{j}+10.0\hat{k}$.

2D-M498:

$\hat{n}_{13}=-0.82\hat{i}+0.41\hat{j}+0.41\hat{k}$,\;\;\;$\hat{n}_{24}=0.57\hat{i}+0.64\hat{j}+0.51\hat{k}$,\;\;\;$\hat{n}_{25}=0.0\hat{i}+0.71\hat{j}-0.71\hat{k}$,\;\;\;$\hat{n}_{35}=-0.58\hat{i}-0.56\hat{j}-0.59\hat{k}$,\newline
$\vec{r}_{13}=0.0\hat{i}+0.0\hat{j}+0.0\hat{k}$,\;\;\;$\vec{r}_{14}=10.0\hat{i}+10.0\hat{j}+10.0\hat{k}$,\;\;\;$\vec{r}_{25}=0.0\hat{i}+0.0\hat{j}+0.0\hat{k}$.

2D-M499:

$\hat{n}_{13}=-0.48\hat{i}-0.31\hat{j}-0.82\hat{k}$,\;\;\;$\hat{n}_{24}=0.38\hat{i}+0.41\hat{j}+0.83\hat{k}$,\;\;\;$\hat{n}_{25}=0.54\hat{i}+0.63\hat{j}-0.56\hat{k}$,\;\;\;$\hat{n}_{35}=0.0\hat{i}+0.63\hat{j}+0.78\hat{k}$,\newline
$\vec{r}_{13}=0.0\hat{i}+0.0\hat{j}+10.0\hat{k}$,\;\;\;$\vec{r}_{14}=10.0\hat{i}+10.0\hat{j}+0.0\hat{k}$,\;\;\;$\vec{r}_{35}=0.0\hat{i}+10.0\hat{j}+10.0\hat{k}$.

2D-M500:

$\hat{n}_{13}=-0.75\hat{i}+0.66\hat{j}+0.02\hat{k}$,\;\;\;$\hat{n}_{23}=0.5\hat{i}+0.0\hat{j}-0.86\hat{k}$,\;\;\;$\hat{n}_{25}=0.0\hat{i}+0.0\hat{j}-1.0\hat{k}$,\;\;\;$\hat{n}_{45}=0.45\hat{i}+0.67\hat{j}+0.59\hat{k}$,\newline
$\vec{r}_{13}=0.0\hat{i}+0.0\hat{j}+0.0\hat{k}$,\;\;\;$\vec{r}_{14}=10.0\hat{i}+10.0\hat{j}+10.0\hat{k}$,\;\;\;$\vec{r}_{23}=0.0\hat{i}+10.0\hat{j}+10.0\hat{k}$.

2D-M501:

$\hat{n}_{13}=0.59\hat{i}+0.19\hat{j}-0.79\hat{k}$,\;\;\;$\hat{n}_{23}=-0.59\hat{i}+0.68\hat{j}-0.44\hat{k}$,\;\;\;$\hat{n}_{24}=-0.59\hat{i}-0.56\hat{j}-0.58\hat{k}$,\;\;\;$\hat{n}_{45}=-0.14\hat{i}+0.98\hat{j}-0.14\hat{k}$,\newline
$\vec{r}_{13}=0.0\hat{i}+0.0\hat{j}+0.0\hat{k}$,\;\;\;$\vec{r}_{14}=10.0\hat{i}+10.0\hat{j}+10.0\hat{k}$,\;\;\;$\vec{r}_{23}=10.0\hat{i}+10.0\hat{j}+0.0\hat{k}$.

2D-M502:

$\hat{n}_{13}=0.78\hat{i}-0.6\hat{j}-0.17\hat{k}$,\;\;\;$\hat{n}_{23}=0.25\hat{i}+0.55\hat{j}-0.8\hat{k}$,\;\;\;$\hat{n}_{24}=-0.58\hat{i}-0.58\hat{j}-0.58\hat{k}$,\;\;\;$\hat{n}_{35}=-0.12\hat{i}+0.13\hat{j}-0.98\hat{k}$,\newline
$\vec{r}_{13}=10.0\hat{i}+10.0\hat{j}+10.0\hat{k}$,\;\;\;$\vec{r}_{14}=0.0\hat{i}+0.0\hat{j}+0.0\hat{k}$,\;\;\;$\vec{r}_{23}=10.0\hat{i}+10.0\hat{j}+10.0\hat{k}$.

2D-M503:

$\hat{n}_{13}=0.72\hat{i}-0.66\hat{j}+0.23\hat{k}$,\;\;\;$\hat{n}_{23}=0.17\hat{i}+0.67\hat{j}+0.72\hat{k}$,\;\;\;$\hat{n}_{24}=-0.51\hat{i}-0.61\hat{j}+0.61\hat{k}$,\;\;\;$\hat{n}_{25}=0.22\hat{i}-0.58\hat{j}-0.78\hat{k}$,\newline
$\vec{r}_{13}=10.0\hat{i}+10.0\hat{j}+0.0\hat{k}$,\;\;\;$\vec{r}_{14}=0.0\hat{i}+0.0\hat{j}+10.0\hat{k}$,\;\;\;$\vec{r}_{23}=10.0\hat{i}+0.0\hat{j}+0.0\hat{k}$.

2D-M504:

$\hat{n}_{13}=-0.78\hat{i}-0.25\hat{j}+0.57\hat{k}$,\;\;\;$\hat{n}_{23}=-0.0\hat{i}+0.57\hat{j}+0.82\hat{k}$,\;\;\;$\hat{n}_{25}=-0.09\hat{i}-0.62\hat{j}-0.78\hat{k}$,\;\;\;$\hat{n}_{45}=-0.47\hat{i}+0.17\hat{j}-0.87\hat{k}$,\newline
$\vec{r}_{13}=10.0\hat{i}+10.0\hat{j}+10.0\hat{k}$,\;\;\;$\vec{r}_{14}=10.0\hat{i}+0.0\hat{j}+0.0\hat{k}$,\;\;\;$\vec{r}_{25}=0.0\hat{i}+0.0\hat{j}+10.0\hat{k}$.

2D-M505:

$\hat{n}_{13}=-0.53\hat{i}+0.27\hat{j}-0.8\hat{k}$,\;\;\;$\hat{n}_{23}=-0.62\hat{i}-0.77\hat{j}+0.15\hat{k}$,\;\;\;$\hat{n}_{25}=-0.58\hat{i}+0.58\hat{j}+0.58\hat{k}$,\;\;\;$\hat{n}_{45}=-0.62\hat{i}-0.77\hat{j}+0.15\hat{k}$,\newline
$\vec{r}_{13}=10.0\hat{i}+0.0\hat{j}+10.0\hat{k}$,\;\;\;$\vec{r}_{14}=0.0\hat{i}+10.0\hat{j}+0.0\hat{k}$,\;\;\;$\vec{r}_{45}=10.0\hat{i}+0.0\hat{j}+10.0\hat{k}$.

2D-M506:

$\hat{n}_{13}=-0.0\hat{i}+0.7\hat{j}+0.71\hat{k}$,\;\;\;$\hat{n}_{23}=0.58\hat{i}-0.58\hat{j}+0.58\hat{k}$,\;\;\;$\hat{n}_{24}=-0.0\hat{i}+0.0\hat{j}-1.0\hat{k}$,\;\;\;$\hat{n}_{45}=0.0\hat{i}-0.0\hat{j}-1.0\hat{k}$,\newline
$\vec{r}_{13}=0.0\hat{i}+10.0\hat{j}+10.0\hat{k}$,\;\;\;$\vec{r}_{14}=10.0\hat{i}+0.0\hat{j}+0.0\hat{k}$,\;\;\;$\vec{r}_{24}=10.0\hat{i}+0.0\hat{j}+9.98\hat{k}$.

2D-M507:

$\hat{n}_{13}=-0.37\hat{i}+0.44\hat{j}-0.82\hat{k}$,\;\;\;$\hat{n}_{23}=0.58\hat{i}-0.58\hat{j}-0.58\hat{k}$,\;\;\;$\hat{n}_{24}=0.73\hat{i}+0.69\hat{j}+0.04\hat{k}$,\;\;\;$\hat{n}_{35}=0.24\hat{i}+0.89\hat{j}+0.37\hat{k}$,\newline
$\vec{r}_{13}=10.0\hat{i}+0.0\hat{j}+10.0\hat{k}$,\;\;\;$\vec{r}_{14}=0.0\hat{i}+10.0\hat{j}+0.0\hat{k}$,\;\;\;$\vec{r}_{24}=10.0\hat{i}+0.0\hat{j}+10.0\hat{k}$.

2D-M508:

$\hat{n}_{13}=-0.79\hat{i}-0.58\hat{j}+0.21\hat{k}$,\;\;\;$\hat{n}_{23}=0.58\hat{i}-0.58\hat{j}+0.58\hat{k}$,\;\;\;$\hat{n}_{24}=0.0\hat{i}+0.56\hat{j}+0.83\hat{k}$,\;\;\;$\hat{n}_{25}=0.0\hat{i}+0.0\hat{j}-1.0\hat{k}$,\newline
$\vec{r}_{13}=0.0\hat{i}+10.0\hat{j}+10.0\hat{k}$,\;\;\;$\vec{r}_{14}=10.0\hat{i}+0.0\hat{j}+0.0\hat{k}$,\;\;\;$\vec{r}_{24}=0.0\hat{i}+10.0\hat{j}+10.0\hat{k}$.

2D-M509:

$\hat{n}_{13}=0.94\hat{i}+0.17\hat{j}-0.3\hat{k}$,\;\;\;$\hat{n}_{23}=-0.0\hat{i}+0.73\hat{j}+0.69\hat{k}$,\;\;\;$\hat{n}_{24}=0.0\hat{i}+0.69\hat{j}-0.73\hat{k}$,\;\;\;$\hat{n}_{45}=-0.2\hat{i}+0.68\hat{j}+0.71\hat{k}$,\newline
$\vec{r}_{13}=10.0\hat{i}+0.0\hat{j}+0.0\hat{k}$,\;\;\;$\vec{r}_{14}=0.0\hat{i}+10.0\hat{j}+10.0\hat{k}$,\;\;\;$\vec{r}_{45}=10.0\hat{i}+10.0\hat{j}+0.0\hat{k}$.

2D-M510:

$\hat{n}_{13}=-0.82\hat{i}+0.19\hat{j}+0.54\hat{k}$,\;\;\;$\hat{n}_{23}=-0.85\hat{i}+0.44\hat{j}+0.28\hat{k}$,\;\;\;$\hat{n}_{24}=0.0\hat{i}+0.53\hat{j}-0.85\hat{k}$,\;\;\;$\hat{n}_{35}=-0.0\hat{i}-0.0\hat{j}+1.0\hat{k}$,\newline
$\vec{r}_{13}=0.0\hat{i}+10.0\hat{j}+10.0\hat{k}$,\;\;\;$\vec{r}_{14}=10.0\hat{i}+0.0\hat{j}+0.0\hat{k}$,\;\;\;$\vec{r}_{35}=0.0\hat{i}+10.0\hat{j}+3.67\hat{k}$.

2D-M511:

$\hat{n}_{13}=0.82\hat{i}-0.41\hat{j}+0.41\hat{k}$,\;\;\;$\hat{n}_{23}=0.57\hat{i}+0.49\hat{j}-0.66\hat{k}$,\;\;\;$\hat{n}_{24}=0.58\hat{i}+0.59\hat{j}-0.56\hat{k}$,\;\;\;$\hat{n}_{25}=-0.38\hat{i}-0.3\hat{j}+0.87\hat{k}$,\newline
$\vec{r}_{13}=0.0\hat{i}+0.0\hat{j}+10.0\hat{k}$,\;\;\;$\vec{r}_{14}=10.0\hat{i}+10.0\hat{j}+0.0\hat{k}$,\;\;\;$\vec{r}_{25}=10.0\hat{i}+10.0\hat{j}+10.0\hat{k}$.
