# Supplementary material for: Dimensional synthesis of spatial manipulators for velocity and force transmission for operation around a specified task point
Source: arXiv:2210.04446 source file (2022-10-10)
Supplement: Supplementary file 13 [file classappendix9.tex]

\subsection{Class 9} \label{appendix_five_2_1}
2D-M512:

$\hat{n}_{14}=-0.65\hat{i}-0.65\hat{j}-0.39\hat{k}$,\;\;\;$\hat{n}_{24}=0.97\hat{i}+0.15\hat{j}-0.2\hat{k}$,\;\;\;$\hat{n}_{25}=-0.04\hat{i}-0.7\hat{j}-0.71\hat{k}$,\;\;\;$\hat{n}_{34}=-0.73\hat{i}-0.47\hat{j}+0.5\hat{k}$,\newline
$\hat{n}_{35}=0.68\hat{i}-0.54\hat{j}+0.49\hat{k}$,\;\;\;$\vec{r}_{14}=0.0\hat{i}+10.0\hat{j}+0.0\hat{k}$,\;\;\;$\vec{r}_{25}=5.09\hat{i}+4.91\hat{j}+4.99\hat{k}$,\;\;\;$\vec{r}_{34}=5.11\hat{i}+4.91\hat{j}+5.0\hat{k}$,\newline
$\vec{r}_{35}=5.08\hat{i}+5.03\hat{j}+4.93\hat{k}$.

2D-M513:

$\hat{n}_{14}=0.66\hat{i}-0.72\hat{j}-0.22\hat{k}$,\;\;\;$\hat{n}_{24}=0.5\hat{i}+0.79\hat{j}+0.35\hat{k}$,\;\;\;$\hat{n}_{25}=-0.84\hat{i}+0.35\hat{j}+0.4\hat{k}$,\;\;\;$\hat{n}_{34}=0.67\hat{i}-0.1\hat{j}-0.73\hat{k}$,\newline
$\hat{n}_{35}=-0.55\hat{i}+0.6\hat{j}-0.58\hat{k}$,\;\;\;$\vec{r}_{14}=10.0\hat{i}+10.0\hat{j}+0.0\hat{k}$,\;\;\;$\vec{r}_{24}=4.85\hat{i}+4.97\hat{j}+4.83\hat{k}$,\;\;\;$\vec{r}_{34}=4.85\hat{i}+5.11\hat{j}+5.32\hat{k}$,\newline
$\vec{r}_{35}=4.88\hat{i}+5.11\hat{j}+4.95\hat{k}$.

2D-M514:

$\hat{n}_{14}=-0.69\hat{i}-0.46\hat{j}-0.56\hat{k}$,\;\;\;$\hat{n}_{23}=-0.0\hat{i}+0.58\hat{j}+0.82\hat{k}$,\;\;\;$\hat{n}_{25}=0.71\hat{i}-0.58\hat{j}+0.41\hat{k}$,\;\;\;$\hat{n}_{34}=-0.71\hat{i}-0.58\hat{j}+0.41\hat{k}$,\newline
$\hat{n}_{45}=0.0\hat{i}+0.58\hat{j}+0.82\hat{k}$,\;\;\;$\vec{r}_{14}=0.0\hat{i}+10.0\hat{j}+0.0\hat{k}$,\;\;\;$\vec{r}_{25}=4.91\hat{i}+5.04\hat{j}+5.07\hat{k}$,\;\;\;$\vec{r}_{34}=4.92\hat{i}+5.13\hat{j}+5.13\hat{k}$,\newline
$\vec{r}_{45}=4.95\hat{i}+4.99\hat{j}+4.77\hat{k}$.

2D-M515:

$\hat{n}_{14}=-0.79\hat{i}+0.28\hat{j}+0.55\hat{k}$,\;\;\;$\hat{n}_{23}=0.29\hat{i}-0.55\hat{j}+0.78\hat{k}$,\;\;\;$\hat{n}_{25}=0.91\hat{i}-0.11\hat{j}-0.41\hat{k}$,\;\;\;$\hat{n}_{34}=-0.31\hat{i}-0.83\hat{j}-0.47\hat{k}$,\newline
$\hat{n}_{45}=-0.91\hat{i}+0.11\hat{j}+0.41\hat{k}$,\;\;\;$\vec{r}_{14}=10.0\hat{i}+10.0\hat{j}+10.0\hat{k}$,\;\;\;$\vec{r}_{23}=5.19\hat{i}+4.83\hat{j}+5.04\hat{k}$,\;\;\;$\vec{r}_{34}=5.19\hat{i}+5.16\hat{j}+4.96\hat{k}$,\newline
$\vec{r}_{45}=5.19\hat{i}+5.18\hat{j}+5.07\hat{k}$.

2D-M516:

$\hat{n}_{14}=-0.4\hat{i}-0.67\hat{j}+0.62\hat{k}$,\;\;\;$\hat{n}_{23}=-0.36\hat{i}+0.04\hat{j}-0.93\hat{k}$,\;\;\;$\hat{n}_{25}=-0.93\hat{i}-0.14\hat{j}+0.35\hat{k}$,\;\;\;$\hat{n}_{34}=0.12\hat{i}-0.99\hat{j}-0.08\hat{k}$,\newline
$\hat{n}_{45}=0.12\hat{i}-0.99\hat{j}-0.08\hat{k}$,\;\;\;$\vec{r}_{14}=10.0\hat{i}+0.0\hat{j}+10.0\hat{k}$,\;\;\;$\vec{r}_{23}=2.78\hat{i}+7.13\hat{j}+5.98\hat{k}$,\;\;\;$\vec{r}_{25}=2.95\hat{i}+2.59\hat{j}+6.99\hat{k}$,\newline
$\vec{r}_{45}=6.19\hat{i}+6.76\hat{j}+5.93\hat{k}$.

2D-M517:

$\hat{n}_{14}=0.66\hat{i}-0.72\hat{j}-0.21\hat{k}$,\;\;\;$\hat{n}_{23}=0.29\hat{i}-0.67\hat{j}+0.68\hat{k}$,\;\;\;$\hat{n}_{25}=0.45\hat{i}-0.53\hat{j}-0.71\hat{k}$,\;\;\;$\hat{n}_{34}=-0.84\hat{i}-0.52\hat{j}-0.15\hat{k}$,\newline
$\hat{n}_{45}=0.22\hat{i}-0.97\hat{j}+0.1\hat{k}$,\;\;\;$\vec{r}_{14}=10.0\hat{i}+10.0\hat{j}+0.0\hat{k}$,\;\;\;$\vec{r}_{23}=4.99\hat{i}+4.87\hat{j}+4.99\hat{k}$,\;\;\;$\vec{r}_{25}=4.99\hat{i}+4.93\hat{j}+5.12\hat{k}$,\newline
$\vec{r}_{34}=5.08\hat{i}+5.07\hat{j}+5.09\hat{k}$.

2D-M518:

$\hat{n}_{14}=0.8\hat{i}-0.31\hat{j}+0.52\hat{k}$,\;\;\;$\hat{n}_{15}=-0.8\hat{i}+0.31\hat{j}-0.52\hat{k}$,\;\;\;$\hat{n}_{23}=-0.8\hat{i}+0.31\hat{j}-0.52\hat{k}$,\;\;\;$\hat{n}_{25}=-0.56\hat{i}-0.69\hat{j}+0.45\hat{k}$,\newline
$\hat{n}_{34}=0.22\hat{i}-0.65\hat{j}-0.72\hat{k}$,\;\;\;$\vec{r}_{14}=5.05\hat{i}+5.06\hat{j}+5.07\hat{k}$,\;\;\;$\vec{r}_{15}=10.0\hat{i}+10.0\hat{j}+0.0\hat{k}$,\;\;\;$\vec{r}_{25}=5.08\hat{i}+5.01\hat{j}+5.01\hat{k}$,\newline
$\vec{r}_{34}=4.95\hat{i}+5.09\hat{j}+4.94\hat{k}$.

2D-M519:

$\hat{n}_{14}=0.77\hat{i}-0.64\hat{j}-0.03\hat{k}$,\;\;\;$\hat{n}_{15}=0.77\hat{i}-0.64\hat{j}-0.03\hat{k}$,\;\;\;$\hat{n}_{23}=-0.49\hat{i}-0.62\hat{j}+0.61\hat{k}$,\;\;\;$\hat{n}_{25}=-0.41\hat{i}-0.45\hat{j}-0.79\hat{k}$,\newline
$\hat{n}_{34}=0.77\hat{i}-0.64\hat{j}-0.03\hat{k}$,\;\;\;$\vec{r}_{14}=5.13\hat{i}+4.73\hat{j}+4.83\hat{k}$,\;\;\;$\vec{r}_{15}=10.0\hat{i}+10.0\hat{j}+10.0\hat{k}$,\;\;\;$\vec{r}_{23}=4.73\hat{i}+4.93\hat{j}+5.0\hat{k}$,\newline
$\vec{r}_{25}=5.18\hat{i}+5.26\hat{j}+5.24\hat{k}$.

2D-M520:

$\hat{n}_{14}=0.74\hat{i}-0.53\hat{j}-0.42\hat{k}$,\;\;\;$\hat{n}_{24}=-0.8\hat{i}-0.6\hat{j}-0.05\hat{k}$,\;\;\;$\hat{n}_{25}=-0.93\hat{i}+0.23\hat{j}+0.28\hat{k}$,\;\;\;$\hat{n}_{34}=-0.39\hat{i}+0.73\hat{j}-0.55\hat{k}$,\newline
$\hat{n}_{35}=-0.34\hat{i}+0.42\hat{j}+0.84\hat{k}$,\;\;\;$\vec{r}_{24}=0.0\hat{i}+10.0\hat{j}+0.0\hat{k}$,\;\;\;$\vec{r}_{25}=10.0\hat{i}+10.0\hat{j}+10.0\hat{k}$,\;\;\;$\vec{r}_{34}=10.0\hat{i}+0.0\hat{j}+10.0\hat{k}$,\newline
$\vec{r}_{35}=0.0\hat{i}+10.0\hat{j}+10.0\hat{k}$.

2D-M521:

$\hat{n}_{14}=-0.28\hat{i}+0.06\hat{j}-0.96\hat{k}$,\;\;\;$\hat{n}_{23}=-0.71\hat{i}-0.71\hat{j}-0.02\hat{k}$,\;\;\;$\hat{n}_{25}=0.76\hat{i}-0.51\hat{j}+0.39\hat{k}$,\;\;\;$\hat{n}_{34}=-0.73\hat{i}-0.55\hat{j}-0.4\hat{k}$,\newline
$\hat{n}_{45}=0.48\hat{i}-0.37\hat{j}-0.8\hat{k}$,\;\;\;$\vec{r}_{23}=3.91\hat{i}+4.94\hat{j}+2.63\hat{k}$,\;\;\;$\vec{r}_{25}=3.26\hat{i}+3.3\hat{j}+4.41\hat{k}$,\;\;\;$\vec{r}_{34}=4.82\hat{i}+8.11\hat{j}+7.6\hat{k}$,\newline
$\vec{r}_{45}=0.0\hat{i}+10.0\hat{j}+10.0\hat{k}$.

2D-M522:

$\hat{n}_{14}=-0.66\hat{i}-0.28\hat{j}-0.7\hat{k}$,\;\;\;$\hat{n}_{15}=0.66\hat{i}+0.28\hat{j}+0.7\hat{k}$,\;\;\;$\hat{n}_{23}=-0.66\hat{i}-0.28\hat{j}-0.7\hat{k}$,\;\;\;$\hat{n}_{25}=-0.71\hat{i}-0.07\hat{j}+0.7\hat{k}$,\newline
$\hat{n}_{34}=0.24\hat{i}-0.96\hat{j}+0.15\hat{k}$,\;\;\;$\vec{r}_{15}=0.0\hat{i}+0.0\hat{j}+10.0\hat{k}$,\;\;\;$\vec{r}_{23}=4.9\hat{i}+5.02\hat{j}+4.99\hat{k}$,\;\;\;$\vec{r}_{25}=4.98\hat{i}+4.98\hat{j}+4.98\hat{k}$,\newline
$\vec{r}_{34}=4.77\hat{i}+4.96\hat{j}+4.55\hat{k}$.

2D-M523:

$\hat{n}_{14}=-0.64\hat{i}-0.31\hat{j}+0.7\hat{k}$,\;\;\;$\hat{n}_{15}=0.64\hat{i}+0.31\hat{j}-0.7\hat{k}$,\;\;\;$\hat{n}_{23}=0.63\hat{i}+0.31\hat{j}+0.71\hat{k}$,\;\;\;$\hat{n}_{25}=-0.44\hat{i}+0.9\hat{j}+0.0\hat{k}$,\newline
$\hat{n}_{34}=0.64\hat{i}+0.31\hat{j}-0.7\hat{k}$,\;\;\;$\vec{r}_{15}=0.0\hat{i}+0.0\hat{j}+0.0\hat{k}$,\;\;\;$\vec{r}_{23}=4.8\hat{i}+4.95\hat{j}+5.4\hat{k}$,\;\;\;$\vec{r}_{25}=4.13\hat{i}+5.81\hat{j}+5.24\hat{k}$,\newline
$\vec{r}_{34}=5.88\hat{i}+5.51\hat{j}+5.09\hat{k}$.

2D-M524:

$\hat{n}_{14}=0.97\hat{i}-0.26\hat{j}+0.03\hat{k}$,\;\;\;$\hat{n}_{15}=-0.26\hat{i}-0.93\hat{j}+0.25\hat{k}$,\;\;\;$\hat{n}_{23}=0.26\hat{i}+0.93\hat{j}-0.25\hat{k}$,\;\;\;$\hat{n}_{25}=-0.26\hat{i}-0.93\hat{j}+0.25\hat{k}$,\newline
$\hat{n}_{34}=-0.03\hat{i}-0.25\hat{j}-0.97\hat{k}$,\;\;\;$\vec{r}_{14}=4.83\hat{i}+5.06\hat{j}+4.87\hat{k}$,\;\;\;$\vec{r}_{15}=0.0\hat{i}+10.0\hat{j}+0.0\hat{k}$,\;\;\;$\vec{r}_{23}=4.76\hat{i}+5.11\hat{j}+4.74\hat{k}$,\newline
$\vec{r}_{34}=4.59\hat{i}+4.77\hat{j}+5.0\hat{k}$.

2D-M525:

$\hat{n}_{14}=0.62\hat{i}+0.78\hat{j}+0.12\hat{k}$,\;\;\;$\hat{n}_{15}=-0.52\hat{i}+0.3\hat{j}+0.8\hat{k}$,\;\;\;$\hat{n}_{23}=0.52\hat{i}-0.3\hat{j}-0.8\hat{k}$,\;\;\;$\hat{n}_{25}=-0.59\hat{i}+0.56\hat{j}-0.59\hat{k}$,\newline
$\hat{n}_{34}=0.52\hat{i}-0.3\hat{j}-0.8\hat{k}$,\;\;\;$\vec{r}_{14}=5.42\hat{i}+5.0\hat{j}+5.0\hat{k}$,\;\;\;$\vec{r}_{15}=0.0\hat{i}+10.0\hat{j}+10.0\hat{k}$,\;\;\;$\vec{r}_{23}=4.88\hat{i}+5.04\hat{j}+4.86\hat{k}$,\newline
$\vec{r}_{25}=5.12\hat{i}+5.09\hat{j}+4.89\hat{k}$.

2D-M526:

$\hat{n}_{14}=-0.54\hat{i}-0.38\hat{j}+0.75\hat{k}$,\;\;\;$\hat{n}_{15}=-0.73\hat{i}+0.65\hat{j}-0.2\hat{k}$,\;\;\;$\hat{n}_{23}=-0.73\hat{i}+0.65\hat{j}-0.2\hat{k}$,\;\;\;$\hat{n}_{25}=-0.73\hat{i}+0.65\hat{j}-0.2\hat{k}$,\newline
$\hat{n}_{34}=0.42\hat{i}+0.66\hat{j}+0.63\hat{k}$,\;\;\;$\vec{r}_{14}=5.0\hat{i}+4.99\hat{j}+4.94\hat{k}$,\;\;\;$\vec{r}_{15}=0.0\hat{i}+0.0\hat{j}+10.0\hat{k}$,\;\;\;$\vec{r}_{25}=4.98\hat{i}+5.01\hat{j}+5.0\hat{k}$,\newline
$\vec{r}_{34}=5.0\hat{i}+5.0\hat{j}+5.0\hat{k}$.

2D-M527:

$\hat{n}_{14}=-0.67\hat{i}+0.21\hat{j}-0.72\hat{k}$,\;\;\;$\hat{n}_{15}=-0.38\hat{i}-0.92\hat{j}+0.09\hat{k}$,\;\;\;$\hat{n}_{23}=-0.38\hat{i}-0.92\hat{j}+0.09\hat{k}$,\;\;\;$\hat{n}_{25}=0.64\hat{i}-0.34\hat{j}-0.69\hat{k}$,\newline
$\hat{n}_{34}=0.38\hat{i}+0.92\hat{j}-0.09\hat{k}$,\;\;\;$\vec{r}_{14}=5.47\hat{i}+4.86\hat{j}+5.19\hat{k}$,\;\;\;$\vec{r}_{15}=0.0\hat{i}+10.0\hat{j}+0.0\hat{k}$,\;\;\;$\vec{r}_{25}=4.97\hat{i}+4.57\hat{j}+5.17\hat{k}$,\newline
$\vec{r}_{34}=4.95\hat{i}+5.09\hat{j}+4.54\hat{k}$.

2D-M528:

$\hat{n}_{14}=0.75\hat{i}-0.54\hat{j}+0.39\hat{k}$,\;\;\;$\hat{n}_{15}=0.0\hat{i}+0.58\hat{j}+0.81\hat{k}$,\;\;\;$\hat{n}_{23}=-0.66\hat{i}-0.61\hat{j}+0.43\hat{k}$,\;\;\;$\hat{n}_{25}=-0.0\hat{i}-0.58\hat{j}-0.81\hat{k}$,\newline
$\hat{n}_{34}=-0.0\hat{i}+0.58\hat{j}+0.81\hat{k}$,\;\;\;$\vec{r}_{14}=5.73\hat{i}+5.7\hat{j}+5.77\hat{k}$,\;\;\;$\vec{r}_{15}=10.0\hat{i}+10.0\hat{j}+0.0\hat{k}$,\;\;\;$\vec{r}_{23}=4.6\hat{i}+4.7\hat{j}+4.35\hat{k}$,\newline
$\vec{r}_{25}=5.72\hat{i}+4.61\hat{j}+5.19\hat{k}$.

2D-M529:

$\hat{n}_{14}=0.34\hat{i}-0.16\hat{j}+0.93\hat{k}$,\;\;\;$\hat{n}_{15}=-0.82\hat{i}+0.44\hat{j}+0.37\hat{k}$,\;\;\;$\hat{n}_{23}=0.46\hat{i}+0.89\hat{j}-0.02\hat{k}$,\;\;\;$\hat{n}_{25}=0.82\hat{i}-0.44\hat{j}-0.37\hat{k}$,\newline
$\hat{n}_{34}=0.82\hat{i}-0.44\hat{j}-0.37\hat{k}$,\;\;\;$\vec{r}_{14}=5.06\hat{i}+5.11\hat{j}+5.03\hat{k}$,\;\;\;$\vec{r}_{15}=10.0\hat{i}+10.0\hat{j}+10.0\hat{k}$,\;\;\;$\vec{r}_{23}=5.14\hat{i}+5.03\hat{j}+5.14\hat{k}$,\newline
$\vec{r}_{34}=5.04\hat{i}+5.0\hat{j}+5.12\hat{k}$.

2D-M530:

$\hat{n}_{13}=0.03\hat{i}-0.67\hat{j}-0.74\hat{k}$,\;\;\;$\hat{n}_{14}=0.04\hat{i}+0.75\hat{j}+0.67\hat{k}$,\;\;\;$\hat{n}_{24}=0.06\hat{i}-0.67\hat{j}+0.74\hat{k}$,\;\;\;$\hat{n}_{25}=1.0\hat{i}+0.01\hat{j}-0.07\hat{k}$,\newline
$\hat{n}_{35}=-0.05\hat{i}-0.75\hat{j}-0.66\hat{k}$,\;\;\;$\vec{r}_{13}=10.0\hat{i}+10.0\hat{j}+0.0\hat{k}$,\;\;\;$\vec{r}_{24}=5.04\hat{i}+5.04\hat{j}+4.97\hat{k}$,\;\;\;$\vec{r}_{25}=4.93\hat{i}+5.1\hat{j}+5.09\hat{k}$,\newline
$\vec{r}_{35}=0.0\hat{i}+0.0\hat{j}+10.0\hat{k}$.

2D-M531:

$\hat{n}_{13}=-0.66\hat{i}-0.72\hat{j}+0.2\hat{k}$,\;\;\;$\hat{n}_{14}=-0.57\hat{i}+0.49\hat{j}+0.66\hat{k}$,\;\;\;$\hat{n}_{24}=-0.57\hat{i}-0.81\hat{j}+0.11\hat{k}$,\;\;\;$\hat{n}_{25}=0.59\hat{i}-0.32\hat{j}+0.74\hat{k}$,\newline
$\hat{n}_{35}=-0.56\hat{i}-0.82\hat{j}+0.1\hat{k}$,\;\;\;$\vec{r}_{13}=10.0\hat{i}+0.0\hat{j}+10.0\hat{k}$,\;\;\;$\vec{r}_{14}=4.79\hat{i}+5.0\hat{j}+5.1\hat{k}$,\;\;\;$\vec{r}_{25}=5.07\hat{i}+5.02\hat{j}+4.79\hat{k}$,\newline
$\vec{r}_{35}=0.0\hat{i}+10.0\hat{j}+0.0\hat{k}$.

2D-M532:

$\hat{n}_{13}=0.06\hat{i}-0.73\hat{j}+0.68\hat{k}$,\;\;\;$\hat{n}_{14}=-0.5\hat{i}-0.64\hat{j}-0.59\hat{k}$,\;\;\;$\hat{n}_{24}=0.87\hat{i}-0.36\hat{j}-0.34\hat{k}$,\;\;\;$\hat{n}_{25}=0.01\hat{i}-0.68\hat{j}+0.74\hat{k}$,\newline
$\hat{n}_{35}=-0.0\hat{i}+0.67\hat{j}-0.74\hat{k}$,\;\;\;$\vec{r}_{13}=0.0\hat{i}+10.0\hat{j}+0.0\hat{k}$,\;\;\;$\vec{r}_{14}=5.48\hat{i}+4.46\hat{j}+4.21\hat{k}$,\;\;\;$\vec{r}_{24}=4.62\hat{i}+5.53\hat{j}+4.44\hat{k}$,\newline
$\vec{r}_{35}=10.0\hat{i}+0.0\hat{j}+10.0\hat{k}$.

2D-M533:

$\hat{n}_{13}=-0.0\hat{i}+0.71\hat{j}+0.71\hat{k}$,\;\;\;$\hat{n}_{14}=0.06\hat{i}-0.94\hat{j}-0.33\hat{k}$,\;\;\;$\hat{n}_{24}=-0.9\hat{i}-0.44\hat{j}-0.04\hat{k}$,\;\;\;$\hat{n}_{25}=-0.08\hat{i}-0.8\hat{j}-0.59\hat{k}$,\newline
$\hat{n}_{35}=0.0\hat{i}-0.0\hat{j}+1.0\hat{k}$,\;\;\;$\vec{r}_{13}=0.0\hat{i}+0.0\hat{j}+10.0\hat{k}$,\;\;\;$\vec{r}_{14}=1.77\hat{i}+2.39\hat{j}+8.5\hat{k}$,\;\;\;$\vec{r}_{24}=6.02\hat{i}+6.41\hat{j}+1.13\hat{k}$,\newline
$\vec{r}_{25}=2.33\hat{i}+7.66\hat{j}+6.24\hat{k}$.

2D-M534:

$\hat{n}_{13}=0.25\hat{i}-0.91\hat{j}-0.34\hat{k}$,\;\;\;$\hat{n}_{14}=0.4\hat{i}-0.29\hat{j}-0.87\hat{k}$,\;\;\;$\hat{n}_{23}=-0.61\hat{i}+0.45\hat{j}+0.65\hat{k}$,\;\;\;$\hat{n}_{25}=0.55\hat{i}+0.83\hat{j}-0.06\hat{k}$,\newline
$\hat{n}_{45}=0.78\hat{i}-0.36\hat{j}+0.51\hat{k}$,\;\;\;$\vec{r}_{13}=10.0\hat{i}+10.0\hat{j}+0.0\hat{k}$,\;\;\;$\vec{r}_{14}=10.0\hat{i}+0.0\hat{j}+0.0\hat{k}$,\;\;\;$\vec{r}_{25}=10.0\hat{i}+0.0\hat{j}+10.0\hat{k}$,\newline
$\vec{r}_{45}=0.0\hat{i}+10.0\hat{j}+0.0\hat{k}$.

2D-M535:

$\hat{n}_{13}=-0.0\hat{i}+0.7\hat{j}-0.72\hat{k}$,\;\;\;$\hat{n}_{14}=0.75\hat{i}-0.43\hat{j}+0.5\hat{k}$,\;\;\;$\hat{n}_{23}=-0.57\hat{i}-0.82\hat{j}-0.01\hat{k}$,\;\;\;$\hat{n}_{25}=-0.44\hat{i}+0.31\hat{j}-0.84\hat{k}$,\newline
$\hat{n}_{45}=0.44\hat{i}-0.27\hat{j}-0.86\hat{k}$,\;\;\;$\vec{r}_{13}=10.0\hat{i}+10.0\hat{j}+10.0\hat{k}$,\;\;\;$\vec{r}_{14}=10.0\hat{i}+0.0\hat{j}+10.0\hat{k}$,\;\;\;$\vec{r}_{23}=10.0\hat{i}+0.0\hat{j}+0.0\hat{k}$,\newline
$\vec{r}_{45}=10.0\hat{i}+0.0\hat{j}+0.0\hat{k}$.

2D-M536:

$\hat{n}_{13}=0.71\hat{i}+0.0\hat{j}+0.71\hat{k}$,\;\;\;$\hat{n}_{14}=0.58\hat{i}+0.58\hat{j}-0.58\hat{k}$,\;\;\;$\hat{n}_{23}=-0.19\hat{i}-0.6\hat{j}-0.78\hat{k}$,\;\;\;$\hat{n}_{25}=-0.78\hat{i}+0.6\hat{j}-0.19\hat{k}$,\newline
$\hat{n}_{45}=0.48\hat{i}-0.81\hat{j}-0.33\hat{k}$,\;\;\;$\vec{r}_{13}=10.0\hat{i}+0.0\hat{j}+10.0\hat{k}$,\;\;\;$\vec{r}_{14}=5.21\hat{i}+5.43\hat{j}+4.46\hat{k}$,\;\;\;$\vec{r}_{23}=0.0\hat{i}+10.0\hat{j}+10.0\hat{k}$,\newline
$\vec{r}_{25}=0.0\hat{i}+0.0\hat{j}+0.0\hat{k}$.

2D-M537:

$\hat{n}_{13}=-0.23\hat{i}-0.94\hat{j}-0.23\hat{k}$,\;\;\;$\hat{n}_{14}=-0.71\hat{i}-0.0\hat{j}+0.71\hat{k}$,\;\;\;$\hat{n}_{23}=0.42\hat{i}-0.8\hat{j}+0.42\hat{k}$,\;\;\;$\hat{n}_{24}=0.58\hat{i}+0.56\hat{j}+0.58\hat{k}$,\newline
$\hat{n}_{45}=0.01\hat{i}-1.0\hat{j}+0.01\hat{k}$,\;\;\;$\vec{r}_{13}=10.0\hat{i}+0.0\hat{j}+0.0\hat{k}$,\;\;\;$\vec{r}_{14}=5.01\hat{i}+4.97\hat{j}+4.94\hat{k}$,\;\;\;$\vec{r}_{23}=10.0\hat{i}+10.0\hat{j}+10.0\hat{k}$,\newline
$\vec{r}_{24}=0.0\hat{i}+10.0\hat{j}+10.0\hat{k}$.

2D-M538:

$\hat{n}_{13}=-0.0\hat{i}+0.42\hat{j}-0.91\hat{k}$,\;\;\;$\hat{n}_{14}=-0.55\hat{i}-0.67\hat{j}+0.51\hat{k}$,\;\;\;$\hat{n}_{23}=0.53\hat{i}-0.84\hat{j}-0.09\hat{k}$,\;\;\;$\hat{n}_{24}=-0.99\hat{i}-0.08\hat{j}-0.14\hat{k}$,\newline
$\hat{n}_{35}=-0.0\hat{i}+0.0\hat{j}+1.0\hat{k}$,\;\;\;$\vec{r}_{13}=10.0\hat{i}+10.0\hat{j}+10.0\hat{k}$,\;\;\;$\vec{r}_{14}=6.34\hat{i}+1.41\hat{j}+3.89\hat{k}$,\;\;\;$\vec{r}_{23}=4.42\hat{i}+4.13\hat{j}+2.91\hat{k}$,\newline
$\vec{r}_{24}=2.54\hat{i}+7.19\hat{j}+8.33\hat{k}$.

2D-M539:

$\hat{n}_{13}=0.71\hat{i}-0.71\hat{j}+0.02\hat{k}$,\;\;\;$\hat{n}_{14}=-0.58\hat{i}+0.58\hat{j}-0.56\hat{k}$,\;\;\;$\hat{n}_{24}=-0.23\hat{i}+0.23\hat{j}-0.94\hat{k}$,\;\;\;$\hat{n}_{25}=-0.42\hat{i}+0.42\hat{j}+0.8\hat{k}$,\newline
$\hat{n}_{35}=0.71\hat{i}+0.71\hat{j}-0.0\hat{k}$,\;\;\;$\vec{r}_{14}=10.0\hat{i}+0.0\hat{j}+10.0\hat{k}$,\;\;\;$\vec{r}_{24}=0.0\hat{i}+10.0\hat{j}+0.0\hat{k}$,\;\;\;$\vec{r}_{25}=10.0\hat{i}+0.0\hat{j}+0.0\hat{k}$,\newline
$\vec{r}_{35}=5.15\hat{i}+5.24\hat{j}+4.97\hat{k}$.

2D-M540:

$\hat{n}_{13}=0.76\hat{i}-0.46\hat{j}+0.46\hat{k}$,\;\;\;$\hat{n}_{14}=0.8\hat{i}-0.42\hat{j}+0.42\hat{k}$,\;\;\;$\hat{n}_{24}=0.56\hat{i}+0.58\hat{j}-0.58\hat{k}$,\;\;\;$\hat{n}_{25}=-0.94\hat{i}-0.23\hat{j}+0.23\hat{k}$,\newline
$\hat{n}_{35}=0.0\hat{i}+0.71\hat{j}+0.71\hat{k}$,\;\;\;$\vec{r}_{14}=0.0\hat{i}+0.0\hat{j}+10.0\hat{k}$,\;\;\;$\vec{r}_{24}=0.0\hat{i}+10.0\hat{j}+10.0\hat{k}$,\;\;\;$\vec{r}_{25}=10.0\hat{i}+0.0\hat{j}+0.0\hat{k}$,\newline
$\vec{r}_{35}=5.21\hat{i}+5.03\hat{j}+5.18\hat{k}$.

2D-M541:

$\hat{n}_{13}=-0.15\hat{i}-0.31\hat{j}-0.94\hat{k}$,\;\;\;$\hat{n}_{14}=0.12\hat{i}-0.88\hat{j}-0.46\hat{k}$,\;\;\;$\hat{n}_{24}=-0.25\hat{i}-0.83\hat{j}-0.49\hat{k}$,\;\;\;$\hat{n}_{25}=0.07\hat{i}-0.68\hat{j}+0.73\hat{k}$,\newline
$\hat{n}_{35}=0.67\hat{i}+0.13\hat{j}+0.73\hat{k}$,\;\;\;$\vec{r}_{14}=6.24\hat{i}+3.46\hat{j}+3.16\hat{k}$,\;\;\;$\vec{r}_{24}=3.45\hat{i}+3.71\hat{j}+3.74\hat{k}$,\;\;\;$\vec{r}_{25}=5.31\hat{i}+6.47\hat{j}+6.68\hat{k}$,\newline
$\vec{r}_{35}=0.0\hat{i}+10.0\hat{j}+0.0\hat{k}$.

2D-M542:

$\hat{n}_{13}=0.64\hat{i}-0.4\hat{j}+0.66\hat{k}$,\;\;\;$\hat{n}_{14}=0.45\hat{i}-0.21\hat{j}+0.87\hat{k}$,\;\;\;$\hat{n}_{23}=0.18\hat{i}-0.93\hat{j}+0.32\hat{k}$,\;\;\;$\hat{n}_{25}=0.49\hat{i}+0.87\hat{j}+0.05\hat{k}$,\newline
$\hat{n}_{45}=0.72\hat{i}-0.46\hat{j}-0.51\hat{k}$,\;\;\;$\vec{r}_{14}=10.0\hat{i}+0.0\hat{j}+10.0\hat{k}$,\;\;\;$\vec{r}_{23}=0.0\hat{i}+0.0\hat{j}+0.0\hat{k}$,\;\;\;$\vec{r}_{25}=0.0\hat{i}+10.0\hat{j}+10.0\hat{k}$,\newline
$\vec{r}_{45}=0.0\hat{i}+10.0\hat{j}+10.0\hat{k}$.

2D-M543:

$\hat{n}_{13}=0.57\hat{i}+0.4\hat{j}-0.72\hat{k}$,\;\;\;$\hat{n}_{14}=-0.82\hat{i}+0.47\hat{j}-0.33\hat{k}$,\;\;\;$\hat{n}_{23}=0.27\hat{i}+0.74\hat{j}+0.62\hat{k}$,\;\;\;$\hat{n}_{25}=0.16\hat{i}-0.63\hat{j}-0.76\hat{k}$,\newline
$\hat{n}_{45}=-0.54\hat{i}-0.45\hat{j}+0.72\hat{k}$,\;\;\;$\vec{r}_{14}=10.0\hat{i}+10.0\hat{j}+0.0\hat{k}$,\;\;\;$\vec{r}_{23}=0.0\hat{i}+0.0\hat{j}+10.0\hat{k}$,\;\;\;$\vec{r}_{25}=10.0\hat{i}+10.0\hat{j}+0.0\hat{k}$,\newline
$\vec{r}_{45}=10.0\hat{i}+0.0\hat{j}+0.0\hat{k}$.

2D-M544:

$\hat{n}_{13}=-0.65\hat{i}-0.74\hat{j}-0.19\hat{k}$,\;\;\;$\hat{n}_{14}=-0.66\hat{i}-0.72\hat{j}-0.2\hat{k}$,\;\;\;$\hat{n}_{23}=-0.76\hat{i}+0.63\hat{j}+0.16\hat{k}$,\;\;\;$\hat{n}_{25}=0.0\hat{i}+0.25\hat{j}-0.97\hat{k}$,\newline
$\hat{n}_{45}=-0.56\hat{i}-0.82\hat{j}-0.1\hat{k}$,\;\;\;$\vec{r}_{14}=10.0\hat{i}+0.0\hat{j}+0.0\hat{k}$,\;\;\;$\vec{r}_{23}=5.73\hat{i}+2.72\hat{j}+3.96\hat{k}$,\;\;\;$\vec{r}_{25}=3.27\hat{i}+2.79\hat{j}+2.7\hat{k}$,\newline
$\vec{r}_{45}=0.0\hat{i}+10.0\hat{j}+10.0\hat{k}$.

2D-M545:

$\hat{n}_{13}=-0.16\hat{i}-0.91\hat{j}-0.37\hat{k}$,\;\;\;$\hat{n}_{14}=-0.16\hat{i}-0.91\hat{j}-0.37\hat{k}$,\;\;\;$\hat{n}_{23}=0.31\hat{i}-0.41\hat{j}+0.86\hat{k}$,\;\;\;$\hat{n}_{24}=0.94\hat{i}-0.03\hat{j}-0.35\hat{k}$,\newline
$\hat{n}_{45}=0.16\hat{i}-0.66\hat{j}-0.73\hat{k}$,\;\;\;$\vec{r}_{14}=4.95\hat{i}+4.99\hat{j}+5.02\hat{k}$,\;\;\;$\vec{r}_{23}=5.0\hat{i}+5.13\hat{j}+4.97\hat{k}$,\;\;\;$\vec{r}_{24}=5.07\hat{i}+4.88\hat{j}+4.86\hat{k}$,\newline
$\vec{r}_{45}=10.0\hat{i}+10.0\hat{j}+0.0\hat{k}$.

2D-M546:

$\hat{n}_{13}=0.19\hat{i}-0.98\hat{j}-0.05\hat{k}$,\;\;\;$\hat{n}_{14}=0.88\hat{i}-0.45\hat{j}-0.12\hat{k}$,\;\;\;$\hat{n}_{23}=-0.4\hat{i}-0.62\hat{j}-0.68\hat{k}$,\;\;\;$\hat{n}_{24}=-0.23\hat{i}-0.64\hat{j}+0.73\hat{k}$,\newline
$\hat{n}_{35}=0.41\hat{i}-0.89\hat{j}+0.21\hat{k}$,\;\;\;$\vec{r}_{14}=4.91\hat{i}+4.92\hat{j}+5.06\hat{k}$,\;\;\;$\vec{r}_{23}=4.99\hat{i}+4.92\hat{j}+4.96\hat{k}$,\;\;\;$\vec{r}_{24}=5.07\hat{i}+5.07\hat{j}+5.17\hat{k}$,\newline
$\vec{r}_{35}=0.0\hat{i}+0.0\hat{j}+0.0\hat{k}$.

2D-M547:

$\hat{n}_{13}=-0.01\hat{i}-0.01\hat{j}-1.0\hat{k}$,\;\;\;$\hat{n}_{14}=0.2\hat{i}-0.98\hat{j}+0.0\hat{k}$,\;\;\;$\hat{n}_{23}=-0.98\hat{i}-0.2\hat{j}+0.01\hat{k}$,\;\;\;$\hat{n}_{24}=-0.01\hat{i}-0.01\hat{j}-1.0\hat{k}$,\newline
$\hat{n}_{25}=-0.0\hat{i}-0.0\hat{j}-1.0\hat{k}$,\;\;\;$\vec{r}_{14}=6.43\hat{i}+7.63\hat{j}+2.17\hat{k}$,\;\;\;$\vec{r}_{23}=2.2\hat{i}+5.86\hat{j}+6.27\hat{k}$,\;\;\;$\vec{r}_{24}=2.38\hat{i}+6.94\hat{j}+2.16\hat{k}$,\newline
$\vec{r}_{25}=10.0\hat{i}+10.0\hat{j}+7.76\hat{k}$.

2D-M548:

$\hat{n}_{13}=-0.4\hat{i}+0.52\hat{j}+0.76\hat{k}$,\;\;\;$\hat{n}_{14}=-0.9\hat{i}-0.34\hat{j}-0.28\hat{k}$,\;\;\;$\hat{n}_{24}=0.88\hat{i}-0.47\hat{j}+0.01\hat{k}$,\;\;\;$\hat{n}_{25}=0.43\hat{i}-0.75\hat{j}-0.5\hat{k}$,\newline
$\hat{n}_{35}=0.0\hat{i}+0.81\hat{j}-0.59\hat{k}$,\;\;\;$\vec{r}_{13}=0.0\hat{i}+10.0\hat{j}+10.0\hat{k}$,\;\;\;$\vec{r}_{14}=0.0\hat{i}+10.0\hat{j}+0.0\hat{k}$,\;\;\;$\vec{r}_{24}=10.0\hat{i}+10.0\hat{j}+10.0\hat{k}$,\newline
$\vec{r}_{35}=10.0\hat{i}+0.0\hat{j}+10.0\hat{k}$.

2D-M549:

$\hat{n}_{13}=0.71\hat{i}+0.71\hat{j}+0.0\hat{k}$,\;\;\;$\hat{n}_{14}=0.58\hat{i}-0.58\hat{j}-0.56\hat{k}$,\;\;\;$\hat{n}_{24}=0.23\hat{i}-0.23\hat{j}-0.94\hat{k}$,\;\;\;$\hat{n}_{25}=0.42\hat{i}-0.42\hat{j}+0.8\hat{k}$,\newline
$\hat{n}_{35}=0.7\hat{i}-0.7\hat{j}+0.12\hat{k}$,\;\;\;$\vec{r}_{13}=2.94\hat{i}+5.77\hat{j}+5.56\hat{k}$,\;\;\;$\vec{r}_{14}=0.0\hat{i}+10.0\hat{j}+10.0\hat{k}$,\;\;\;$\vec{r}_{24}=10.0\hat{i}+0.0\hat{j}+0.0\hat{k}$,\newline
$\vec{r}_{25}=0.0\hat{i}+10.0\hat{j}+0.0\hat{k}$.

2D-M550:

$\hat{n}_{13}=-0.19\hat{i}+0.86\hat{j}-0.46\hat{k}$,\;\;\;$\hat{n}_{14}=0.67\hat{i}-0.25\hat{j}-0.7\hat{k}$,\;\;\;$\hat{n}_{24}=0.42\hat{i}-0.65\hat{j}+0.64\hat{k}$,\;\;\;$\hat{n}_{25}=0.0\hat{i}+0.26\hat{j}-0.96\hat{k}$,\newline
$\hat{n}_{35}=-0.78\hat{i}-0.45\hat{j}-0.44\hat{k}$,\;\;\;$\vec{r}_{13}=10.0\hat{i}+10.0\hat{j}+10.0\hat{k}$,\;\;\;$\vec{r}_{14}=0.0\hat{i}+10.0\hat{j}+10.0\hat{k}$,\;\;\;$\vec{r}_{25}=10.0\hat{i}+0.0\hat{j}+10.0\hat{k}$,\newline
$\vec{r}_{35}=10.0\hat{i}+0.0\hat{j}+0.0\hat{k}$.

2D-M551:

$\hat{n}_{13}=-0.08\hat{i}-0.7\hat{j}+0.71\hat{k}$,\;\;\;$\hat{n}_{14}=-0.61\hat{i}-0.53\hat{j}-0.6\hat{k}$,\;\;\;$\hat{n}_{24}=0.07\hat{i}+0.71\hat{j}-0.7\hat{k}$,\;\;\;$\hat{n}_{25}=0.79\hat{i}-0.47\hat{j}-0.39\hat{k}$,\newline
$\hat{n}_{35}=-0.0\hat{i}+0.77\hat{j}-0.64\hat{k}$,\;\;\;$\vec{r}_{13}=10.0\hat{i}+0.0\hat{j}+10.0\hat{k}$,\;\;\;$\vec{r}_{14}=4.99\hat{i}+4.98\hat{j}+4.98\hat{k}$,\;\;\;$\vec{r}_{25}=5.01\hat{i}+4.99\hat{j}+5.01\hat{k}$,\newline
$\vec{r}_{35}=0.0\hat{i}+10.0\hat{j}+0.0\hat{k}$.

2D-M552:

$\hat{n}_{13}=-0.71\hat{i}+0.0\hat{j}+0.71\hat{k}$,\;\;\;$\hat{n}_{14}=-0.58\hat{i}-0.56\hat{j}-0.58\hat{k}$,\;\;\;$\hat{n}_{24}=0.42\hat{i}-0.8\hat{j}+0.42\hat{k}$,\;\;\;$\hat{n}_{25}=0.23\hat{i}+0.94\hat{j}+0.23\hat{k}$,\newline
$\hat{n}_{35}=-0.05\hat{i}-1.0\hat{j}-0.05\hat{k}$,\;\;\;$\vec{r}_{13}=4.97\hat{i}+4.99\hat{j}+4.94\hat{k}$,\;\;\;$\vec{r}_{14}=0.0\hat{i}+10.0\hat{j}+10.0\hat{k}$,\;\;\;$\vec{r}_{24}=10.0\hat{i}+10.0\hat{j}+10.0\hat{k}$,\newline
$\vec{r}_{25}=10.0\hat{i}+0.0\hat{j}+0.0\hat{k}$.

2D-M553:

$\hat{n}_{13}=0.27\hat{i}+0.95\hat{j}-0.13\hat{k}$,\;\;\;$\hat{n}_{14}=0.72\hat{i}-0.1\hat{j}+0.69\hat{k}$,\;\;\;$\hat{n}_{24}=0.66\hat{i}-0.23\hat{j}-0.72\hat{k}$,\;\;\;$\hat{n}_{25}=0.23\hat{i}+0.97\hat{j}-0.09\hat{k}$,\newline
$\hat{n}_{35}=-0.16\hat{i}+0.94\hat{j}+0.29\hat{k}$,\;\;\;$\vec{r}_{13}=10.0\hat{i}+0.0\hat{j}+10.0\hat{k}$,\;\;\;$\vec{r}_{14}=5.05\hat{i}+4.92\hat{j}+4.92\hat{k}$,\;\;\;$\vec{r}_{24}=5.05\hat{i}+5.0\hat{j}+4.99\hat{k}$,\newline
$\vec{r}_{35}=10.0\hat{i}+10.0\hat{j}+0.0\hat{k}$.

2D-M554:

$\hat{n}_{13}=-0.64\hat{i}-0.14\hat{j}+0.75\hat{k}$,\;\;\;$\hat{n}_{14}=0.57\hat{i}-0.74\hat{j}+0.35\hat{k}$,\;\;\;$\hat{n}_{23}=0.57\hat{i}-0.74\hat{j}+0.35\hat{k}$,\;\;\;$\hat{n}_{24}=0.51\hat{i}+0.66\hat{j}+0.56\hat{k}$,\newline
$\hat{n}_{45}=0.03\hat{i}-1.0\hat{j}-0.06\hat{k}$,\;\;\;$\vec{r}_{13}=4.92\hat{i}+5.04\hat{j}+4.91\hat{k}$,\;\;\;$\vec{r}_{14}=10.0\hat{i}+10.0\hat{j}+10.0\hat{k}$,\;\;\;$\vec{r}_{23}=4.98\hat{i}+4.91\hat{j}+4.97\hat{k}$,\newline
$\vec{r}_{24}=4.94\hat{i}+5.08\hat{j}+4.94\hat{k}$.

2D-M555:

$\hat{n}_{13}=0.16\hat{i}-0.75\hat{j}+0.64\hat{k}$,\;\;\;$\hat{n}_{14}=0.44\hat{i}-0.53\hat{j}-0.73\hat{k}$,\;\;\;$\hat{n}_{23}=0.16\hat{i}-0.75\hat{j}+0.64\hat{k}$,\;\;\;$\hat{n}_{24}=-0.89\hat{i}-0.39\hat{j}-0.24\hat{k}$,\newline
$\hat{n}_{35}=0.6\hat{i}-0.8\hat{j}+0.07\hat{k}$,\;\;\;$\vec{r}_{13}=0.0\hat{i}+10.0\hat{j}+0.0\hat{k}$,\;\;\;$\vec{r}_{14}=5.03\hat{i}+4.83\hat{j}+5.0\hat{k}$,\;\;\;$\vec{r}_{23}=4.81\hat{i}+4.8\hat{j}+5.08\hat{k}$,\newline
$\vec{r}_{24}=4.89\hat{i}+4.91\hat{j}+5.2\hat{k}$.

2D-M556:

$\hat{n}_{13}=0.27\hat{i}-0.66\hat{j}+0.7\hat{k}$,\;\;\;$\hat{n}_{14}=-0.64\hat{i}+0.41\hat{j}+0.65\hat{k}$,\;\;\;$\hat{n}_{23}=-0.78\hat{i}-0.36\hat{j}+0.5\hat{k}$,\;\;\;$\hat{n}_{24}=-0.72\hat{i}-0.57\hat{j}-0.41\hat{k}$,\newline
$\hat{n}_{25}=-0.73\hat{i}-0.66\hat{j}+0.18\hat{k}$,\;\;\;$\vec{r}_{13}=10.0\hat{i}+10.0\hat{j}+0.0\hat{k}$,\;\;\;$\vec{r}_{14}=10.0\hat{i}+10.0\hat{j}+10.0\hat{k}$,\;\;\;$\vec{r}_{23}=10.0\hat{i}+0.0\hat{j}+0.0\hat{k}$,\newline
$\vec{r}_{24}=10.0\hat{i}+0.0\hat{j}+10.0\hat{k}$.

2D-M557:

$\hat{n}_{13}=0.74\hat{i}+0.35\hat{j}+0.57\hat{k}$,\;\;\;$\hat{n}_{14}=-0.62\hat{i}+0.67\hat{j}+0.4\hat{k}$,\;\;\;$\hat{n}_{23}=0.62\hat{i}-0.67\hat{j}-0.4\hat{k}$,\;\;\;$\hat{n}_{24}=-0.24\hat{i}-0.65\hat{j}+0.72\hat{k}$,\newline
$\hat{n}_{45}=0.88\hat{i}+0.18\hat{j}+0.44\hat{k}$,\;\;\;$\vec{r}_{13}=4.95\hat{i}+4.94\hat{j}+5.0\hat{k}$,\;\;\;$\vec{r}_{14}=4.95\hat{i}+4.95\hat{j}+4.95\hat{k}$,\;\;\;$\vec{r}_{24}=5.06\hat{i}+5.05\hat{j}+5.06\hat{k}$,\newline
$\vec{r}_{45}=10.0\hat{i}+0.0\hat{j}+10.0\hat{k}$.

2D-M558:

$\hat{n}_{13}=-0.01\hat{i}-0.88\hat{j}+0.47\hat{k}$,\;\;\;$\hat{n}_{14}=-0.58\hat{i}-0.38\hat{j}-0.72\hat{k}$,\;\;\;$\hat{n}_{23}=-0.01\hat{i}-0.88\hat{j}+0.47\hat{k}$,\;\;\;$\hat{n}_{24}=0.82\hat{i}-0.28\hat{j}-0.5\hat{k}$,\newline
$\hat{n}_{35}=0.8\hat{i}-0.59\hat{j}+0.14\hat{k}$,\;\;\;$\vec{r}_{13}=5.0\hat{i}+5.04\hat{j}+4.87\hat{k}$,\;\;\;$\vec{r}_{14}=5.14\hat{i}+4.88\hat{j}+4.93\hat{k}$,\;\;\;$\vec{r}_{24}=5.06\hat{i}+5.14\hat{j}+4.94\hat{k}$,\newline
$\vec{r}_{35}=10.0\hat{i}+10.0\hat{j}+0.0\hat{k}$.

2D-M559:

$\hat{n}_{13}=-0.52\hat{i}+0.68\hat{j}+0.52\hat{k}$,\;\;\;$\hat{n}_{14}=0.69\hat{i}+0.69\hat{j}-0.23\hat{k}$,\;\;\;$\hat{n}_{23}=-0.39\hat{i}-0.72\hat{j}+0.57\hat{k}$,\;\;\;$\hat{n}_{24}=0.51\hat{i}-0.24\hat{j}+0.83\hat{k}$,\newline
$\hat{n}_{25}=-0.8\hat{i}+0.34\hat{j}-0.49\hat{k}$,\;\;\;$\vec{r}_{13}=5.36\hat{i}+4.71\hat{j}+5.12\hat{k}$,\;\;\;$\vec{r}_{14}=5.38\hat{i}+5.66\hat{j}+5.16\hat{k}$,\;\;\;$\vec{r}_{24}=5.07\hat{i}+4.73\hat{j}+5.36\hat{k}$,\newline
$\vec{r}_{25}=10.0\hat{i}+10.0\hat{j}+0.0\hat{k}$.
