# Supplementary material for: Dimensional synthesis of spatial manipulators for velocity and force transmission for operation around a specified task point
Source: arXiv:2210.04446 source file (2022-10-10)
Supplement: Supplementary file 15 [file AppendixE.tex]

% Appendix Template

\chapter{Results of optimisation for manipulators of of DOF 3} % Main appendix title

\label{AppendixE} % Change X to a consecutive letter; for referencing this appendix elsewhere, use \ref{AppendixX}

\lhead{Appendix E. \emph{Results of optimisation for manipulators of of DOF 3}} % Change X to a consecutive letter; this is for the header on each page - perhaps a shortened title
%\subsection{Class 1} \label{appendix_five_3_1}
\begingroup\makeatletter\def\f@size{5}\check@mathfonts
\subsection{Class 1} \label{appendix_five_2_1}
{\tiny 3D-M1:}

$\hat{n}_{13}=-0.71\hat{i}+0.11\hat{j}-0.7\hat{k}$,\;\;\;$\hat{n}_{23}=-0.0\hat{i}+0.58\hat{j}-0.81\hat{k}$,\;\;\;$\hat{n}_{24}=0.82\hat{i}-0.46\hat{j}-0.34\hat{k}$,\;\;\;$\vec{r}_{13}=10.0\hat{i}+10.0\hat{j}+0.0\hat{k}$,\newline
$\vec{r}_{23}=10.0\hat{i}+0.0\hat{j}+10.0\hat{k}$,\;\;\;$\vec{r}_{24}=10.0\hat{i}+10.0\hat{j}+10.0\hat{k}$.

\subsection{Class 2} \label{appendix_five_2_1}
{\tiny 3D-M2:}

$\hat{n}_{13}=-0.8\hat{i}+0.33\hat{j}+0.49\hat{k}$,\;\;\;$\hat{n}_{23}=-0.17\hat{i}+0.67\hat{j}-0.73\hat{k}$,\;\;\;$\hat{n}_{24}=-0.57\hat{i}-0.67\hat{j}-0.48\hat{k}$,\;\;\;$\vec{r}_{13}=10.0\hat{i}+10.0\hat{j}+10.0\hat{k}$,\newline
$\vec{r}_{23}=10.0\hat{i}+10.0\hat{j}+10.0\hat{k}$.

{\tiny 3D-M3:}

$\hat{n}_{13}=-0.8\hat{i}+0.58\hat{j}+0.14\hat{k}$,\;\;\;$\hat{n}_{23}=-0.74\hat{i}-0.51\hat{j}-0.43\hat{k}$,\;\;\;$\hat{n}_{24}=0.51\hat{i}+0.16\hat{j}+0.84\hat{k}$,\;\;\;$\vec{r}_{13}=10.0\hat{i}+10.0\hat{j}+10.0\hat{k}$,\newline
$\vec{r}_{24}=10.0\hat{i}+10.0\hat{j}+0.0\hat{k}$.

{\tiny 3D-M4:}

$\hat{n}_{13}=-0.57\hat{i}-0.67\hat{j}-0.48\hat{k}$,\;\;\;$\hat{n}_{23}=-0.31\hat{i}-0.36\hat{j}-0.88\hat{k}$,\;\;\;$\hat{n}_{24}=0.76\hat{i}-0.65\hat{j}+0.0\hat{k}$,\;\;\;$\vec{r}_{23}=10.0\hat{i}+10.0\hat{j}+0.0\hat{k}$,\newline
$\vec{r}_{24}=10.0\hat{i}+10.0\hat{j}+10.0\hat{k}$.

\subsection{Class 3} \label{appendix_five_2_1}
{\tiny 3D-M5:}

$\hat{n}_{13}=0.5\hat{i}+0.18\hat{j}+0.85\hat{k}$,\;\;\;$\hat{n}_{23}=-0.76\hat{i}-0.61\hat{j}-0.24\hat{k}$,\;\;\;$\hat{n}_{24}=0.03\hat{i}+0.33\hat{j}-0.94\hat{k}$,\;\;\;$\vec{r}_{13}=10.0\hat{i}+10.0\hat{j}+0.0\hat{k}$.

{\tiny 3D-M6:}

$\hat{n}_{13}=-0.6\hat{i}-0.76\hat{j}-0.26\hat{k}$,\;\;\;$\hat{n}_{23}=0.26\hat{i}+0.4\hat{j}+0.88\hat{k}$,\;\;\;$\hat{n}_{24}=-0.21\hat{i}-0.17\hat{j}+0.96\hat{k}$,\;\;\;$\vec{r}_{23}=10.0\hat{i}+10.0\hat{j}+0.0\hat{k}$.

{\tiny 3D-M7:}

$\hat{n}_{13}=-0.54\hat{i}-0.83\hat{j}+0.12\hat{k}$,\;\;\;$\hat{n}_{23}=0.18\hat{i}-0.26\hat{j}-0.95\hat{k}$,\;\;\;$\hat{n}_{24}=-0.04\hat{i}-0.56\hat{j}-0.83\hat{k}$,\;\;\;$\vec{r}_{24}=10.0\hat{i}+10.0\hat{j}+0.0\hat{k}$.

\subsection{Class 4} \label{appendix_five_2_1}
{\tiny 3D-M8:}

$\hat{n}_{13}=0.41\hat{i}+0.89\hat{j}-0.2\hat{k}$,\;\;\;$\hat{n}_{23}=-0.62\hat{i}+0.11\hat{j}-0.78\hat{k}$,\;\;\;$\hat{n}_{24}=-0.67\hat{i}+0.44\hat{j}+0.59\hat{k}$.

\endgroup
