# Supplementary material for: Dimensional synthesis of spatial manipulators for velocity and force transmission for operation around a specified task point
Source: arXiv:2210.04446 source file (2022-10-10)
Supplement: Supplementary file 16 [file AppendixF.tex]

% Appendix Template

\chapter{Results of optimisation for manipulators of of DOF 4} % Main appendix title

\label{AppendixF} % Change X to a consecutive letter; for referencing this appendix elsewhere, use \ref{AppendixX}

\lhead{Appendix F. \emph{Results of optimisation for manipulators of of DOF 4}} % Change X to a consecutive letter; this is for the header on each page - perhaps a shortened title
%\subsection{Class 1} \label{appendix_five_4_1}
\begingroup\makeatletter\def\f@size{5}\check@mathfonts
\subsection{Class 1} \label{appendix_five_2_1}
{\tiny 4D-M1:}

$\hat{n}_{14}=-0.29\hat{i}+0.57\hat{j}-0.77\hat{k}$,\;\;\;$\hat{n}_{23}=0.75\hat{i}-0.53\hat{j}+0.4\hat{k}$,\;\;\;$\hat{n}_{25}=-0.34\hat{i}+0.83\hat{j}-0.45\hat{k}$,\;\;\;$\hat{n}_{34}=-0.72\hat{i}+0.12\hat{j}+0.69\hat{k}$,\newline
$\vec{r}_{14}=10.0\hat{i}+0.0\hat{j}+10.0\hat{k}$,\;\;\;$\vec{r}_{23}=10.0\hat{i}+10.0\hat{j}+0.0\hat{k}$,\;\;\;$\vec{r}_{25}=0.0\hat{i}+0.0\hat{j}+0.0\hat{k}$,\;\;\;$\vec{r}_{34}=10.0\hat{i}+10.0\hat{j}+10.0\hat{k}$.

\subsection{Class 2} \label{appendix_five_2_1}
{\tiny 4D-M2:}

$\hat{n}_{14}=0.82\hat{i}+0.49\hat{j}+0.3\hat{k}$,\;\;\;$\hat{n}_{23}=-0.39\hat{i}-0.47\hat{j}-0.79\hat{k}$,\;\;\;$\hat{n}_{25}=-0.42\hat{i}-0.85\hat{j}-0.32\hat{k}$,\;\;\;$\hat{n}_{34}=0.57\hat{i}+0.69\hat{j}+0.45\hat{k}$,\newline
$\vec{r}_{14}=10.0\hat{i}+0.0\hat{j}+10.0\hat{k}$,\;\;\;$\vec{r}_{23}=10.0\hat{i}+10.0\hat{j}+0.0\hat{k}$,\;\;\;$\vec{r}_{25}=0.0\hat{i}+10.0\hat{j}+10.0\hat{k}$.

{\tiny 4D-M3:}

$\hat{n}_{14}=0.39\hat{i}+0.47\hat{j}-0.79\hat{k}$,\;\;\;$\hat{n}_{23}=-0.42\hat{i}-0.85\hat{j}+0.32\hat{k}$,\;\;\;$\hat{n}_{25}=-0.57\hat{i}-0.69\hat{j}+0.45\hat{k}$,\;\;\;$\hat{n}_{34}=0.82\hat{i}+0.49\hat{j}-0.3\hat{k}$,\newline
$\vec{r}_{14}=10.0\hat{i}+10.0\hat{j}+10.0\hat{k}$,\;\;\;$\vec{r}_{23}=0.0\hat{i}+10.0\hat{j}+0.0\hat{k}$,\;\;\;$\vec{r}_{34}=10.0\hat{i}+0.0\hat{j}+0.0\hat{k}$.

{\tiny 4D-M4:}

$\hat{n}_{14}=0.42\hat{i}+0.85\hat{j}-0.32\hat{k}$,\;\;\;$\hat{n}_{23}=-0.57\hat{i}-0.69\hat{j}+0.45\hat{k}$,\;\;\;$\hat{n}_{25}=-0.39\hat{i}-0.47\hat{j}+0.79\hat{k}$,\;\;\;$\hat{n}_{34}=0.82\hat{i}+0.49\hat{j}-0.3\hat{k}$,\newline
$\vec{r}_{14}=0.0\hat{i}+10.0\hat{j}+0.0\hat{k}$,\;\;\;$\vec{r}_{25}=10.0\hat{i}+10.0\hat{j}+10.0\hat{k}$,\;\;\;$\vec{r}_{34}=10.0\hat{i}+0.0\hat{j}+0.0\hat{k}$.

{\tiny 4D-M5:}

$\hat{n}_{14}=-0.57\hat{i}-0.69\hat{j}-0.45\hat{k}$,\;\;\;$\hat{n}_{23}=0.42\hat{i}+0.85\hat{j}+0.32\hat{k}$,\;\;\;$\hat{n}_{25}=0.82\hat{i}+0.49\hat{j}+0.3\hat{k}$,\;\;\;$\hat{n}_{34}=-0.39\hat{i}-0.47\hat{j}-0.79\hat{k}$,\newline
$\vec{r}_{23}=0.0\hat{i}+10.0\hat{j}+10.0\hat{k}$,\;\;\;$\vec{r}_{25}=10.0\hat{i}+0.0\hat{j}+10.0\hat{k}$,\;\;\;$\vec{r}_{34}=10.0\hat{i}+10.0\hat{j}+0.0\hat{k}$.

\subsection{Class 3} \label{appendix_five_2_1}
{\tiny 4D-M6:}

$\hat{n}_{14}=-0.54\hat{i}-0.84\hat{j}-0.08\hat{k}$,\;\;\;$\hat{n}_{23}=-0.68\hat{i}-0.7\hat{j}-0.22\hat{k}$,\;\;\;$\hat{n}_{25}=0.62\hat{i}-0.53\hat{j}+0.59\hat{k}$,\;\;\;$\hat{n}_{34}=-0.58\hat{i}-0.81\hat{j}-0.12\hat{k}$,\newline
$\vec{r}_{14}=0.0\hat{i}+10.0\hat{j}+10.0\hat{k}$,\;\;\;$\vec{r}_{23}=10.0\hat{i}+0.0\hat{j}+0.0\hat{k}$.

{\tiny 4D-M7:}

$\hat{n}_{14}=0.54\hat{i}+0.84\hat{j}-0.08\hat{k}$,\;\;\;$\hat{n}_{23}=-0.05\hat{i}+0.94\hat{j}+0.34\hat{k}$,\;\;\;$\hat{n}_{25}=-0.68\hat{i}-0.7\hat{j}+0.22\hat{k}$,\;\;\;$\hat{n}_{34}=0.84\hat{i}+0.22\hat{j}-0.49\hat{k}$,\newline
$\vec{r}_{14}=0.0\hat{i}+10.0\hat{j}+0.0\hat{k}$,\;\;\;$\vec{r}_{25}=10.0\hat{i}+0.0\hat{j}+10.0\hat{k}$.

{\tiny 4D-M8:}

$\hat{n}_{14}=0.54\hat{i}+0.84\hat{j}-0.08\hat{k}$,\;\;\;$\hat{n}_{23}=-0.26\hat{i}+0.85\hat{j}+0.46\hat{k}$,\;\;\;$\hat{n}_{25}=-0.8\hat{i}-0.46\hat{j}+0.38\hat{k}$,\;\;\;$\hat{n}_{34}=-0.68\hat{i}-0.7\hat{j}+0.22\hat{k}$,\newline
$\vec{r}_{14}=0.0\hat{i}+10.0\hat{j}+0.0\hat{k}$,\;\;\;$\vec{r}_{34}=10.0\hat{i}+0.0\hat{j}+10.0\hat{k}$.

{\tiny 4D-M9:}

$\hat{n}_{14}=-0.08\hat{i}-0.96\hat{j}-0.27\hat{k}$,\;\;\;$\hat{n}_{23}=0.54\hat{i}+0.84\hat{j}-0.08\hat{k}$,\;\;\;$\hat{n}_{25}=-0.68\hat{i}-0.7\hat{j}+0.22\hat{k}$,\;\;\;$\hat{n}_{34}=-0.84\hat{i}-0.08\hat{j}+0.53\hat{k}$,\newline
$\vec{r}_{23}=0.0\hat{i}+10.0\hat{j}+0.0\hat{k}$,\;\;\;$\vec{r}_{25}=10.0\hat{i}+0.0\hat{j}+10.0\hat{k}$.

{\tiny 4D-M10:}

$\hat{n}_{14}=-0.63\hat{i}-0.76\hat{j}-0.17\hat{k}$,\;\;\;$\hat{n}_{23}=-0.54\hat{i}-0.84\hat{j}-0.08\hat{k}$,\;\;\;$\hat{n}_{25}=-0.56\hat{i}+0.59\hat{j}-0.57\hat{k}$,\;\;\;$\hat{n}_{34}=-0.68\hat{i}-0.7\hat{j}-0.22\hat{k}$,\newline
$\vec{r}_{23}=0.0\hat{i}+10.0\hat{j}+10.0\hat{k}$,\;\;\;$\vec{r}_{34}=10.0\hat{i}+0.0\hat{j}+0.0\hat{k}$.

{\tiny 4D-M11:}

$\hat{n}_{14}=-0.32\hat{i}+0.81\hat{j}-0.49\hat{k}$,\;\;\;$\hat{n}_{23}=0.78\hat{i}+0.52\hat{j}+0.35\hat{k}$,\;\;\;$\hat{n}_{25}=-0.68\hat{i}-0.7\hat{j}-0.22\hat{k}$,\;\;\;$\hat{n}_{34}=0.54\hat{i}+0.84\hat{j}+0.08\hat{k}$,\newline
$\vec{r}_{25}=10.0\hat{i}+0.0\hat{j}+0.0\hat{k}$,\;\;\;$\vec{r}_{34}=0.0\hat{i}+10.0\hat{j}+10.0\hat{k}$.

\subsection{Class 4} \label{appendix_five_2_1}
{\tiny 4D-M12:}

$\hat{n}_{14}=0.09\hat{i}-1.0\hat{j}+0.05\hat{k}$,\;\;\;$\hat{n}_{23}=0.67\hat{i}+0.35\hat{j}+0.66\hat{k}$,\;\;\;$\hat{n}_{25}=0.01\hat{i}-0.88\hat{j}+0.47\hat{k}$,\;\;\;$\hat{n}_{34}=-0.75\hat{i}+0.31\hat{j}+0.59\hat{k}$,\newline
$\vec{r}_{14}=4.0\hat{i}+2.99\hat{j}+5.94\hat{k}$.

{\tiny 4D-M13:}

$\hat{n}_{14}=-0.94\hat{i}-0.18\hat{j}-0.29\hat{k}$,\;\;\;$\hat{n}_{23}=0.32\hat{i}-0.95\hat{j}+0.01\hat{k}$,\;\;\;$\hat{n}_{25}=-0.03\hat{i}-0.8\hat{j}+0.59\hat{k}$,\;\;\;$\hat{n}_{34}=0.34\hat{i}-0.57\hat{j}-0.75\hat{k}$,\newline
$\vec{r}_{23}=7.59\hat{i}+3.33\hat{j}+4.0\hat{k}$.

{\tiny 4D-M14:}

$\hat{n}_{14}=-0.38\hat{i}-0.54\hat{j}-0.75\hat{k}$,\;\;\;$\hat{n}_{23}=-0.54\hat{i}-0.53\hat{j}+0.65\hat{k}$,\;\;\;$\hat{n}_{25}=0.34\hat{i}-0.93\hat{j}-0.12\hat{k}$,\;\;\;$\hat{n}_{34}=0.75\hat{i}-0.65\hat{j}+0.1\hat{k}$,\newline
$\vec{r}_{25}=3.55\hat{i}+6.33\hat{j}+6.15\hat{k}$.

{\tiny 4D-M15:}

$\hat{n}_{14}=-0.19\hat{i}-0.68\hat{j}-0.71\hat{k}$,\;\;\;$\hat{n}_{23}=0.56\hat{i}-0.67\hat{j}+0.49\hat{k}$,\;\;\;$\hat{n}_{25}=-0.8\hat{i}-0.3\hat{j}+0.51\hat{k}$,\;\;\;$\hat{n}_{34}=0.84\hat{i}-0.54\hat{j}+0.05\hat{k}$,\newline
$\vec{r}_{34}=3.99\hat{i}+5.66\hat{j}+6.62\hat{k}$.

\endgroup
