# Supplementary material for: Dimensional synthesis of spatial manipulators for velocity and force transmission for operation around a specified task point
Source: arXiv:2210.04446 source file (2022-10-10)
Supplement: Supplementary file 27 [file Appendix_main.tex]

\section*{Appendix A}
\label{AppendixA}

%\input{contentfolder/mechanisms2/manipulabilitytable2}
% \section*{Appendix A}
% \label{AppendixA}

\tiny
\begin{center}
%\label{Tab:table_dof2mt_1}
\tablefirsthead{%
\hline
%\multicolumn{1}{|c}{\tbsp S.No.} &
\multicolumn{1}{|c|}{S.No.} &
%\tbsp S.No. &
%\multicolumn{1}{c}{Name} &
Name &
$\bar{\mu}$ &
$\kappa$ &
$i_{\kappa}$ &
%\multicolumn{1}{c}{$\mu$} &
$\mu$ &
\multicolumn{1}{c|}{$f$} &
AJV \\
\hline}
\tablehead{%
\hline
%\multicolumn{5}{|l|}{\small\sl continued from previous page}\\
\multicolumn{8}{|l|}{\tiny\sl continuing...}\\
\hline
\multicolumn{1}{|c|}{S.No.} &
Name &
$\bar{\mu}$ &
$\kappa$ &
$i_{\kappa}$ &
$\mu$ &
\multicolumn{1}{c|}{$f$} &
AJV \\
\hline}
\tabletail{%
\hline
%\multicolumn{5}{|r|}{\small\sl continued on next page}\\
\multicolumn{8}{|r|}{\tiny\sl ...continued}\\
\hline}
\tablelasttail{\hline}
%\vskip -0.20cm
\bottomcaption{Prescription of 2-DOF Manipulators.}

%\tablehead{S.No. & Name & $\bar{\mu}$ & $\mu$ & $f$ \\}

%% [inline block 0: 1 envs, 61192 chars -> data_tex | \begin{supertabular}{||c|c|c|c|c||} \begin{supertabular}{|r|r|r|r|r|r|r|r|}...]

\end{center}

%\end{longtable}

\normalsize
