# Supplementary material for: Dimensional synthesis of spatial manipulators for velocity and force transmission for operation around a specified task point
Source: arXiv:2210.04446 source file (2022-10-10)
Supplement: Supplementary file 28 [file classappendix1.tex]

\subsection*{Class 1} \label{appendix_five_2_1}

{\tiny 1D-M1:}

$\hat{n}_{13}=0.0\hat{i}+0.0\hat{j}+1.0\hat{k}$,\;\;\;$\hat{n}_{14}=0.02\hat{i}-0.52\hat{j}+0.85\hat{k}$,\;\;\;$\hat{n}_{23}=0.75\hat{i}-0.51\hat{j}+0.42\hat{k}$,\;\;\;$\vec{r}_{13}=10.0\hat{i}+0.0\hat{j}+0.53\hat{k}$,\;\;\;$\vec{r}_{14}=10.0\hat{i}+0.0\hat{j}+10.0\hat{k}$,\;\;\;$\vec{r}_{23}=0.0\hat{i}+0.0\hat{j}+0.0\hat{k}$,\;\;\;$\vec{r}_{24}=10.0\hat{i}+10.0\hat{j}+10.0\hat{k}$.

{\tiny 1D-M2:}

$\hat{n}_{13}=0.58\hat{i}+0.58\hat{j}-0.58\hat{k}$,\;\;\;$\hat{n}_{14}=0.0\hat{i}+0.77\hat{j}+0.63\hat{k}$,\;\;\;$\hat{n}_{24}=0.29\hat{i}+0.95\hat{j}-0.09\hat{k}$,\;\;\;$\vec{r}_{13}=0.0\hat{i}+10.0\hat{j}+0.0\hat{k}$,\;\;\;$\vec{r}_{14}=0.0\hat{i}+0.0\hat{j}+10.0\hat{k}$,\;\;\;$\vec{r}_{23}=10.0\hat{i}+0.0\hat{j}+0.0\hat{k}$,\;\;\;$\vec{r}_{24}=0.0\hat{i}+10.0\hat{j}+10.0\hat{k}$.

{\tiny 1D-M3:}

$\hat{n}_{13}=-0.03\hat{i}-0.71\hat{j}-0.71\hat{k}$,\;\;\;$\hat{n}_{14}=0.71\hat{i}-0.68\hat{j}-0.18\hat{k}$,\;\;\;$\hat{n}_{23}=-0.82\hat{i}-0.37\hat{j}+0.44\hat{k}$,\;\;\;$\vec{r}_{13}=10.0\hat{i}+10.0\hat{j}+0.0\hat{k}$,\;\;\;$\vec{r}_{14}=0.0\hat{i}+0.0\hat{j}+0.0\hat{k}$,\;\;\;$\vec{r}_{23}=10.0\hat{i}+0.0\hat{j}+0.0\hat{k}$,\;\;\;$\vec{r}_{24}=0.0\hat{i}+10.0\hat{j}+10.0\hat{k}$.

{\tiny 1D-M4:}

$\hat{n}_{13}=-0.0\hat{i}+0.0\hat{j}-1.0\hat{k}$,\;\;\;$\hat{n}_{14}=-0.58\hat{i}-0.8\hat{j}+0.15\hat{k}$,\;\;\;$\hat{n}_{24}=0.53\hat{i}+0.6\hat{j}+0.6\hat{k}$,\;\;\;$\vec{r}_{13}=10.0\hat{i}+0.0\hat{j}+10.0\hat{k}$,\;\;\;$\vec{r}_{14}=10.0\hat{i}+0.0\hat{j}+10.0\hat{k}$,\;\;\;$\vec{r}_{23}=0.0\hat{i}+10.0\hat{j}+10.0\hat{k}$,\;\;\;$\vec{r}_{24}=10.0\hat{i}+10.0\hat{j}+0.0\hat{k}$.

{\tiny 1D-M5:}

$\hat{n}_{13}=-0.08\hat{i}+0.46\hat{j}+0.89\hat{k}$,\;\;\;$\hat{n}_{23}=0.61\hat{i}-0.33\hat{j}+0.72\hat{k}$,\;\;\;$\hat{n}_{24}=0.79\hat{i}-0.58\hat{j}-0.19\hat{k}$,\;\;\;$\vec{r}_{13}=0.0\hat{i}+10.0\hat{j}+10.0\hat{k}$,\;\;\;$\vec{r}_{14}=10.0\hat{i}+10.0\hat{j}+0.0\hat{k}$,\;\;\;$\vec{r}_{23}=10.0\hat{i}+0.0\hat{j}+10.0\hat{k}$,\;\;\;$\vec{r}_{24}=0.0\hat{i}+0.0\hat{j}+0.0\hat{k}$.

{\tiny 1D-M6:}

$\hat{n}_{13}=0.0\hat{i}+0.37\hat{j}+0.93\hat{k}$,\;\;\;$\hat{n}_{23}=0.33\hat{i}-0.66\hat{j}+0.67\hat{k}$,\;\;\;$\hat{n}_{24}=0.84\hat{i}-0.53\hat{j}-0.09\hat{k}$,\;\;\;$\vec{r}_{13}=0.0\hat{i}+10.0\hat{j}+10.0\hat{k}$,\;\;\;$\vec{r}_{14}=10.0\hat{i}+10.0\hat{j}+10.0\hat{k}$,\;\;\;$\vec{r}_{23}=0.0\hat{i}+0.0\hat{j}+0.0\hat{k}$,\;\;\;$\vec{r}_{24}=10.0\hat{i}+10.0\hat{j}+0.0\hat{k}$.

{\tiny 1D-M7:}

$\hat{n}_{13}=-0.21\hat{i}-0.95\hat{j}-0.24\hat{k}$,\;\;\;$\hat{n}_{14}=0.41\hat{i}-0.48\hat{j}-0.78\hat{k}$,\;\;\;$\hat{n}_{23}=-0.17\hat{i}-0.96\hat{j}+0.24\hat{k}$,\;\;\;$\vec{r}_{13}=5.38\hat{i}+6.86\hat{j}+4.63\hat{k}$,\;\;\;$\vec{r}_{14}=0.0\hat{i}+10.0\hat{j}+10.0\hat{k}$,\;\;\;$\vec{r}_{23}=6.61\hat{i}+5.26\hat{j}+5.64\hat{k}$,\;\;\;$\vec{r}_{24}=5.08\hat{i}+5.88\hat{j}+3.64\hat{k}$.

{\tiny 1D-M8:}

$\hat{n}_{13}=-0.72\hat{i}-0.39\hat{j}+0.57\hat{k}$,\;\;\;$\hat{n}_{14}=0.31\hat{i}-0.9\hat{j}+0.29\hat{k}$,\;\;\;$\hat{n}_{24}=-0.04\hat{i}-1.0\hat{j}+0.06\hat{k}$,\;\;\;$\vec{r}_{13}=6.43\hat{i}+4.57\hat{j}+5.96\hat{k}$,\;\;\;$\vec{r}_{14}=0.0\hat{i}+0.0\hat{j}+0.0\hat{k}$,\;\;\;$\vec{r}_{23}=3.69\hat{i}+6.29\hat{j}+5.5\hat{k}$,\;\;\;$\vec{r}_{24}=5.32\hat{i}+3.65\hat{j}+6.36\hat{k}$.

{\tiny 1D-M9:}

$\hat{n}_{13}=0.44\hat{i}+0.64\hat{j}+0.63\hat{k}$,\;\;\;$\hat{n}_{23}=0.15\hat{i}+0.42\hat{j}-0.9\hat{k}$,\;\;\;$\hat{n}_{24}=0.5\hat{i}+0.61\hat{j}-0.62\hat{k}$,\;\;\;$\vec{r}_{13}=0.0\hat{i}+10.0\hat{j}+10.0\hat{k}$,\;\;\;$\vec{r}_{14}=10.0\hat{i}+0.0\hat{j}+10.0\hat{k}$,\;\;\;$\vec{r}_{23}=10.0\hat{i}+10.0\hat{j}+10.0\hat{k}$,\;\;\;$\vec{r}_{24}=0.0\hat{i}+0.0\hat{j}+0.0\hat{k}$.

{\tiny 1D-M10:}

$\hat{n}_{14}=0.0\hat{i}+0.0\hat{j}-1.0\hat{k}$,\;\;\;$\hat{n}_{23}=0.04\hat{i}-0.71\hat{j}+0.7\hat{k}$,\;\;\;$\hat{n}_{24}=-0.84\hat{i}-0.49\hat{j}-0.25\hat{k}$,\;\;\;$\vec{r}_{13}=3.76\hat{i}+5.51\hat{j}+5.34\hat{k}$,\;\;\;$\vec{r}_{14}=10.0\hat{i}+0.0\hat{j}+1.6\hat{k}$,\;\;\;$\vec{r}_{23}=4.11\hat{i}+6.4\hat{j}+4.81\hat{k}$,\;\;\;$\vec{r}_{24}=4.67\hat{i}+3.62\hat{j}+5.9\hat{k}$.

{\tiny 1D-M11:}

$\hat{n}_{14}=0.16\hat{i}-0.66\hat{j}+0.74\hat{k}$,\;\;\;$\hat{n}_{23}=0.89\hat{i}-0.47\hat{j}-0.02\hat{k}$,\;\;\;$\hat{n}_{24}=-0.96\hat{i}-0.28\hat{j}-0.02\hat{k}$,\;\;\;$\vec{r}_{13}=2.15\hat{i}+6.75\hat{j}+2.1\hat{k}$,\;\;\;$\vec{r}_{14}=10.0\hat{i}+10.0\hat{j}+10.0\hat{k}$,\;\;\;$\vec{r}_{23}=1.36\hat{i}+8.7\hat{j}+7.55\hat{k}$,\;\;\;$\vec{r}_{24}=4.88\hat{i}+4.39\hat{j}+4.5\hat{k}$.

{\tiny 1D-M12:}

$\hat{n}_{14}=-0.0\hat{i}+0.0\hat{j}+1.0\hat{k}$,\;\;\;$\hat{n}_{23}=0.0\hat{i}+0.76\hat{j}-0.65\hat{k}$,\;\;\;$\hat{n}_{24}=0.21\hat{i}-0.79\hat{j}-0.58\hat{k}$,\;\;\;$\vec{r}_{13}=0.0\hat{i}+0.0\hat{j}+10.0\hat{k}$,\;\;\;$\vec{r}_{14}=0.0\hat{i}+10.0\hat{j}+2.63\hat{k}$,\;\;\;$\vec{r}_{23}=10.0\hat{i}+10.0\hat{j}+10.0\hat{k}$,\;\;\;$\vec{r}_{24}=10.0\hat{i}+10.0\hat{j}+0.0\hat{k}$.

{\tiny 1D-M13:}

$\hat{n}_{12}=-0.82\hat{i}-0.54\hat{j}+0.19\hat{k}$,\;\;\;$\hat{n}_{13}=0.82\hat{i}+0.0\hat{j}-0.57\hat{k}$,\;\;\;$\hat{n}_{24}=0.03\hat{i}-0.82\hat{j}-0.57\hat{k}$,\;\;\;$\vec{r}_{12}=10.0\hat{i}+0.0\hat{j}+10.0\hat{k}$,\;\;\;$\vec{r}_{13}=0.0\hat{i}+0.0\hat{j}+0.0\hat{k}$,\;\;\;$\vec{r}_{24}=0.0\hat{i}+10.0\hat{j}+10.0\hat{k}$,\;\;\;$\vec{r}_{34}=10.0\hat{i}+0.0\hat{j}+0.0\hat{k}$.

{\tiny 1D-M14:}

$\hat{n}_{12}=0.59\hat{i}-0.79\hat{j}-0.17\hat{k}$,\;\;\;$\hat{n}_{13}=0.55\hat{i}+0.02\hat{j}+0.84\hat{k}$,\;\;\;$\hat{n}_{24}=0.58\hat{i}-0.57\hat{j}-0.59\hat{k}$,\;\;\;$\vec{r}_{12}=0.0\hat{i}+0.0\hat{j}+10.0\hat{k}$,\;\;\;$\vec{r}_{13}=0.0\hat{i}+0.0\hat{j}+10.0\hat{k}$,\;\;\;$\vec{r}_{24}=10.0\hat{i}+0.0\hat{j}+0.0\hat{k}$,\;\;\;$\vec{r}_{34}=10.0\hat{i}+10.0\hat{j}+10.0\hat{k}$.

{\tiny 1D-M15:}

$\hat{n}_{12}=0.0\hat{i}+0.71\hat{j}-0.71\hat{k}$,\;\;\;$\hat{n}_{13}=0.88\hat{i}-0.37\hat{j}-0.3\hat{k}$,\;\;\;$\hat{n}_{34}=-0.0\hat{i}+0.69\hat{j}-0.73\hat{k}$,\;\;\;$\vec{r}_{12}=0.0\hat{i}+10.0\hat{j}+0.0\hat{k}$,\;\;\;$\vec{r}_{13}=0.0\hat{i}+0.0\hat{j}+0.0\hat{k}$,\;\;\;$\vec{r}_{24}=10.0\hat{i}+10.0\hat{j}+10.0\hat{k}$,\;\;\;$\vec{r}_{34}=10.0\hat{i}+0.0\hat{j}+10.0\hat{k}$.

{\tiny 1D-M16:}

$\hat{n}_{12}=0.0\hat{i}+0.0\hat{j}-1.0\hat{k}$,\;\;\;$\hat{n}_{24}=-0.58\hat{i}+0.58\hat{j}+0.58\hat{k}$,\;\;\;$\hat{n}_{34}=-0.0\hat{i}+0.0\hat{j}-1.0\hat{k}$,\;\;\;$\vec{r}_{12}=10.0\hat{i}+10.0\hat{j}+0.0\hat{k}$,\;\;\;$\vec{r}_{13}=0.0\hat{i}+0.0\hat{j}+0.0\hat{k}$,\;\;\;$\vec{r}_{24}=0.0\hat{i}+10.0\hat{j}+10.0\hat{k}$,\;\;\;$\vec{r}_{34}=10.0\hat{i}+10.0\hat{j}+0.45\hat{k}$.

{\tiny 1D-M17:}

$\hat{n}_{12}=0.47\hat{i}-0.44\hat{j}+0.77\hat{k}$,\;\;\;$\hat{n}_{24}=0.11\hat{i}+0.39\hat{j}+0.92\hat{k}$,\;\;\;$\hat{n}_{34}=0.69\hat{i}-0.19\hat{j}-0.69\hat{k}$,\;\;\;$\vec{r}_{12}=0.0\hat{i}+10.0\hat{j}+0.0\hat{k}$,\;\;\;$\vec{r}_{13}=0.0\hat{i}+10.0\hat{j}+10.0\hat{k}$,\;\;\;$\vec{r}_{24}=10.0\hat{i}+10.0\hat{j}+0.0\hat{k}$,\;\;\;$\vec{r}_{34}=0.0\hat{i}+0.0\hat{j}+0.0\hat{k}$.

{\tiny 1D-M18:}

$\hat{n}_{12}=0.08\hat{i}-0.58\hat{j}+0.81\hat{k}$,\;\;\;$\hat{n}_{24}=0.45\hat{i}-0.53\hat{j}+0.72\hat{k}$,\;\;\;$\hat{n}_{34}=0.39\hat{i}-0.82\hat{j}-0.42\hat{k}$,\;\;\;$\vec{r}_{12}=10.0\hat{i}+10.0\hat{j}+10.0\hat{k}$,\;\;\;$\vec{r}_{13}=0.0\hat{i}+0.0\hat{j}+10.0\hat{k}$,\;\;\;$\vec{r}_{24}=0.0\hat{i}+10.0\hat{j}+0.0\hat{k}$,\;\;\;$\vec{r}_{34}=10.0\hat{i}+10.0\hat{j}+0.0\hat{k}$.
