# Supplementary material for: Dimensional synthesis of spatial manipulators for velocity and force transmission for operation around a specified task point
Source: arXiv:2210.04446 source file (2022-10-10)
Supplement: Supplementary file 29 [file classappendix2.tex]

\subsection{Class 2} \label{appendix_five_2_1}
{\tiny 1D-M19:}

$\hat{n}_{13}=0.58\hat{i}+0.58\hat{j}+0.58\hat{k}$,\;\;\;$\hat{n}_{14}=-0.63\hat{i}-0.77\hat{j}-0.08\hat{k}$,\;\;\;$\vec{r}_{13}=10.0\hat{i}+10.0\hat{j}+0.0\hat{k}$,\;\;\;$\vec{r}_{14}=0.0\hat{i}+10.0\hat{j}+0.0\hat{k}$,\;\;\;$\vec{r}_{23}=0.0\hat{i}+10.0\hat{j}+10.0\hat{k}$,\;\;\;$\vec{r}_{24}=10.0\hat{i}+0.0\hat{j}+10.0\hat{k}$.

{\tiny 1D-M20:}

$\hat{n}_{14}=-0.62\hat{i}+0.73\hat{j}-0.29\hat{k}$,\;\;\;$\hat{n}_{24}=0.59\hat{i}-0.56\hat{j}+0.58\hat{k}$,\;\;\;$\vec{r}_{13}=4.05\hat{i}+6.66\hat{j}+3.38\hat{k}$,\;\;\;$\vec{r}_{14}=10.0\hat{i}+10.0\hat{j}+10.0\hat{k}$,\;\;\;$\vec{r}_{23}=4.38\hat{i}+5.09\hat{j}+3.57\hat{k}$,\;\;\;$\vec{r}_{24}=6.45\hat{i}+6.22\hat{j}+5.3\hat{k}$.

{\tiny 1D-M21:}

$\hat{n}_{12}=0.78\hat{i}-0.25\hat{j}-0.58\hat{k}$,\;\;\;$\hat{n}_{24}=-0.0\hat{i}+0.71\hat{j}-0.71\hat{k}$,\;\;\;$\vec{r}_{12}=10.0\hat{i}+10.0\hat{j}+10.0\hat{k}$,\;\;\;$\vec{r}_{13}=10.0\hat{i}+10.0\hat{j}+10.0\hat{k}$,\;\;\;$\vec{r}_{24}=10.0\hat{i}+0.0\hat{j}+10.0\hat{k}$,\;\;\;$\vec{r}_{34}=0.0\hat{i}+0.0\hat{j}+0.0\hat{k}$.
