# Supplementary material for: Dimensional synthesis of spatial manipulators for velocity and force transmission for operation around a specified task point
Source: arXiv:2210.04446 source file (2022-10-10)
Supplement: Supplementary file 30 [file classappendix3.tex]

\subsection{Class 3} \label{appendix_five_2_1}
{\tiny 1D-M22:}

$\hat{n}_{13}=0.58\hat{i}+0.58\hat{j}+0.58\hat{k}$,\;\;\;$\hat{n}_{14}=0.0\hat{i}+1.0\hat{j}-0.0\hat{k}$,\;\;\;$\hat{n}_{23}=0.0\hat{i}+0.0\hat{j}+1.0\hat{k}$,\;\;\;$\vec{r}_{13}=10.0\hat{i}+10.0\hat{j}+0.0\hat{k}$,\;\;\;$\vec{r}_{23}=0.0\hat{i}+10.0\hat{j}+5.3\hat{k}$,\;\;\;$\vec{r}_{24}=10.0\hat{i}+0.0\hat{j}+10.0\hat{k}$.

{\tiny 1D-M23:}

$\hat{n}_{13}=0.77\hat{i}+0.0\hat{j}-0.64\hat{k}$,\;\;\;$\hat{n}_{14}=0.0\hat{i}+0.0\hat{j}-1.0\hat{k}$,\;\;\;$\hat{n}_{24}=-0.0\hat{i}+0.92\hat{j}-0.38\hat{k}$,\;\;\;$\vec{r}_{13}=10.0\hat{i}+0.0\hat{j}+0.0\hat{k}$,\;\;\;$\vec{r}_{23}=0.0\hat{i}+0.0\hat{j}+0.0\hat{k}$,\;\;\;$\vec{r}_{24}=10.0\hat{i}+10.0\hat{j}+10.0\hat{k}$.

{\tiny 1D-M24:}

$\hat{n}_{13}=0.0\hat{i}+0.71\hat{j}-0.71\hat{k}$,\;\;\;$\hat{n}_{14}=0.82\hat{i}-0.41\hat{j}-0.41\hat{k}$,\;\;\;$\hat{n}_{23}=-0.58\hat{i}-0.58\hat{j}-0.58\hat{k}$,\;\;\;$\vec{r}_{13}=10.0\hat{i}+10.0\hat{j}+10.0\hat{k}$,\;\;\;$\vec{r}_{14}=10.0\hat{i}+10.0\hat{j}+10.0\hat{k}$,\;\;\;$\vec{r}_{24}=0.0\hat{i}+0.0\hat{j}+0.0\hat{k}$.

{\tiny 1D-M25:}

$\hat{n}_{13}=0.16\hat{i}+0.61\hat{j}-0.77\hat{k}$,\;\;\;$\hat{n}_{14}=-0.8\hat{i}+0.54\hat{j}+0.26\hat{k}$,\;\;\;$\hat{n}_{24}=0.58\hat{i}+0.58\hat{j}+0.58\hat{k}$,\;\;\;$\vec{r}_{13}=0.0\hat{i}+0.0\hat{j}+0.0\hat{k}$,\;\;\;$\vec{r}_{14}=0.0\hat{i}+0.0\hat{j}+0.0\hat{k}$,\;\;\;$\vec{r}_{23}=10.0\hat{i}+10.0\hat{j}+10.0\hat{k}$.

{\tiny 1D-M26:}

$\hat{n}_{13}=-0.0\hat{i}+0.56\hat{j}+0.83\hat{k}$,\;\;\;$\hat{n}_{23}=-0.58\hat{i}+0.56\hat{j}-0.59\hat{k}$,\;\;\;$\hat{n}_{24}=0.81\hat{i}+0.46\hat{j}-0.36\hat{k}$,\;\;\;$\vec{r}_{13}=0.0\hat{i}+0.0\hat{j}+10.0\hat{k}$,\;\;\;$\vec{r}_{14}=10.0\hat{i}+0.0\hat{j}+0.0\hat{k}$,\;\;\;$\vec{r}_{24}=0.0\hat{i}+10.0\hat{j}+10.0\hat{k}$.

{\tiny 1D-M27:}

$\hat{n}_{13}=0.0\hat{i}-0.0\hat{j}+1.0\hat{k}$,\;\;\;$\hat{n}_{23}=-0.17\hat{i}-0.6\hat{j}+0.78\hat{k}$,\;\;\;$\hat{n}_{24}=-0.58\hat{i}-0.58\hat{j}-0.58\hat{k}$,\;\;\;$\vec{r}_{13}=10.0\hat{i}+10.0\hat{j}+2.83\hat{k}$,\;\;\;$\vec{r}_{14}=10.0\hat{i}+10.0\hat{j}+10.0\hat{k}$,\;\;\;$\vec{r}_{23}=0.0\hat{i}+0.0\hat{j}+0.0\hat{k}$.

{\tiny 1D-M28:}

$\hat{n}_{13}=-0.08\hat{i}-0.95\hat{j}-0.3\hat{k}$,\;\;\;$\hat{n}_{14}=0.0\hat{i}+0.0\hat{j}+1.0\hat{k}$,\;\;\;$\hat{n}_{23}=-0.31\hat{i}-0.44\hat{j}+0.84\hat{k}$,\;\;\;$\vec{r}_{14}=10.0\hat{i}+0.0\hat{j}+7.16\hat{k}$,\;\;\;$\vec{r}_{23}=4.62\hat{i}+3.55\hat{j}+4.57\hat{k}$,\;\;\;$\vec{r}_{24}=5.36\hat{i}+4.87\hat{j}+4.55\hat{k}$.

{\tiny 1D-M29:}

$\hat{n}_{13}=0.94\hat{i}-0.34\hat{j}-0.08\hat{k}$,\;\;\;$\hat{n}_{14}=0.36\hat{i}+0.32\hat{j}+0.88\hat{k}$,\;\;\;$\hat{n}_{24}=0.14\hat{i}-0.99\hat{j}-0.03\hat{k}$,\;\;\;$\vec{r}_{14}=10.0\hat{i}+10.0\hat{j}+0.0\hat{k}$,\;\;\;$\vec{r}_{23}=6.04\hat{i}+4.16\hat{j}+5.3\hat{k}$,\;\;\;$\vec{r}_{24}=3.09\hat{i}+4.06\hat{j}+2.83\hat{k}$.

{\tiny 1D-M30:}

$\hat{n}_{13}=0.0\hat{i}+0.53\hat{j}-0.85\hat{k}$,\;\;\;$\hat{n}_{14}=0.04\hat{i}+0.85\hat{j}-0.53\hat{k}$,\;\;\;$\hat{n}_{23}=-0.59\hat{i}+0.2\hat{j}+0.79\hat{k}$,\;\;\;$\vec{r}_{14}=0.0\hat{i}+0.0\hat{j}+0.0\hat{k}$,\;\;\;$\vec{r}_{23}=10.0\hat{i}+0.0\hat{j}+0.0\hat{k}$,\;\;\;$\vec{r}_{24}=0.0\hat{i}+10.0\hat{j}+10.0\hat{k}$.

{\tiny 1D-M31:}

$\hat{n}_{13}=0.58\hat{i}+0.58\hat{j}-0.58\hat{k}$,\;\;\;$\hat{n}_{14}=0.61\hat{i}+0.72\hat{j}+0.33\hat{k}$,\;\;\;$\hat{n}_{24}=-0.74\hat{i}+0.66\hat{j}-0.08\hat{k}$,\;\;\;$\vec{r}_{14}=0.0\hat{i}+0.0\hat{j}+10.0\hat{k}$,\;\;\;$\vec{r}_{23}=10.0\hat{i}+10.0\hat{j}+0.0\hat{k}$,\;\;\;$\vec{r}_{24}=0.0\hat{i}+0.0\hat{j}+10.0\hat{k}$.

{\tiny 1D-M32:}

$\hat{n}_{13}=0.49\hat{i}-0.6\hat{j}-0.63\hat{k}$,\;\;\;$\hat{n}_{23}=0.71\hat{i}+0.25\hat{j}-0.65\hat{k}$,\;\;\;$\hat{n}_{24}=-0.85\hat{i}-0.47\hat{j}-0.22\hat{k}$,\;\;\;$\vec{r}_{14}=0.0\hat{i}+10.0\hat{j}+10.0\hat{k}$,\;\;\;$\vec{r}_{23}=0.0\hat{i}+0.0\hat{j}+0.0\hat{k}$,\;\;\;$\vec{r}_{24}=10.0\hat{i}+0.0\hat{j}+10.0\hat{k}$.

{\tiny 1D-M33:}

$\hat{n}_{13}=-0.66\hat{i}-0.58\hat{j}+0.49\hat{k}$,\;\;\;$\hat{n}_{23}=0.25\hat{i}+0.44\hat{j}+0.86\hat{k}$,\;\;\;$\hat{n}_{24}=-0.63\hat{i}+0.22\hat{j}+0.75\hat{k}$,\;\;\;$\vec{r}_{14}=0.0\hat{i}+10.0\hat{j}+10.0\hat{k}$,\;\;\;$\vec{r}_{23}=10.0\hat{i}+10.0\hat{j}+0.0\hat{k}$,\;\;\;$\vec{r}_{24}=0.0\hat{i}+0.0\hat{j}+0.0\hat{k}$.

{\tiny 1D-M34:}

$\hat{n}_{13}=-0.74\hat{i}-0.6\hat{j}-0.29\hat{k}$,\;\;\;$\hat{n}_{14}=-0.62\hat{i}-0.35\hat{j}-0.7\hat{k}$,\;\;\;$\hat{n}_{23}=0.27\hat{i}-0.91\hat{j}-0.32\hat{k}$,\;\;\;$\vec{r}_{13}=1.42\hat{i}+3.47\hat{j}+4.31\hat{k}$,\;\;\;$\vec{r}_{14}=0.0\hat{i}+0.0\hat{j}+10.0\hat{k}$,\;\;\;$\vec{r}_{24}=4.36\hat{i}+8.23\hat{j}+4.01\hat{k}$.

{\tiny 1D-M35:}

$\hat{n}_{13}=-0.42\hat{i}-0.91\hat{j}-0.01\hat{k}$,\;\;\;$\hat{n}_{14}=0.43\hat{i}+0.25\hat{j}+0.87\hat{k}$,\;\;\;$\hat{n}_{24}=-0.22\hat{i}-0.98\hat{j}-0.01\hat{k}$,\;\;\;$\vec{r}_{13}=4.89\hat{i}+4.28\hat{j}+3.84\hat{k}$,\;\;\;$\vec{r}_{14}=10.0\hat{i}+10.0\hat{j}+0.0\hat{k}$,\;\;\;$\vec{r}_{23}=4.55\hat{i}+6.12\hat{j}+6.81\hat{k}$.

{\tiny 1D-M36:}

$\hat{n}_{13}=-0.44\hat{i}-0.72\hat{j}-0.53\hat{k}$,\;\;\;$\hat{n}_{14}=0.83\hat{i}+0.56\hat{j}+0.02\hat{k}$,\;\;\;$\hat{n}_{23}=0.53\hat{i}+0.17\hat{j}+0.83\hat{k}$,\;\;\;$\vec{r}_{13}=4.07\hat{i}+7.49\hat{j}+8.26\hat{k}$,\;\;\;$\vec{r}_{23}=7.9\hat{i}+3.19\hat{j}+5.34\hat{k}$,\;\;\;$\vec{r}_{24}=0.9\hat{i}+1.12\hat{j}+1.36\hat{k}$.

{\tiny 1D-M37:}

$\hat{n}_{13}=0.01\hat{i}-0.41\hat{j}-0.91\hat{k}$,\;\;\;$\hat{n}_{14}=0.75\hat{i}+0.56\hat{j}-0.35\hat{k}$,\;\;\;$\hat{n}_{24}=0.01\hat{i}+0.03\hat{j}-1.0\hat{k}$,\;\;\;$\vec{r}_{13}=8.51\hat{i}+5.61\hat{j}+9.3\hat{k}$,\;\;\;$\vec{r}_{23}=6.97\hat{i}+5.83\hat{j}+8.15\hat{k}$,\;\;\;$\vec{r}_{24}=8.79\hat{i}+9.89\hat{j}+0.01\hat{k}$.

{\tiny 1D-M38:}

$\hat{n}_{13}=0.61\hat{i}-0.54\hat{j}-0.58\hat{k}$,\;\;\;$\hat{n}_{23}=0.04\hat{i}-0.37\hat{j}-0.93\hat{k}$,\;\;\;$\hat{n}_{24}=0.2\hat{i}-0.61\hat{j}+0.77\hat{k}$,\;\;\;$\vec{r}_{13}=0.0\hat{i}+10.0\hat{j}+10.0\hat{k}$,\;\;\;$\vec{r}_{14}=10.0\hat{i}+10.0\hat{j}+0.0\hat{k}$,\;\;\;$\vec{r}_{23}=10.0\hat{i}+0.0\hat{j}+0.0\hat{k}$.

{\tiny 1D-M39:}

$\hat{n}_{13}=-0.95\hat{i}-0.16\hat{j}-0.27\hat{k}$,\;\;\;$\hat{n}_{23}=0.0\hat{i}+0.7\hat{j}+0.72\hat{k}$,\;\;\;$\hat{n}_{24}=0.0\hat{i}+0.9\hat{j}-0.45\hat{k}$,\;\;\;$\vec{r}_{13}=10.0\hat{i}+0.0\hat{j}+10.0\hat{k}$,\;\;\;$\vec{r}_{14}=0.0\hat{i}+10.0\hat{j}+0.0\hat{k}$,\;\;\;$\vec{r}_{24}=10.0\hat{i}+10.0\hat{j}+10.0\hat{k}$.

{\tiny 1D-M40:}

$\hat{n}_{14}=0.16\hat{i}+0.79\hat{j}-0.6\hat{k}$,\;\;\;$\hat{n}_{23}=-0.6\hat{i}-0.8\hat{j}-0.08\hat{k}$,\;\;\;$\hat{n}_{24}=0.64\hat{i}-0.67\hat{j}-0.37\hat{k}$,\;\;\;$\vec{r}_{13}=1.1\hat{i}+4.9\hat{j}+2.13\hat{k}$,\;\;\;$\vec{r}_{14}=0.0\hat{i}+0.0\hat{j}+0.0\hat{k}$,\;\;\;$\vec{r}_{24}=2.1\hat{i}+1.07\hat{j}+6.29\hat{k}$.

{\tiny 1D-M41:}

$\hat{n}_{14}=-0.38\hat{i}+0.38\hat{j}+0.84\hat{k}$,\;\;\;$\hat{n}_{23}=-0.1\hat{i}-0.91\hat{j}+0.41\hat{k}$,\;\;\;$\hat{n}_{24}=0.15\hat{i}-0.92\hat{j}-0.37\hat{k}$,\;\;\;$\vec{r}_{13}=2.65\hat{i}+4.93\hat{j}+7.29\hat{k}$,\;\;\;$\vec{r}_{14}=10.0\hat{i}+0.0\hat{j}+0.0\hat{k}$,\;\;\;$\vec{r}_{23}=5.5\hat{i}+6.06\hat{j}+4.36\hat{k}$.

{\tiny 1D-M42:}

$\hat{n}_{14}=0.03\hat{i}+0.04\hat{j}-1.0\hat{k}$,\;\;\;$\hat{n}_{23}=0.33\hat{i}+0.27\hat{j}-0.9\hat{k}$,\;\;\;$\hat{n}_{24}=0.54\hat{i}+0.31\hat{j}-0.78\hat{k}$,\;\;\;$\vec{r}_{13}=6.21\hat{i}+5.74\hat{j}+0.52\hat{k}$,\;\;\;$\vec{r}_{23}=9.31\hat{i}+7.29\hat{j}+7.38\hat{k}$,\;\;\;$\vec{r}_{24}=0.63\hat{i}+8.6\hat{j}+9.34\hat{k}$.

{\tiny 1D-M43:}

$\hat{n}_{14}=-0.04\hat{i}-0.47\hat{j}-0.88\hat{k}$,\;\;\;$\hat{n}_{23}=0.88\hat{i}+0.43\hat{j}-0.18\hat{k}$,\;\;\;$\hat{n}_{24}=0.26\hat{i}-0.36\hat{j}-0.9\hat{k}$,\;\;\;$\vec{r}_{13}=1.34\hat{i}+0.31\hat{j}+9.39\hat{k}$,\;\;\;$\vec{r}_{23}=3.01\hat{i}+2.96\hat{j}+3.33\hat{k}$,\;\;\;$\vec{r}_{24}=4.67\hat{i}+6.48\hat{j}+0.25\hat{k}$.

{\tiny 1D-M44:}

$\hat{n}_{14}=-0.44\hat{i}-0.37\hat{j}+0.82\hat{k}$,\;\;\;$\hat{n}_{23}=0.69\hat{i}-0.73\hat{j}+0.04\hat{k}$,\;\;\;$\hat{n}_{24}=0.58\hat{i}+0.58\hat{j}+0.58\hat{k}$,\;\;\;$\vec{r}_{13}=10.0\hat{i}+10.0\hat{j}+10.0\hat{k}$,\;\;\;$\vec{r}_{14}=0.0\hat{i}+0.0\hat{j}+0.0\hat{k}$,\;\;\;$\vec{r}_{23}=0.0\hat{i}+0.0\hat{j}+0.0\hat{k}$.

{\tiny 1D-M45:}

$\hat{n}_{14}=-0.8\hat{i}-0.26\hat{j}-0.54\hat{k}$,\;\;\;$\hat{n}_{23}=0.58\hat{i}-0.58\hat{j}-0.58\hat{k}$,\;\;\;$\hat{n}_{24}=0.17\hat{i}+0.78\hat{j}-0.61\hat{k}$,\;\;\;$\vec{r}_{13}=0.0\hat{i}+10.0\hat{j}+0.0\hat{k}$,\;\;\;$\vec{r}_{14}=10.0\hat{i}+0.0\hat{j}+10.0\hat{k}$,\;\;\;$\vec{r}_{24}=10.0\hat{i}+0.0\hat{j}+10.0\hat{k}$.

{\tiny 1D-M46:}

$\hat{n}_{12}=-0.15\hat{i}+0.71\hat{j}-0.68\hat{k}$,\;\;\;$\hat{n}_{13}=-0.42\hat{i}-0.63\hat{j}-0.66\hat{k}$,\;\;\;$\hat{n}_{24}=-0.75\hat{i}+0.29\hat{j}+0.59\hat{k}$,\;\;\;$\vec{r}_{12}=0.0\hat{i}+10.0\hat{j}+0.0\hat{k}$,\;\;\;$\vec{r}_{24}=0.0\hat{i}+0.0\hat{j}+0.0\hat{k}$,\;\;\;$\vec{r}_{34}=10.0\hat{i}+10.0\hat{j}+10.0\hat{k}$.

{\tiny 1D-M47:}

$\hat{n}_{12}=-0.47\hat{i}+0.81\hat{j}-0.34\hat{k}$,\;\;\;$\hat{n}_{13}=-0.58\hat{i}-0.58\hat{j}-0.58\hat{k}$,\;\;\;$\hat{n}_{34}=0.67\hat{i}+0.08\hat{j}-0.74\hat{k}$,\;\;\;$\vec{r}_{12}=10.0\hat{i}+10.0\hat{j}+10.0\hat{k}$,\;\;\;$\vec{r}_{24}=0.0\hat{i}+0.0\hat{j}+0.0\hat{k}$,\;\;\;$\vec{r}_{34}=10.0\hat{i}+10.0\hat{j}+10.0\hat{k}$.

{\tiny 1D-M48:}

$\hat{n}_{12}=-0.78\hat{i}+0.61\hat{j}-0.14\hat{k}$,\;\;\;$\hat{n}_{13}=-0.0\hat{i}+0.0\hat{j}+1.0\hat{k}$,\;\;\;$\hat{n}_{24}=-0.71\hat{i}-0.61\hat{j}+0.34\hat{k}$,\;\;\;$\vec{r}_{12}=10.0\hat{i}+10.0\hat{j}+0.0\hat{k}$,\;\;\;$\vec{r}_{13}=0.0\hat{i}+0.0\hat{j}+1.46\hat{k}$,\;\;\;$\vec{r}_{34}=10.0\hat{i}+10.0\hat{j}+10.0\hat{k}$.

{\tiny 1D-M49:}

$\hat{n}_{12}=-0.0\hat{i}+0.94\hat{j}-0.34\hat{k}$,\;\;\;$\hat{n}_{13}=0.0\hat{i}+0.0\hat{j}-1.0\hat{k}$,\;\;\;$\hat{n}_{34}=-0.73\hat{i}+0.69\hat{j}-0.0\hat{k}$,\;\;\;$\vec{r}_{12}=10.0\hat{i}+0.0\hat{j}+10.0\hat{k}$,\;\;\;$\vec{r}_{13}=10.0\hat{i}+0.0\hat{j}+4.77\hat{k}$,\;\;\;$\vec{r}_{24}=0.0\hat{i}+10.0\hat{j}+0.0\hat{k}$.

{\tiny 1D-M50:}

$\hat{n}_{12}=0.82\hat{i}-0.44\hat{j}+0.36\hat{k}$,\;\;\;$\hat{n}_{24}=-0.58\hat{i}-0.6\hat{j}+0.55\hat{k}$,\;\;\;$\hat{n}_{34}=0.0\hat{i}+0.57\hat{j}+0.82\hat{k}$,\;\;\;$\vec{r}_{12}=10.0\hat{i}+10.0\hat{j}+0.0\hat{k}$,\;\;\;$\vec{r}_{13}=0.0\hat{i}+0.0\hat{j}+10.0\hat{k}$,\;\;\;$\vec{r}_{34}=10.0\hat{i}+10.0\hat{j}+0.0\hat{k}$.

{\tiny 1D-M51:}

$\hat{n}_{12}=-0.0\hat{i}+0.62\hat{j}-0.78\hat{k}$,\;\;\;$\hat{n}_{24}=-0.79\hat{i}+0.53\hat{j}+0.31\hat{k}$,\;\;\;$\hat{n}_{34}=0.77\hat{i}+0.44\hat{j}+0.47\hat{k}$,\;\;\;$\vec{r}_{12}=10.0\hat{i}+0.0\hat{j}+10.0\hat{k}$,\;\;\;$\vec{r}_{13}=10.0\hat{i}+10.0\hat{j}+10.0\hat{k}$,\;\;\;$\vec{r}_{24}=0.0\hat{i}+0.0\hat{j}+0.0\hat{k}$.

{\tiny 1D-M52:}

$\hat{n}_{12}=0.69\hat{i}+0.51\hat{j}+0.52\hat{k}$,\;\;\;$\hat{n}_{13}=-0.91\hat{i}-0.28\hat{j}-0.3\hat{k}$,\;\;\;$\hat{n}_{24}=-0.0\hat{i}+0.69\hat{j}-0.72\hat{k}$,\;\;\;$\vec{r}_{13}=10.0\hat{i}+0.0\hat{j}+10.0\hat{k}$,\;\;\;$\vec{r}_{24}=10.0\hat{i}+10.0\hat{j}+10.0\hat{k}$,\;\;\;$\vec{r}_{34}=0.0\hat{i}+0.0\hat{j}+0.0\hat{k}$.

{\tiny 1D-M53:}

$\hat{n}_{12}=0.61\hat{i}-0.05\hat{j}+0.79\hat{k}$,\;\;\;$\hat{n}_{13}=-0.65\hat{i}-0.37\hat{j}-0.66\hat{k}$,\;\;\;$\hat{n}_{34}=-0.61\hat{i}+0.5\hat{j}+0.61\hat{k}$,\;\;\;$\vec{r}_{13}=10.0\hat{i}+10.0\hat{j}+0.0\hat{k}$,\;\;\;$\vec{r}_{24}=0.0\hat{i}+10.0\hat{j}+10.0\hat{k}$,\;\;\;$\vec{r}_{34}=0.0\hat{i}+0.0\hat{j}+0.0\hat{k}$.

{\tiny 1D-M54:}

$\hat{n}_{12}=-0.86\hat{i}+0.41\hat{j}-0.3\hat{k}$,\;\;\;$\hat{n}_{24}=-0.6\hat{i}-0.48\hat{j}+0.64\hat{k}$,\;\;\;$\hat{n}_{34}=-0.68\hat{i}+0.26\hat{j}-0.69\hat{k}$,\;\;\;$\vec{r}_{13}=10.0\hat{i}+10.0\hat{j}+10.0\hat{k}$,\;\;\;$\vec{r}_{24}=10.0\hat{i}+0.0\hat{j}+0.0\hat{k}$,\;\;\;$\vec{r}_{34}=0.0\hat{i}+10.0\hat{j}+0.0\hat{k}$.

{\tiny 1D-M55:}

$\hat{n}_{12}=-0.0\hat{i}+0.75\hat{j}+0.66\hat{k}$,\;\;\;$\hat{n}_{24}=-0.96\hat{i}+0.16\hat{j}+0.22\hat{k}$,\;\;\;$\hat{n}_{34}=-0.0\hat{i}+0.71\hat{j}-0.7\hat{k}$,\;\;\;$\vec{r}_{13}=0.0\hat{i}+10.0\hat{j}+0.0\hat{k}$,\;\;\;$\vec{r}_{24}=10.0\hat{i}+10.0\hat{j}+10.0\hat{k}$,\;\;\;$\vec{r}_{34}=10.0\hat{i}+0.0\hat{j}+10.0\hat{k}$.

{\tiny 1D-M56:}

$\hat{n}_{12}=-0.74\hat{i}+0.08\hat{j}+0.66\hat{k}$,\;\;\;$\hat{n}_{24}=0.77\hat{i}-0.64\hat{j}-0.02\hat{k}$,\;\;\;$\hat{n}_{34}=0.58\hat{i}+0.58\hat{j}+0.58\hat{k}$,\;\;\;$\vec{r}_{12}=0.0\hat{i}+0.0\hat{j}+0.0\hat{k}$,\;\;\;$\vec{r}_{13}=10.0\hat{i}+10.0\hat{j}+10.0\hat{k}$,\;\;\;$\vec{r}_{24}=10.0\hat{i}+10.0\hat{j}+10.0\hat{k}$.

{\tiny 1D-M57:}

$\hat{n}_{12}=0.0\hat{i}+0.79\hat{j}-0.61\hat{k}$,\;\;\;$\hat{n}_{24}=0.6\hat{i}+0.48\hat{j}+0.63\hat{k}$,\;\;\;$\hat{n}_{34}=0.0\hat{i}+0.57\hat{j}+0.82\hat{k}$,\;\;\;$\vec{r}_{12}=10.0\hat{i}+10.0\hat{j}+10.0\hat{k}$,\;\;\;$\vec{r}_{13}=0.0\hat{i}+0.0\hat{j}+0.0\hat{k}$,\;\;\;$\vec{r}_{34}=10.0\hat{i}+10.0\hat{j}+0.0\hat{k}$.
