# Supplementary material for: Dimensional synthesis of spatial manipulators for velocity and force transmission for operation around a specified task point
Source: arXiv:2210.04446 source file (2022-10-10)
Supplement: Supplementary file 31 [file classappendix4.tex]

\subsection{Class 4} \label{appendix_five_2_1}
{\tiny 1D-M58:}

$\hat{n}_{13}=0.71\hat{i}-0.71\hat{j}+0.0\hat{k}$,\;\;\;$\hat{n}_{14}=0.58\hat{i}+0.58\hat{j}-0.58\hat{k}$,\;\;\;$\vec{r}_{13}=0.0\hat{i}+0.0\hat{j}+0.0\hat{k}$,\;\;\;$\vec{r}_{23}=10.0\hat{i}+10.0\hat{j}+0.0\hat{k}$,\;\;\;$\vec{r}_{24}=0.0\hat{i}+0.0\hat{j}+10.0\hat{k}$.

{\tiny 1D-M59:}

$\hat{n}_{13}=0.57\hat{i}-0.61\hat{j}-0.55\hat{k}$,\;\;\;$\hat{n}_{14}=-0.63\hat{i}-0.66\hat{j}-0.41\hat{k}$,\;\;\;$\vec{r}_{14}=10.0\hat{i}+0.0\hat{j}+0.0\hat{k}$,\;\;\;$\vec{r}_{23}=1.65\hat{i}+1.14\hat{j}+3.04\hat{k}$,\;\;\;$\vec{r}_{24}=3.29\hat{i}+6.44\hat{j}+8.8\hat{k}$.

{\tiny 1D-M60:}

$\hat{n}_{14}=0.62\hat{i}-0.06\hat{j}+0.78\hat{k}$,\;\;\;$\hat{n}_{24}=-0.71\hat{i}-0.53\hat{j}+0.46\hat{k}$,\;\;\;$\vec{r}_{13}=7.06\hat{i}+6.93\hat{j}+6.95\hat{k}$,\;\;\;$\vec{r}_{14}=0.0\hat{i}+10.0\hat{j}+0.0\hat{k}$,\;\;\;$\vec{r}_{23}=2.75\hat{i}+2.12\hat{j}+7.47\hat{k}$.

{\tiny 1D-M61:}

$\hat{n}_{14}=-0.32\hat{i}-0.19\hat{j}+0.93\hat{k}$,\;\;\;$\hat{n}_{24}=-0.61\hat{i}+0.79\hat{j}-0.08\hat{k}$,\;\;\;$\vec{r}_{13}=5.17\hat{i}+7.03\hat{j}+1.54\hat{k}$,\;\;\;$\vec{r}_{23}=9.53\hat{i}+5.41\hat{j}+6.8\hat{k}$,\;\;\;$\vec{r}_{24}=0.37\hat{i}+8.09\hat{j}+7.49\hat{k}$.

{\tiny 1D-M62:}

$\hat{n}_{12}=0.28\hat{i}+0.64\hat{j}+0.71\hat{k}$,\;\;\;$\hat{n}_{24}=0.0\hat{i}+0.52\hat{j}+0.85\hat{k}$,\;\;\;$\vec{r}_{12}=0.0\hat{i}+0.0\hat{j}+10.0\hat{k}$,\;\;\;$\vec{r}_{13}=10.0\hat{i}+0.0\hat{j}+10.0\hat{k}$,\;\;\;$\vec{r}_{34}=0.0\hat{i}+10.0\hat{j}+0.0\hat{k}$.

{\tiny 1D-M63:}

$\hat{n}_{12}=-0.46\hat{i}-0.43\hat{j}+0.78\hat{k}$,\;\;\;$\hat{n}_{24}=-0.07\hat{i}-0.66\hat{j}-0.75\hat{k}$,\;\;\;$\vec{r}_{13}=0.0\hat{i}+10.0\hat{j}+10.0\hat{k}$,\;\;\;$\vec{r}_{24}=10.0\hat{i}+10.0\hat{j}+0.0\hat{k}$,\;\;\;$\vec{r}_{34}=10.0\hat{i}+0.0\hat{j}+0.0\hat{k}$.
