# Supplementary material for: Dimensional synthesis of spatial manipulators for velocity and force transmission for operation around a specified task point
Source: arXiv:2210.04446 source file (2022-10-10)
Supplement: Supplementary file 32 [file classappendix5.tex]

\subsection{Class 5} \label{appendix_five_2_1}
{\tiny 1D-M64:}

$\hat{n}_{13}=-0.23\hat{i}+0.23\hat{j}-0.95\hat{k}$,\;\;\;$\hat{n}_{14}=-0.71\hat{i}-0.71\hat{j}+0.0\hat{k}$,\;\;\;$\hat{n}_{23}=0.59\hat{i}-0.59\hat{j}+0.55\hat{k}$,\;\;\;$\hat{n}_{24}=0.43\hat{i}-0.43\hat{j}-0.8\hat{k}$,\;\;\;$\vec{r}_{13}=10.0\hat{i}+0.0\hat{j}+10.0\hat{k}$,\;\;\;$\vec{r}_{14}=5.01\hat{i}+5.01\hat{j}+5.01\hat{k}$,\;\;\;$\vec{r}_{23}=0.0\hat{i}+10.0\hat{j}+0.0\hat{k}$,\;\;\;$\vec{r}_{24}=0.0\hat{i}+10.0\hat{j}+10.0\hat{k}$.

{\tiny 1D-M65:}

$\hat{n}_{13}=0.31\hat{i}-0.63\hat{j}+0.71\hat{k}$,\;\;\;$\hat{n}_{14}=-0.62\hat{i}-0.02\hat{j}-0.78\hat{k}$,\;\;\;$\hat{n}_{23}=-0.89\hat{i}-0.46\hat{j}-0.01\hat{k}$,\;\;\;$\hat{n}_{24}=0.33\hat{i}-0.63\hat{j}-0.7\hat{k}$,\;\;\;$\vec{r}_{13}=5.12\hat{i}+4.88\hat{j}+5.02\hat{k}$,\;\;\;$\vec{r}_{14}=10.0\hat{i}+10.0\hat{j}+0.0\hat{k}$,\;\;\;$\vec{r}_{23}=4.82\hat{i}+4.82\hat{j}+4.97\hat{k}$,\;\;\;$\vec{r}_{24}=4.86\hat{i}+5.18\hat{j}+4.92\hat{k}$.

{\tiny 1D-M66:}

$\hat{n}_{13}=0.61\hat{i}-0.61\hat{j}+0.51\hat{k}$,\;\;\;$\hat{n}_{14}=-0.71\hat{i}-0.71\hat{j}-0.0\hat{k}$,\;\;\;$\hat{n}_{23}=-0.59\hat{i}+0.59\hat{j}+0.56\hat{k}$,\;\;\;$\hat{n}_{24}=0.31\hat{i}-0.31\hat{j}-0.9\hat{k}$,\;\;\;$\vec{r}_{13}=10.0\hat{i}+0.0\hat{j}+10.0\hat{k}$,\;\;\;$\vec{r}_{14}=5.06\hat{i}+5.03\hat{j}+5.17\hat{k}$,\;\;\;$\vec{r}_{23}=10.0\hat{i}+0.0\hat{j}+0.0\hat{k}$,\;\;\;$\vec{r}_{24}=0.0\hat{i}+10.0\hat{j}+10.0\hat{k}$.

{\tiny 1D-M67:}

$\hat{n}_{13}=-0.58\hat{i}+0.8\hat{j}-0.16\hat{k}$,\;\;\;$\hat{n}_{14}=0.0\hat{i}-0.0\hat{j}+1.0\hat{k}$,\;\;\;$\hat{n}_{23}=-0.86\hat{i}-0.52\hat{j}+0.03\hat{k}$,\;\;\;$\hat{n}_{24}=-0.44\hat{i}-0.89\hat{j}-0.05\hat{k}$,\;\;\;$\vec{r}_{13}=10.0\hat{i}+10.0\hat{j}+0.0\hat{k}$,\;\;\;$\vec{r}_{14}=0.0\hat{i}+0.0\hat{j}+3.07\hat{k}$,\;\;\;$\vec{r}_{23}=0.0\hat{i}+10.0\hat{j}+10.0\hat{k}$,\;\;\;$\vec{r}_{24}=10.0\hat{i}+0.0\hat{j}+0.0\hat{k}$.

{\tiny 1D-M68:}

$\hat{n}_{12}=0.34\hat{i}-0.89\hat{j}+0.31\hat{k}$,\;\;\;$\hat{n}_{13}=0.56\hat{i}+0.34\hat{j}-0.76\hat{k}$,\;\;\;$\hat{n}_{24}=-0.0\hat{i}+0.82\hat{j}+0.57\hat{k}$,\;\;\;$\hat{n}_{34}=-0.85\hat{i}+0.27\hat{j}-0.44\hat{k}$,\;\;\;$\vec{r}_{12}=10.0\hat{i}+10.0\hat{j}+10.0\hat{k}$,\;\;\;$\vec{r}_{13}=0.0\hat{i}+10.0\hat{j}+10.0\hat{k}$,\;\;\;$\vec{r}_{24}=10.0\hat{i}+0.0\hat{j}+0.0\hat{k}$,\;\;\;$\vec{r}_{34}=10.0\hat{i}+10.0\hat{j}+0.0\hat{k}$.

{\tiny 1D-M69:}

$\hat{n}_{12}=-0.0\hat{i}+0.77\hat{j}+0.64\hat{k}$,\;\;\;$\hat{n}_{13}=0.55\hat{i}-0.44\hat{j}+0.71\hat{k}$,\;\;\;$\hat{n}_{24}=-0.79\hat{i}+0.61\hat{j}+0.1\hat{k}$,\;\;\;$\hat{n}_{34}=-0.82\hat{i}-0.32\hat{j}+0.48\hat{k}$,\;\;\;$\vec{r}_{12}=10.0\hat{i}+0.0\hat{j}+0.0\hat{k}$,\;\;\;$\vec{r}_{13}=10.0\hat{i}+10.0\hat{j}+0.0\hat{k}$,\;\;\;$\vec{r}_{24}=10.0\hat{i}+10.0\hat{j}+10.0\hat{k}$,\;\;\;$\vec{r}_{34}=10.0\hat{i}+0.0\hat{j}+0.0\hat{k}$.
