# Supplementary material for: Dimensional synthesis of spatial manipulators for velocity and force transmission for operation around a specified task point
Source: arXiv:2210.04446 source file (2022-10-10)
Supplement: Supplementary file 33 [file classappendix6.tex]

\subsection{Class 6} \label{appendix_five_2_1}
{\tiny 1D-M70:}

$\hat{n}_{13}=-0.58\hat{i}+0.58\hat{j}+0.58\hat{k}$,\;\;\;$\hat{n}_{14}=0.58\hat{i}-0.58\hat{j}-0.58\hat{k}$,\;\;\;$\hat{n}_{23}=-0.05\hat{i}+0.68\hat{j}-0.73\hat{k}$,\;\;\;$\vec{r}_{23}=10.0\hat{i}+0.0\hat{j}+10.0\hat{k}$,\;\;\;$\vec{r}_{24}=0.0\hat{i}+10.0\hat{j}+0.0\hat{k}$.

{\tiny 1D-M71:}

$\hat{n}_{13}=-0.58\hat{i}-0.58\hat{j}+0.58\hat{k}$,\;\;\;$\hat{n}_{14}=0.58\hat{i}+0.58\hat{j}-0.58\hat{k}$,\;\;\;$\hat{n}_{24}=-0.12\hat{i}+0.76\hat{j}+0.64\hat{k}$,\;\;\;$\vec{r}_{23}=10.0\hat{i}+10.0\hat{j}+0.0\hat{k}$,\;\;\;$\vec{r}_{24}=0.0\hat{i}+0.0\hat{j}+10.0\hat{k}$.

{\tiny 1D-M72:}

$\hat{n}_{13}=-0.21\hat{i}-0.79\hat{j}+0.58\hat{k}$,\;\;\;$\hat{n}_{14}=0.21\hat{i}+0.79\hat{j}-0.58\hat{k}$,\;\;\;$\hat{n}_{23}=-0.58\hat{i}+0.58\hat{j}+0.58\hat{k}$,\;\;\;$\vec{r}_{14}=0.0\hat{i}+10.0\hat{j}+0.0\hat{k}$,\;\;\;$\vec{r}_{24}=10.0\hat{i}+0.0\hat{j}+10.0\hat{k}$.

{\tiny 1D-M73:}

$\hat{n}_{13}=-0.3\hat{i}+0.81\hat{j}-0.51\hat{k}$,\;\;\;$\hat{n}_{14}=-0.3\hat{i}+0.81\hat{j}-0.51\hat{k}$,\;\;\;$\hat{n}_{24}=0.58\hat{i}+0.58\hat{j}+0.58\hat{k}$,\;\;\;$\vec{r}_{14}=0.0\hat{i}+0.0\hat{j}+0.0\hat{k}$,\;\;\;$\vec{r}_{23}=10.0\hat{i}+10.0\hat{j}+10.0\hat{k}$.

{\tiny 1D-M74:}

$\hat{n}_{13}=-0.62\hat{i}-0.77\hat{j}-0.15\hat{k}$,\;\;\;$\hat{n}_{23}=-0.58\hat{i}+0.58\hat{j}-0.58\hat{k}$,\;\;\;$\hat{n}_{24}=0.53\hat{i}-0.27\hat{j}-0.8\hat{k}$,\;\;\;$\vec{r}_{14}=10.0\hat{i}+0.0\hat{j}+0.0\hat{k}$,\;\;\;$\vec{r}_{24}=0.0\hat{i}+10.0\hat{j}+10.0\hat{k}$.

{\tiny 1D-M75:}

$\hat{n}_{13}=0.0\hat{i}-0.71\hat{j}+0.71\hat{k}$,\;\;\;$\hat{n}_{23}=-0.82\hat{i}+0.41\hat{j}+0.41\hat{k}$,\;\;\;$\hat{n}_{24}=0.58\hat{i}+0.58\hat{j}+0.58\hat{k}$,\;\;\;$\vec{r}_{14}=0.0\hat{i}+0.0\hat{j}+0.0\hat{k}$,\;\;\;$\vec{r}_{23}=10.0\hat{i}+10.0\hat{j}+10.0\hat{k}$.

{\tiny 1D-M76:}

$\hat{n}_{13}=-0.42\hat{i}-0.11\hat{j}-0.9\hat{k}$,\;\;\;$\hat{n}_{14}=-0.55\hat{i}-0.55\hat{j}+0.63\hat{k}$,\;\;\;$\hat{n}_{23}=-0.4\hat{i}-0.63\hat{j}-0.66\hat{k}$,\;\;\;$\vec{r}_{13}=6.6\hat{i}+0.48\hat{j}+3.49\hat{k}$,\;\;\;$\vec{r}_{24}=4.51\hat{i}+2.41\hat{j}+7.15\hat{k}$.

{\tiny 1D-M77:}

$\hat{n}_{13}=0.68\hat{i}+0.58\hat{j}+0.45\hat{k}$,\;\;\;$\hat{n}_{14}=-0.84\hat{i}+0.51\hat{j}+0.16\hat{k}$,\;\;\;$\hat{n}_{24}=0.09\hat{i}+0.07\hat{j}-0.99\hat{k}$,\;\;\;$\vec{r}_{13}=5.88\hat{i}+3.66\hat{j}+8.07\hat{k}$,\;\;\;$\vec{r}_{23}=5.04\hat{i}+4.9\hat{j}+8.77\hat{k}$.

{\tiny 1D-M78:}

$\hat{n}_{13}=-0.82\hat{i}+0.41\hat{j}+0.41\hat{k}$,\;\;\;$\hat{n}_{23}=0.0\hat{i}-0.71\hat{j}+0.71\hat{k}$,\;\;\;$\hat{n}_{24}=-0.58\hat{i}-0.58\hat{j}-0.58\hat{k}$,\;\;\;$\vec{r}_{13}=0.0\hat{i}+0.0\hat{j}+0.0\hat{k}$,\;\;\;$\vec{r}_{14}=10.0\hat{i}+10.0\hat{j}+10.0\hat{k}$.

{\tiny 1D-M79:}

$\hat{n}_{14}=-0.3\hat{i}-0.22\hat{j}+0.93\hat{k}$,\;\;\;$\hat{n}_{23}=0.35\hat{i}+0.04\hat{j}-0.93\hat{k}$,\;\;\;$\hat{n}_{24}=0.17\hat{i}-0.24\hat{j}+0.96\hat{k}$,\;\;\;$\vec{r}_{13}=1.22\hat{i}+2.68\hat{j}+2.58\hat{k}$,\;\;\;$\vec{r}_{24}=3.32\hat{i}+1.52\hat{j}+3.48\hat{k}$.

{\tiny 1D-M80:}

$\hat{n}_{14}=-0.07\hat{i}+0.16\hat{j}+0.99\hat{k}$,\;\;\;$\hat{n}_{23}=0.48\hat{i}-0.66\hat{j}+0.58\hat{k}$,\;\;\;$\hat{n}_{24}=0.04\hat{i}+0.14\hat{j}+0.99\hat{k}$,\;\;\;$\vec{r}_{13}=3.42\hat{i}+7.36\hat{j}+7.95\hat{k}$,\;\;\;$\vec{r}_{23}=5.45\hat{i}+6.86\hat{j}+8.94\hat{k}$.

{\tiny 1D-M81:}

$\hat{n}_{14}=-0.66\hat{i}+0.09\hat{j}+0.75\hat{k}$,\;\;\;$\hat{n}_{23}=-0.66\hat{i}+0.09\hat{j}+0.75\hat{k}$,\;\;\;$\hat{n}_{24}=-0.58\hat{i}+0.58\hat{j}-0.58\hat{k}$,\;\;\;$\vec{r}_{13}=10.0\hat{i}+0.0\hat{j}+0.0\hat{k}$,\;\;\;$\vec{r}_{14}=0.0\hat{i}+10.0\hat{j}+10.0\hat{k}$.

{\tiny 1D-M82:}

$\hat{n}_{12}=-0.67\hat{i}+0.45\hat{j}+0.59\hat{k}$,\;\;\;$\hat{n}_{13}=0.55\hat{i}-0.61\hat{j}-0.57\hat{k}$,\;\;\;$\hat{n}_{24}=0.53\hat{i}-0.27\hat{j}+0.8\hat{k}$,\;\;\;$\vec{r}_{24}=0.0\hat{i}+10.0\hat{j}+0.0\hat{k}$,\;\;\;$\vec{r}_{34}=10.0\hat{i}+0.0\hat{j}+10.0\hat{k}$.

{\tiny 1D-M83:}

$\hat{n}_{12}=-0.0\hat{i}+0.0\hat{j}-1.0\hat{k}$,\;\;\;$\hat{n}_{13}=0.0\hat{i}+0.0\hat{j}+1.0\hat{k}$,\;\;\;$\hat{n}_{24}=0.71\hat{i}+0.71\hat{j}+0.0\hat{k}$,\;\;\;$\vec{r}_{13}=10.0\hat{i}+10.0\hat{j}+9.32\hat{k}$,\;\;\;$\vec{r}_{34}=0.0\hat{i}+0.0\hat{j}+0.29\hat{k}$.

{\tiny 1D-M84:}

$\hat{n}_{12}=-0.57\hat{i}-0.49\hat{j}-0.66\hat{k}$,\;\;\;$\hat{n}_{13}=-0.82\hat{i}+0.41\hat{j}+0.41\hat{k}$,\;\;\;$\hat{n}_{34}=0.58\hat{i}+0.6\hat{j}+0.56\hat{k}$,\;\;\;$\vec{r}_{13}=10.0\hat{i}+10.0\hat{j}+10.0\hat{k}$,\;\;\;$\vec{r}_{24}=0.0\hat{i}+0.0\hat{j}+0.0\hat{k}$.

{\tiny 1D-M85:}

$\hat{n}_{12}=-0.77\hat{i}-0.61\hat{j}-0.16\hat{k}$,\;\;\;$\hat{n}_{24}=0.58\hat{i}-0.58\hat{j}-0.58\hat{k}$,\;\;\;$\hat{n}_{34}=0.01\hat{i}-0.7\hat{j}+0.71\hat{k}$,\;\;\;$\vec{r}_{13}=0.0\hat{i}+10.0\hat{j}+0.0\hat{k}$,\;\;\;$\vec{r}_{34}=10.0\hat{i}+0.0\hat{j}+10.0\hat{k}$.

{\tiny 1D-M86:}

$\hat{n}_{12}=0.58\hat{i}-0.81\hat{j}-0.0\hat{k}$,\;\;\;$\hat{n}_{24}=0.0\hat{i}-0.0\hat{j}-1.0\hat{k}$,\;\;\;$\hat{n}_{34}=0.75\hat{i}-0.66\hat{j}+0.0\hat{k}$,\;\;\;$\vec{r}_{13}=0.0\hat{i}+10.0\hat{j}+1.51\hat{k}$,\;\;\;$\vec{r}_{24}=10.0\hat{i}+0.0\hat{j}+6.87\hat{k}$.

{\tiny 1D-M87:}

$\hat{n}_{12}=-0.82\hat{i}+0.41\hat{j}-0.41\hat{k}$,\;\;\;$\hat{n}_{24}=-0.58\hat{i}-0.64\hat{j}+0.51\hat{k}$,\;\;\;$\hat{n}_{34}=-0.58\hat{i}-0.55\hat{j}+0.6\hat{k}$,\;\;\;$\vec{r}_{12}=10.0\hat{i}+10.0\hat{j}+0.0\hat{k}$,\;\;\;$\vec{r}_{13}=0.0\hat{i}+0.0\hat{j}+10.0\hat{k}$.
