# Supplementary material for: Dimensional synthesis of spatial manipulators for velocity and force transmission for operation around a specified task point
Source: arXiv:2210.04446 source file (2022-10-10)
Supplement: Supplementary file 34 [file classappendix7.tex]

\subsection{Class 7} \label{appendix_five_2_1}
{\tiny 1D-M88:}

$\hat{n}_{13}=-0.58\hat{i}+0.58\hat{j}-0.58\hat{k}$,\;\;\;$\hat{n}_{14}=0.58\hat{i}-0.58\hat{j}+0.58\hat{k}$,\;\;\;$\vec{r}_{23}=0.0\hat{i}+10.0\hat{j}+10.0\hat{k}$,\;\;\;$\vec{r}_{24}=10.0\hat{i}+0.0\hat{j}+0.0\hat{k}$.

{\tiny 1D-M89:}

$\hat{n}_{14}=0.0\hat{i}-0.36\hat{j}-0.93\hat{k}$,\;\;\;$\hat{n}_{24}=-0.72\hat{i}-0.26\hat{j}-0.64\hat{k}$,\;\;\;$\vec{r}_{13}=8.34\hat{i}+6.1\hat{j}+5.75\hat{k}$,\;\;\;$\vec{r}_{23}=3.26\hat{i}+4.56\hat{j}+7.14\hat{k}$.

{\tiny 1D-M90:}

$\hat{n}_{12}=0.0\hat{i}+0.0\hat{j}+1.0\hat{k}$,\;\;\;$\hat{n}_{24}=-0.0\hat{i}+0.92\hat{j}+0.38\hat{k}$,\;\;\;$\vec{r}_{13}=10.0\hat{i}+10.0\hat{j}+10.0\hat{k}$,\;\;\;$\vec{r}_{34}=0.0\hat{i}+0.0\hat{j}+0.0\hat{k}$.
