# Supplementary material for: Dimensional synthesis of spatial manipulators for velocity and force transmission for operation around a specified task point
Source: arXiv:2210.04446 source file (2022-10-10)
Supplement: Supplementary file 35 [file classappendix8.tex]

\subsection{Class 8} \label{appendix_five_2_1}
{\tiny 1D-M91:}

$\hat{n}_{13}=-0.24\hat{i}-0.85\hat{j}+0.47\hat{k}$,\;\;\;$\hat{n}_{14}=-0.24\hat{i}-0.85\hat{j}+0.47\hat{k}$,\;\;\;$\hat{n}_{23}=-0.35\hat{i}-0.37\hat{j}-0.86\hat{k}$,\;\;\;$\hat{n}_{24}=0.91\hat{i}-0.37\hat{j}-0.21\hat{k}$,\;\;\;$\vec{r}_{14}=4.82\hat{i}+5.35\hat{j}+4.24\hat{k}$,\;\;\;$\vec{r}_{23}=5.77\hat{i}+5.14\hat{j}+4.2\hat{k}$,\;\;\;$\vec{r}_{24}=5.35\hat{i}+5.81\hat{j}+5.53\hat{k}$.

{\tiny 1D-M92:}

$\hat{n}_{13}=-0.05\hat{i}-0.21\hat{j}+0.98\hat{k}$,\;\;\;$\hat{n}_{14}=0.19\hat{i}+0.29\hat{j}-0.94\hat{k}$,\;\;\;$\hat{n}_{23}=0.16\hat{i}+0.12\hat{j}+0.98\hat{k}$,\;\;\;$\hat{n}_{24}=-0.72\hat{i}-0.67\hat{j}+0.2\hat{k}$,\;\;\;$\vec{r}_{13}=8.59\hat{i}+9.74\hat{j}+5.71\hat{k}$,\;\;\;$\vec{r}_{23}=9.97\hat{i}+5.54\hat{j}+5.15\hat{k}$,\;\;\;$\vec{r}_{24}=3.31\hat{i}+4.3\hat{j}+4.92\hat{k}$.

{\tiny 1D-M93:}

$\hat{n}_{13}=-0.63\hat{i}+0.17\hat{j}+0.75\hat{k}$,\;\;\;$\hat{n}_{14}=0.76\hat{i}-0.05\hat{j}+0.65\hat{k}$,\;\;\;$\hat{n}_{23}=0.76\hat{i}-0.05\hat{j}+0.65\hat{k}$,\;\;\;$\hat{n}_{24}=-0.14\hat{i}-0.98\hat{j}+0.1\hat{k}$,\;\;\;$\vec{r}_{13}=5.68\hat{i}+5.82\hat{j}+5.13\hat{k}$,\;\;\;$\vec{r}_{14}=4.08\hat{i}+5.92\hat{j}+4.4\hat{k}$,\;\;\;$\vec{r}_{24}=5.36\hat{i}+5.32\hat{j}+5.78\hat{k}$.

{\tiny 1D-M94:}

$\hat{n}_{13}=0.4\hat{i}-0.48\hat{j}+0.78\hat{k}$,\;\;\;$\hat{n}_{14}=0.26\hat{i}-0.75\hat{j}-0.61\hat{k}$,\;\;\;$\hat{n}_{23}=-0.88\hat{i}-0.45\hat{j}+0.18\hat{k}$,\;\;\;$\hat{n}_{24}=0.26\hat{i}-0.75\hat{j}-0.61\hat{k}$,\;\;\;$\vec{r}_{13}=4.92\hat{i}+4.88\hat{j}+5.04\hat{k}$,\;\;\;$\vec{r}_{14}=4.81\hat{i}+4.88\hat{j}+4.88\hat{k}$,\;\;\;$\vec{r}_{23}=4.93\hat{i}+4.88\hat{j}+5.07\hat{k}$.

{\tiny 1D-M95:}

$\hat{n}_{12}=-0.89\hat{i}-0.29\hat{j}-0.36\hat{k}$,\;\;\;$\hat{n}_{13}=0.66\hat{i}+0.57\hat{j}+0.49\hat{k}$,\;\;\;$\hat{n}_{24}=-0.16\hat{i}-0.53\hat{j}+0.83\hat{k}$,\;\;\;$\hat{n}_{34}=-0.73\hat{i}+0.63\hat{j}+0.26\hat{k}$,\;\;\;$\vec{r}_{13}=4.73\hat{i}+4.26\hat{j}+4.77\hat{k}$,\;\;\;$\vec{r}_{24}=5.36\hat{i}+5.47\hat{j}+4.87\hat{k}$,\;\;\;$\vec{r}_{34}=4.74\hat{i}+5.76\hat{j}+4.86\hat{k}$.

{\tiny 1D-M96:}

$\hat{n}_{12}=-0.52\hat{i}-0.13\hat{j}+0.84\hat{k}$,\;\;\;$\hat{n}_{13}=0.7\hat{i}-0.64\hat{j}+0.33\hat{k}$,\;\;\;$\hat{n}_{24}=-0.18\hat{i}-0.95\hat{j}-0.26\hat{k}$,\;\;\;$\hat{n}_{34}=-0.49\hat{i}-0.76\hat{j}-0.42\hat{k}$,\;\;\;$\vec{r}_{12}=3.53\hat{i}+7.37\hat{j}+5.85\hat{k}$,\;\;\;$\vec{r}_{13}=7.27\hat{i}+7.33\hat{j}+2.16\hat{k}$,\;\;\;$\vec{r}_{34}=3.23\hat{i}+6.27\hat{j}+4.91\hat{k}$.
