# Supplementary material for: Dimensional synthesis of spatial manipulators for velocity and force transmission for operation around a specified task point
Source: arXiv:2210.04446 source file (2022-10-10)
Supplement: Supplementary file 36 [file classappendix1.tex]

\subsection{Class 1} \label{appendix_five_2_1}
Manipulator 1:

$\vec{r}_{12}=0.0\hat{i}+8.21\hat{j}+10.0\hat{k}$\newline
$\vec{r}_{23}=0.02\hat{i}+7.16\hat{j}+6.31\hat{k}$\newline
$\hat{n}_{23}=-0.29\hat{i}-0.45\hat{j}-0.85\hat{k}$\newline
$\hat{n}_{12}=-0.31\hat{i}+0.15\hat{j}+0.94\hat{k}$
