# Supplementary material for: Dimensional synthesis of spatial manipulators for velocity and force transmission for operation around a specified task point
Source: arXiv:2210.04446 source file (2022-10-10)
Supplement: Supplementary file 37 [file classappendix12.tex]

\subsection{Class 12} \label{appendix_five_2_1}
{\tiny 2D-M642:}

$\hat{n}_{12}=0.05\hat{i}+0.55\hat{j}-0.83\hat{k}$,\;\;\;$\hat{n}_{23}=0.82\hat{i}-0.5\hat{j}-0.28\hat{k}$,\;\;\;$\vec{r}_{12}=10.0\hat{i}+10.0\hat{j}+10.0\hat{k}$,\;\;\;$\vec{r}_{23}=10.0\hat{i}+10.0\hat{j}+10.0\hat{k}$.
