# Supplementary material for: Dimensional synthesis of spatial manipulators for velocity and force transmission for operation around a specified task point
Source: arXiv:2210.04446 source file (2022-10-10)
Supplement: Supplementary file 38 [file classappendix13.tex]

\subsection{Class 13} \label{appendix_five_2_1}
{\tiny 2D-M643:}

$\hat{n}_{12}=0.73\hat{i}-0.15\hat{j}+0.66\hat{k}$,\;\;\;$\hat{n}_{23}=-0.03\hat{i}-0.63\hat{j}+0.78\hat{k}$,\;\;\;$\vec{r}_{12}=10.0\hat{i}+10.0\hat{j}+0.0\hat{k}$.

{\tiny 2D-M644:}

$\hat{n}_{12}=-0.68\hat{i}-0.48\hat{j}+0.55\hat{k}$,\;\;\;$\hat{n}_{23}=0.55\hat{i}-0.74\hat{j}-0.39\hat{k}$,\;\;\;$\vec{r}_{23}=10.0\hat{i}+10.0\hat{j}+0.0\hat{k}$.
