# Supplementary material for: Dimensional synthesis of spatial manipulators for velocity and force transmission for operation around a specified task point
Source: arXiv:2210.04446 source file (2022-10-10)
Supplement: Supplementary file 39 [file classappendix14.tex]

\subsection{Class 14} \label{appendix_five_2_1}
{\tiny 2D-M645:}

$\hat{n}_{12}=0.97\hat{i}+0.03\hat{j}+0.24\hat{k}$,\;\;\;$\hat{n}_{23}=0.03\hat{i}-1.0\hat{j}-0.01\hat{k}$.
