# Supplementary material for: Dimensional synthesis of spatial manipulators for velocity and force transmission for operation around a specified task point
Source: arXiv:2210.04446 source file (2022-10-10)
Supplement: Supplementary file 40 [file classappendix2.tex]

\subsection{Class 2} \label{appendix_five_2_1}
Manipulator 2:

$\vec{r}_{12}=1.83\hat{i}+2.97\hat{j}+1.26\hat{k}$\newline
$\vec{r}_{23}=0.83\hat{i}+6.09\hat{j}+0.81\hat{k}$\newline
$\hat{n}_{23}=-0.0\hat{i}-0.71\hat{j}+0.71\hat{k}$\newline
$\hat{n}_{12}=0.0\hat{i}+0.0\hat{j}+1.0\hat{k}$

Manipulator 3:

$\vec{r}_{23}=5.55\hat{i}+9.95\hat{j}+0.02\hat{k}$\newline
$\hat{n}_{23}=0.02\hat{i}+0.79\hat{j}-0.61\hat{k}$\newline
$\hat{n}_{12}=-0.0\hat{i}-0.54\hat{j}-0.84\hat{k}$
