# Supplementary material for: Dimensional synthesis of spatial manipulators for velocity and force transmission for operation around a specified task point
Source: arXiv:2210.04446 source file (2022-10-10)
Supplement: Supplementary file 41 [file classappendix3.tex]

\subsection{Class 3} \label{appendix_five_2_1}
Manipulator 4:

$\hat{n}_{23}=0.1\hat{i}-0.12\hat{j}-0.99\hat{k}$\newline
$\hat{n}_{12}=0.0\hat{i}+0.66\hat{j}+0.75\hat{k}$
