# Supplementary material for: Dimensional synthesis of spatial manipulators for velocity and force transmission for operation around a specified task point
Source: arXiv:2210.04446 source file (2022-10-10)
Supplement: Supplementary file 42 [file classappendix1.tex]

\subsection{Class 1} \label{appendix_five_2_1}
{\tiny 2D-M1:}

$\hat{n}_{14}=0.0\hat{i}+0.96\hat{j}+0.28\hat{k}$,\;\;\;$\hat{n}_{24}=-0.79\hat{i}+0.32\hat{j}-0.52\hat{k}$,\;\;\;$\hat{n}_{25}=0.1\hat{i}-0.67\hat{j}+0.74\hat{k}$,\;\;\;$\vec{r}_{14}=0.0\hat{i}+0.0\hat{j}+10.0\hat{k}$,\newline
$\vec{r}_{24}=10.0\hat{i}+10.0\hat{j}+0.0\hat{k}$,\;\;\;$\vec{r}_{25}=10.0\hat{i}+0.0\hat{j}+10.0\hat{k}$,\;\;\;$\vec{r}_{34}=0.0\hat{i}+0.0\hat{j}+0.0\hat{k}$,\;\;\;$\vec{r}_{35}=10.0\hat{i}+10.0\hat{j}+10.0\hat{k}$.

{\tiny 2D-M2:}

$\hat{n}_{14}=-0.31\hat{i}+0.43\hat{j}+0.85\hat{k}$,\;\;\;$\hat{n}_{25}=-0.71\hat{i}+0.0\hat{j}-0.71\hat{k}$,\;\;\;$\hat{n}_{45}=0.7\hat{i}-0.01\hat{j}+0.72\hat{k}$,\;\;\;$\vec{r}_{14}=10.0\hat{i}+0.0\hat{j}+0.0\hat{k}$,\newline
$\vec{r}_{23}=10.0\hat{i}+0.0\hat{j}+10.0\hat{k}$,\;\;\;$\vec{r}_{25}=10.0\hat{i}+10.0\hat{j}+0.0\hat{k}$,\;\;\;$\vec{r}_{34}=0.0\hat{i}+10.0\hat{j}+0.0\hat{k}$,\;\;\;$\vec{r}_{45}=10.0\hat{i}+10.0\hat{j}+0.0\hat{k}$.

{\tiny 2D-M3:}

$\hat{n}_{14}=-0.56\hat{i}+0.74\hat{j}-0.37\hat{k}$,\;\;\;$\hat{n}_{34}=-0.0\hat{i}+0.71\hat{j}-0.71\hat{k}$,\;\;\;$\hat{n}_{45}=-0.69\hat{i}-0.01\hat{j}+0.73\hat{k}$,\;\;\;$\vec{r}_{14}=10.0\hat{i}+10.0\hat{j}+10.0\hat{k}$,\newline
$\vec{r}_{23}=10.0\hat{i}+10.0\hat{j}+10.0\hat{k}$,\;\;\;$\vec{r}_{25}=0.0\hat{i}+0.0\hat{j}+0.0\hat{k}$,\;\;\;$\vec{r}_{34}=0.0\hat{i}+10.0\hat{j}+0.0\hat{k}$,\;\;\;$\vec{r}_{45}=0.0\hat{i}+10.0\hat{j}+10.0\hat{k}$.

{\tiny 2D-M4:}

$\hat{n}_{13}=-0.59\hat{i}+0.81\hat{j}-0.01\hat{k}$,\;\;\;$\hat{n}_{14}=0.58\hat{i}-0.58\hat{j}-0.58\hat{k}$,\;\;\;$\hat{n}_{35}=-0.04\hat{i}-0.74\hat{j}-0.67\hat{k}$,\;\;\;$\vec{r}_{13}=0.0\hat{i}+0.0\hat{j}+0.0\hat{k}$,\newline
$\vec{r}_{14}=0.0\hat{i}+0.0\hat{j}+0.0\hat{k}$,\;\;\;$\vec{r}_{24}=10.0\hat{i}+10.0\hat{j}+0.0\hat{k}$,\;\;\;$\vec{r}_{25}=0.0\hat{i}+10.0\hat{j}+10.0\hat{k}$,\;\;\;$\vec{r}_{35}=0.0\hat{i}+0.0\hat{j}+10.0\hat{k}$.

{\tiny 2D-M5:}

$\hat{n}_{13}=-0.0\hat{i}+0.71\hat{j}+0.71\hat{k}$,\;\;\;$\hat{n}_{14}=-0.02\hat{i}-0.67\hat{j}-0.74\hat{k}$,\;\;\;$\hat{n}_{45}=0.71\hat{i}-0.11\hat{j}-0.7\hat{k}$,\;\;\;$\vec{r}_{13}=0.0\hat{i}+10.0\hat{j}+10.0\hat{k}$,\newline
$\vec{r}_{14}=10.0\hat{i}+0.0\hat{j}+0.0\hat{k}$,\;\;\;$\vec{r}_{23}=10.0\hat{i}+10.0\hat{j}+0.0\hat{k}$,\;\;\;$\vec{r}_{24}=0.0\hat{i}+0.0\hat{j}+10.0\hat{k}$,\;\;\;$\vec{r}_{45}=10.0\hat{i}+10.0\hat{j}+10.0\hat{k}$.
