# Supplementary material for: Dimensional synthesis of spatial manipulators for velocity and force transmission for operation around a specified task point
Source: arXiv:2210.04446 source file (2022-10-10)
Supplement: Supplementary file 45 [file classappendix12.tex]

\subsection{Class 12} \label{appendix_five_2_1}
{\tiny 2D-M19:}

$\hat{n}_{13}=-0.0\hat{i}-0.71\hat{j}+0.71\hat{k}$,\;\;\;$\hat{n}_{14}=-0.0\hat{i}+0.86\hat{j}+0.51\hat{k}$,\;\;\;$\hat{n}_{45}=-0.0\hat{i}+0.86\hat{j}+0.51\hat{k}$,\;\;\;$\vec{r}_{13}=0.0\hat{i}+10.0\hat{j}+0.0\hat{k}$,\newline
$\vec{r}_{23}=0.0\hat{i}+0.0\hat{j}+0.0\hat{k}$,\;\;\;$\vec{r}_{24}=10.0\hat{i}+10.0\hat{j}+10.0\hat{k}$,\;\;\;$\vec{r}_{45}=0.0\hat{i}+0.0\hat{j}+10.0\hat{k}$.

{\tiny 2D-M35:}

$\hat{n}_{13}=-0.58\hat{i}+0.58\hat{j}-0.58\hat{k}$,\;\;\;$\hat{n}_{14}=0.0\hat{i}+0.71\hat{j}-0.71\hat{k}$,\;\;\;$\hat{n}_{45}=-0.08\hat{i}+0.62\hat{j}-0.78\hat{k}$,\;\;\;$\vec{r}_{23}=10.0\hat{i}+0.0\hat{j}+0.0\hat{k}$,\newline
$\vec{r}_{24}=0.0\hat{i}+10.0\hat{j}+10.0\hat{k}$,\;\;\;$\vec{r}_{45}=10.0\hat{i}+10.0\hat{j}+10.0\hat{k}$.

{\tiny 2D-M39:}

$\hat{n}_{13}=-0.0\hat{i}+0.71\hat{j}-0.71\hat{k}$,\;\;\;$\hat{n}_{14}=-0.58\hat{i}+0.58\hat{j}+0.58\hat{k}$,\;\;\;$\hat{n}_{35}=0.0\hat{i}+0.71\hat{j}+0.71\hat{k}$,\;\;\;$\vec{r}_{24}=10.0\hat{i}+0.0\hat{j}+10.0\hat{k}$,\newline
$\vec{r}_{25}=0.0\hat{i}+10.0\hat{j}+0.0\hat{k}$.

{\tiny 2D-M44:}

$\hat{n}_{14}=0.7\hat{i}-0.1\hat{j}+0.7\hat{k}$,\;\;\;$\hat{n}_{24}=0.74\hat{i}-0.18\hat{j}+0.65\hat{k}$,\;\;\;$\hat{n}_{25}=-0.87\hat{i}-0.07\hat{j}-0.48\hat{k}$,\;\;\;$\hat{n}_{35}=-0.19\hat{i}-0.59\hat{j}+0.78\hat{k}$,\newline
$\vec{r}_{14}=10.0\hat{i}+0.0\hat{j}+10.0\hat{k}$,\;\;\;$\vec{r}_{24}=10.0\hat{i}+10.0\hat{j}+0.0\hat{k}$,\;\;\;$\vec{r}_{25}=10.0\hat{i}+0.0\hat{j}+10.0\hat{k}$,\;\;\;$\vec{r}_{34}=0.0\hat{i}+0.0\hat{j}+0.0\hat{k}$,\newline
$\vec{r}_{35}=10.0\hat{i}+10.0\hat{j}+10.0\hat{k}$.

{\tiny 2D-M48:}

$\hat{n}_{14}=0.0\hat{i}+0.0\hat{j}+1.0\hat{k}$,\;\;\;$\hat{n}_{23}=-0.64\hat{i}+0.64\hat{j}-0.43\hat{k}$,\;\;\;$\hat{n}_{25}=0.09\hat{i}-0.7\hat{j}+0.7\hat{k}$,\;\;\;$\hat{n}_{45}=-0.49\hat{i}+0.5\hat{j}+0.72\hat{k}$,\newline
$\vec{r}_{14}=10.0\hat{i}+0.0\hat{j}+10.0\hat{k}$,\;\;\;$\vec{r}_{23}=10.0\hat{i}+10.0\hat{j}+0.0\hat{k}$,\;\;\;$\vec{r}_{25}=10.0\hat{i}+0.0\hat{j}+10.0\hat{k}$,\;\;\;$\vec{r}_{34}=0.0\hat{i}+0.0\hat{j}+0.0\hat{k}$,\newline
$\vec{r}_{45}=10.0\hat{i}+10.0\hat{j}+10.0\hat{k}$.

{\tiny 2D-M63:}

$\hat{n}_{14}=0.68\hat{i}+0.52\hat{j}+0.52\hat{k}$,\;\;\;$\hat{n}_{23}=0.84\hat{i}+0.1\hat{j}-0.53\hat{k}$,\;\;\;$\hat{n}_{25}=0.0\hat{i}+0.0\hat{j}+1.0\hat{k}$,\;\;\;$\hat{n}_{34}=-0.0\hat{i}+0.16\hat{j}-0.99\hat{k}$,\newline
$\vec{r}_{14}=0.0\hat{i}+0.0\hat{j}+10.0\hat{k}$,\;\;\;$\vec{r}_{15}=10.0\hat{i}+0.0\hat{j}+0.0\hat{k}$,\;\;\;$\vec{r}_{23}=10.0\hat{i}+0.0\hat{j}+0.0\hat{k}$,\;\;\;$\vec{r}_{25}=10.0\hat{i}+10.0\hat{j}+1.8\hat{k}$,\newline
$\vec{r}_{34}=0.0\hat{i}+10.0\hat{j}+0.0\hat{k}$.

{\tiny 2D-M69:}

$\hat{n}_{13}=0.69\hat{i}-0.03\hat{j}+0.72\hat{k}$,\;\;\;$\hat{n}_{14}=-0.33\hat{i}+0.9\hat{j}+0.29\hat{k}$,\;\;\;$\hat{n}_{24}=-0.51\hat{i}-0.85\hat{j}+0.12\hat{k}$,\;\;\;$\hat{n}_{25}=0.34\hat{i}+0.69\hat{j}-0.64\hat{k}$,\newline
$\vec{r}_{13}=10.0\hat{i}+0.0\hat{j}+10.0\hat{k}$,\;\;\;$\vec{r}_{14}=10.0\hat{i}+10.0\hat{j}+0.0\hat{k}$,\;\;\;$\vec{r}_{24}=10.0\hat{i}+0.0\hat{j}+0.0\hat{k}$,\;\;\;$\vec{r}_{25}=10.0\hat{i}+10.0\hat{j}+10.0\hat{k}$,\newline
$\vec{r}_{35}=0.0\hat{i}+10.0\hat{j}+0.0\hat{k}$.

{\tiny 2D-M88:}

$\hat{n}_{13}=0.0\hat{i}+0.62\hat{j}-0.79\hat{k}$,\;\;\;$\hat{n}_{24}=0.82\hat{i}+0.42\hat{j}+0.39\hat{k}$,\;\;\;$\hat{n}_{25}=0.0\hat{i}-0.7\hat{j}+0.71\hat{k}$,\;\;\;$\hat{n}_{35}=-0.0\hat{i}+0.7\hat{j}-0.72\hat{k}$,\newline
$\vec{r}_{13}=10.0\hat{i}+10.0\hat{j}+10.0\hat{k}$,\;\;\;$\vec{r}_{14}=10.0\hat{i}+0.0\hat{j}+10.0\hat{k}$,\;\;\;$\vec{r}_{24}=0.0\hat{i}+10.0\hat{j}+0.0\hat{k}$,\;\;\;$\vec{r}_{25}=10.0\hat{i}+10.0\hat{j}+10.0\hat{k}$,\newline
$\vec{r}_{35}=0.0\hat{i}+0.0\hat{j}+0.0\hat{k}$.

{\tiny 2D-M101:}

$\hat{n}_{13}=-0.5\hat{i}-0.83\hat{j}-0.24\hat{k}$,\;\;\;$\hat{n}_{23}=-0.08\hat{i}-0.53\hat{j}-0.84\hat{k}$,\;\;\;$\hat{n}_{25}=0.0\hat{i}+0.97\hat{j}+0.26\hat{k}$,\;\;\;$\hat{n}_{45}=-0.83\hat{i}-0.4\hat{j}-0.4\hat{k}$,\newline
$\vec{r}_{13}=10.0\hat{i}+0.0\hat{j}+10.0\hat{k}$,\;\;\;$\vec{r}_{14}=10.0\hat{i}+10.0\hat{j}+0.0\hat{k}$,\;\;\;$\vec{r}_{23}=10.0\hat{i}+10.0\hat{j}+0.0\hat{k}$,\;\;\;$\vec{r}_{25}=0.0\hat{i}+10.0\hat{j}+10.0\hat{k}$,\newline
$\vec{r}_{45}=0.0\hat{i}+10.0\hat{j}+10.0\hat{k}$.

{\tiny 2D-M107:}

$\hat{n}_{14}=0.53\hat{i}-0.74\hat{j}-0.41\hat{k}$,\;\;\;$\hat{n}_{24}=0.69\hat{i}+0.12\hat{j}+0.72\hat{k}$,\;\;\;$\hat{n}_{25}=-0.6\hat{i}+0.75\hat{j}+0.3\hat{k}$,\;\;\;$\hat{n}_{34}=-0.63\hat{i}-0.48\hat{j}+0.62\hat{k}$,\newline
$\vec{r}_{14}=10.0\hat{i}+10.0\hat{j}+0.0\hat{k}$,\;\;\;$\vec{r}_{24}=0.0\hat{i}+10.0\hat{j}+0.0\hat{k}$,\;\;\;$\vec{r}_{25}=10.0\hat{i}+10.0\hat{j}+0.0\hat{k}$,\;\;\;$\vec{r}_{35}=0.0\hat{i}+0.0\hat{j}+10.0\hat{k}$.
