# Supplementary material for: Dimensional synthesis of spatial manipulators for velocity and force transmission for operation around a specified task point
Source: arXiv:2210.04446 source file (2022-10-10)
Supplement: Supplementary file 46 [file classappendix2.tex]

\subsection{Class 2} \label{appendix_five_2_1}
{\tiny 2D-M6:}

$\hat{n}_{14}=0.74\hat{i}-0.67\hat{j}-0.04\hat{k}$,\;\;\;$\hat{n}_{24}=-0.37\hat{i}-0.31\hat{j}-0.88\hat{k}$,\;\;\;$\hat{n}_{25}=-0.58\hat{i}-0.57\hat{j}-0.58\hat{k}$,\;\;\;$\vec{r}_{14}=10.0\hat{i}+10.0\hat{j}+0.0\hat{k}$,\newline
$\vec{r}_{24}=10.0\hat{i}+10.0\hat{j}+0.0\hat{k}$,\;\;\;$\vec{r}_{34}=0.0\hat{i}+0.0\hat{j}+0.0\hat{k}$,\;\;\;$\vec{r}_{35}=10.0\hat{i}+10.0\hat{j}+10.0\hat{k}$.

{\tiny 2D-M7:}

$\hat{n}_{14}=-0.0\hat{i}+0.58\hat{j}-0.81\hat{k}$,\;\;\;$\hat{n}_{24}=0.58\hat{i}+0.58\hat{j}-0.58\hat{k}$,\;\;\;$\hat{n}_{25}=-0.71\hat{i}+0.11\hat{j}-0.7\hat{k}$,\;\;\;$\vec{r}_{14}=10.0\hat{i}+0.0\hat{j}+10.0\hat{k}$,\newline
$\vec{r}_{25}=10.0\hat{i}+10.0\hat{j}+0.0\hat{k}$,\;\;\;$\vec{r}_{34}=10.0\hat{i}+10.0\hat{j}+0.0\hat{k}$,\;\;\;$\vec{r}_{35}=0.0\hat{i}+0.0\hat{j}+10.0\hat{k}$.

{\tiny 2D-M8:}

$\hat{n}_{14}=-0.46\hat{i}+0.74\hat{j}+0.48\hat{k}$,\;\;\;$\hat{n}_{25}=0.0\hat{i}-0.71\hat{j}+0.71\hat{k}$,\;\;\;$\hat{n}_{45}=0.58\hat{i}-0.58\hat{j}-0.58\hat{k}$,\;\;\;$\vec{r}_{14}=10.0\hat{i}+10.0\hat{j}+0.0\hat{k}$,\newline
$\vec{r}_{23}=0.0\hat{i}+10.0\hat{j}+0.0\hat{k}$,\;\;\;$\vec{r}_{25}=0.0\hat{i}+0.0\hat{j}+0.0\hat{k}$,\;\;\;$\vec{r}_{34}=10.0\hat{i}+0.0\hat{j}+10.0\hat{k}$.

{\tiny 2D-M9:}

$\hat{n}_{14}=-0.0\hat{i}+0.58\hat{j}+0.81\hat{k}$,\;\;\;$\hat{n}_{25}=-0.36\hat{i}-0.93\hat{j}-0.05\hat{k}$,\;\;\;$\hat{n}_{45}=0.71\hat{i}-0.1\hat{j}+0.7\hat{k}$,\;\;\;$\vec{r}_{14}=10.0\hat{i}+10.0\hat{j}+0.0\hat{k}$,\newline
$\vec{r}_{23}=6.41\hat{i}+3.46\hat{j}+3.55\hat{k}$,\;\;\;$\vec{r}_{34}=6.26\hat{i}+6.53\hat{j}+1.95\hat{k}$,\;\;\;$\vec{r}_{45}=10.0\hat{i}+0.0\hat{j}+10.0\hat{k}$.

{\tiny 2D-M10:}

$\hat{n}_{14}=0.0\hat{i}+0.58\hat{j}-0.81\hat{k}$,\;\;\;$\hat{n}_{34}=0.71\hat{i}+0.0\hat{j}-0.71\hat{k}$,\;\;\;$\hat{n}_{45}=0.57\hat{i}+0.58\hat{j}+0.58\hat{k}$,\;\;\;$\vec{r}_{14}=10.0\hat{i}+10.0\hat{j}+10.0\hat{k}$,\newline
$\vec{r}_{23}=10.0\hat{i}+10.0\hat{j}+10.0\hat{k}$,\;\;\;$\vec{r}_{25}=0.0\hat{i}+0.0\hat{j}+0.0\hat{k}$,\;\;\;$\vec{r}_{34}=0.0\hat{i}+10.0\hat{j}+10.0\hat{k}$.

{\tiny 2D-M11:}

$\hat{n}_{14}=0.69\hat{i}+0.47\hat{j}-0.55\hat{k}$,\;\;\;$\hat{n}_{34}=0.03\hat{i}-0.89\hat{j}-0.45\hat{k}$,\;\;\;$\hat{n}_{45}=-0.02\hat{i}+0.86\hat{j}+0.5\hat{k}$,\;\;\;$\vec{r}_{14}=0.0\hat{i}+10.0\hat{j}+10.0\hat{k}$,\newline
$\vec{r}_{23}=5.17\hat{i}+6.28\hat{j}+5.07\hat{k}$,\;\;\;$\vec{r}_{25}=5.29\hat{i}+3.75\hat{j}+5.48\hat{k}$,\;\;\;$\vec{r}_{45}=0.0\hat{i}+0.0\hat{j}+10.0\hat{k}$.

{\tiny 2D-M12:}

$\hat{n}_{14}=0.7\hat{i}+0.53\hat{j}-0.47\hat{k}$,\;\;\;$\hat{n}_{24}=0.0\hat{i}+0.85\hat{j}+0.52\hat{k}$,\;\;\;$\hat{n}_{25}=-0.05\hat{i}+0.72\hat{j}-0.69\hat{k}$,\;\;\;$\vec{r}_{24}=10.0\hat{i}+10.0\hat{j}+0.0\hat{k}$,\newline
$\vec{r}_{25}=0.0\hat{i}+0.0\hat{j}+0.0\hat{k}$,\;\;\;$\vec{r}_{34}=10.0\hat{i}+0.0\hat{j}+10.0\hat{k}$,\;\;\;$\vec{r}_{35}=0.0\hat{i}+10.0\hat{j}+0.0\hat{k}$.

{\tiny 2D-M13:}

$\hat{n}_{14}=-0.0\hat{i}+0.0\hat{j}-1.0\hat{k}$,\;\;\;$\hat{n}_{25}=0.71\hat{i}-0.71\hat{j}+0.0\hat{k}$,\;\;\;$\hat{n}_{45}=0.07\hat{i}-0.64\hat{j}-0.76\hat{k}$,\;\;\;$\vec{r}_{23}=10.0\hat{i}+10.0\hat{j}+0.0\hat{k}$,\newline
$\vec{r}_{25}=10.0\hat{i}+10.0\hat{j}+10.0\hat{k}$,\;\;\;$\vec{r}_{34}=0.0\hat{i}+0.0\hat{j}+10.0\hat{k}$,\;\;\;$\vec{r}_{45}=10.0\hat{i}+0.0\hat{j}+0.0\hat{k}$.

{\tiny 2D-M14:}

$\hat{n}_{14}=0.0\hat{i}+0.0\hat{j}-1.0\hat{k}$,\;\;\;$\hat{n}_{34}=0.0\hat{i}-0.71\hat{j}-0.71\hat{k}$,\;\;\;$\hat{n}_{45}=0.7\hat{i}+0.09\hat{j}-0.71\hat{k}$,\;\;\;$\vec{r}_{23}=10.0\hat{i}+0.0\hat{j}+0.0\hat{k}$,\newline
$\vec{r}_{25}=0.0\hat{i}+10.0\hat{j}+10.0\hat{k}$,\;\;\;$\vec{r}_{34}=0.0\hat{i}+0.0\hat{j}+10.0\hat{k}$,\;\;\;$\vec{r}_{45}=0.0\hat{i}+0.0\hat{j}+0.0\hat{k}$.

{\tiny 2D-M15:}

$\hat{n}_{13}=-0.46\hat{i}+0.74\hat{j}+0.48\hat{k}$,\;\;\;$\hat{n}_{14}=-0.71\hat{i}-0.71\hat{j}+0.0\hat{k}$,\;\;\;$\hat{n}_{35}=0.58\hat{i}-0.58\hat{j}-0.58\hat{k}$,\;\;\;$\vec{r}_{13}=10.0\hat{i}+10.0\hat{j}+0.0\hat{k}$,\newline
$\vec{r}_{14}=0.0\hat{i}+10.0\hat{j}+10.0\hat{k}$,\;\;\;$\vec{r}_{24}=0.0\hat{i}+10.0\hat{j}+0.0\hat{k}$,\;\;\;$\vec{r}_{25}=10.0\hat{i}+0.0\hat{j}+10.0\hat{k}$.

{\tiny 2D-M16:}

$\hat{n}_{13}=-0.0\hat{i}+0.71\hat{j}+0.71\hat{k}$,\;\;\;$\hat{n}_{14}=0.0\hat{i}+0.16\hat{j}-0.99\hat{k}$,\;\;\;$\hat{n}_{45}=-0.27\hat{i}+0.32\hat{j}-0.91\hat{k}$,\;\;\;$\vec{r}_{13}=0.0\hat{i}+10.0\hat{j}+10.0\hat{k}$,\newline
$\vec{r}_{14}=0.0\hat{i}+10.0\hat{j}+0.0\hat{k}$,\;\;\;$\vec{r}_{23}=0.0\hat{i}+0.0\hat{j}+10.0\hat{k}$,\;\;\;$\vec{r}_{24}=10.0\hat{i}+10.0\hat{j}+0.0\hat{k}$.

{\tiny 2D-M17:}

$\hat{n}_{13}=0.71\hat{i}-0.11\hat{j}+0.7\hat{k}$,\;\;\;$\hat{n}_{14}=0.58\hat{i}+0.58\hat{j}+0.58\hat{k}$,\;\;\;$\hat{n}_{35}=-0.0\hat{i}+0.0\hat{j}+1.0\hat{k}$,\;\;\;$\vec{r}_{13}=10.0\hat{i}+10.0\hat{j}+0.0\hat{k}$,\newline
$\vec{r}_{24}=0.0\hat{i}+0.0\hat{j}+0.0\hat{k}$,\;\;\;$\vec{r}_{25}=10.0\hat{i}+10.0\hat{j}+10.0\hat{k}$,\;\;\;$\vec{r}_{35}=10.0\hat{i}+0.0\hat{j}+10.0\hat{k}$.

{\tiny 2D-M18:}

$\hat{n}_{13}=-0.71\hat{i}+0.71\hat{j}-0.0\hat{k}$,\;\;\;$\hat{n}_{14}=0.0\hat{i}+0.71\hat{j}+0.71\hat{k}$,\;\;\;$\hat{n}_{45}=-0.04\hat{i}+0.73\hat{j}+0.68\hat{k}$,\;\;\;$\vec{r}_{13}=10.0\hat{i}+10.0\hat{j}+10.0\hat{k}$,\newline
$\vec{r}_{23}=10.0\hat{i}+10.0\hat{j}+0.0\hat{k}$,\;\;\;$\vec{r}_{25}=0.0\hat{i}+0.0\hat{j}+10.0\hat{k}$,\;\;\;$\vec{r}_{45}=0.0\hat{i}+10.0\hat{j}+10.0\hat{k}$.

{\tiny 2D-M19:}

$\hat{n}_{13}=-0.0\hat{i}-0.71\hat{j}+0.71\hat{k}$,\;\;\;$\hat{n}_{14}=-0.0\hat{i}+0.86\hat{j}+0.51\hat{k}$,\;\;\;$\hat{n}_{45}=-0.0\hat{i}+0.86\hat{j}+0.51\hat{k}$,\;\;\;$\vec{r}_{13}=0.0\hat{i}+10.0\hat{j}+0.0\hat{k}$,\newline
$\vec{r}_{23}=0.0\hat{i}+0.0\hat{j}+0.0\hat{k}$,\;\;\;$\vec{r}_{24}=10.0\hat{i}+10.0\hat{j}+10.0\hat{k}$,\;\;\;$\vec{r}_{45}=0.0\hat{i}+0.0\hat{j}+10.0\hat{k}$.

{\tiny 2D-M20:}

$\hat{n}_{13}=0.28\hat{i}-0.83\hat{j}-0.48\hat{k}$,\;\;\;$\hat{n}_{14}=0.58\hat{i}-0.58\hat{j}+0.58\hat{k}$,\;\;\;$\hat{n}_{35}=-0.0\hat{i}+0.0\hat{j}+1.0\hat{k}$,\;\;\;$\vec{r}_{13}=0.0\hat{i}+0.0\hat{j}+10.0\hat{k}$,\newline
$\vec{r}_{23}=10.0\hat{i}+0.0\hat{j}+0.0\hat{k}$,\;\;\;$\vec{r}_{24}=0.0\hat{i}+10.0\hat{j}+10.0\hat{k}$,\;\;\;$\vec{r}_{35}=10.0\hat{i}+10.0\hat{j}+9.95\hat{k}$.
