# Supplementary material for: Dimensional synthesis of spatial manipulators for velocity and force transmission for operation around a specified task point
Source: arXiv:2210.04446 source file (2022-10-10)
Supplement: Supplementary file 48 [file classappendix4.tex]

\subsection{Class 4} \label{appendix_five_2_1}
{\tiny 2D-M36:}

$\hat{n}_{14}=-0.0\hat{i}+0.71\hat{j}+0.71\hat{k}$,\;\;\;$\hat{n}_{24}=0.0\hat{i}+1.0\hat{j}+0.0\hat{k}$,\;\;\;$\hat{n}_{25}=-0.0\hat{i}+0.0\hat{j}-1.0\hat{k}$,\;\;\;$\vec{r}_{34}=0.0\hat{i}+10.0\hat{j}+0.0\hat{k}$,\newline
$\vec{r}_{35}=10.0\hat{i}+0.0\hat{j}+10.0\hat{k}$.

{\tiny 2D-M37:}

$\hat{n}_{14}=0.0\hat{i}+0.71\hat{j}+0.71\hat{k}$,\;\;\;$\hat{n}_{25}=-0.0\hat{i}+0.71\hat{j}-0.71\hat{k}$,\;\;\;$\hat{n}_{45}=0.58\hat{i}+0.58\hat{j}-0.58\hat{k}$,\;\;\;$\vec{r}_{23}=10.0\hat{i}+10.0\hat{j}+0.0\hat{k}$,\newline
$\vec{r}_{34}=0.0\hat{i}+0.0\hat{j}+10.0\hat{k}$.

{\tiny 2D-M38:}

$\hat{n}_{14}=0.39\hat{i}-0.82\hat{j}+0.43\hat{k}$,\;\;\;$\hat{n}_{34}=-0.0\hat{i}+0.71\hat{j}+0.71\hat{k}$,\;\;\;$\hat{n}_{45}=-0.58\hat{i}-0.58\hat{j}-0.58\hat{k}$,\;\;\;$\vec{r}_{23}=0.0\hat{i}+0.0\hat{j}+0.0\hat{k}$,\newline
$\vec{r}_{25}=10.0\hat{i}+10.0\hat{j}+10.0\hat{k}$.

{\tiny 2D-M39:}

$\hat{n}_{13}=-0.0\hat{i}+0.71\hat{j}-0.71\hat{k}$,\;\;\;$\hat{n}_{14}=-0.58\hat{i}+0.58\hat{j}+0.58\hat{k}$,\;\;\;$\hat{n}_{35}=0.0\hat{i}+0.71\hat{j}+0.71\hat{k}$,\;\;\;$\vec{r}_{24}=10.0\hat{i}+0.0\hat{j}+10.0\hat{k}$,\newline
$\vec{r}_{25}=0.0\hat{i}+10.0\hat{j}+0.0\hat{k}$.

{\tiny 2D-M40:}

$\hat{n}_{13}=0.58\hat{i}+0.58\hat{j}-0.58\hat{k}$,\;\;\;$\hat{n}_{14}=0.0\hat{i}+0.0\hat{j}+1.0\hat{k}$,\;\;\;$\hat{n}_{45}=0.22\hat{i}+0.97\hat{j}-0.0\hat{k}$,\;\;\;$\vec{r}_{23}=0.0\hat{i}+0.0\hat{j}+10.0\hat{k}$,\newline
$\vec{r}_{24}=10.0\hat{i}+10.0\hat{j}+0.0\hat{k}$.
