# Supplementary material for: Dimensional synthesis of spatial manipulators for velocity and force transmission for operation around a specified task point
Source: arXiv:2210.04446 source file (2022-10-10)
Supplement: Supplementary file 54 [file classappendix1.tex]

\subsection{Class 1} \label{appendix_five_2_1}
{\tiny 3D-M1:}

$\hat{n}_{13}=-0.71\hat{i}+0.11\hat{j}-0.7\hat{k}$,\;\;\;$\hat{n}_{23}=-0.0\hat{i}+0.58\hat{j}-0.81\hat{k}$,\;\;\;$\hat{n}_{24}=0.82\hat{i}-0.46\hat{j}-0.34\hat{k}$,\;\;\;$\vec{r}_{13}=10.0\hat{i}+10.0\hat{j}+0.0\hat{k}$,\newline
$\vec{r}_{23}=10.0\hat{i}+0.0\hat{j}+10.0\hat{k}$,\;\;\;$\vec{r}_{24}=10.0\hat{i}+10.0\hat{j}+10.0\hat{k}$.
