# Supplementary material for: Dimensional synthesis of spatial manipulators for velocity and force transmission for operation around a specified task point
Source: arXiv:2210.04446 source file (2022-10-10)
Supplement: Supplementary file 55 [file classappendix2.tex]

\subsection{Class 2} \label{appendix_five_2_1}
{\tiny 3D-M2:}

$\hat{n}_{13}=-0.8\hat{i}+0.33\hat{j}+0.49\hat{k}$,\;\;\;$\hat{n}_{23}=-0.17\hat{i}+0.67\hat{j}-0.73\hat{k}$,\;\;\;$\hat{n}_{24}=-0.57\hat{i}-0.67\hat{j}-0.48\hat{k}$,\;\;\;$\vec{r}_{13}=10.0\hat{i}+10.0\hat{j}+10.0\hat{k}$,\newline
$\vec{r}_{23}=10.0\hat{i}+10.0\hat{j}+10.0\hat{k}$.

{\tiny 3D-M3:}

$\hat{n}_{13}=-0.8\hat{i}+0.58\hat{j}+0.14\hat{k}$,\;\;\;$\hat{n}_{23}=-0.74\hat{i}-0.51\hat{j}-0.43\hat{k}$,\;\;\;$\hat{n}_{24}=0.51\hat{i}+0.16\hat{j}+0.84\hat{k}$,\;\;\;$\vec{r}_{13}=10.0\hat{i}+10.0\hat{j}+10.0\hat{k}$,\newline
$\vec{r}_{24}=10.0\hat{i}+10.0\hat{j}+0.0\hat{k}$.

{\tiny 3D-M4:}

$\hat{n}_{13}=-0.57\hat{i}-0.67\hat{j}-0.48\hat{k}$,\;\;\;$\hat{n}_{23}=-0.31\hat{i}-0.36\hat{j}-0.88\hat{k}$,\;\;\;$\hat{n}_{24}=0.76\hat{i}-0.65\hat{j}+0.0\hat{k}$,\;\;\;$\vec{r}_{23}=10.0\hat{i}+10.0\hat{j}+0.0\hat{k}$,\newline
$\vec{r}_{24}=10.0\hat{i}+10.0\hat{j}+10.0\hat{k}$.
