# Supplementary material for: Dimensional synthesis of spatial manipulators for velocity and force transmission for operation around a specified task point
Source: arXiv:2210.04446 source file (2022-10-10)
Supplement: Supplementary file 56 [file classappendix3.tex]

\subsection{Class 3} \label{appendix_five_2_1}
{\tiny 3D-M5:}

$\hat{n}_{13}=0.5\hat{i}+0.18\hat{j}+0.85\hat{k}$,\;\;\;$\hat{n}_{23}=-0.76\hat{i}-0.61\hat{j}-0.24\hat{k}$,\;\;\;$\hat{n}_{24}=0.03\hat{i}+0.33\hat{j}-0.94\hat{k}$,\;\;\;$\vec{r}_{13}=10.0\hat{i}+10.0\hat{j}+0.0\hat{k}$.

{\tiny 3D-M6:}

$\hat{n}_{13}=-0.6\hat{i}-0.76\hat{j}-0.26\hat{k}$,\;\;\;$\hat{n}_{23}=0.26\hat{i}+0.4\hat{j}+0.88\hat{k}$,\;\;\;$\hat{n}_{24}=-0.21\hat{i}-0.17\hat{j}+0.96\hat{k}$,\;\;\;$\vec{r}_{23}=10.0\hat{i}+10.0\hat{j}+0.0\hat{k}$.

{\tiny 3D-M7:}

$\hat{n}_{13}=-0.54\hat{i}-0.83\hat{j}+0.12\hat{k}$,\;\;\;$\hat{n}_{23}=0.18\hat{i}-0.26\hat{j}-0.95\hat{k}$,\;\;\;$\hat{n}_{24}=-0.04\hat{i}-0.56\hat{j}-0.83\hat{k}$,\;\;\;$\vec{r}_{24}=10.0\hat{i}+10.0\hat{j}+0.0\hat{k}$.
