# Supplementary material for: Dimensional synthesis of spatial manipulators for velocity and force transmission for operation around a specified task point
Source: arXiv:2210.04446 source file (2022-10-10)
Supplement: Supplementary file 57 [file classappendix4.tex]

\subsection{Class 4} \label{appendix_five_2_1}
{\tiny 3D-M8:}

$\hat{n}_{13}=0.41\hat{i}+0.89\hat{j}-0.2\hat{k}$,\;\;\;$\hat{n}_{23}=-0.62\hat{i}+0.11\hat{j}-0.78\hat{k}$,\;\;\;$\hat{n}_{24}=-0.67\hat{i}+0.44\hat{j}+0.59\hat{k}$.
