# Supplementary material for: Dimensional synthesis of spatial manipulators for velocity and force transmission for operation around a specified task point
Source: arXiv:2210.04446 source file (2022-10-10)
Supplement: Supplementary file 58 [file classappendix1.tex]

\subsection{Class 1} \label{appendix_five_2_1}
{\tiny 4D-M1:}

$\hat{n}_{14}=-0.29\hat{i}+0.57\hat{j}-0.77\hat{k}$,\;\;\;$\hat{n}_{23}=0.75\hat{i}-0.53\hat{j}+0.4\hat{k}$,\;\;\;$\hat{n}_{25}=-0.34\hat{i}+0.83\hat{j}-0.45\hat{k}$,\;\;\;$\hat{n}_{34}=-0.72\hat{i}+0.12\hat{j}+0.69\hat{k}$,\newline
$\vec{r}_{14}=10.0\hat{i}+0.0\hat{j}+10.0\hat{k}$,\;\;\;$\vec{r}_{23}=10.0\hat{i}+10.0\hat{j}+0.0\hat{k}$,\;\;\;$\vec{r}_{25}=0.0\hat{i}+0.0\hat{j}+0.0\hat{k}$,\;\;\;$\vec{r}_{34}=10.0\hat{i}+10.0\hat{j}+10.0\hat{k}$.
