# Supplementary material for: Dimensional synthesis of spatial manipulators for velocity and force transmission for operation around a specified task point
Source: arXiv:2210.04446 source file (2022-10-10)
Supplement: Supplementary file 59 [file classappendix2.tex]

\subsection{Class 2} \label{appendix_five_2_1}
{\tiny 4D-M2:}

$\hat{n}_{14}=0.82\hat{i}+0.49\hat{j}+0.3\hat{k}$,\;\;\;$\hat{n}_{23}=-0.39\hat{i}-0.47\hat{j}-0.79\hat{k}$,\;\;\;$\hat{n}_{25}=-0.42\hat{i}-0.85\hat{j}-0.32\hat{k}$,\;\;\;$\hat{n}_{34}=0.57\hat{i}+0.69\hat{j}+0.45\hat{k}$,\newline
$\vec{r}_{14}=10.0\hat{i}+0.0\hat{j}+10.0\hat{k}$,\;\;\;$\vec{r}_{23}=10.0\hat{i}+10.0\hat{j}+0.0\hat{k}$,\;\;\;$\vec{r}_{25}=0.0\hat{i}+10.0\hat{j}+10.0\hat{k}$.

{\tiny 4D-M3:}

$\hat{n}_{14}=0.39\hat{i}+0.47\hat{j}-0.79\hat{k}$,\;\;\;$\hat{n}_{23}=-0.42\hat{i}-0.85\hat{j}+0.32\hat{k}$,\;\;\;$\hat{n}_{25}=-0.57\hat{i}-0.69\hat{j}+0.45\hat{k}$,\;\;\;$\hat{n}_{34}=0.82\hat{i}+0.49\hat{j}-0.3\hat{k}$,\newline
$\vec{r}_{14}=10.0\hat{i}+10.0\hat{j}+10.0\hat{k}$,\;\;\;$\vec{r}_{23}=0.0\hat{i}+10.0\hat{j}+0.0\hat{k}$,\;\;\;$\vec{r}_{34}=10.0\hat{i}+0.0\hat{j}+0.0\hat{k}$.

{\tiny 4D-M4:}

$\hat{n}_{14}=0.42\hat{i}+0.85\hat{j}-0.32\hat{k}$,\;\;\;$\hat{n}_{23}=-0.57\hat{i}-0.69\hat{j}+0.45\hat{k}$,\;\;\;$\hat{n}_{25}=-0.39\hat{i}-0.47\hat{j}+0.79\hat{k}$,\;\;\;$\hat{n}_{34}=0.82\hat{i}+0.49\hat{j}-0.3\hat{k}$,\newline
$\vec{r}_{14}=0.0\hat{i}+10.0\hat{j}+0.0\hat{k}$,\;\;\;$\vec{r}_{25}=10.0\hat{i}+10.0\hat{j}+10.0\hat{k}$,\;\;\;$\vec{r}_{34}=10.0\hat{i}+0.0\hat{j}+0.0\hat{k}$.

{\tiny 4D-M5:}

$\hat{n}_{14}=-0.57\hat{i}-0.69\hat{j}-0.45\hat{k}$,\;\;\;$\hat{n}_{23}=0.42\hat{i}+0.85\hat{j}+0.32\hat{k}$,\;\;\;$\hat{n}_{25}=0.82\hat{i}+0.49\hat{j}+0.3\hat{k}$,\;\;\;$\hat{n}_{34}=-0.39\hat{i}-0.47\hat{j}-0.79\hat{k}$,\newline
$\vec{r}_{23}=0.0\hat{i}+10.0\hat{j}+10.0\hat{k}$,\;\;\;$\vec{r}_{25}=10.0\hat{i}+0.0\hat{j}+10.0\hat{k}$,\;\;\;$\vec{r}_{34}=10.0\hat{i}+10.0\hat{j}+0.0\hat{k}$.
