# Supplementary material for: Dimensional synthesis of spatial manipulators for velocity and force transmission for operation around a specified task point
Source: arXiv:2210.04446 source file (2022-10-10)
Supplement: Supplementary file 60 [file classappendix3.tex]

\subsection{Class 3} \label{appendix_five_2_1}
{\tiny 4D-M6:}

$\hat{n}_{14}=-0.54\hat{i}-0.84\hat{j}-0.08\hat{k}$,\;\;\;$\hat{n}_{23}=-0.68\hat{i}-0.7\hat{j}-0.22\hat{k}$,\;\;\;$\hat{n}_{25}=0.62\hat{i}-0.53\hat{j}+0.59\hat{k}$,\;\;\;$\hat{n}_{34}=-0.58\hat{i}-0.81\hat{j}-0.12\hat{k}$,\newline
$\vec{r}_{14}=0.0\hat{i}+10.0\hat{j}+10.0\hat{k}$,\;\;\;$\vec{r}_{23}=10.0\hat{i}+0.0\hat{j}+0.0\hat{k}$.

{\tiny 4D-M7:}

$\hat{n}_{14}=0.54\hat{i}+0.84\hat{j}-0.08\hat{k}$,\;\;\;$\hat{n}_{23}=-0.05\hat{i}+0.94\hat{j}+0.34\hat{k}$,\;\;\;$\hat{n}_{25}=-0.68\hat{i}-0.7\hat{j}+0.22\hat{k}$,\;\;\;$\hat{n}_{34}=0.84\hat{i}+0.22\hat{j}-0.49\hat{k}$,\newline
$\vec{r}_{14}=0.0\hat{i}+10.0\hat{j}+0.0\hat{k}$,\;\;\;$\vec{r}_{25}=10.0\hat{i}+0.0\hat{j}+10.0\hat{k}$.

{\tiny 4D-M8:}

$\hat{n}_{14}=0.54\hat{i}+0.84\hat{j}-0.08\hat{k}$,\;\;\;$\hat{n}_{23}=-0.26\hat{i}+0.85\hat{j}+0.46\hat{k}$,\;\;\;$\hat{n}_{25}=-0.8\hat{i}-0.46\hat{j}+0.38\hat{k}$,\;\;\;$\hat{n}_{34}=-0.68\hat{i}-0.7\hat{j}+0.22\hat{k}$,\newline
$\vec{r}_{14}=0.0\hat{i}+10.0\hat{j}+0.0\hat{k}$,\;\;\;$\vec{r}_{34}=10.0\hat{i}+0.0\hat{j}+10.0\hat{k}$.

{\tiny 4D-M9:}

$\hat{n}_{14}=-0.08\hat{i}-0.96\hat{j}-0.27\hat{k}$,\;\;\;$\hat{n}_{23}=0.54\hat{i}+0.84\hat{j}-0.08\hat{k}$,\;\;\;$\hat{n}_{25}=-0.68\hat{i}-0.7\hat{j}+0.22\hat{k}$,\;\;\;$\hat{n}_{34}=-0.84\hat{i}-0.08\hat{j}+0.53\hat{k}$,\newline
$\vec{r}_{23}=0.0\hat{i}+10.0\hat{j}+0.0\hat{k}$,\;\;\;$\vec{r}_{25}=10.0\hat{i}+0.0\hat{j}+10.0\hat{k}$.

{\tiny 4D-M10:}

$\hat{n}_{14}=-0.63\hat{i}-0.76\hat{j}-0.17\hat{k}$,\;\;\;$\hat{n}_{23}=-0.54\hat{i}-0.84\hat{j}-0.08\hat{k}$,\;\;\;$\hat{n}_{25}=-0.56\hat{i}+0.59\hat{j}-0.57\hat{k}$,\;\;\;$\hat{n}_{34}=-0.68\hat{i}-0.7\hat{j}-0.22\hat{k}$,\newline
$\vec{r}_{23}=0.0\hat{i}+10.0\hat{j}+10.0\hat{k}$,\;\;\;$\vec{r}_{34}=10.0\hat{i}+0.0\hat{j}+0.0\hat{k}$.

{\tiny 4D-M11:}

$\hat{n}_{14}=-0.32\hat{i}+0.81\hat{j}-0.49\hat{k}$,\;\;\;$\hat{n}_{23}=0.78\hat{i}+0.52\hat{j}+0.35\hat{k}$,\;\;\;$\hat{n}_{25}=-0.68\hat{i}-0.7\hat{j}-0.22\hat{k}$,\;\;\;$\hat{n}_{34}=0.54\hat{i}+0.84\hat{j}+0.08\hat{k}$,\newline
$\vec{r}_{25}=10.0\hat{i}+0.0\hat{j}+0.0\hat{k}$,\;\;\;$\vec{r}_{34}=0.0\hat{i}+10.0\hat{j}+10.0\hat{k}$.
