# Supplementary material for: Dimensional synthesis of spatial manipulators for velocity and force transmission for operation around a specified task point
Source: arXiv:2210.04446 source file (2022-10-10)
Supplement: Supplementary file 61 [file classappendix4.tex]

\subsection{Class 4} \label{appendix_five_2_1}
{\tiny 4D-M12:}

$\hat{n}_{14}=0.09\hat{i}-1.0\hat{j}+0.05\hat{k}$,\;\;\;$\hat{n}_{23}=0.67\hat{i}+0.35\hat{j}+0.66\hat{k}$,\;\;\;$\hat{n}_{25}=0.01\hat{i}-0.88\hat{j}+0.47\hat{k}$,\;\;\;$\hat{n}_{34}=-0.75\hat{i}+0.31\hat{j}+0.59\hat{k}$,\newline
$\vec{r}_{14}=4.0\hat{i}+2.99\hat{j}+5.94\hat{k}$.

{\tiny 4D-M13:}

$\hat{n}_{14}=-0.94\hat{i}-0.18\hat{j}-0.29\hat{k}$,\;\;\;$\hat{n}_{23}=0.32\hat{i}-0.95\hat{j}+0.01\hat{k}$,\;\;\;$\hat{n}_{25}=-0.03\hat{i}-0.8\hat{j}+0.59\hat{k}$,\;\;\;$\hat{n}_{34}=0.34\hat{i}-0.57\hat{j}-0.75\hat{k}$,\newline
$\vec{r}_{23}=7.59\hat{i}+3.33\hat{j}+4.0\hat{k}$.

{\tiny 4D-M14:}

$\hat{n}_{14}=-0.38\hat{i}-0.54\hat{j}-0.75\hat{k}$,\;\;\;$\hat{n}_{23}=-0.54\hat{i}-0.53\hat{j}+0.65\hat{k}$,\;\;\;$\hat{n}_{25}=0.34\hat{i}-0.93\hat{j}-0.12\hat{k}$,\;\;\;$\hat{n}_{34}=0.75\hat{i}-0.65\hat{j}+0.1\hat{k}$,\newline
$\vec{r}_{25}=3.55\hat{i}+6.33\hat{j}+6.15\hat{k}$.

{\tiny 4D-M15:}

$\hat{n}_{14}=-0.19\hat{i}-0.68\hat{j}-0.71\hat{k}$,\;\;\;$\hat{n}_{23}=0.56\hat{i}-0.67\hat{j}+0.49\hat{k}$,\;\;\;$\hat{n}_{25}=-0.8\hat{i}-0.3\hat{j}+0.51\hat{k}$,\;\;\;$\hat{n}_{34}=0.84\hat{i}-0.54\hat{j}+0.05\hat{k}$,\newline
$\vec{r}_{34}=3.99\hat{i}+5.66\hat{j}+6.62\hat{k}$.
